# Supplementary material for: Accelerating Video Object Segmentation with Compressed Video
Source: arXiv:2107.12192 source file (2022-04-06)
Supplement: Supplementary file 1 [file supp_qual2.pdf]

|                                                                                   | MiVOS                                                                               | MiVOS+CoVOS                                                                          | Ground Truth                                                                          |
|-----------------------------------------------------------------------------------|-------------------------------------------------------------------------------------|--------------------------------------------------------------------------------------|---------------------------------------------------------------------------------------|
| 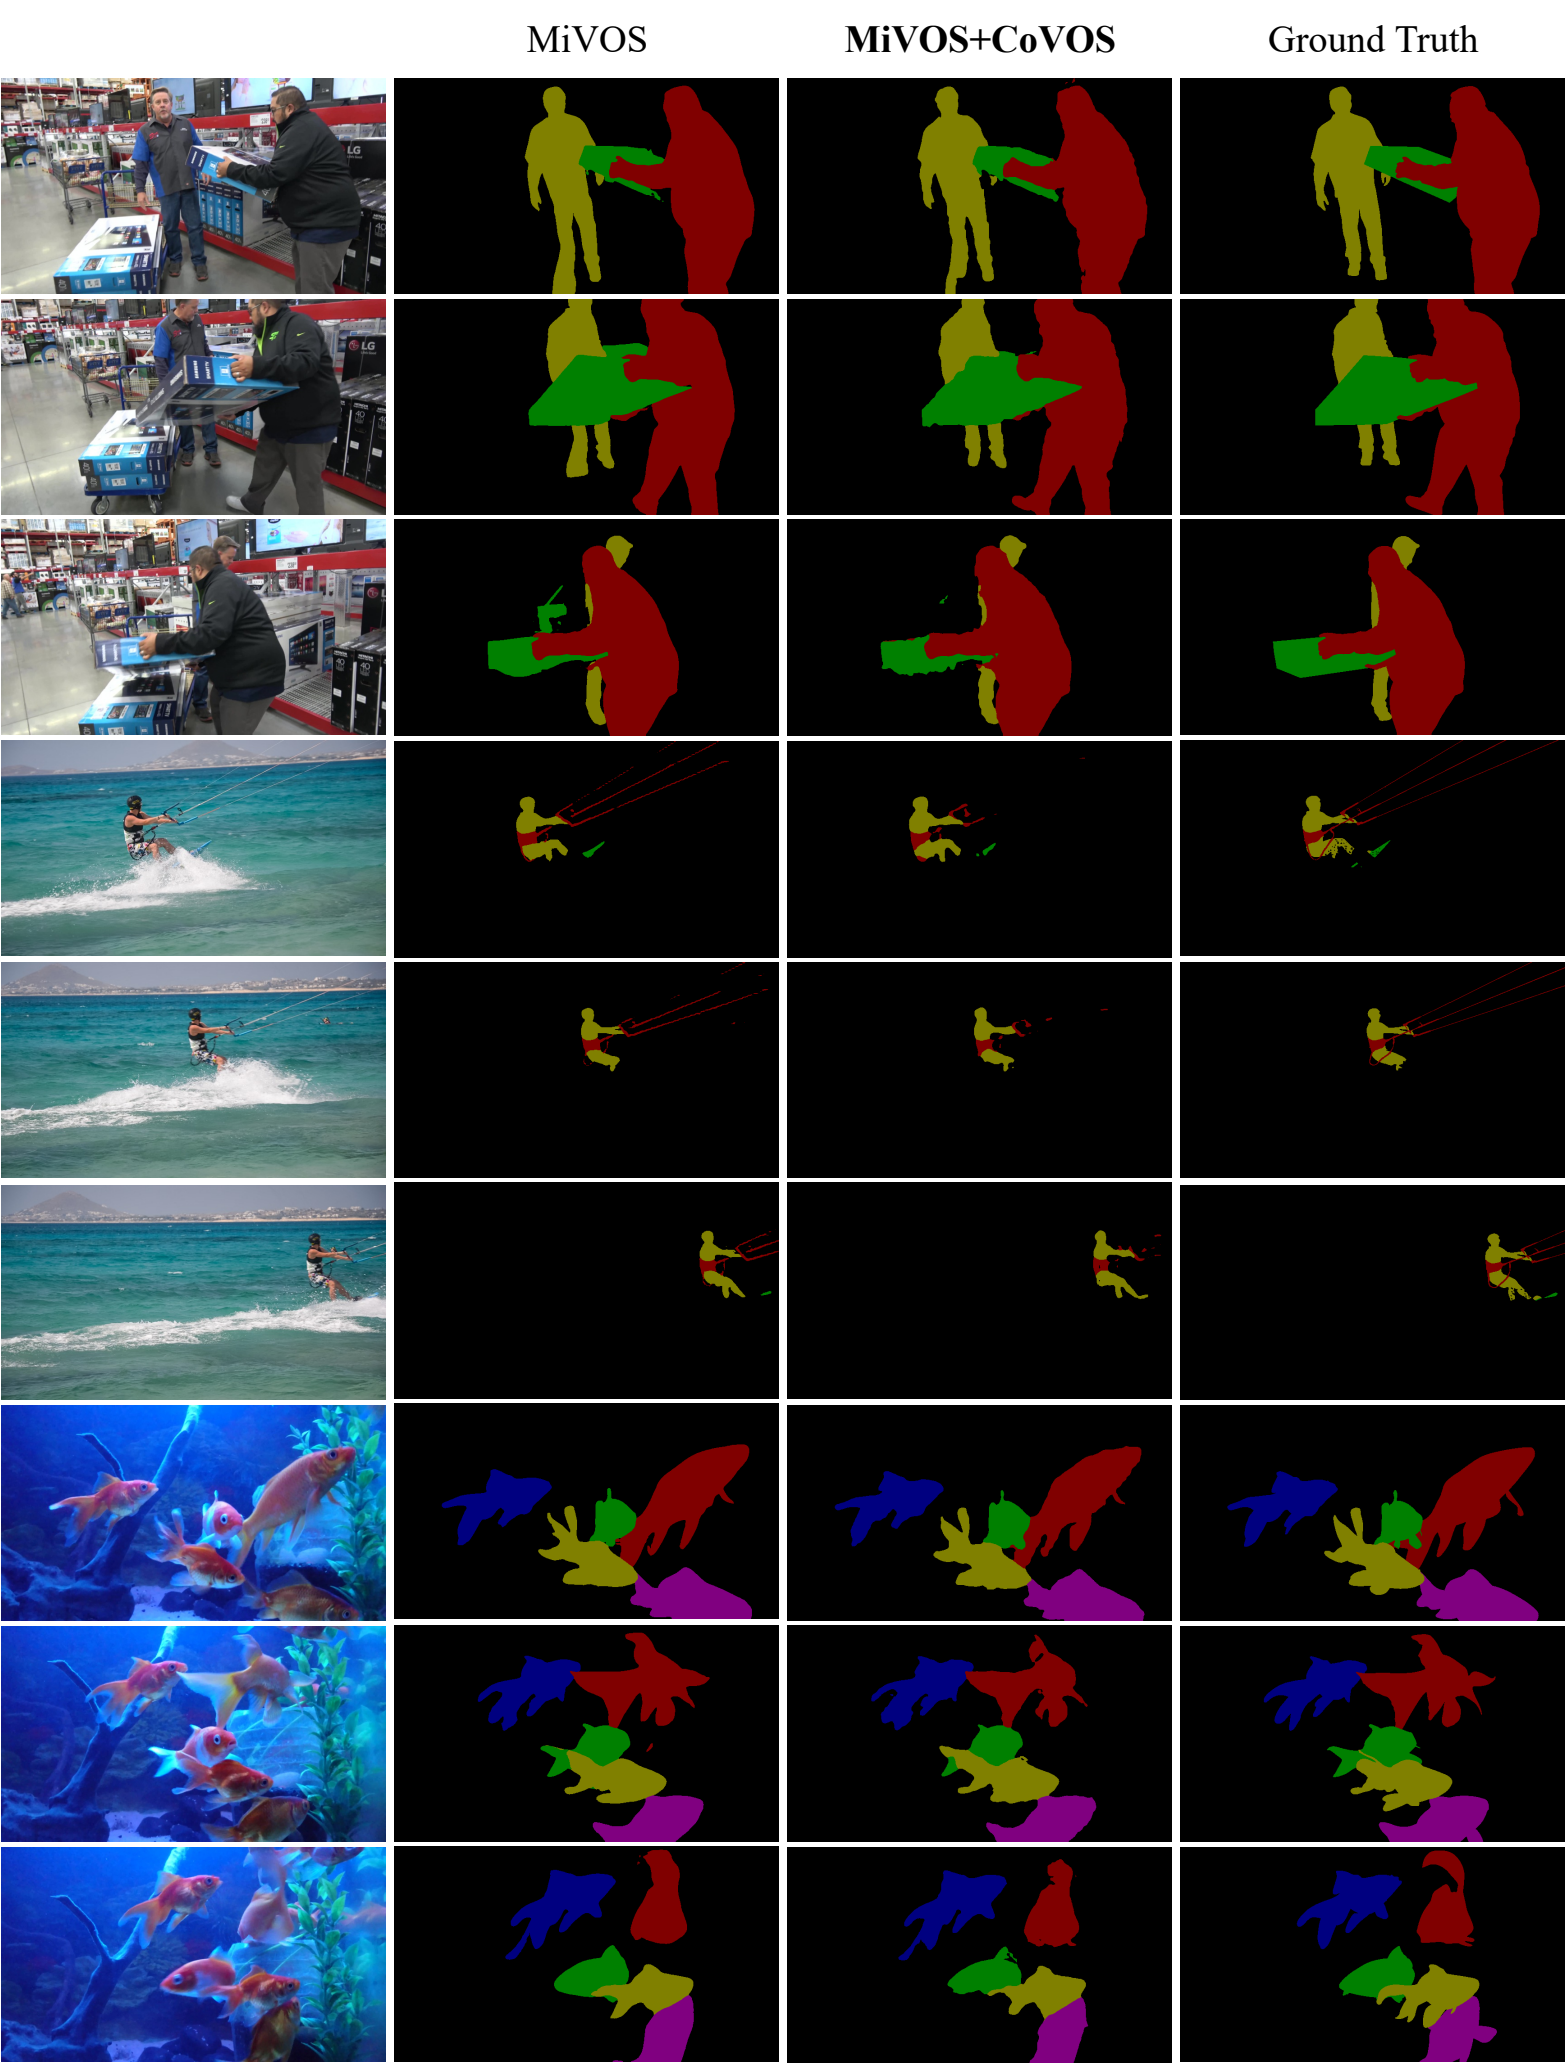    | 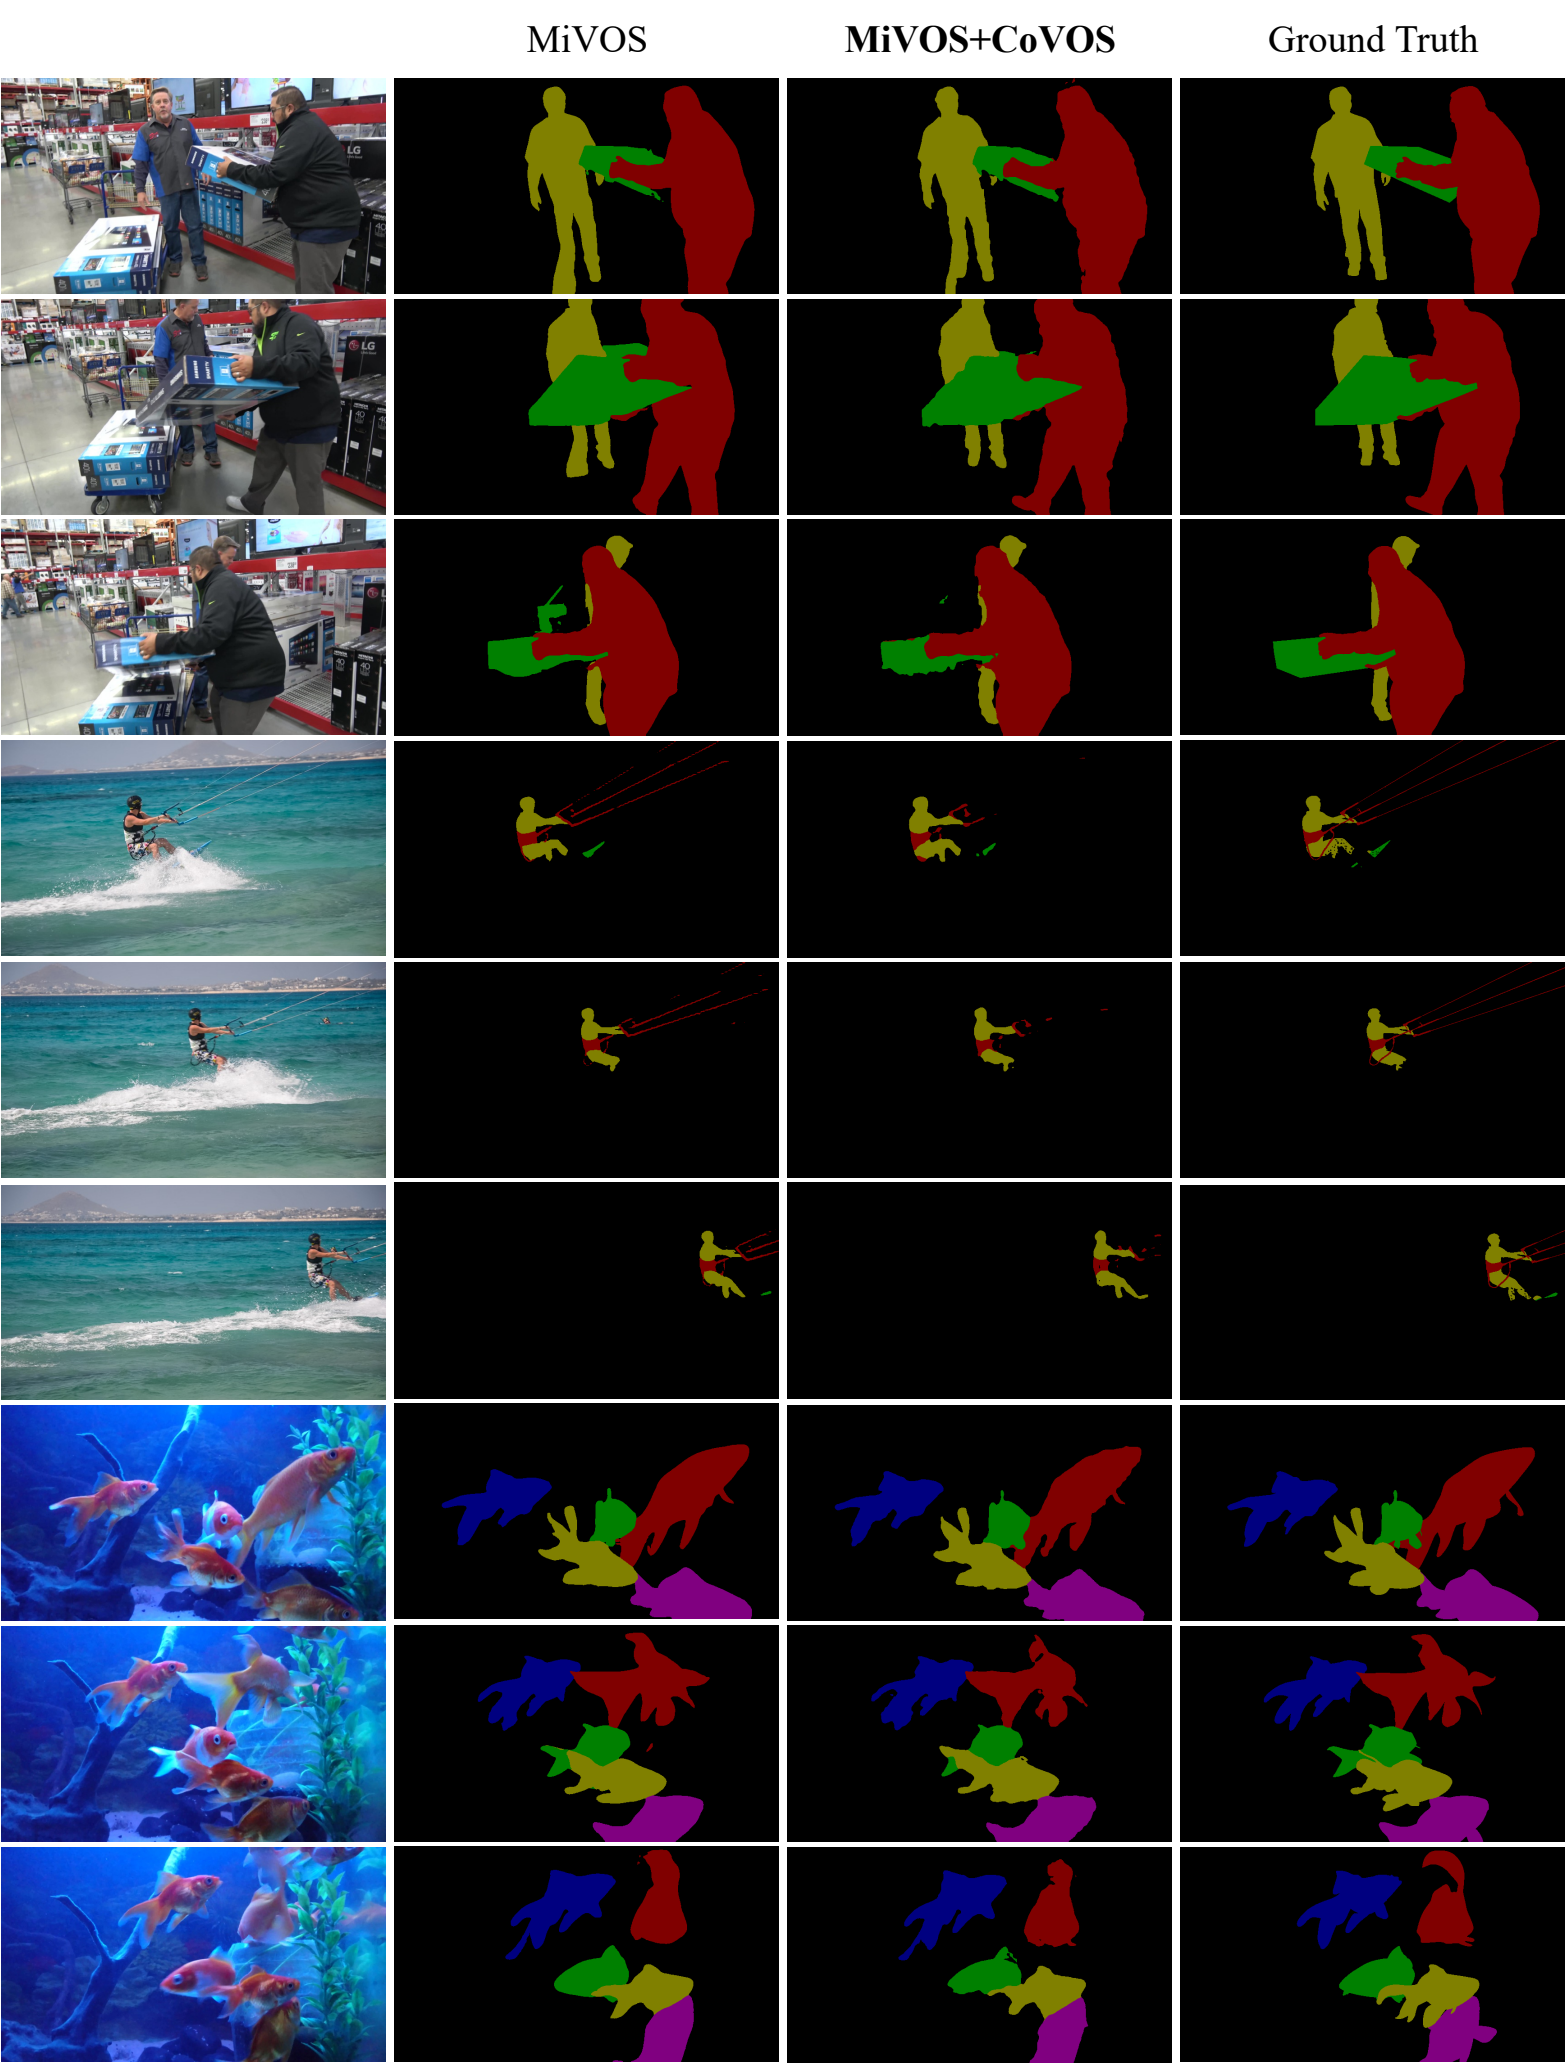    | 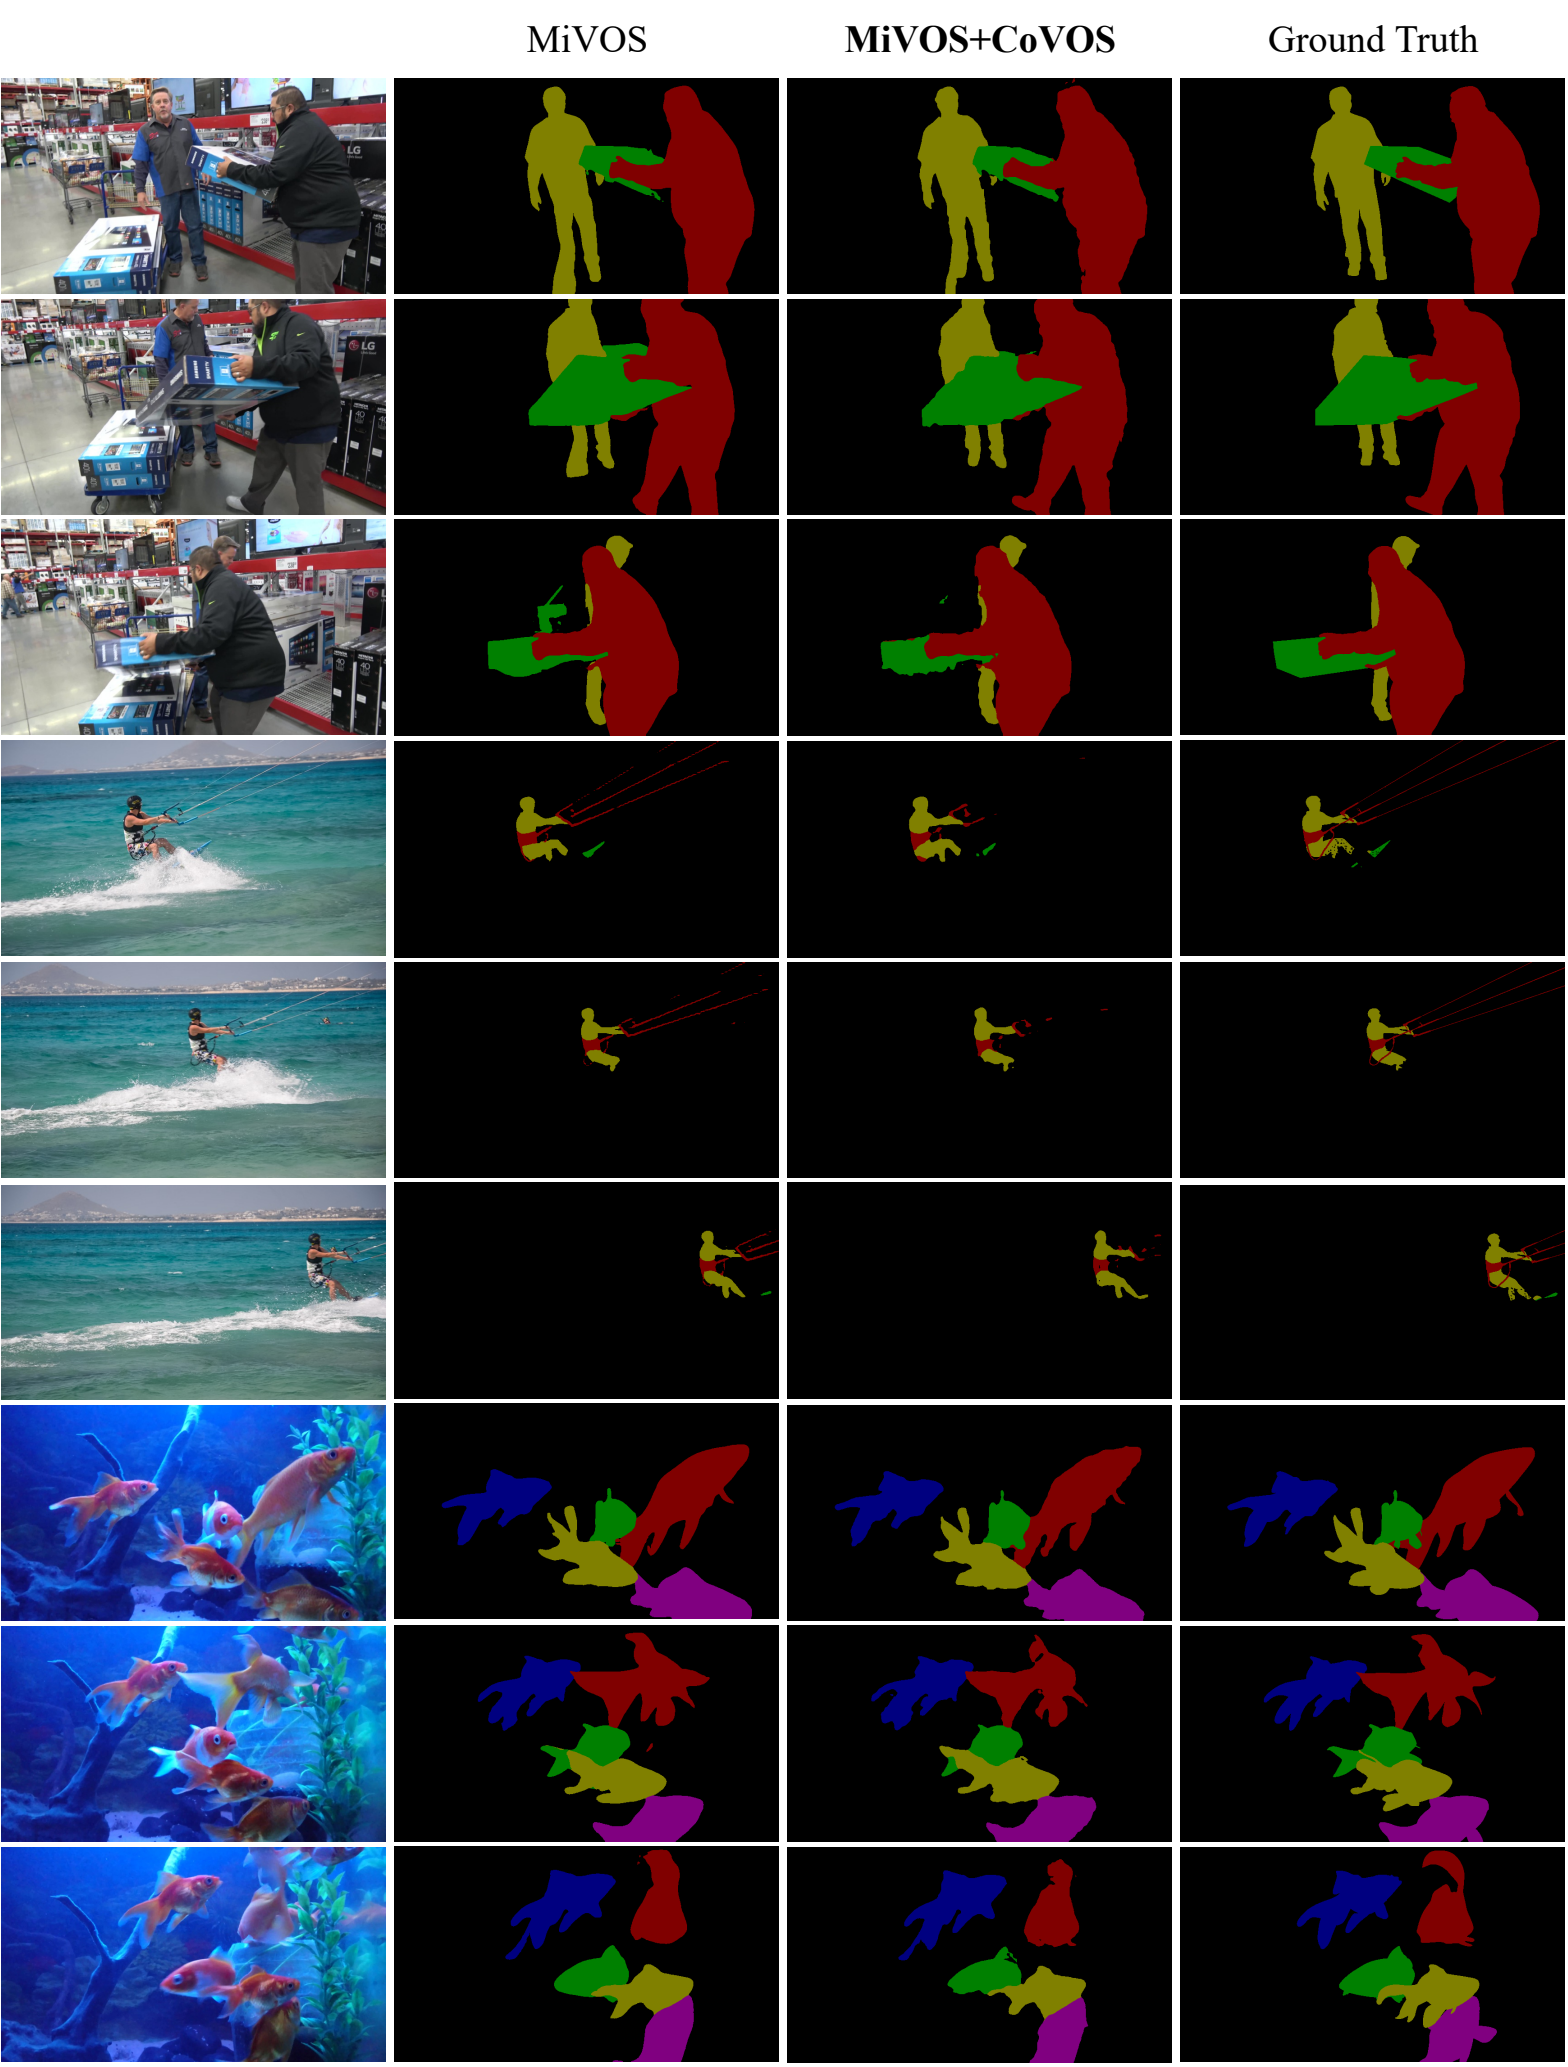    | 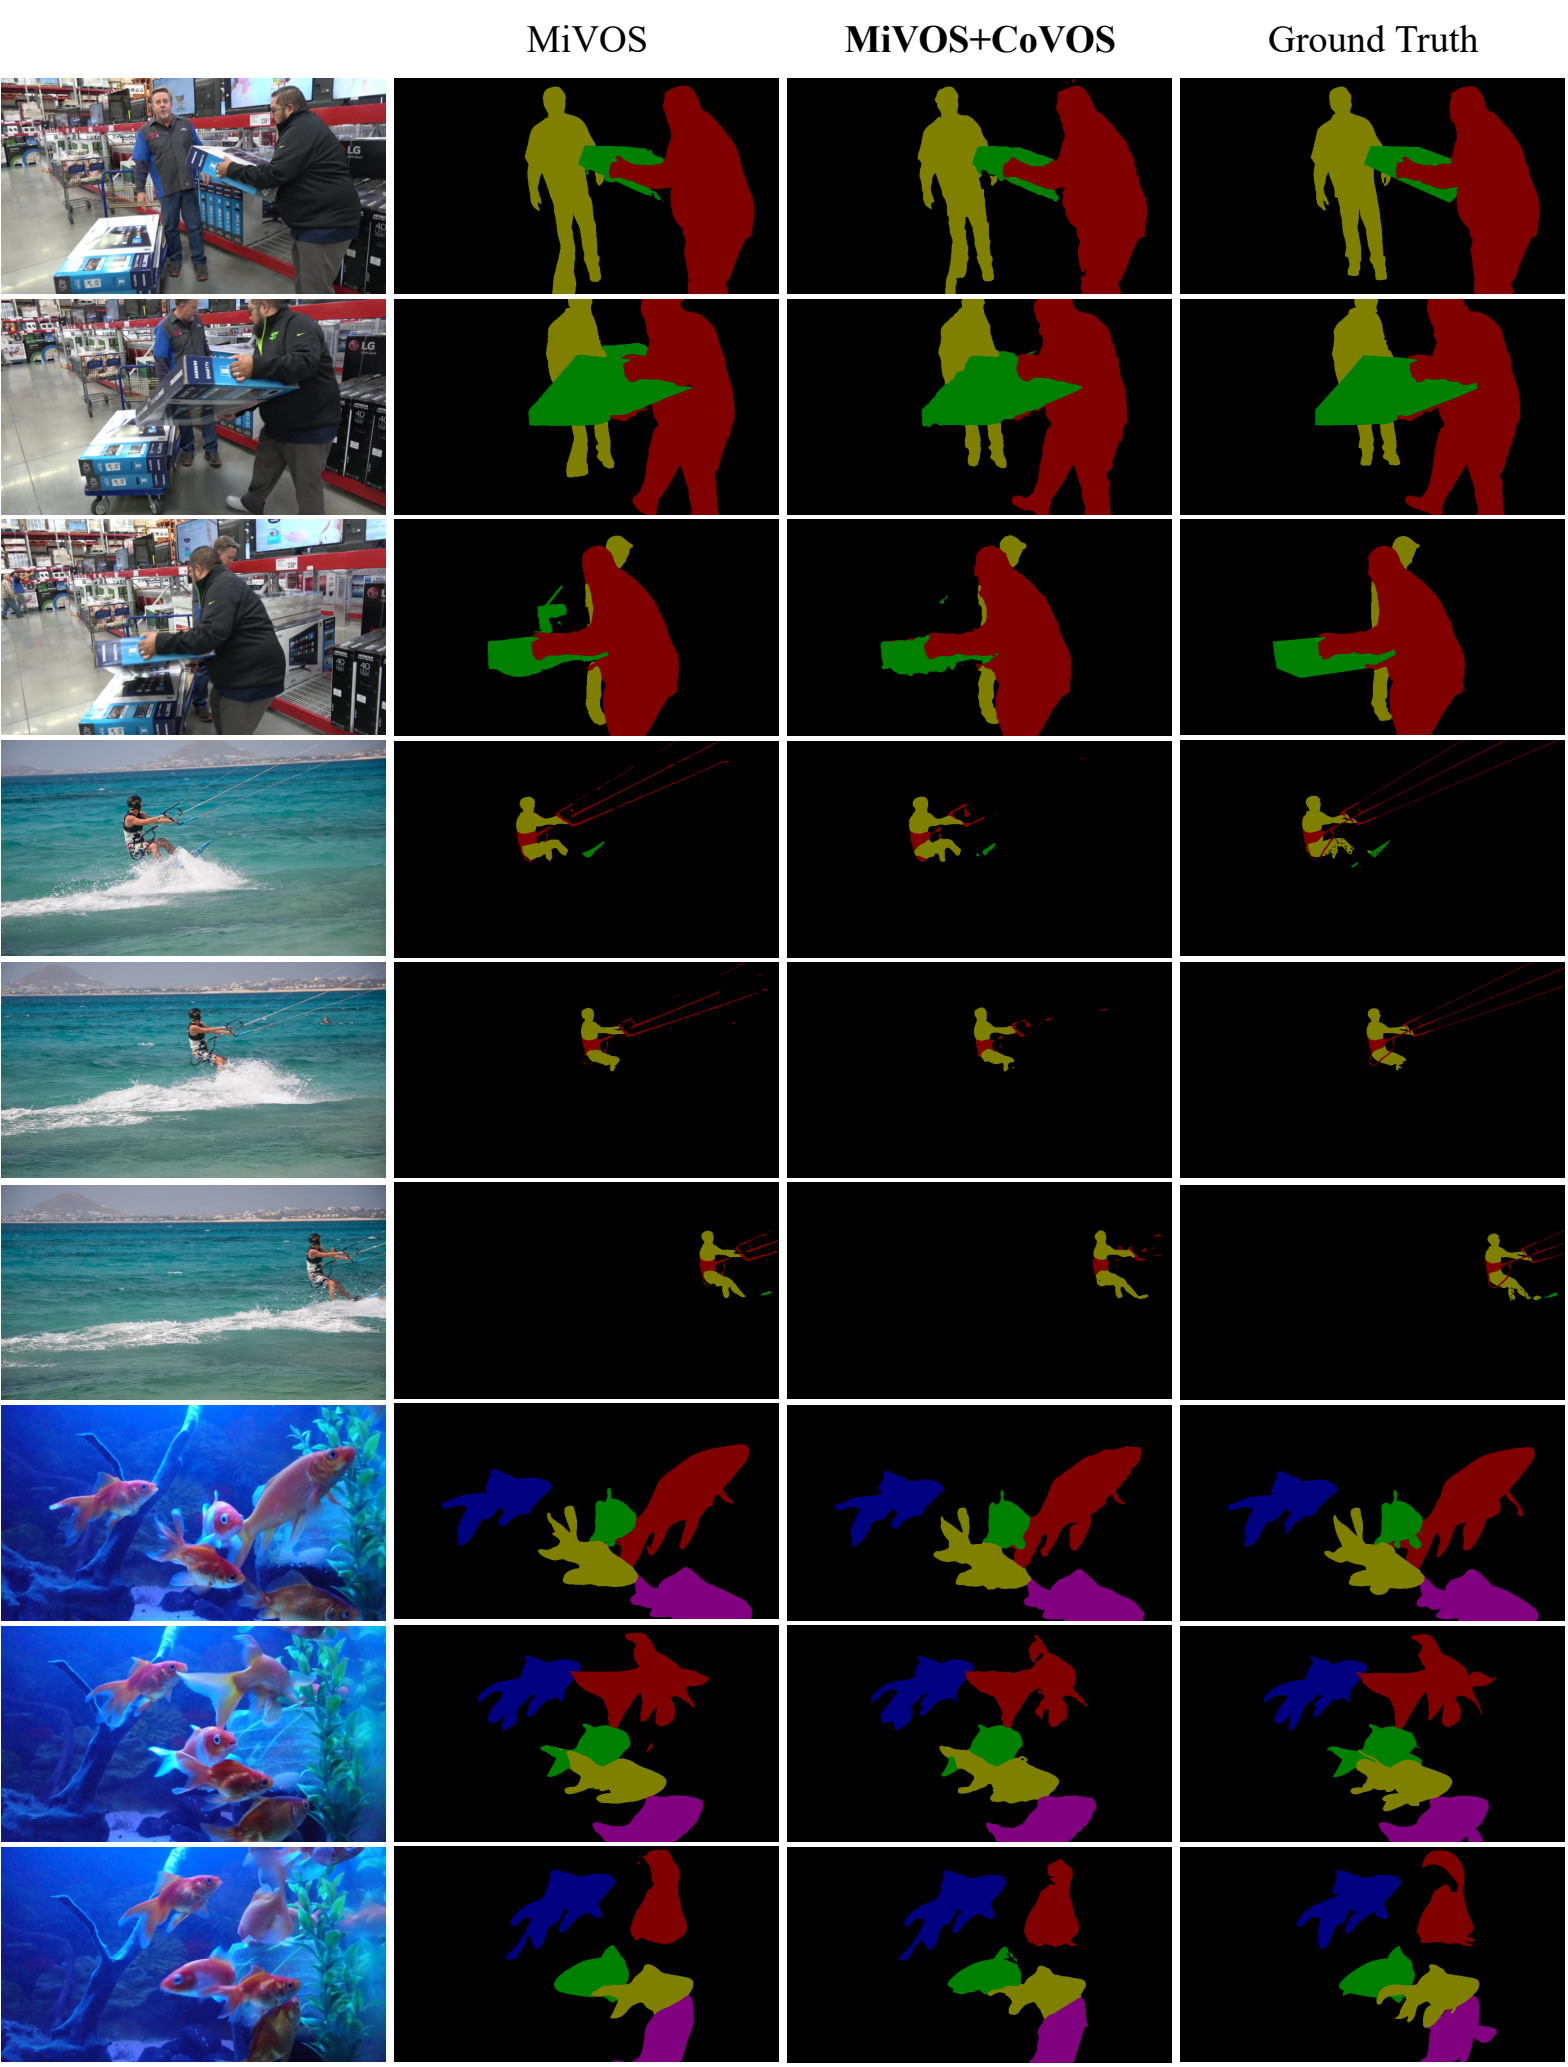    |
| 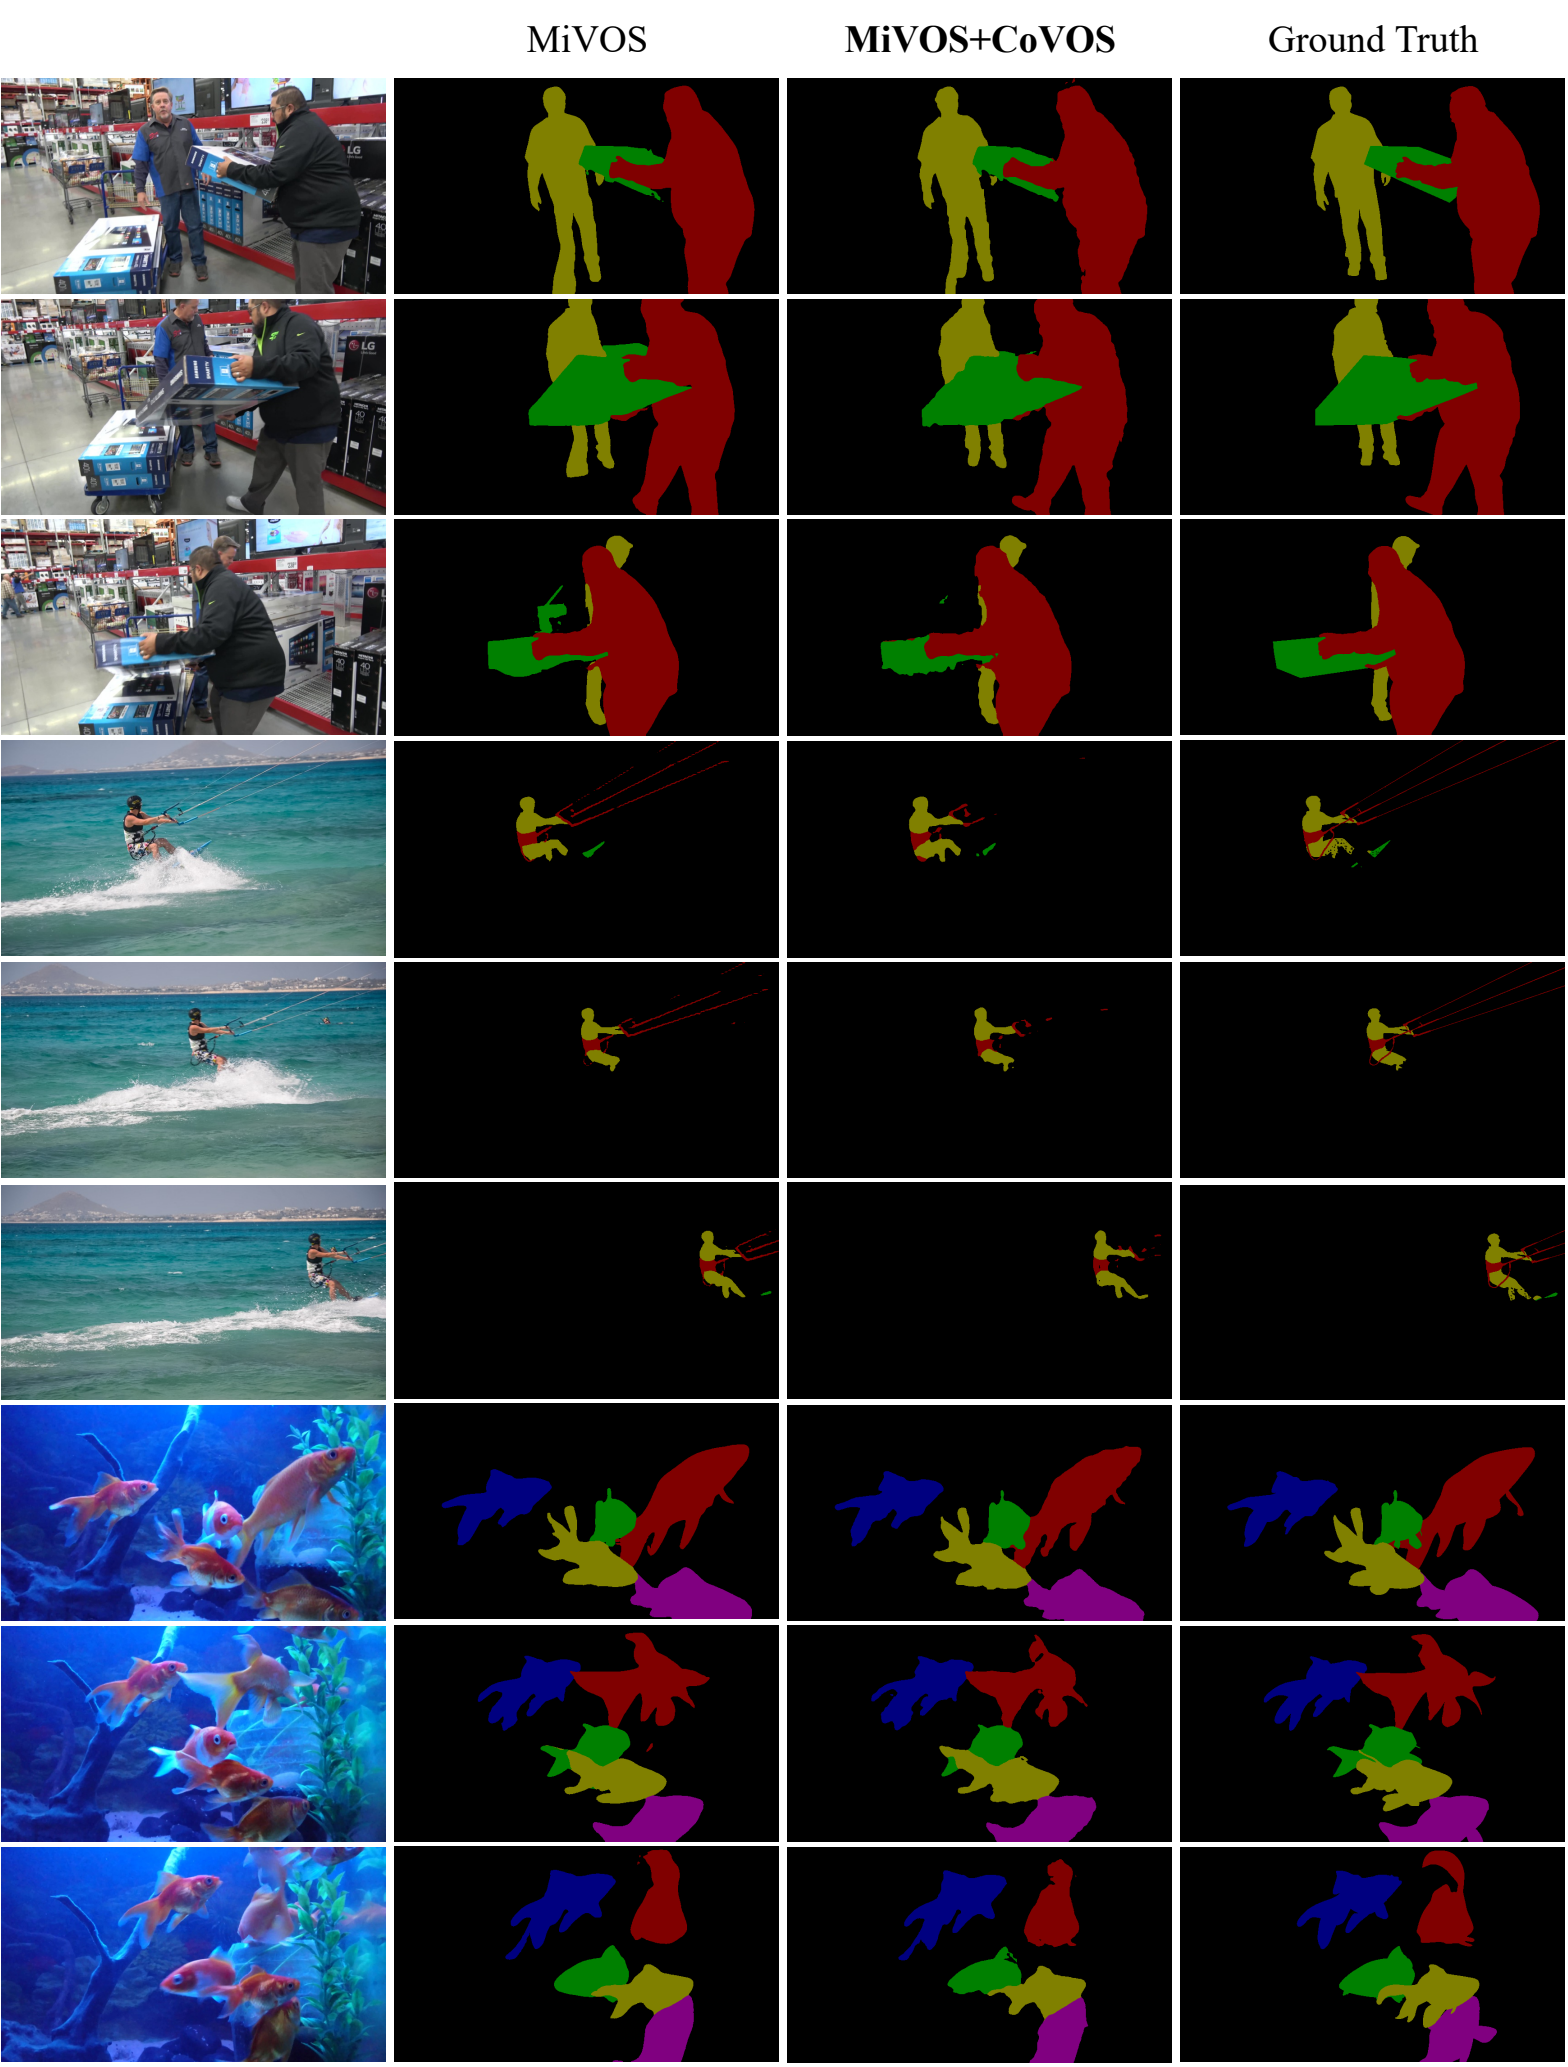   | 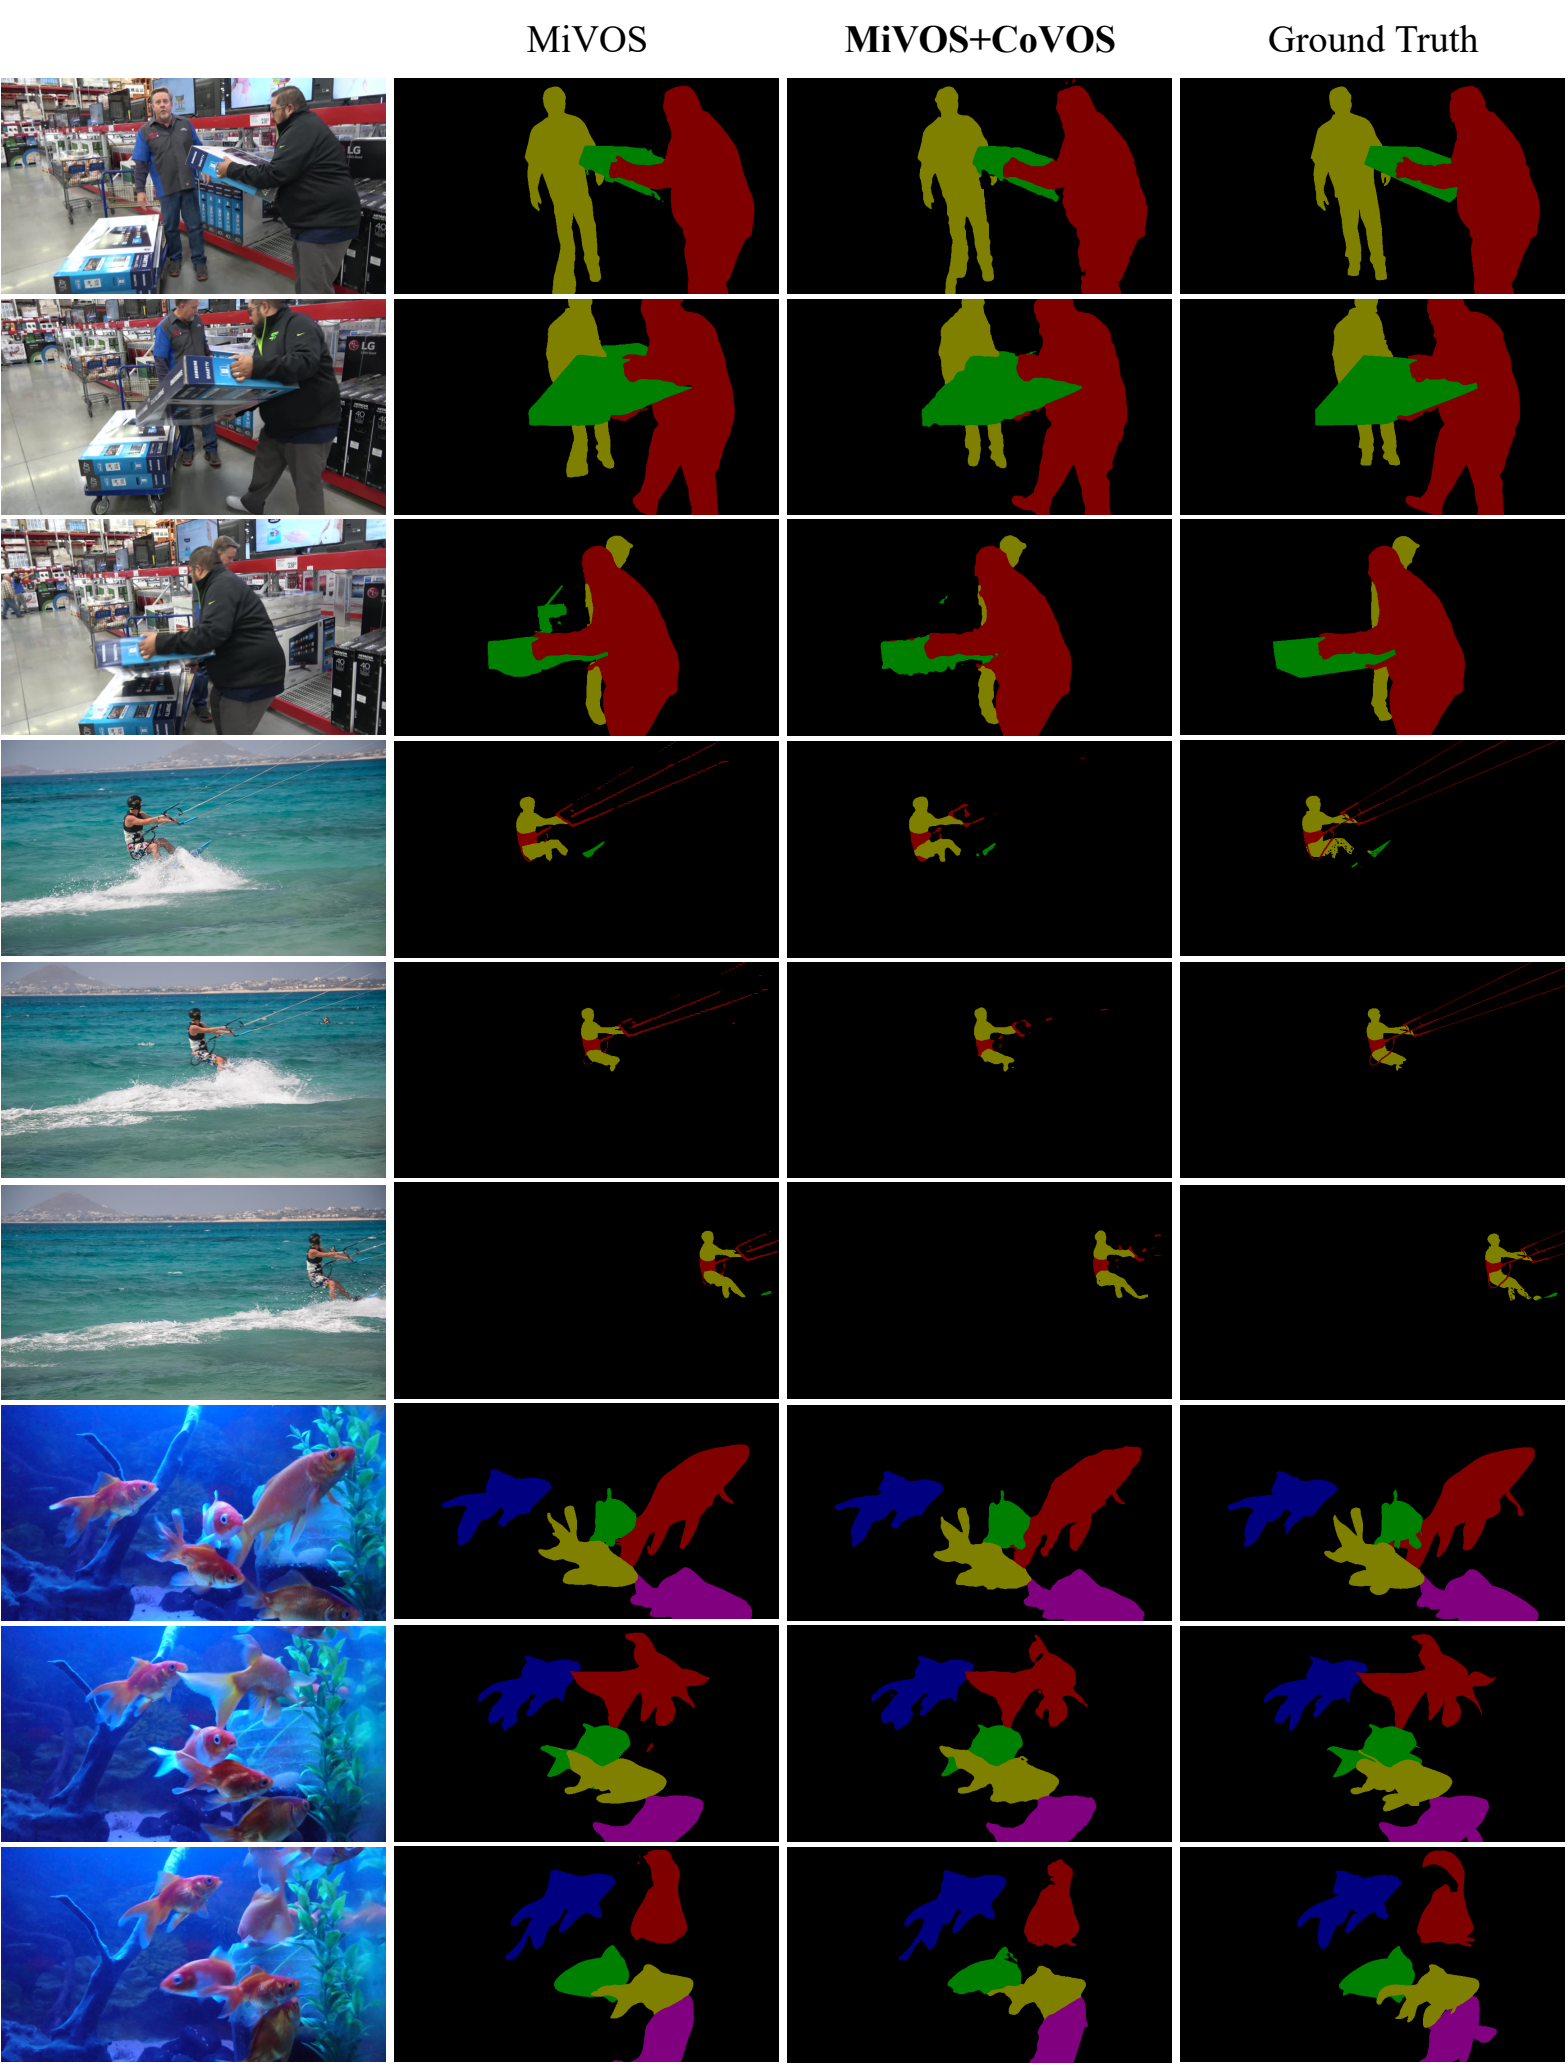   | 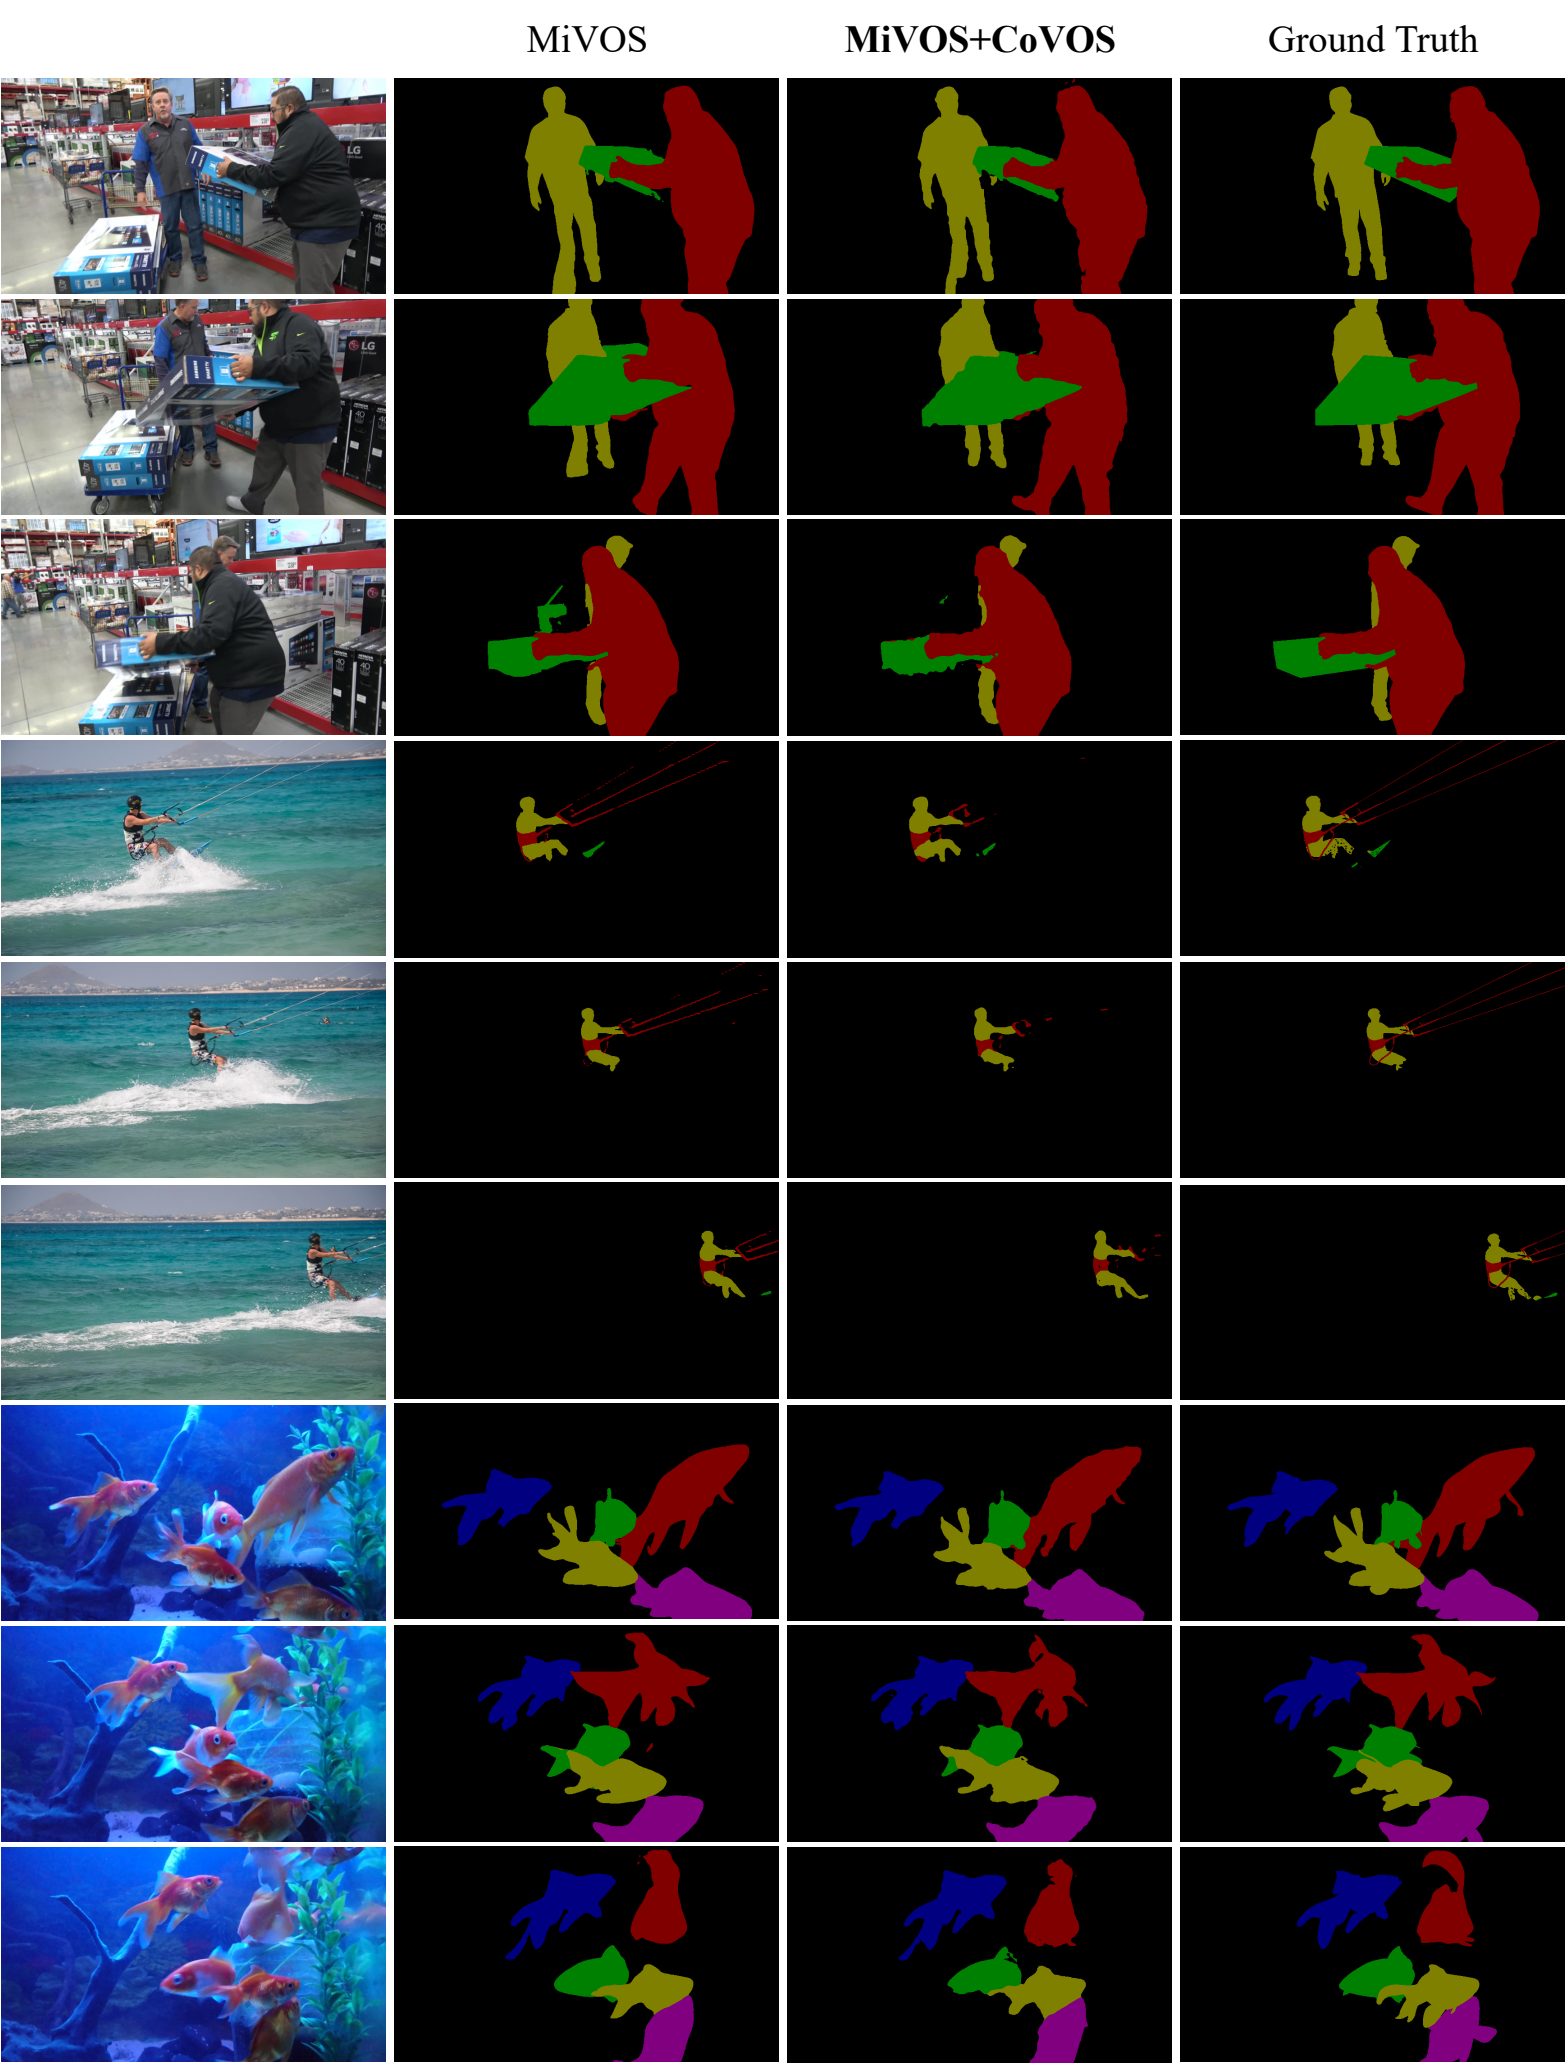   | 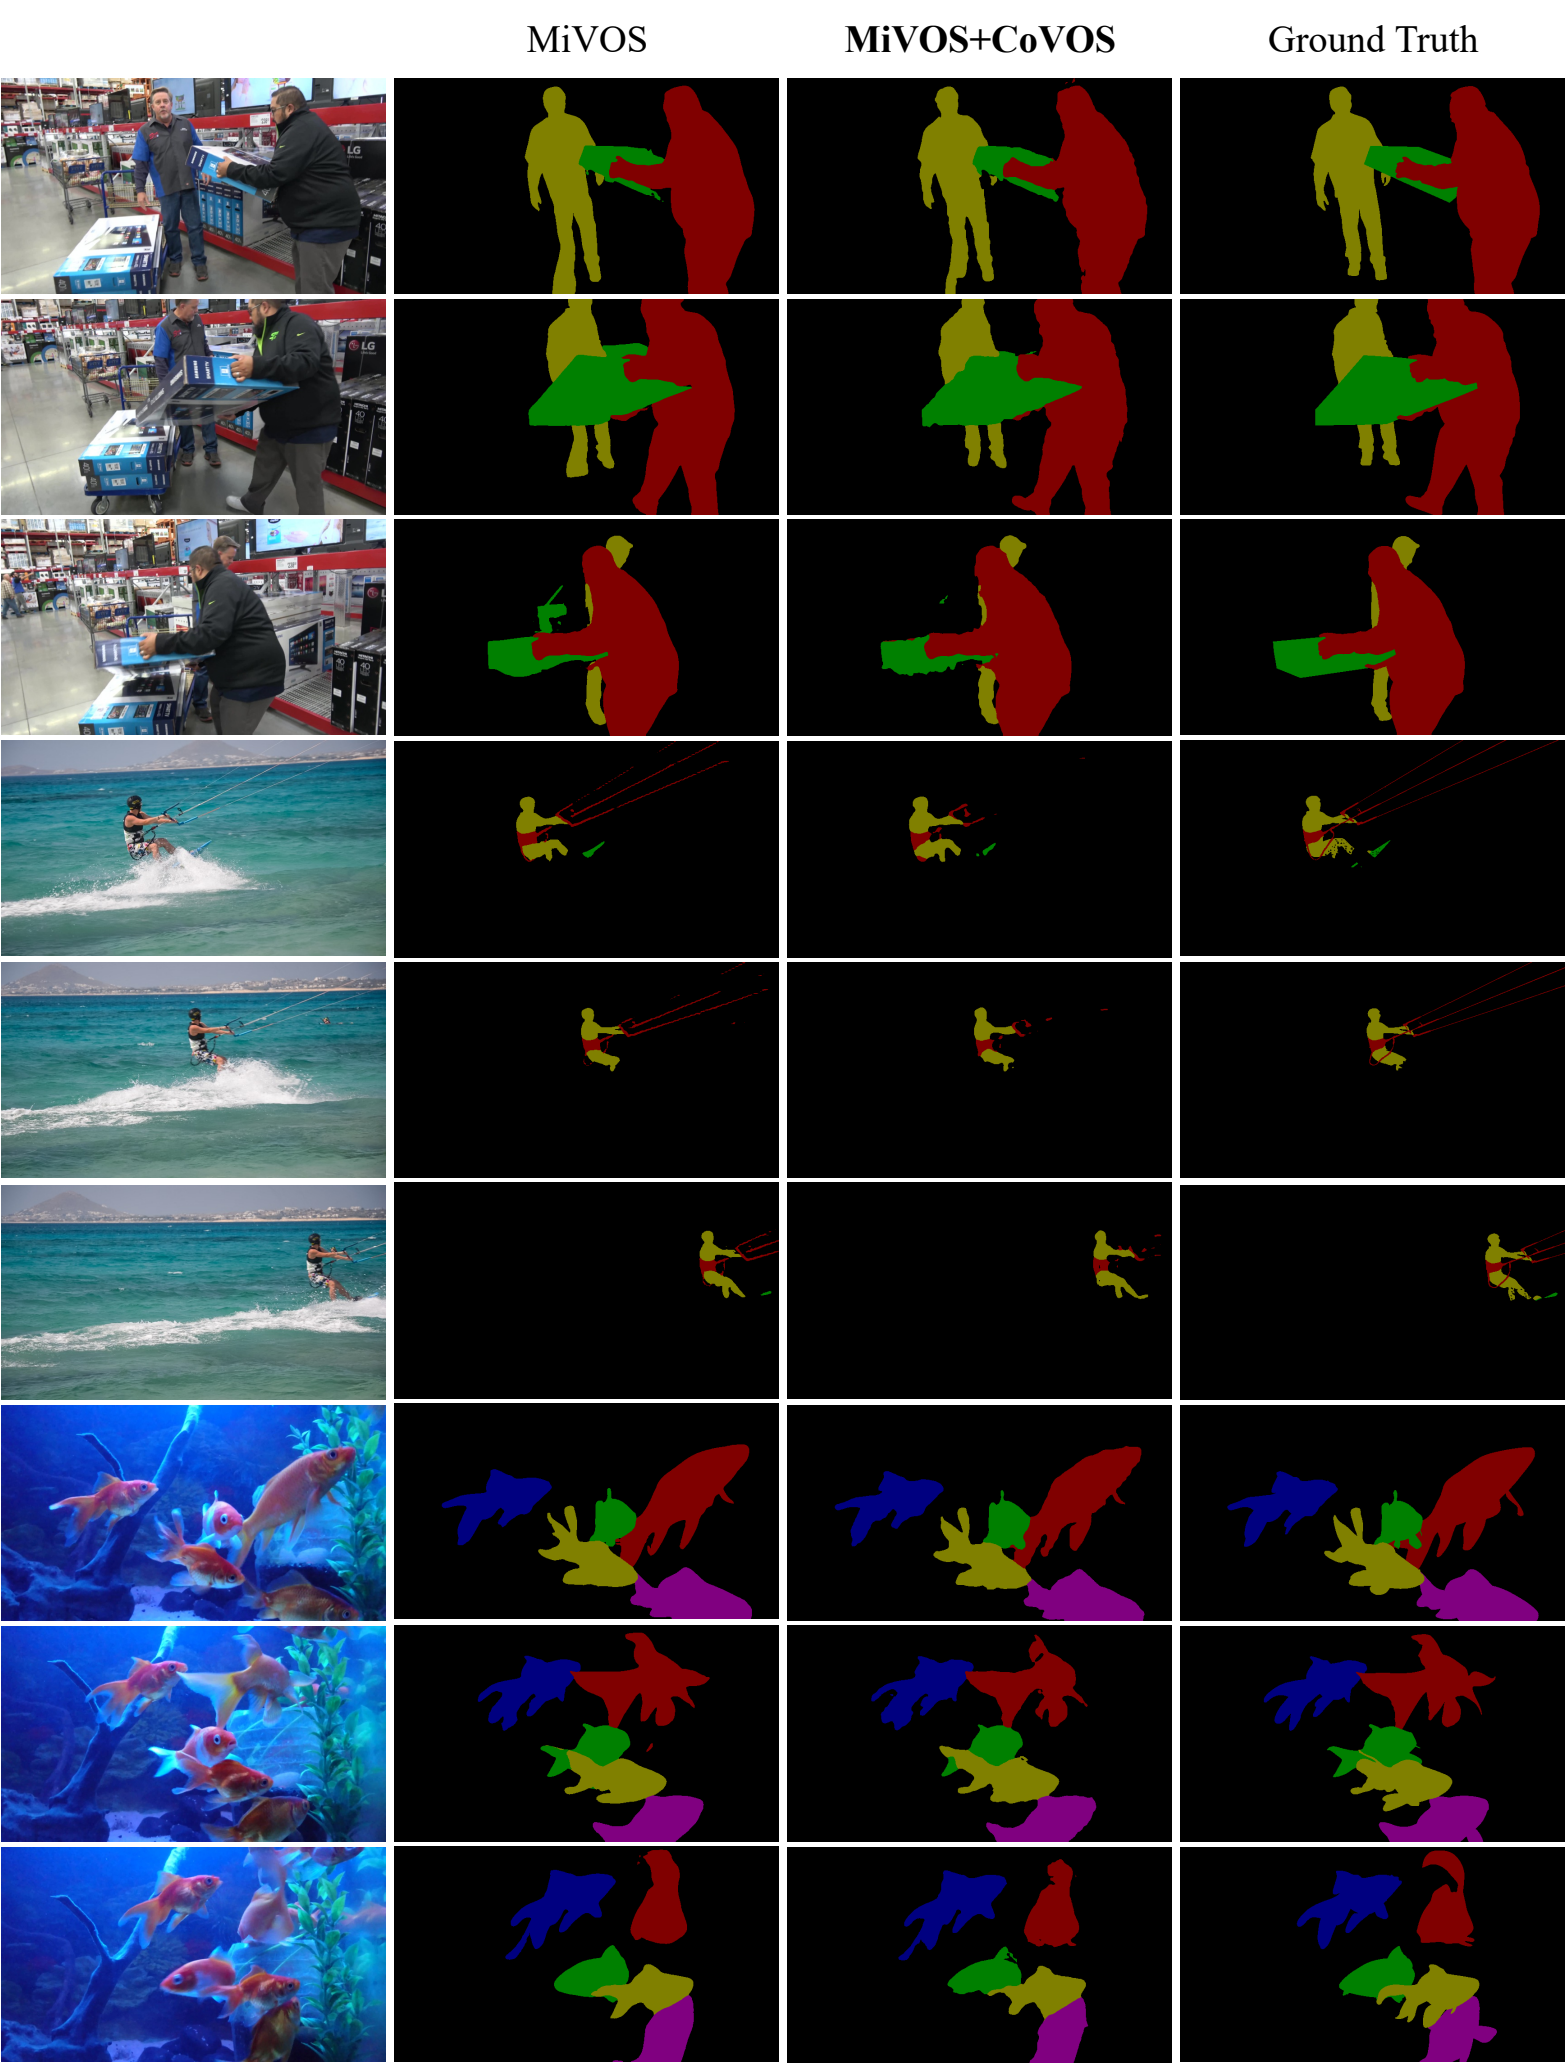   |
| 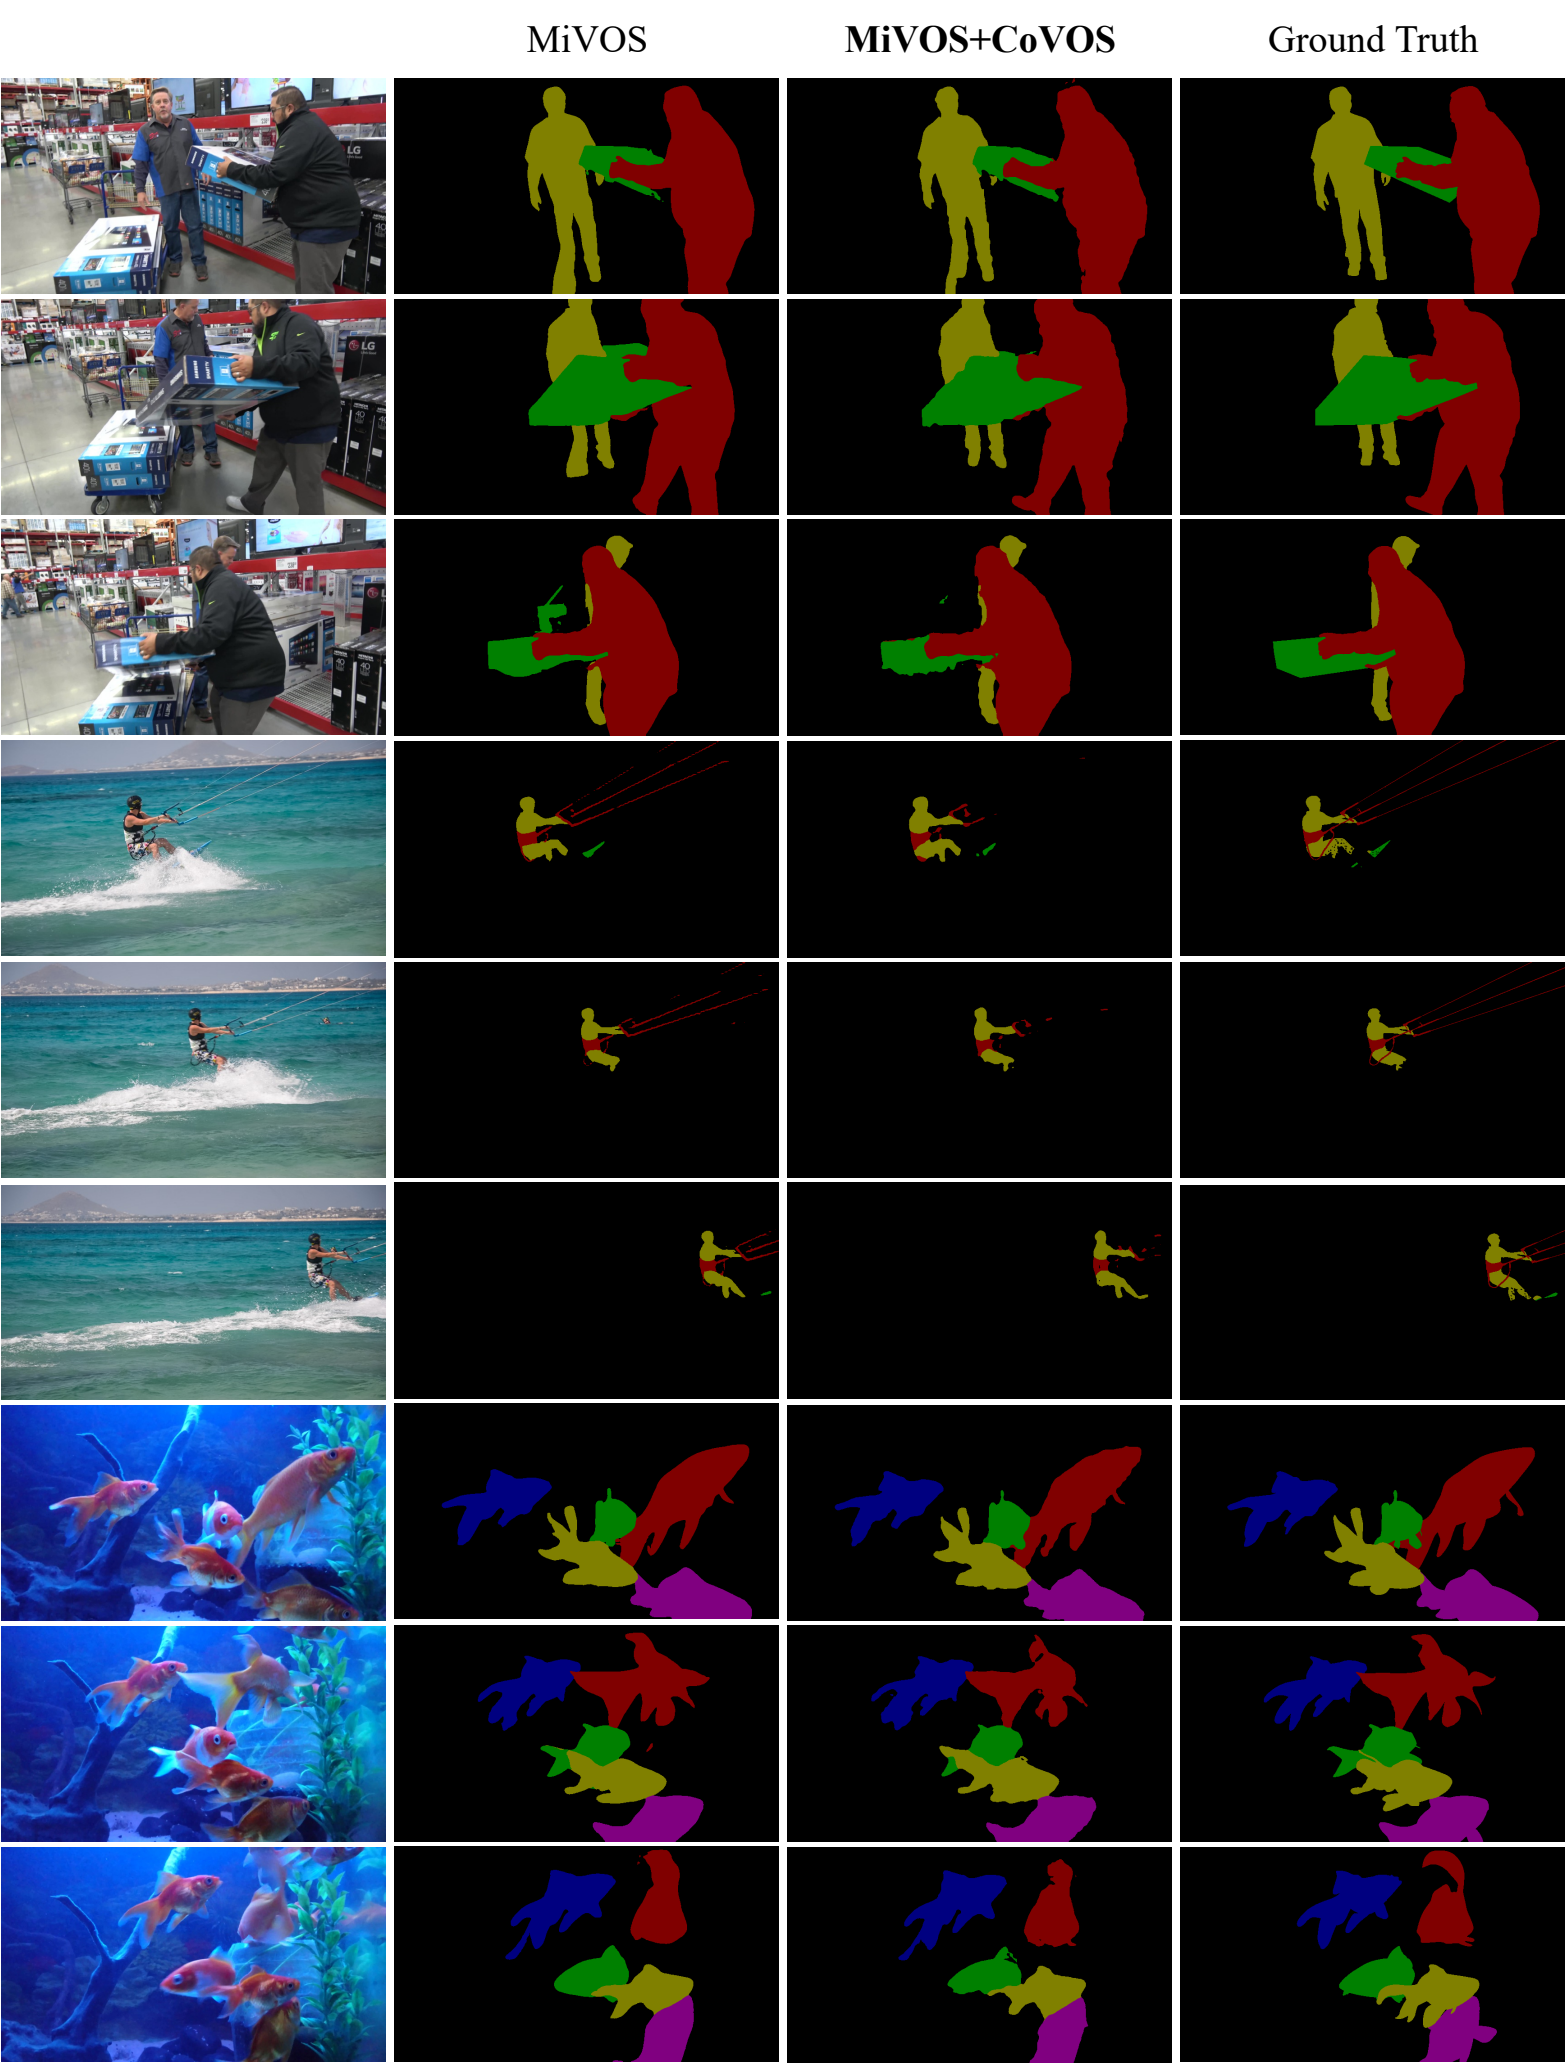   | 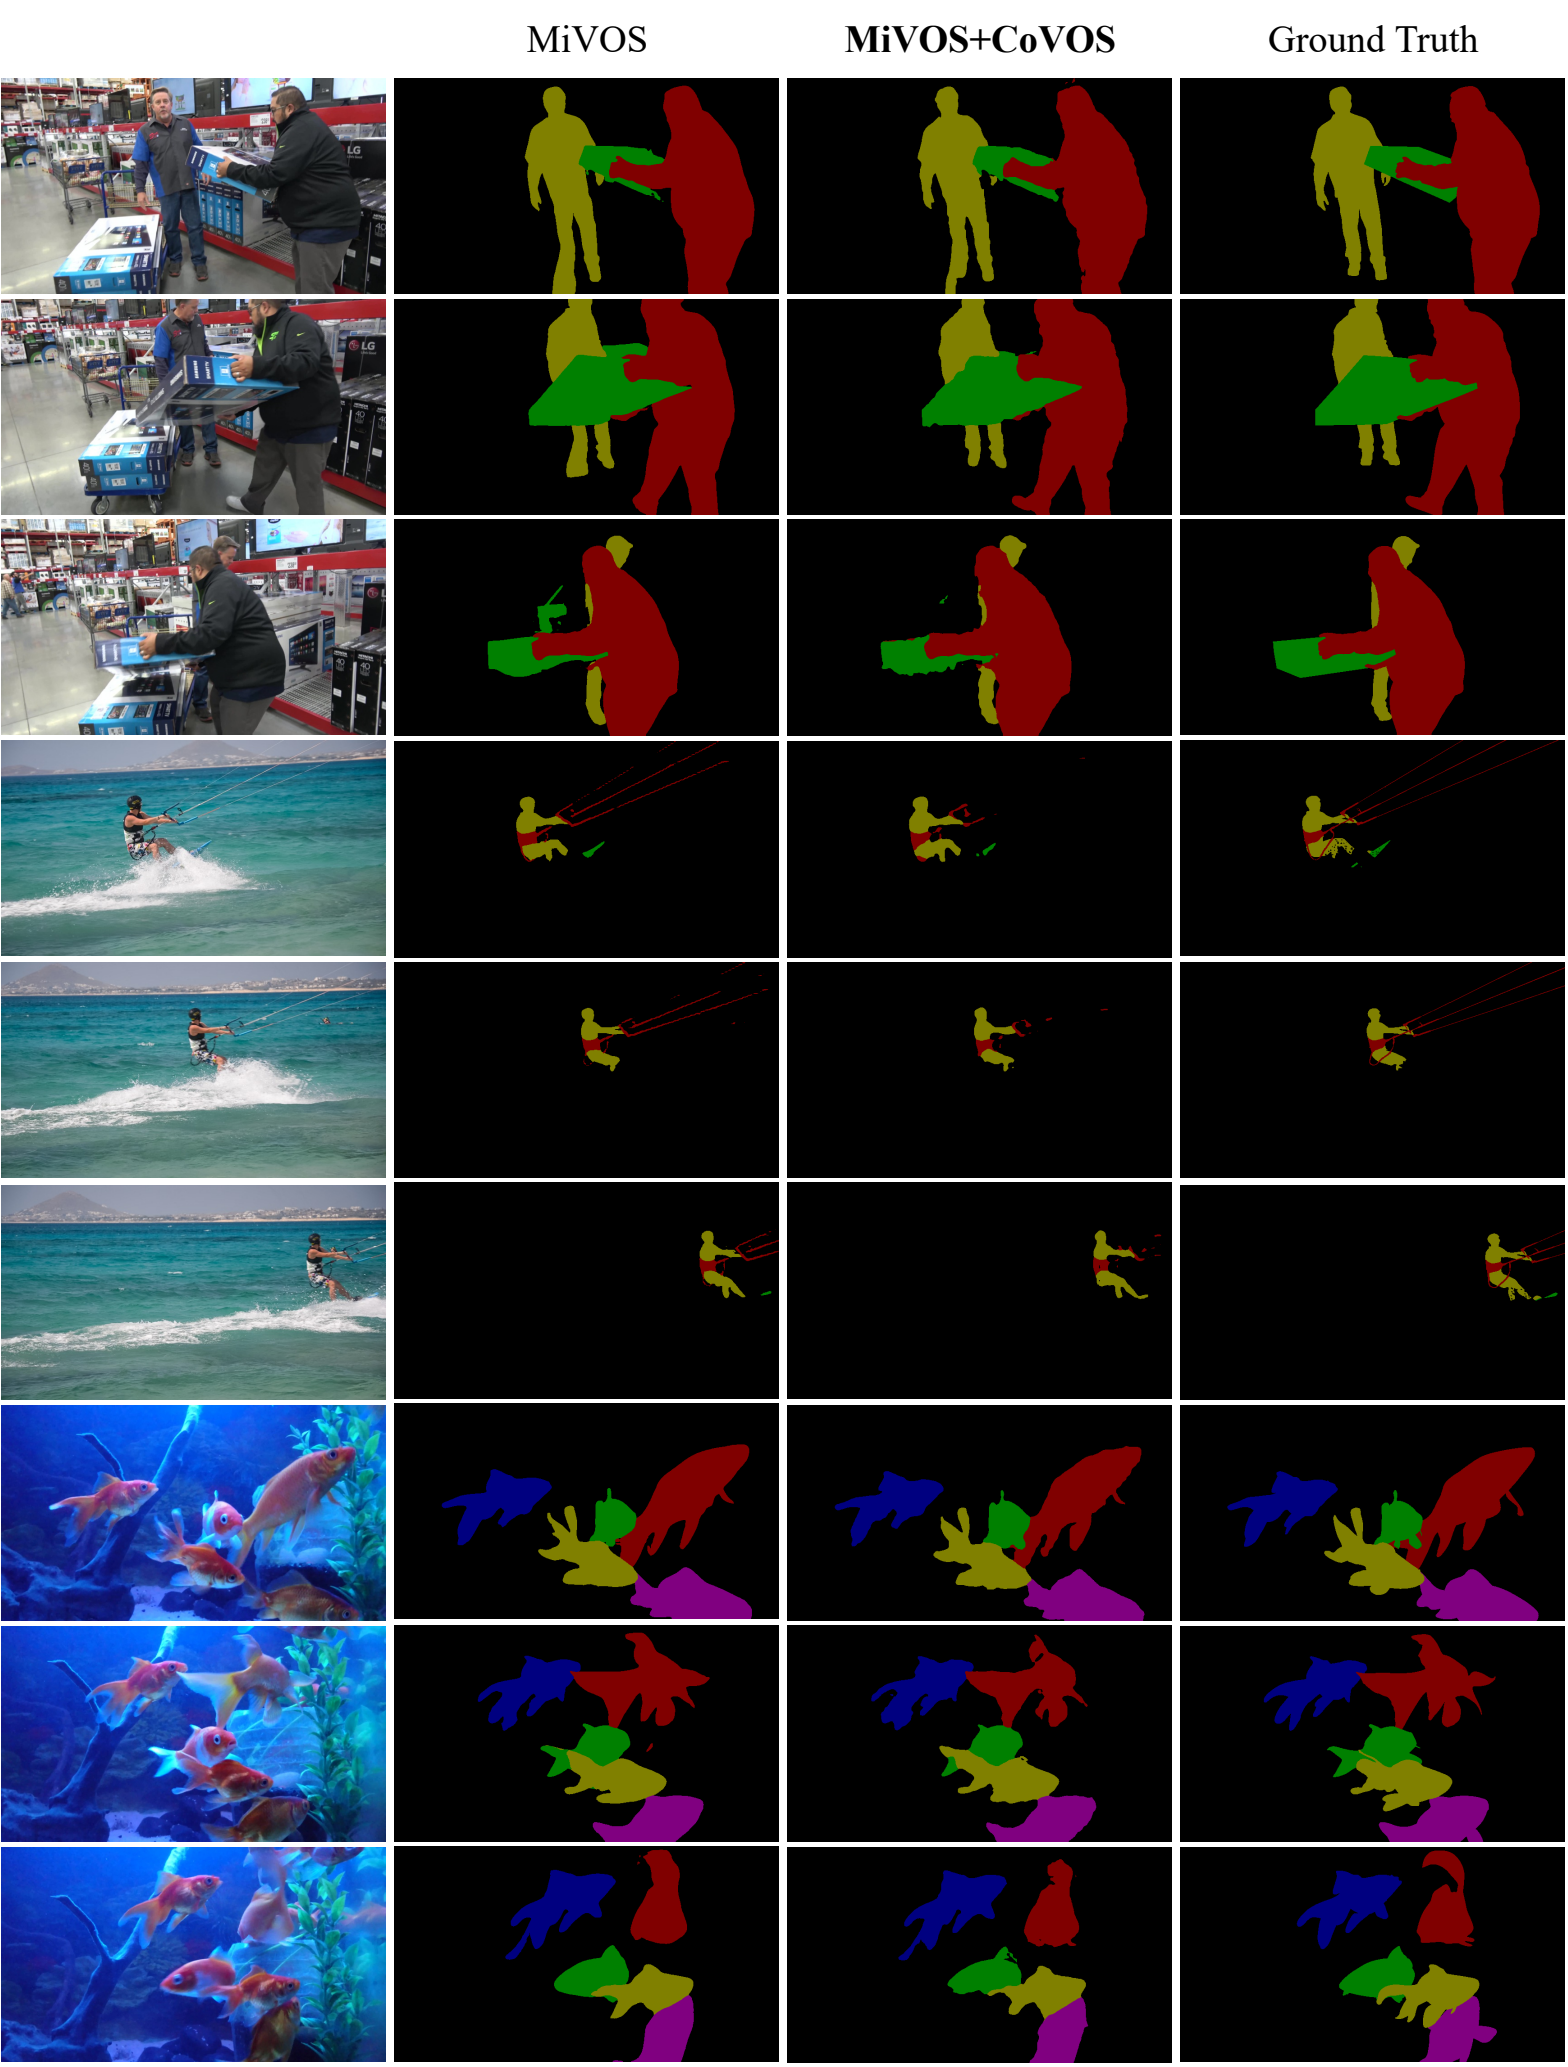   | 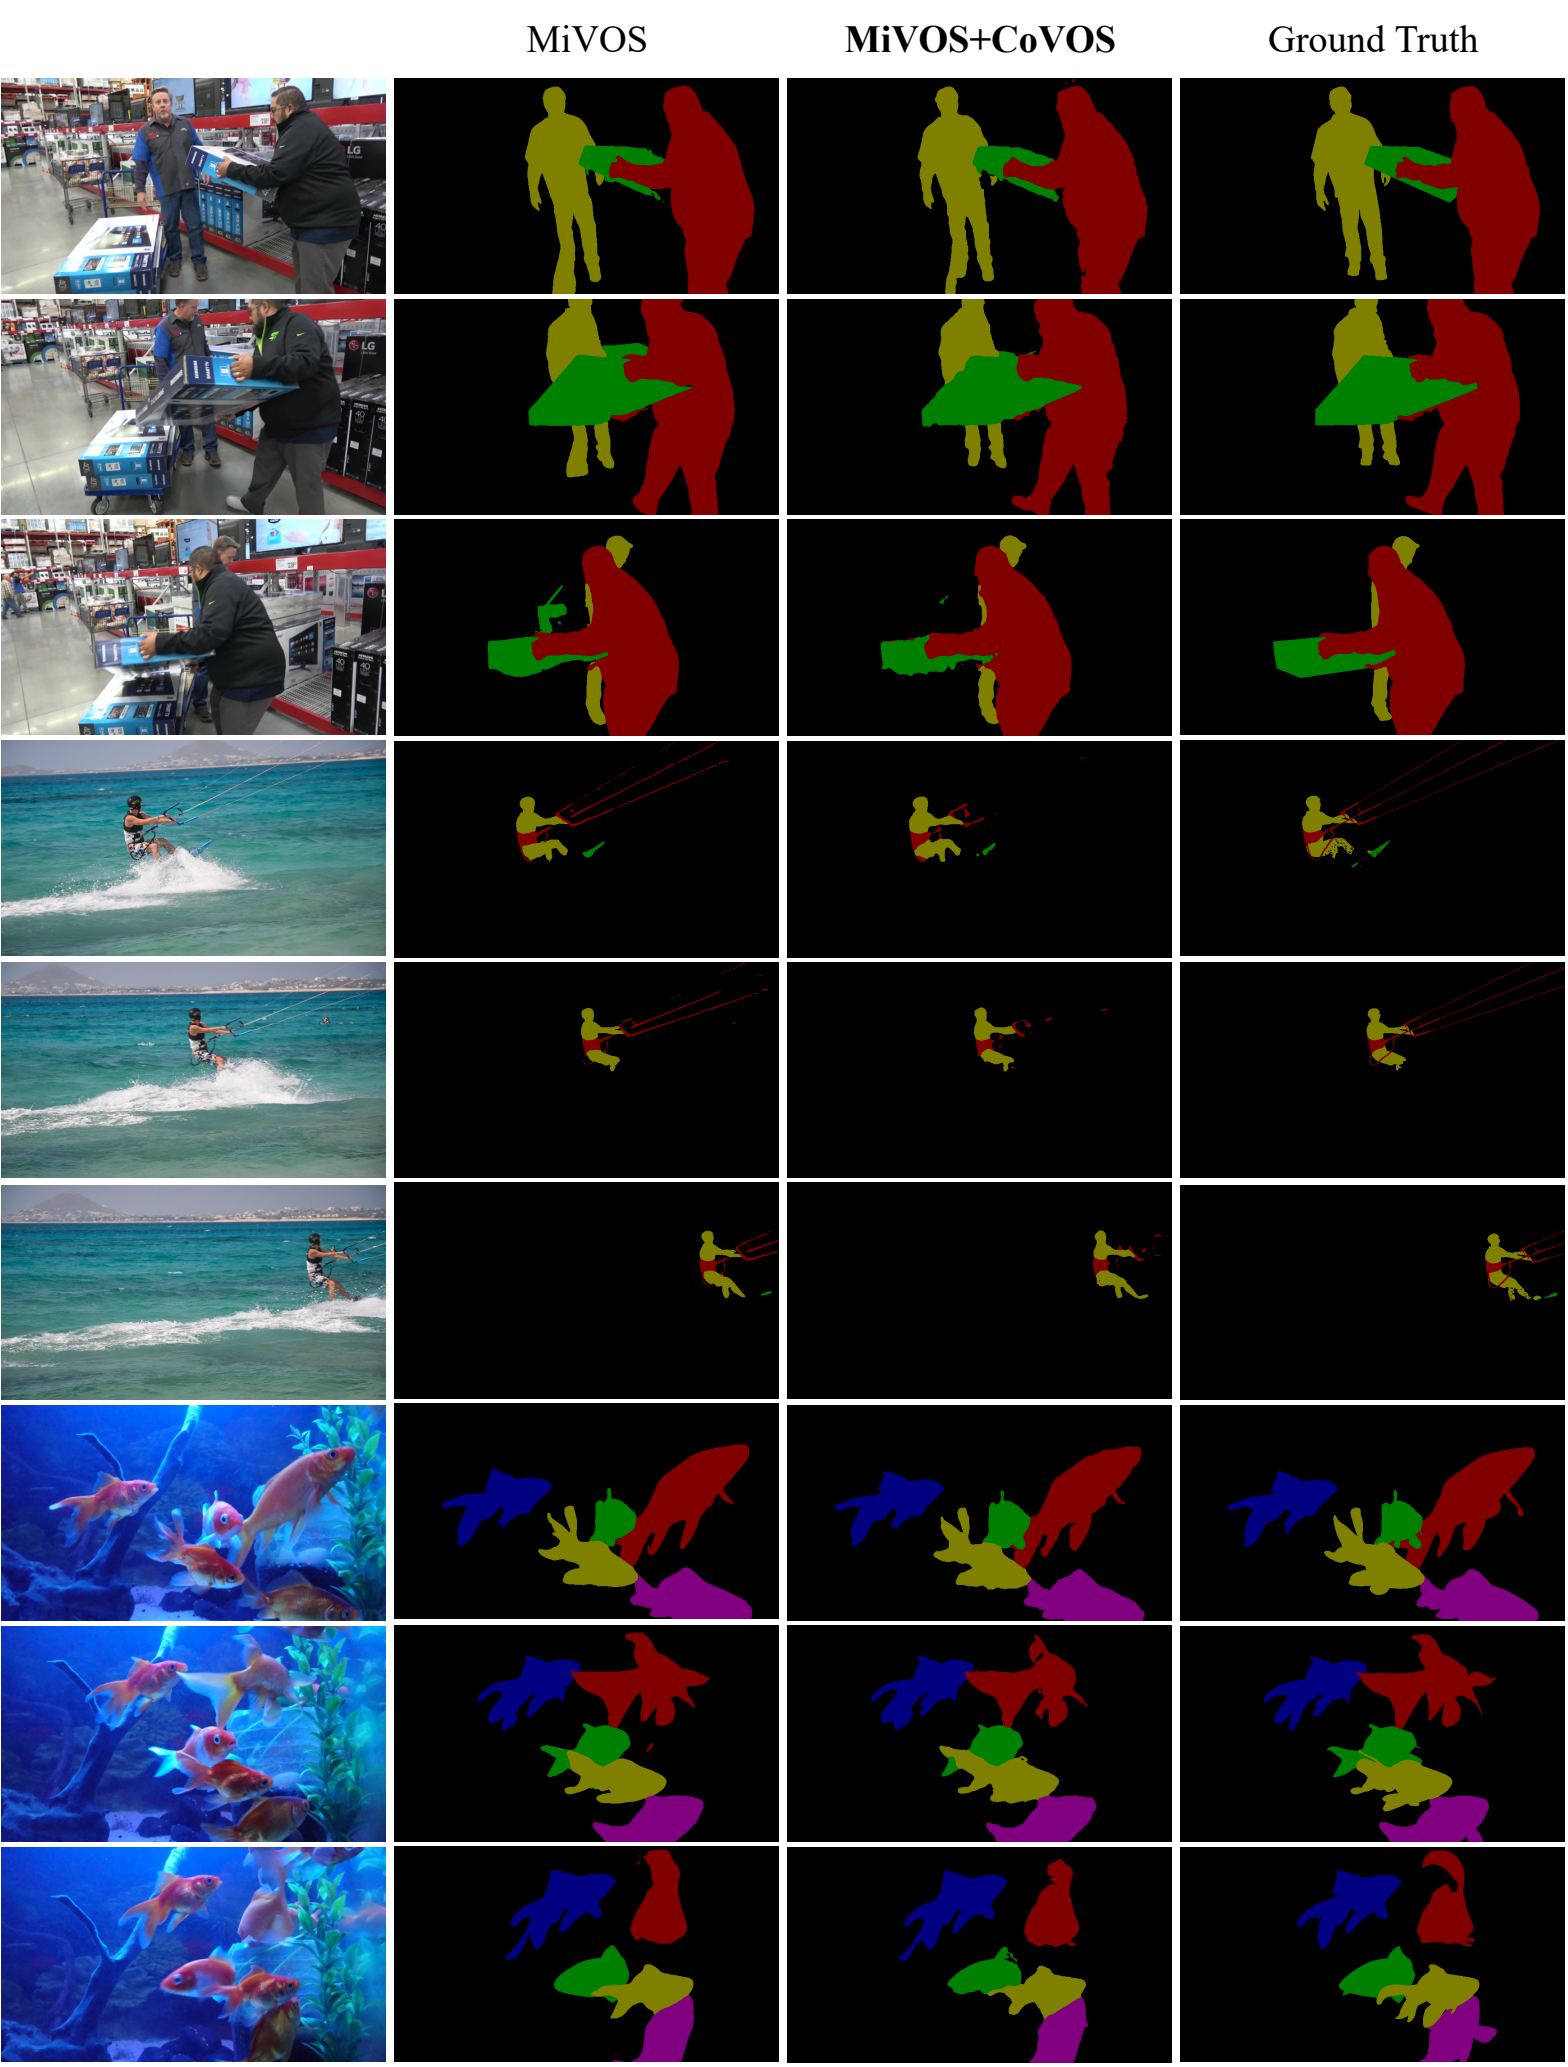   | 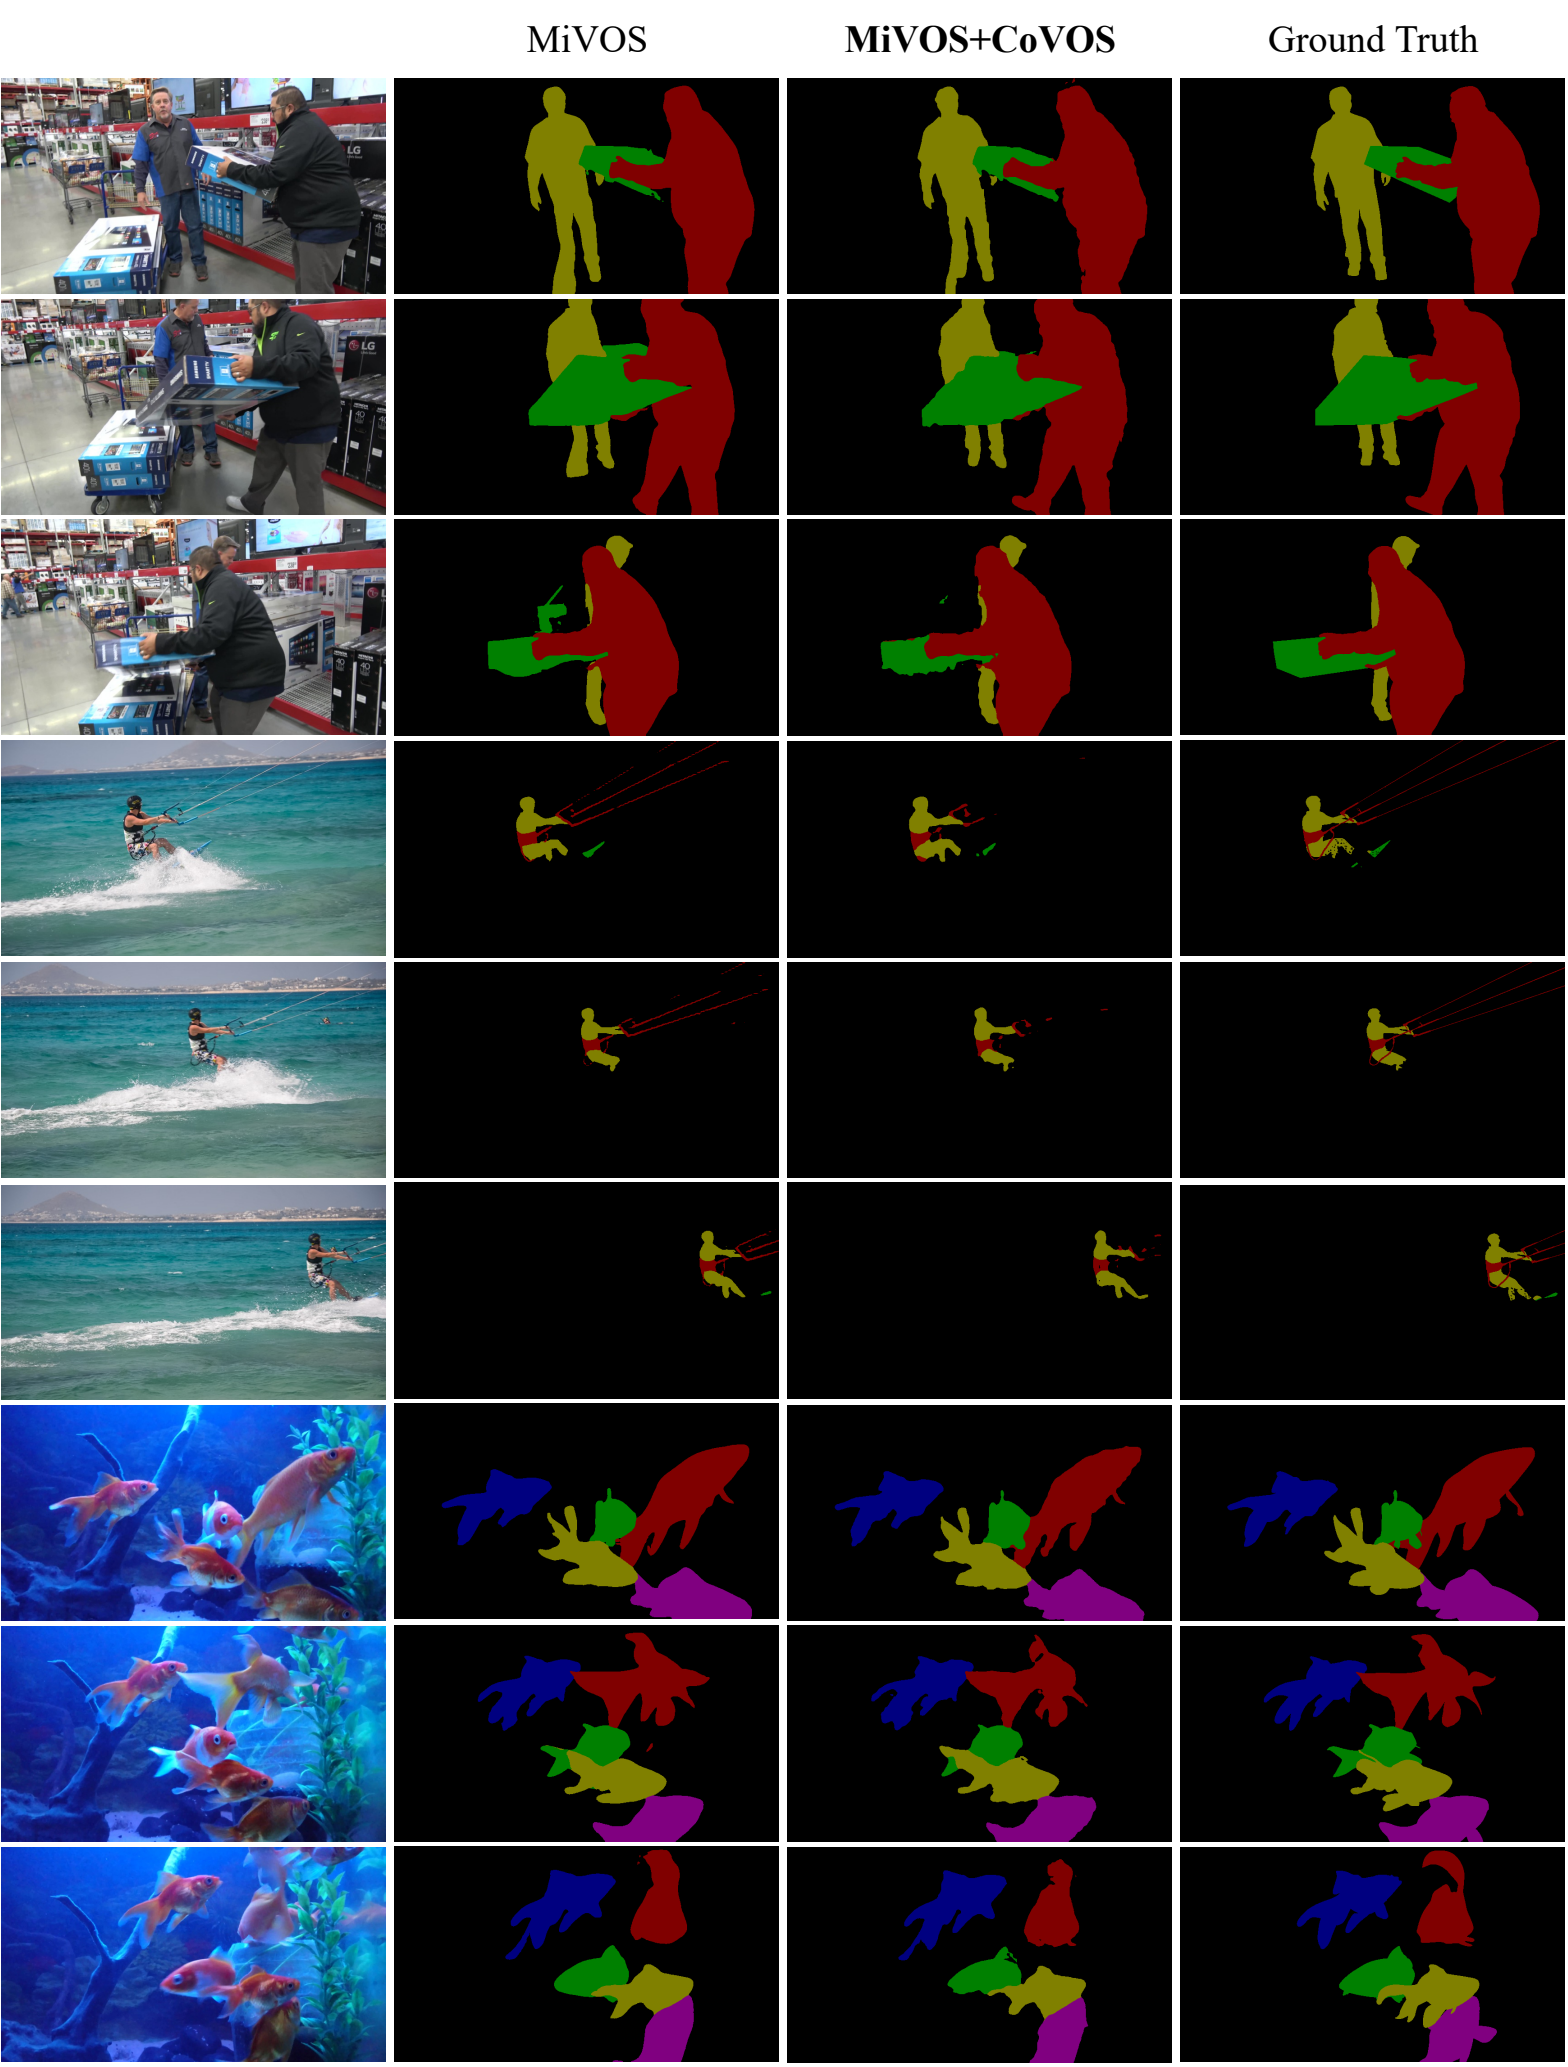   |
| 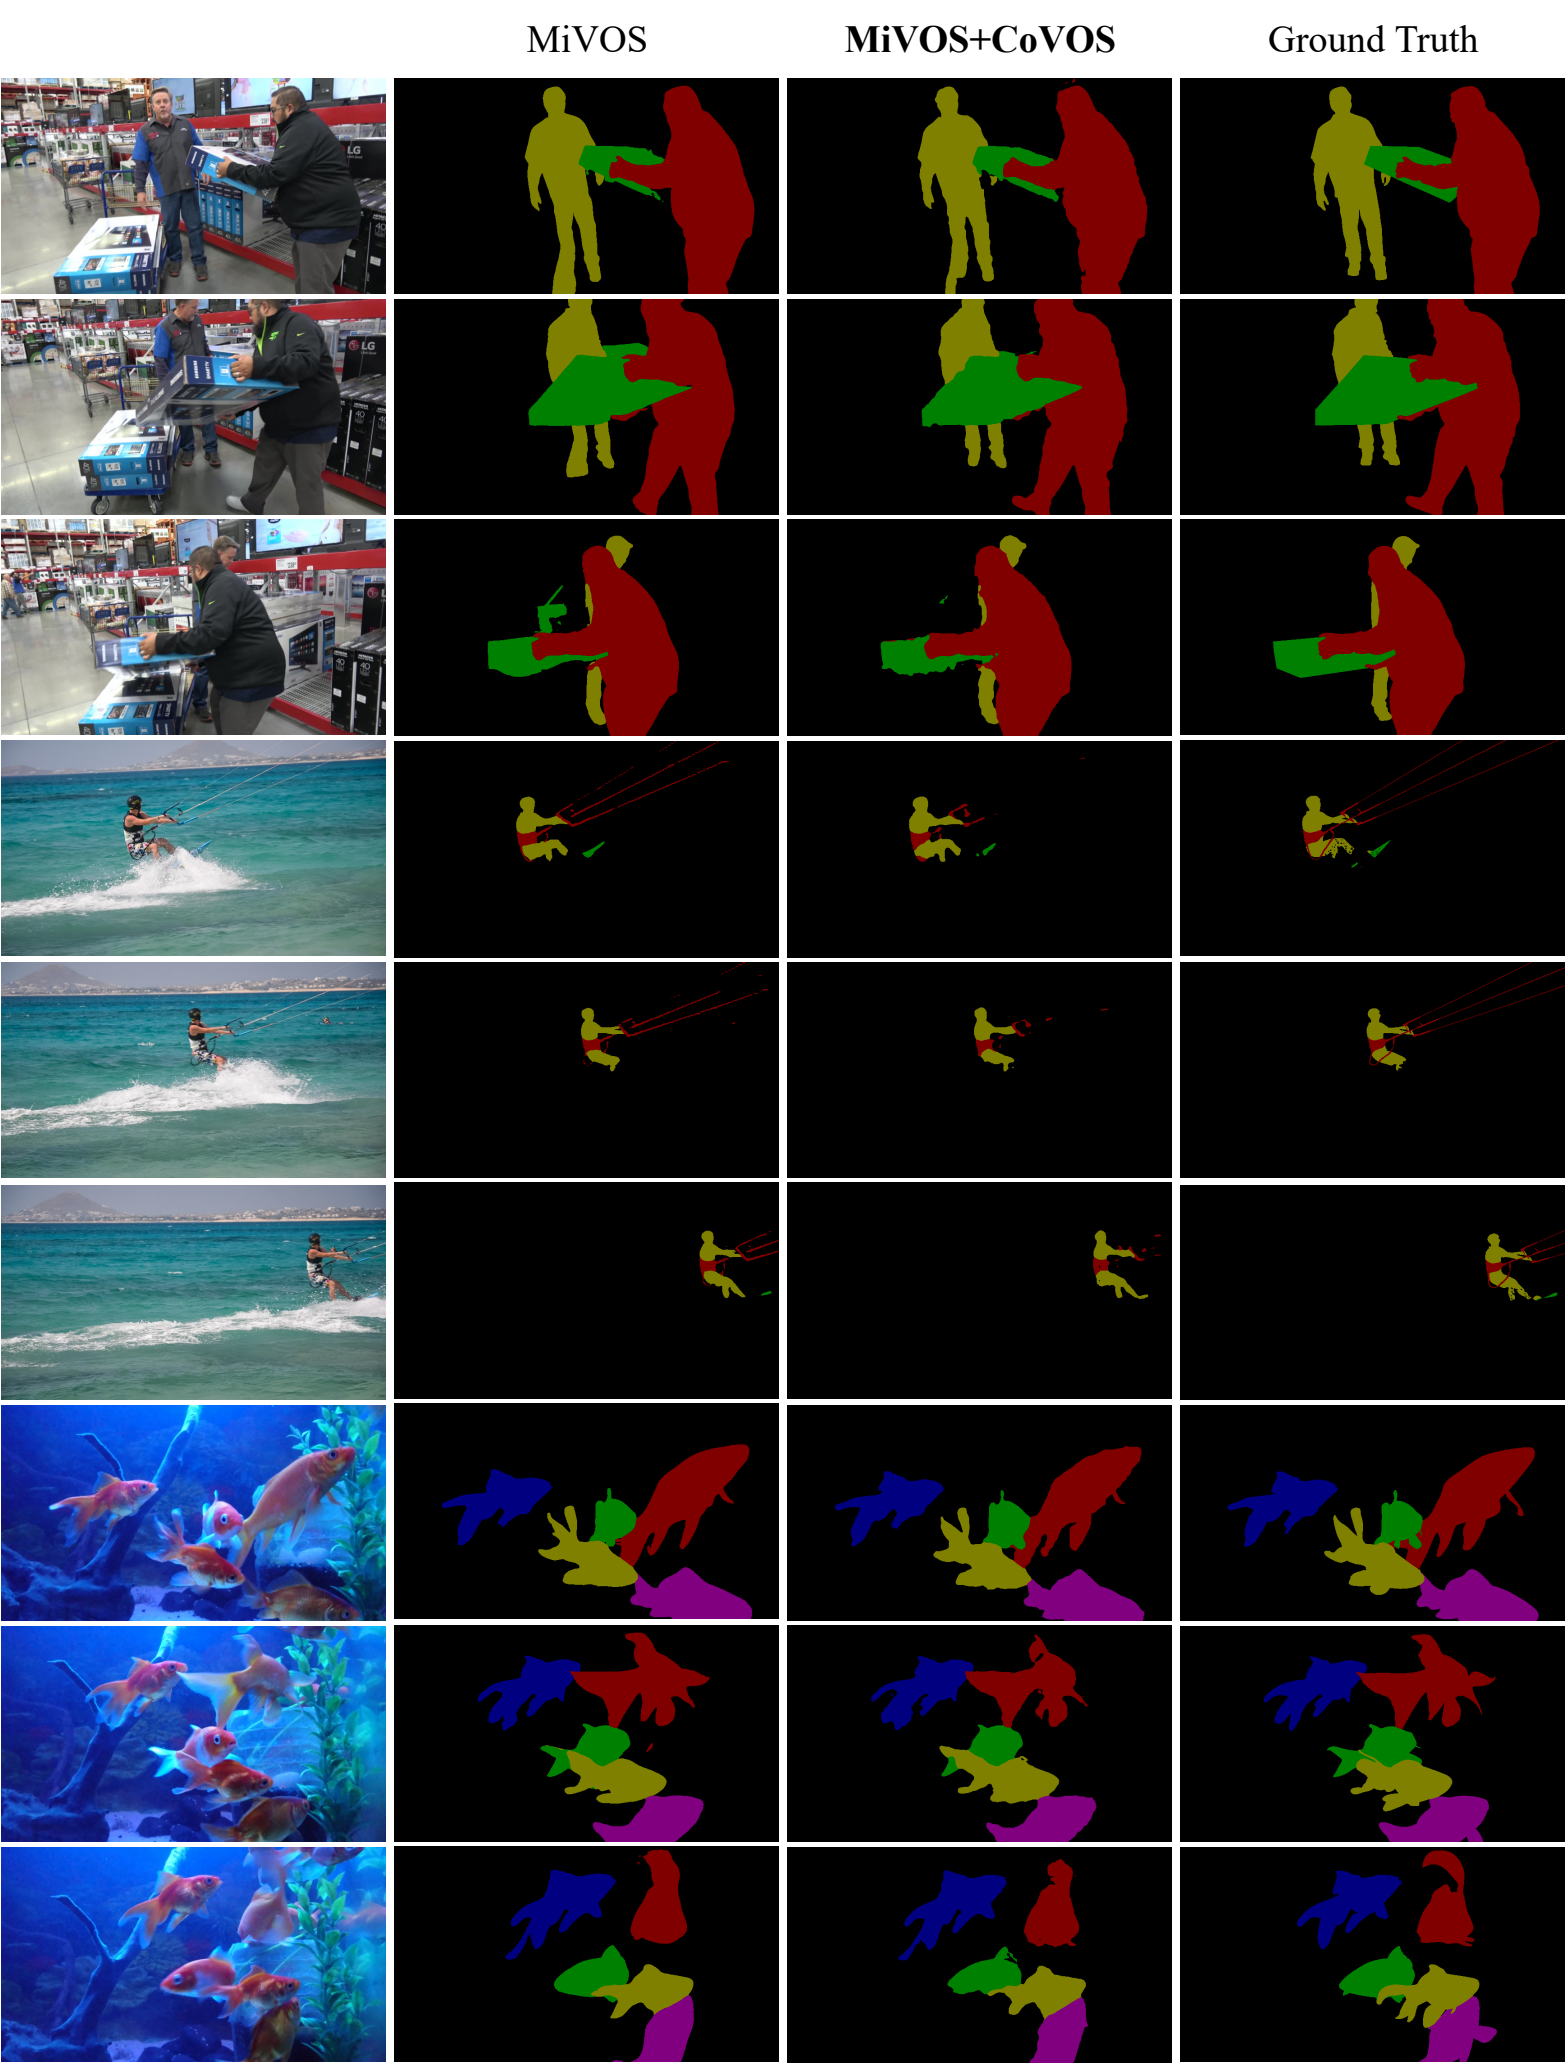   | 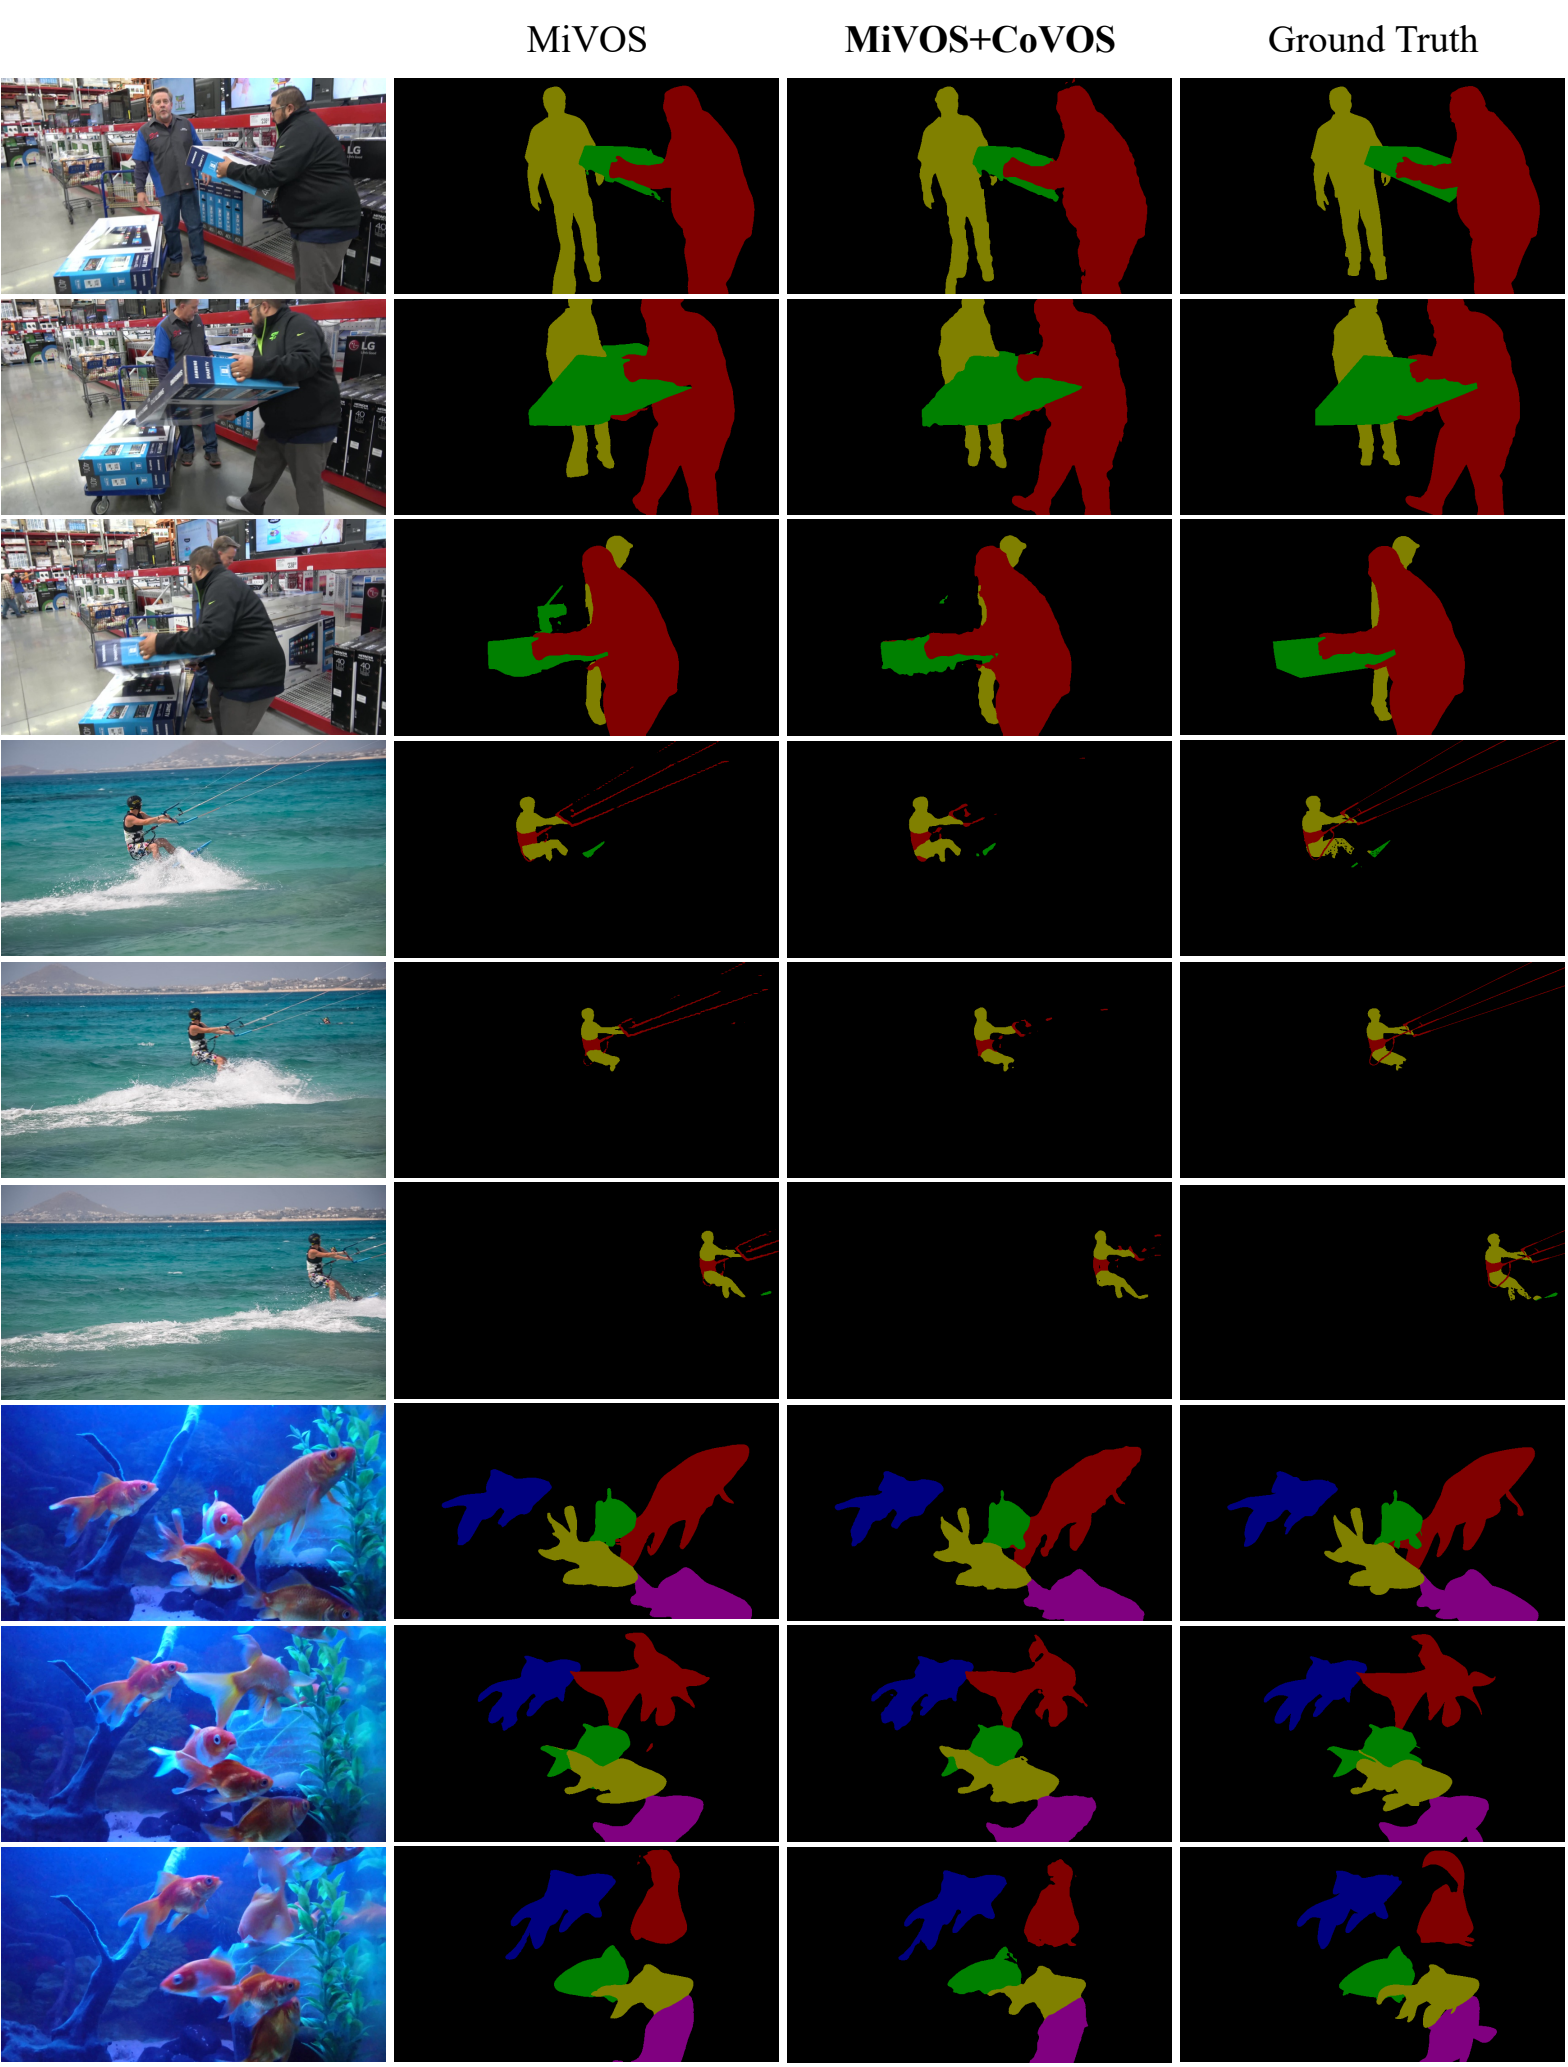   | 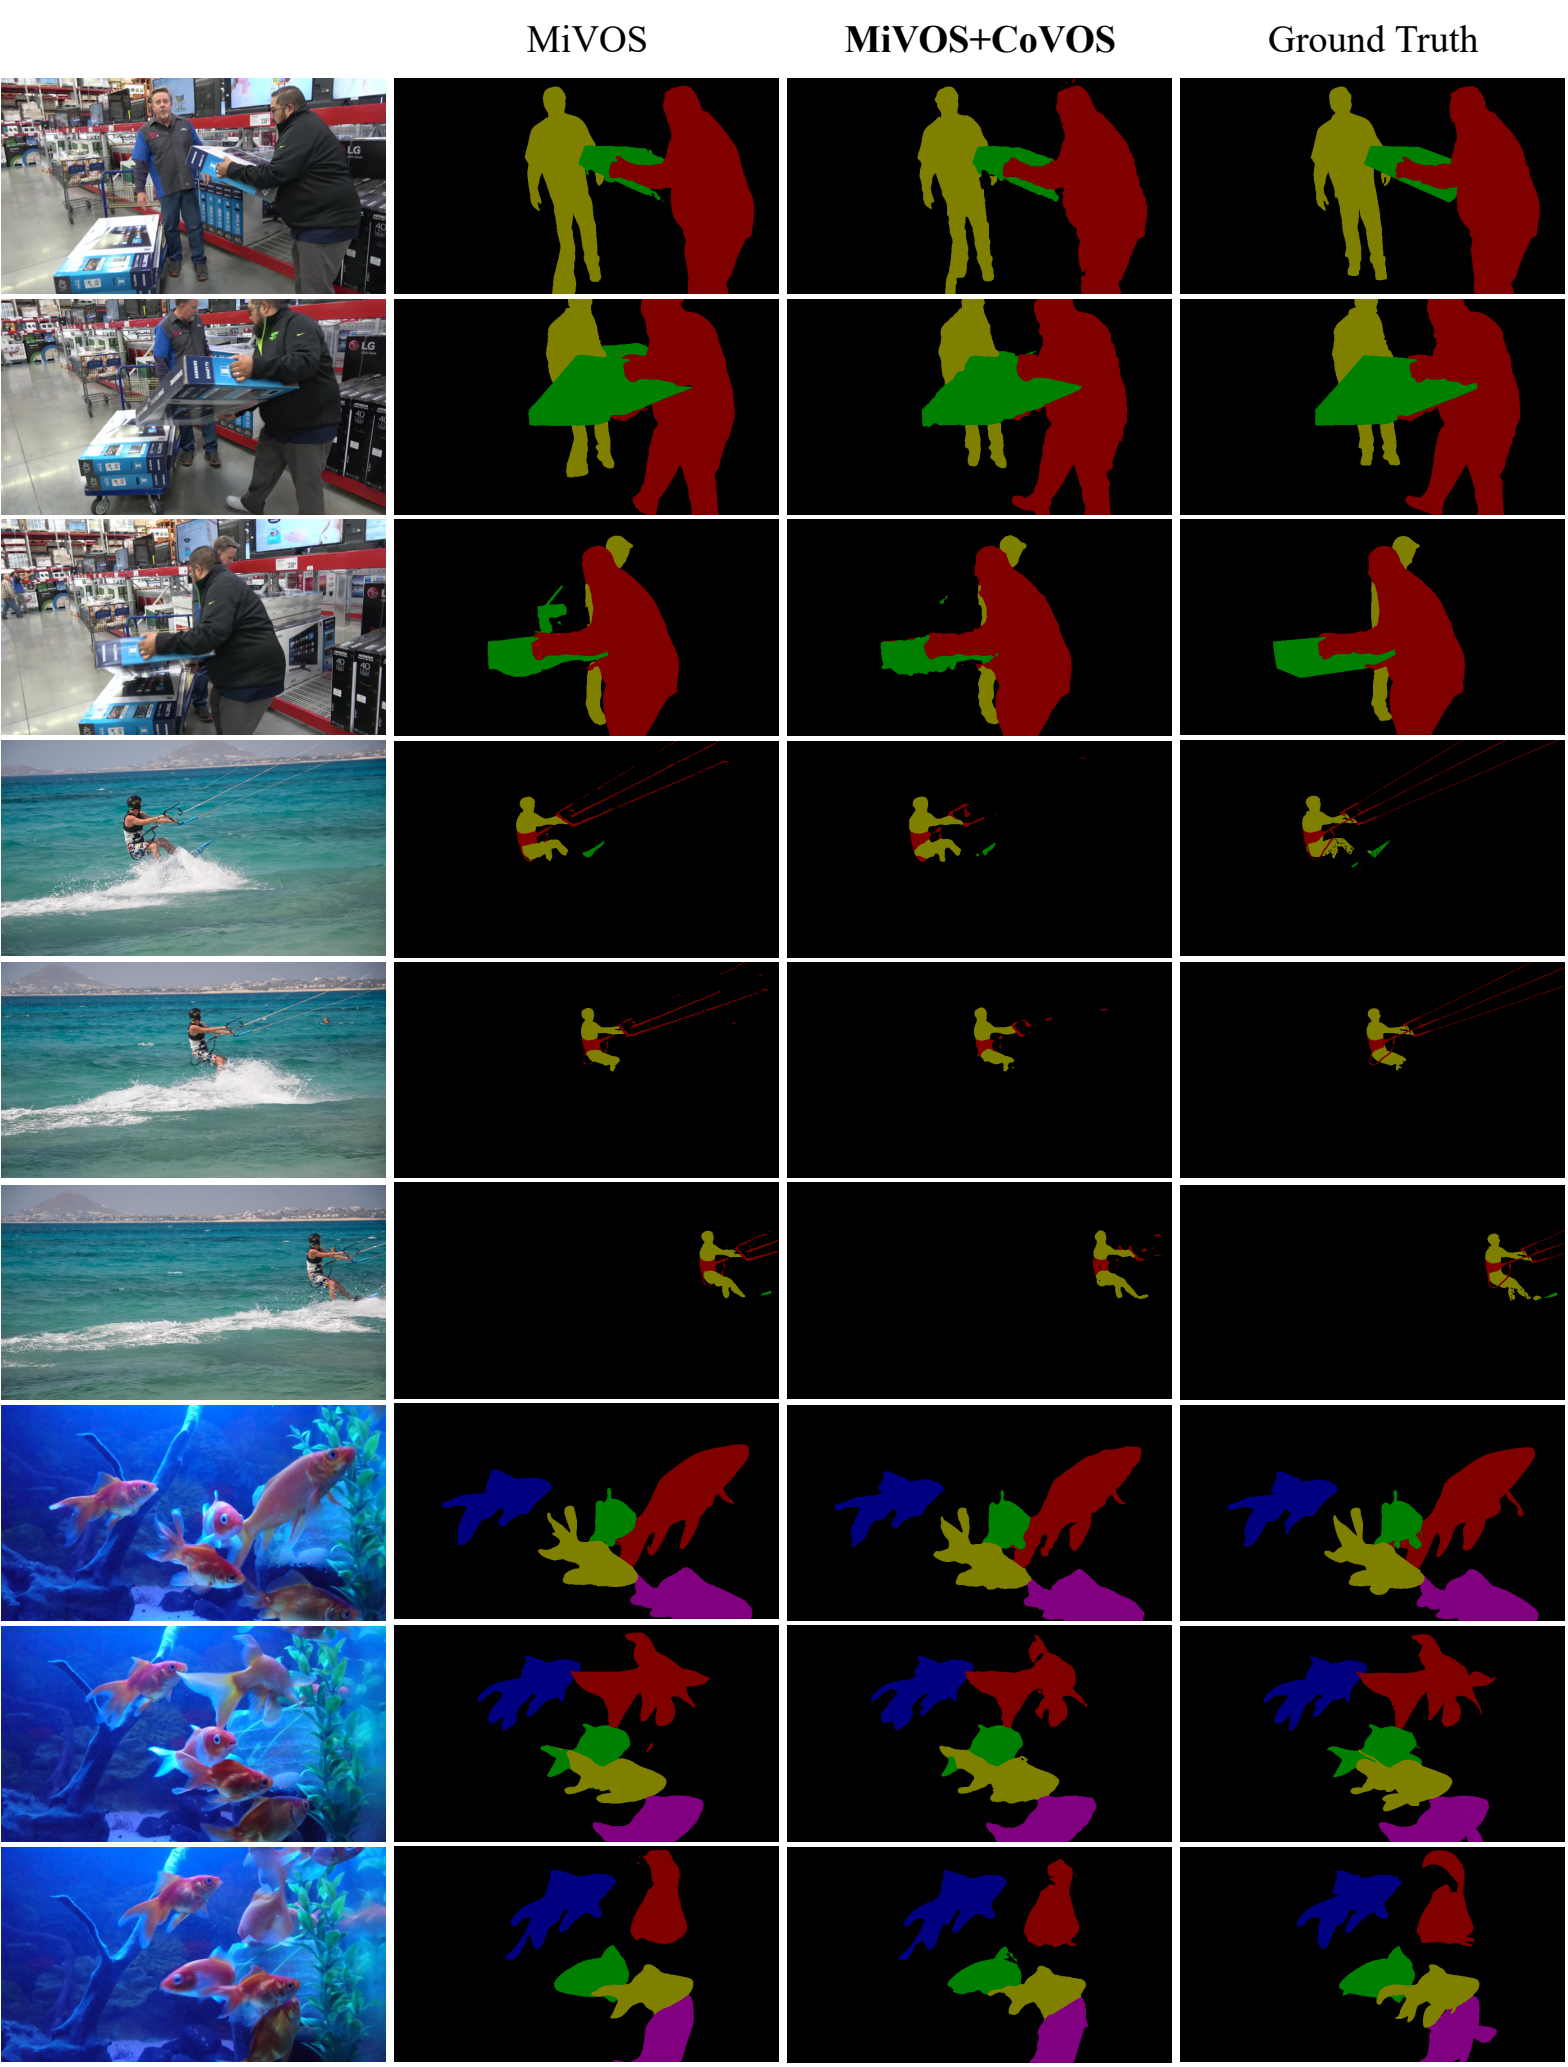   | 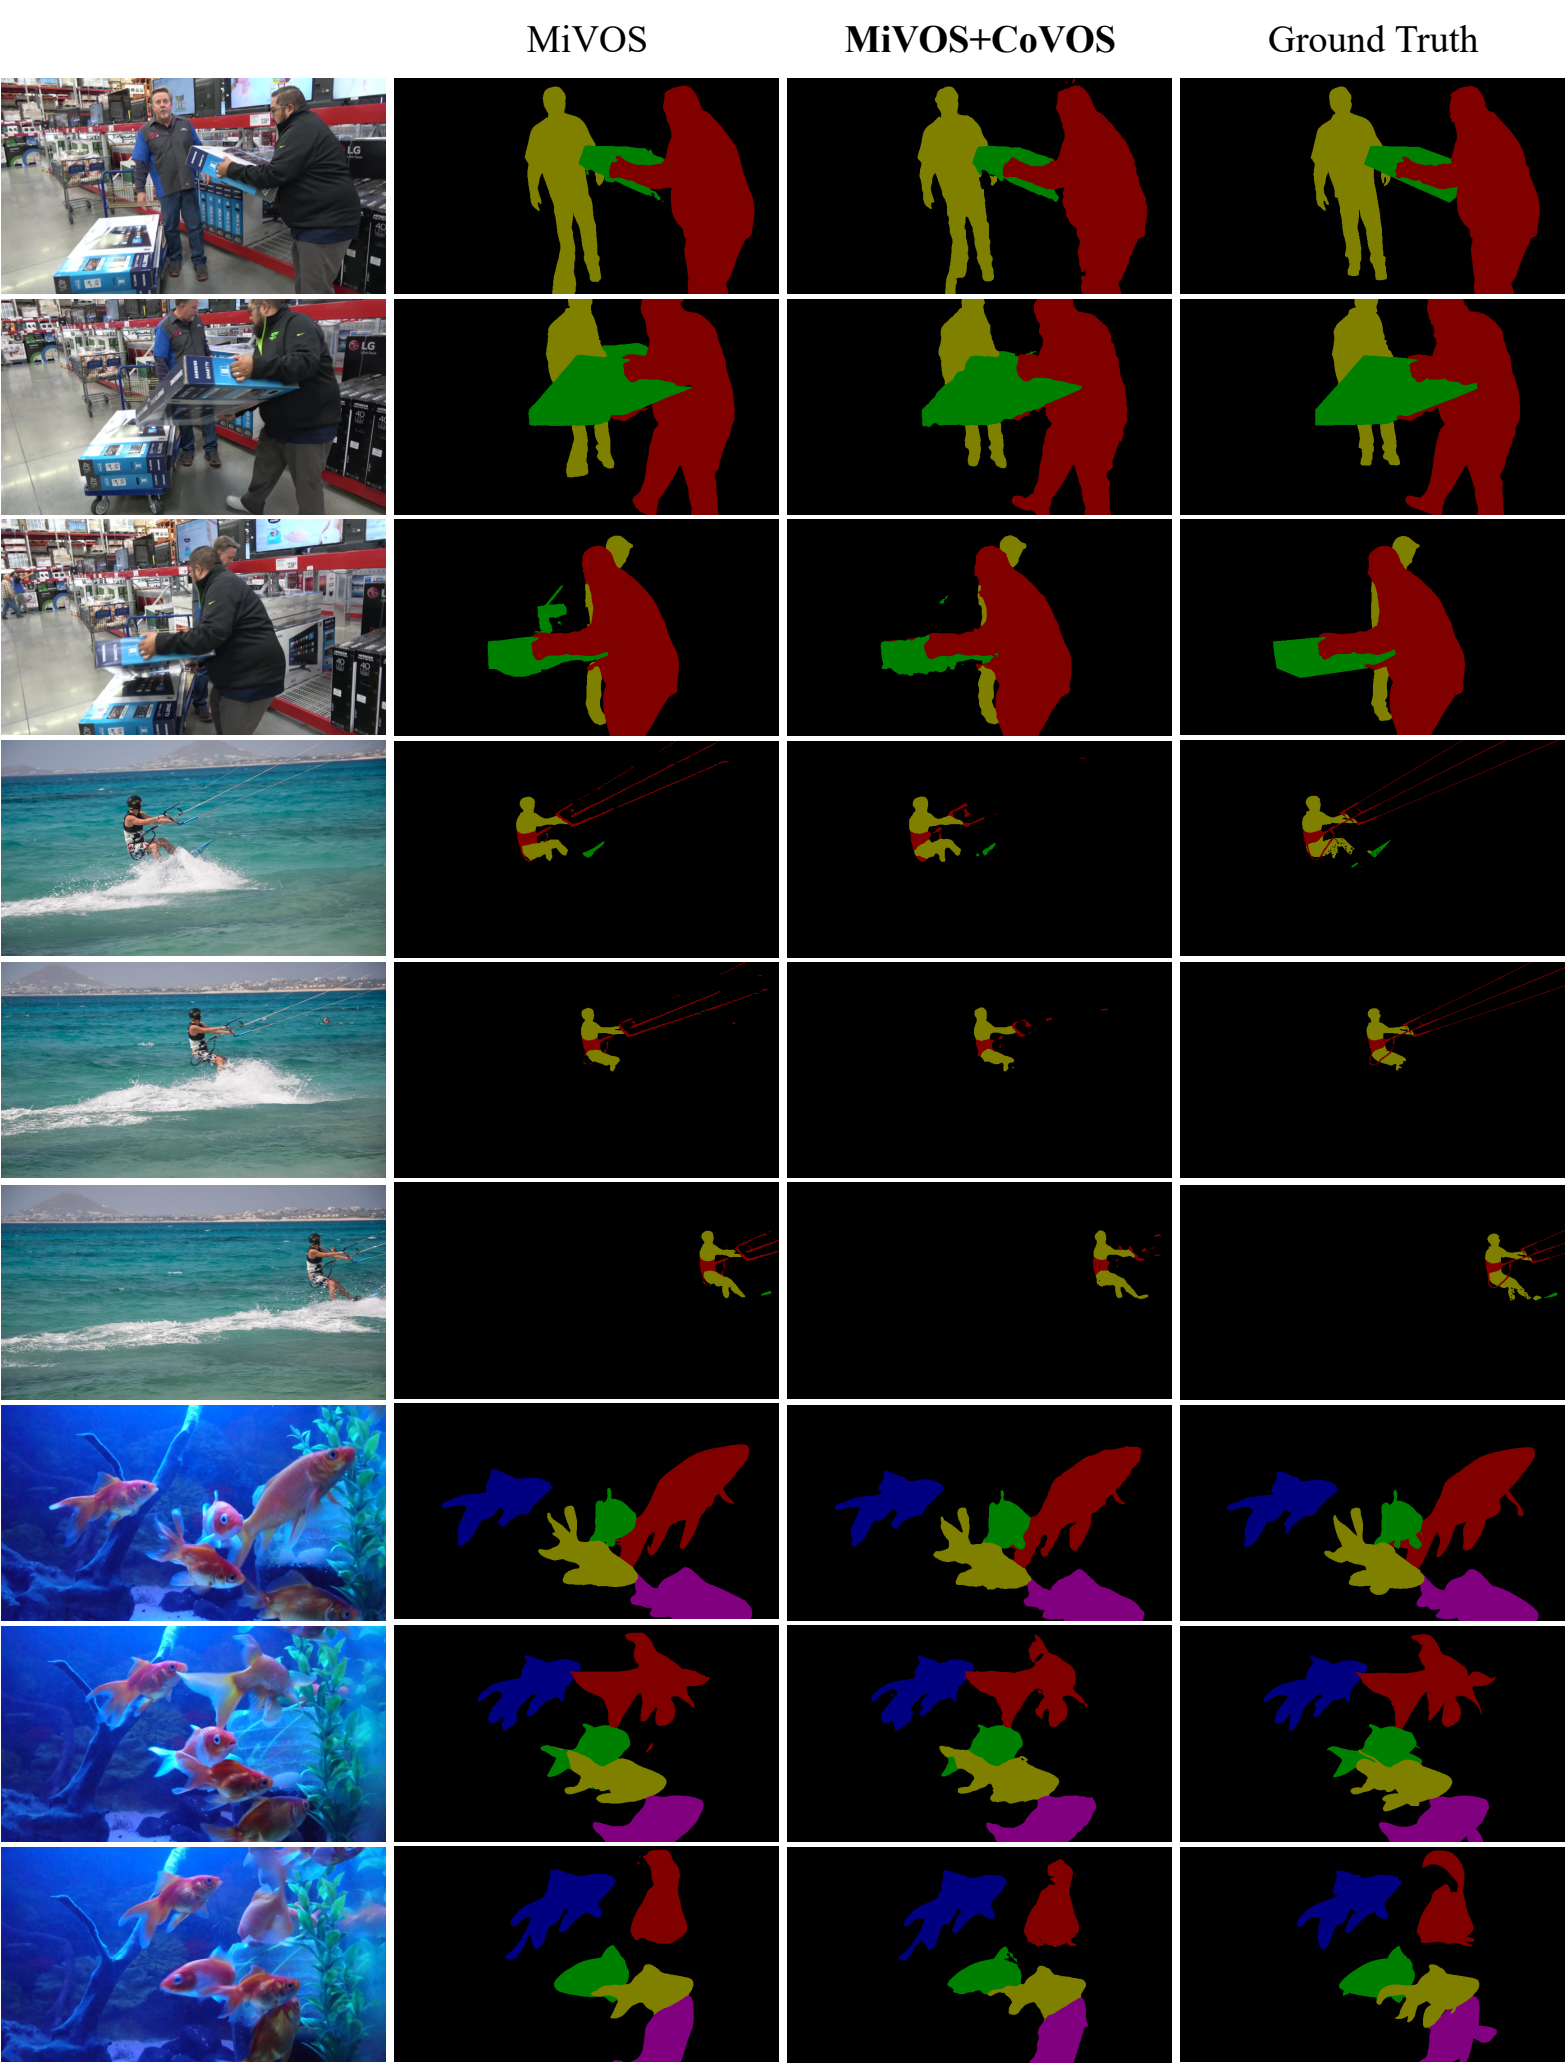   |
| 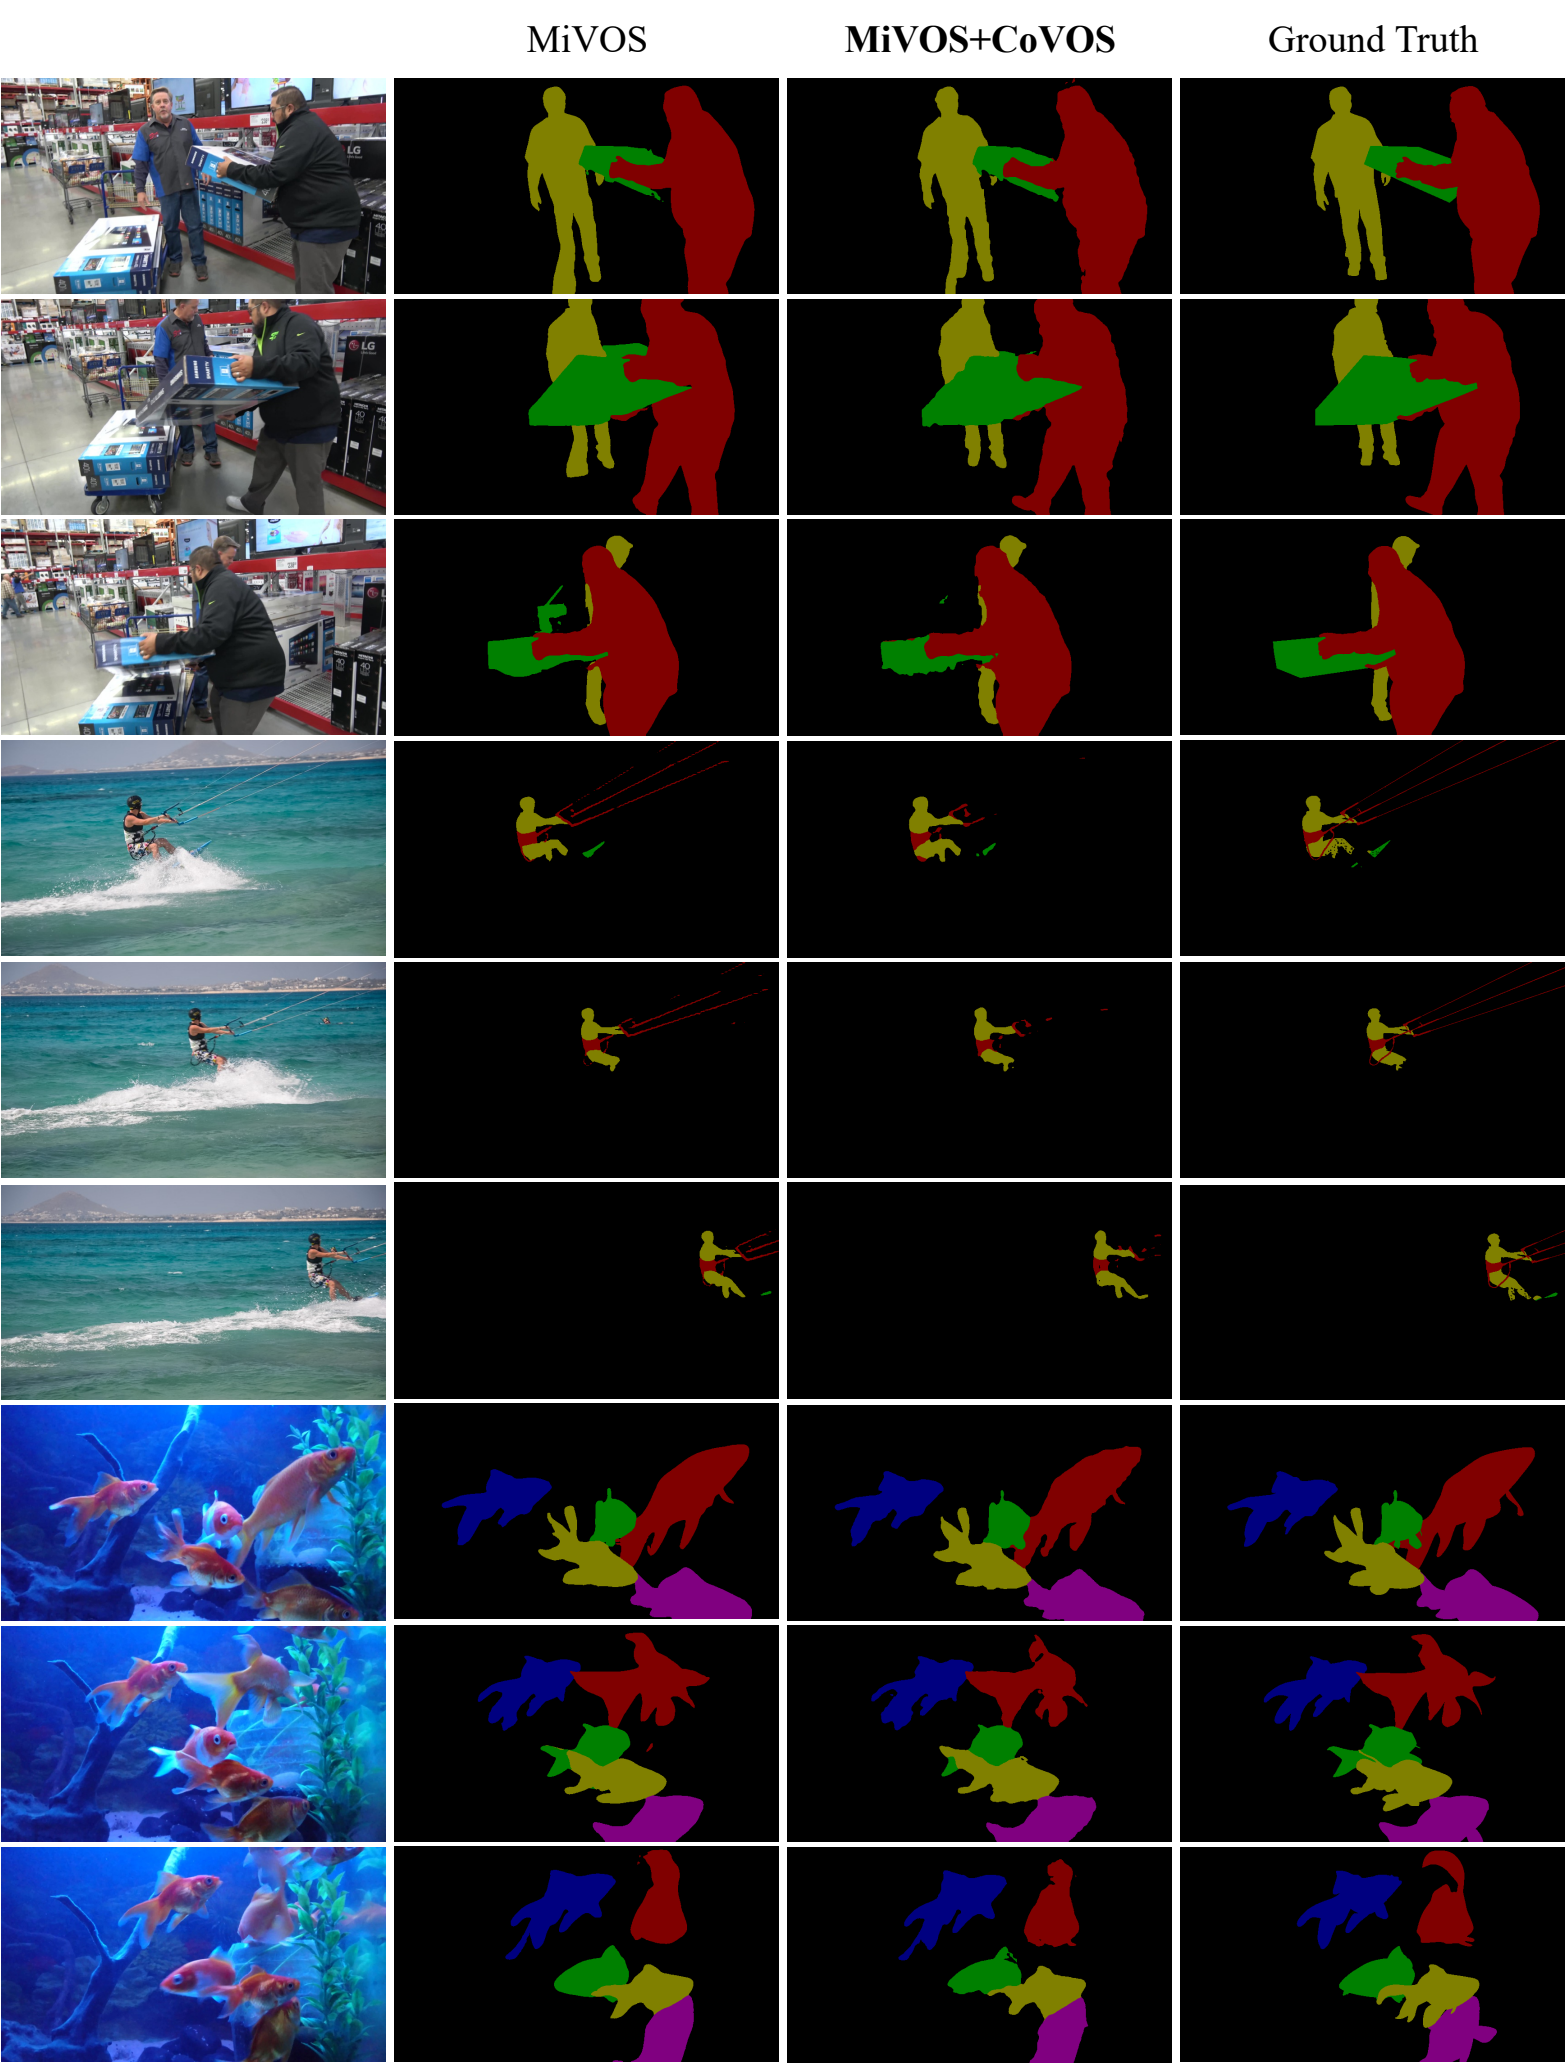  | 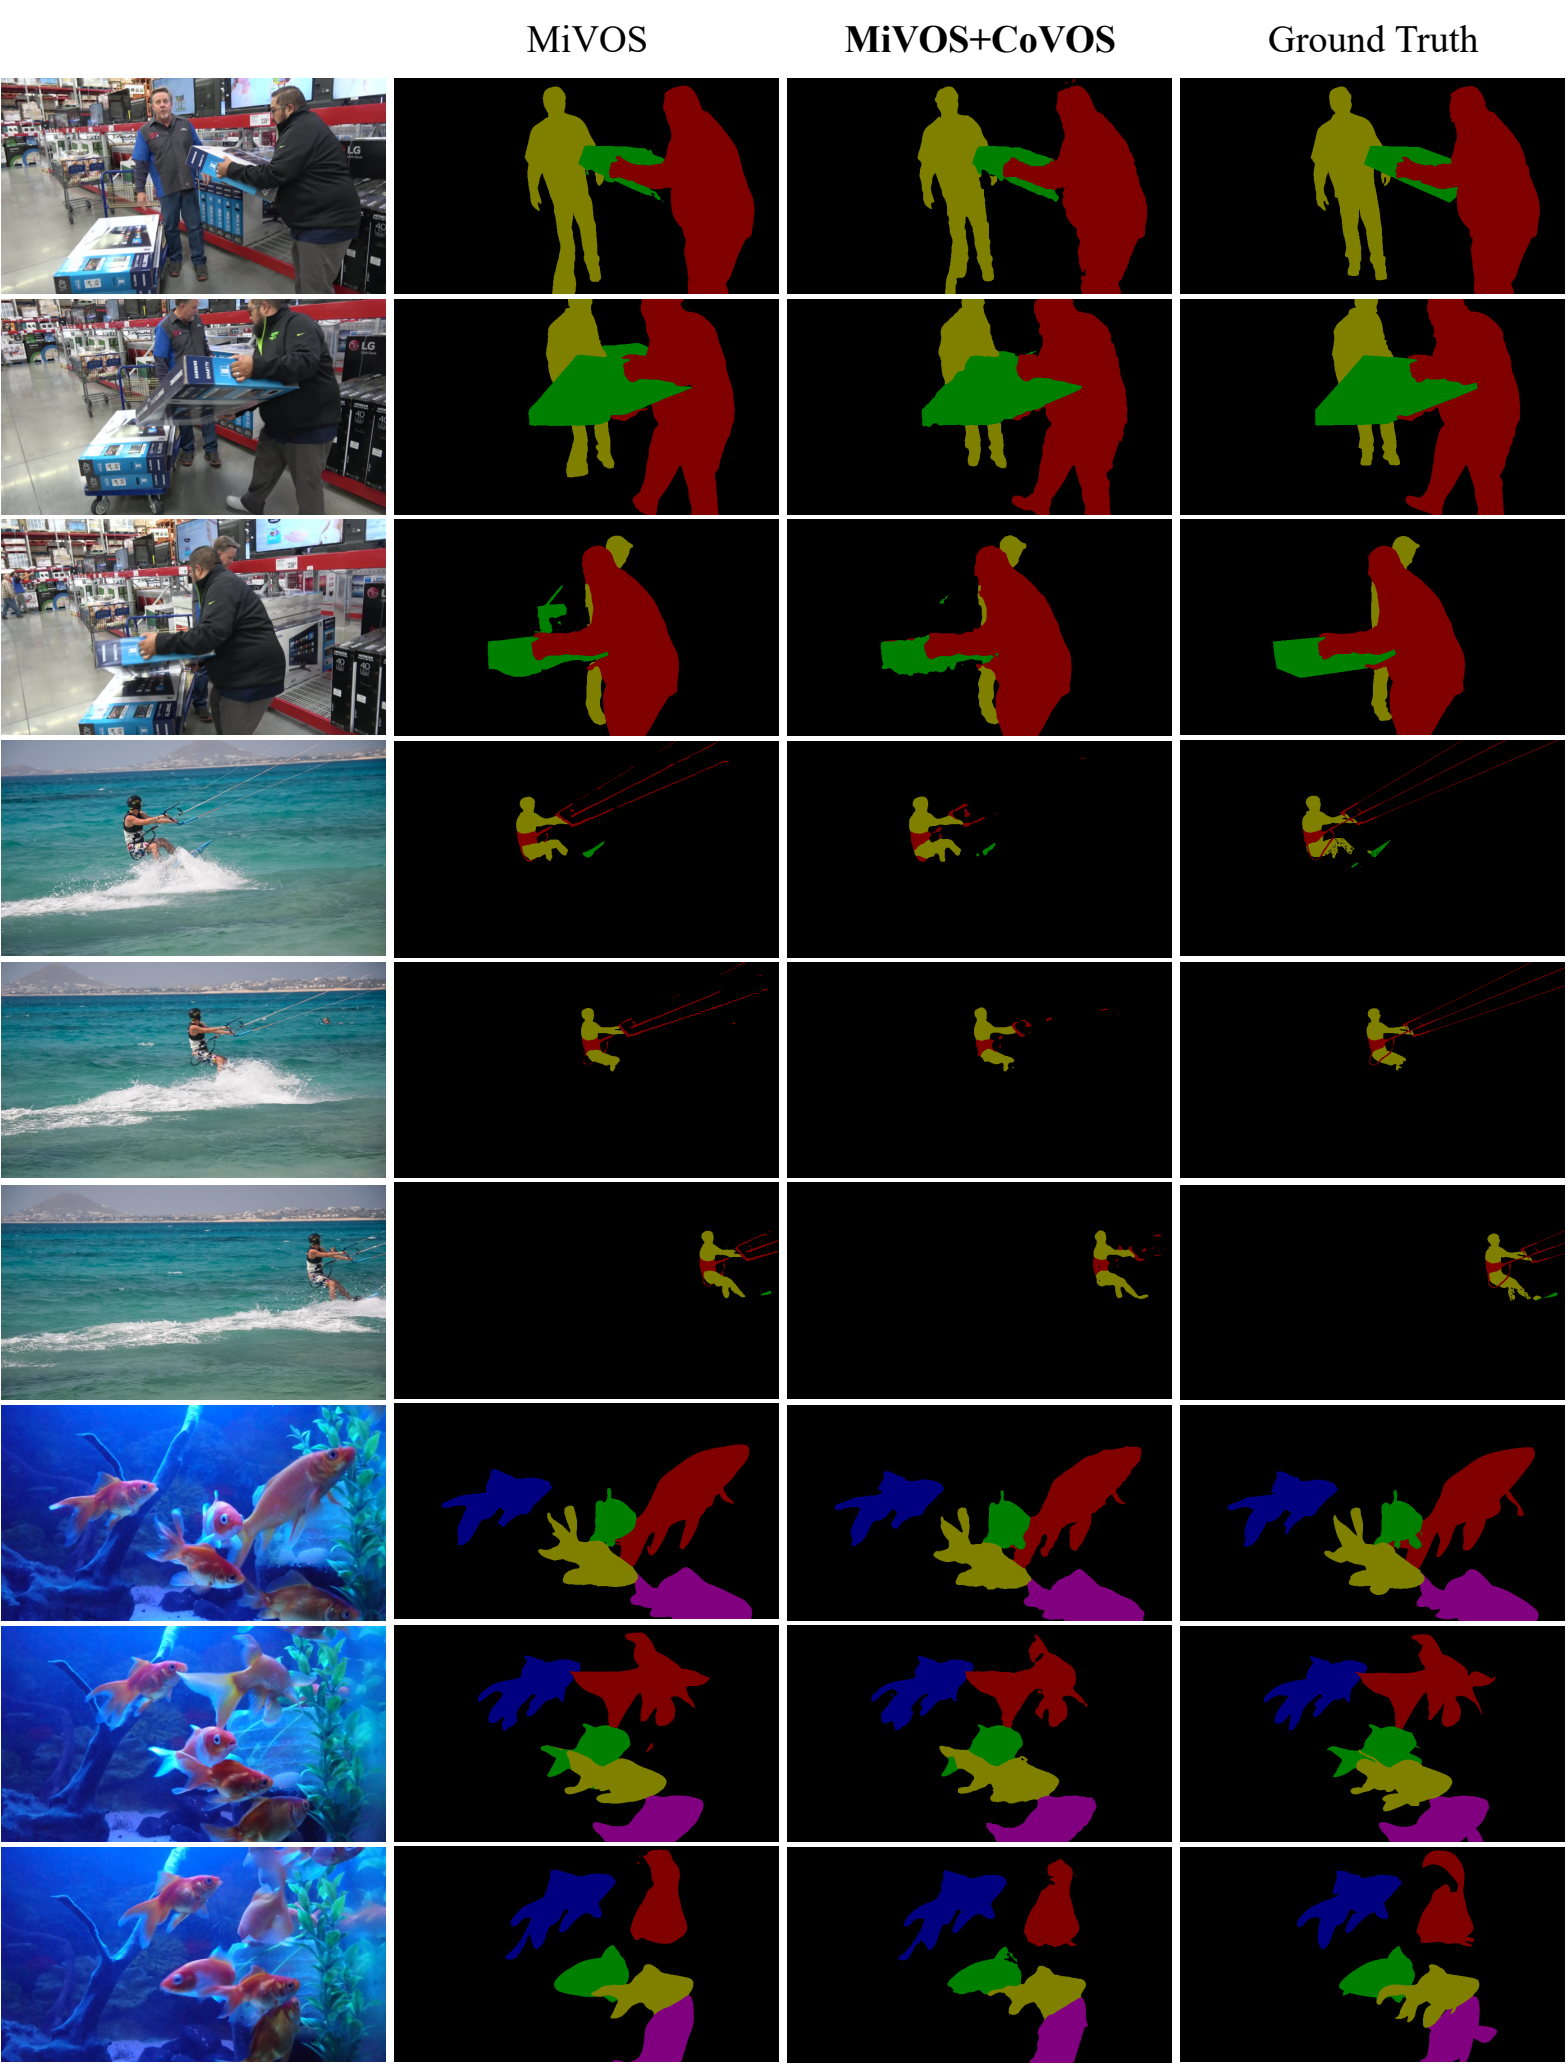  | 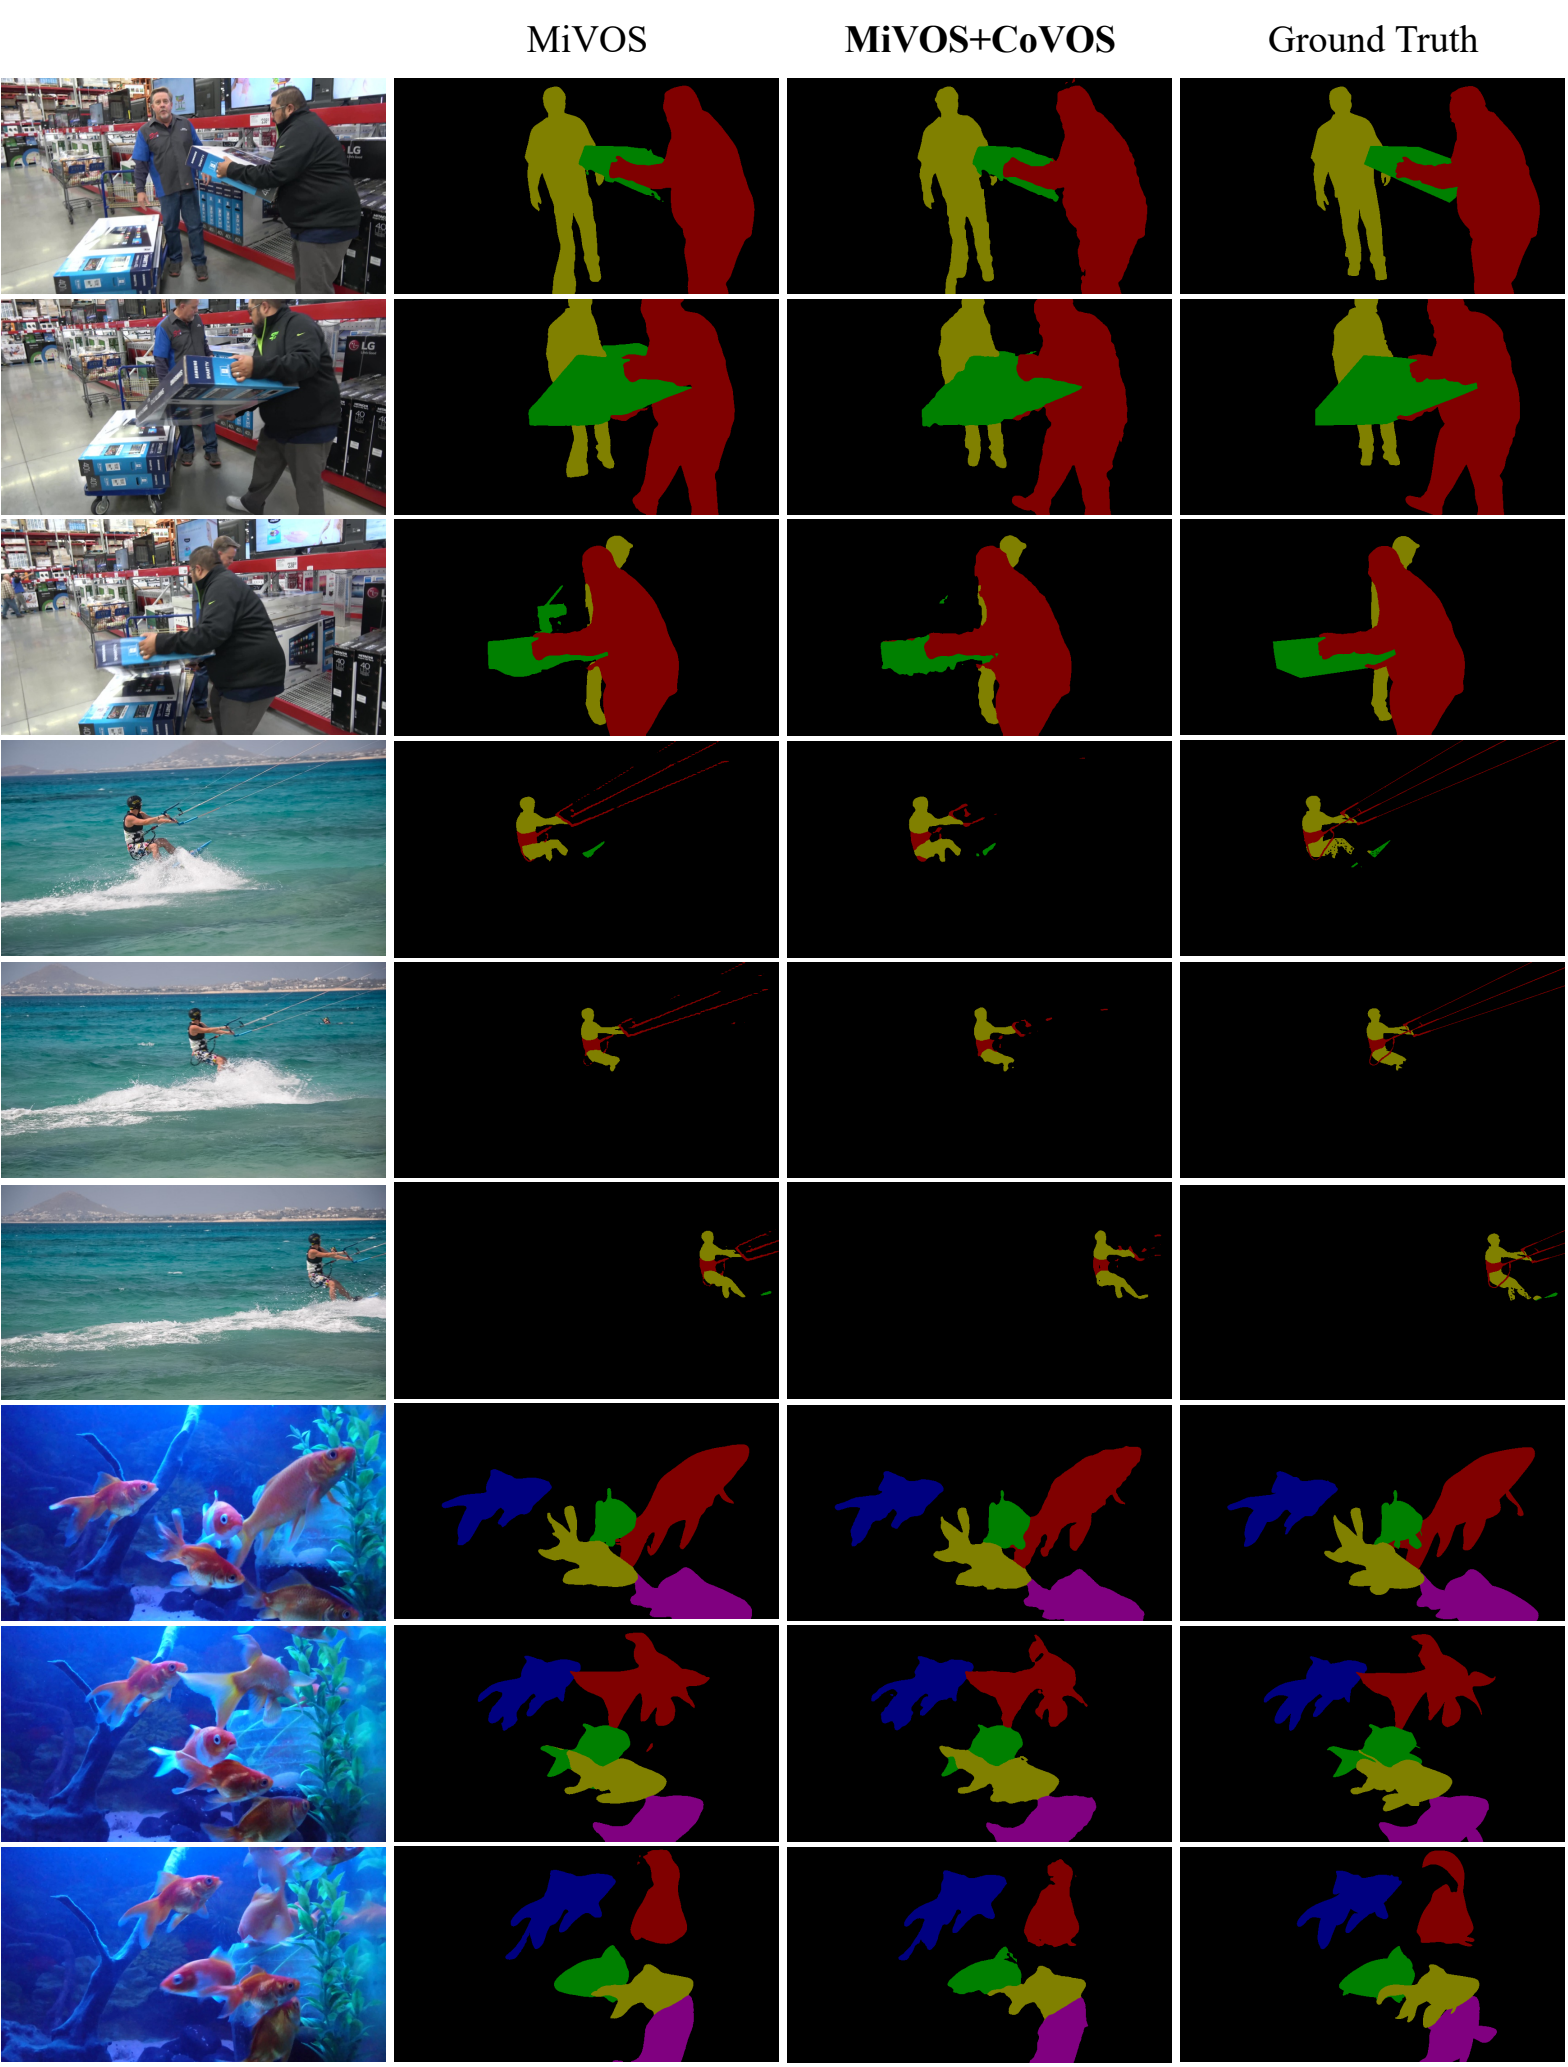  | 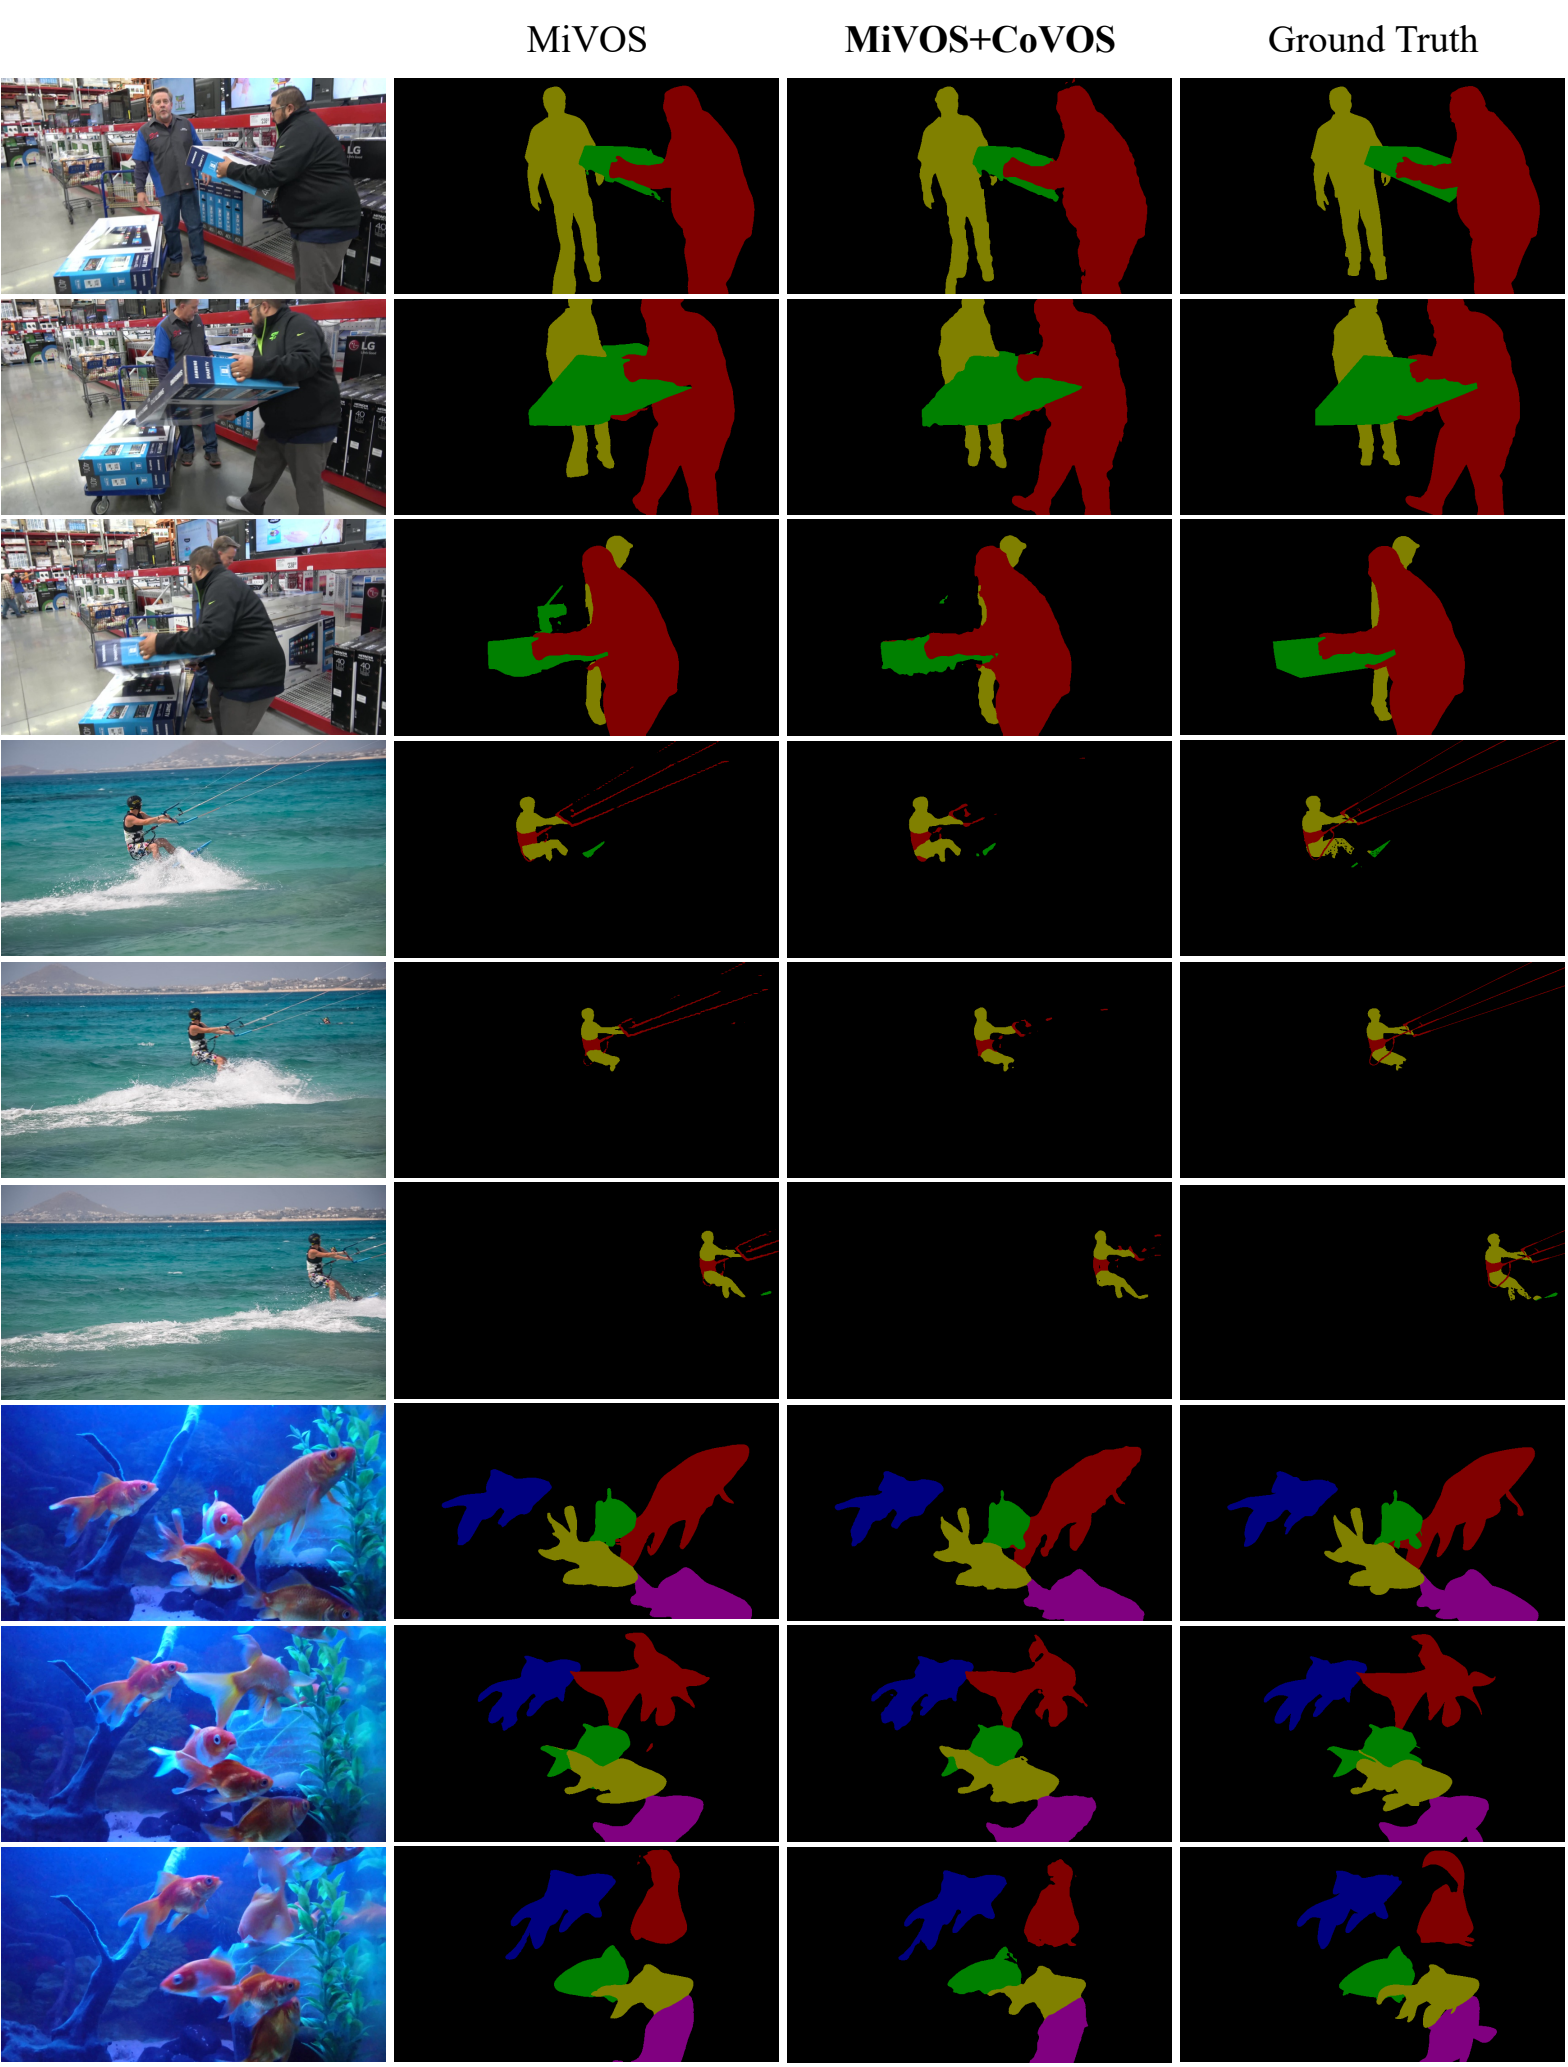  |
| 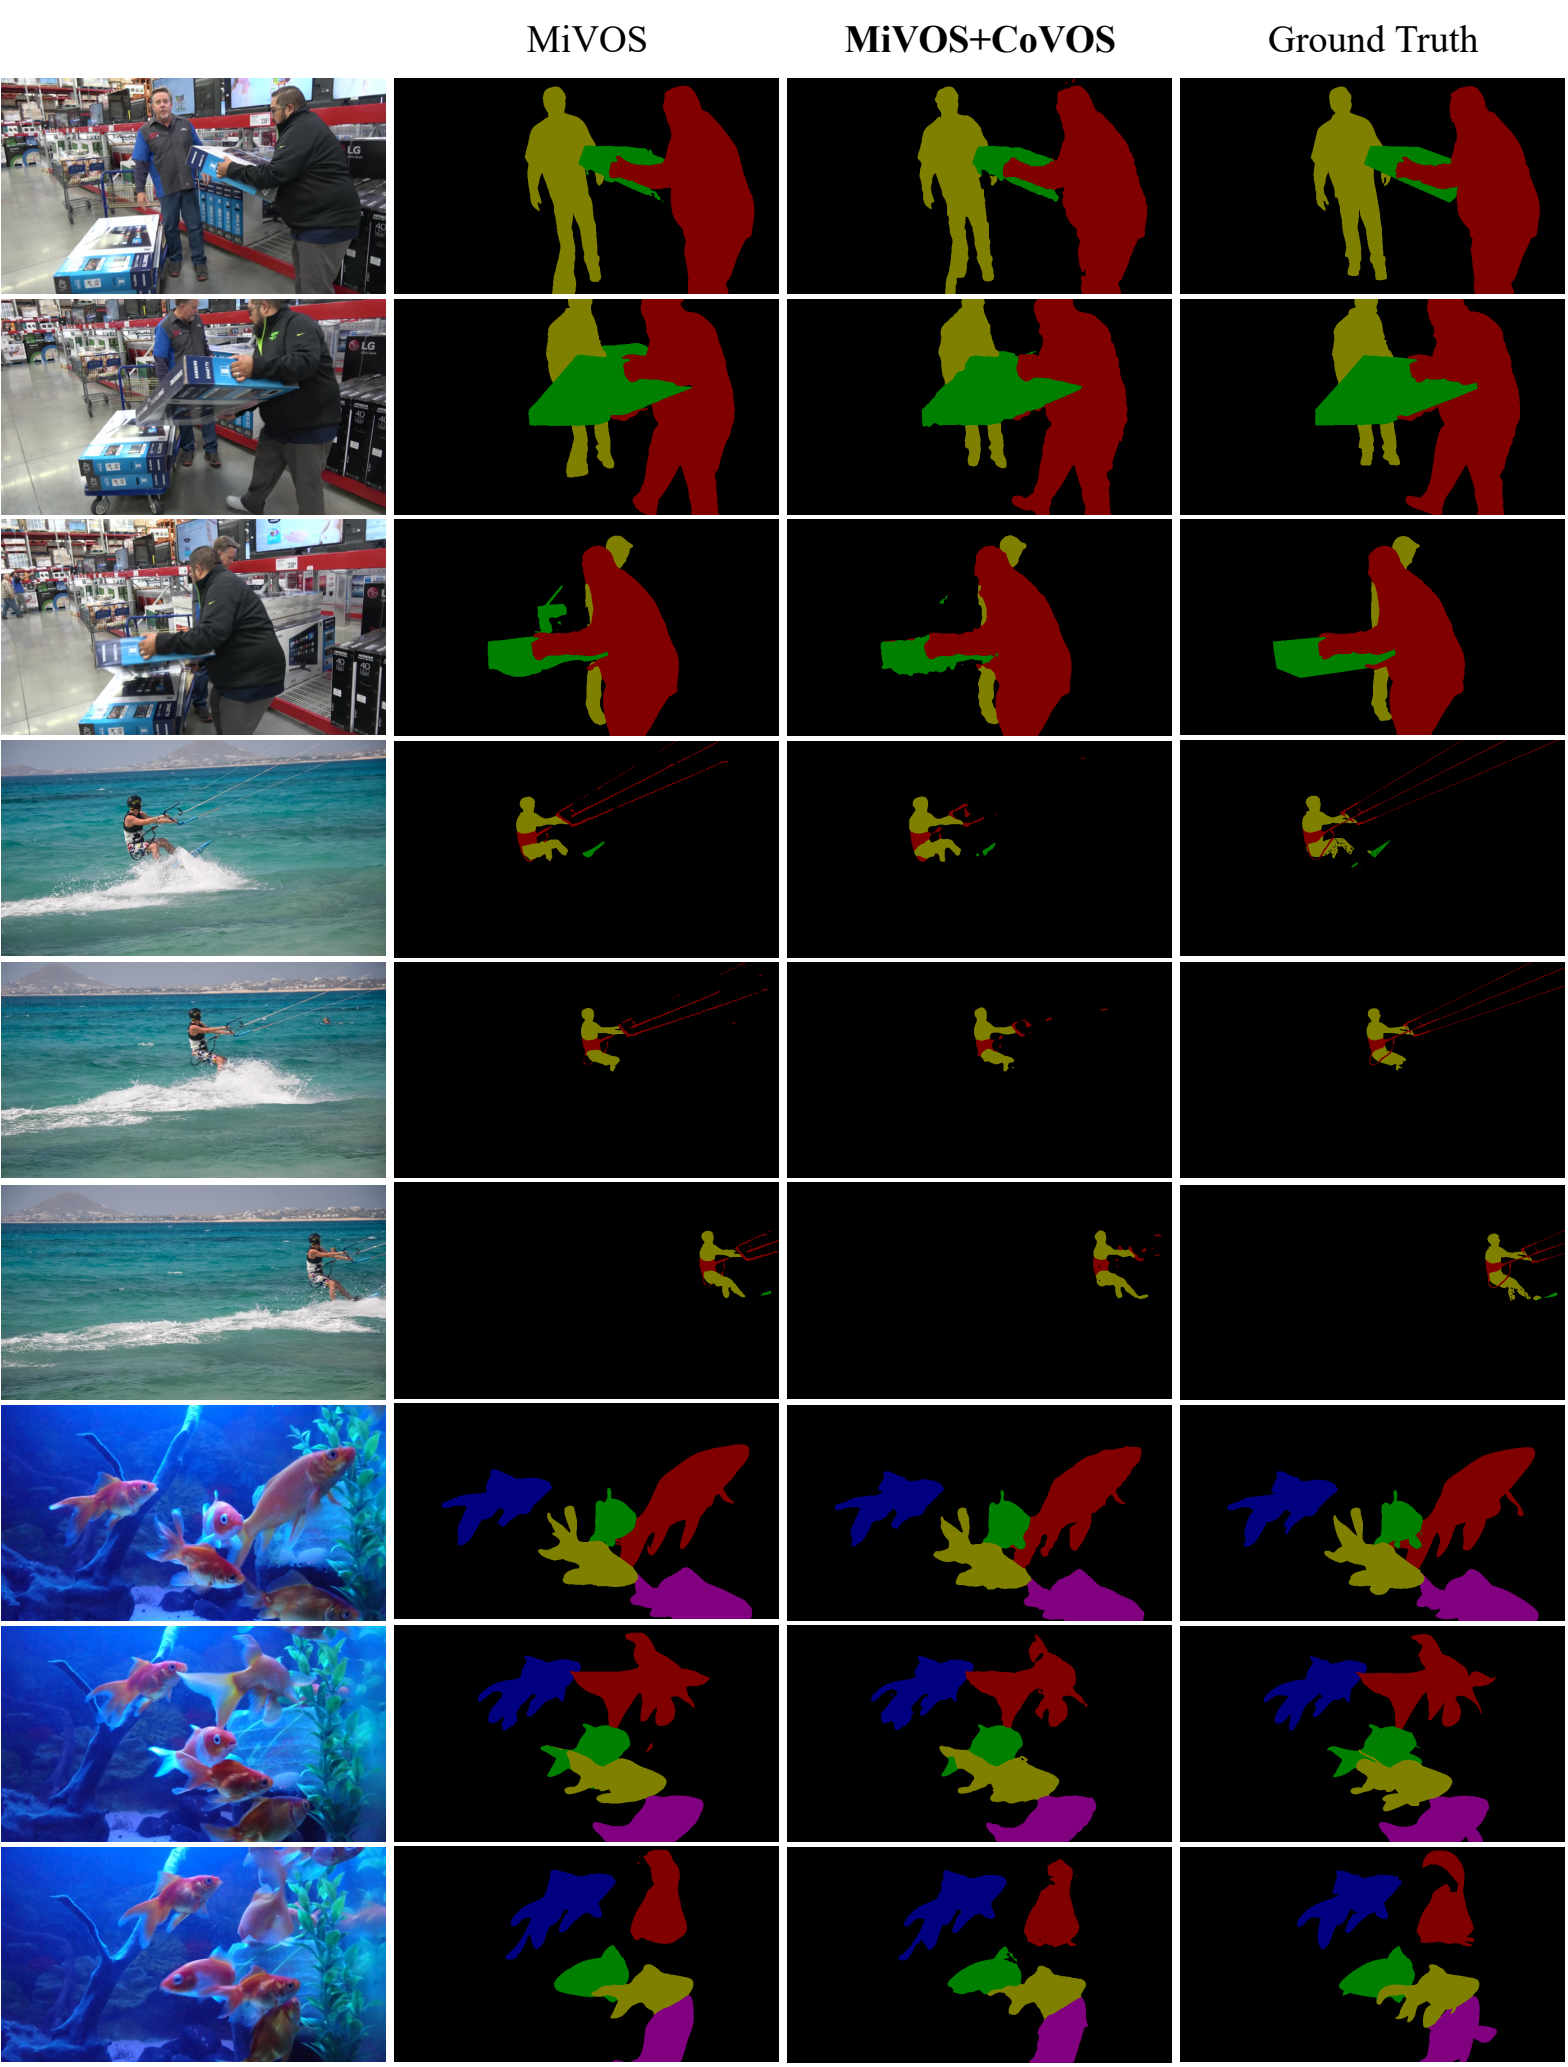 | 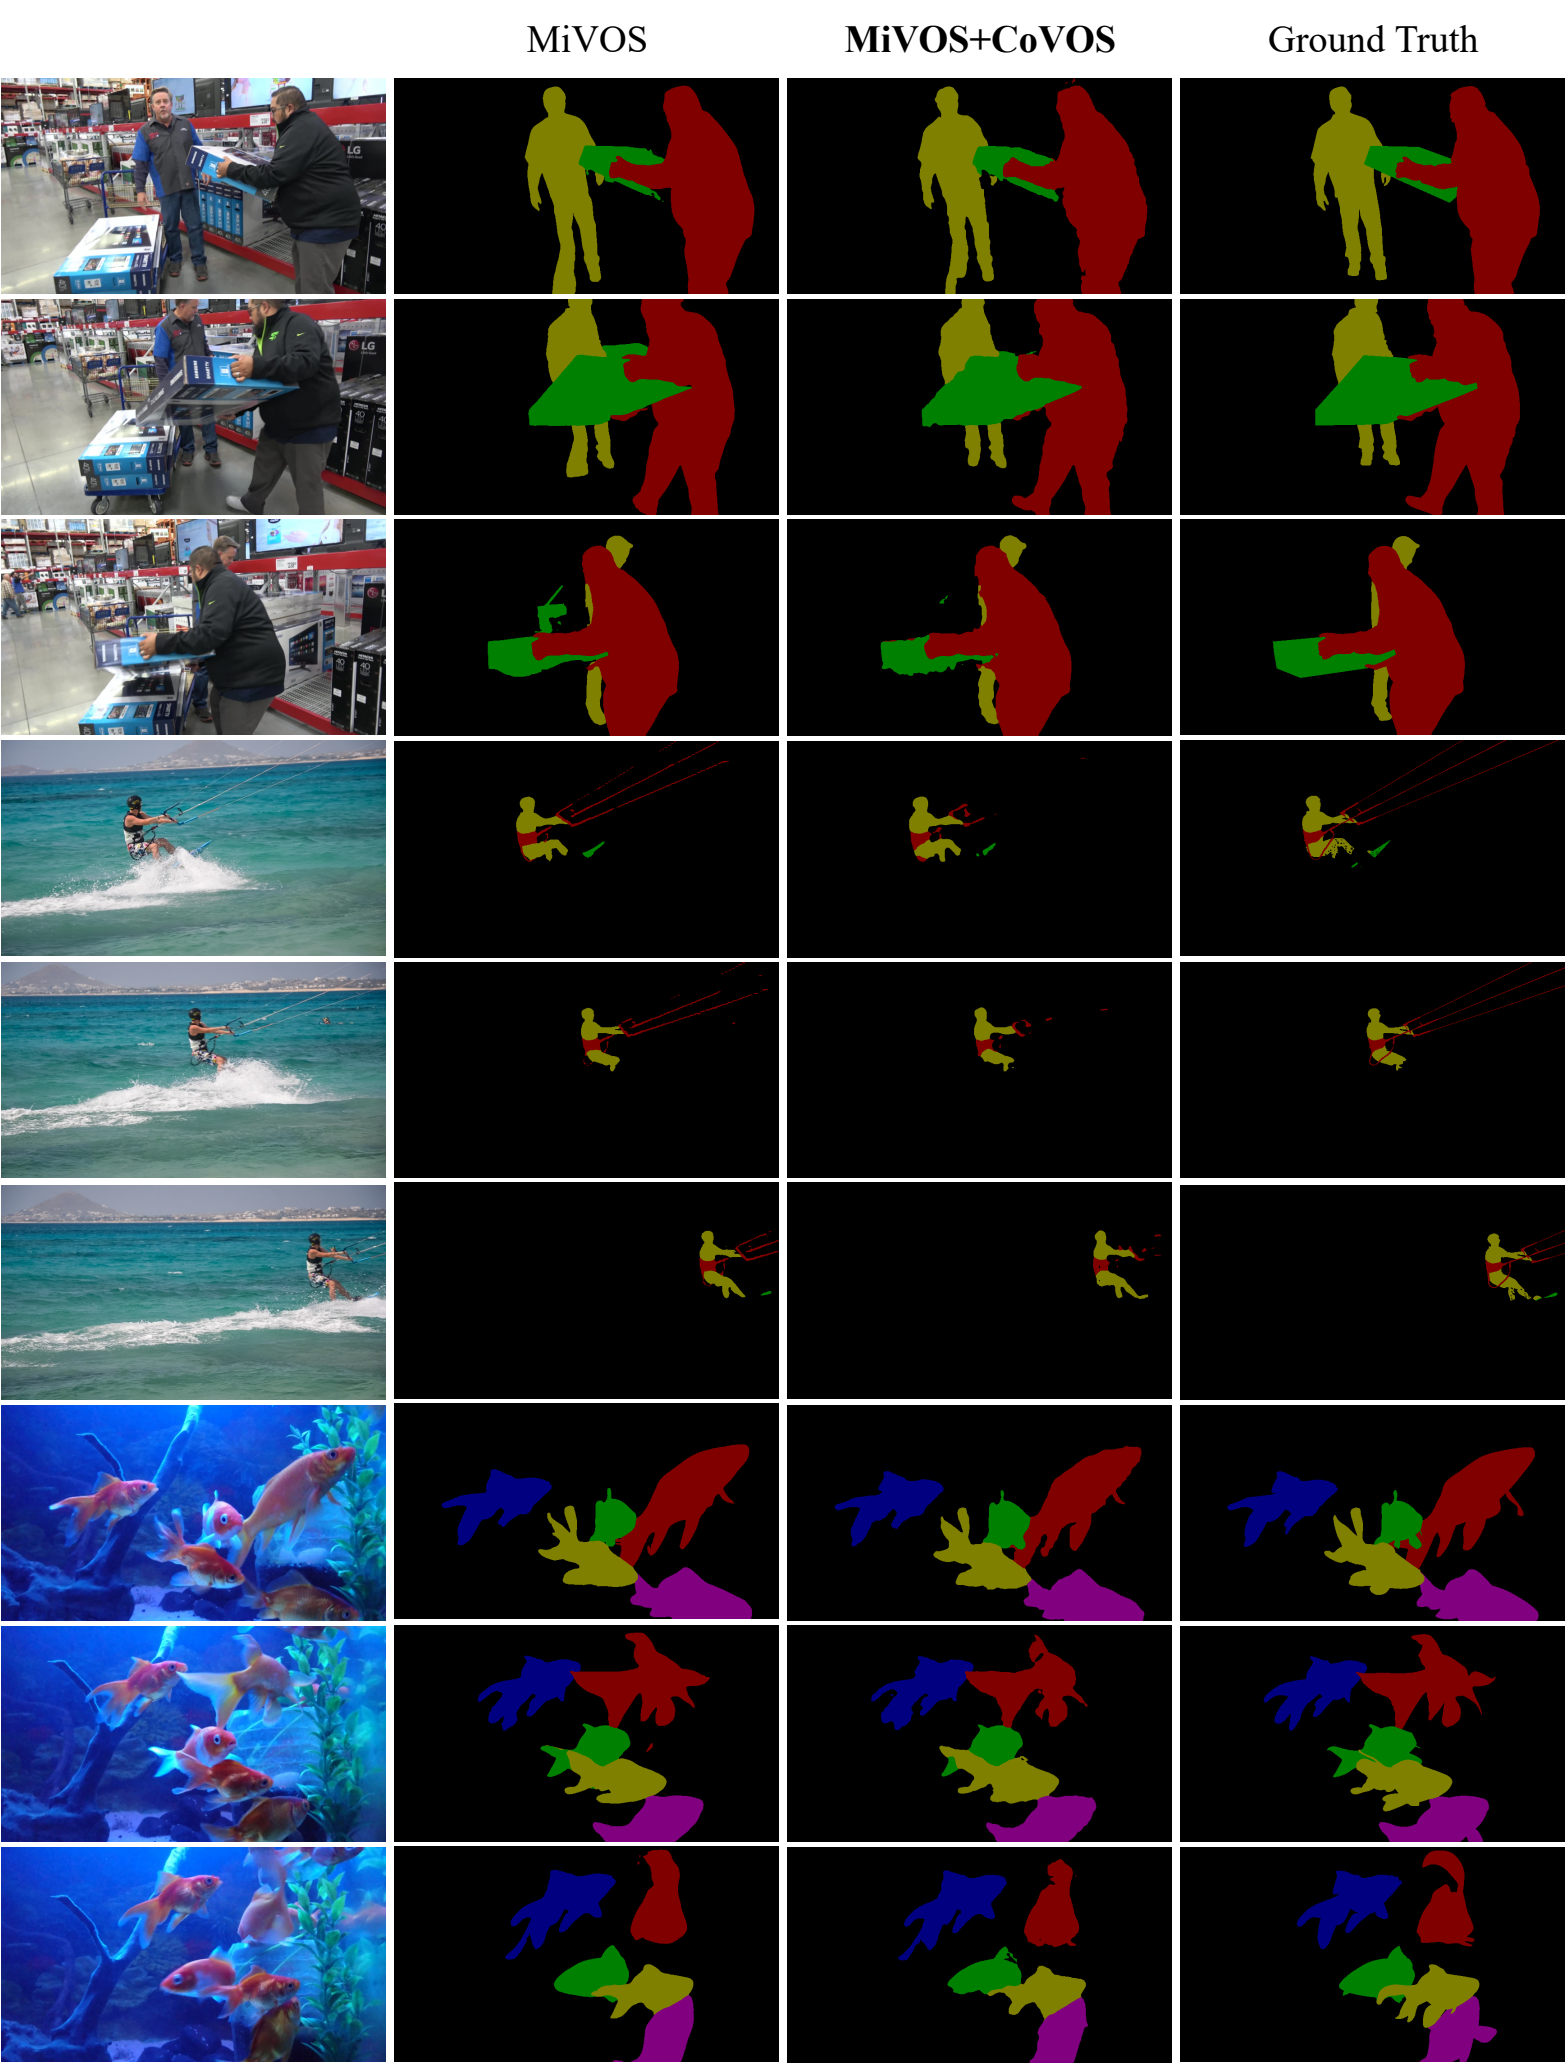 | 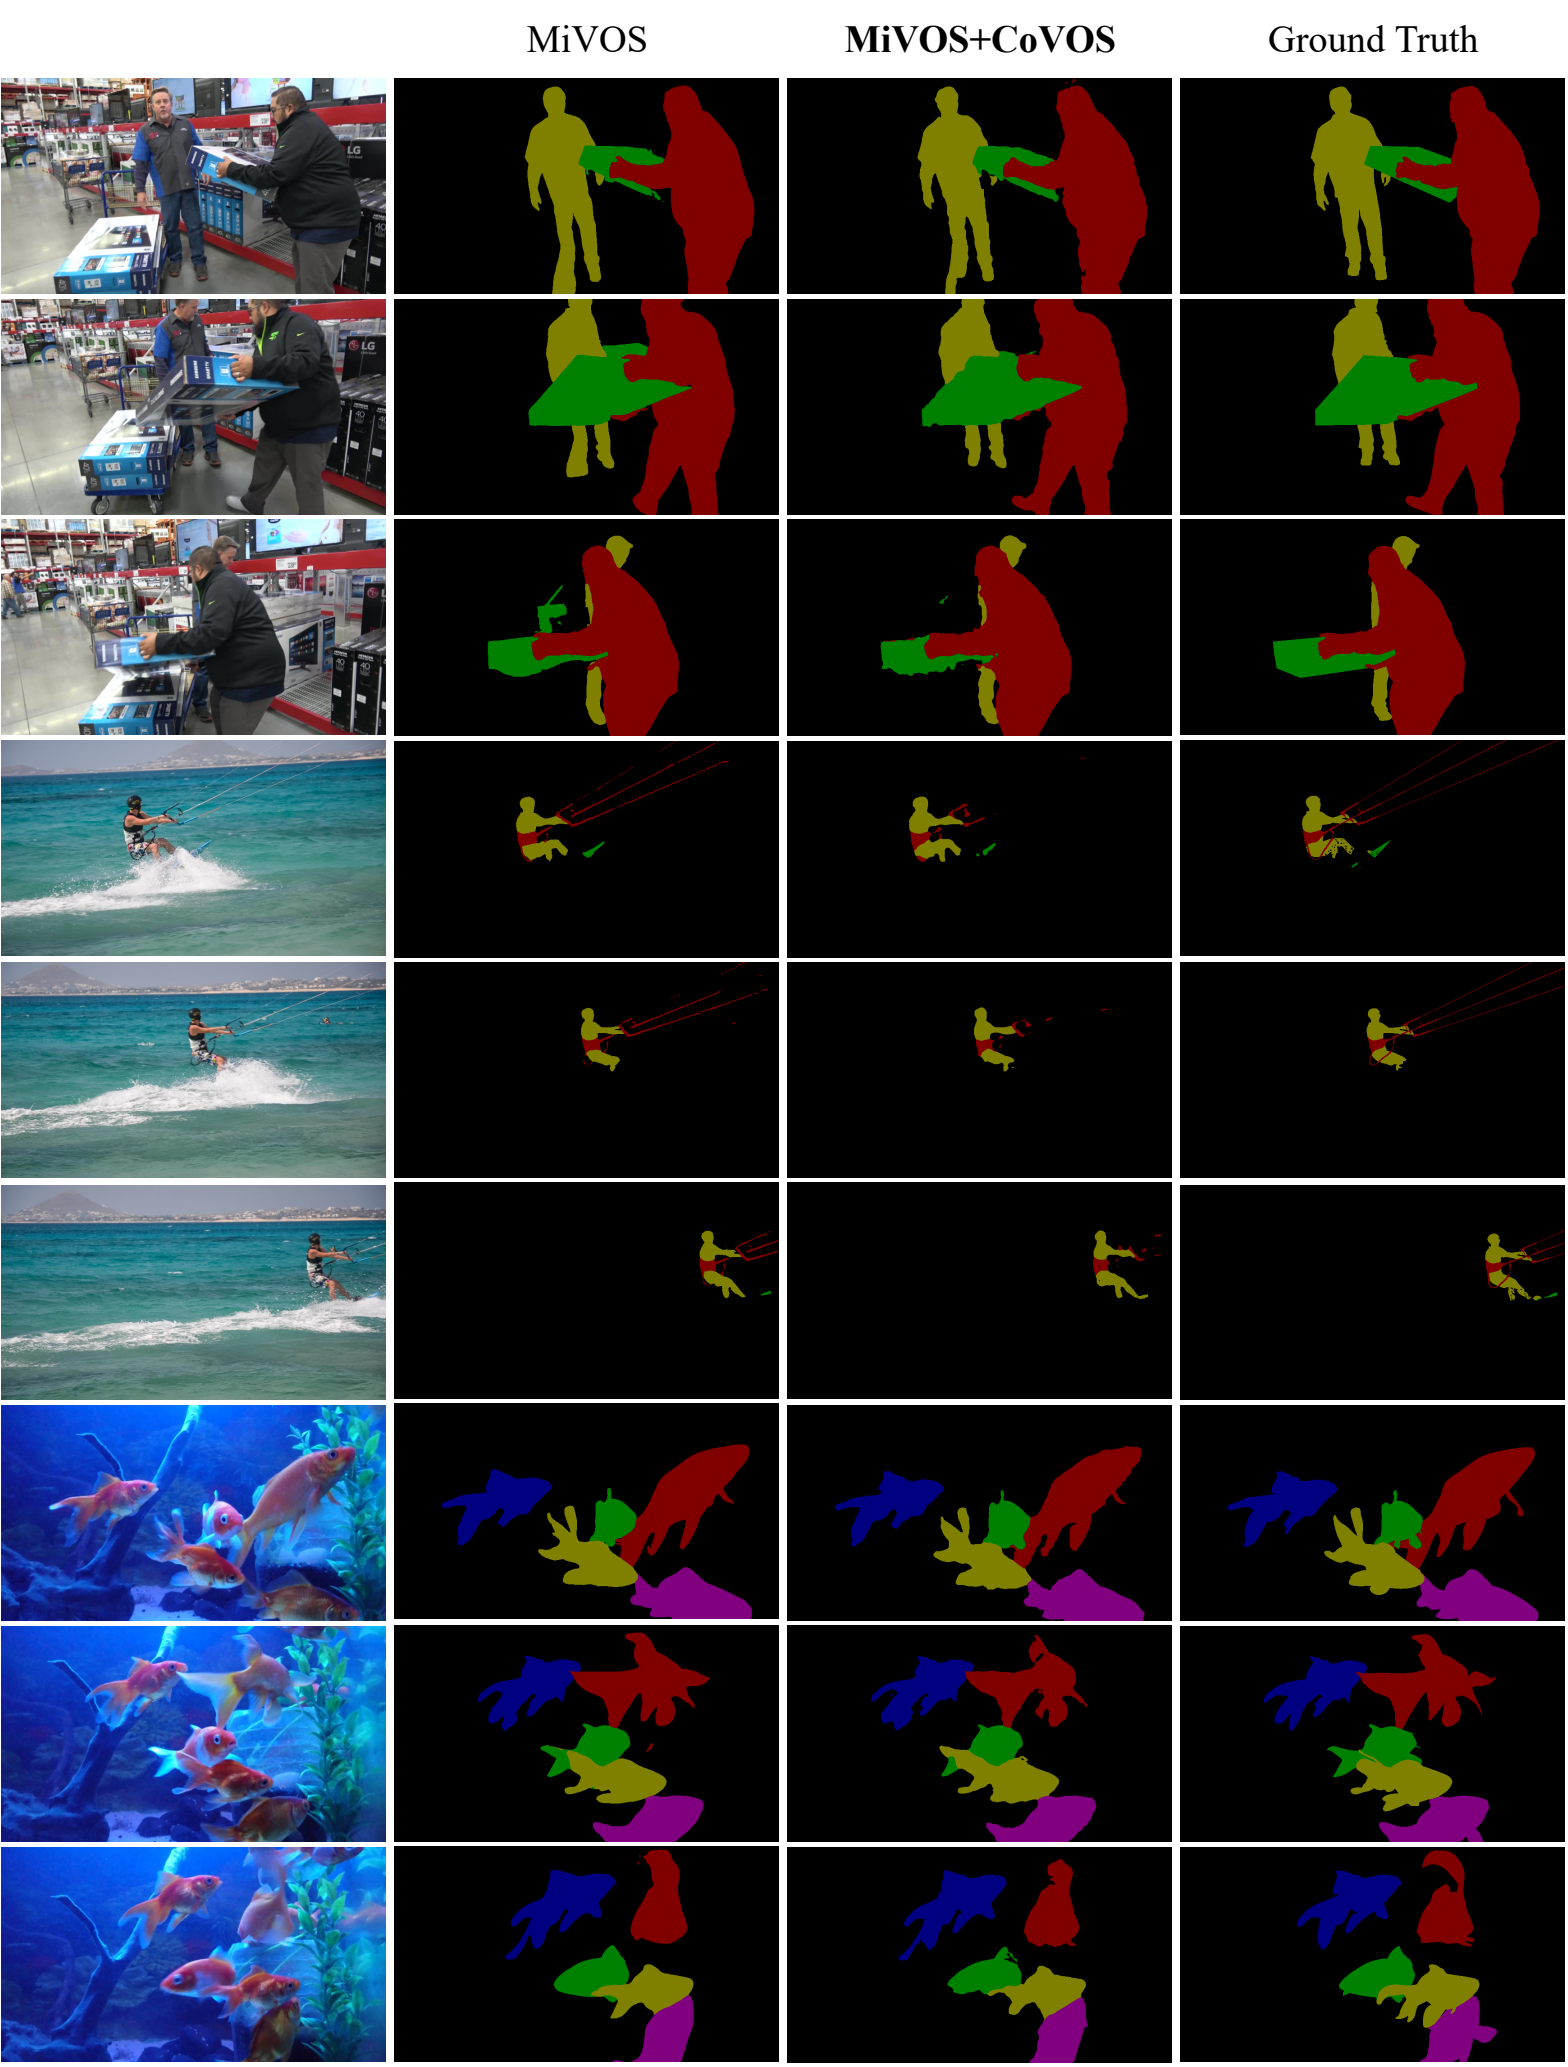 | 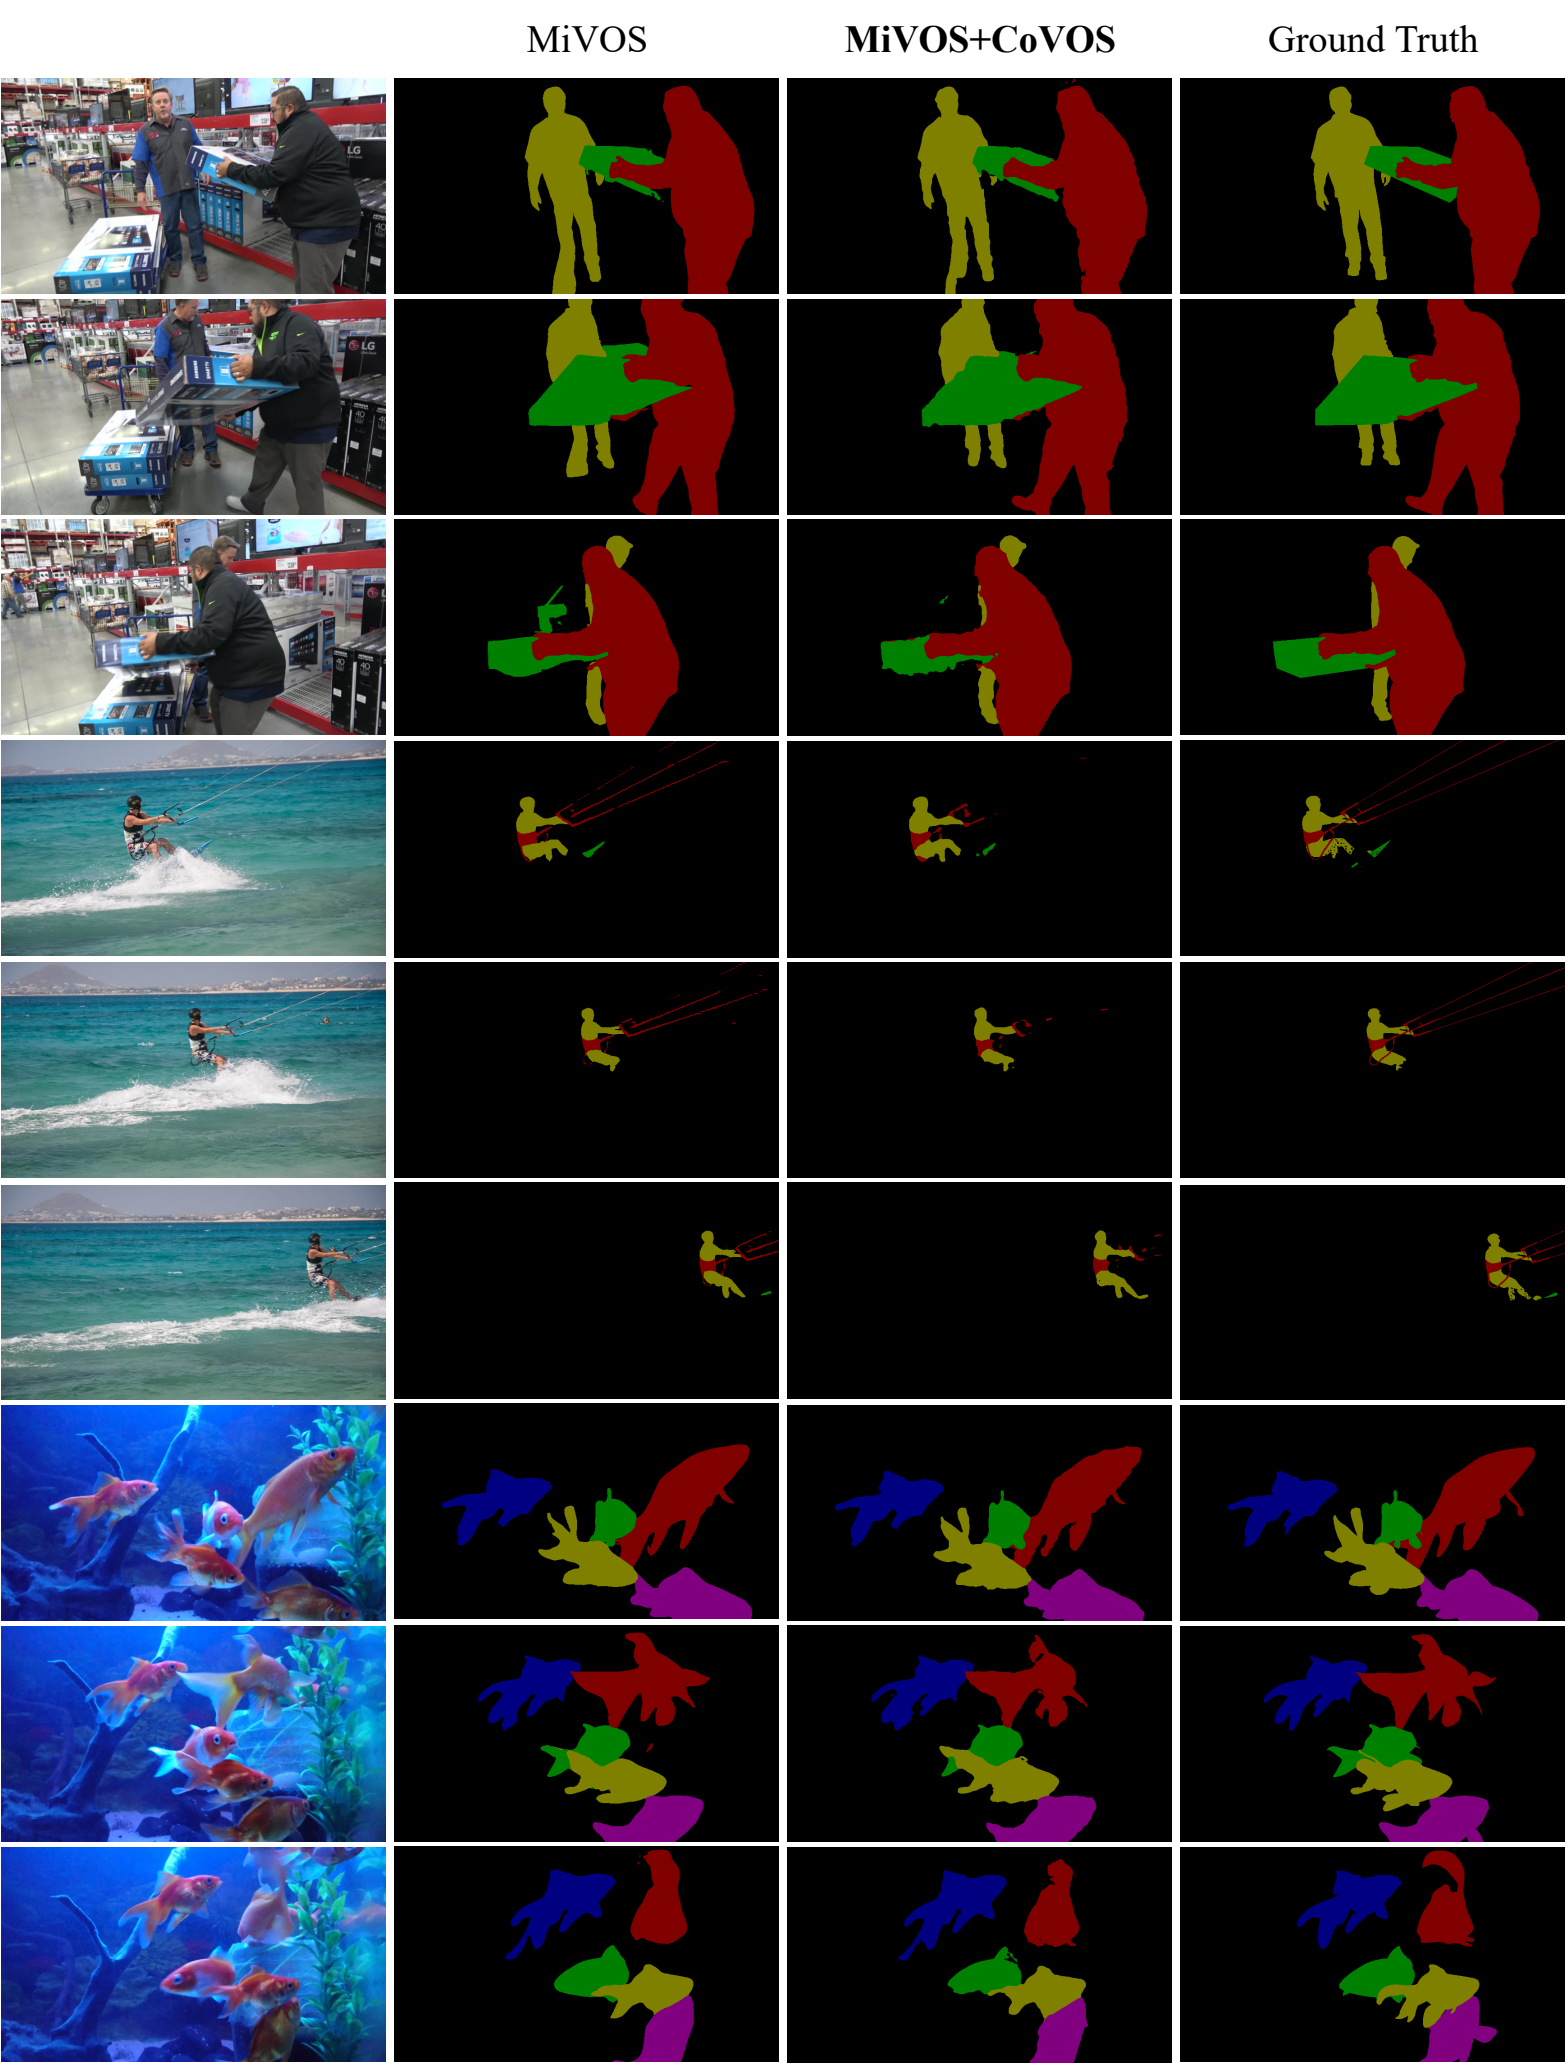 |
| 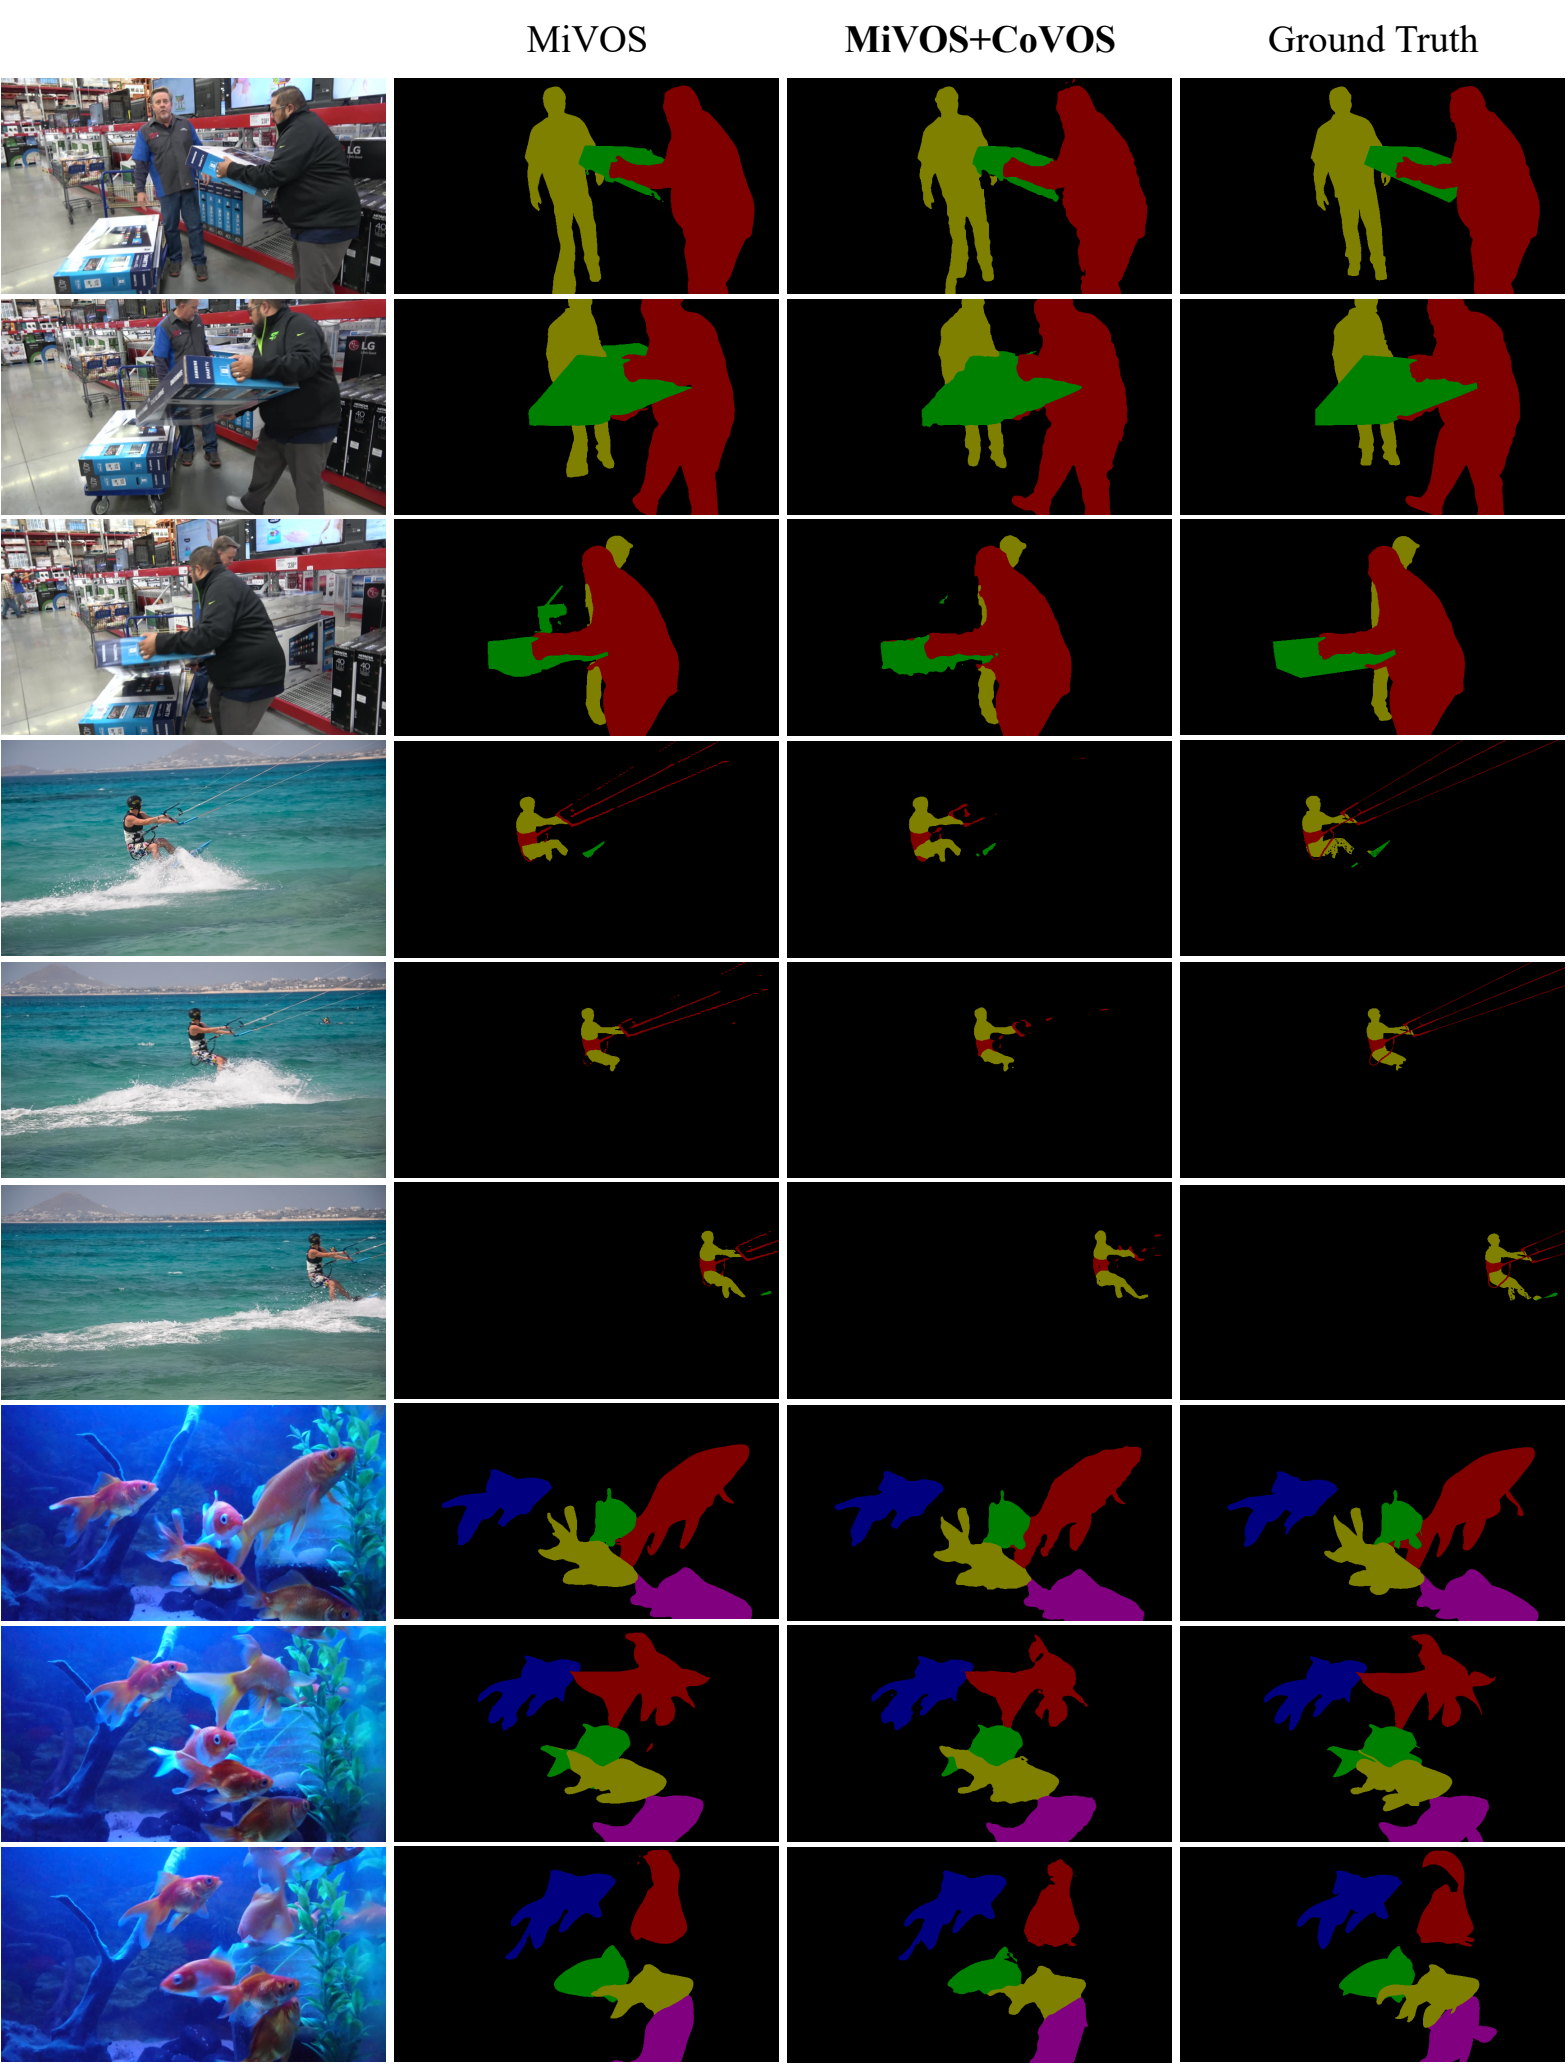 | 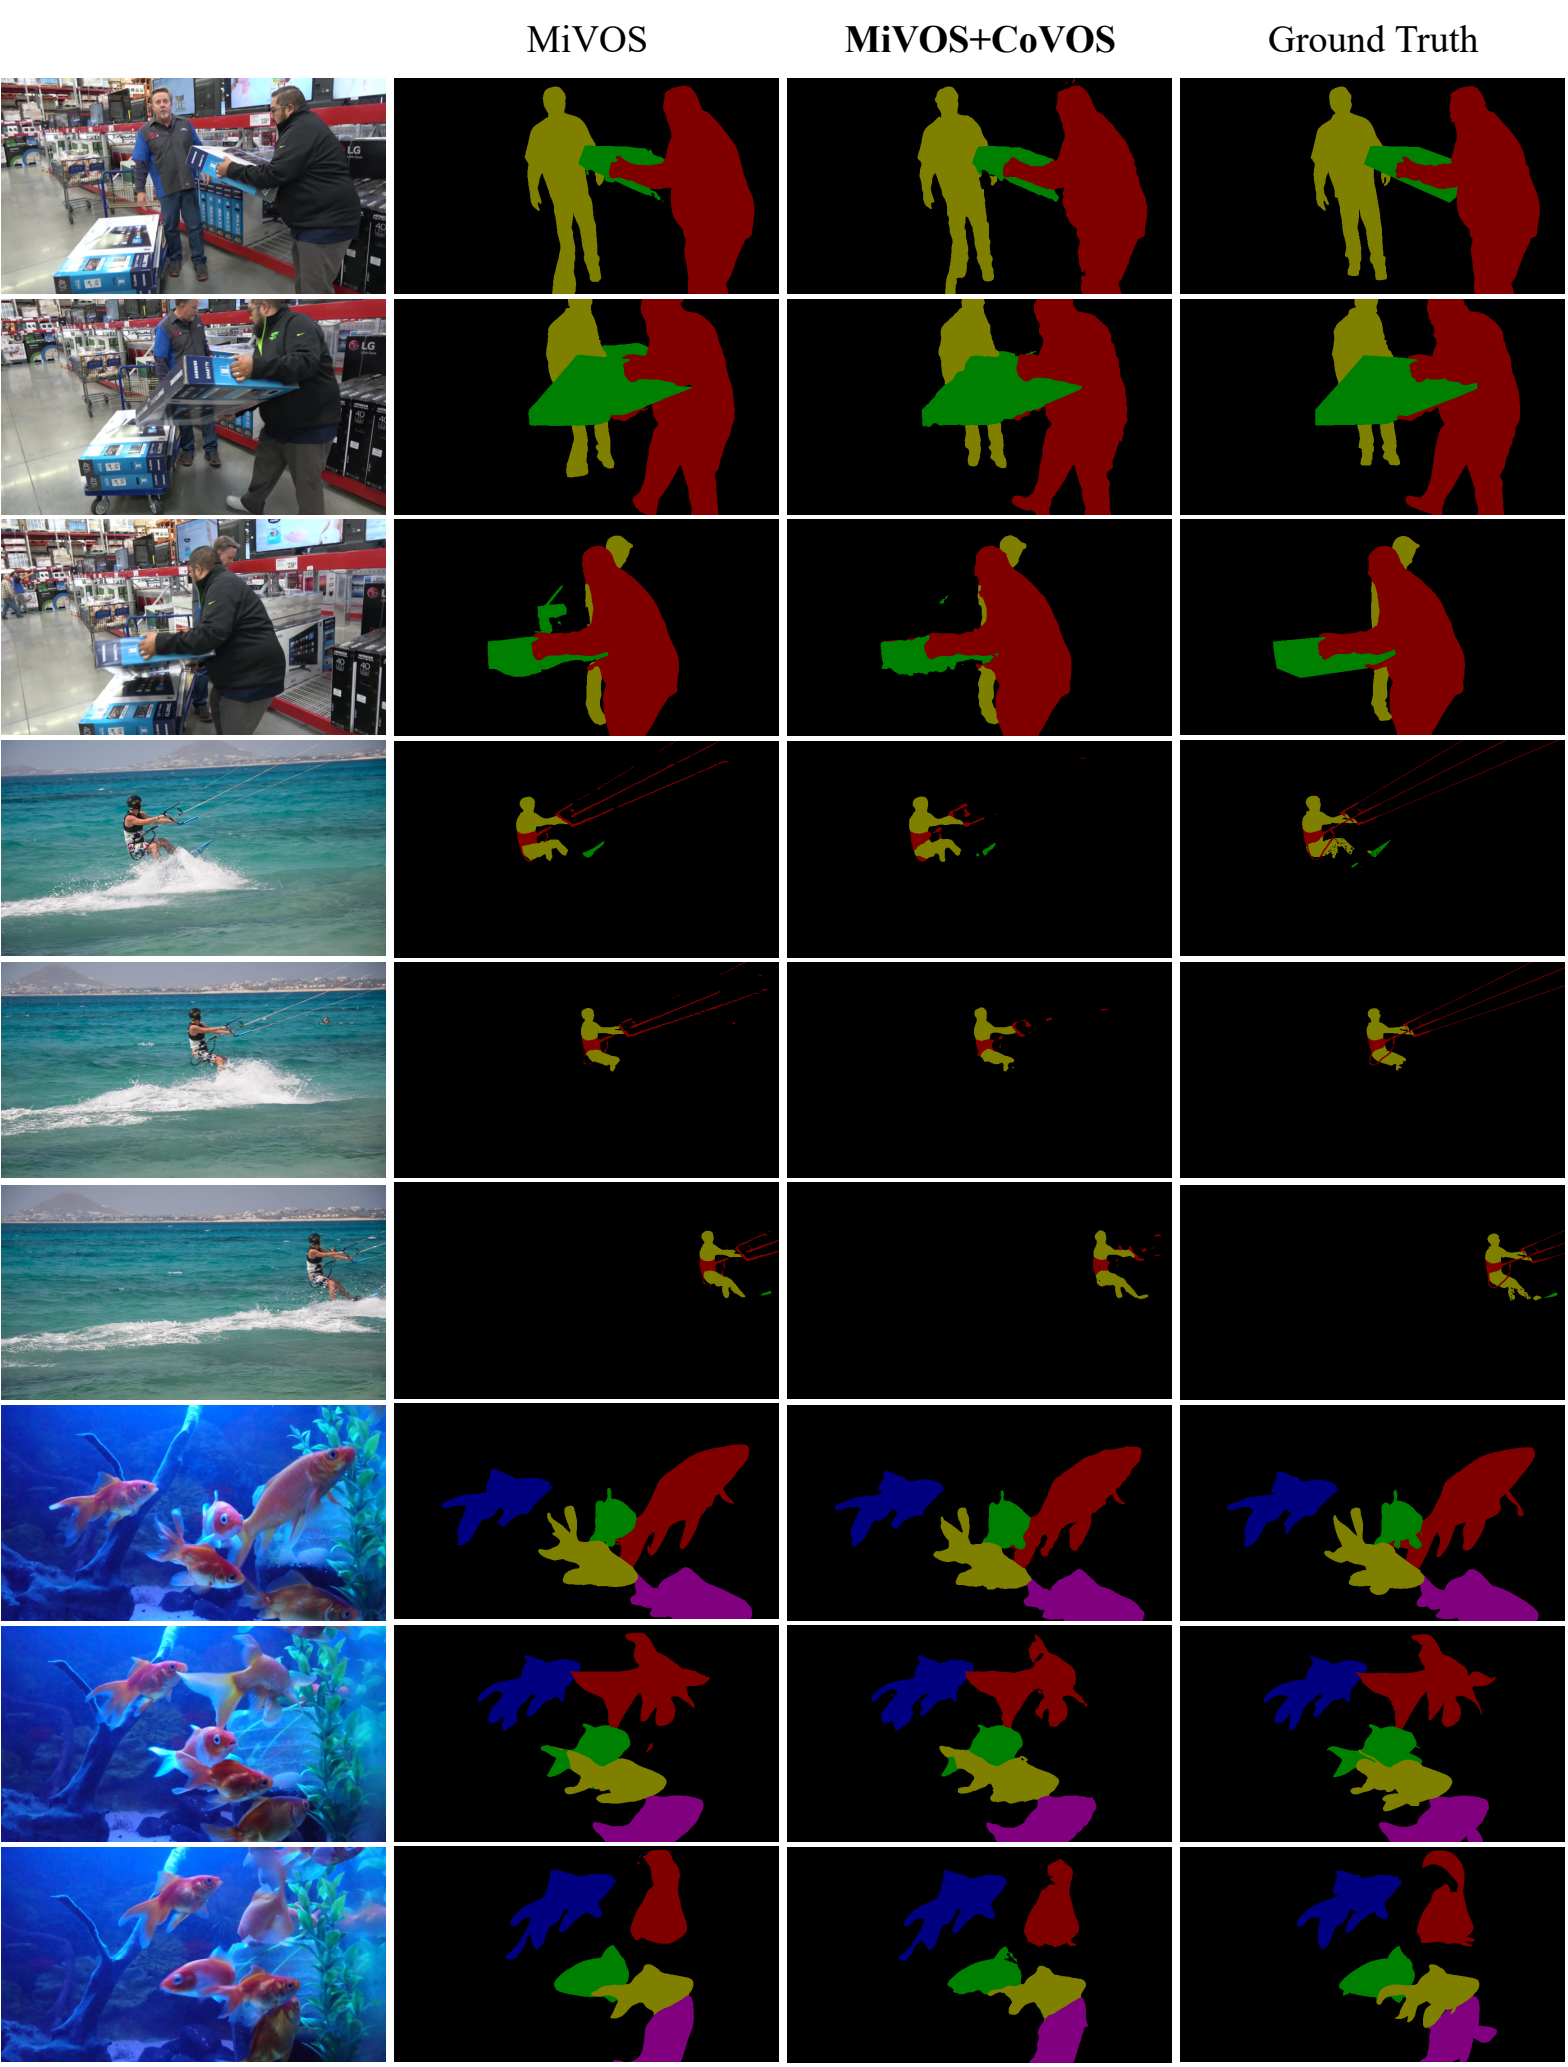 | 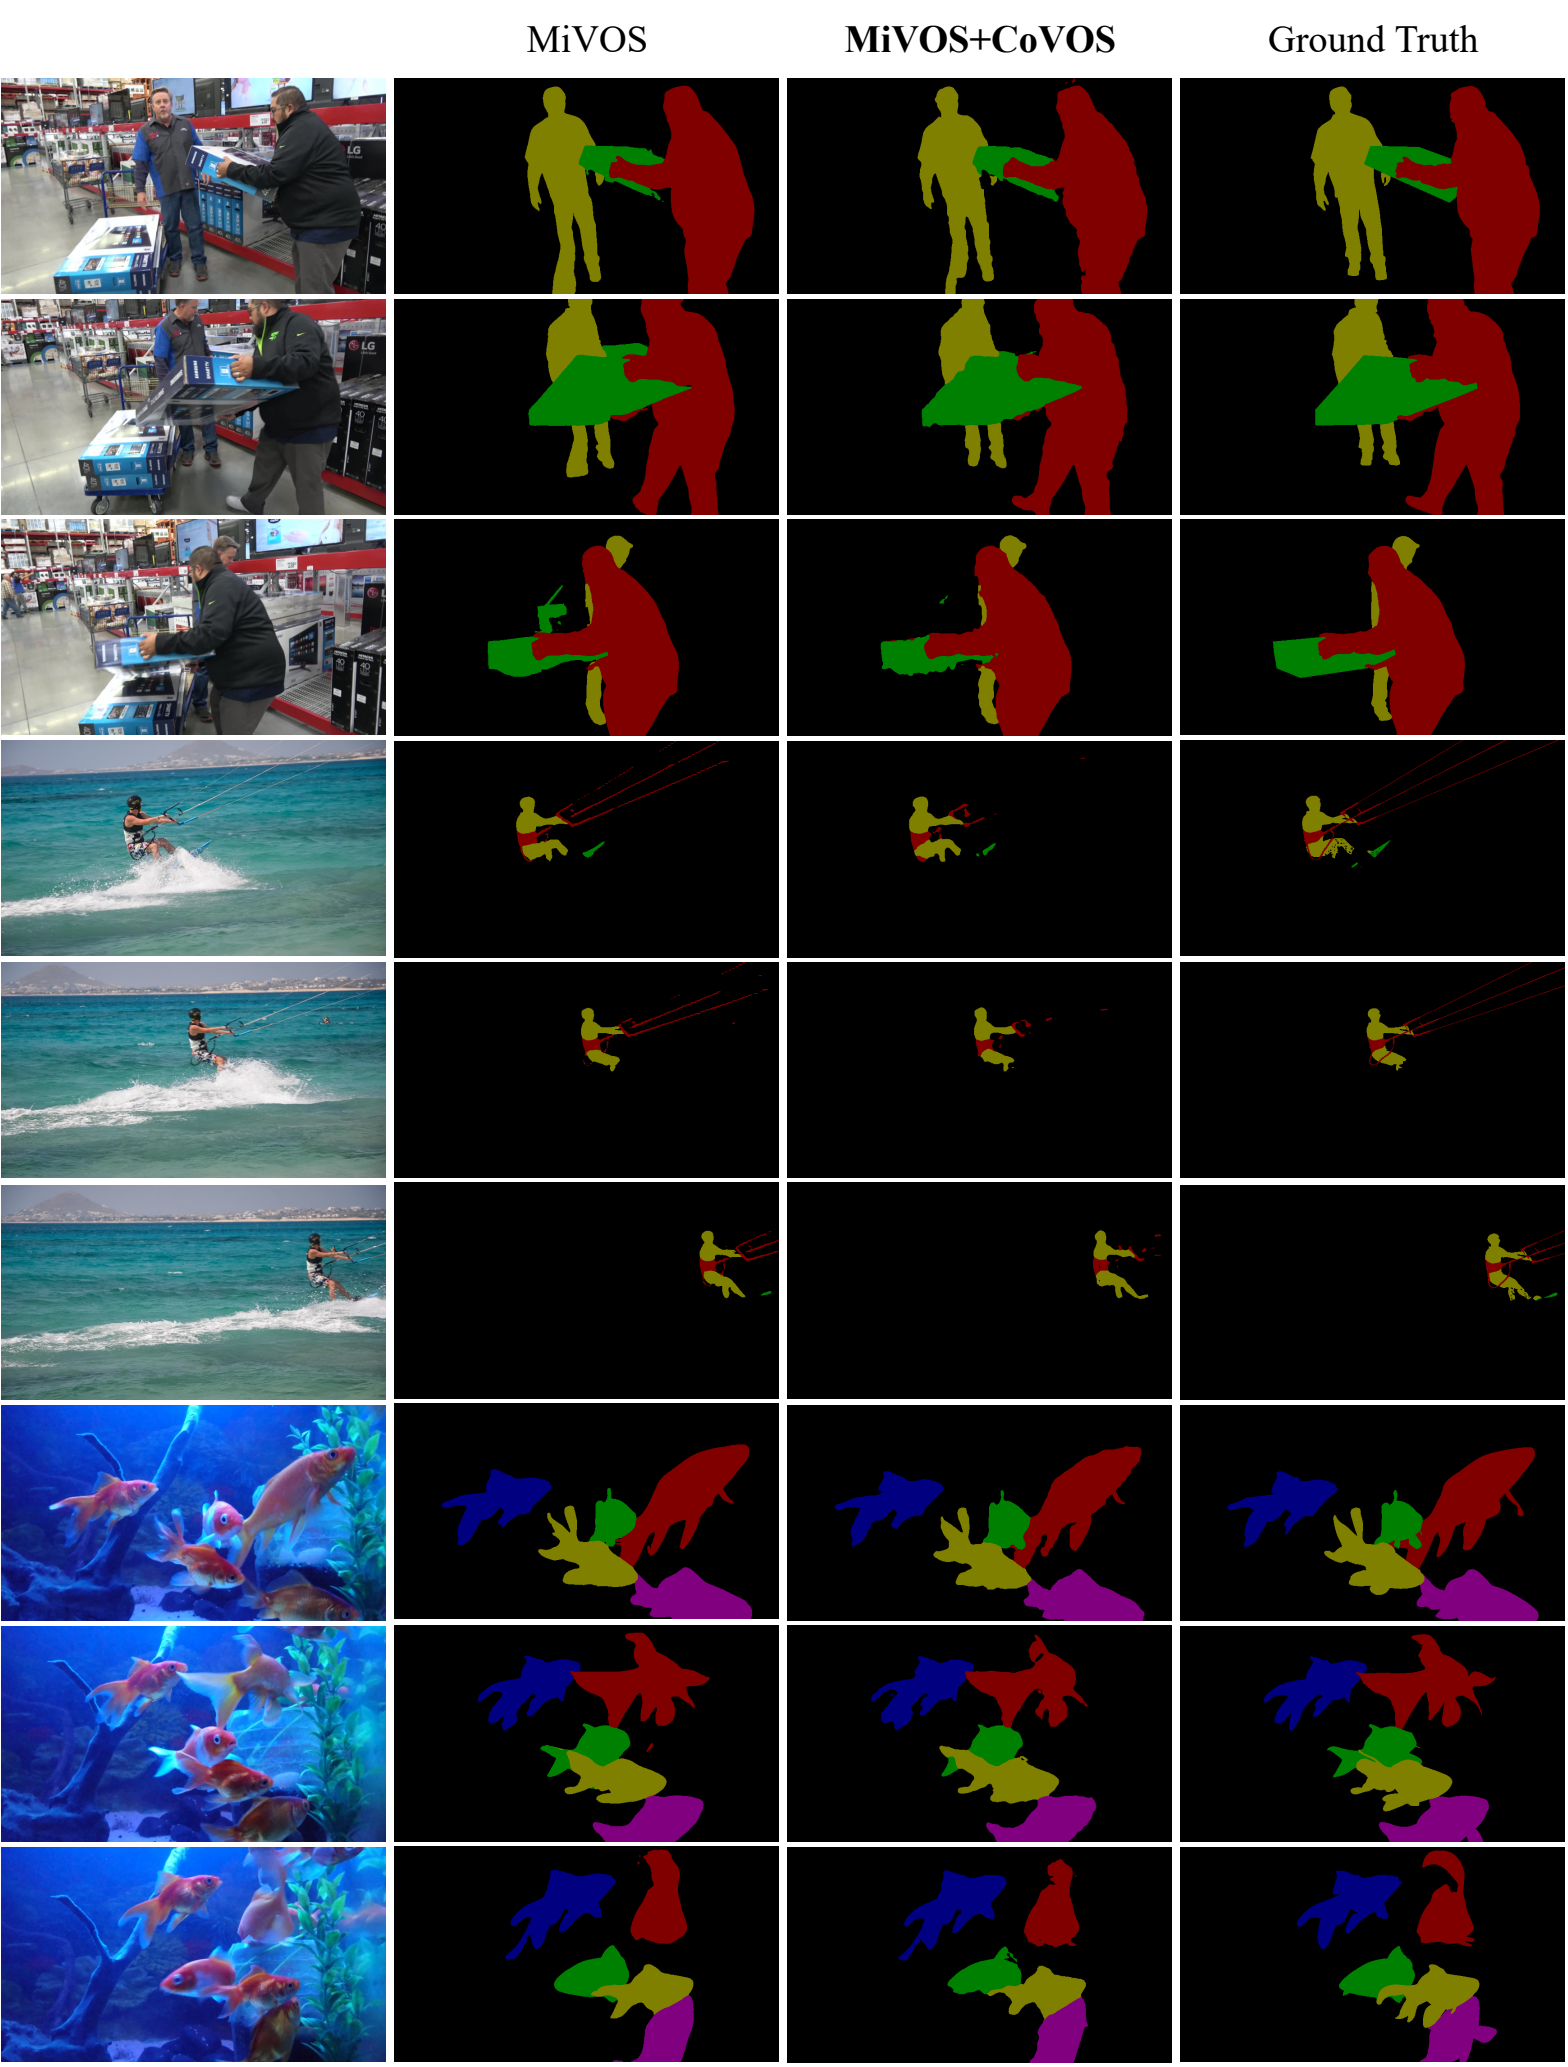 | 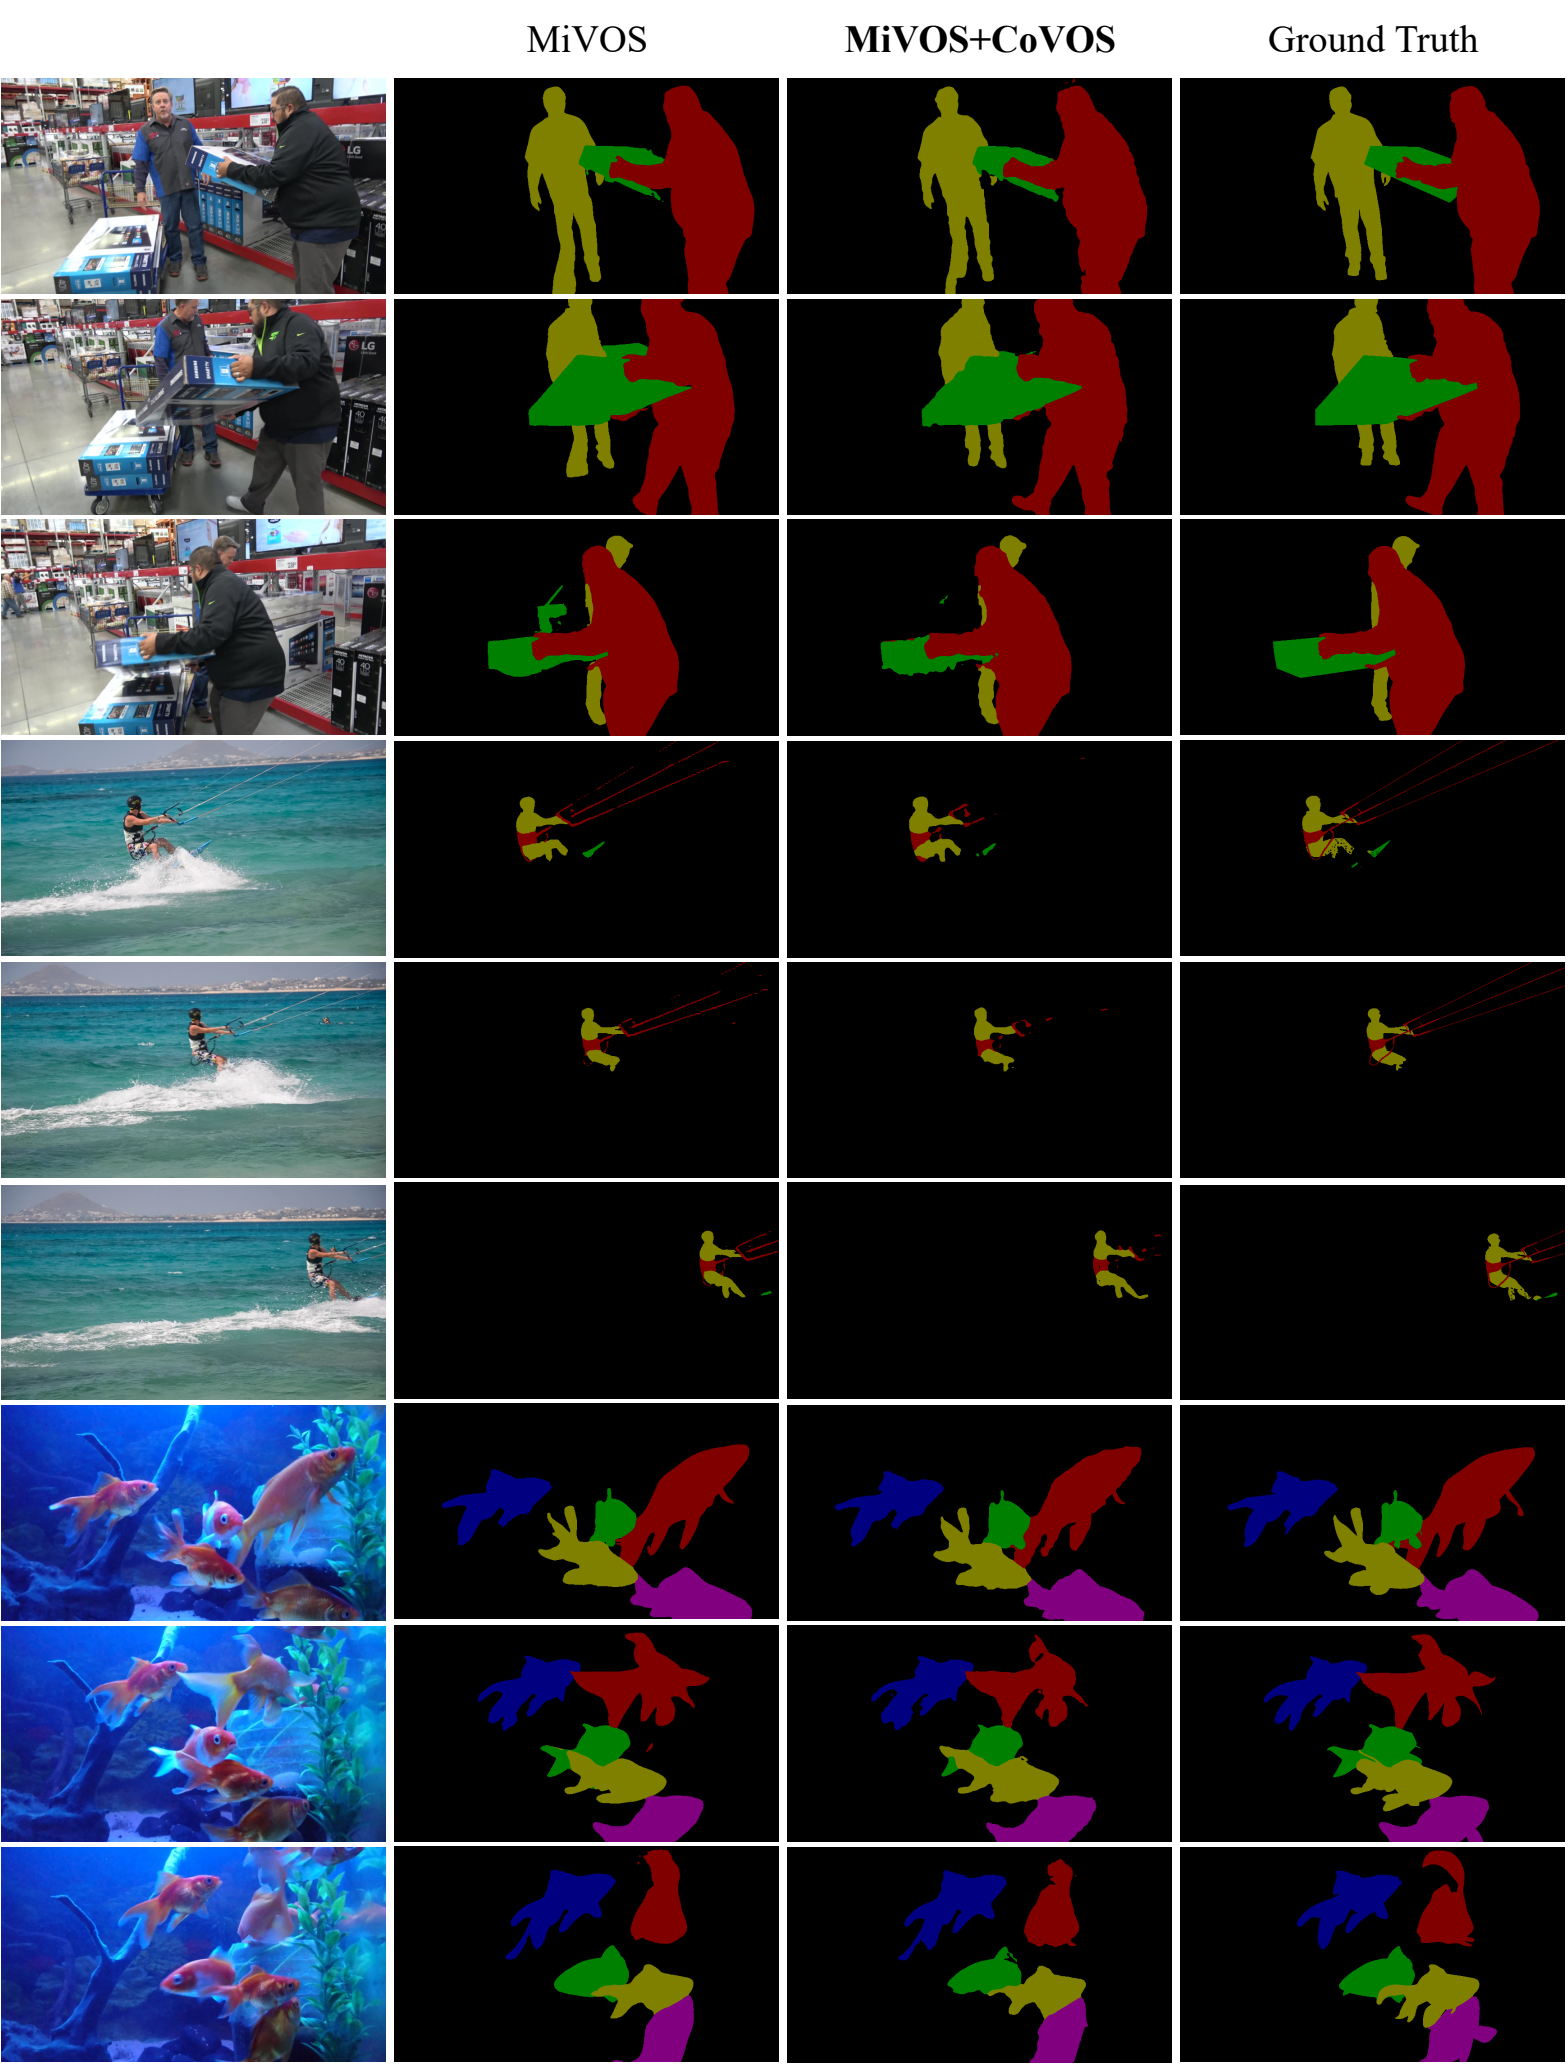 |
| 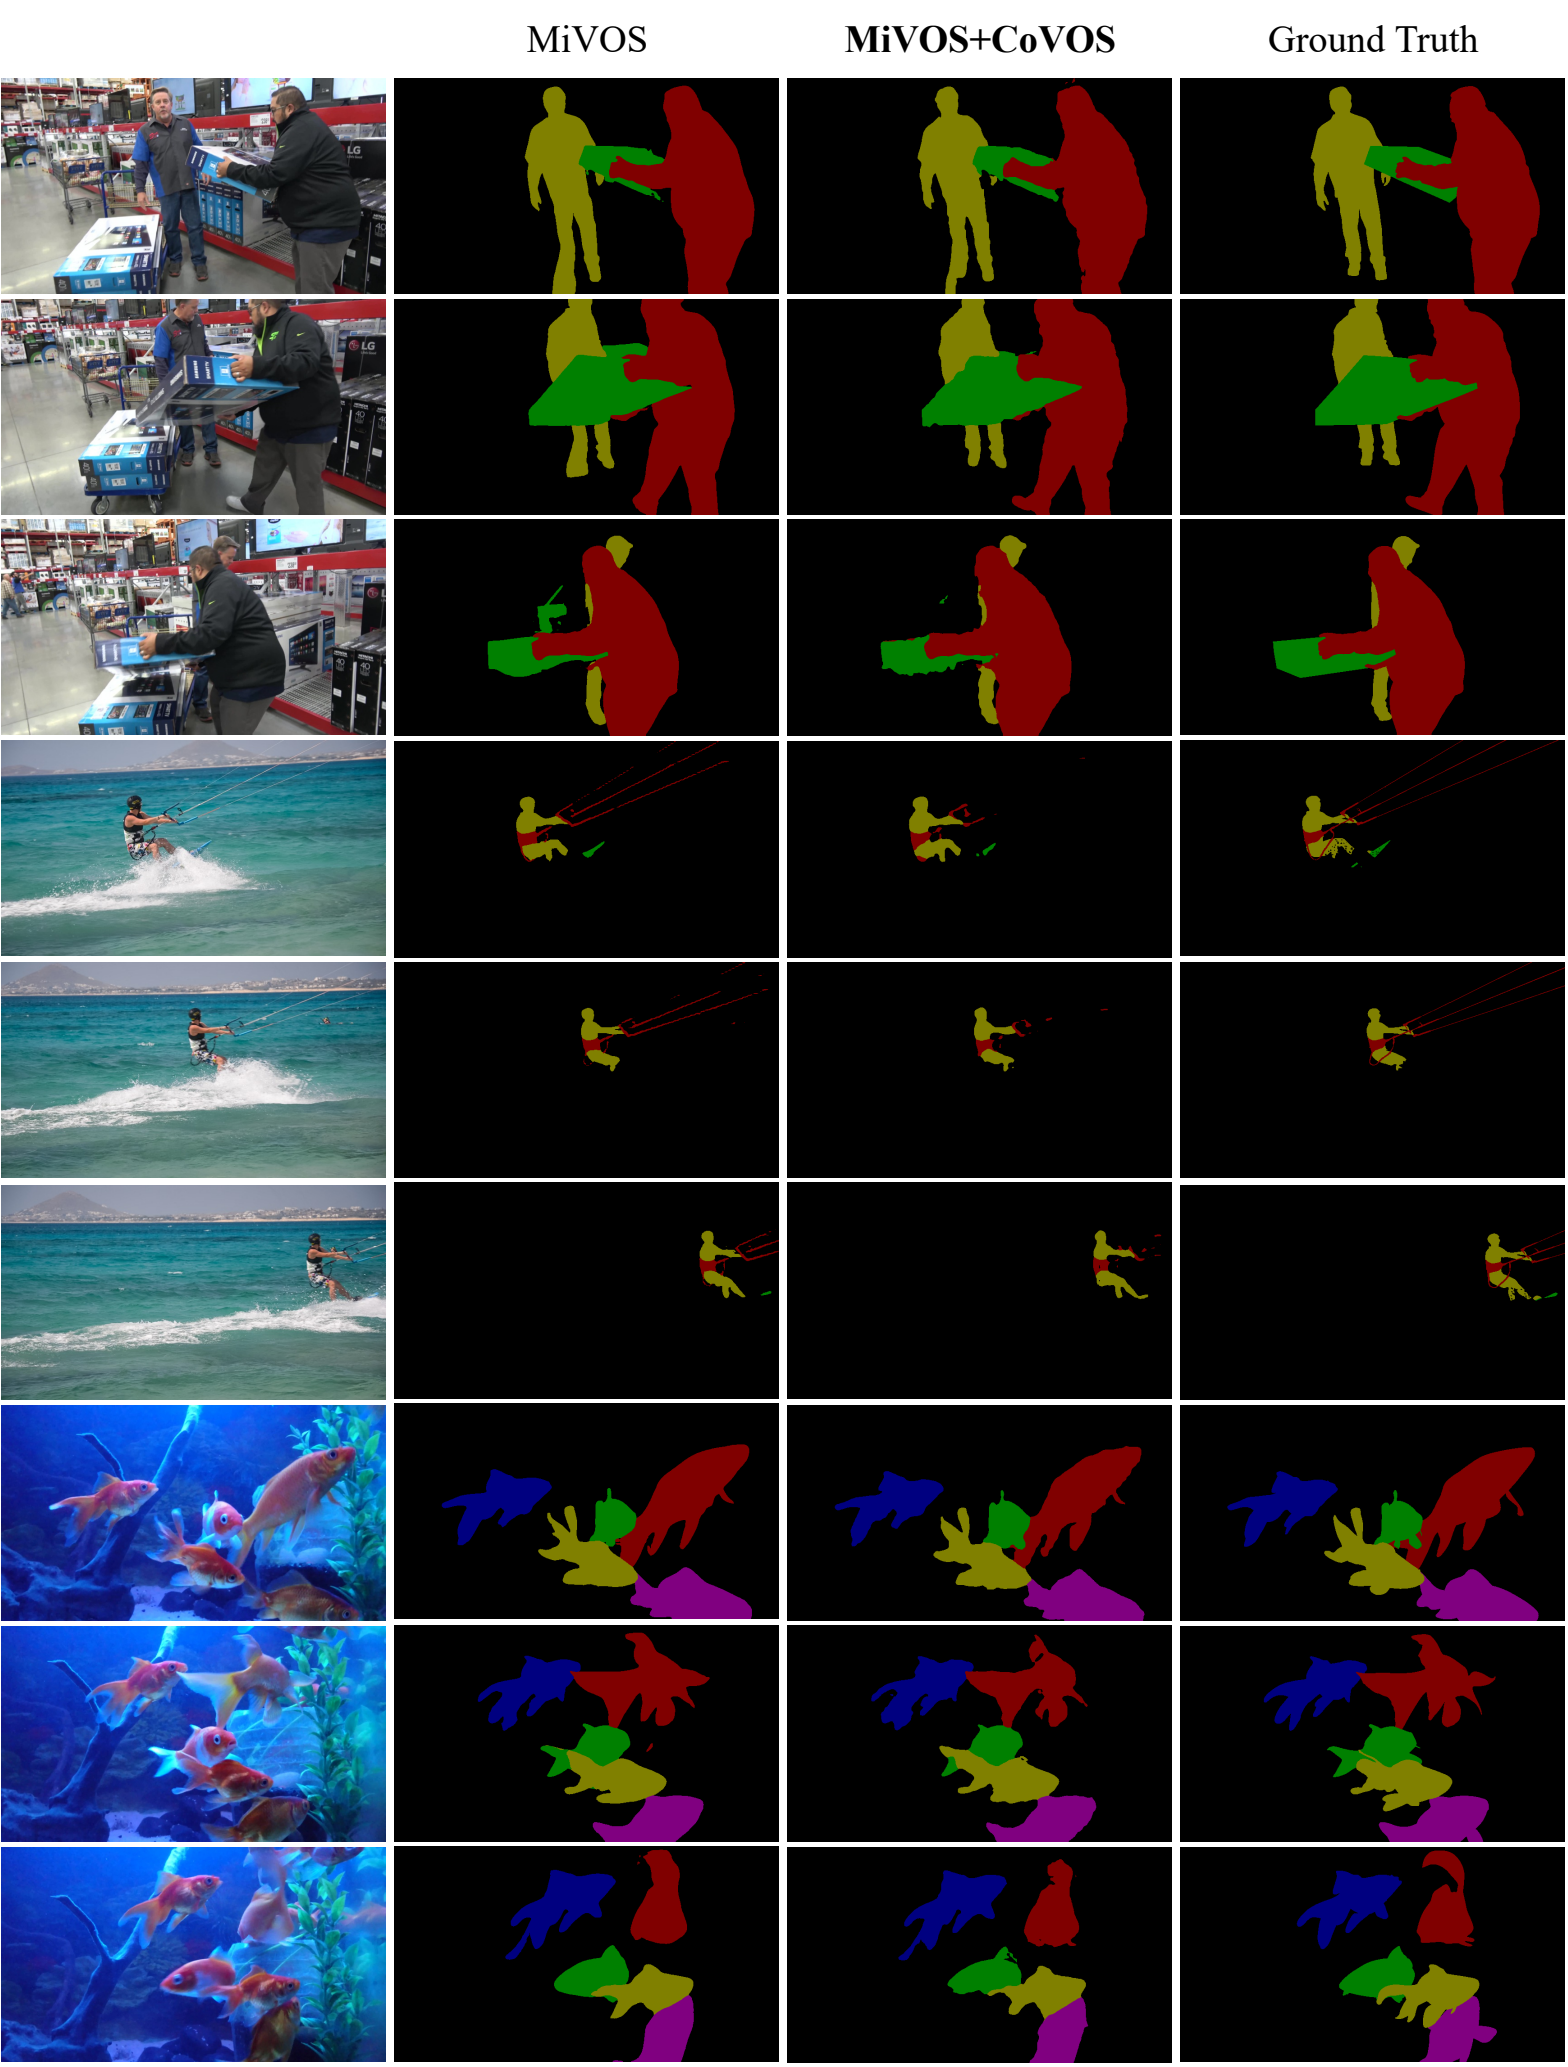 | 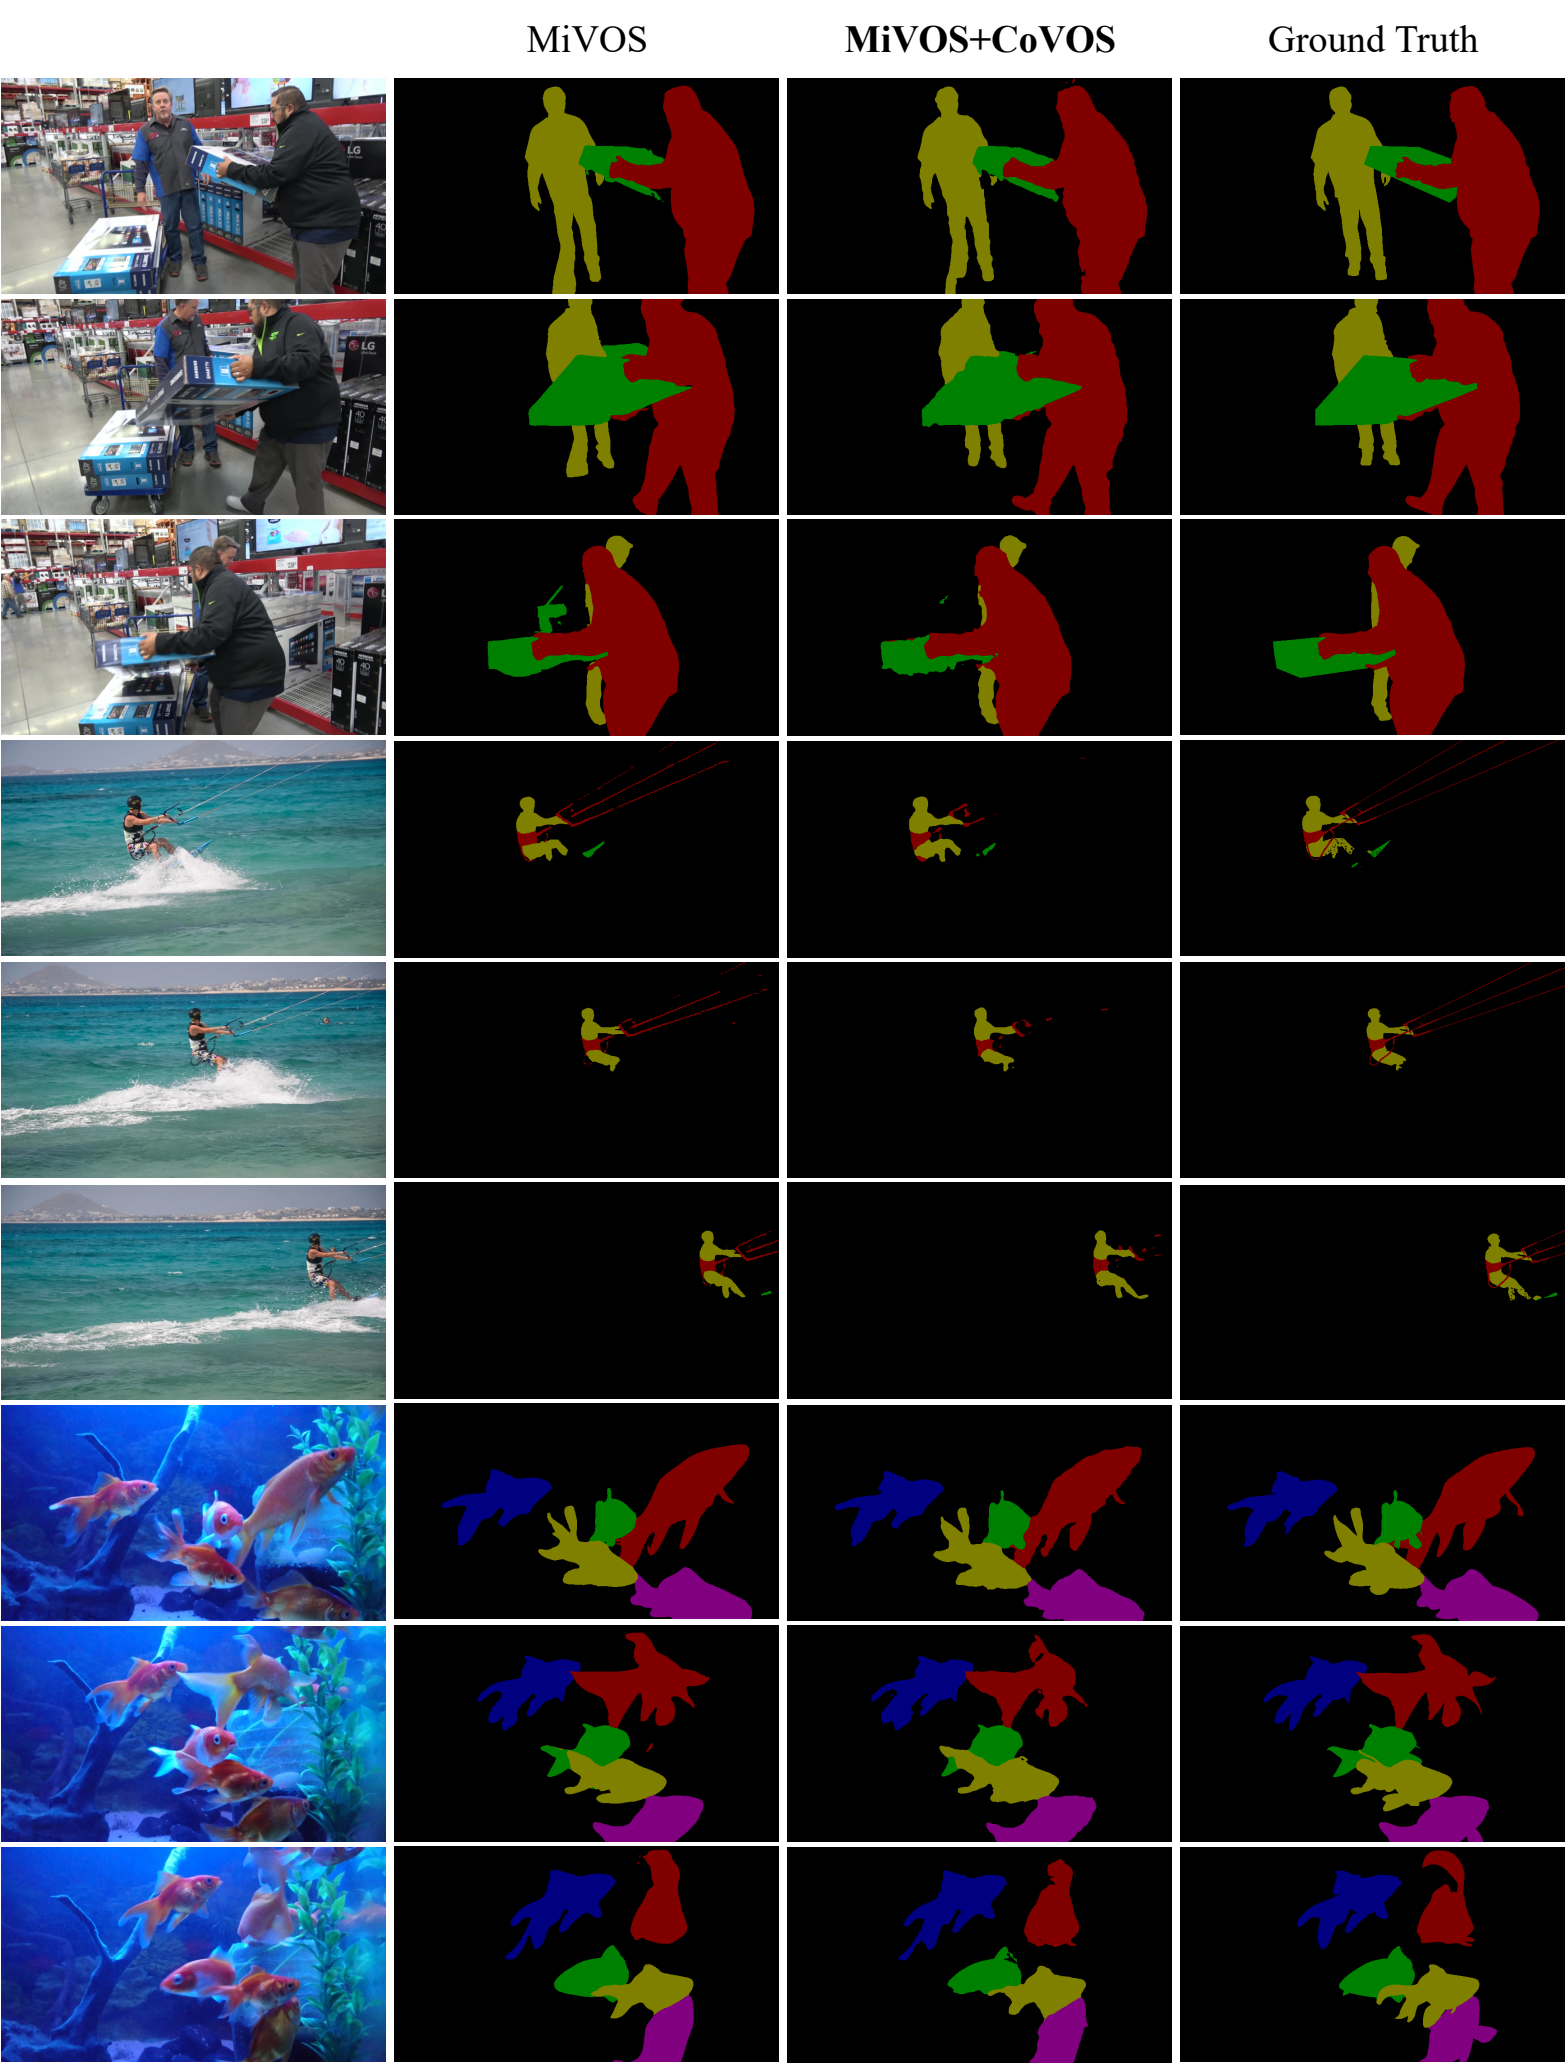 | 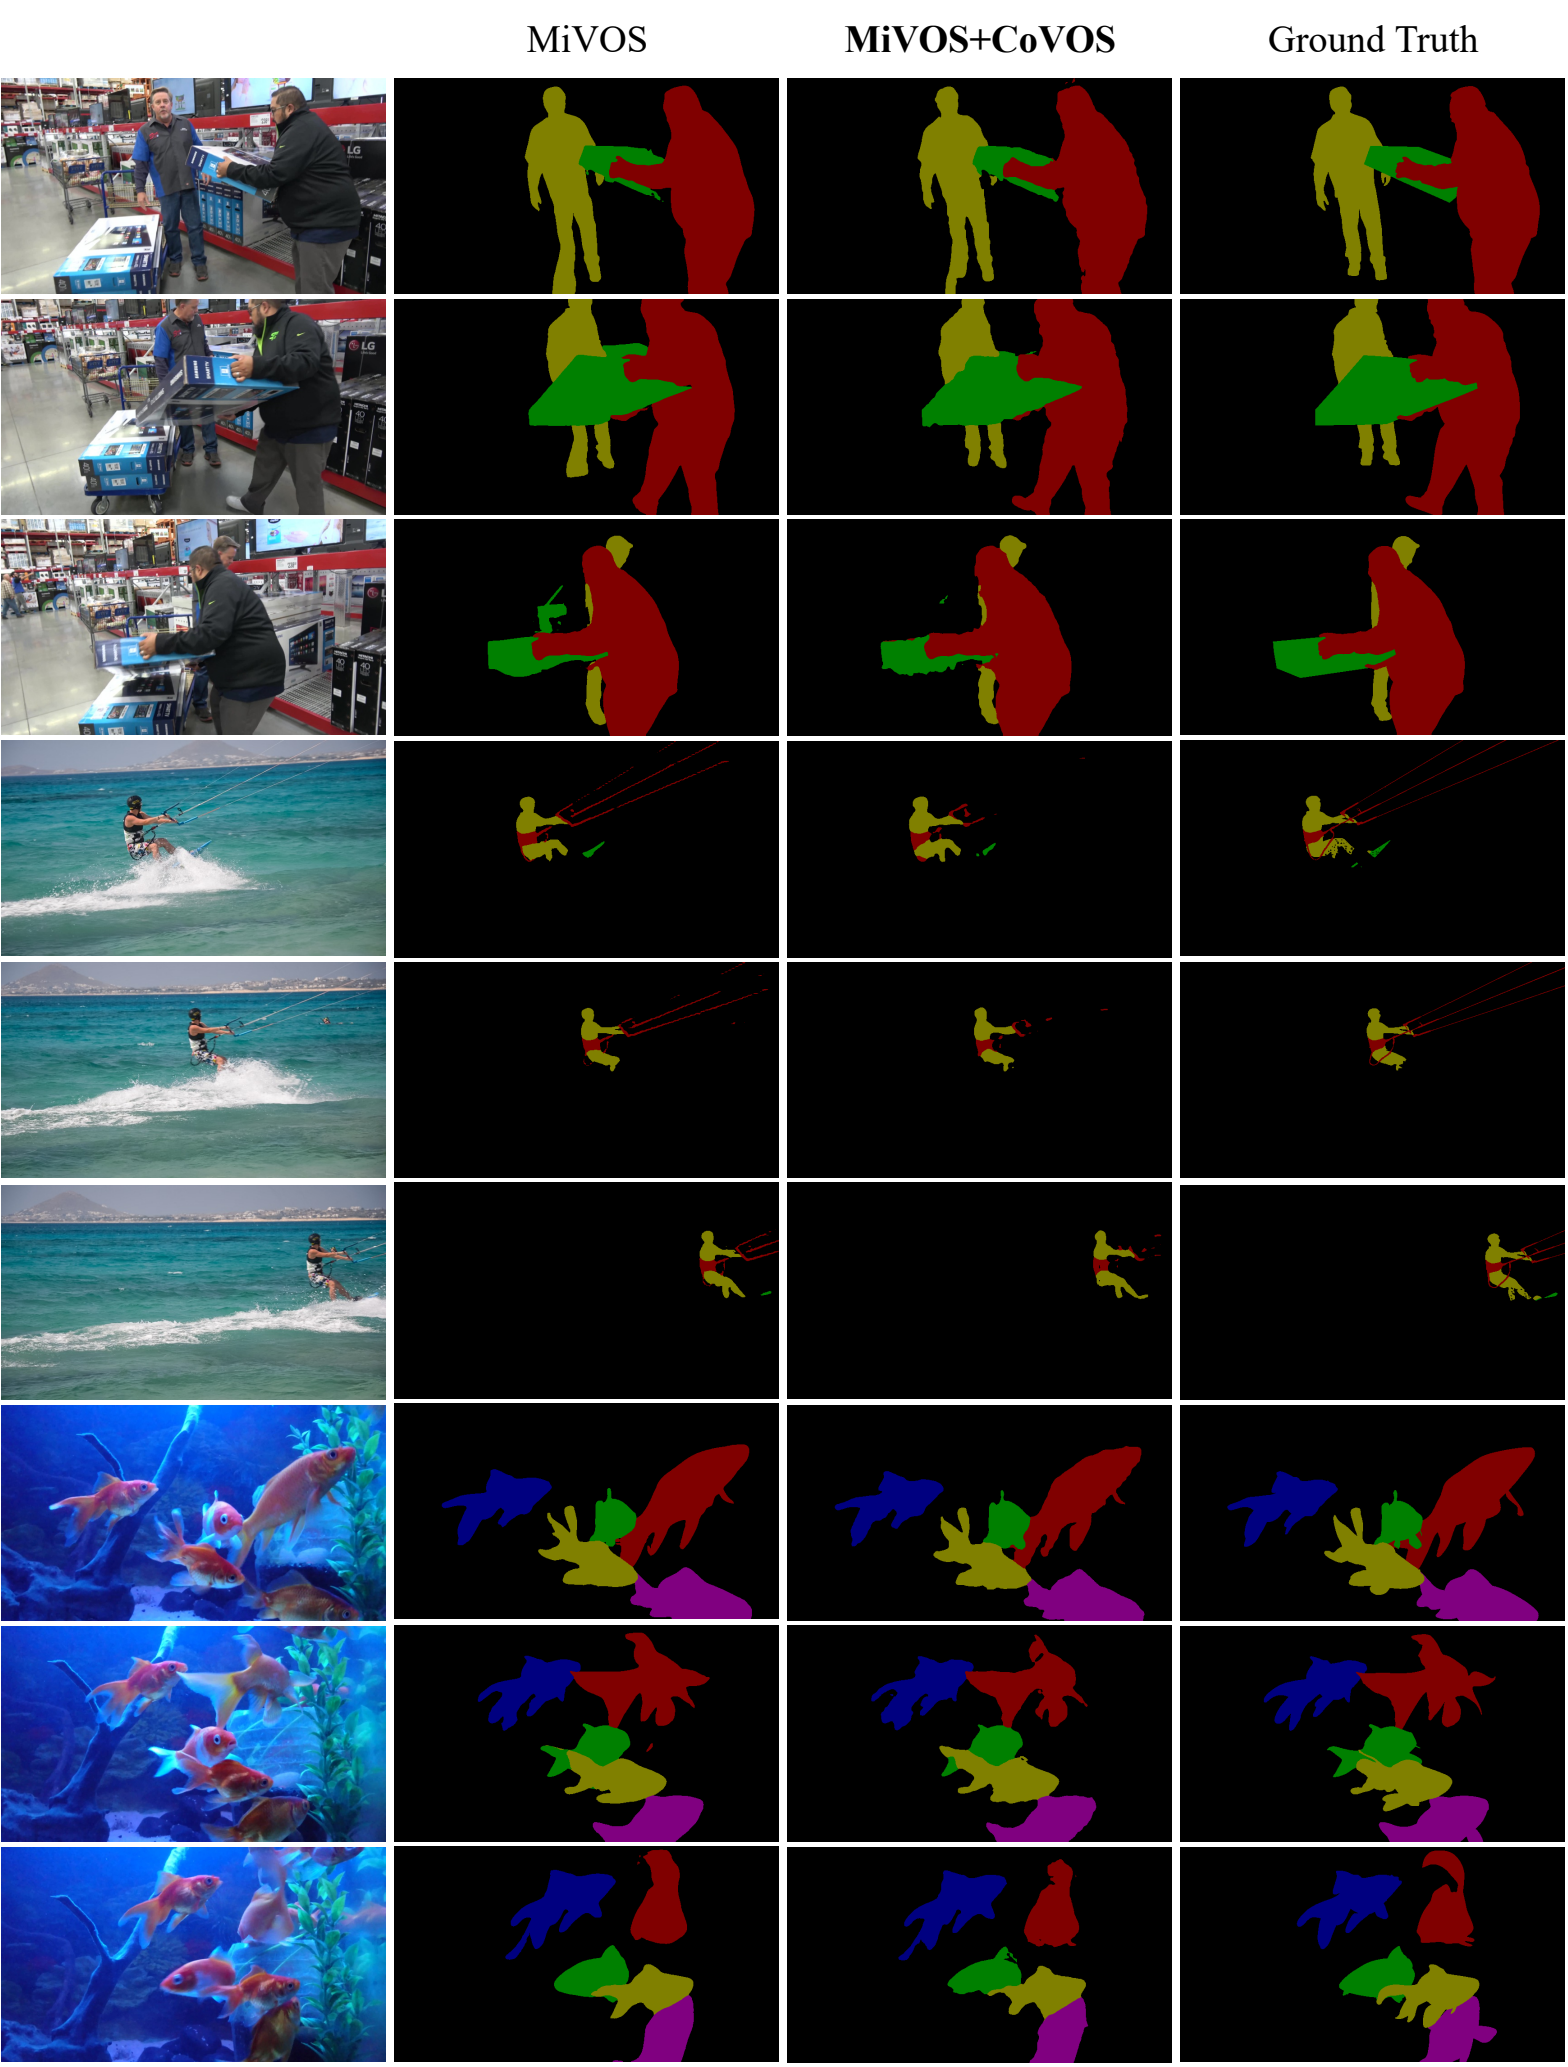 | 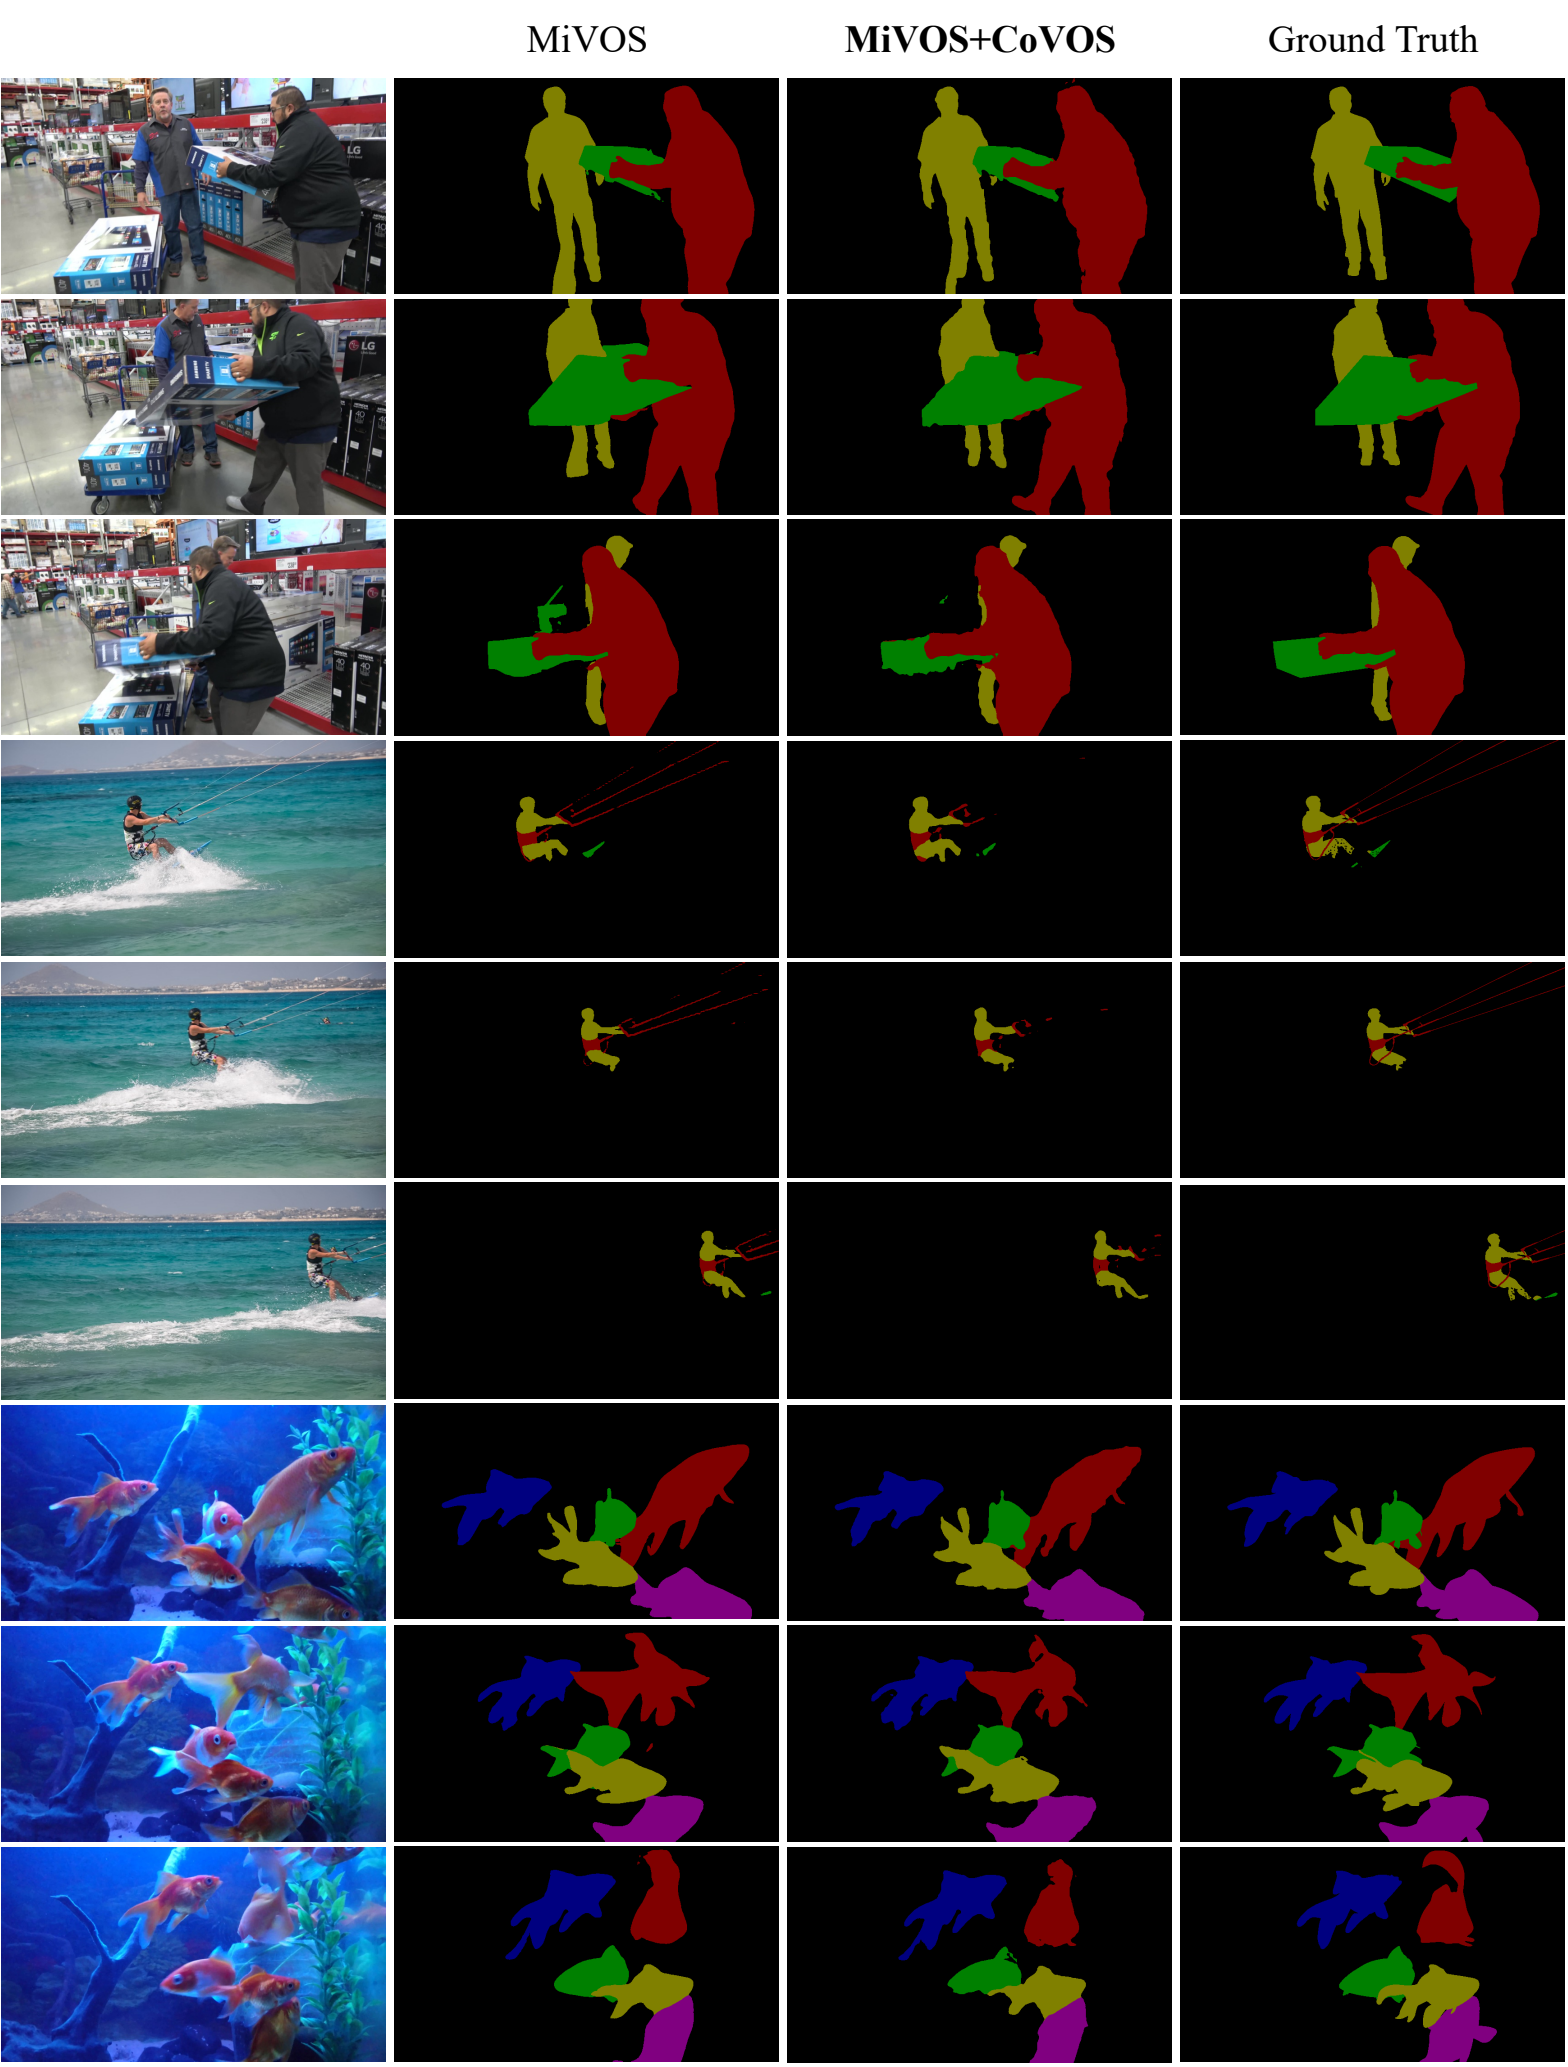 |
| 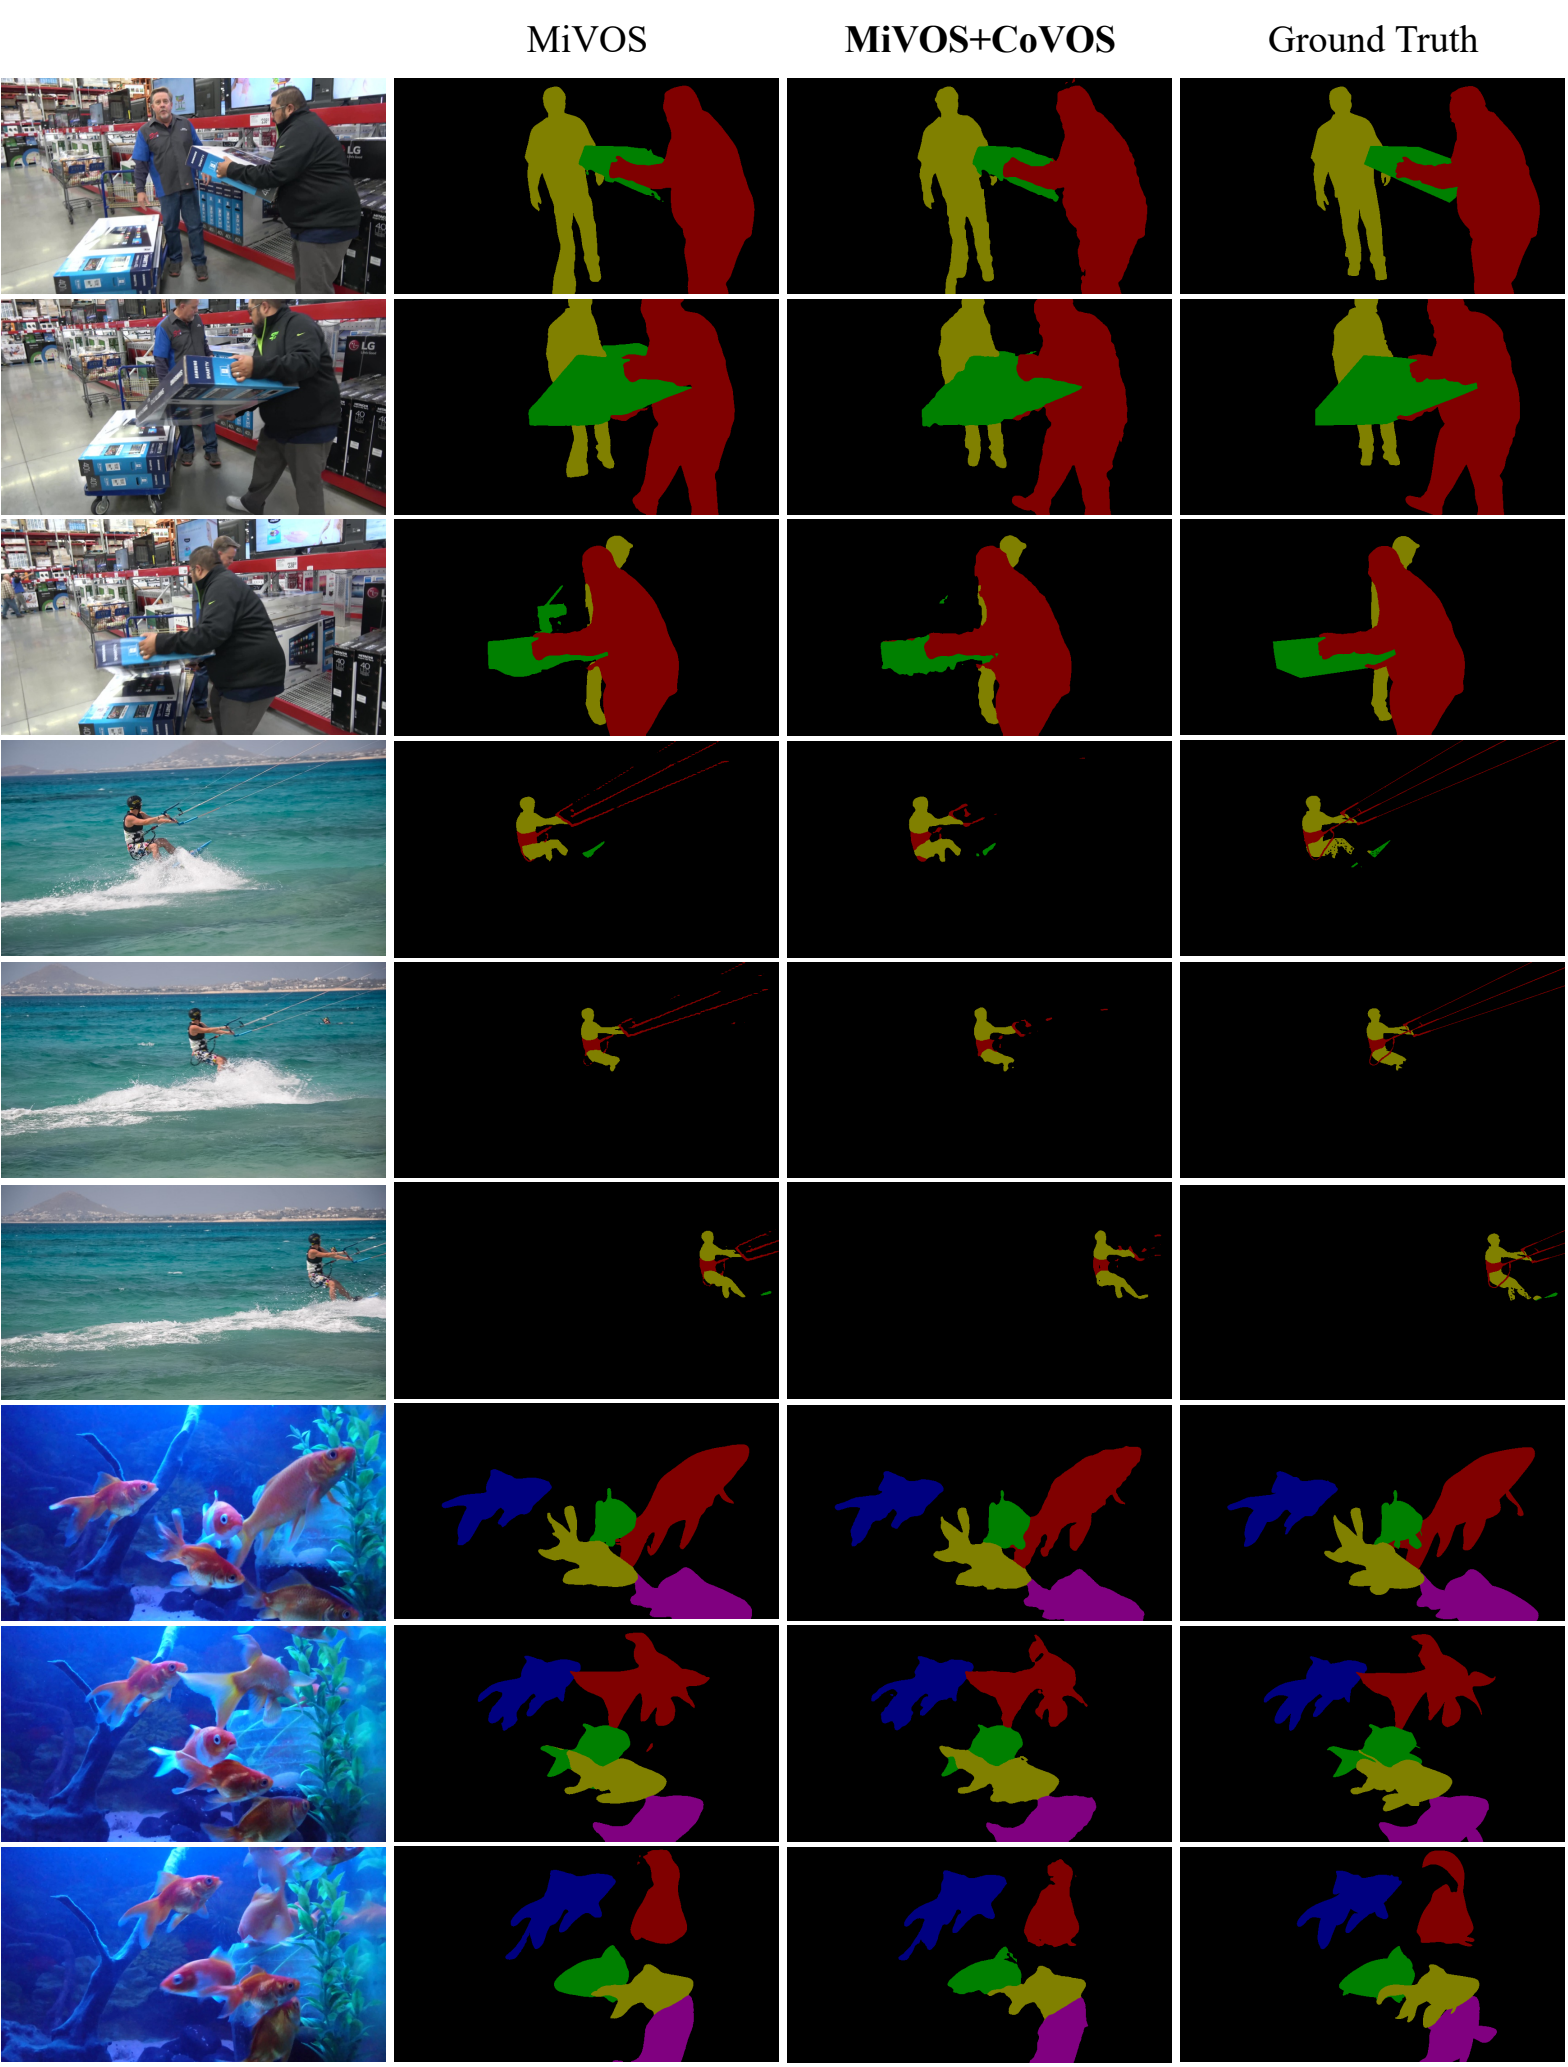 | 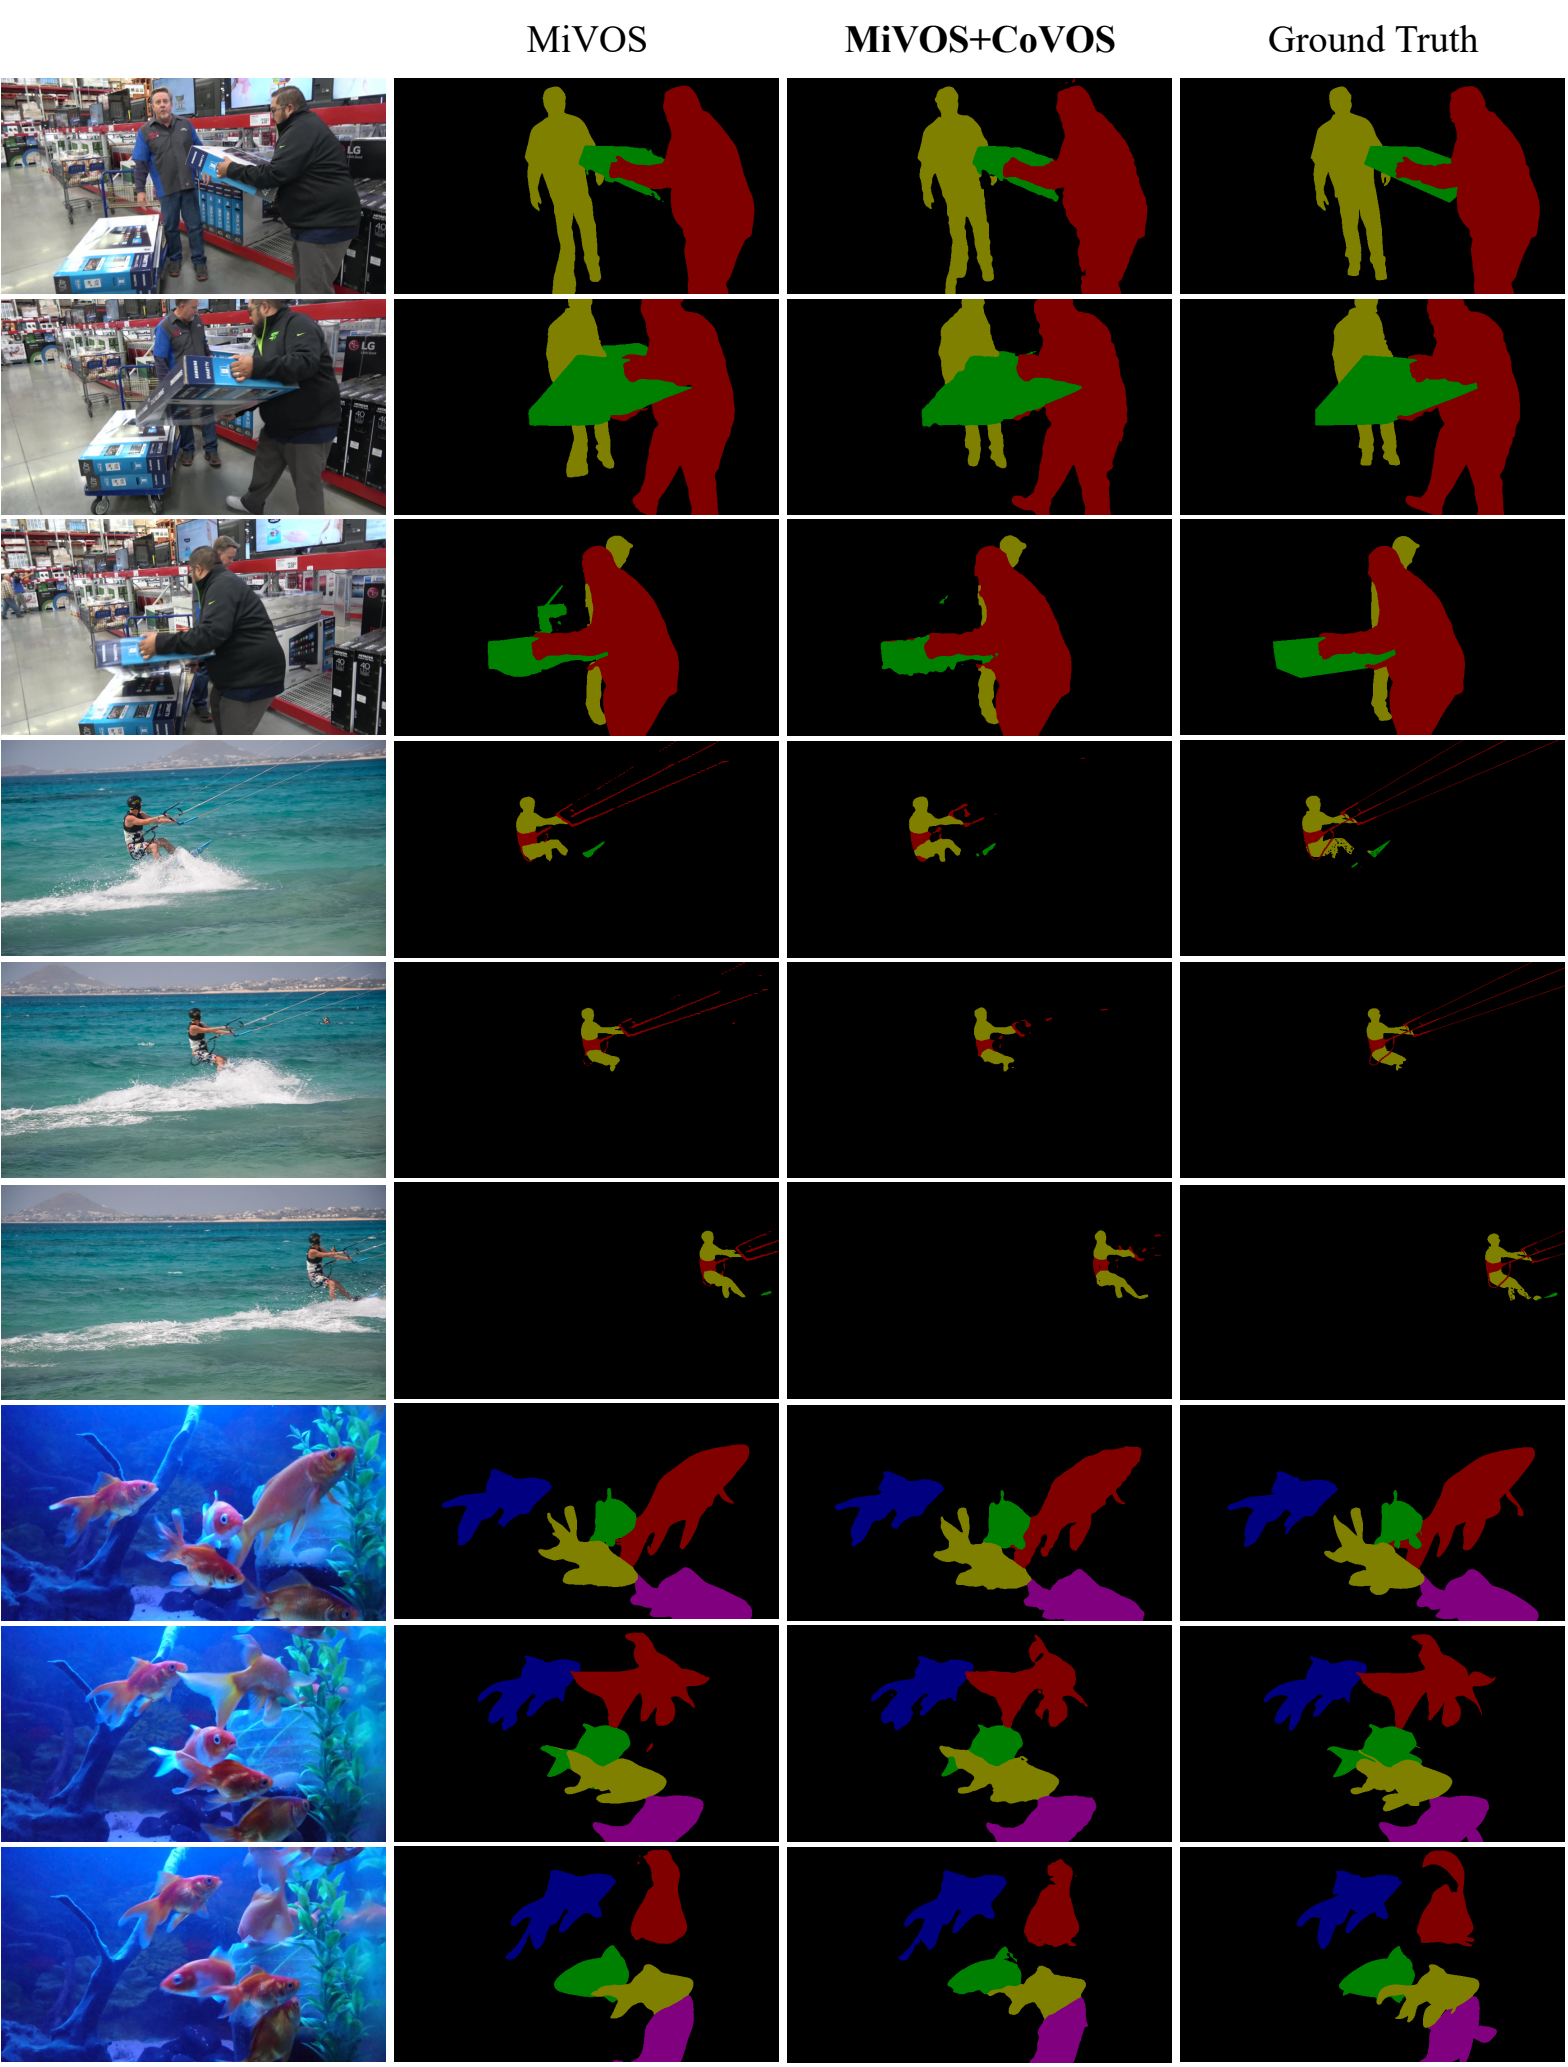 | 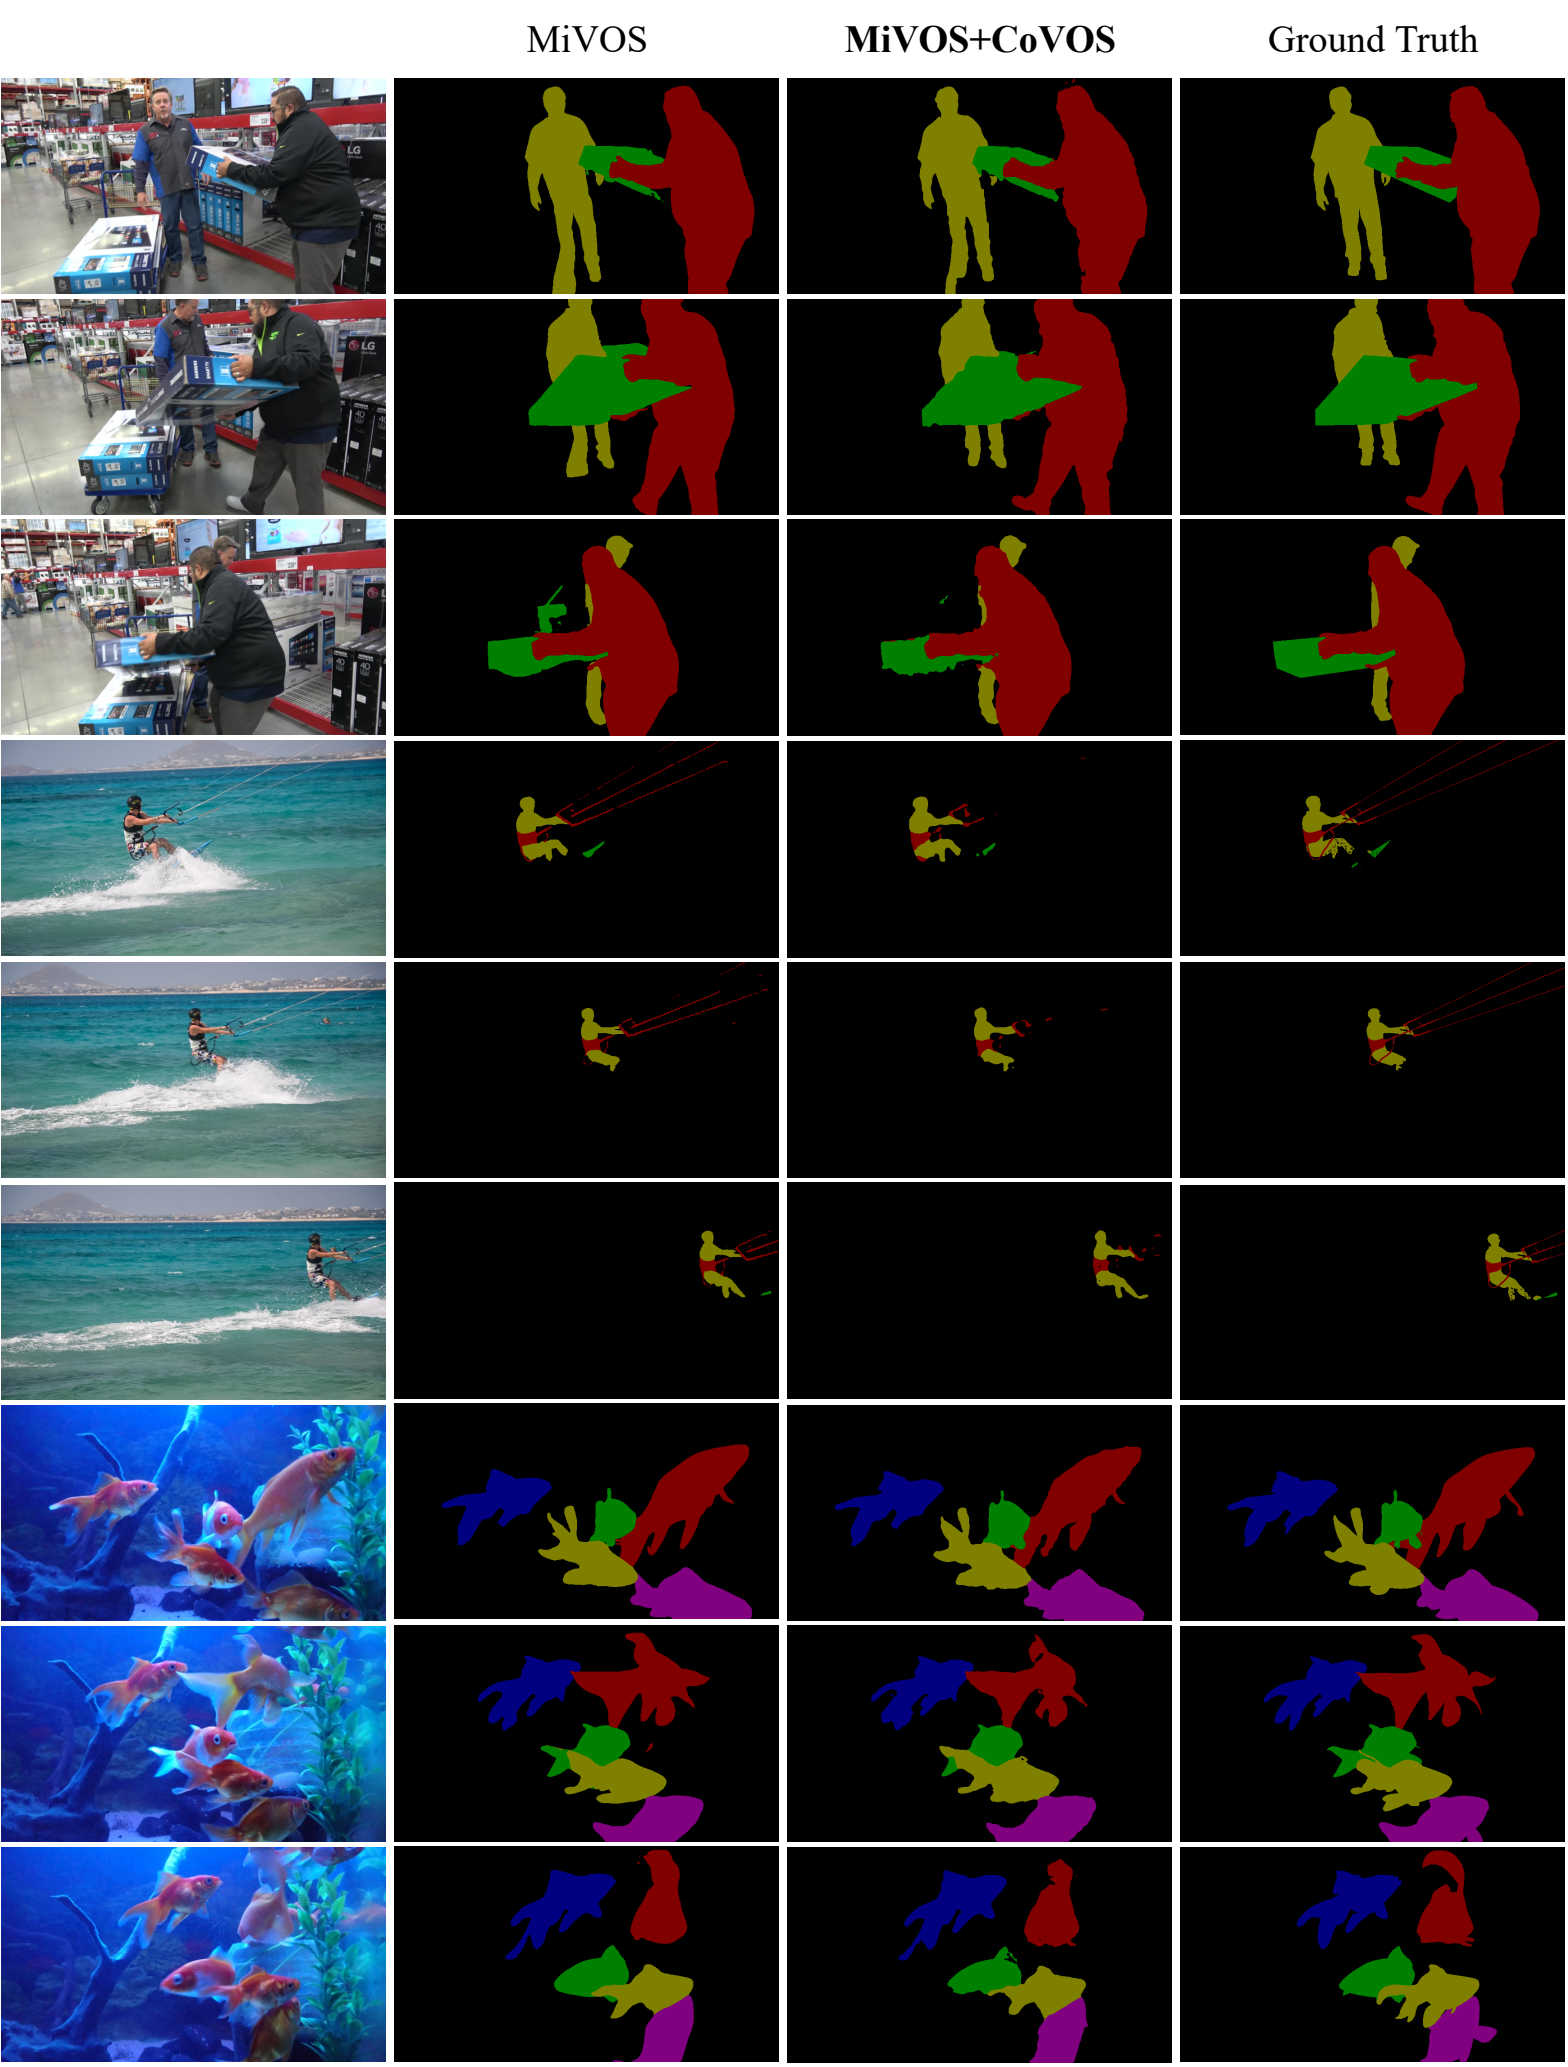 | 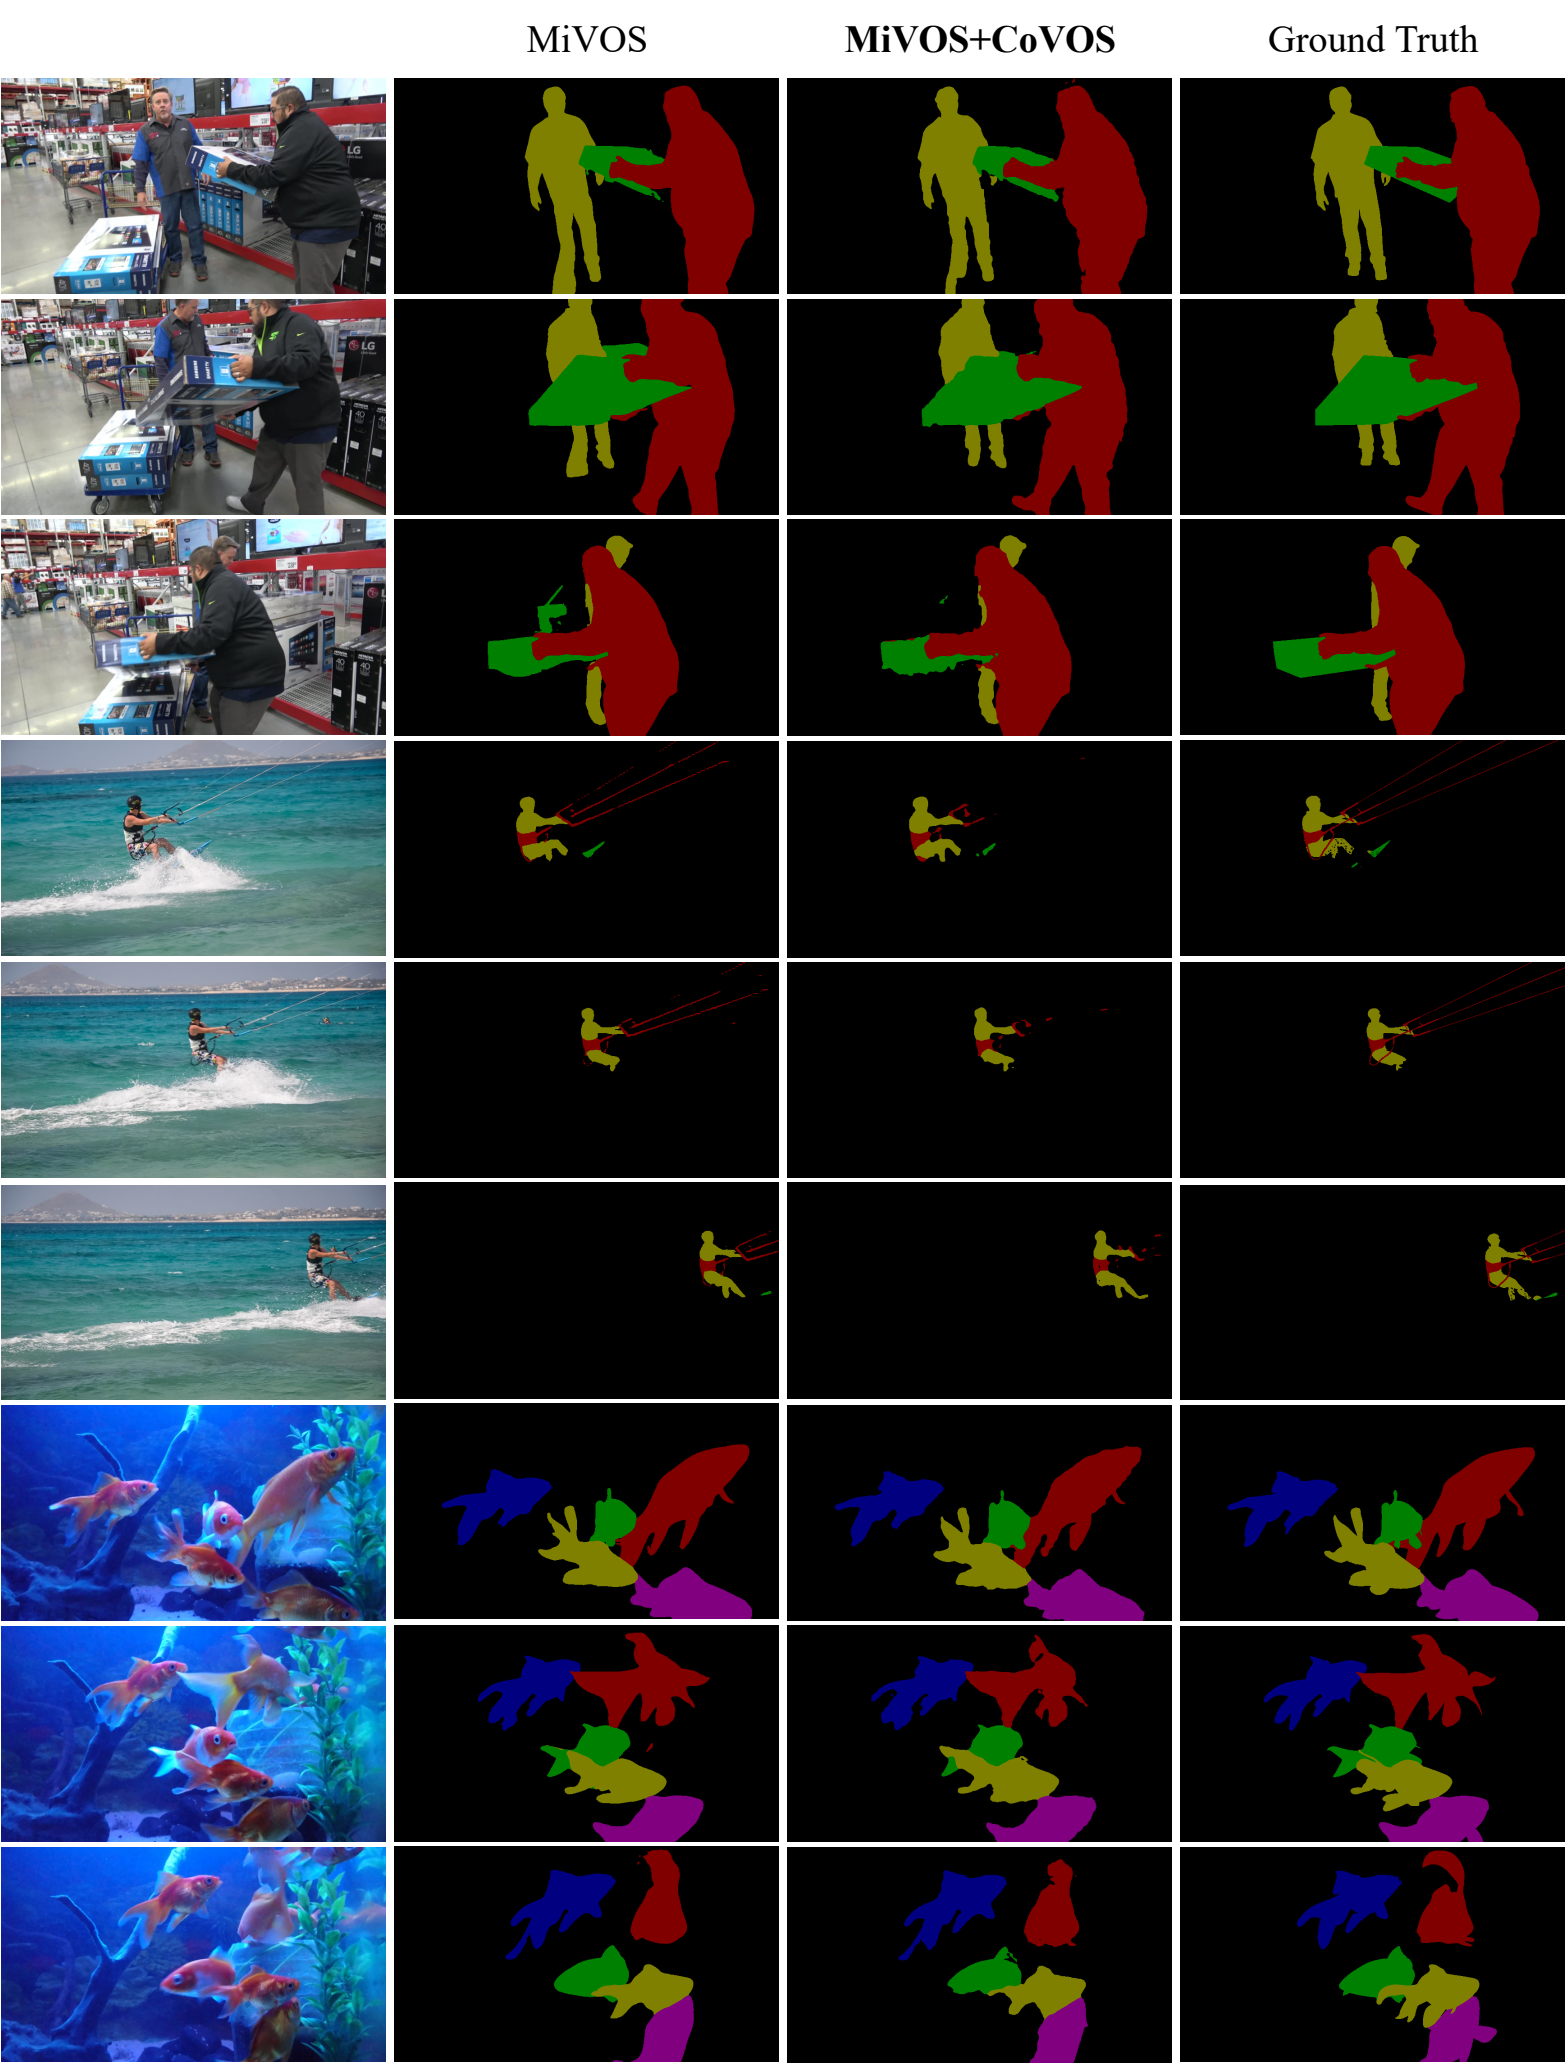 |

|                                                                                   | MiVOS                                                                               | MiVOS+CoVOS                                                                          | Ground Truth                                                                          |
|-----------------------------------------------------------------------------------|-------------------------------------------------------------------------------------|--------------------------------------------------------------------------------------|---------------------------------------------------------------------------------------|
| 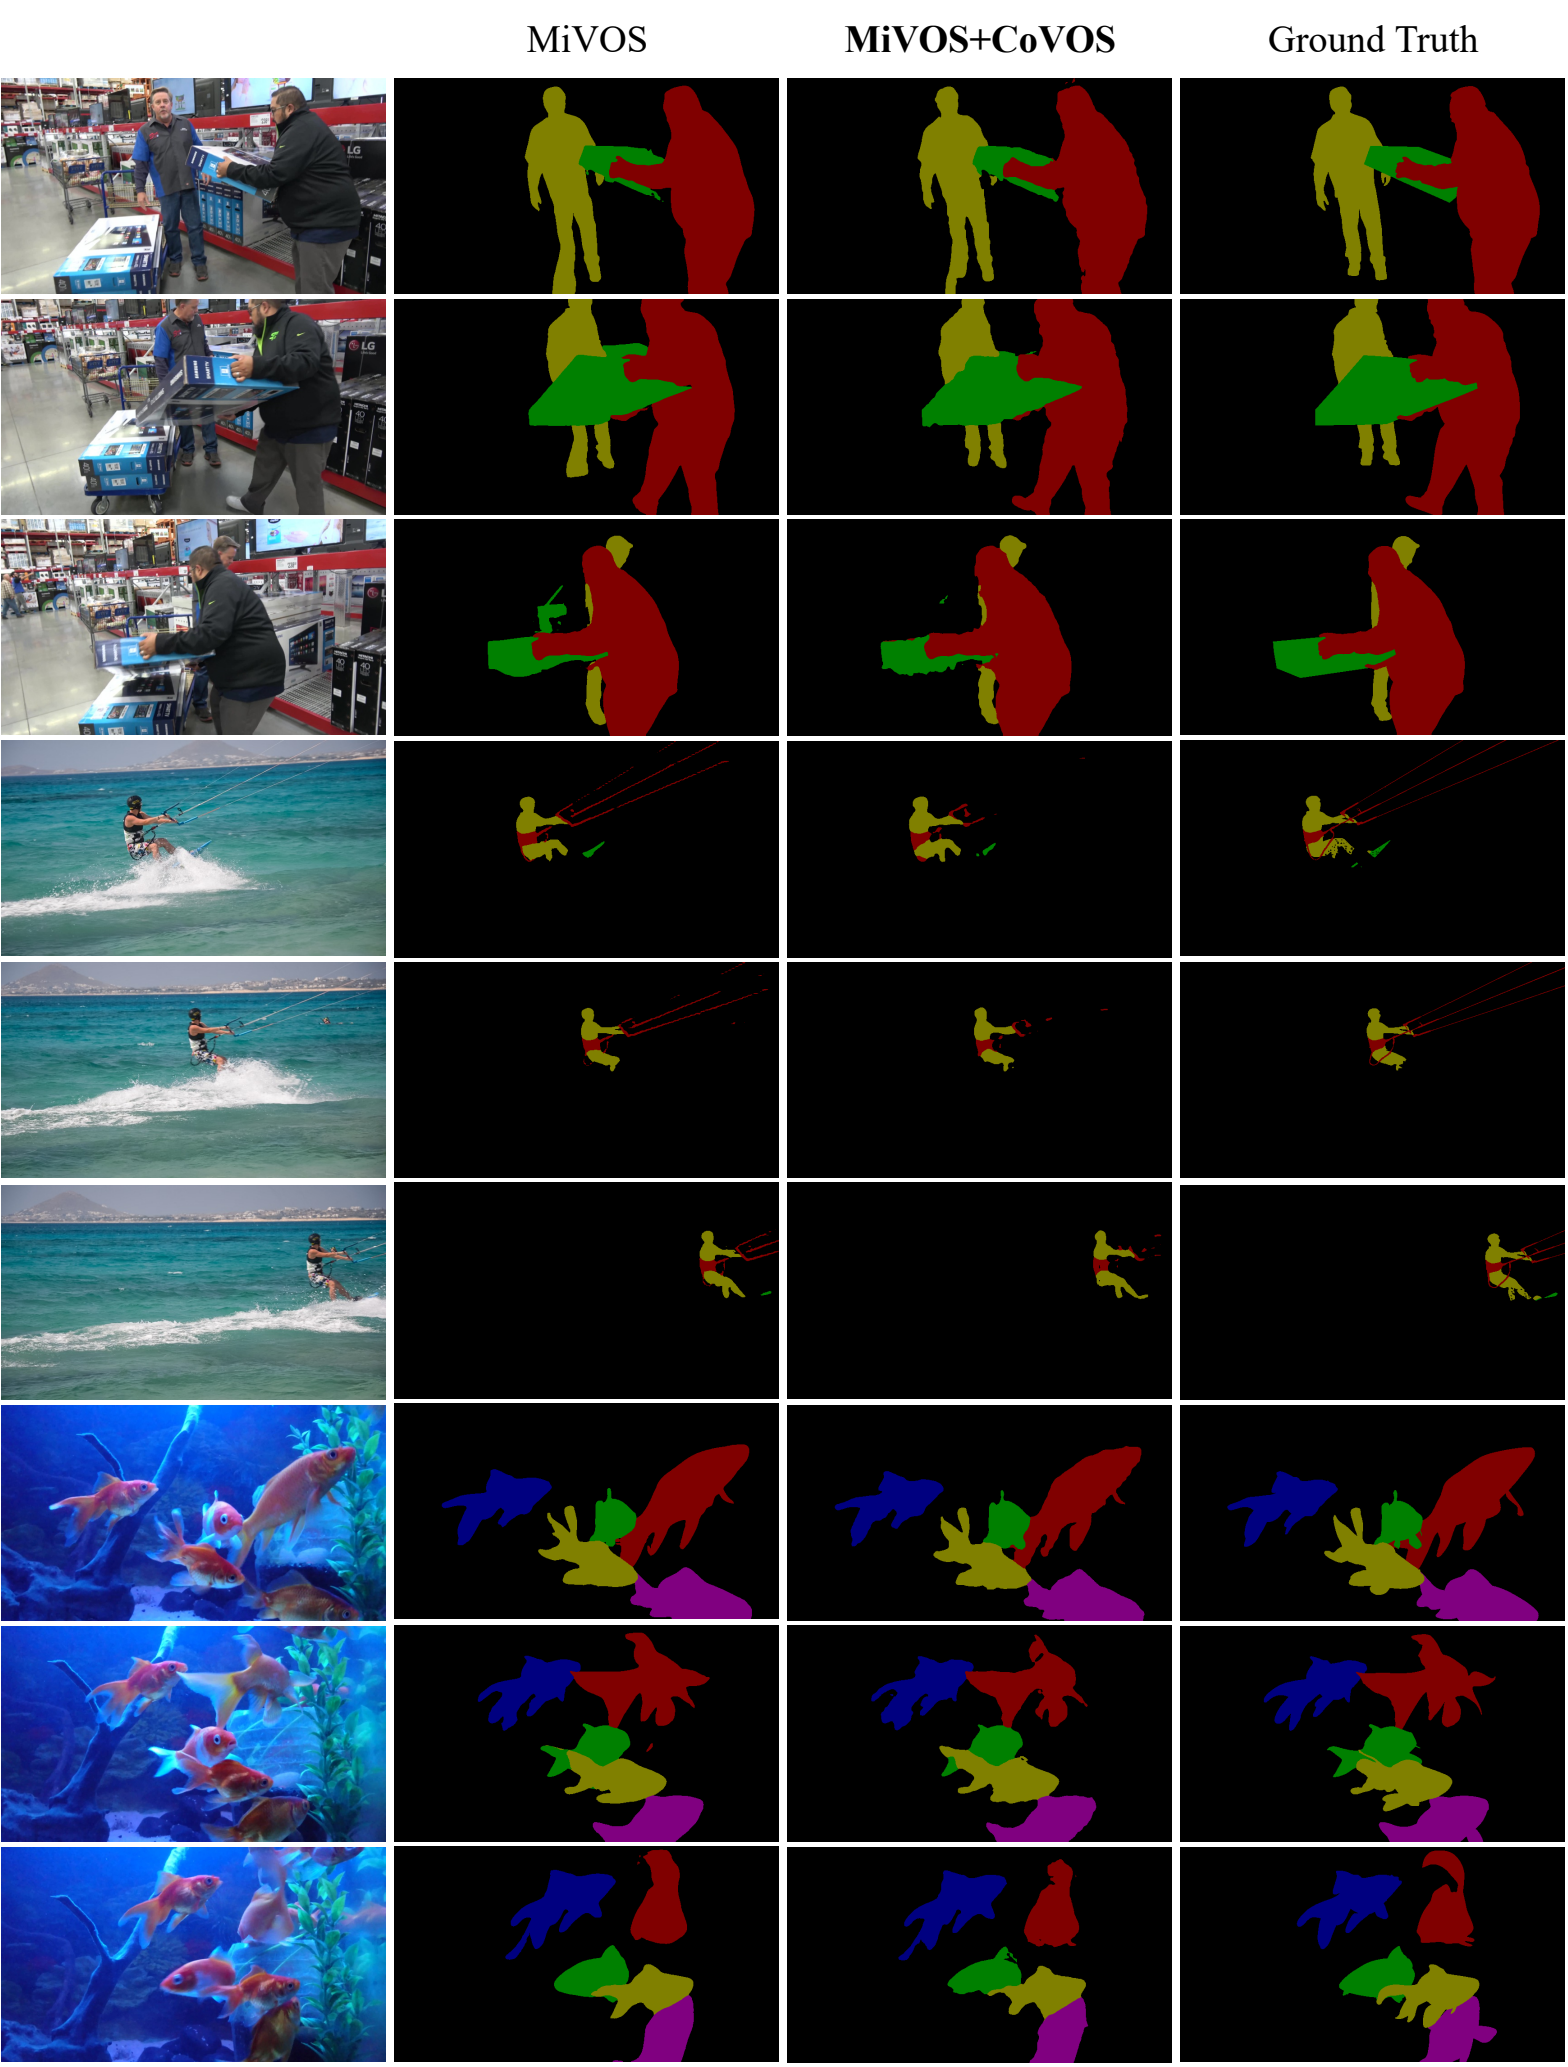    | 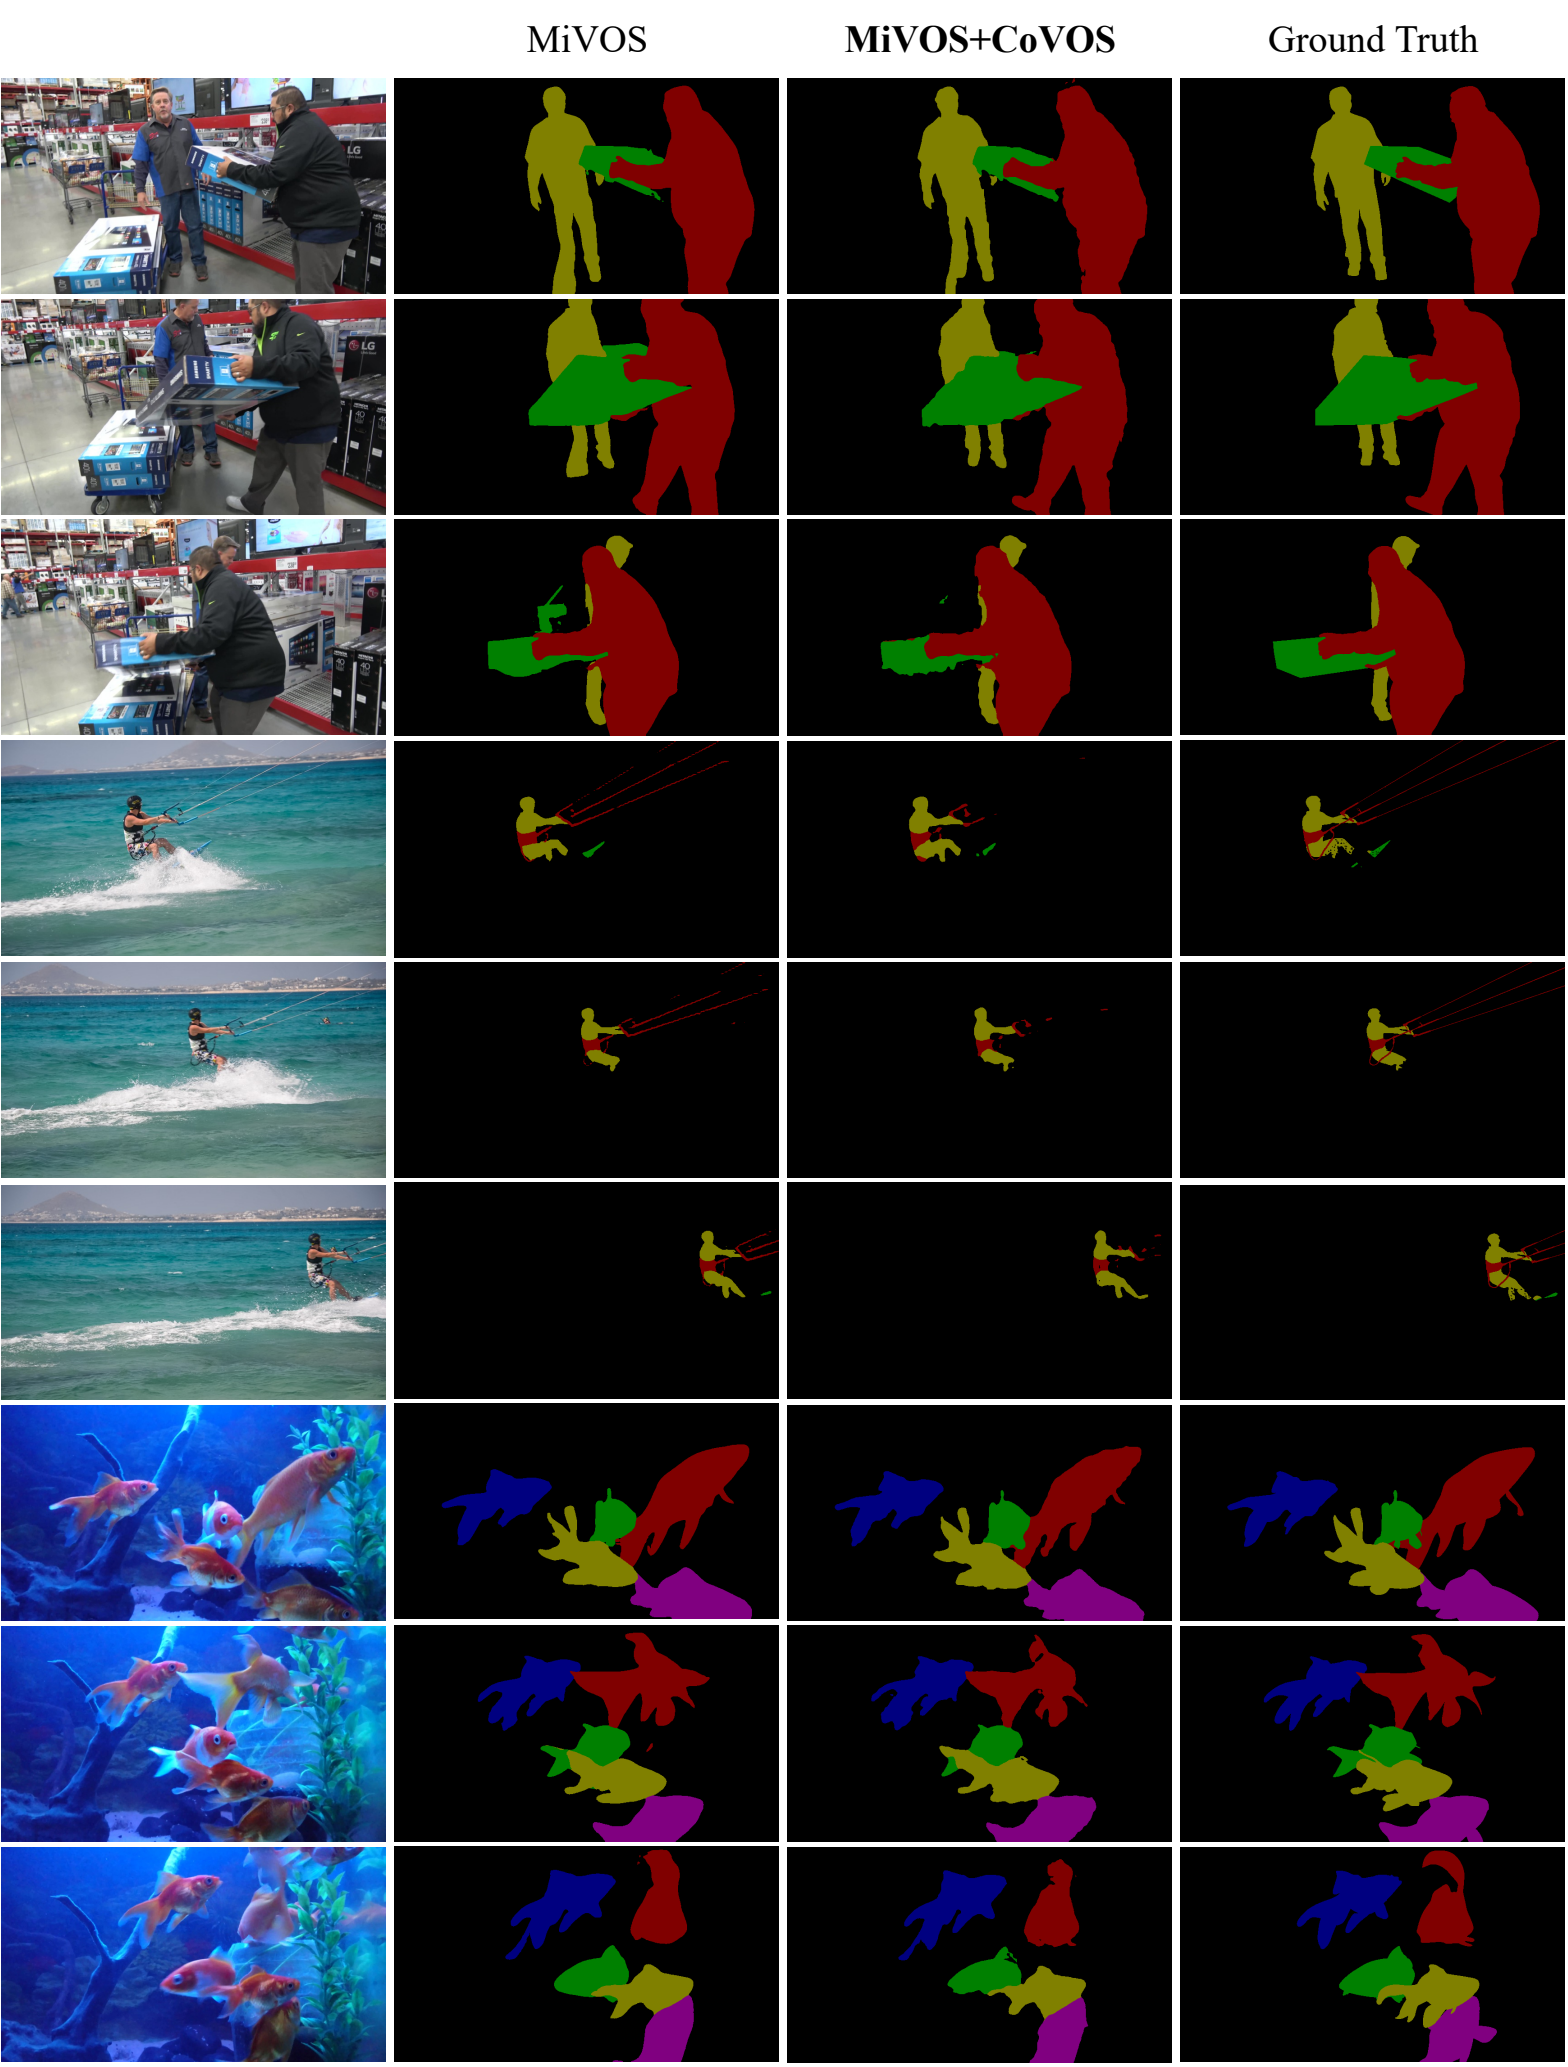    | 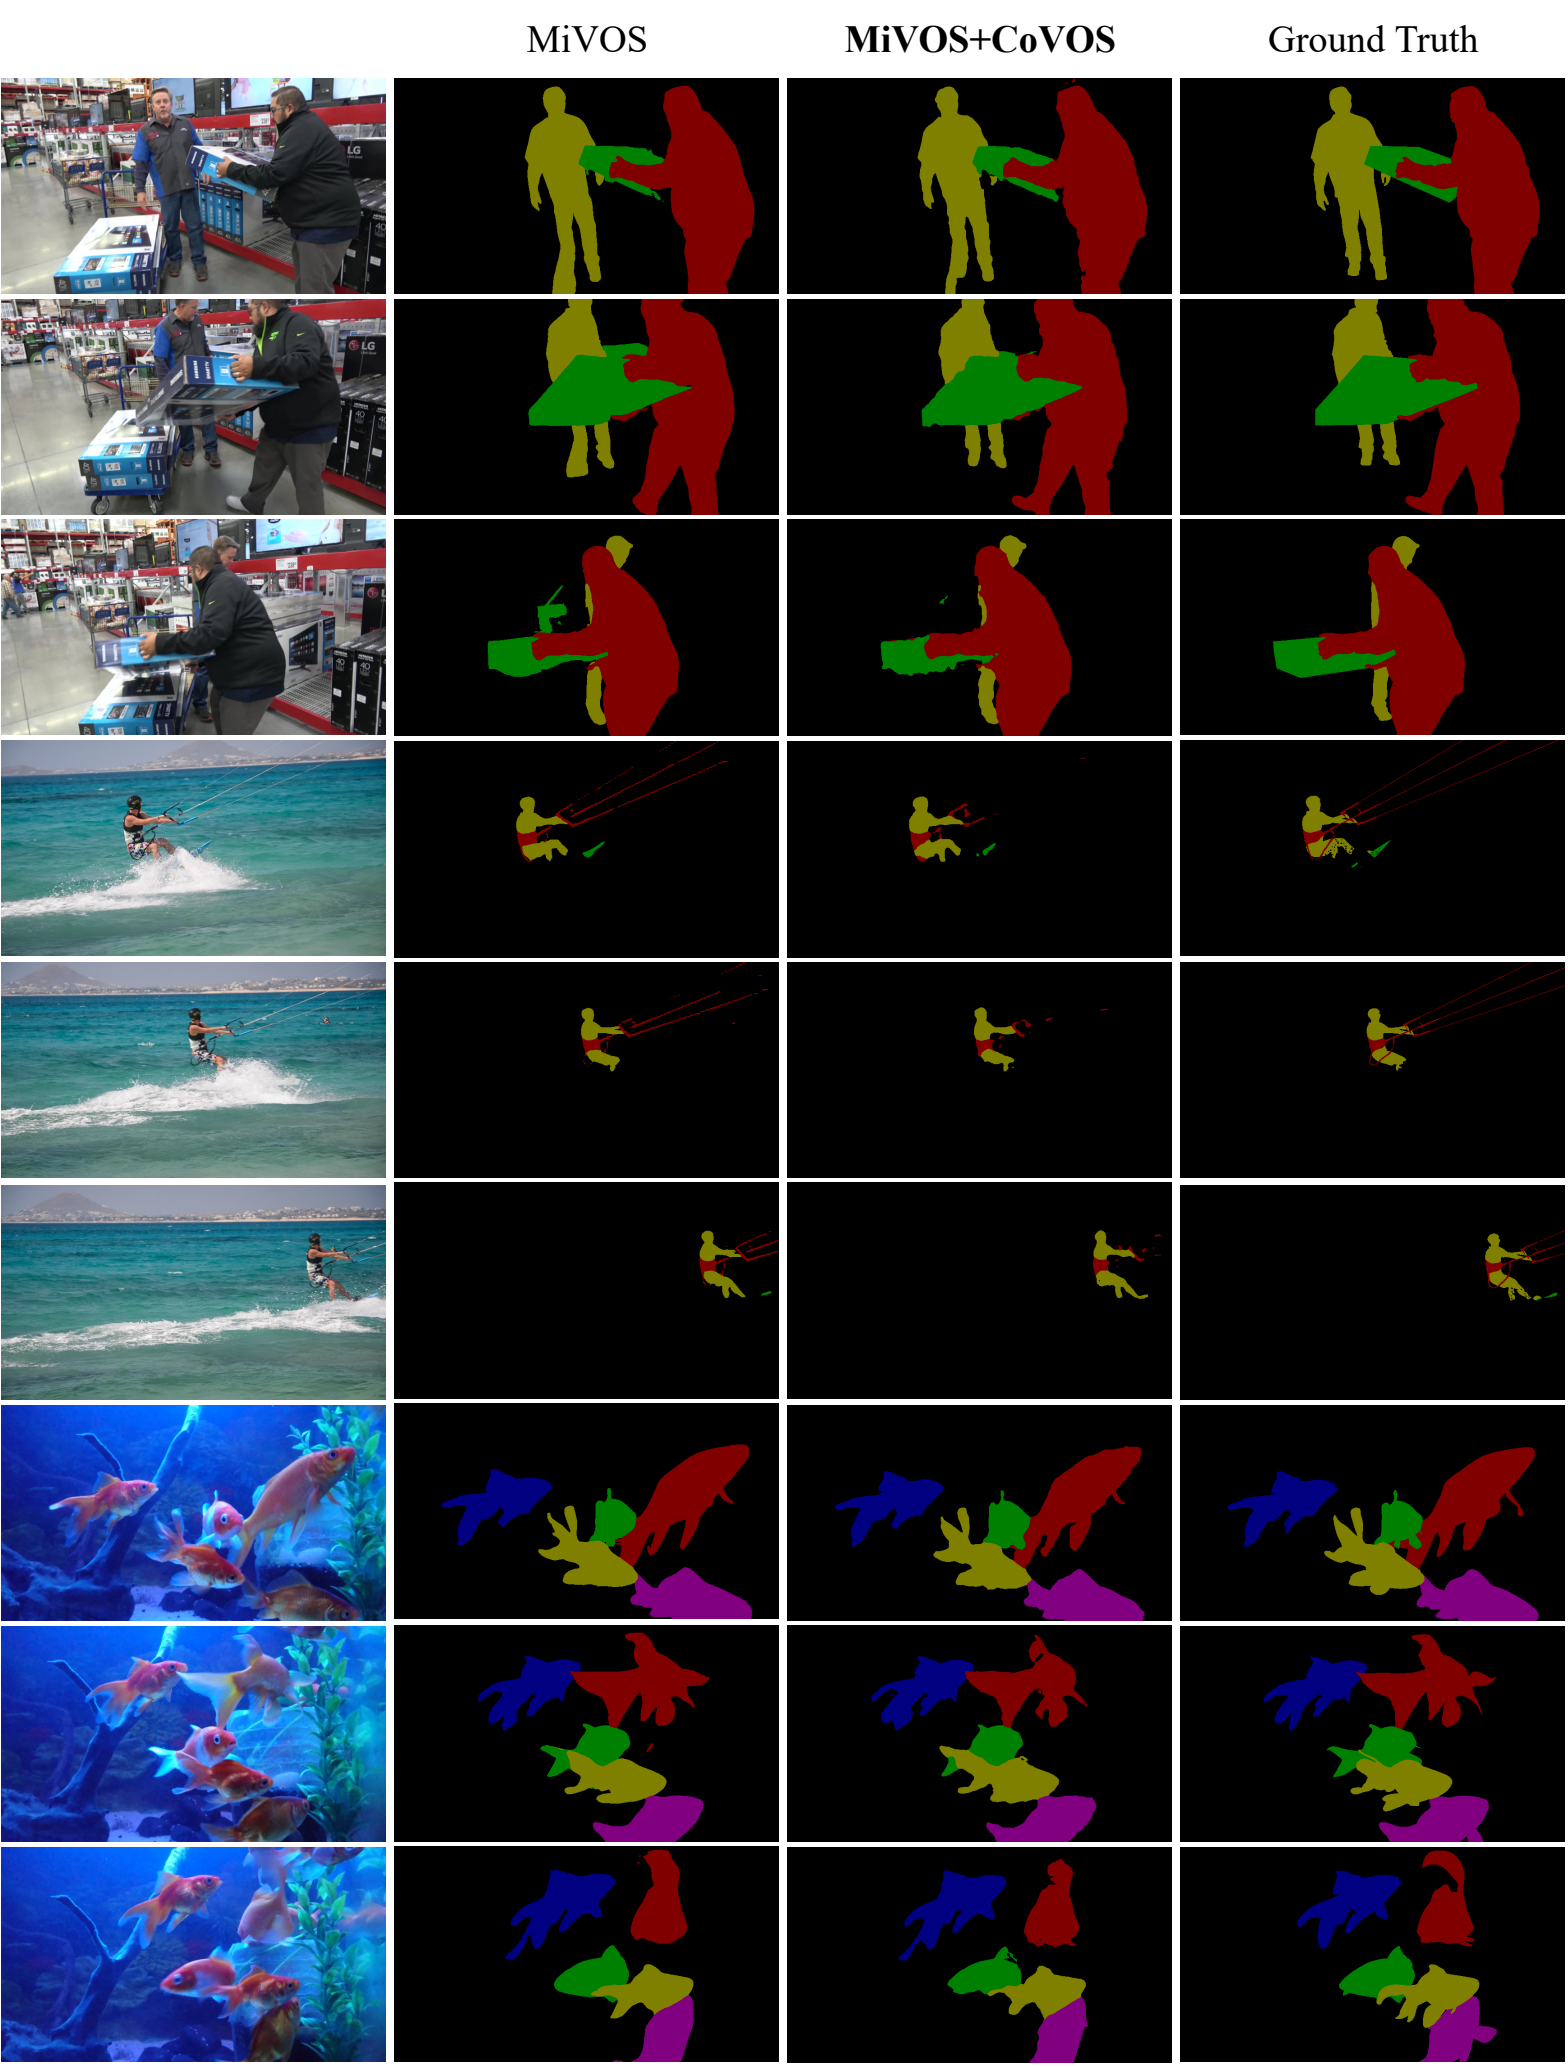    | 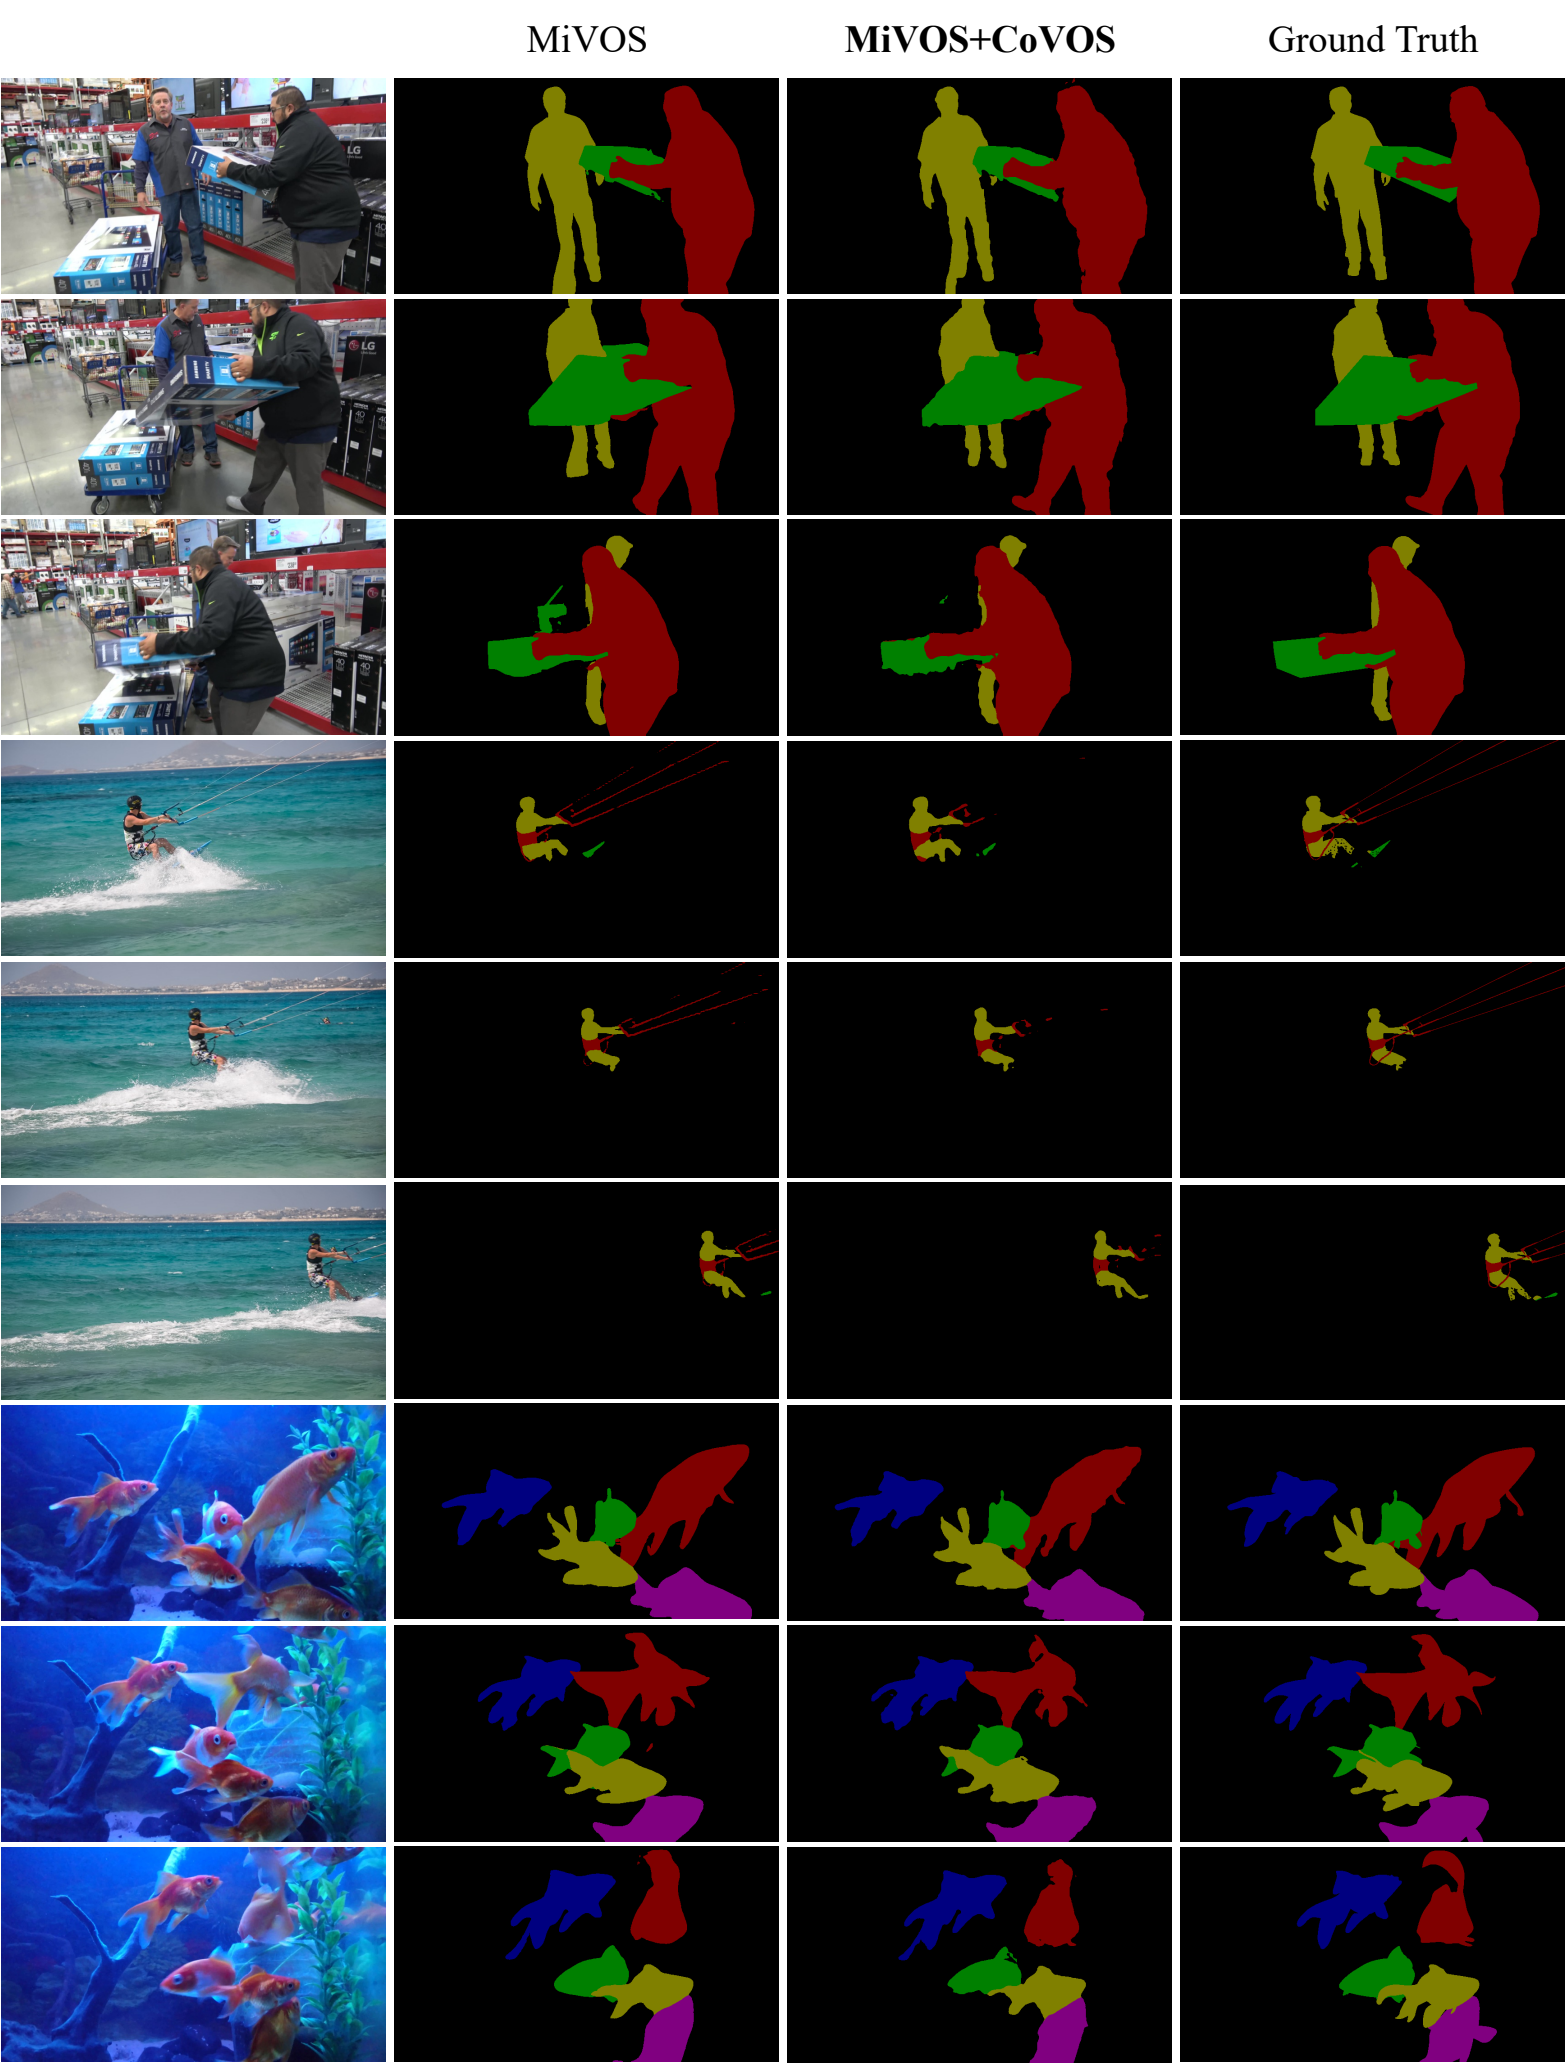    |
| 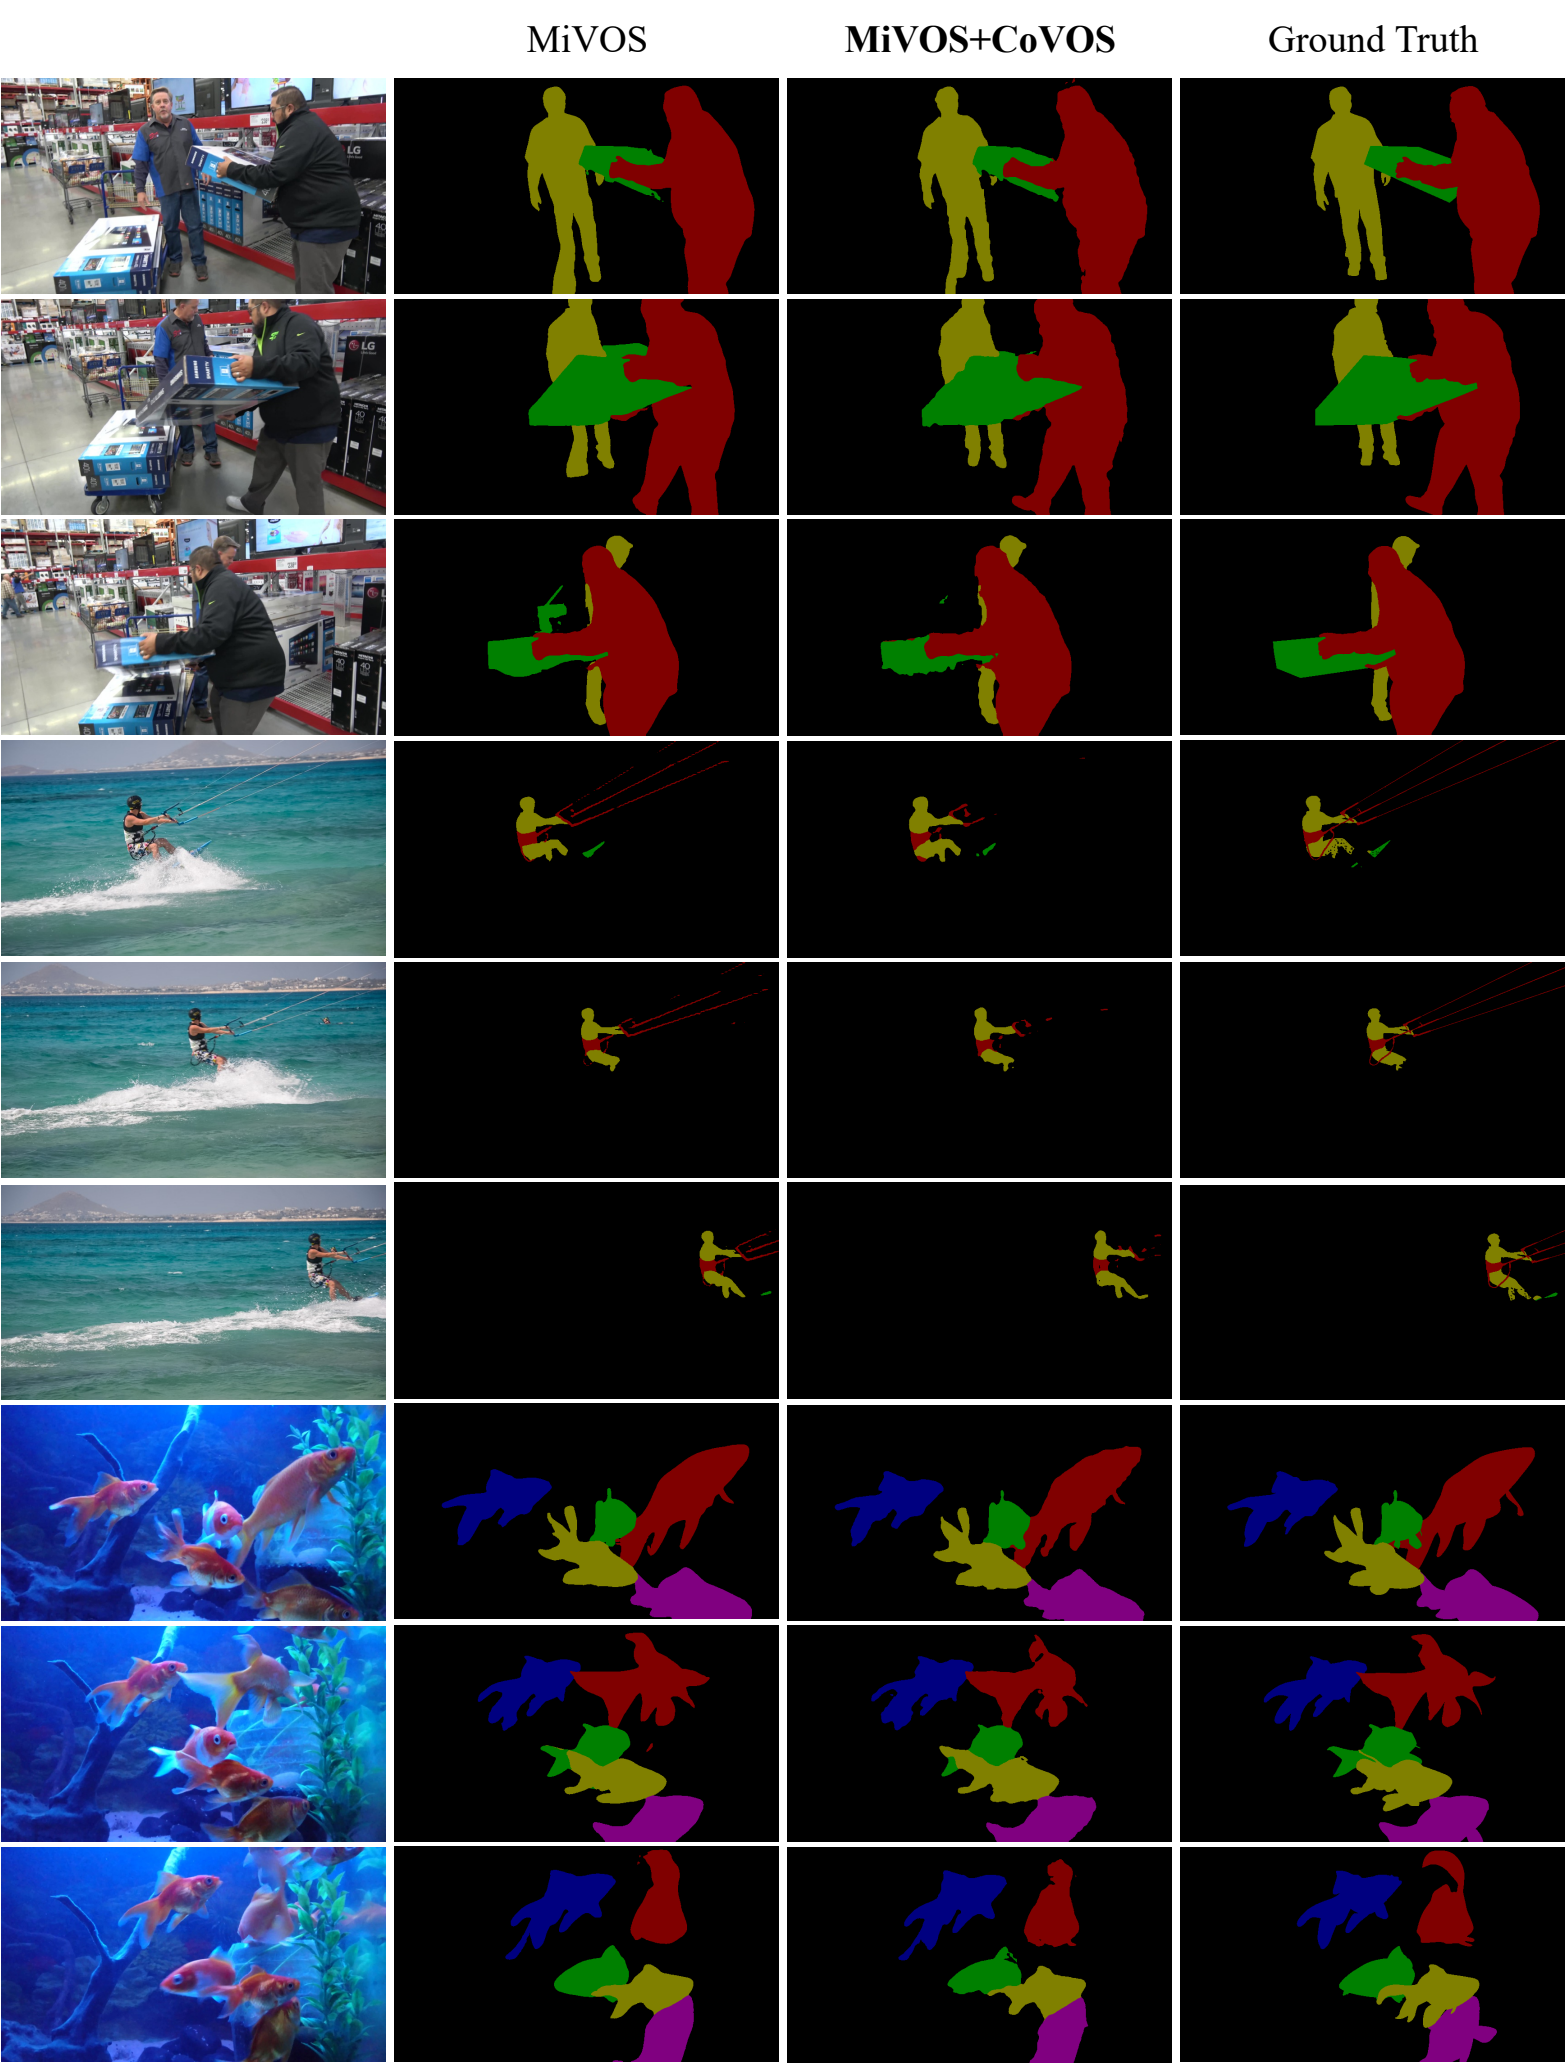   | 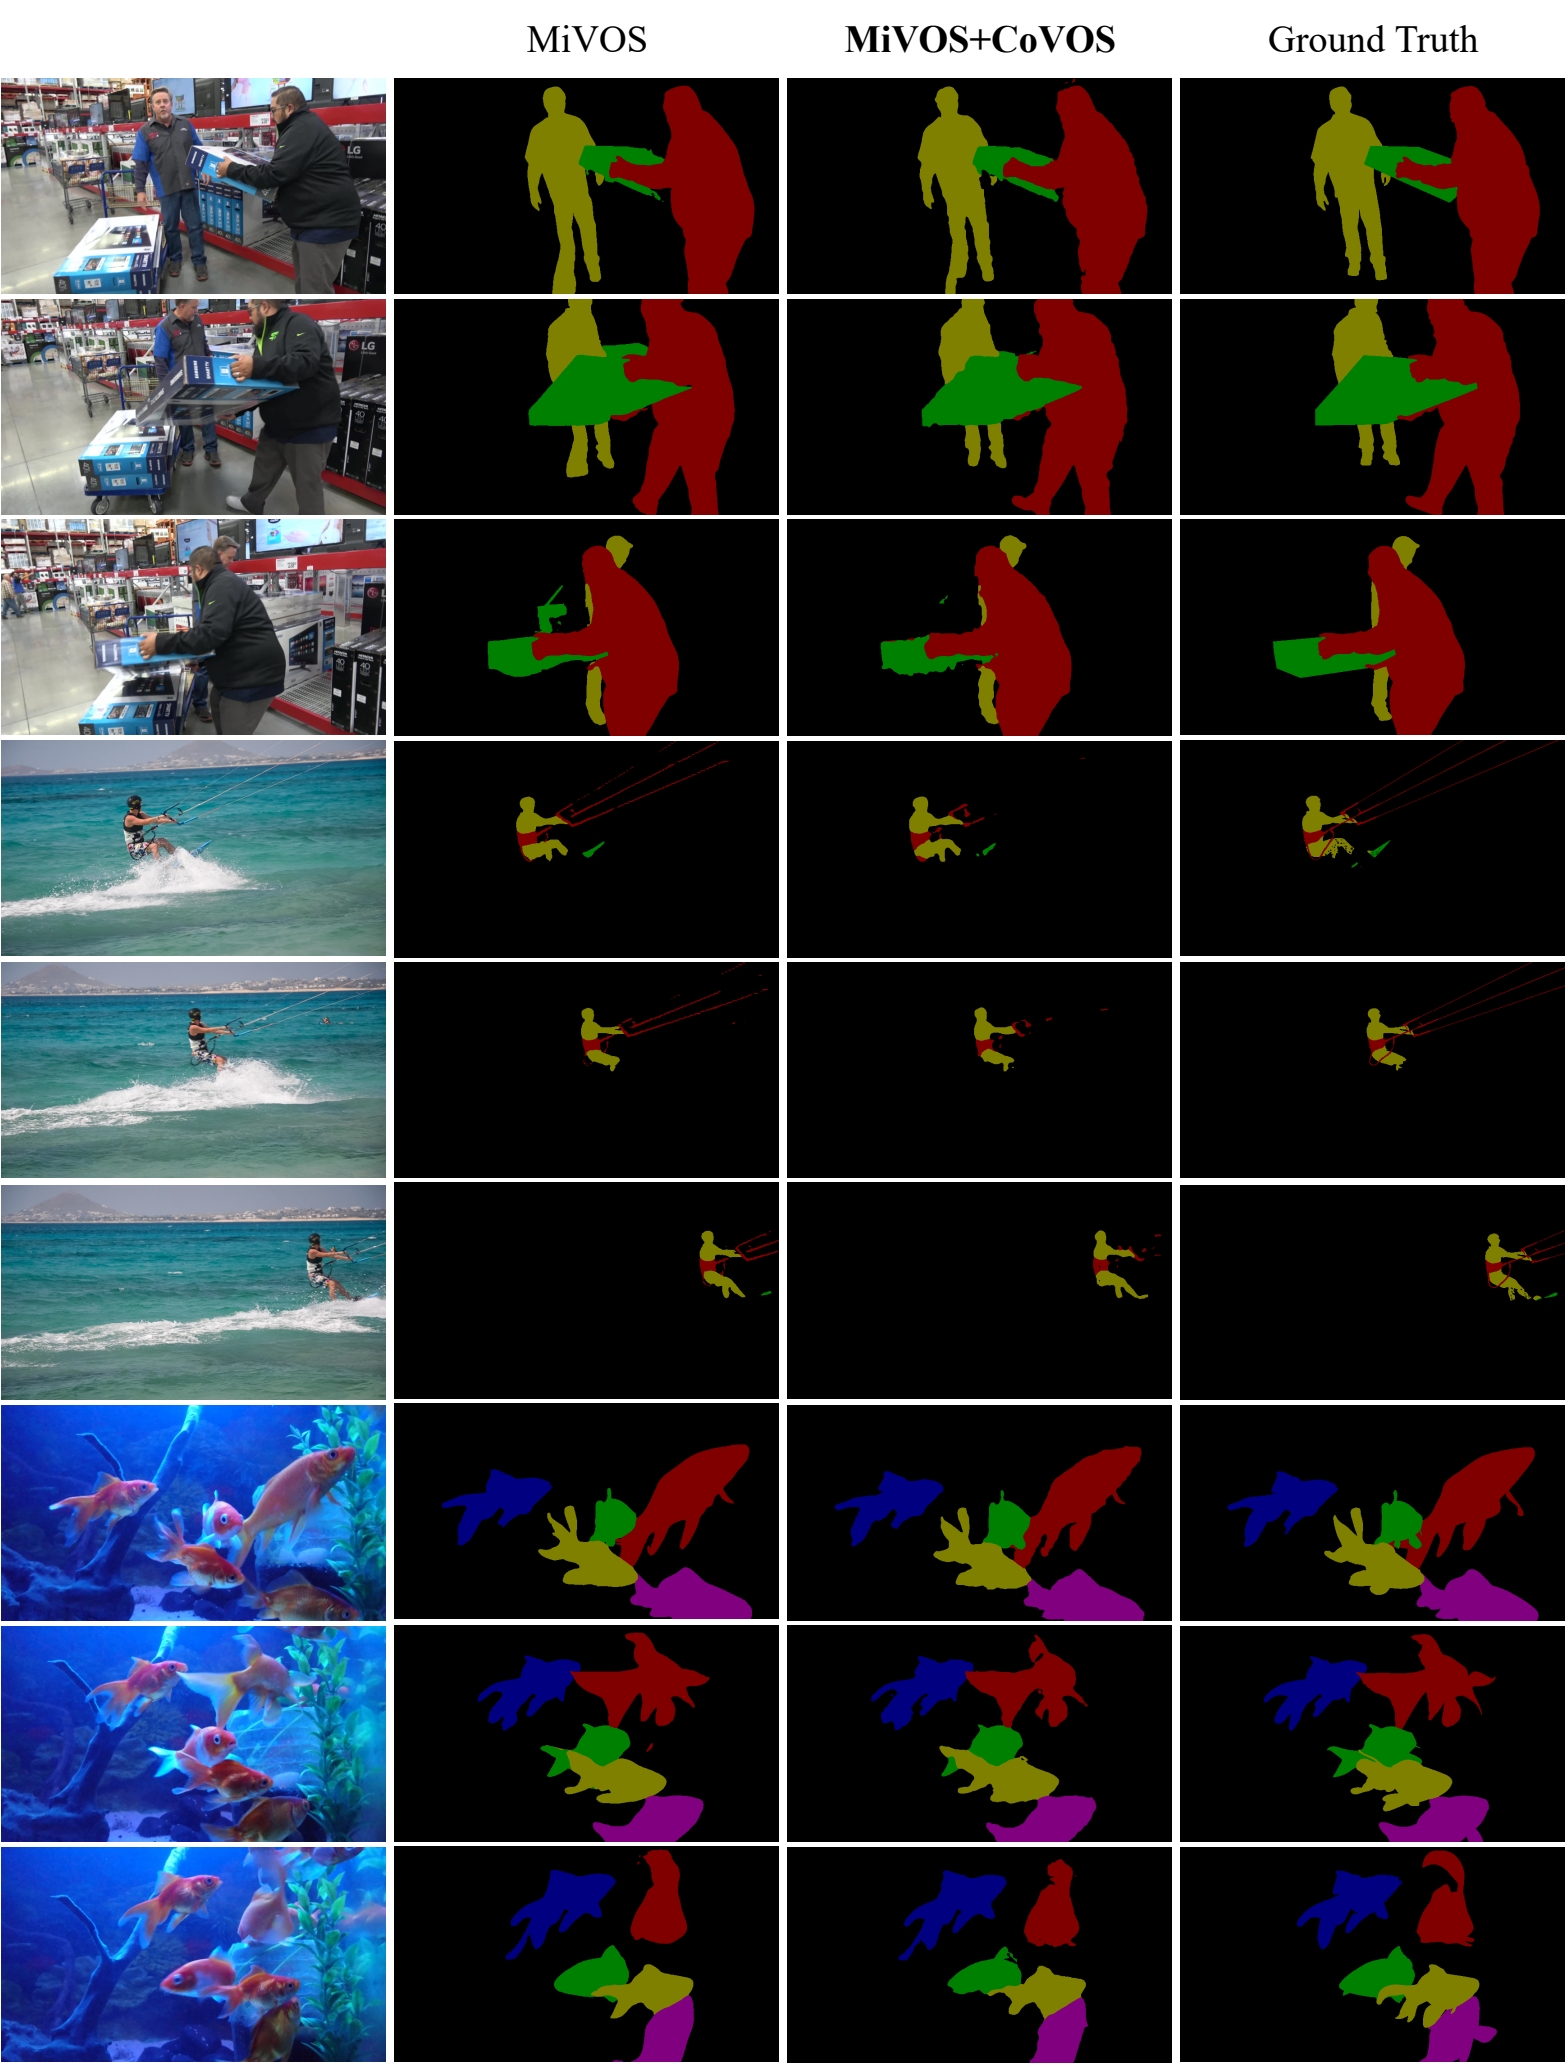   | 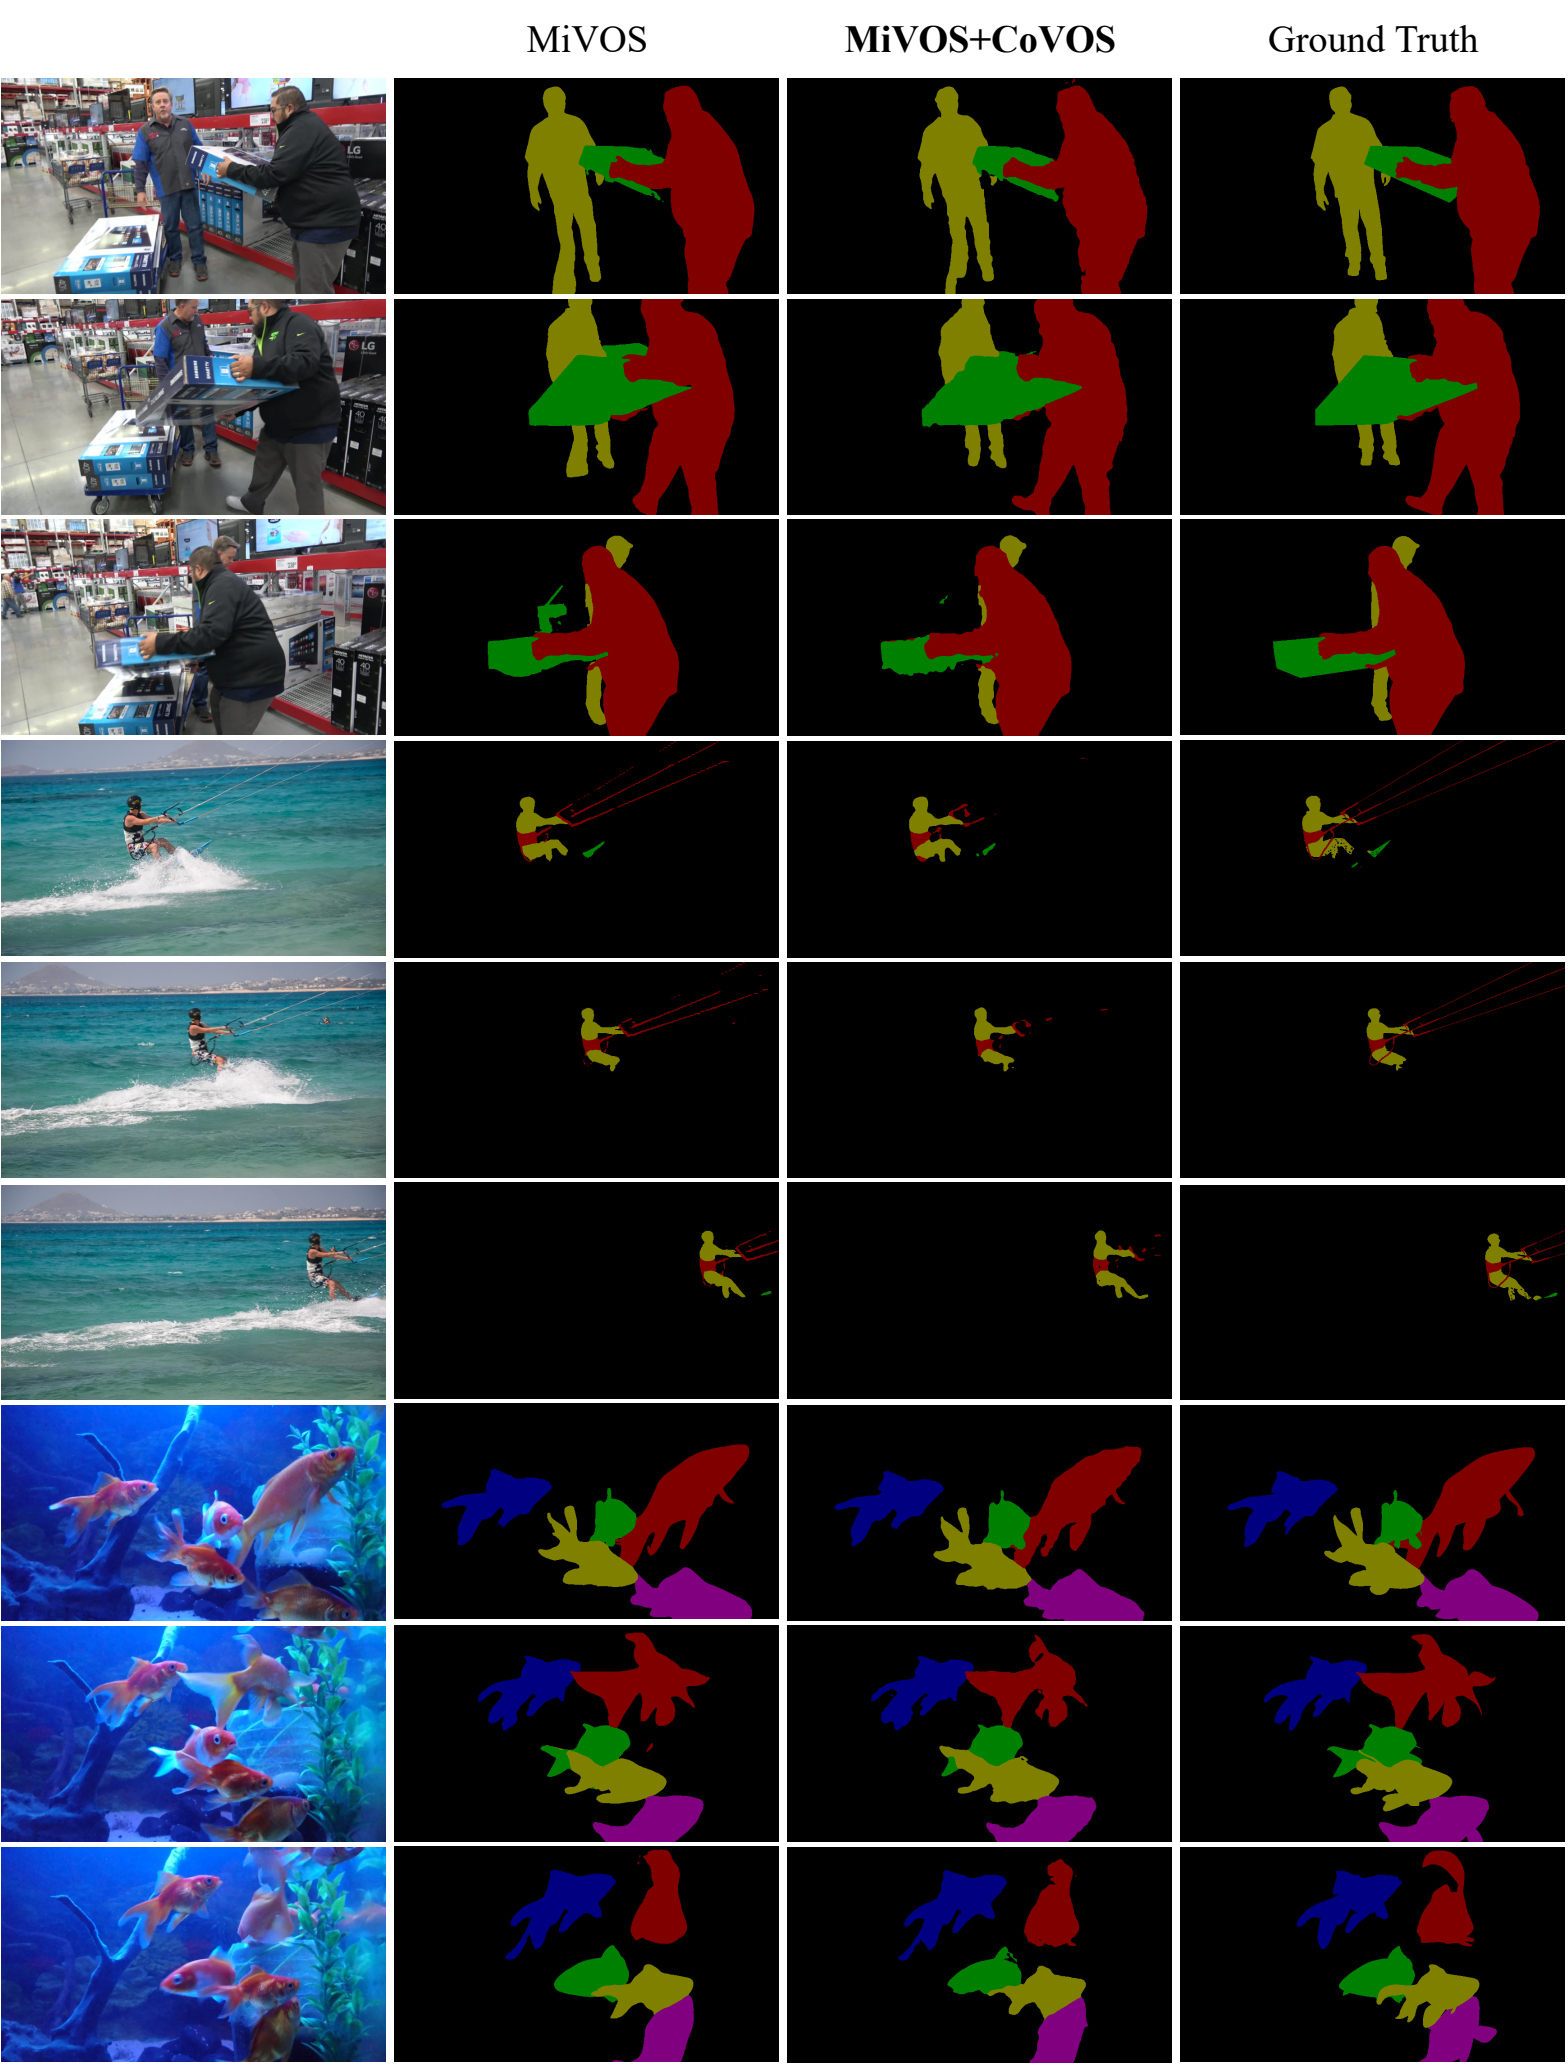   | 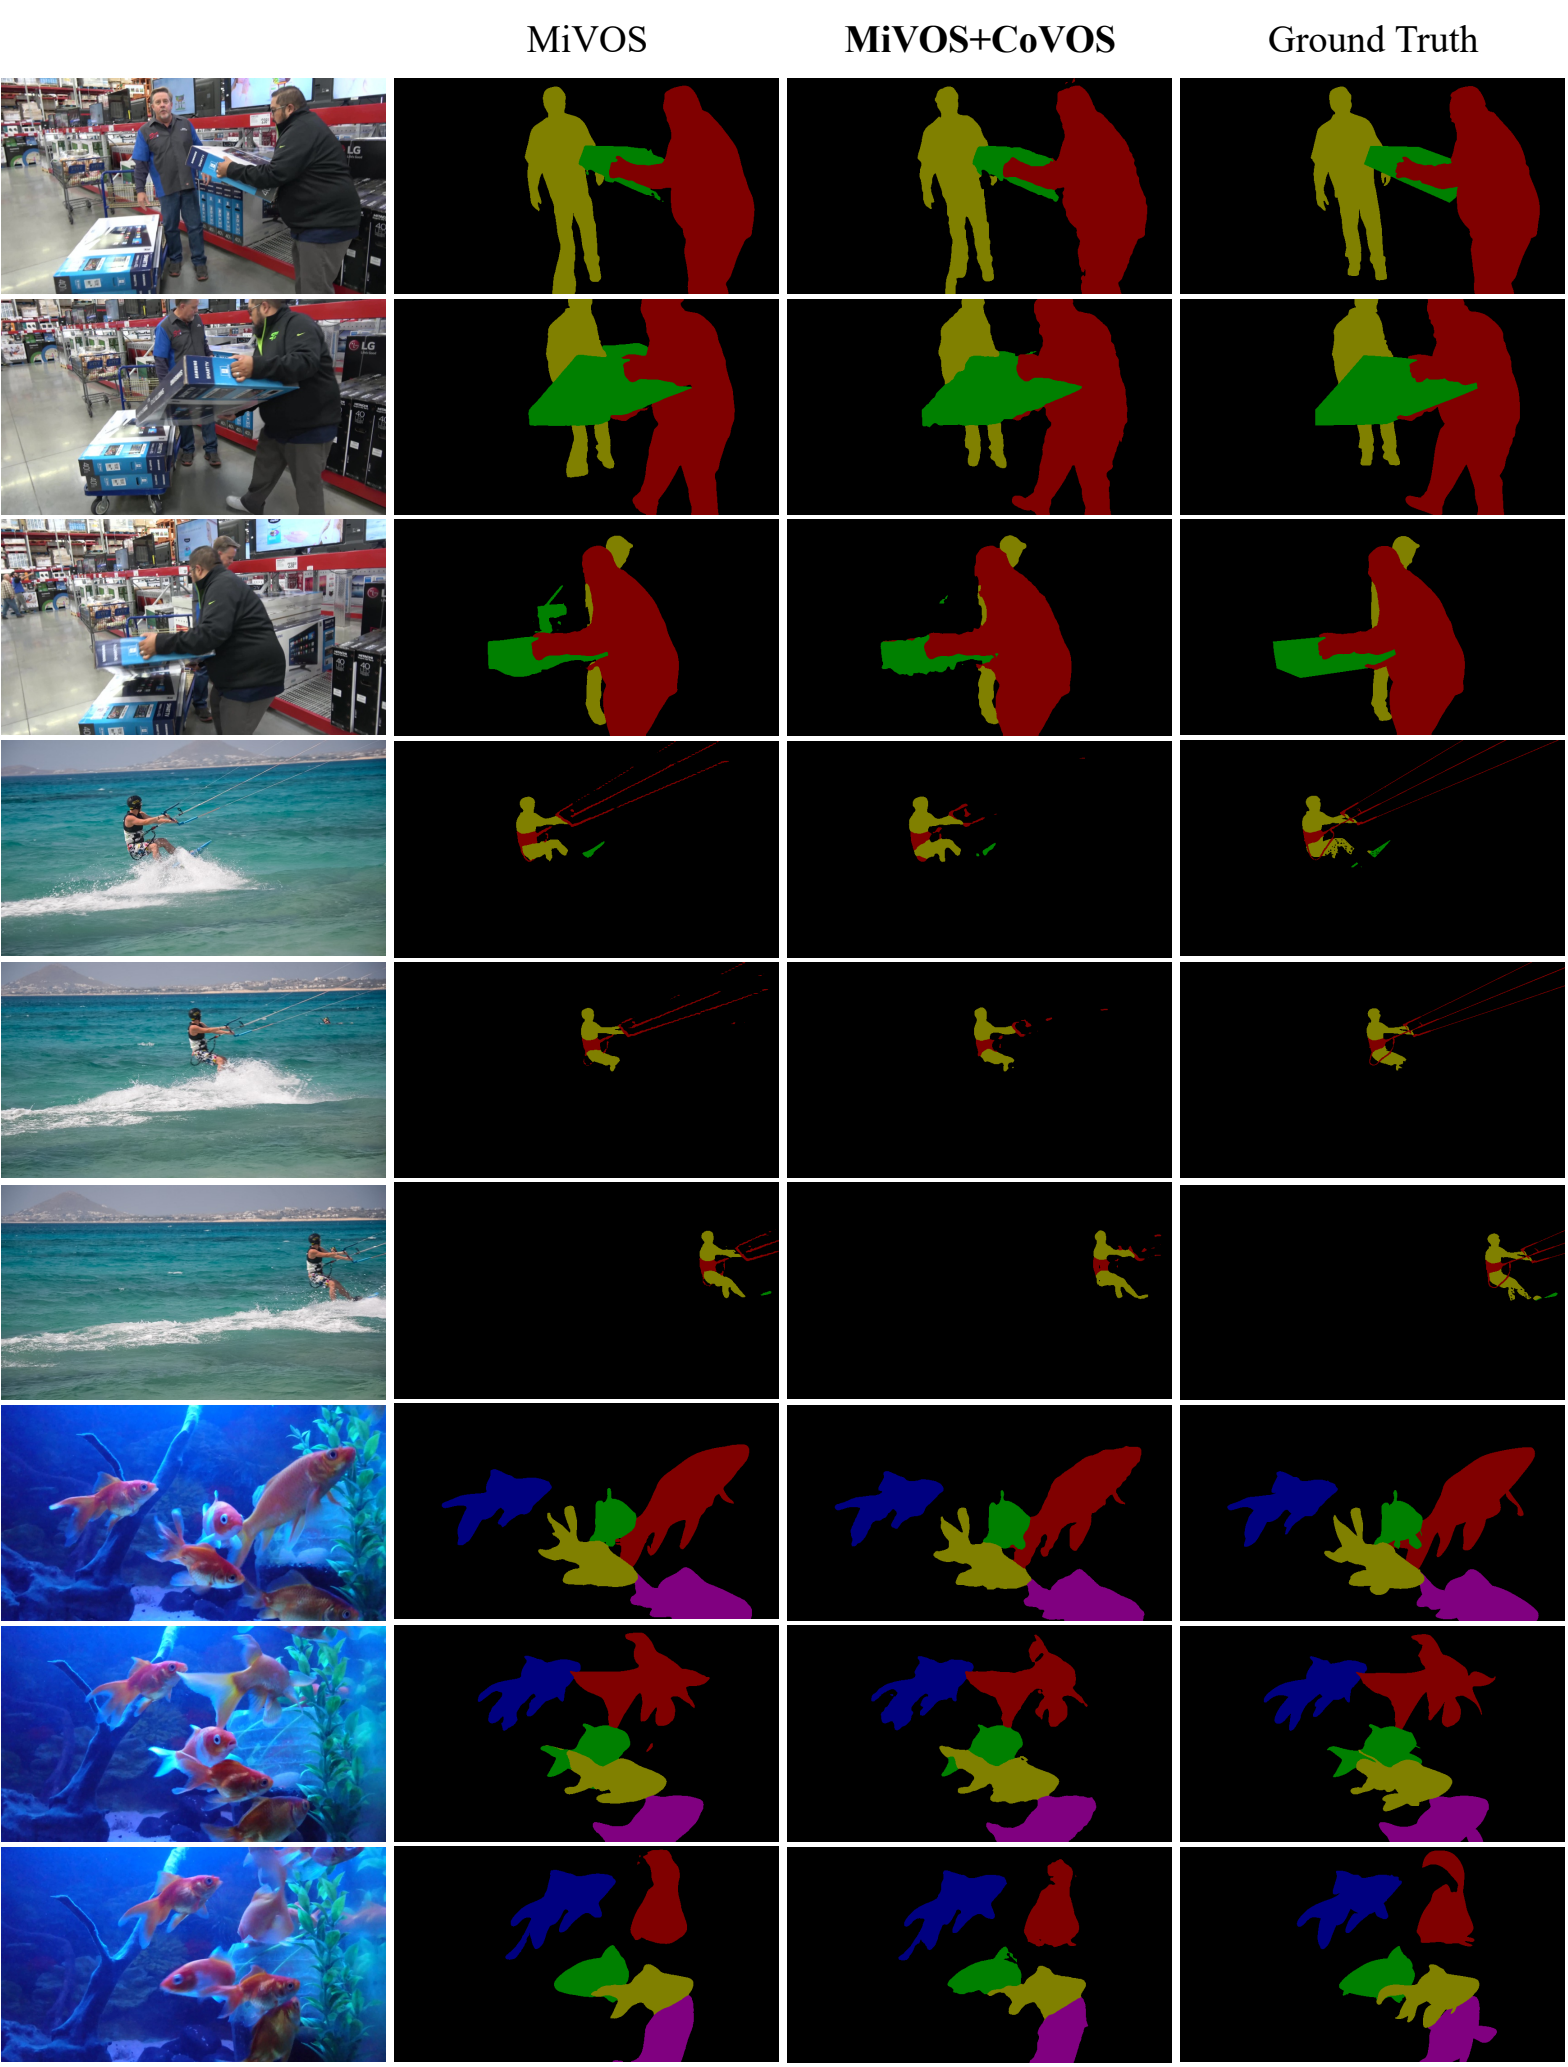   |
| 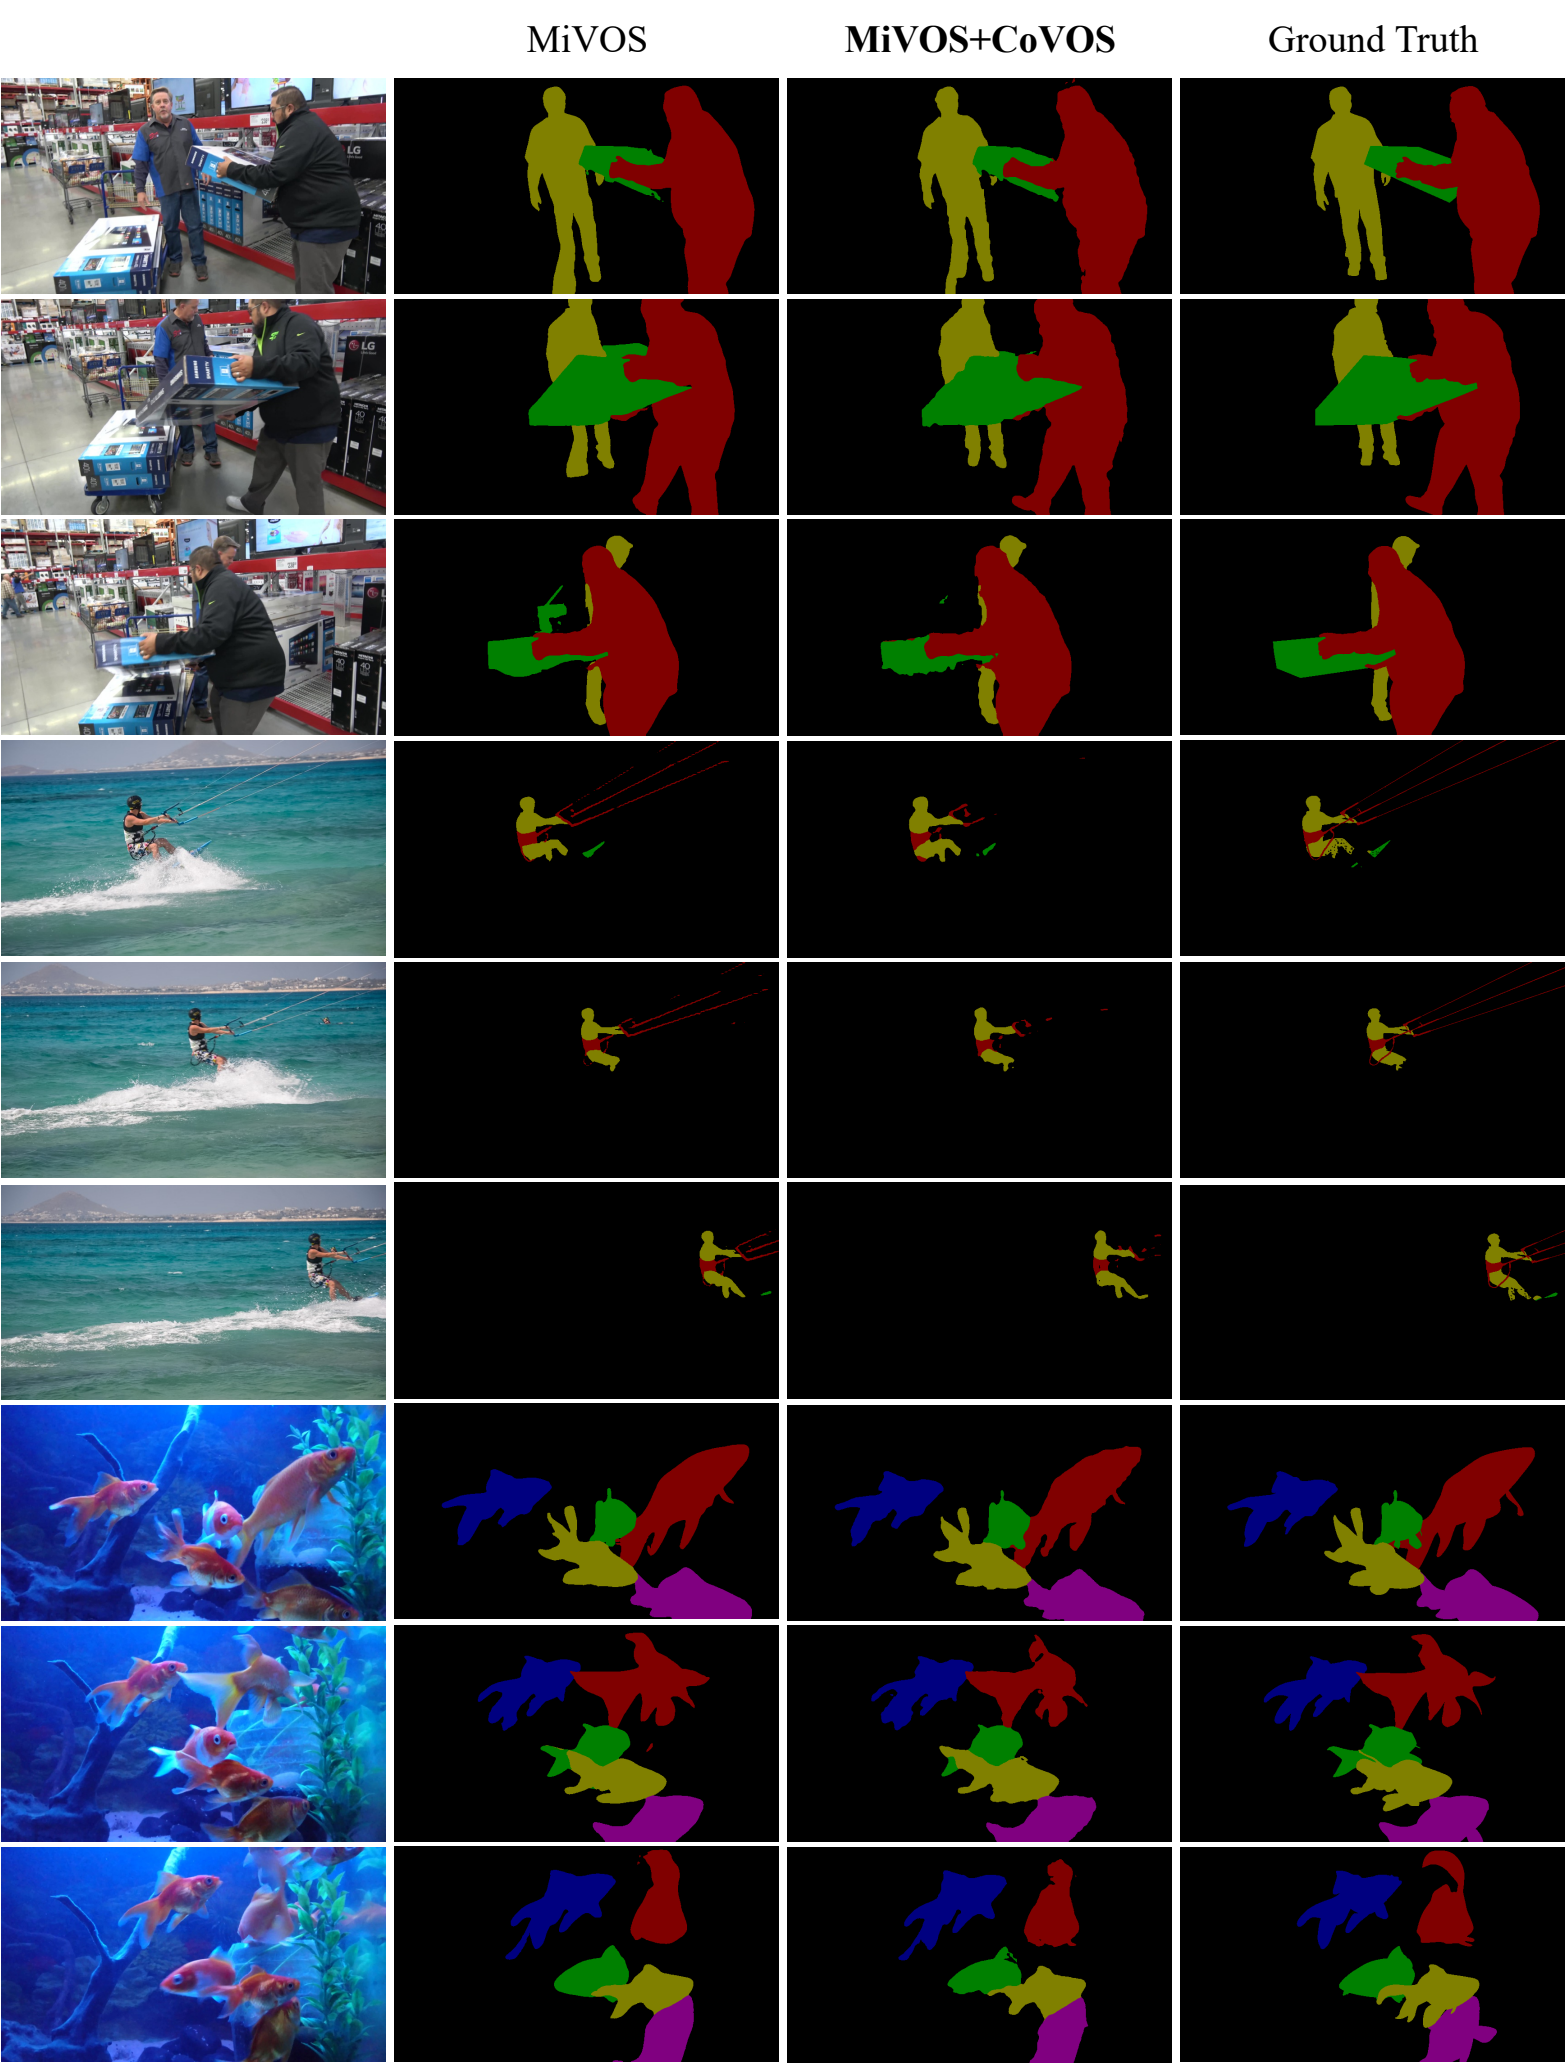   | 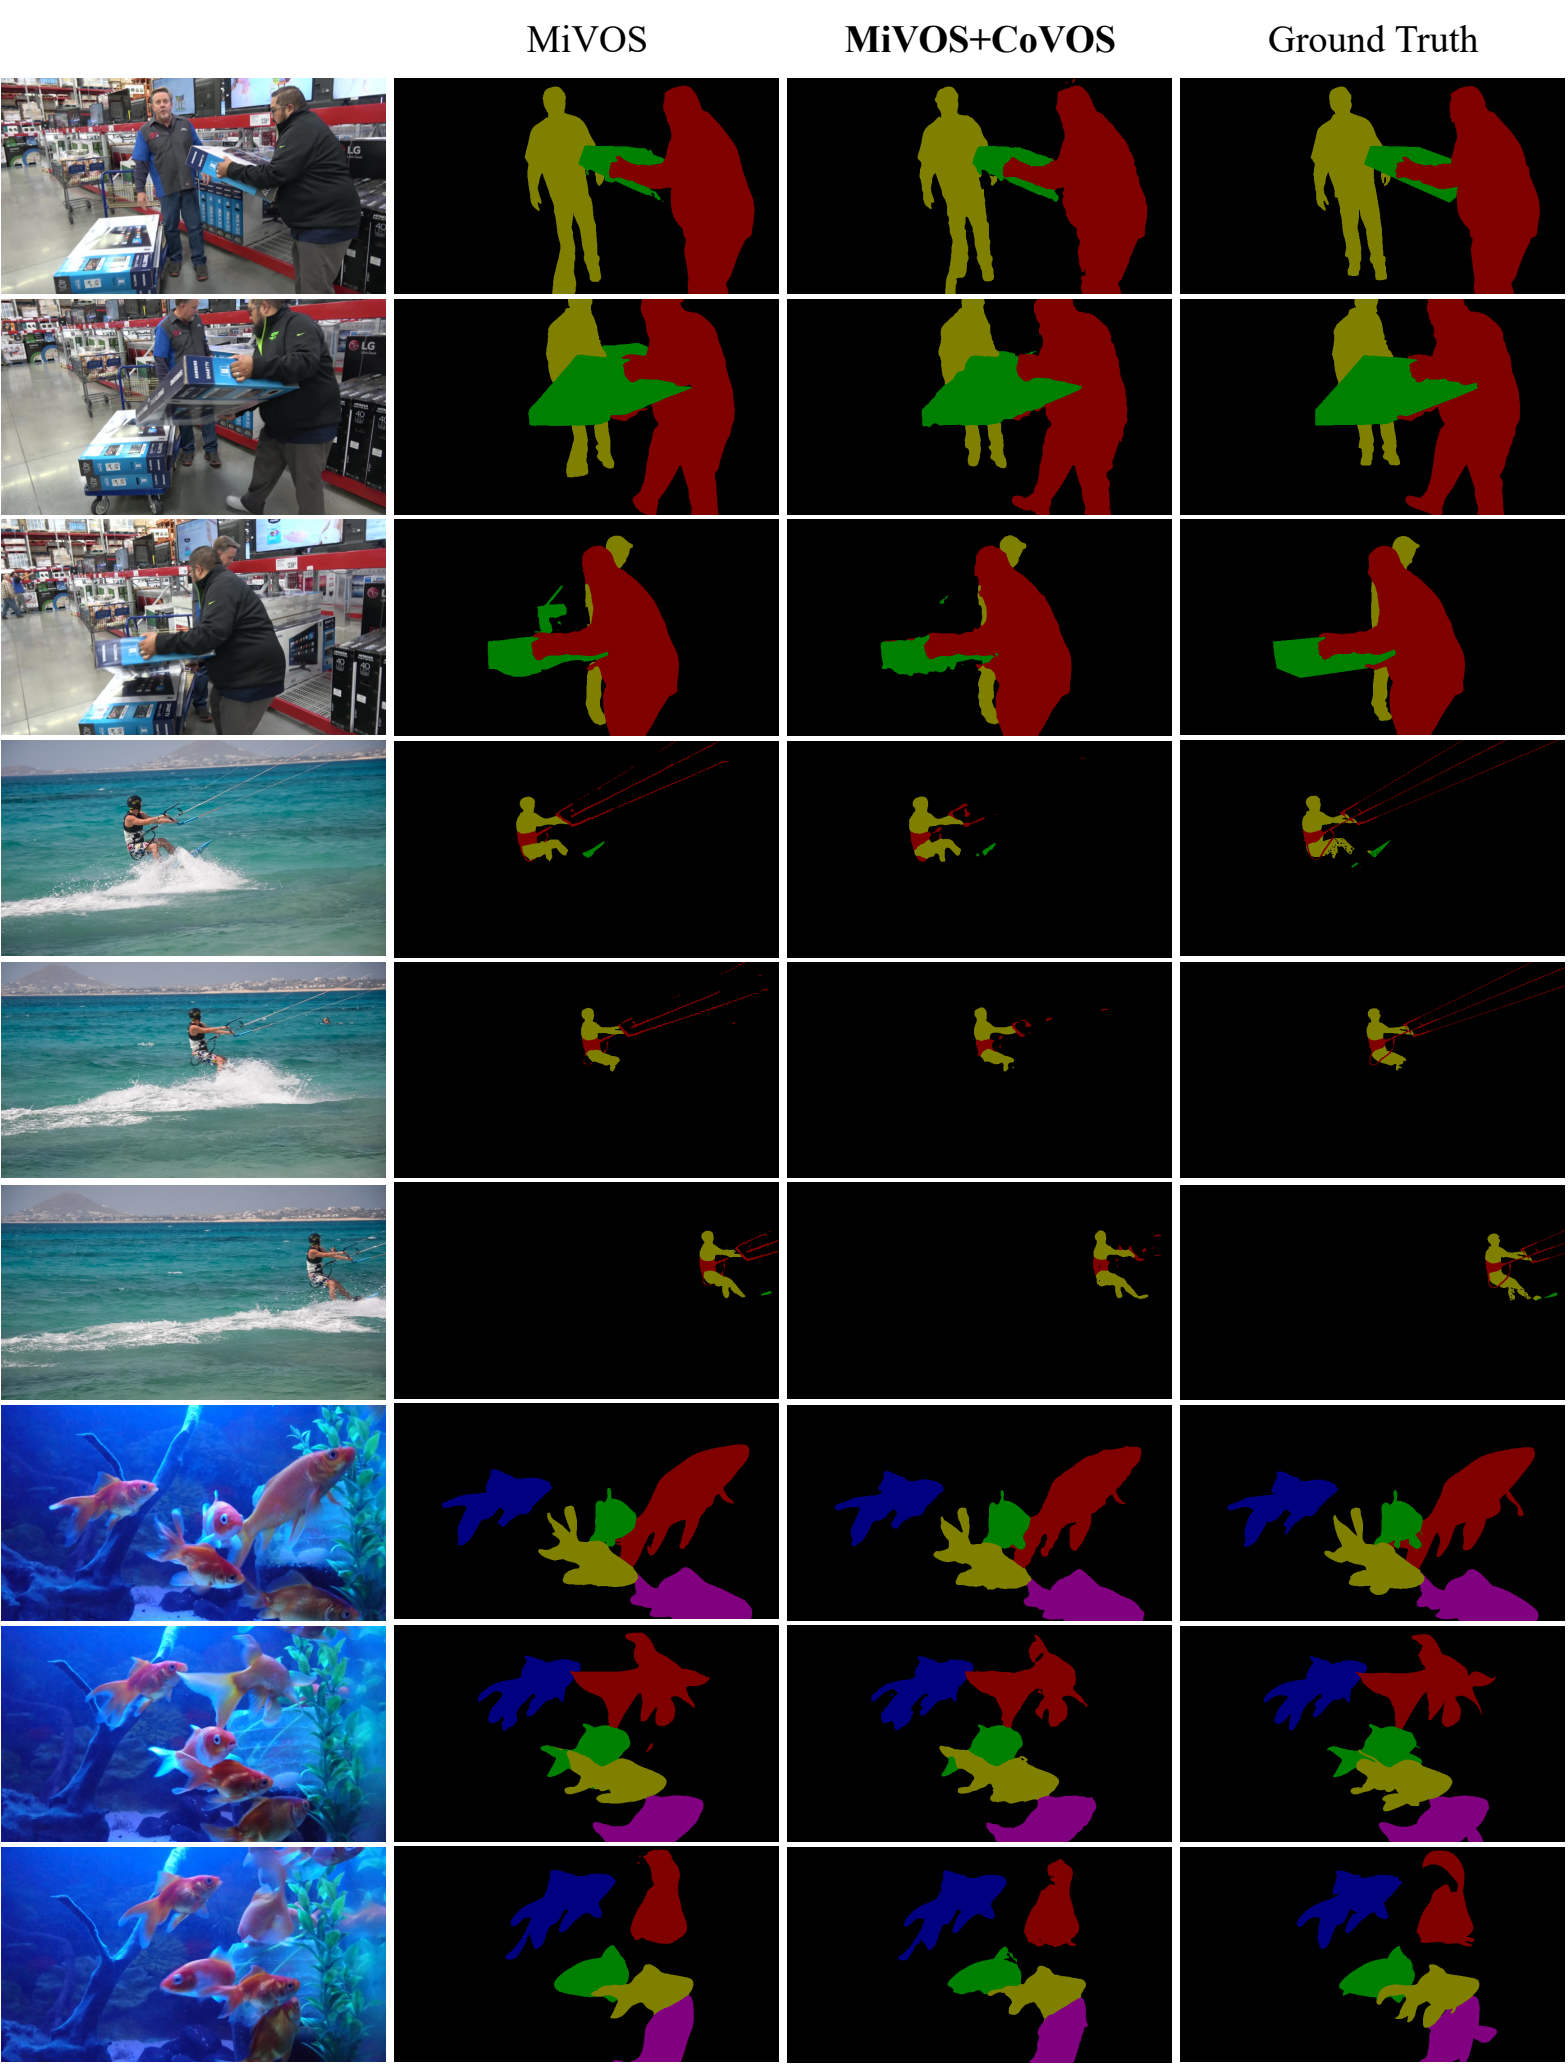   | 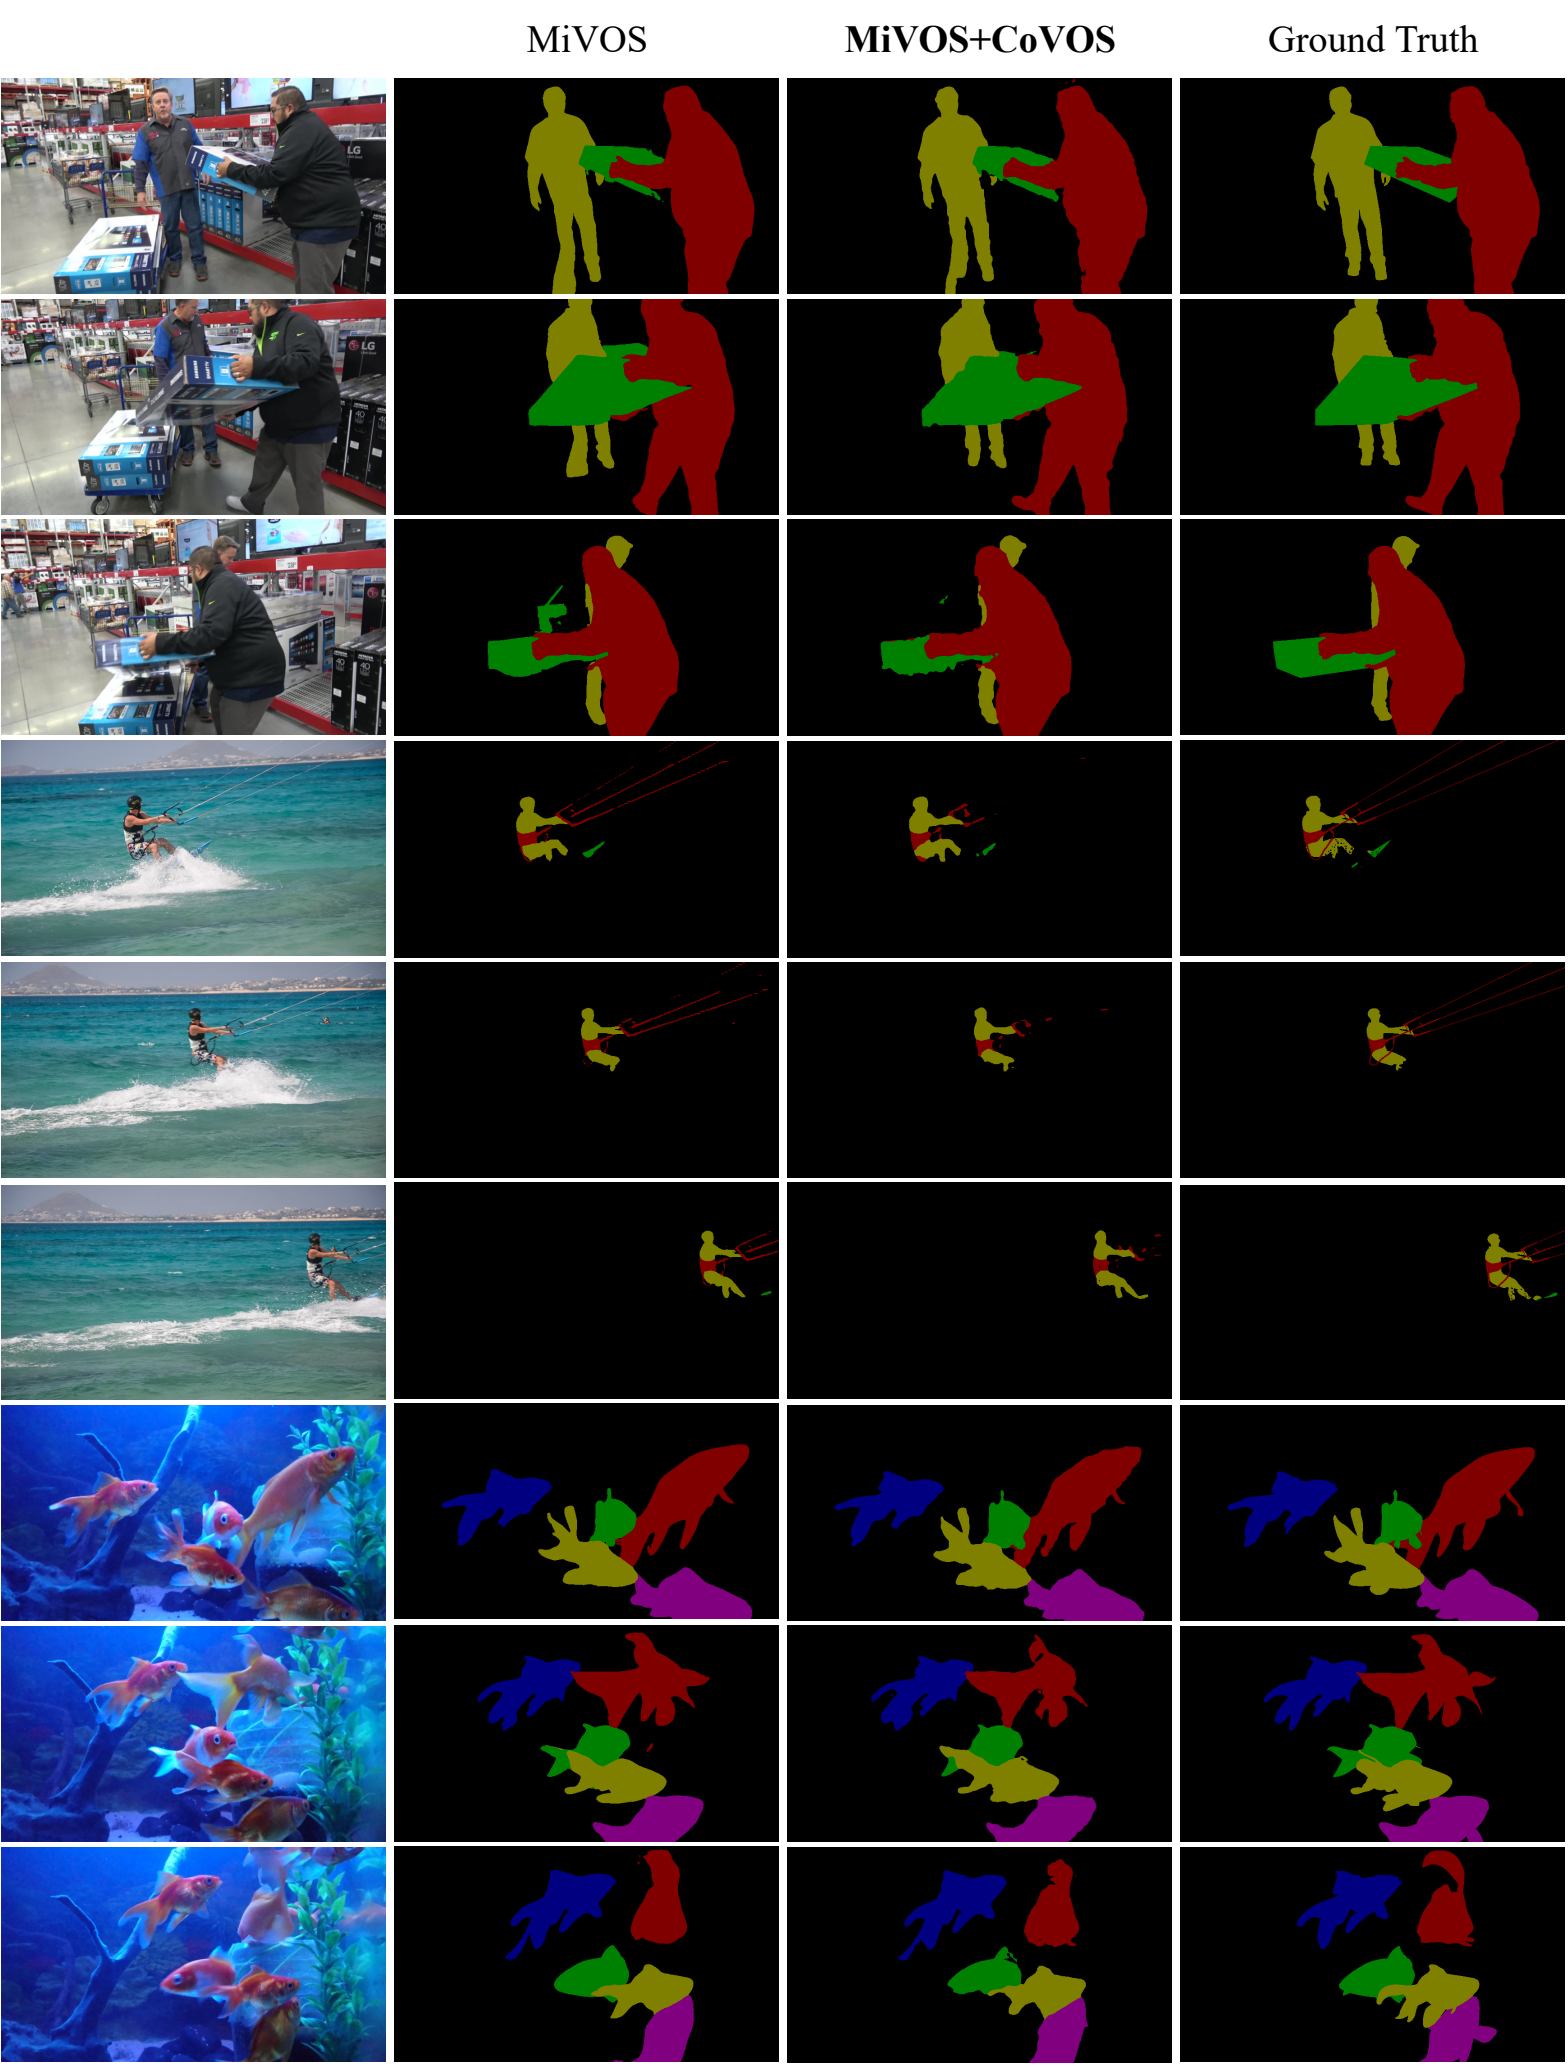   | 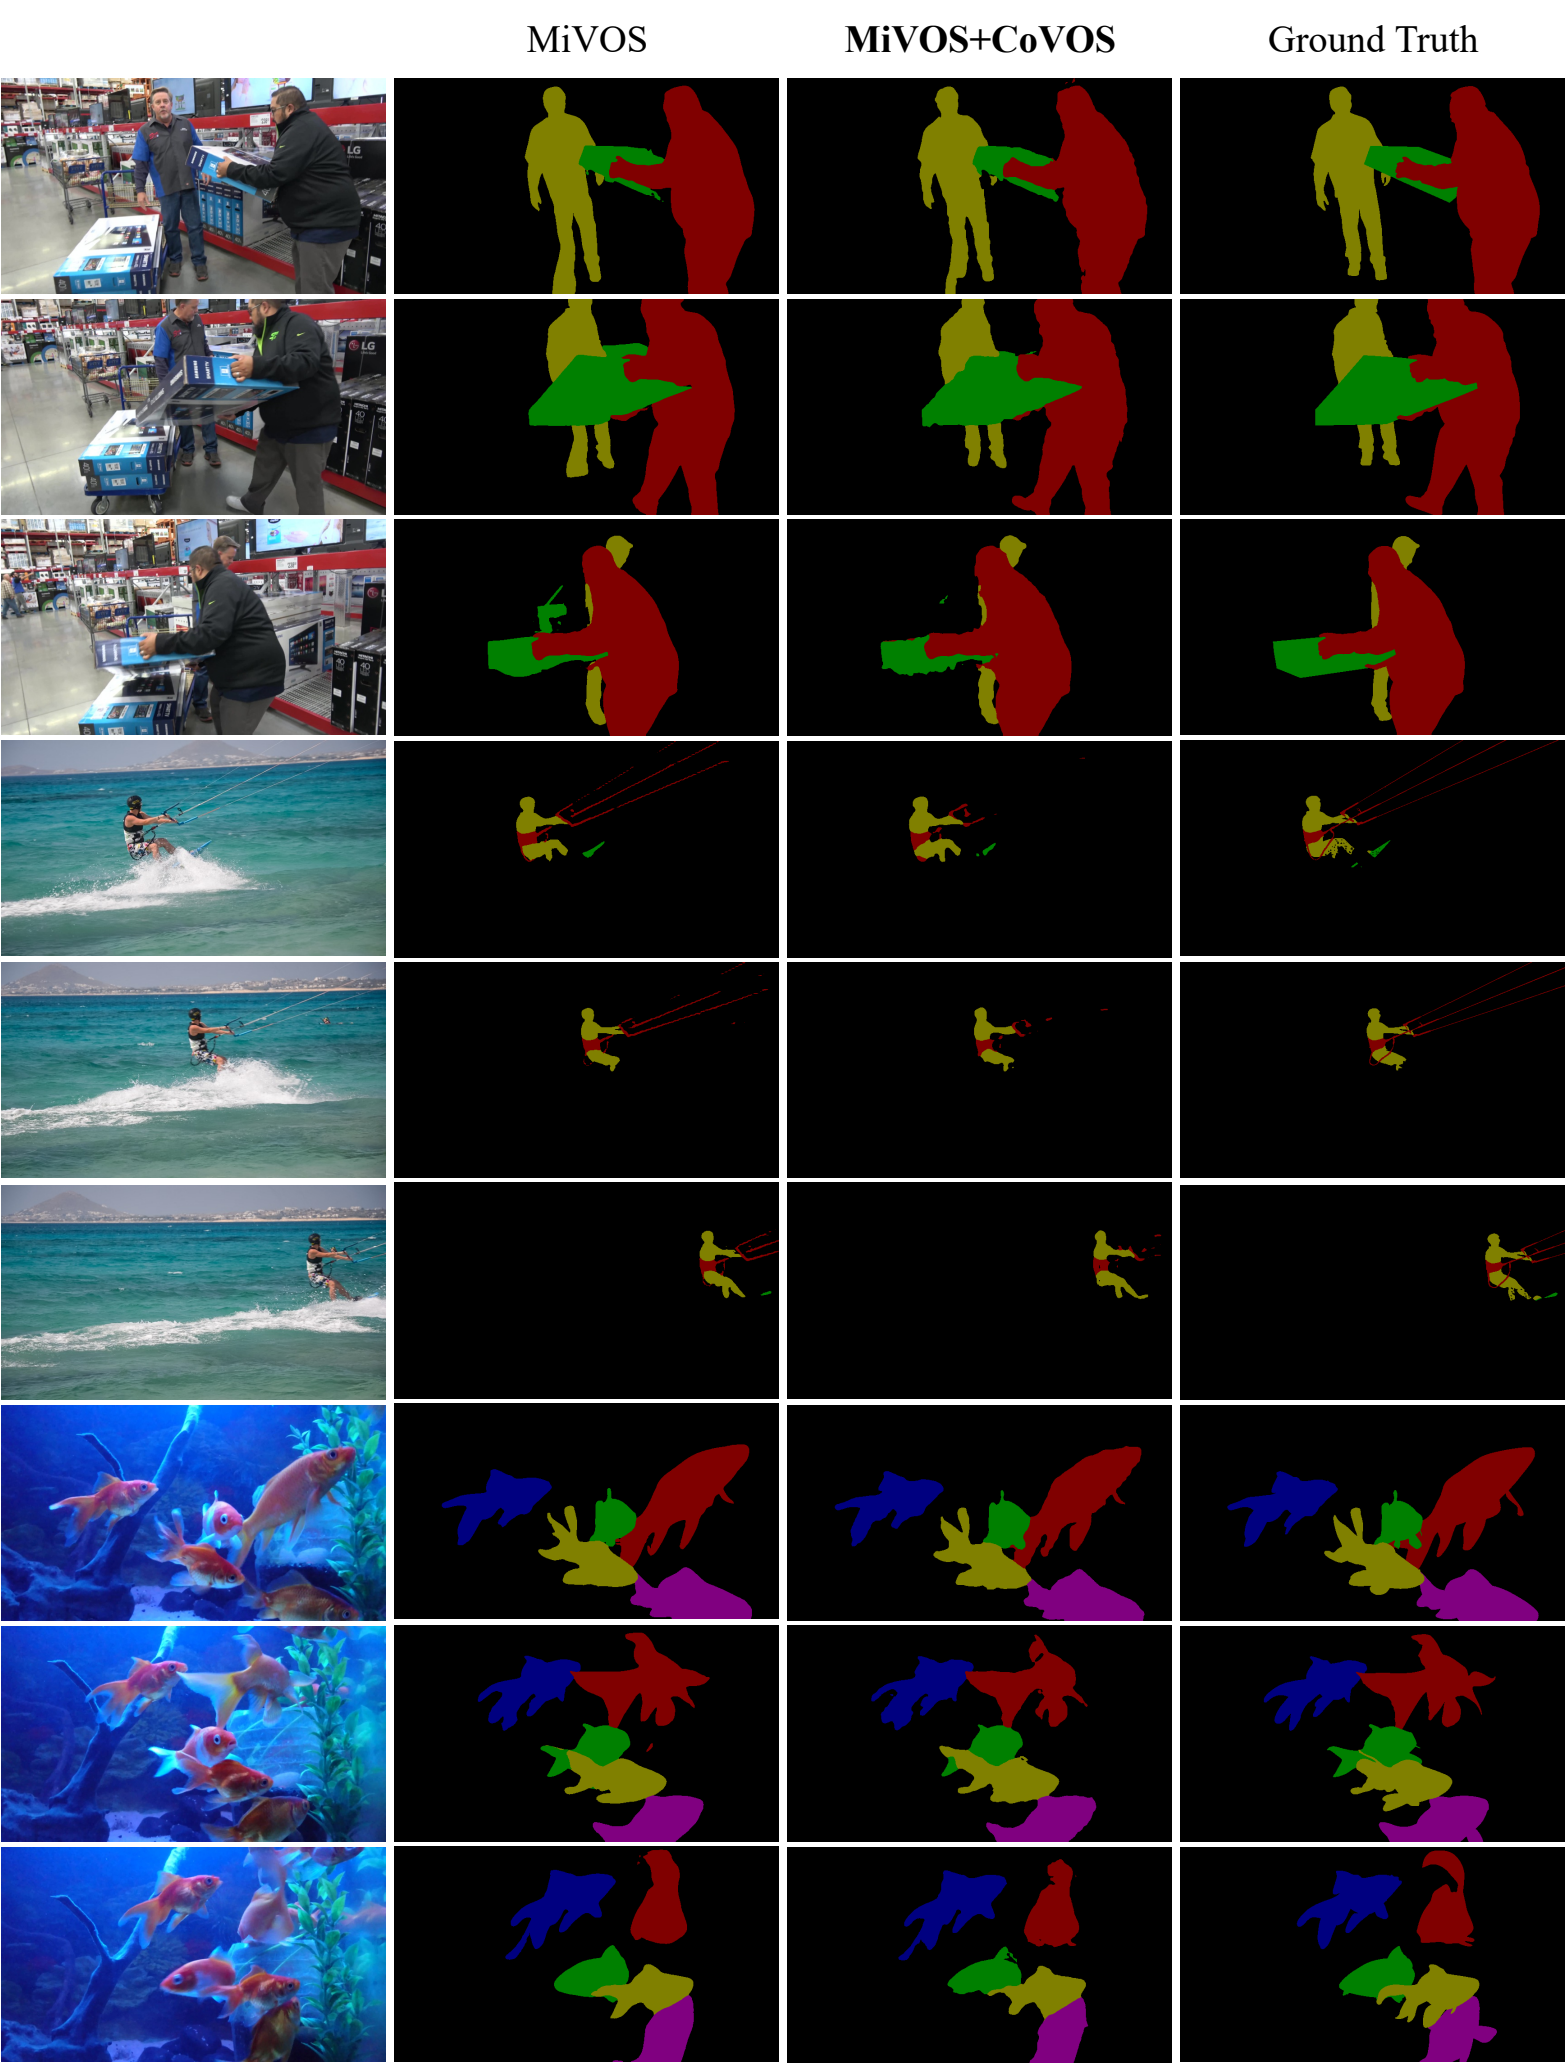   |
| 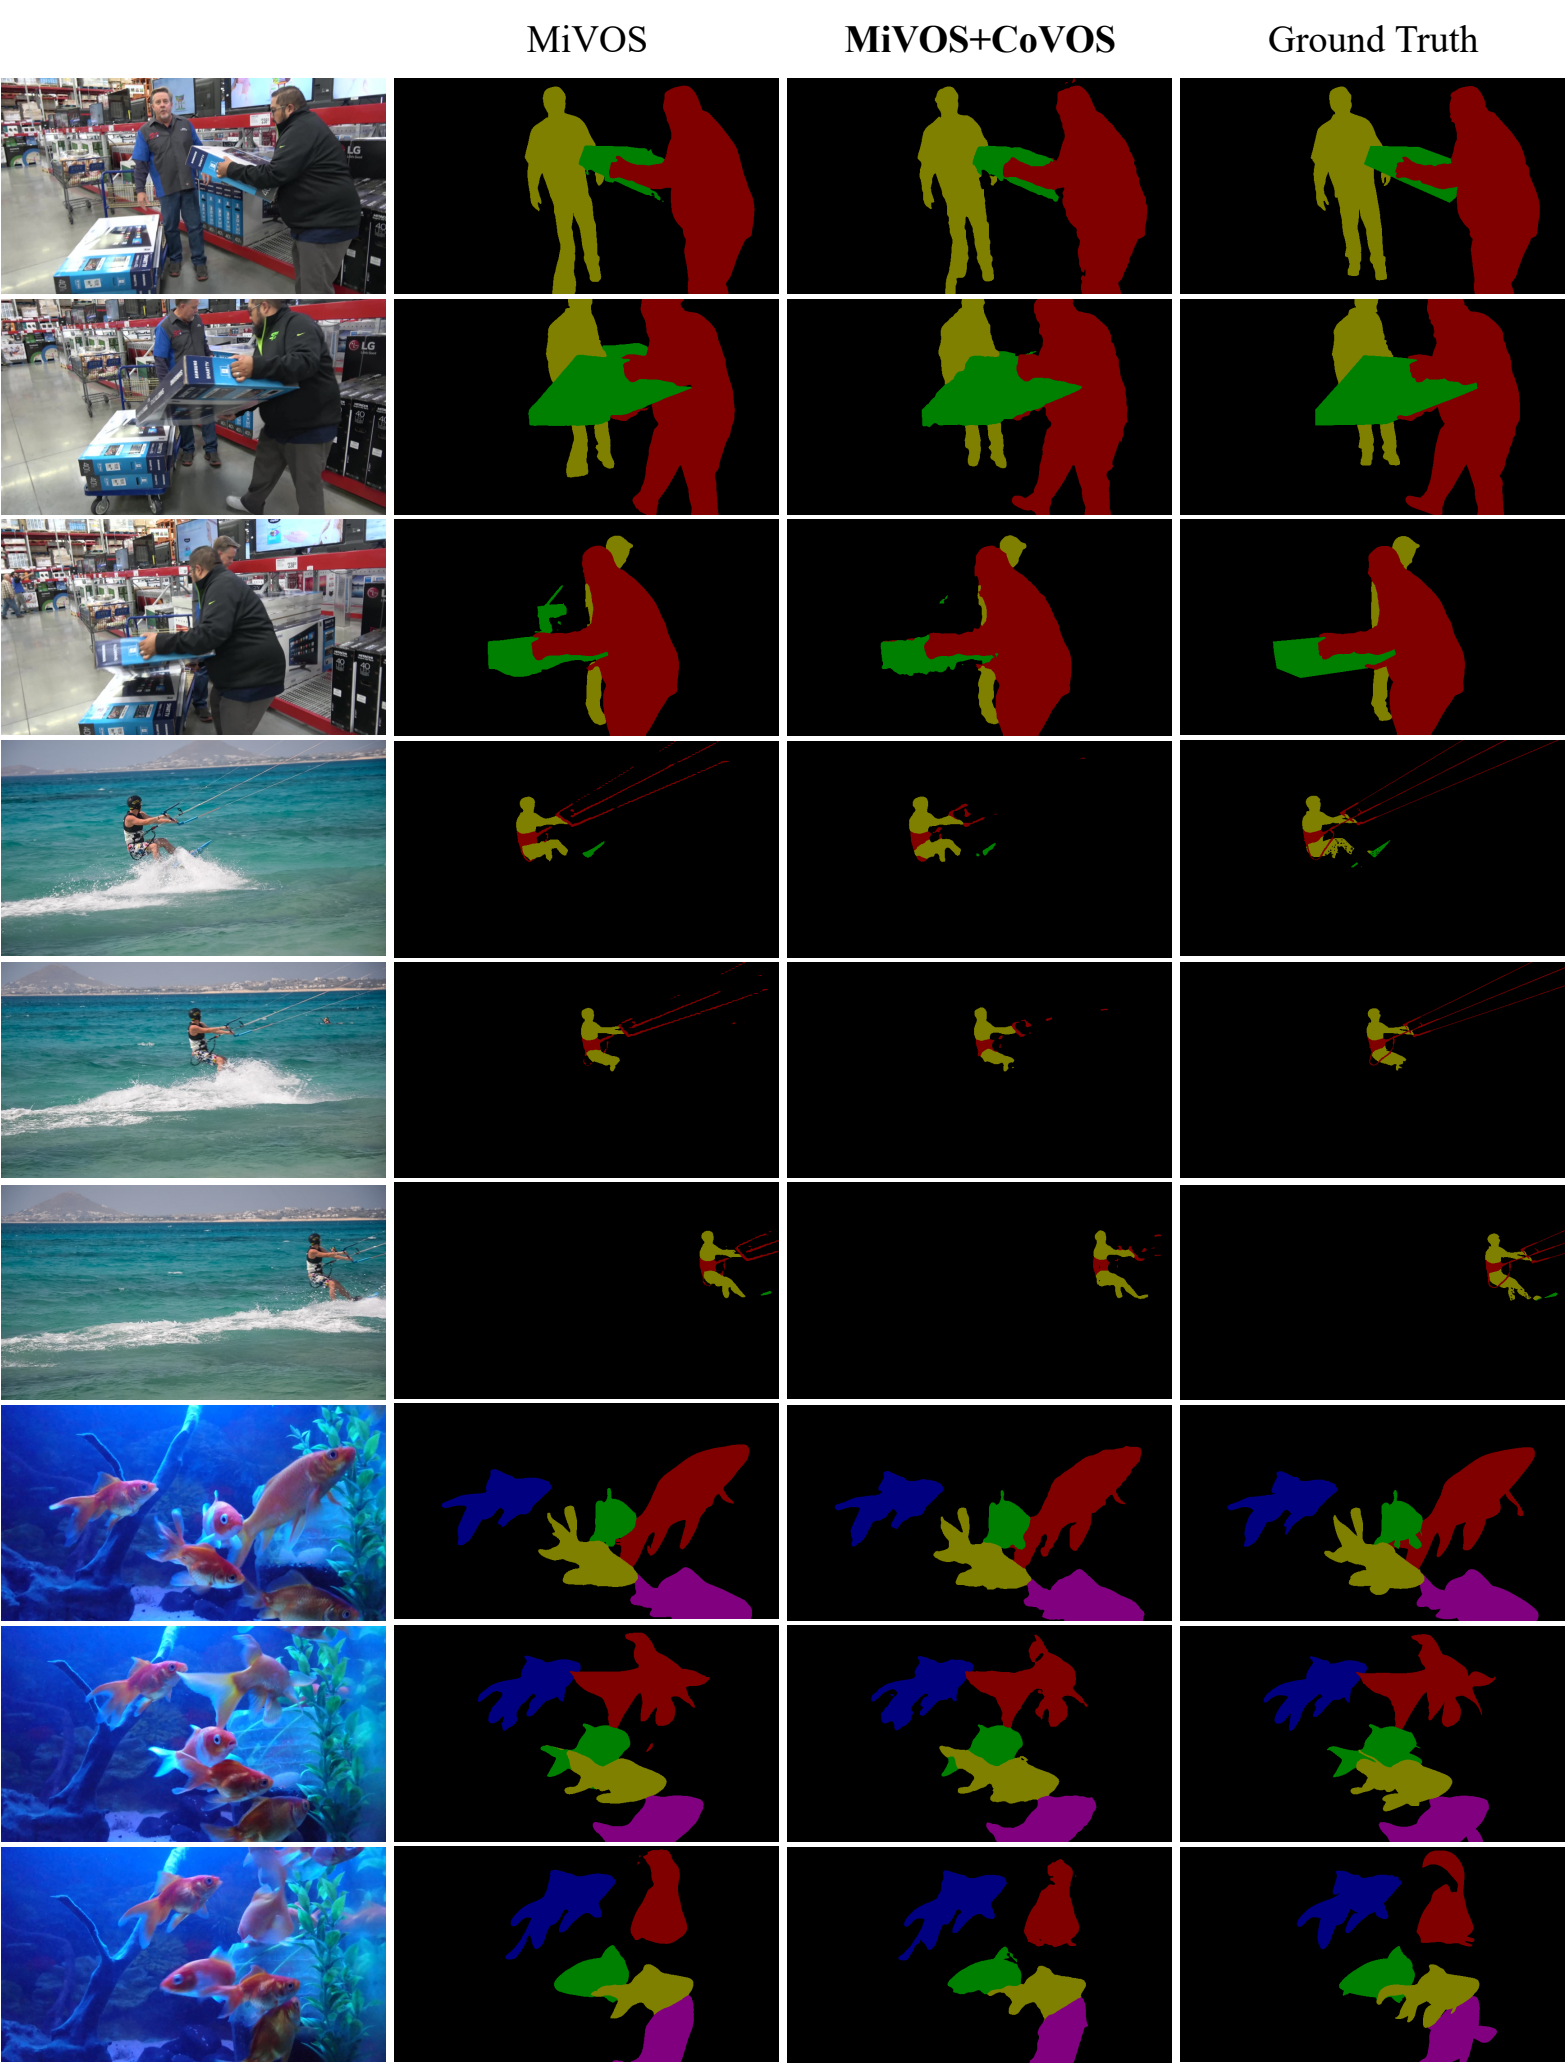   | 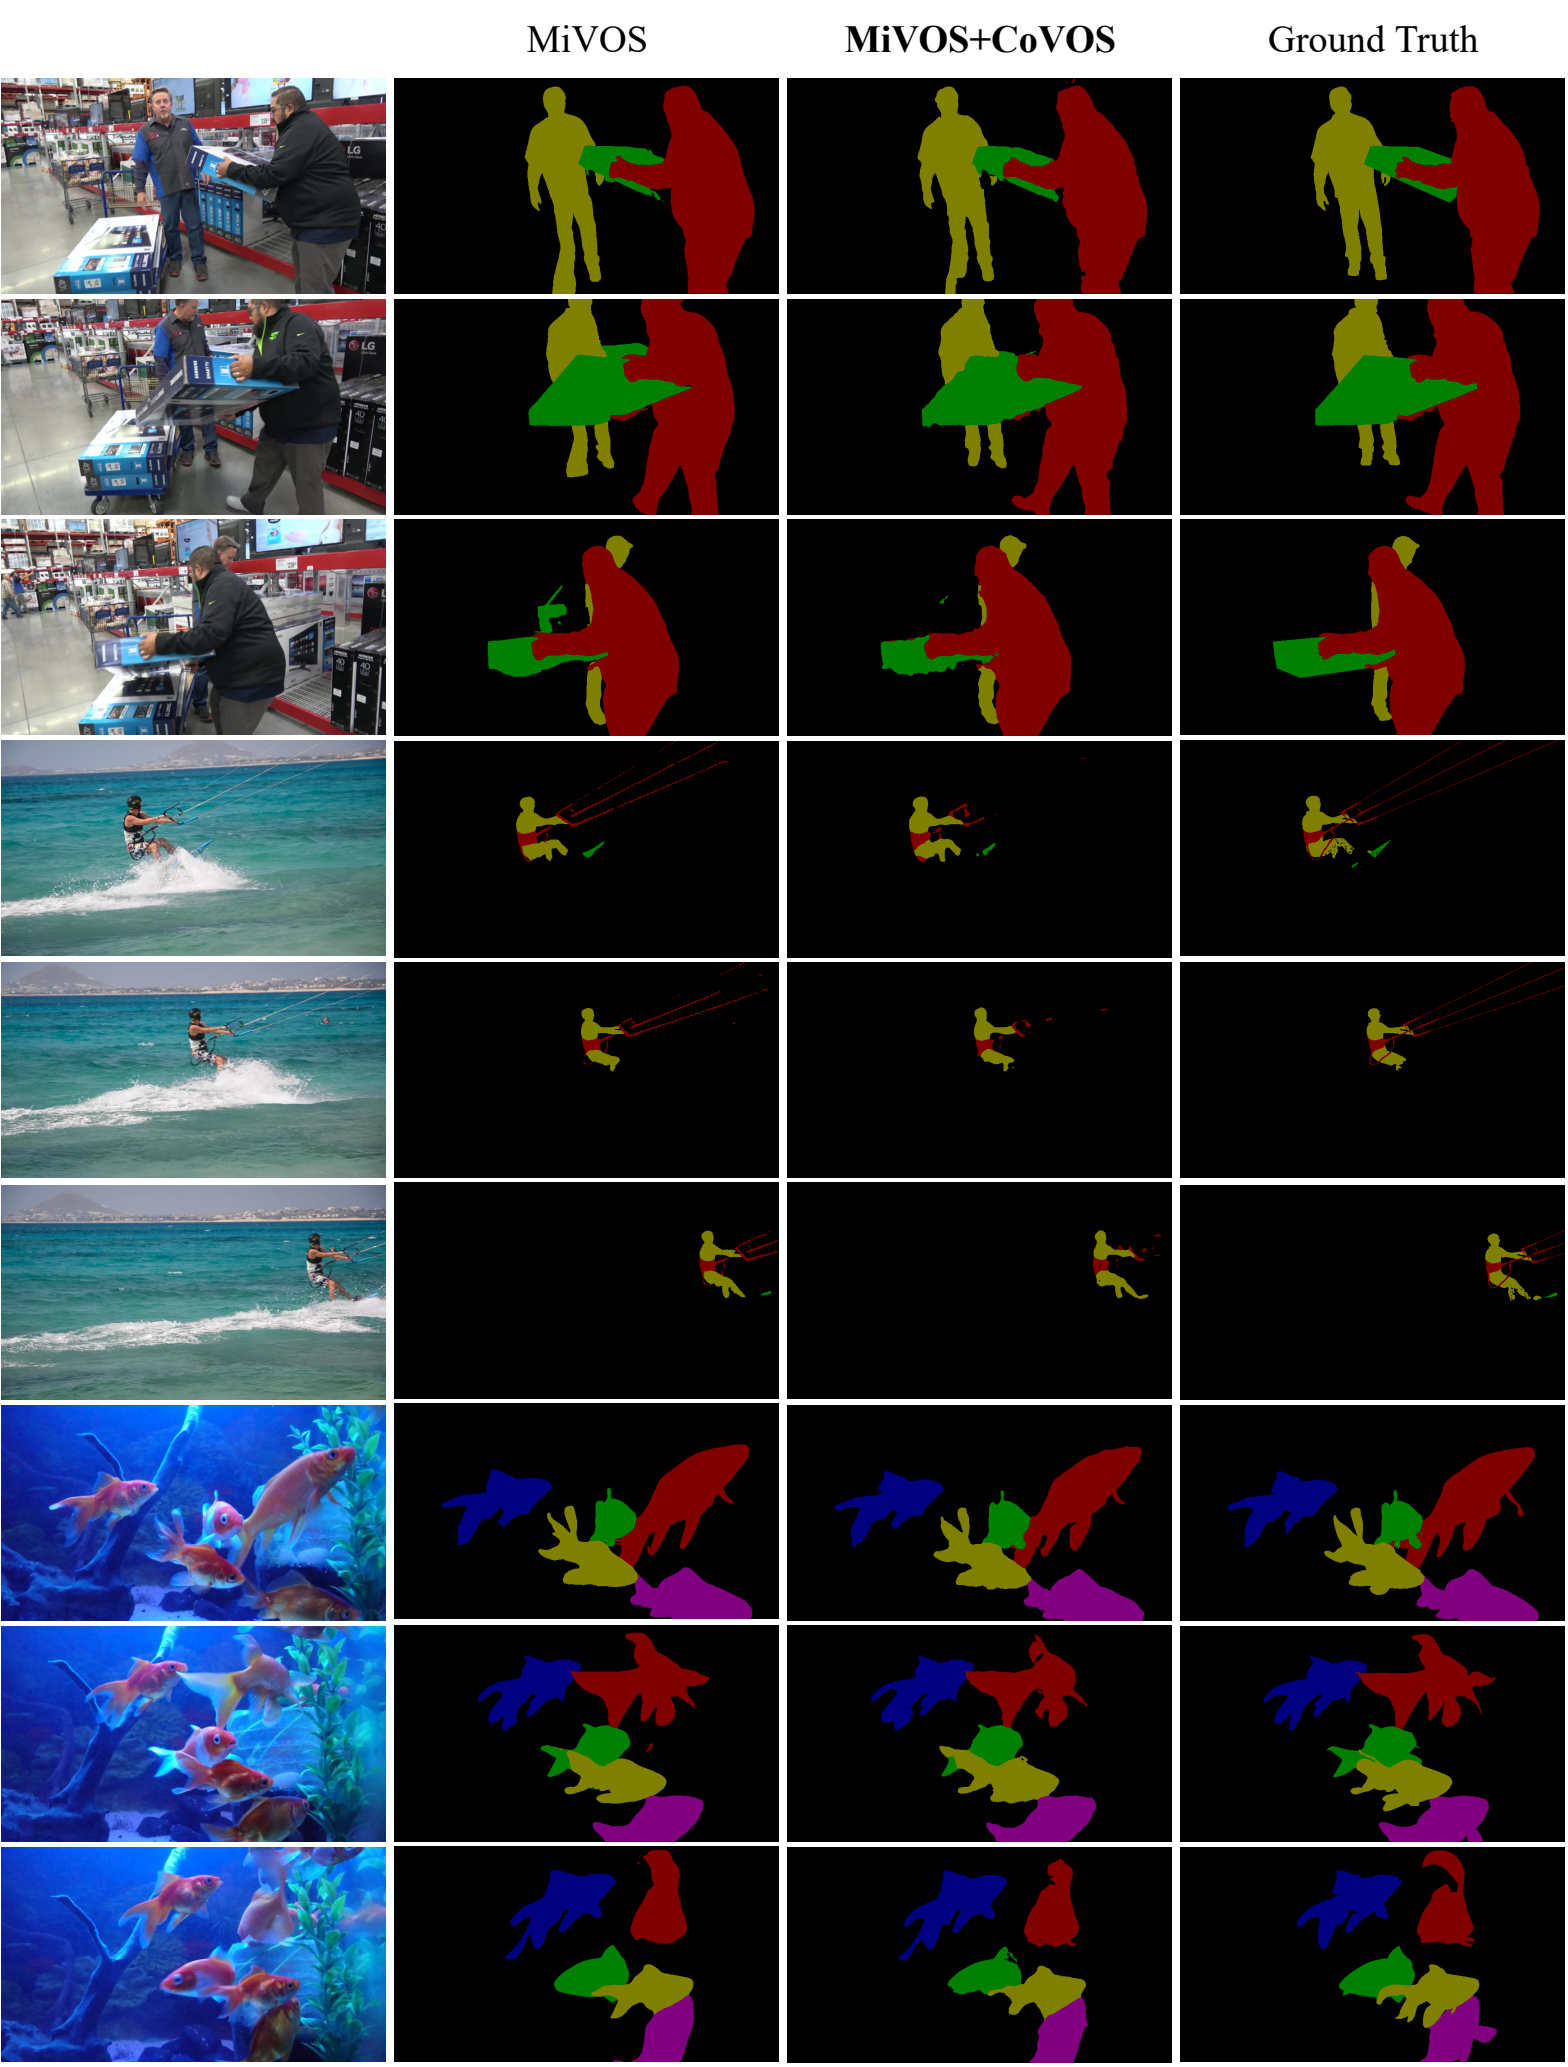   | 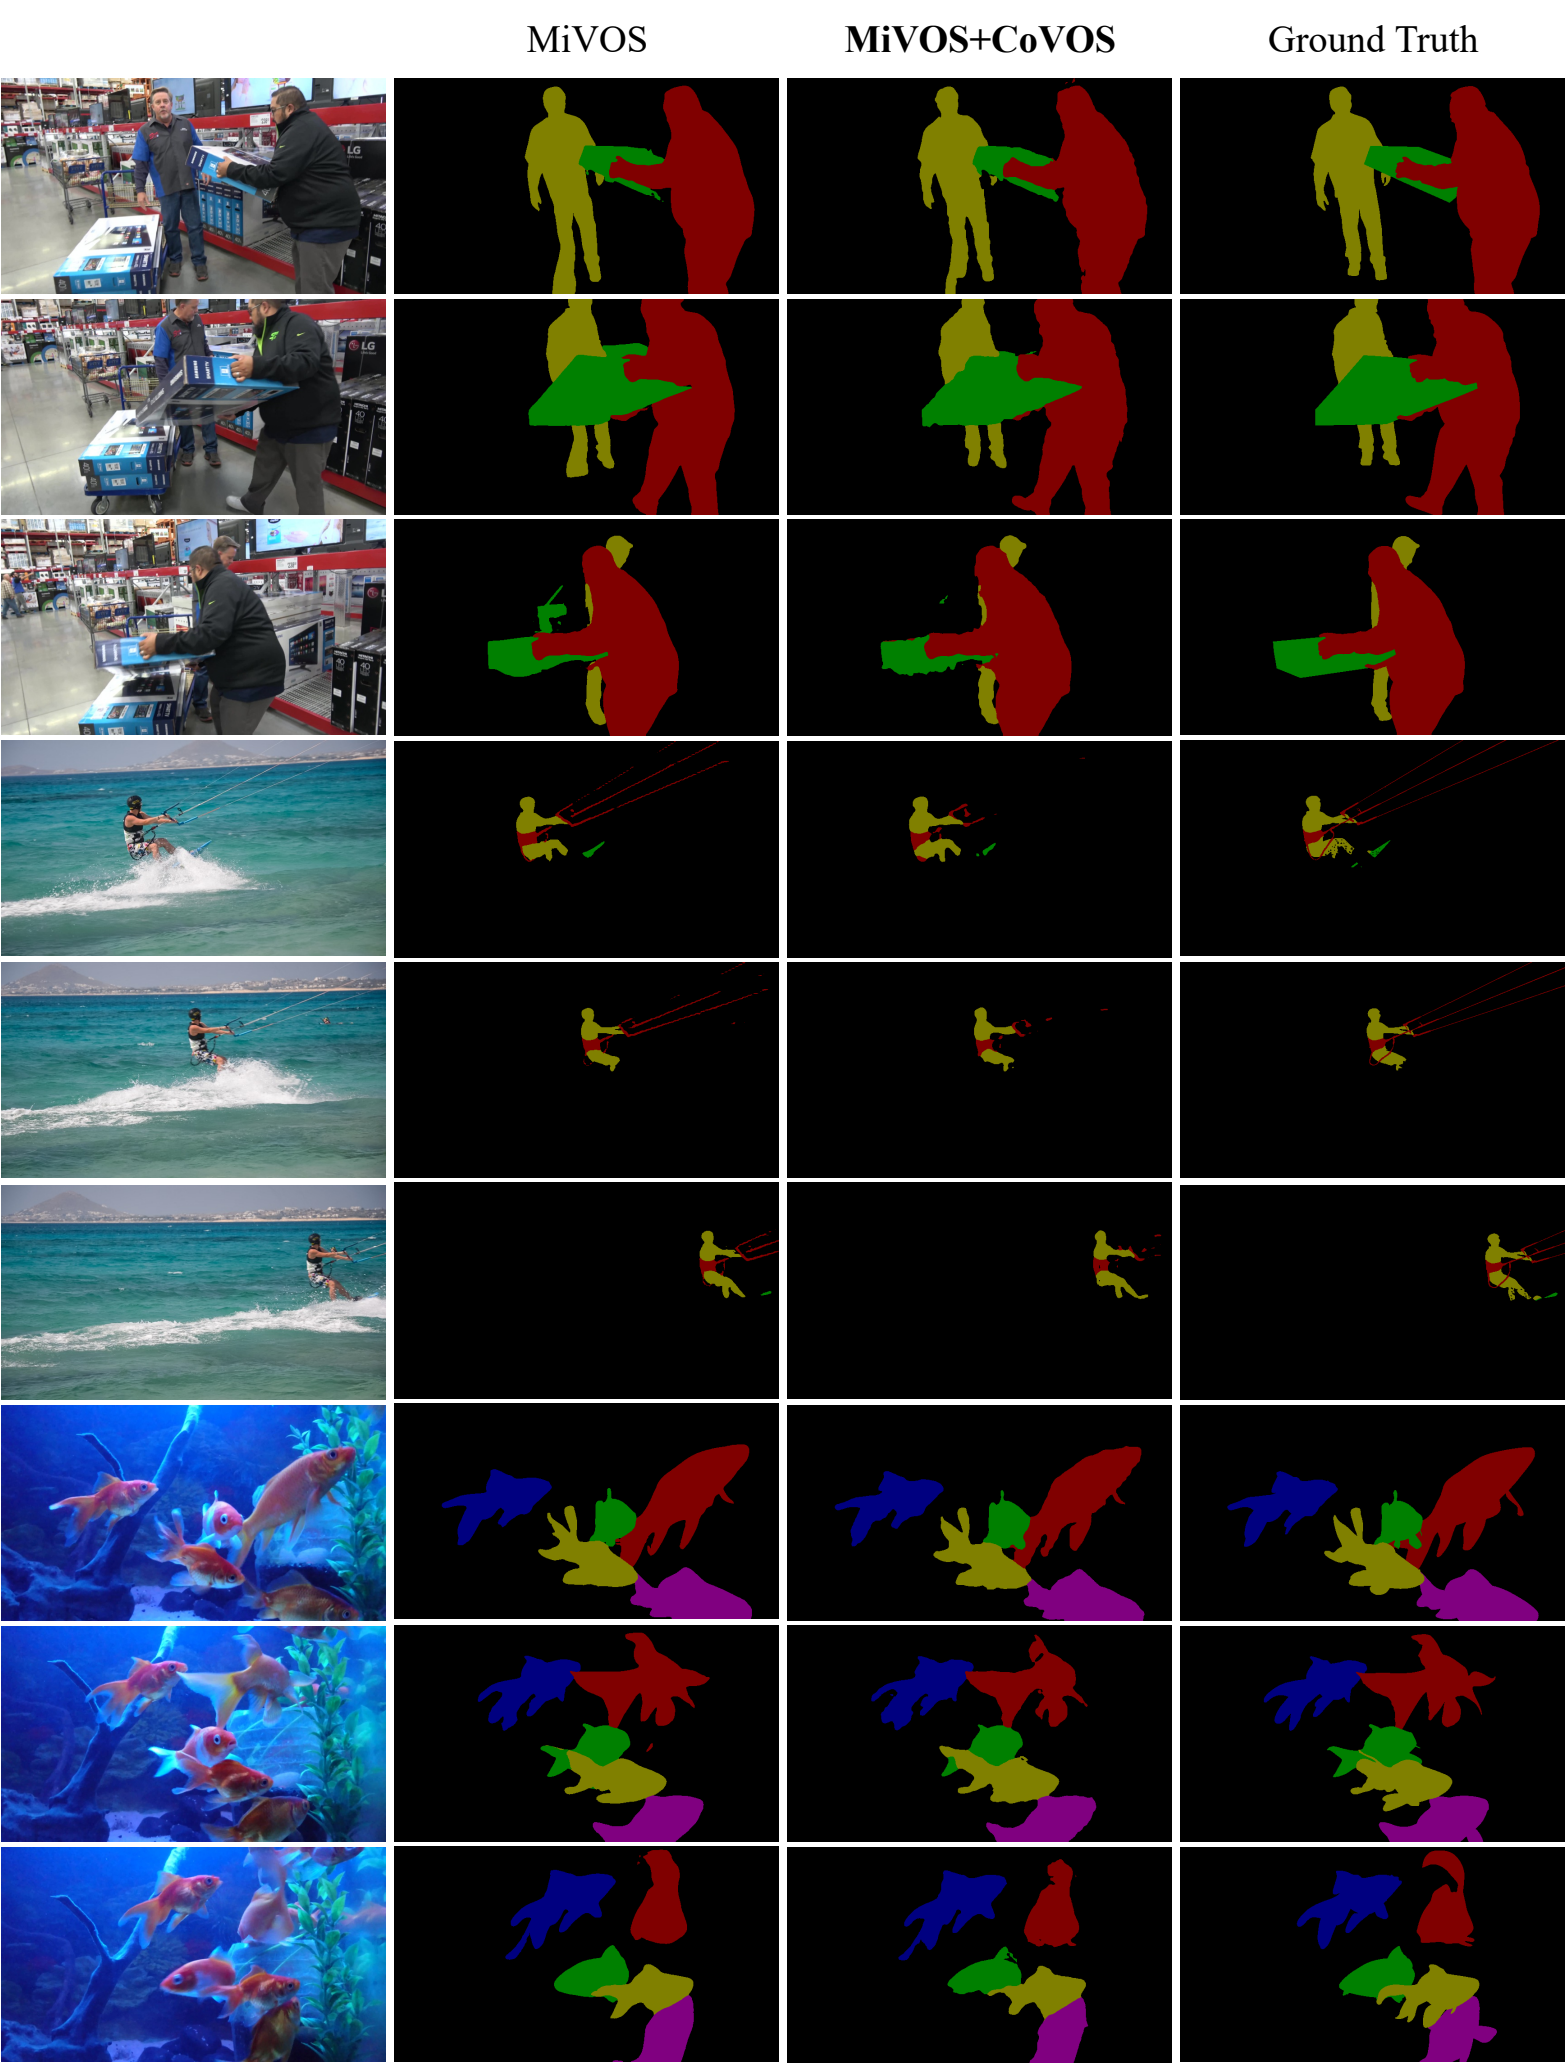   | 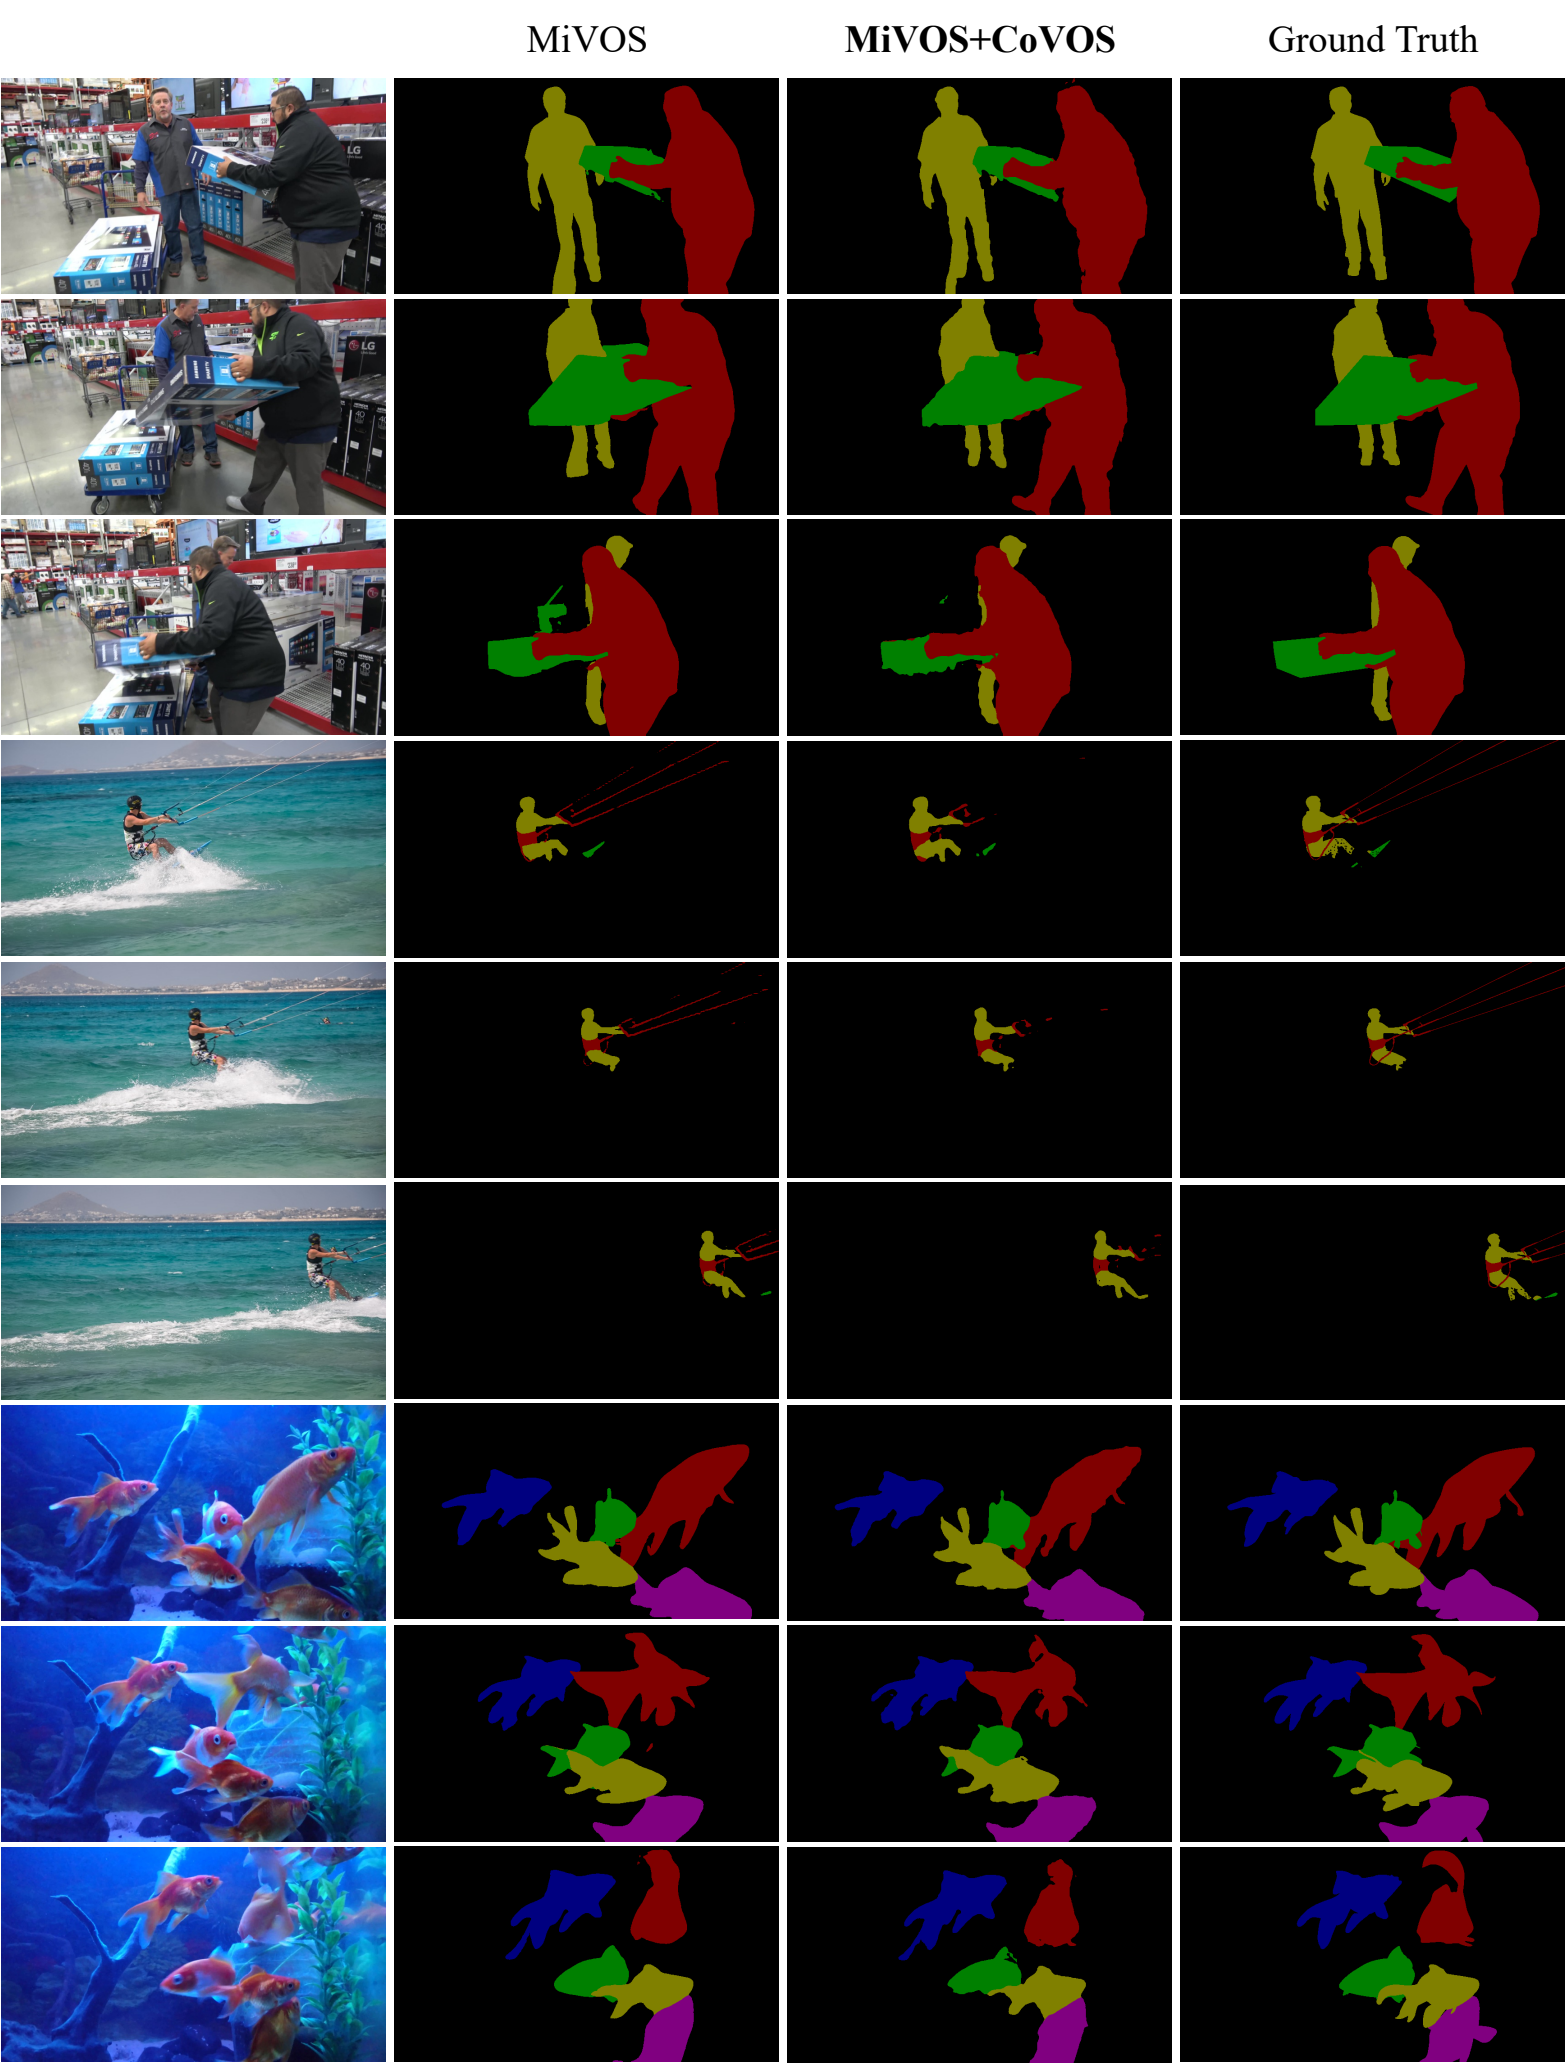   |
| 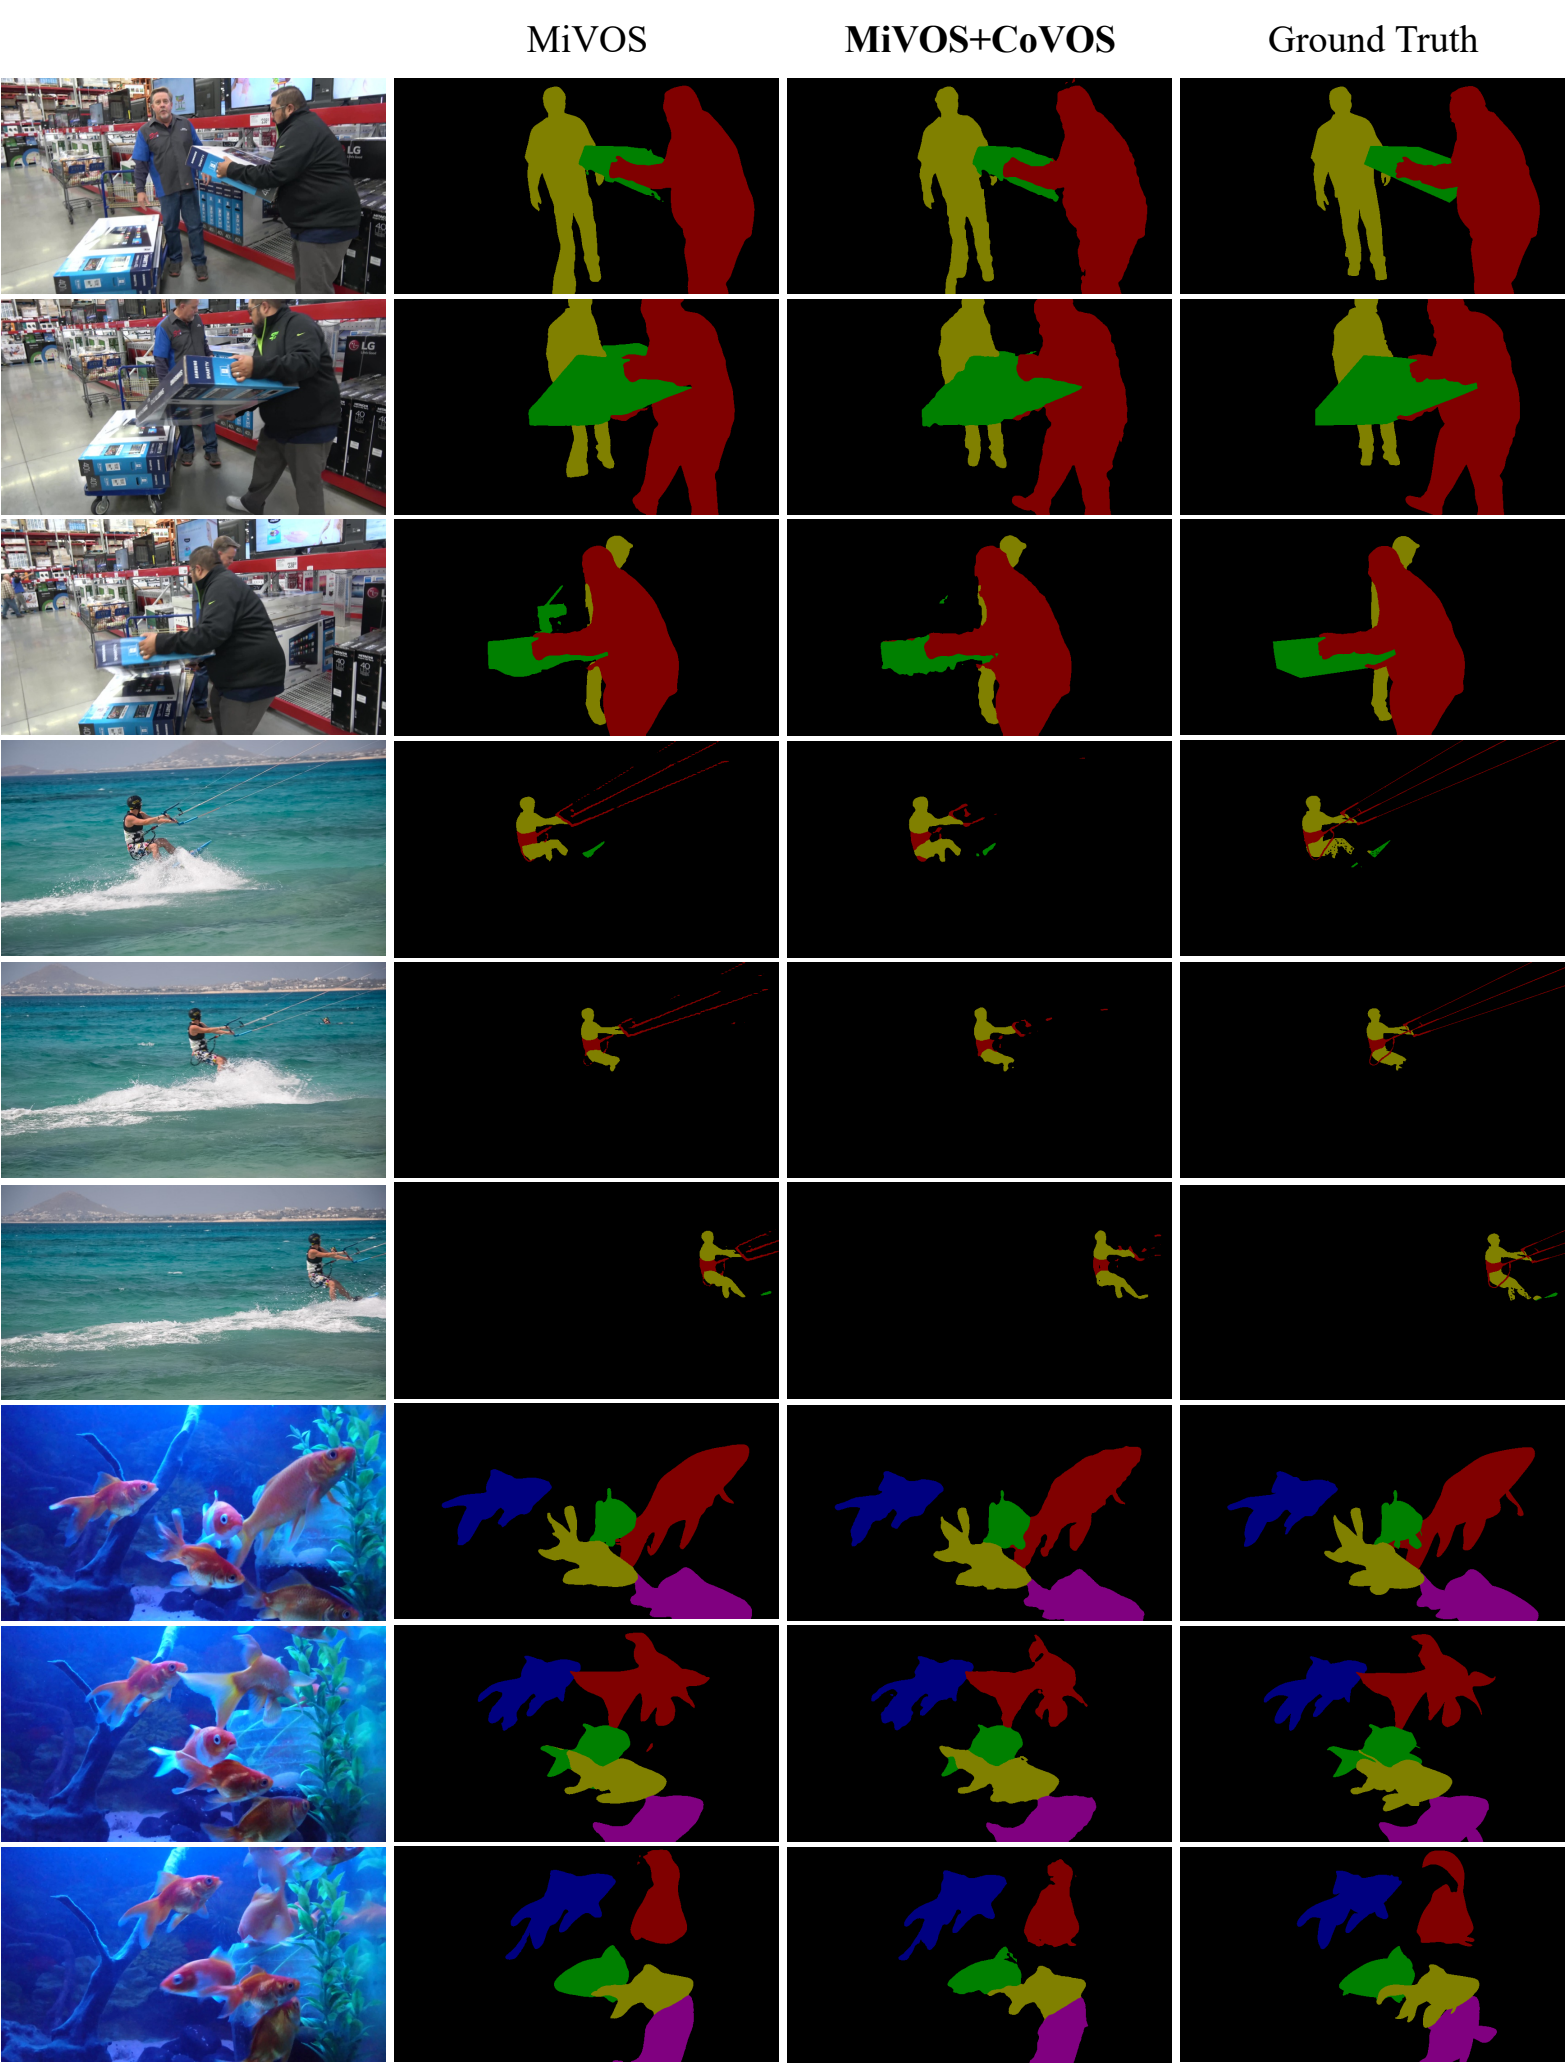  | 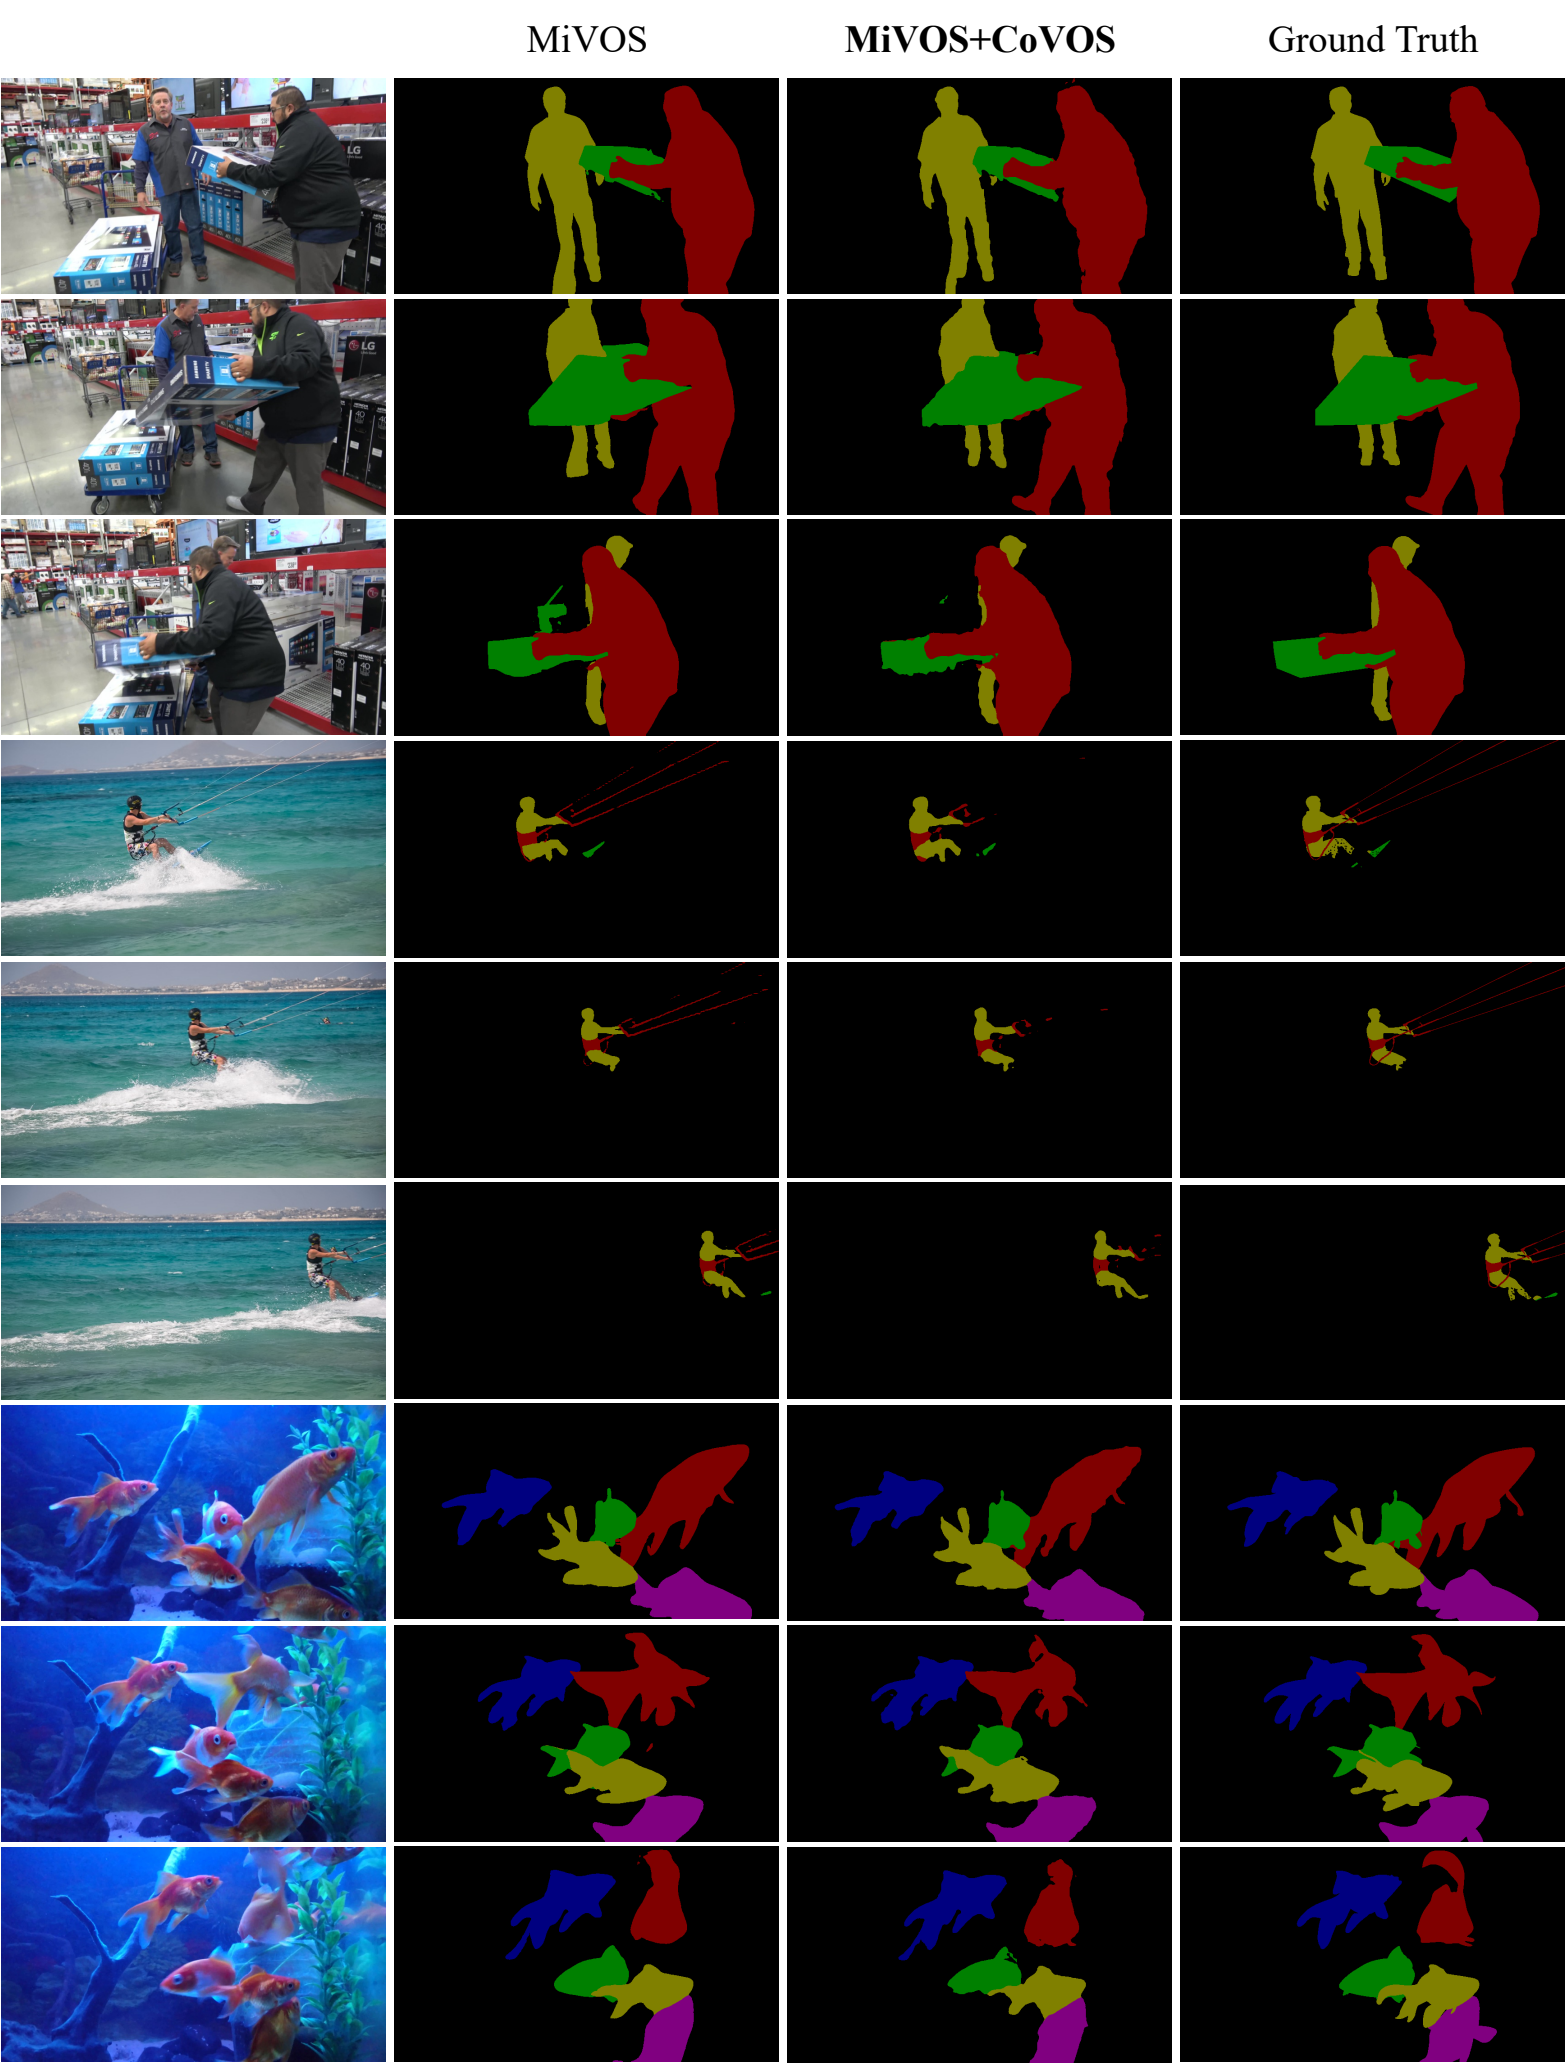  | 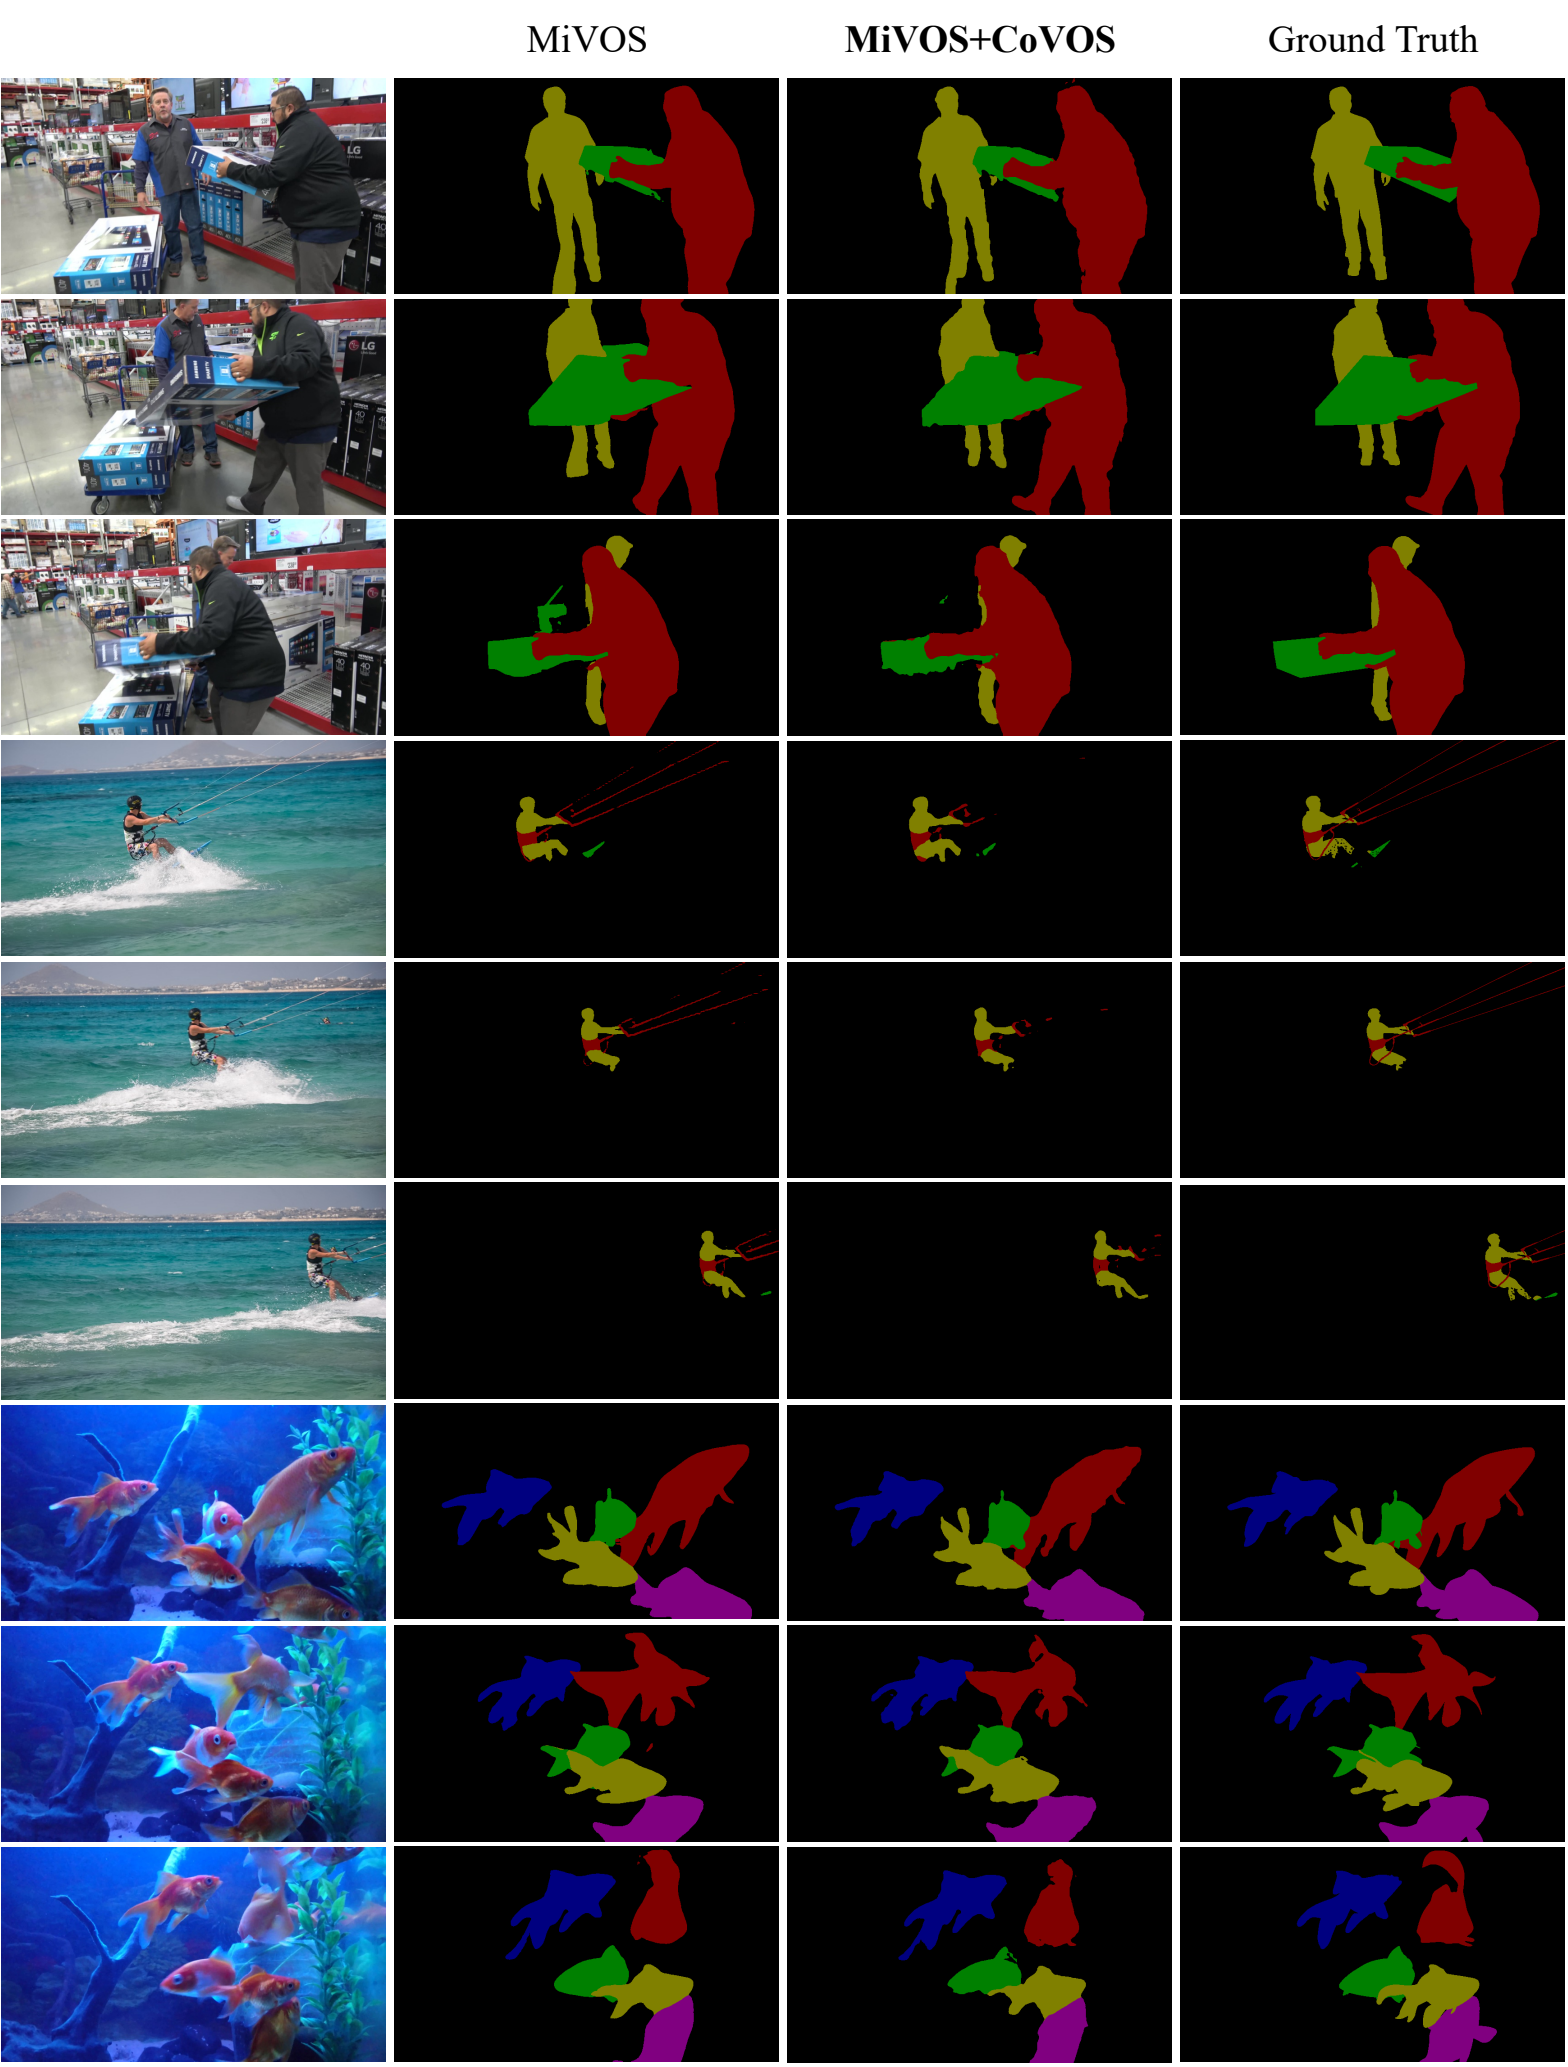  | 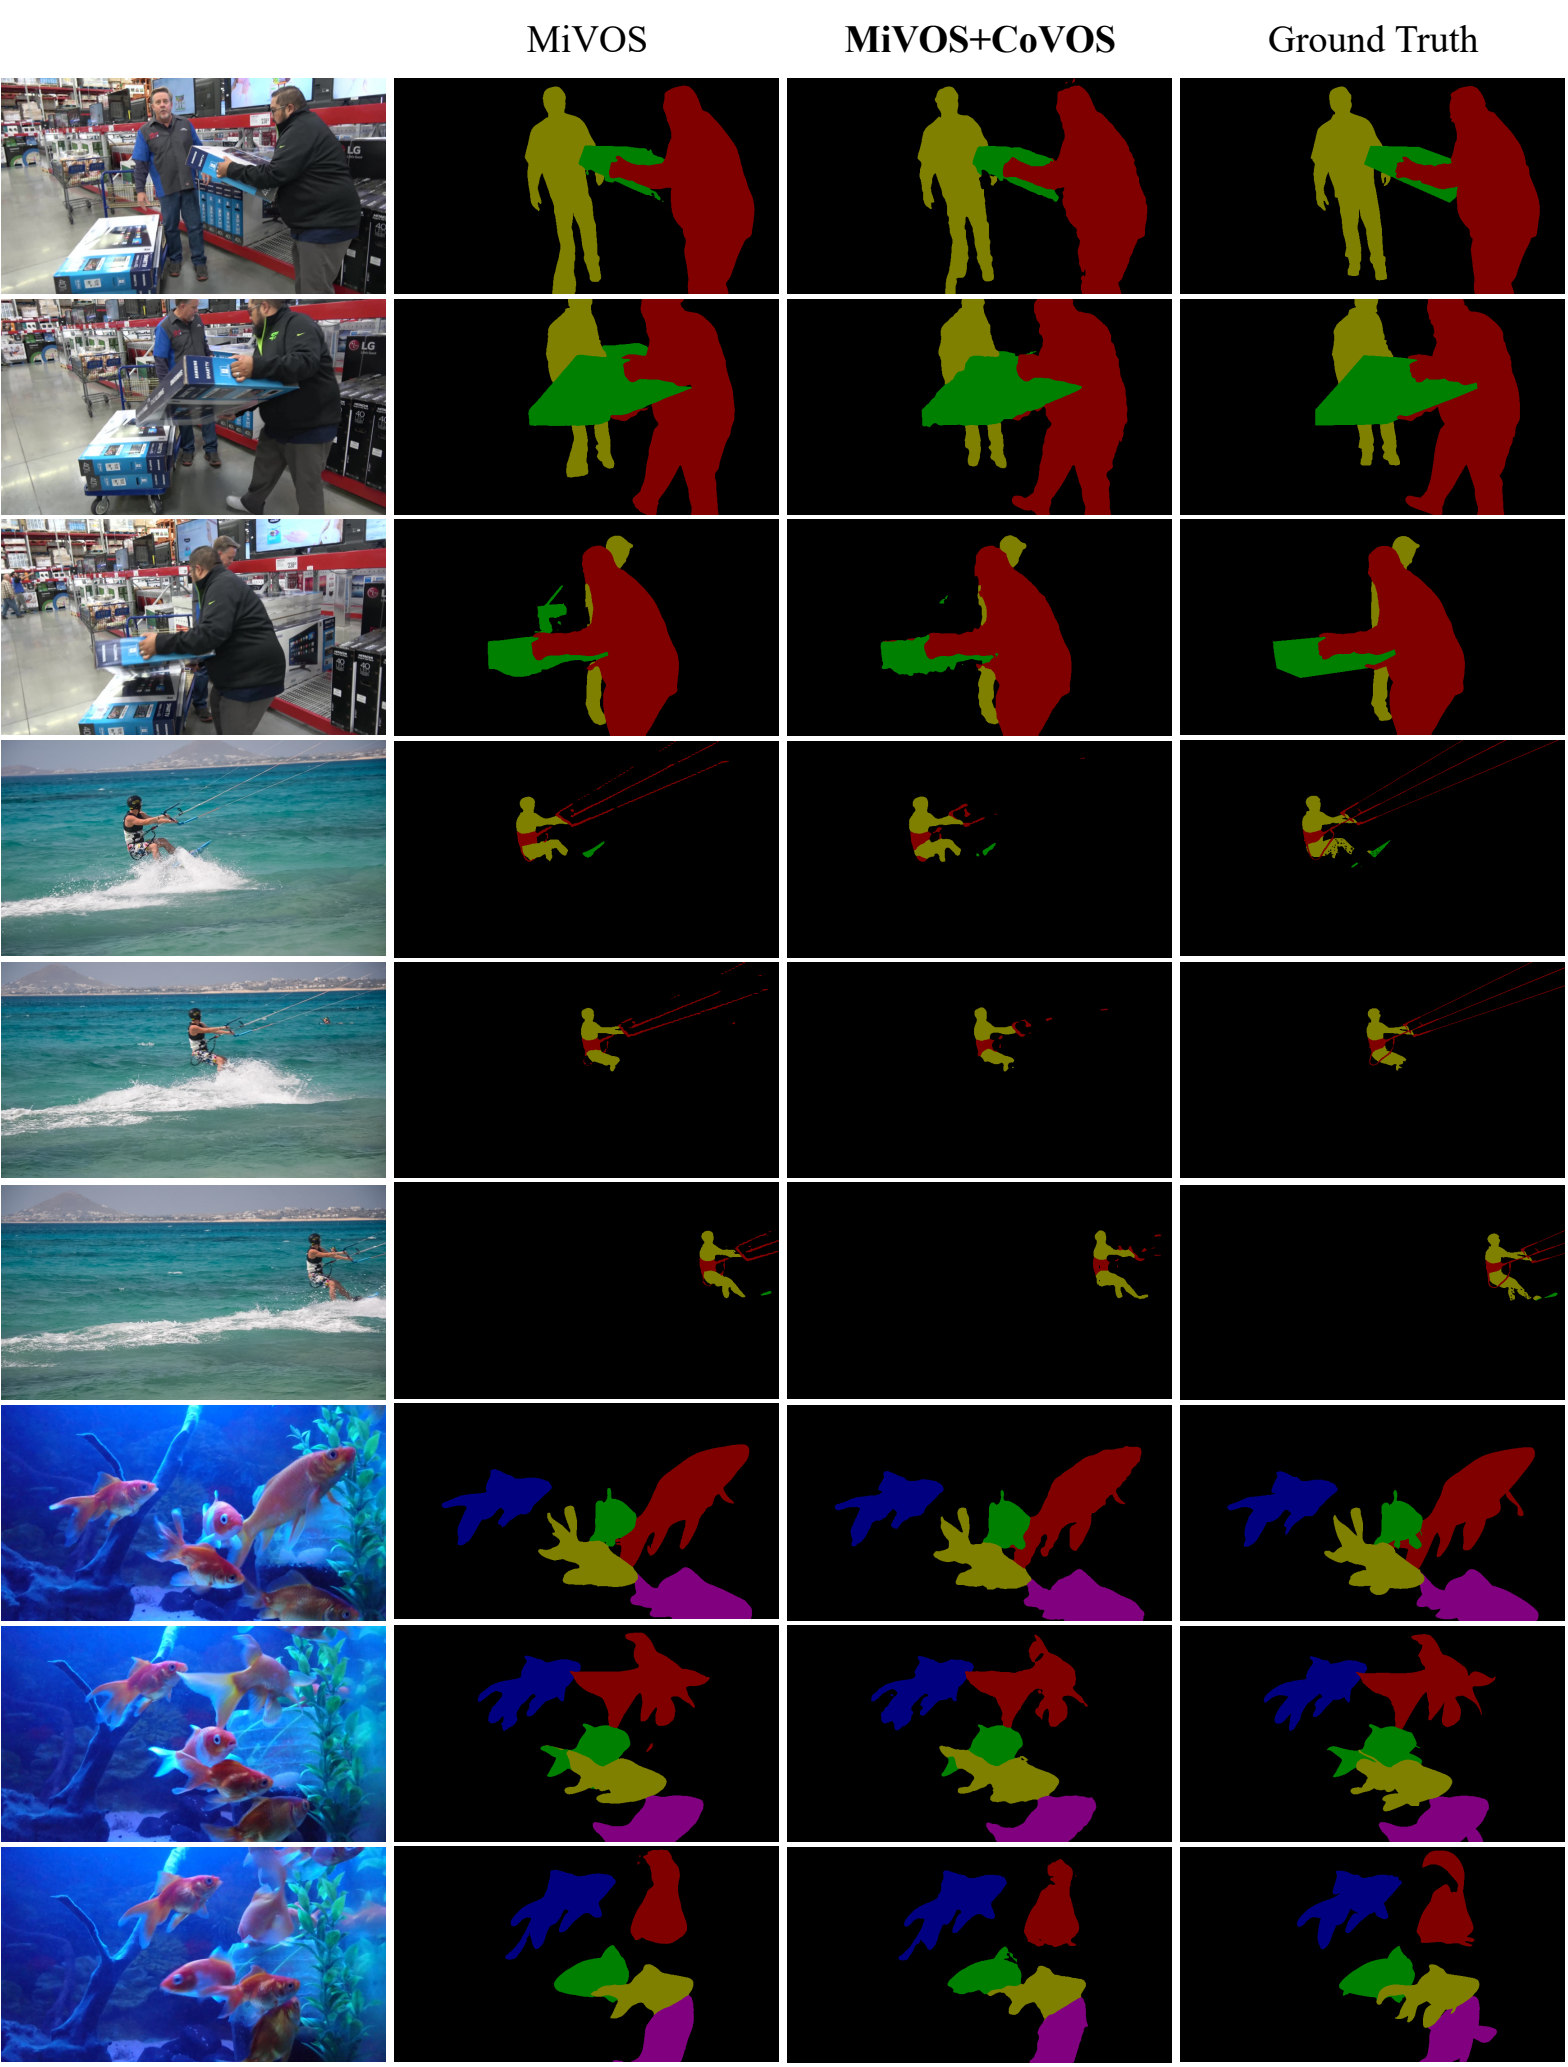  |
| 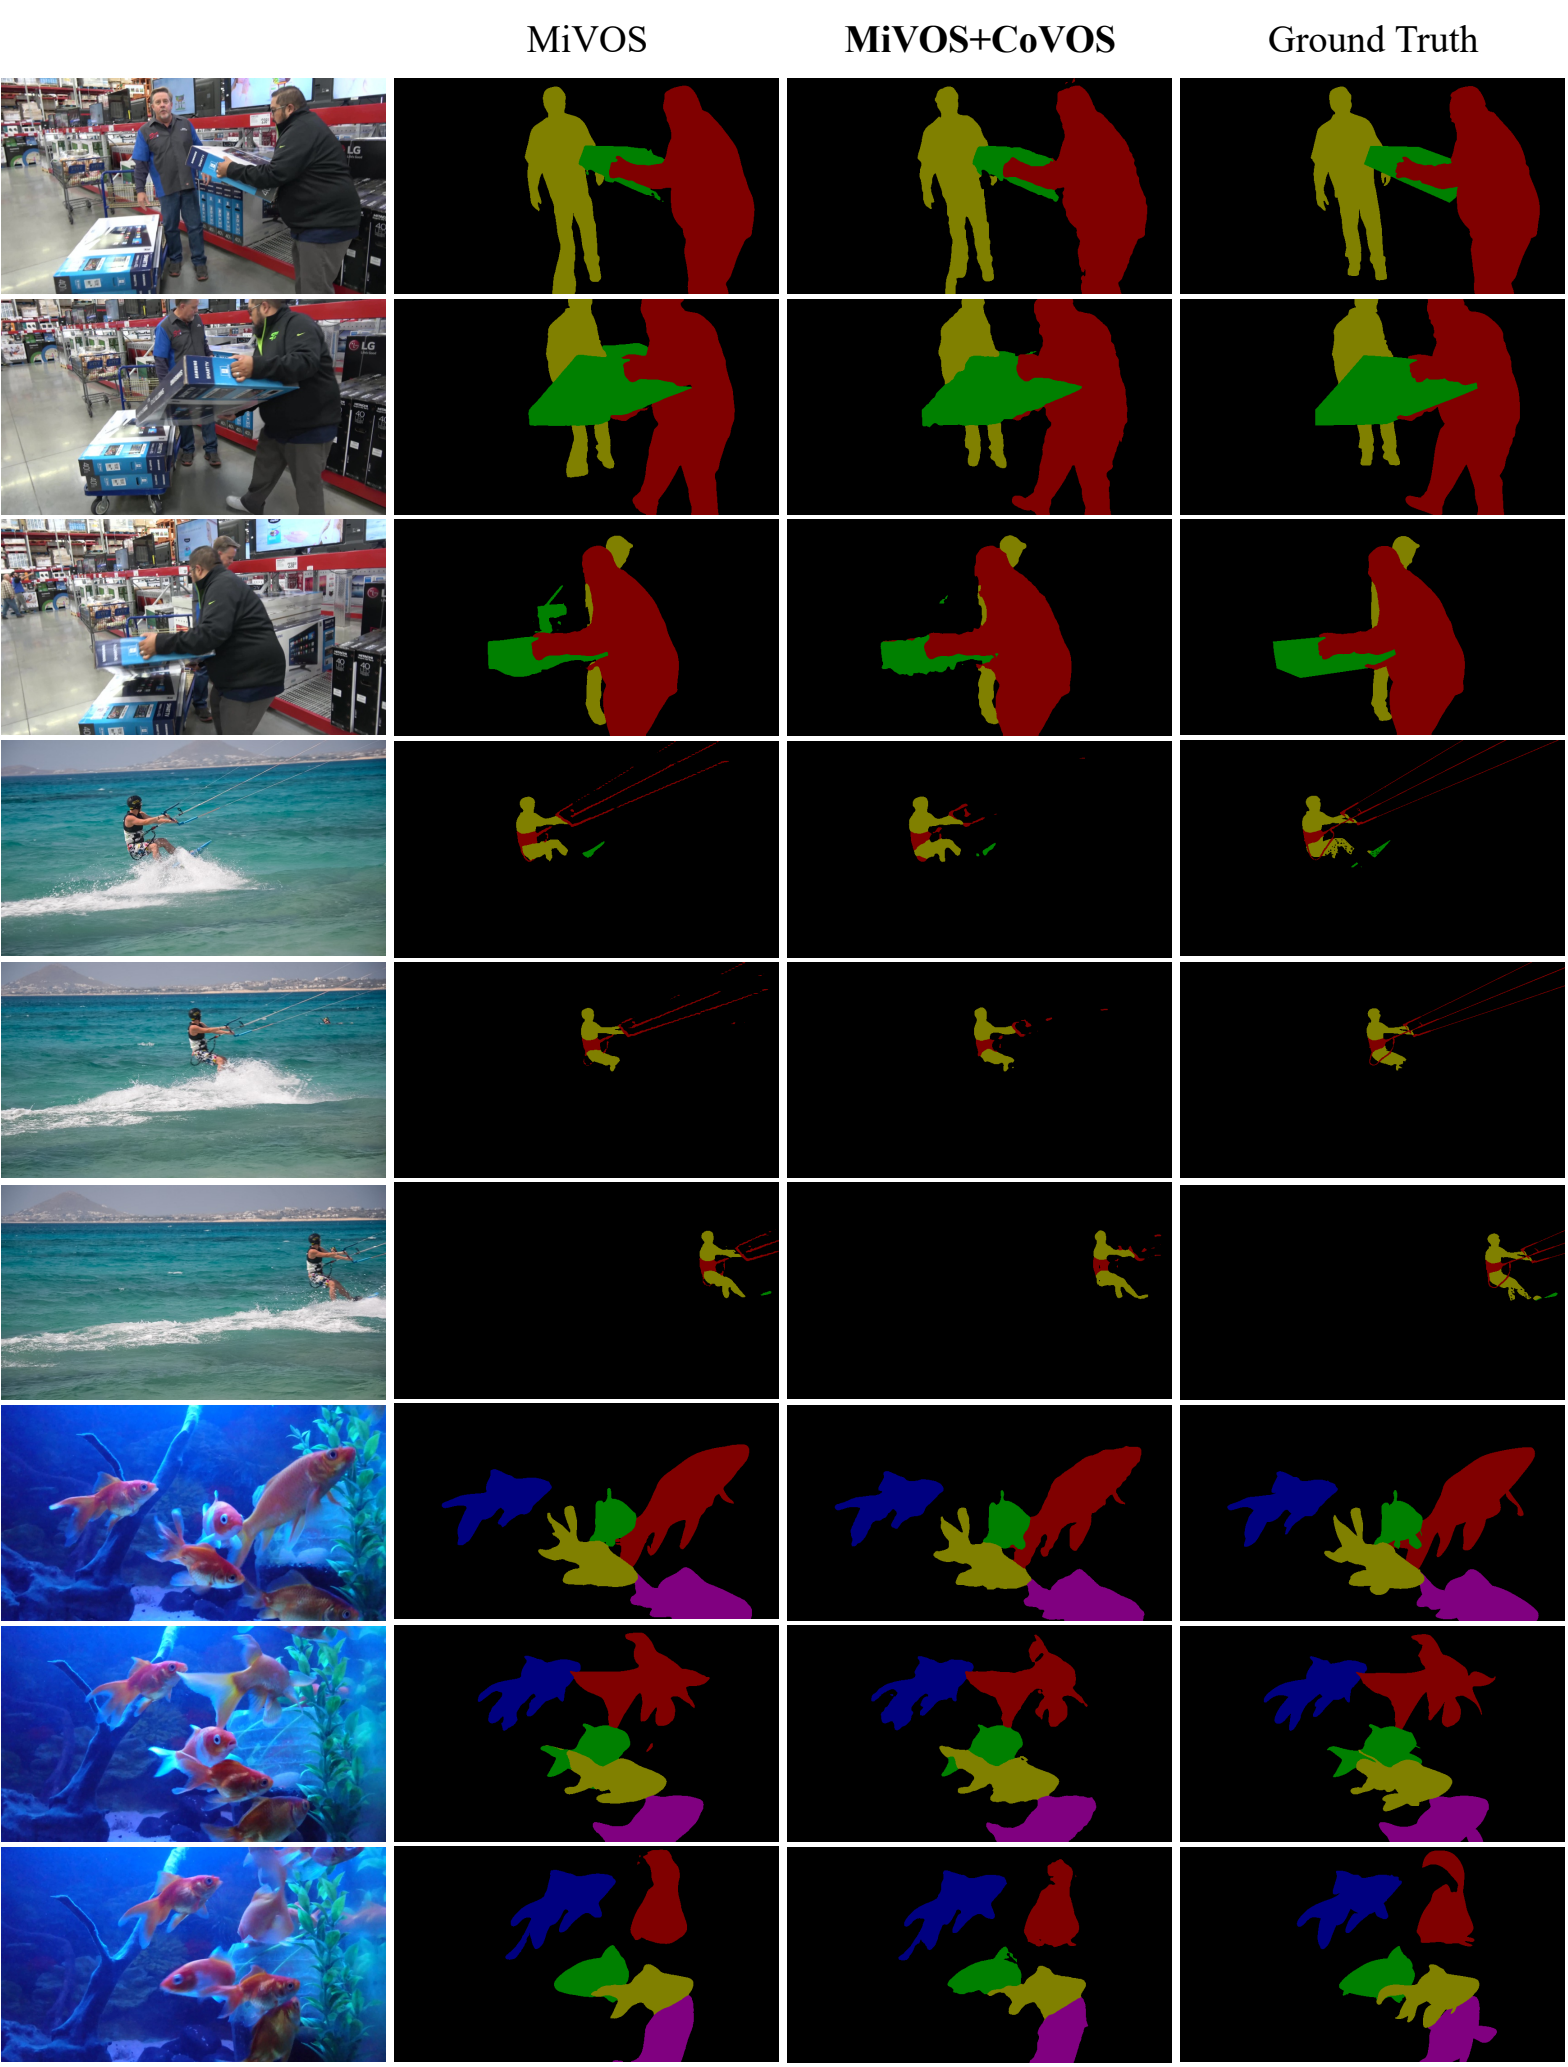 | 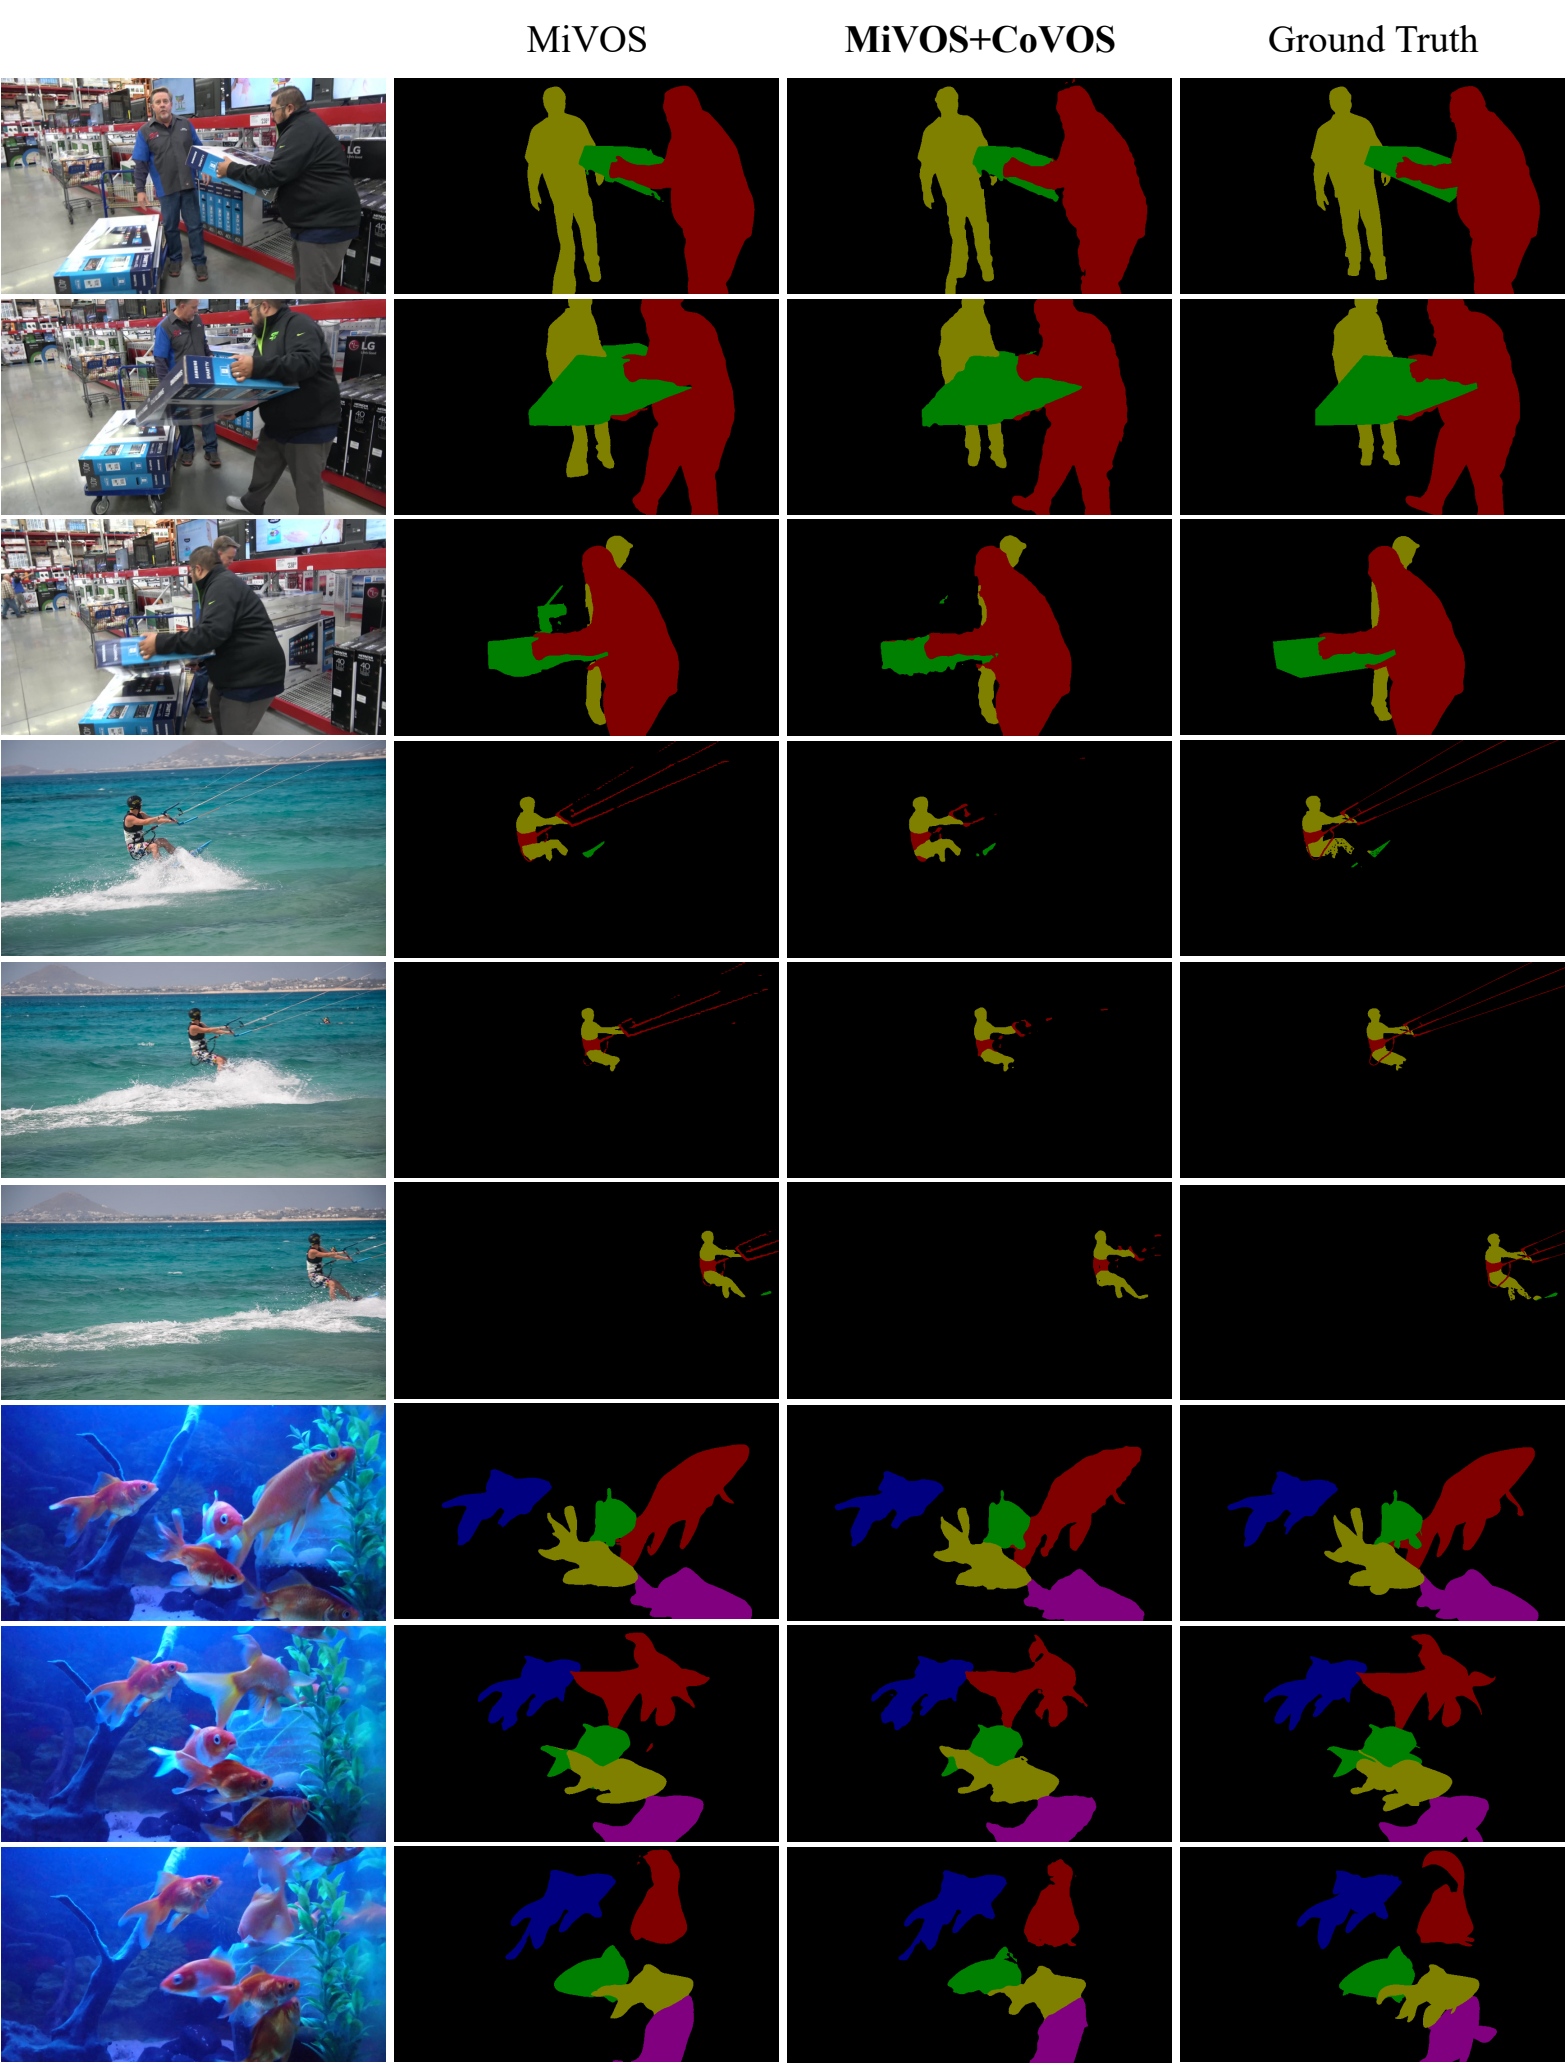 | 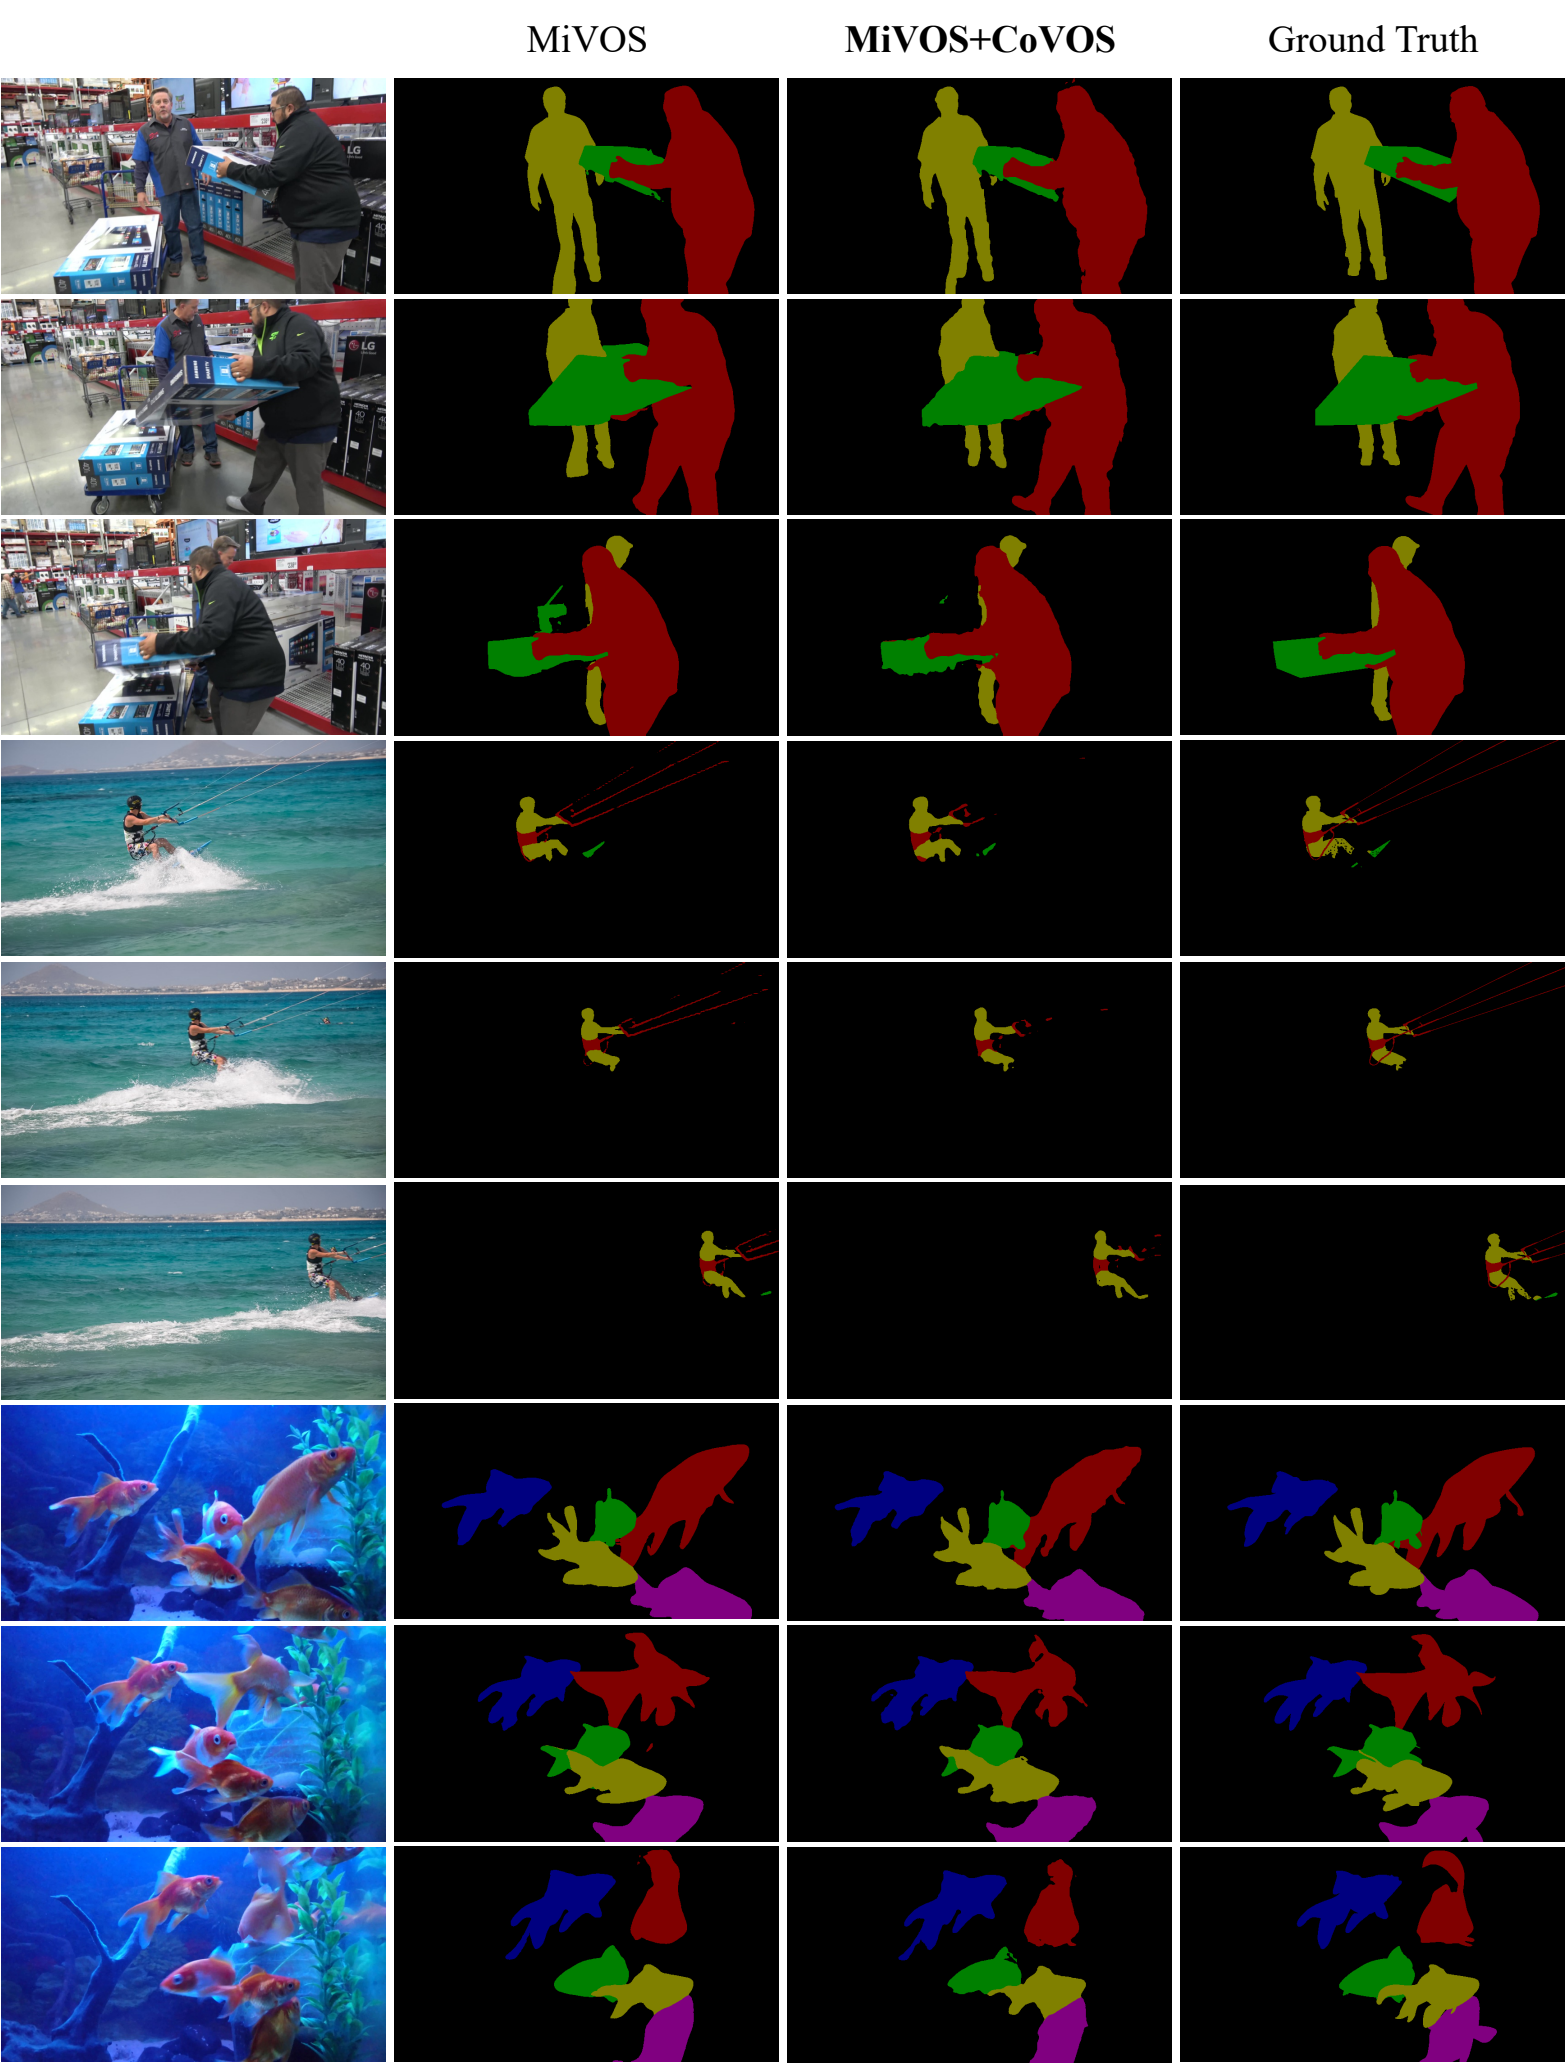 | 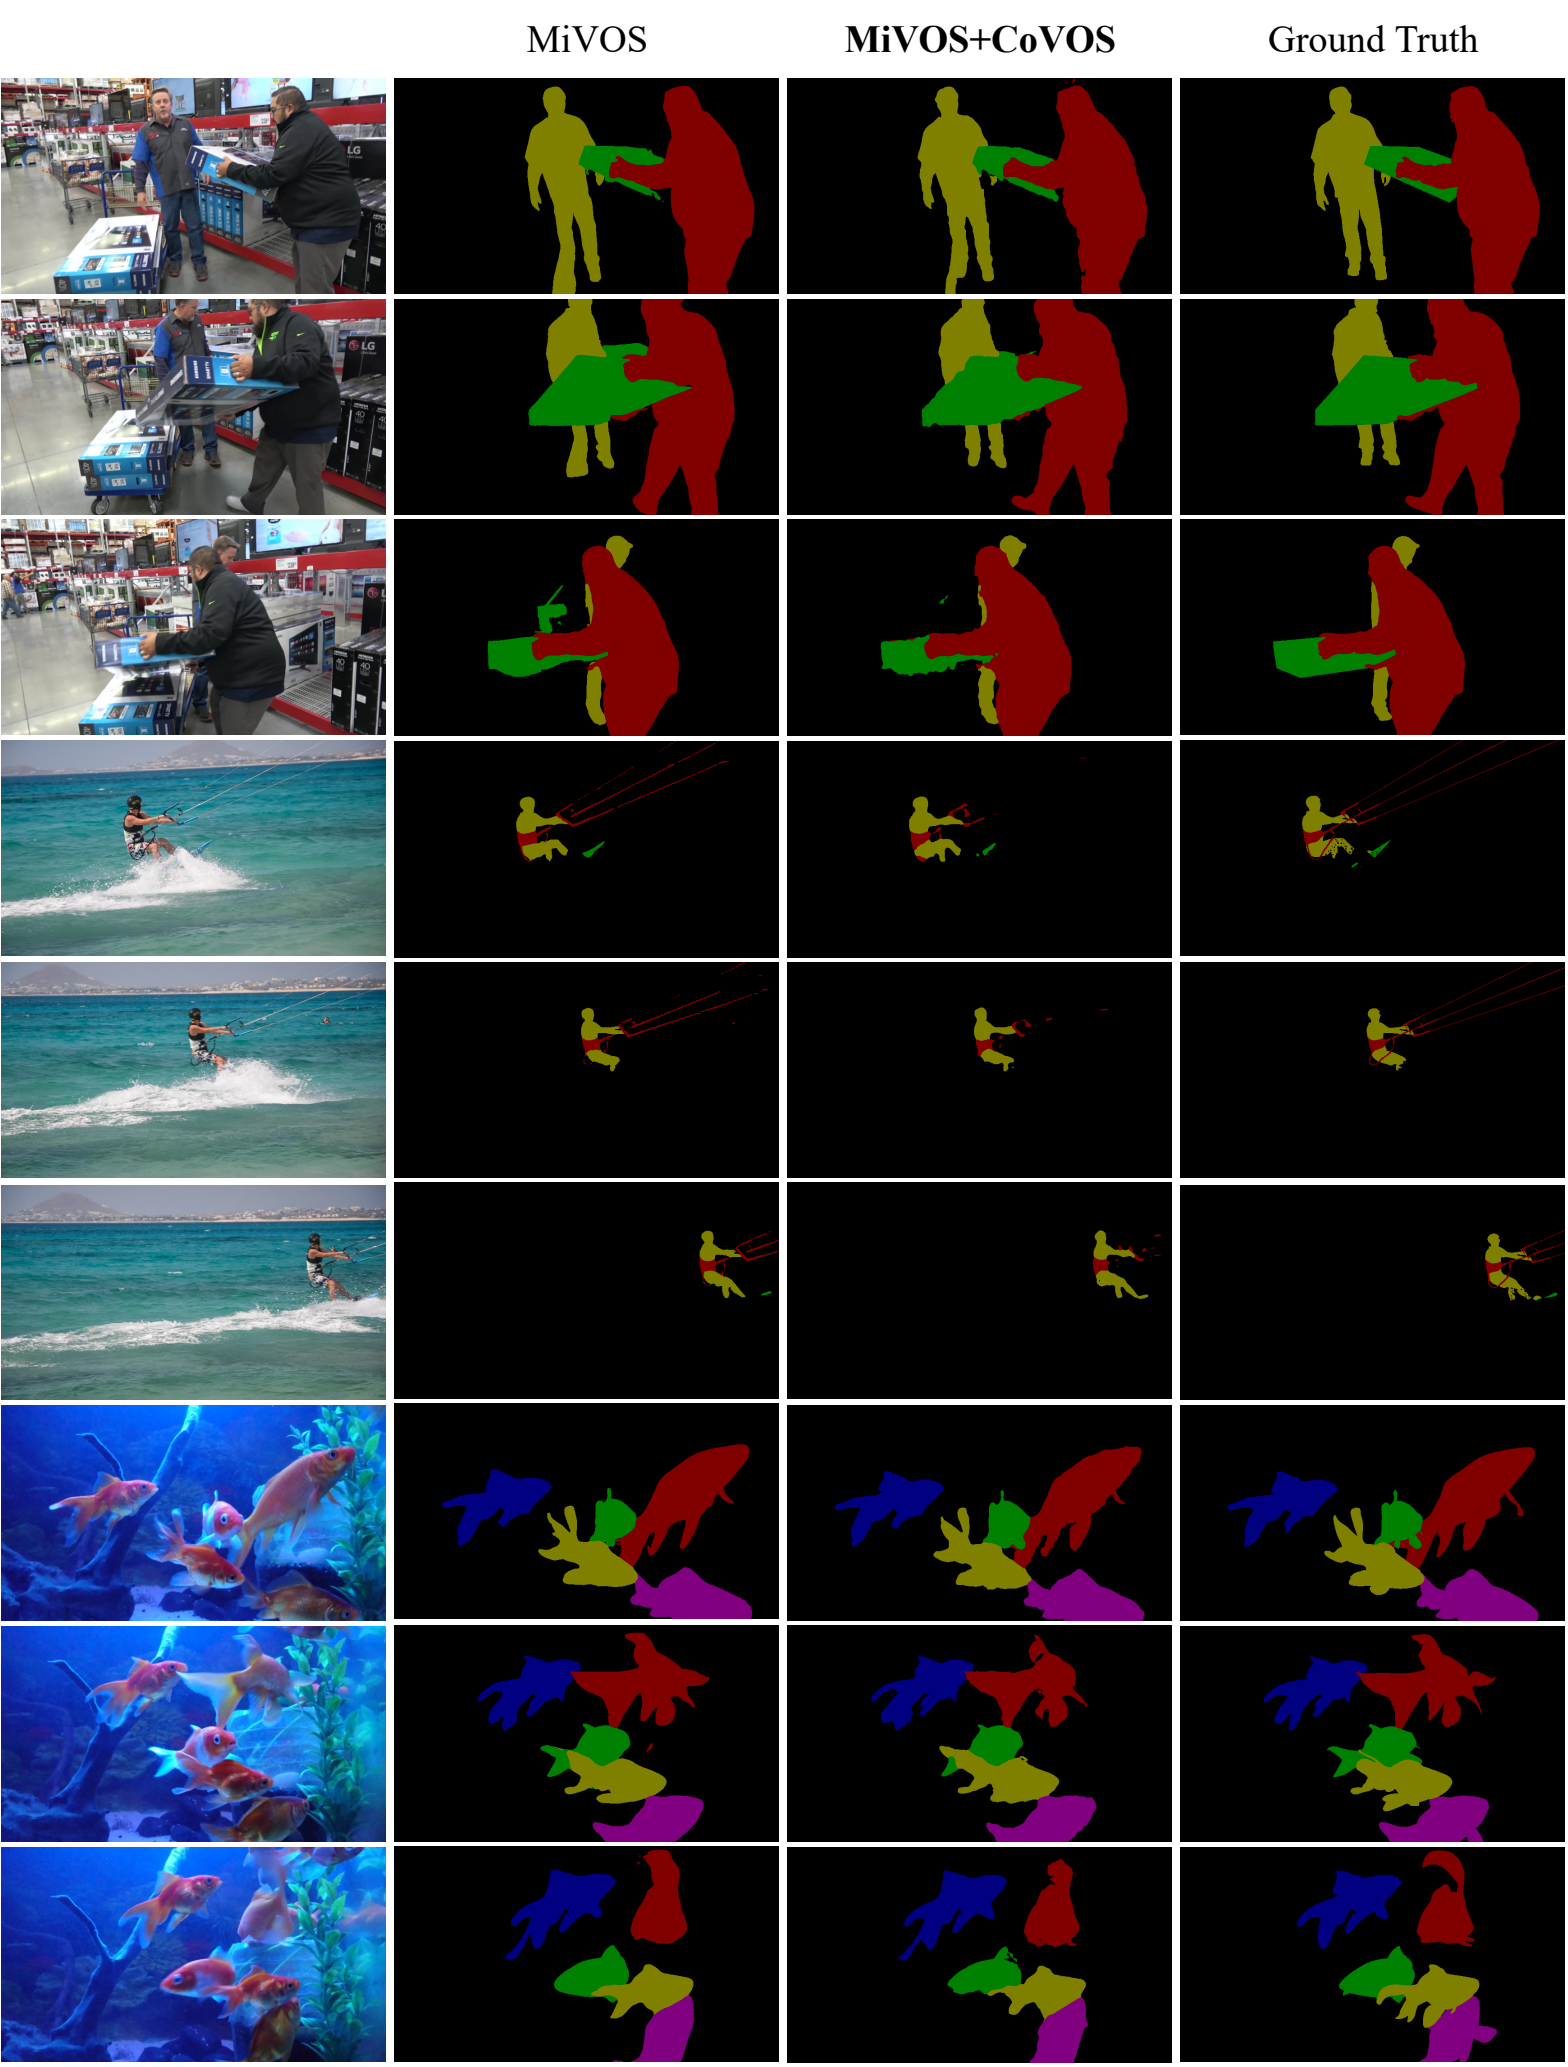 |
| 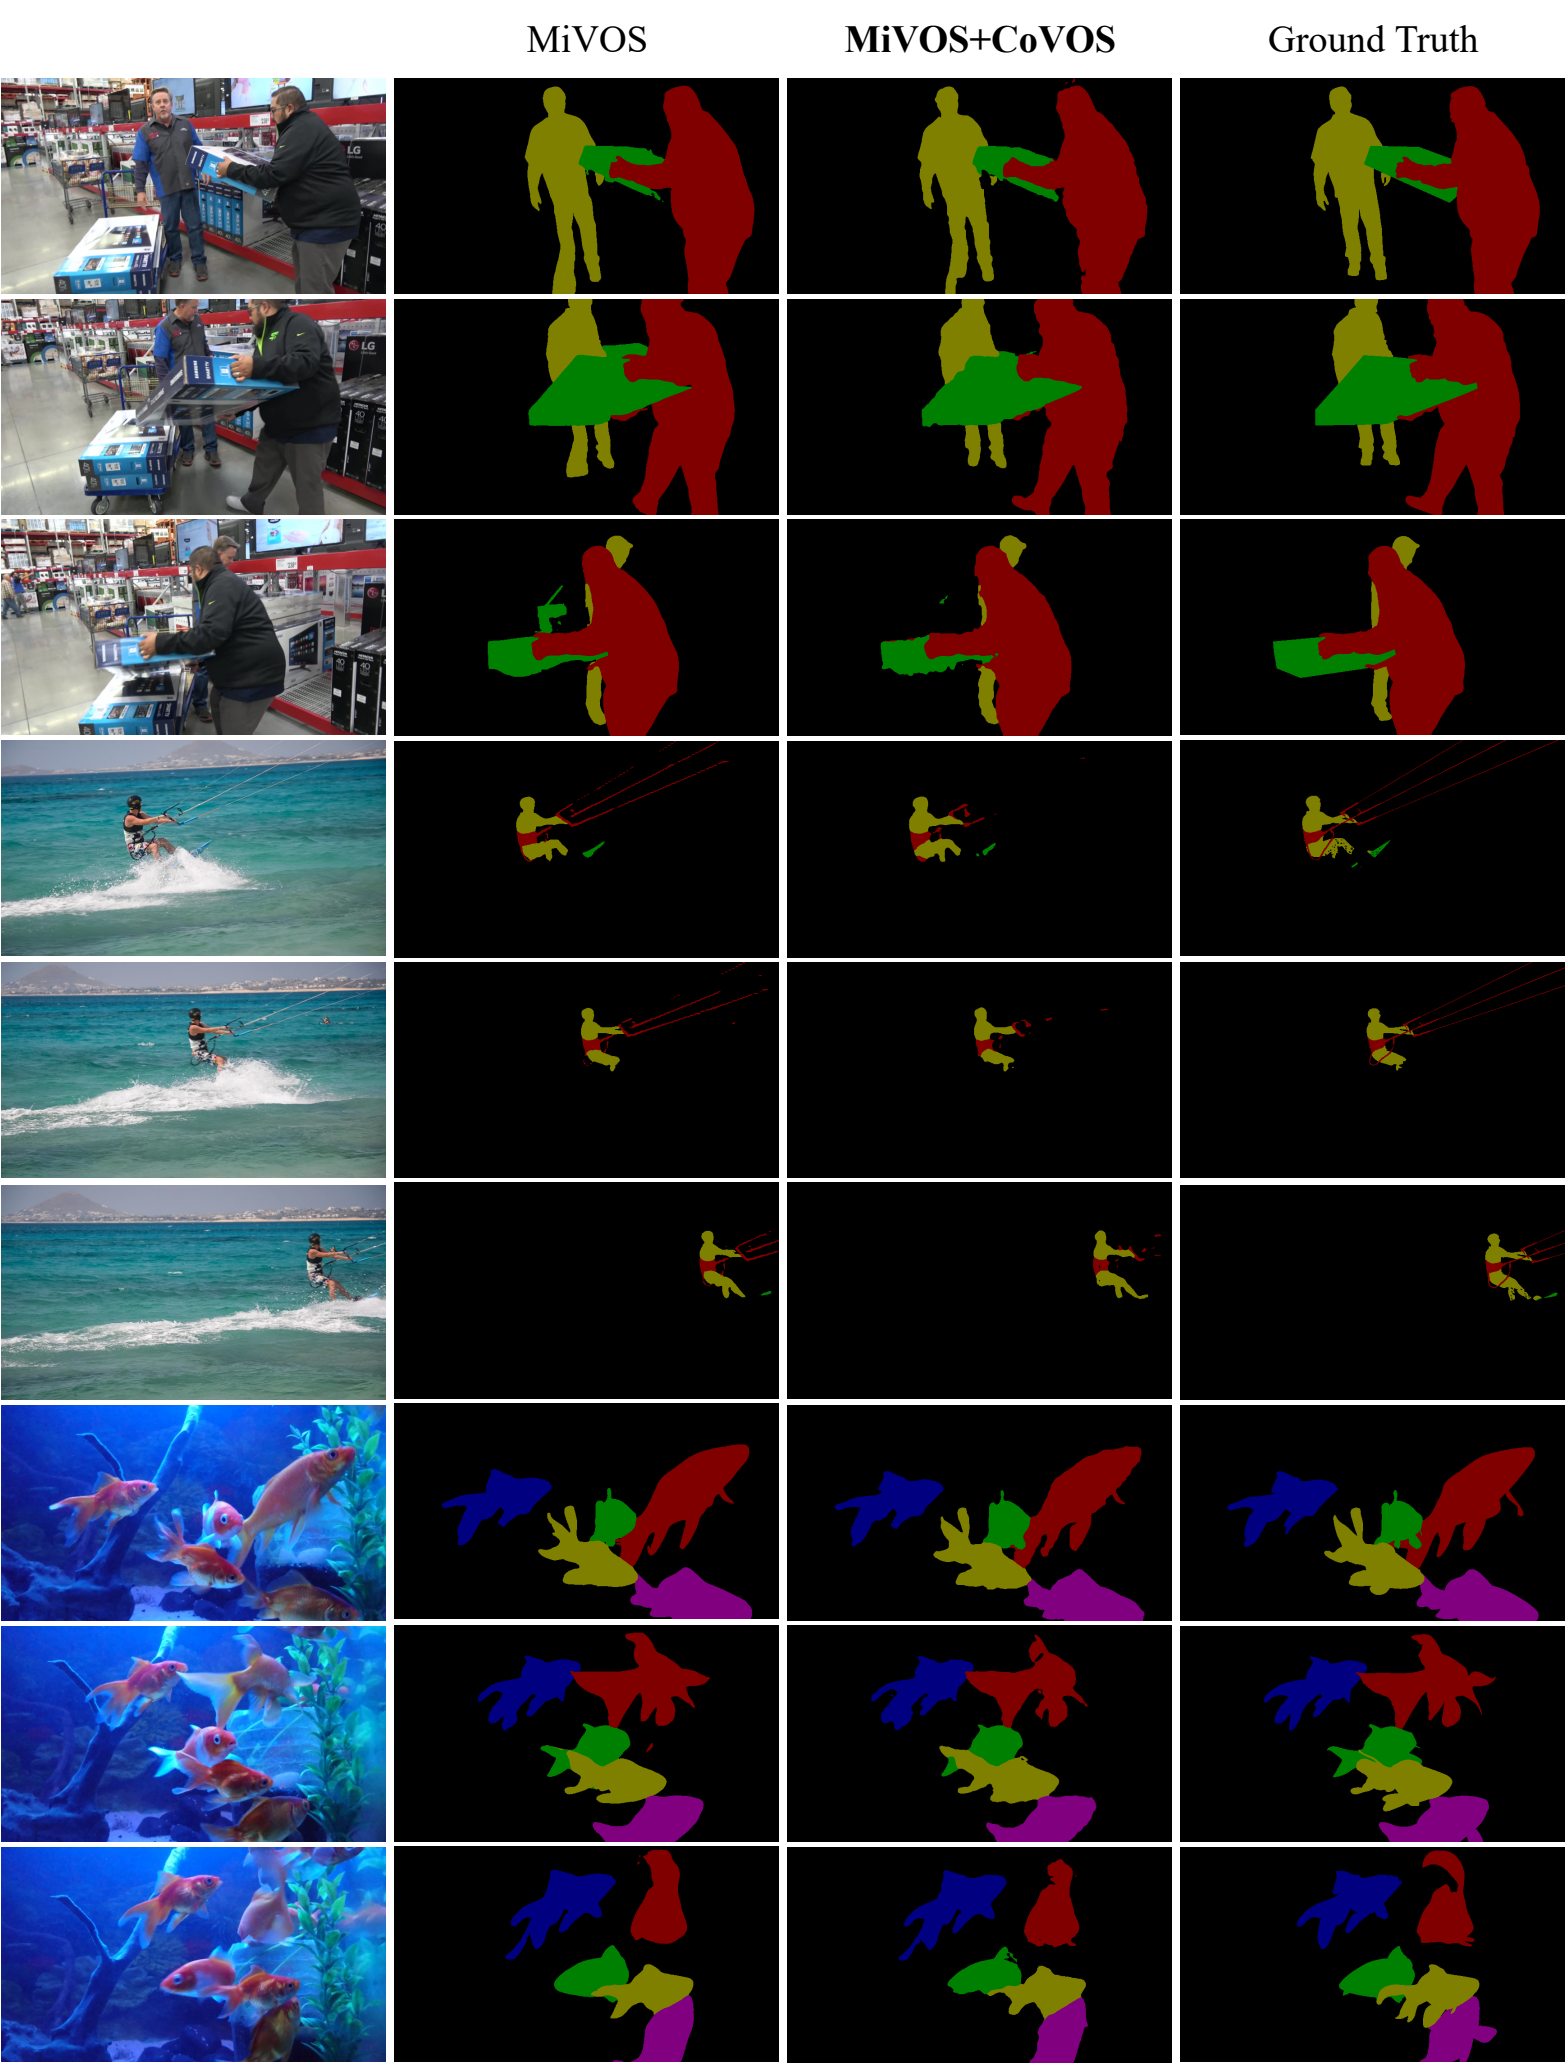 | 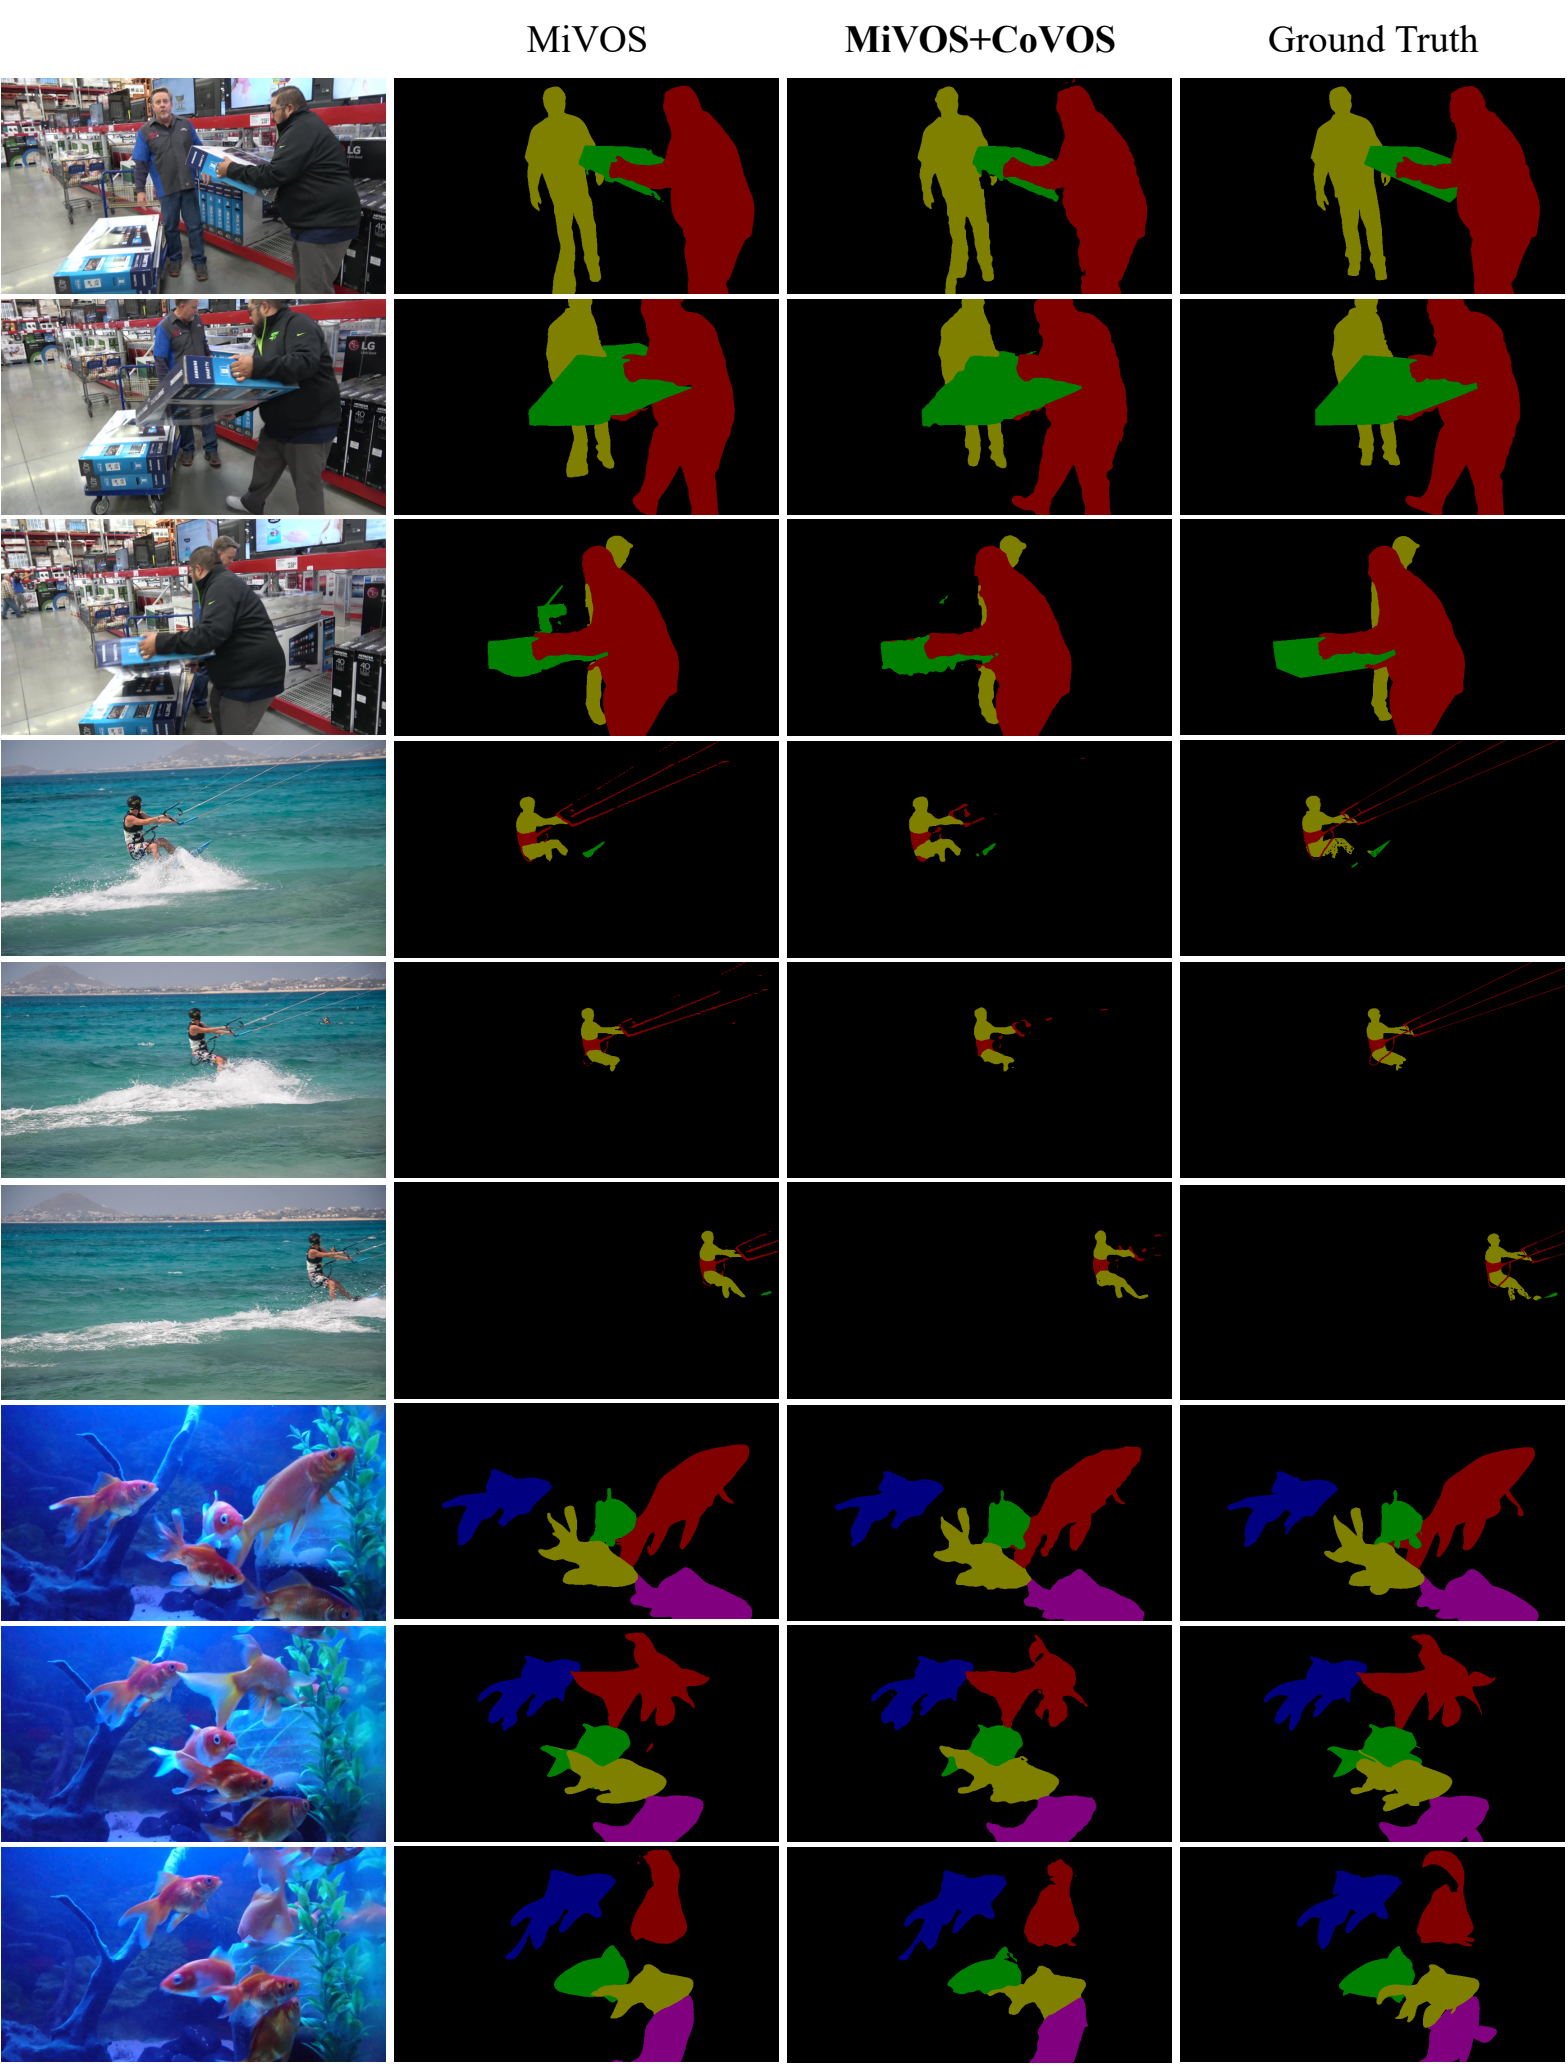 | 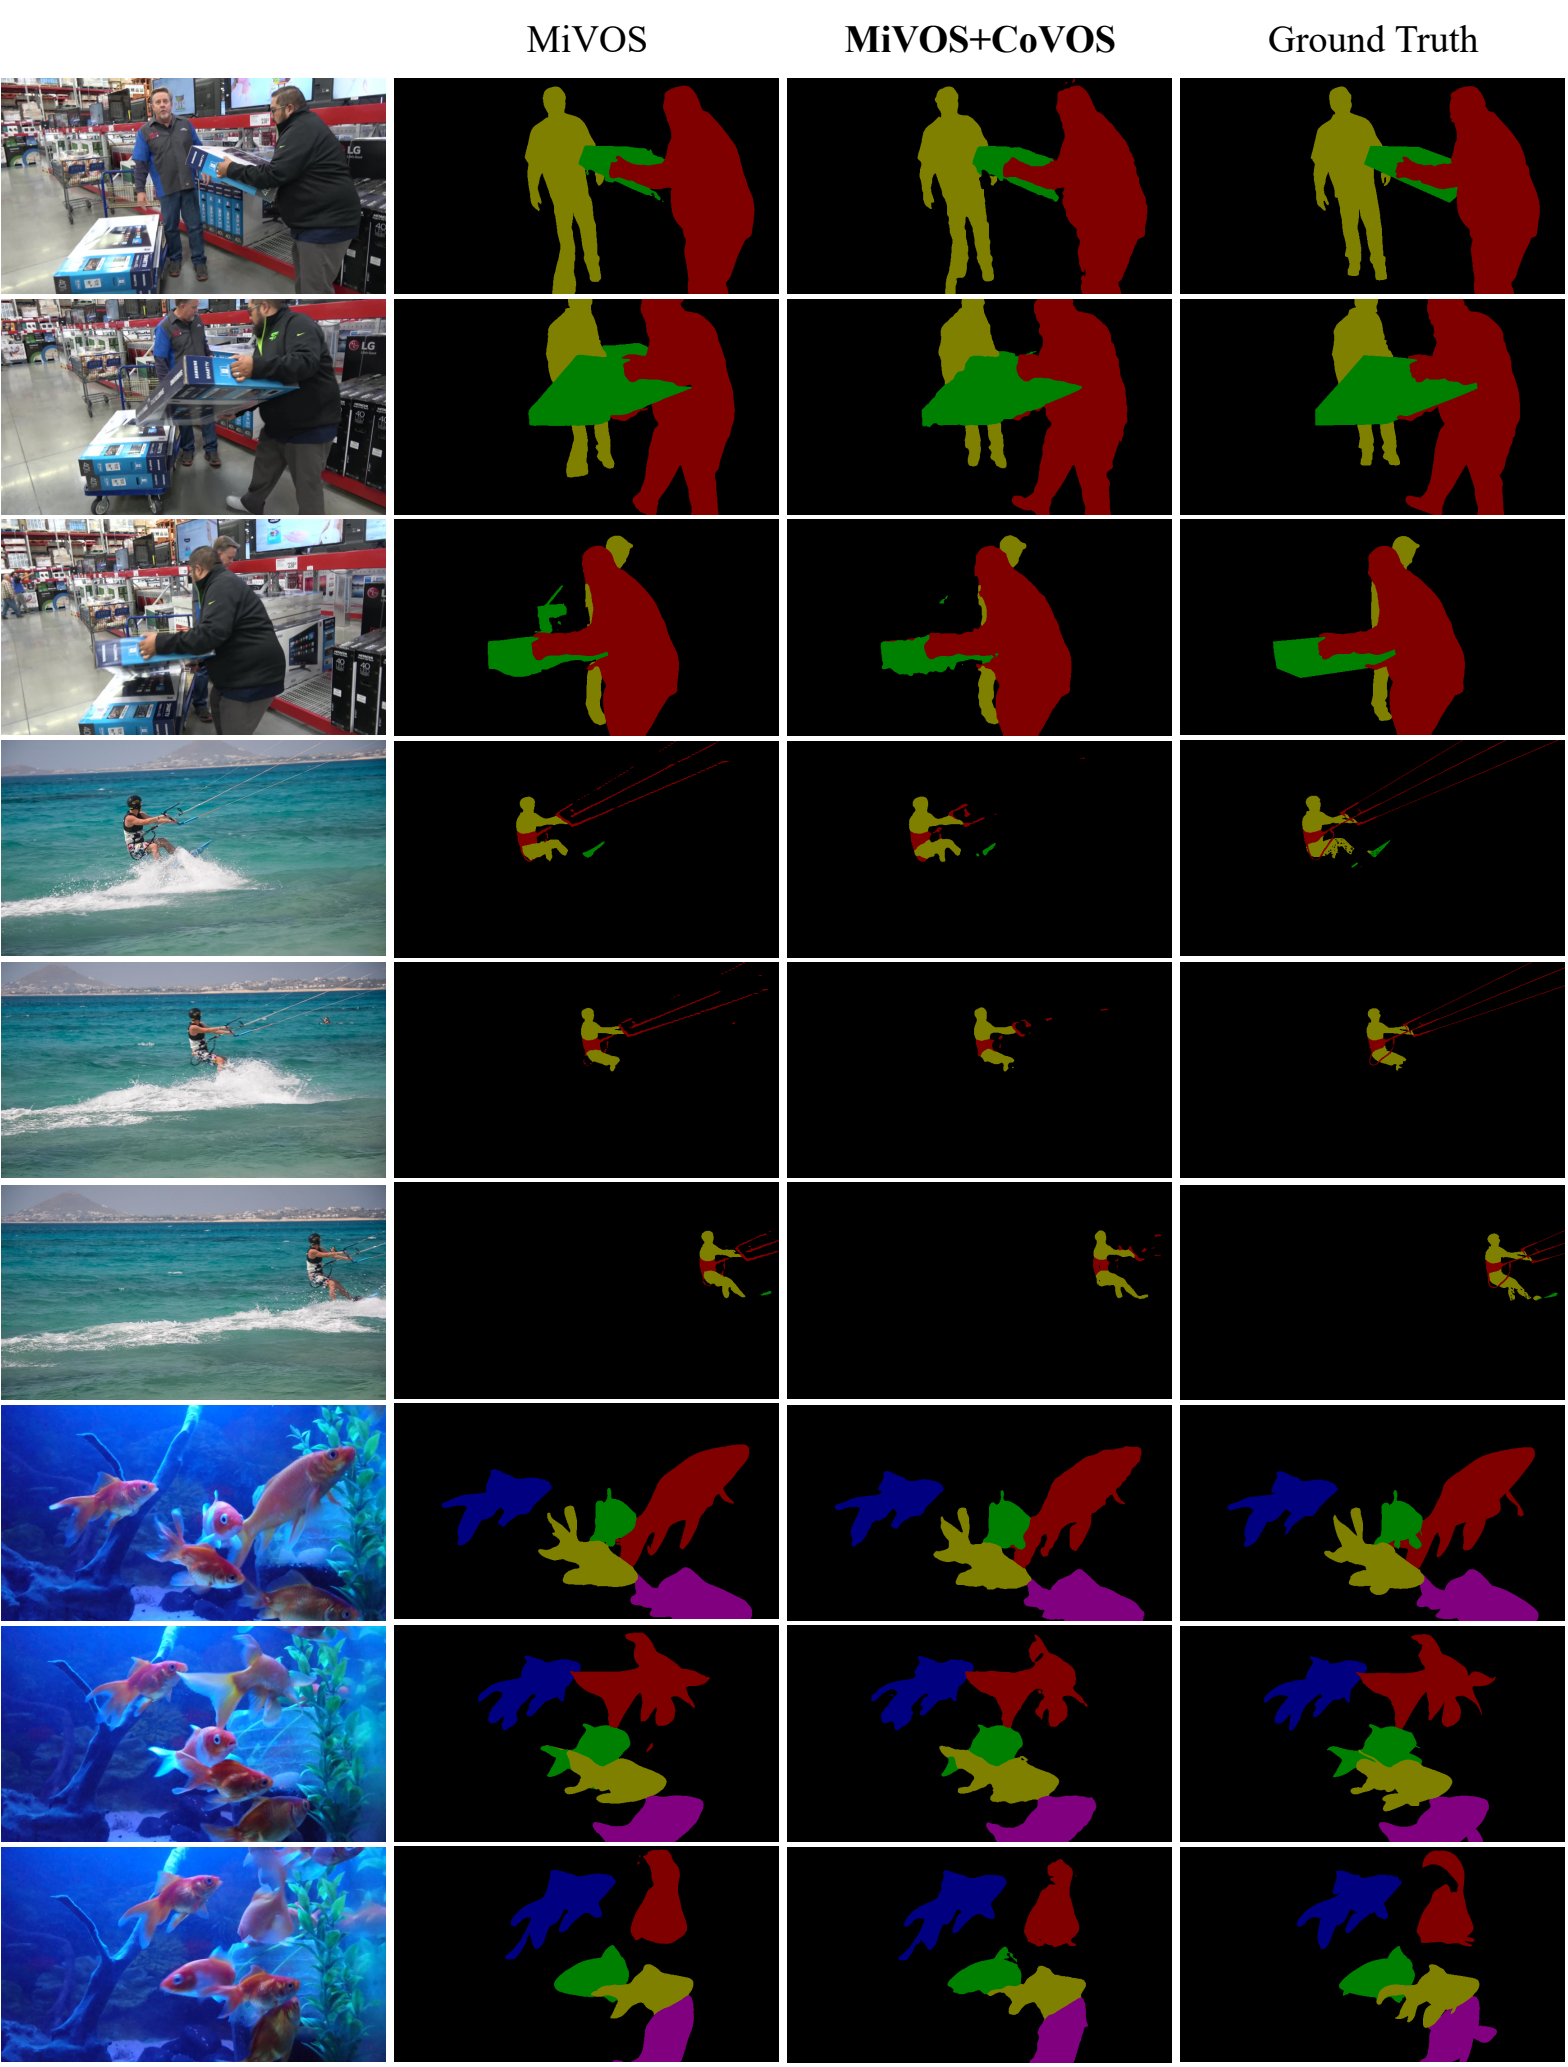 | 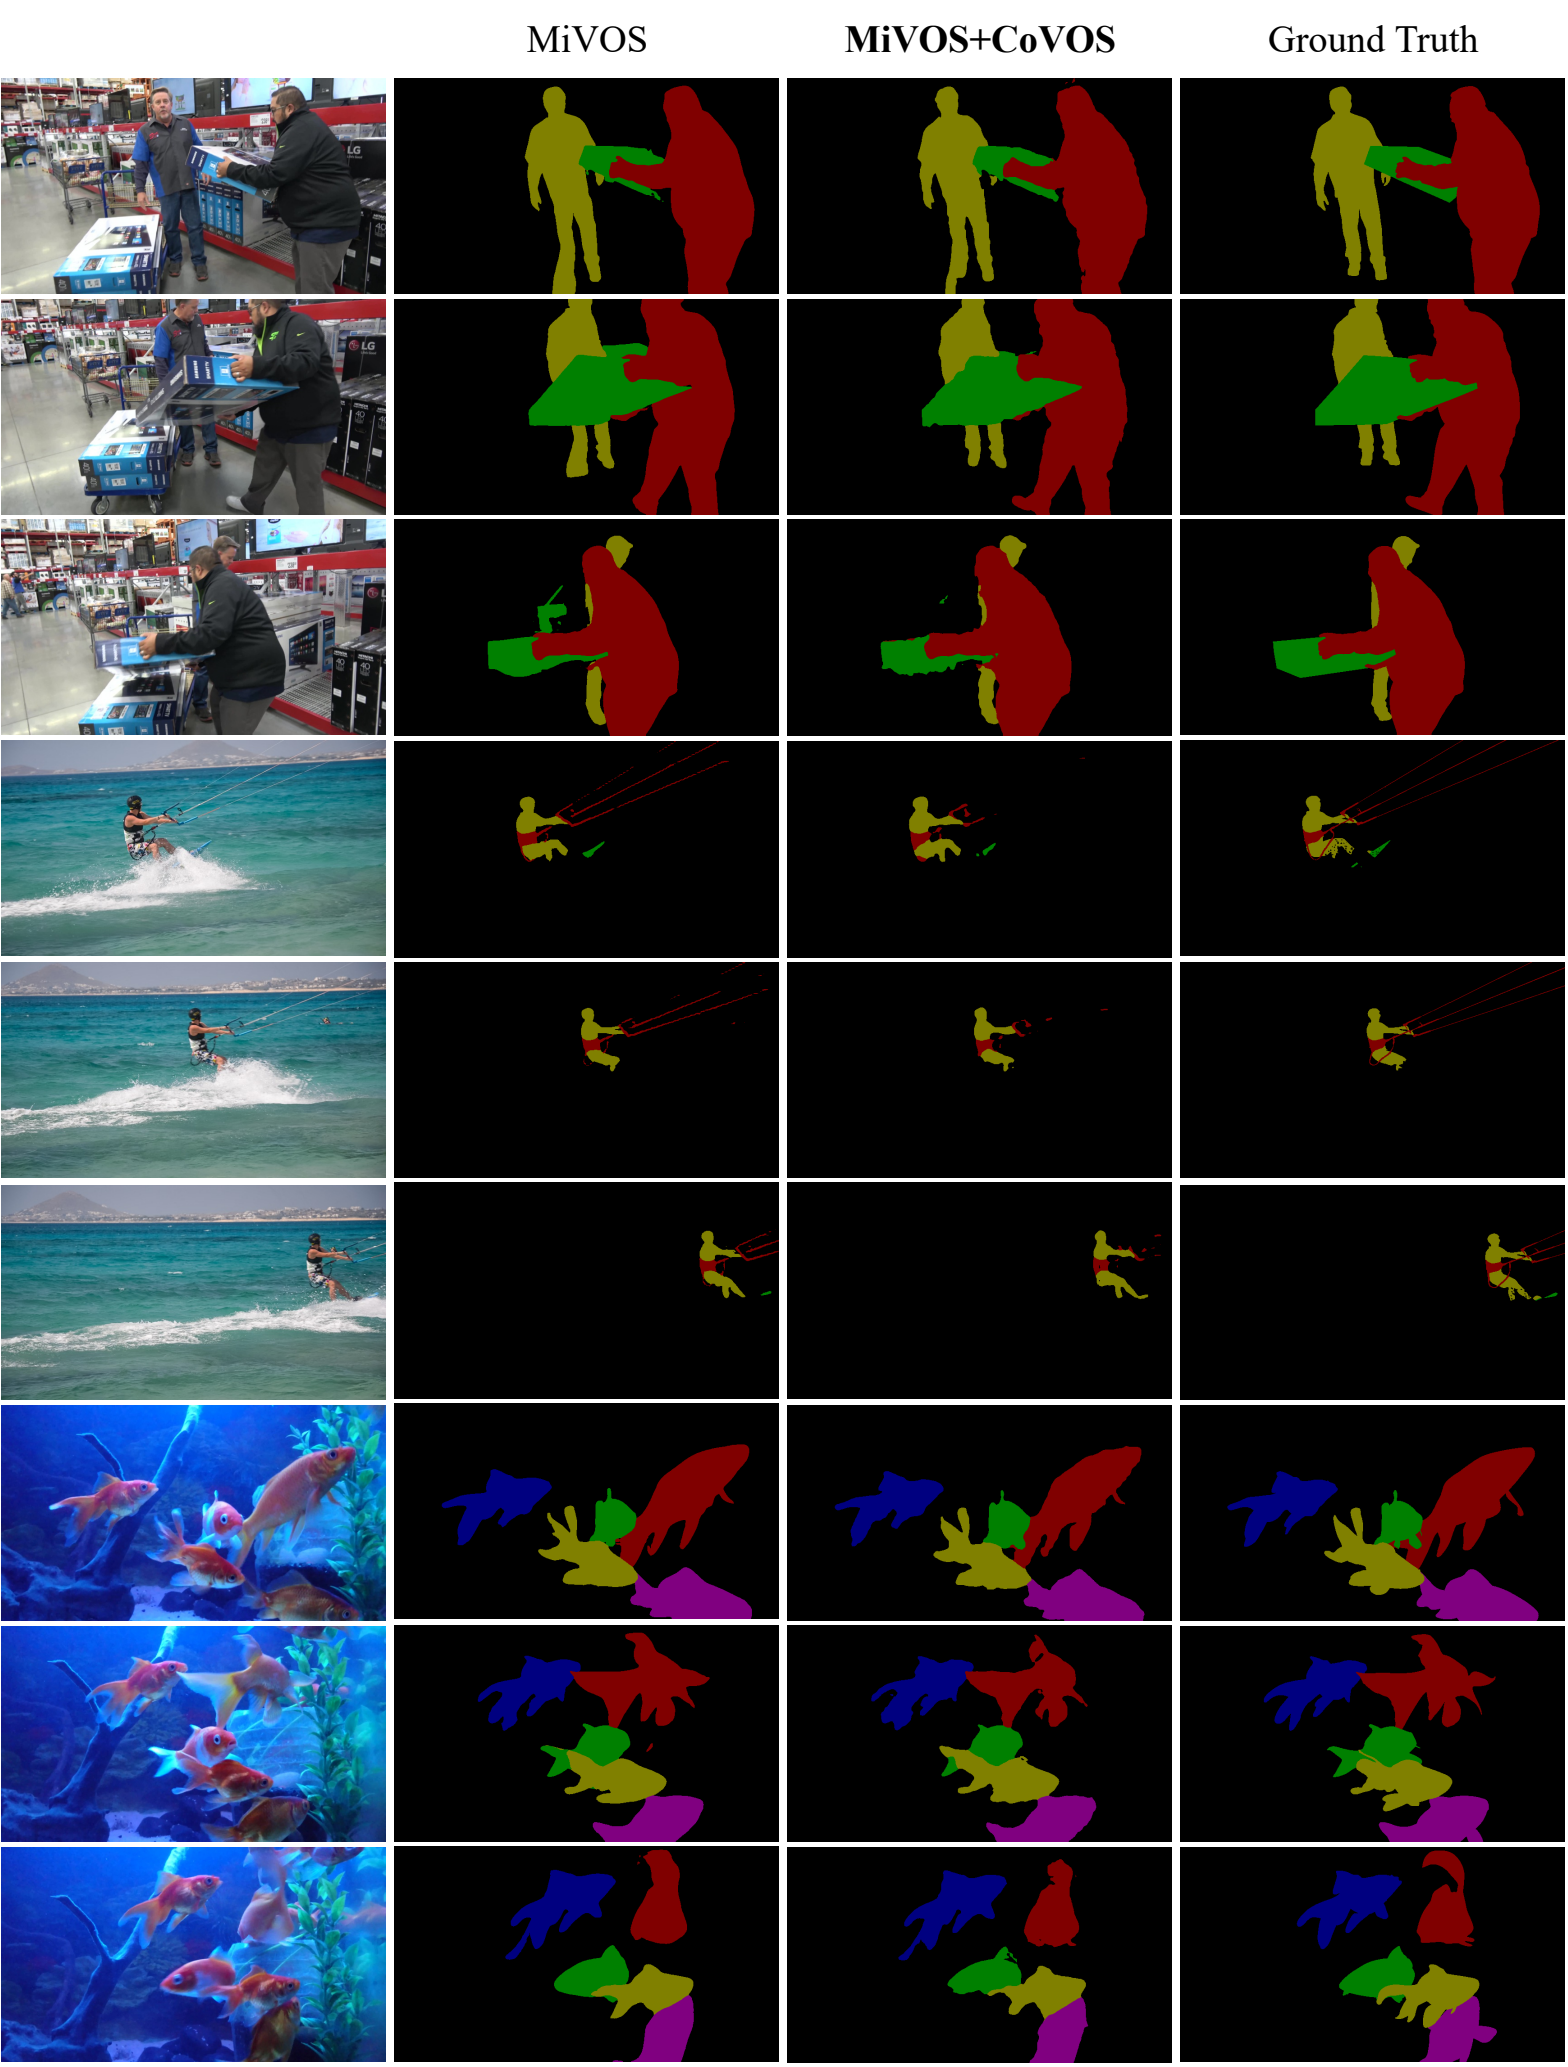 |
| 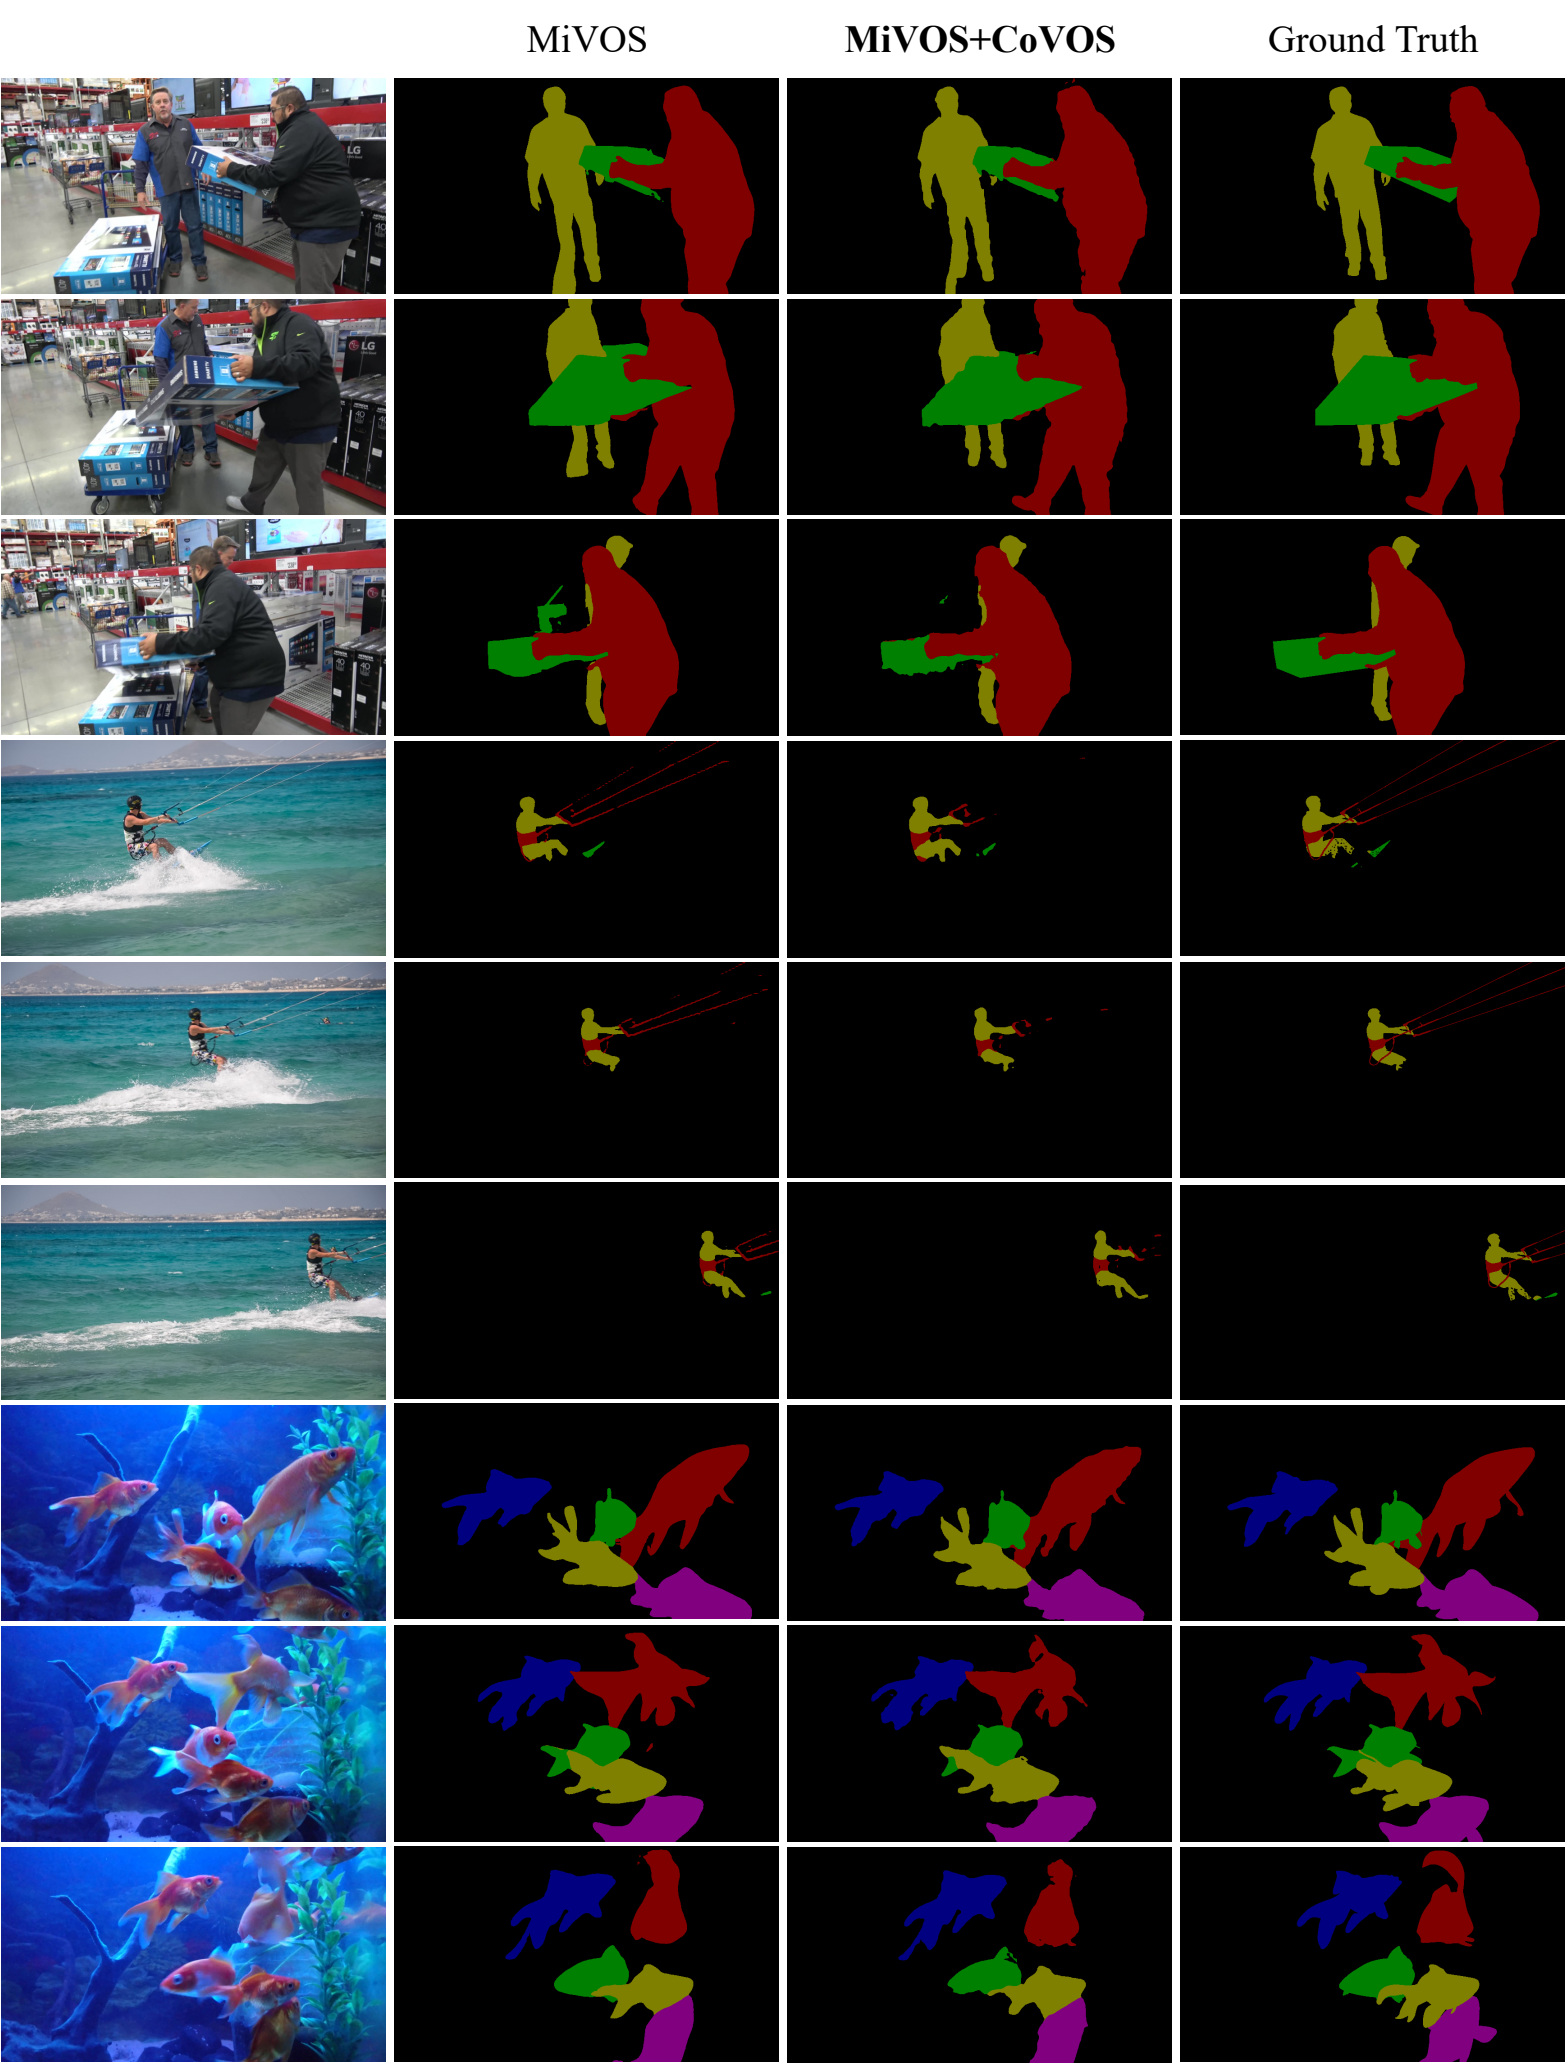 | 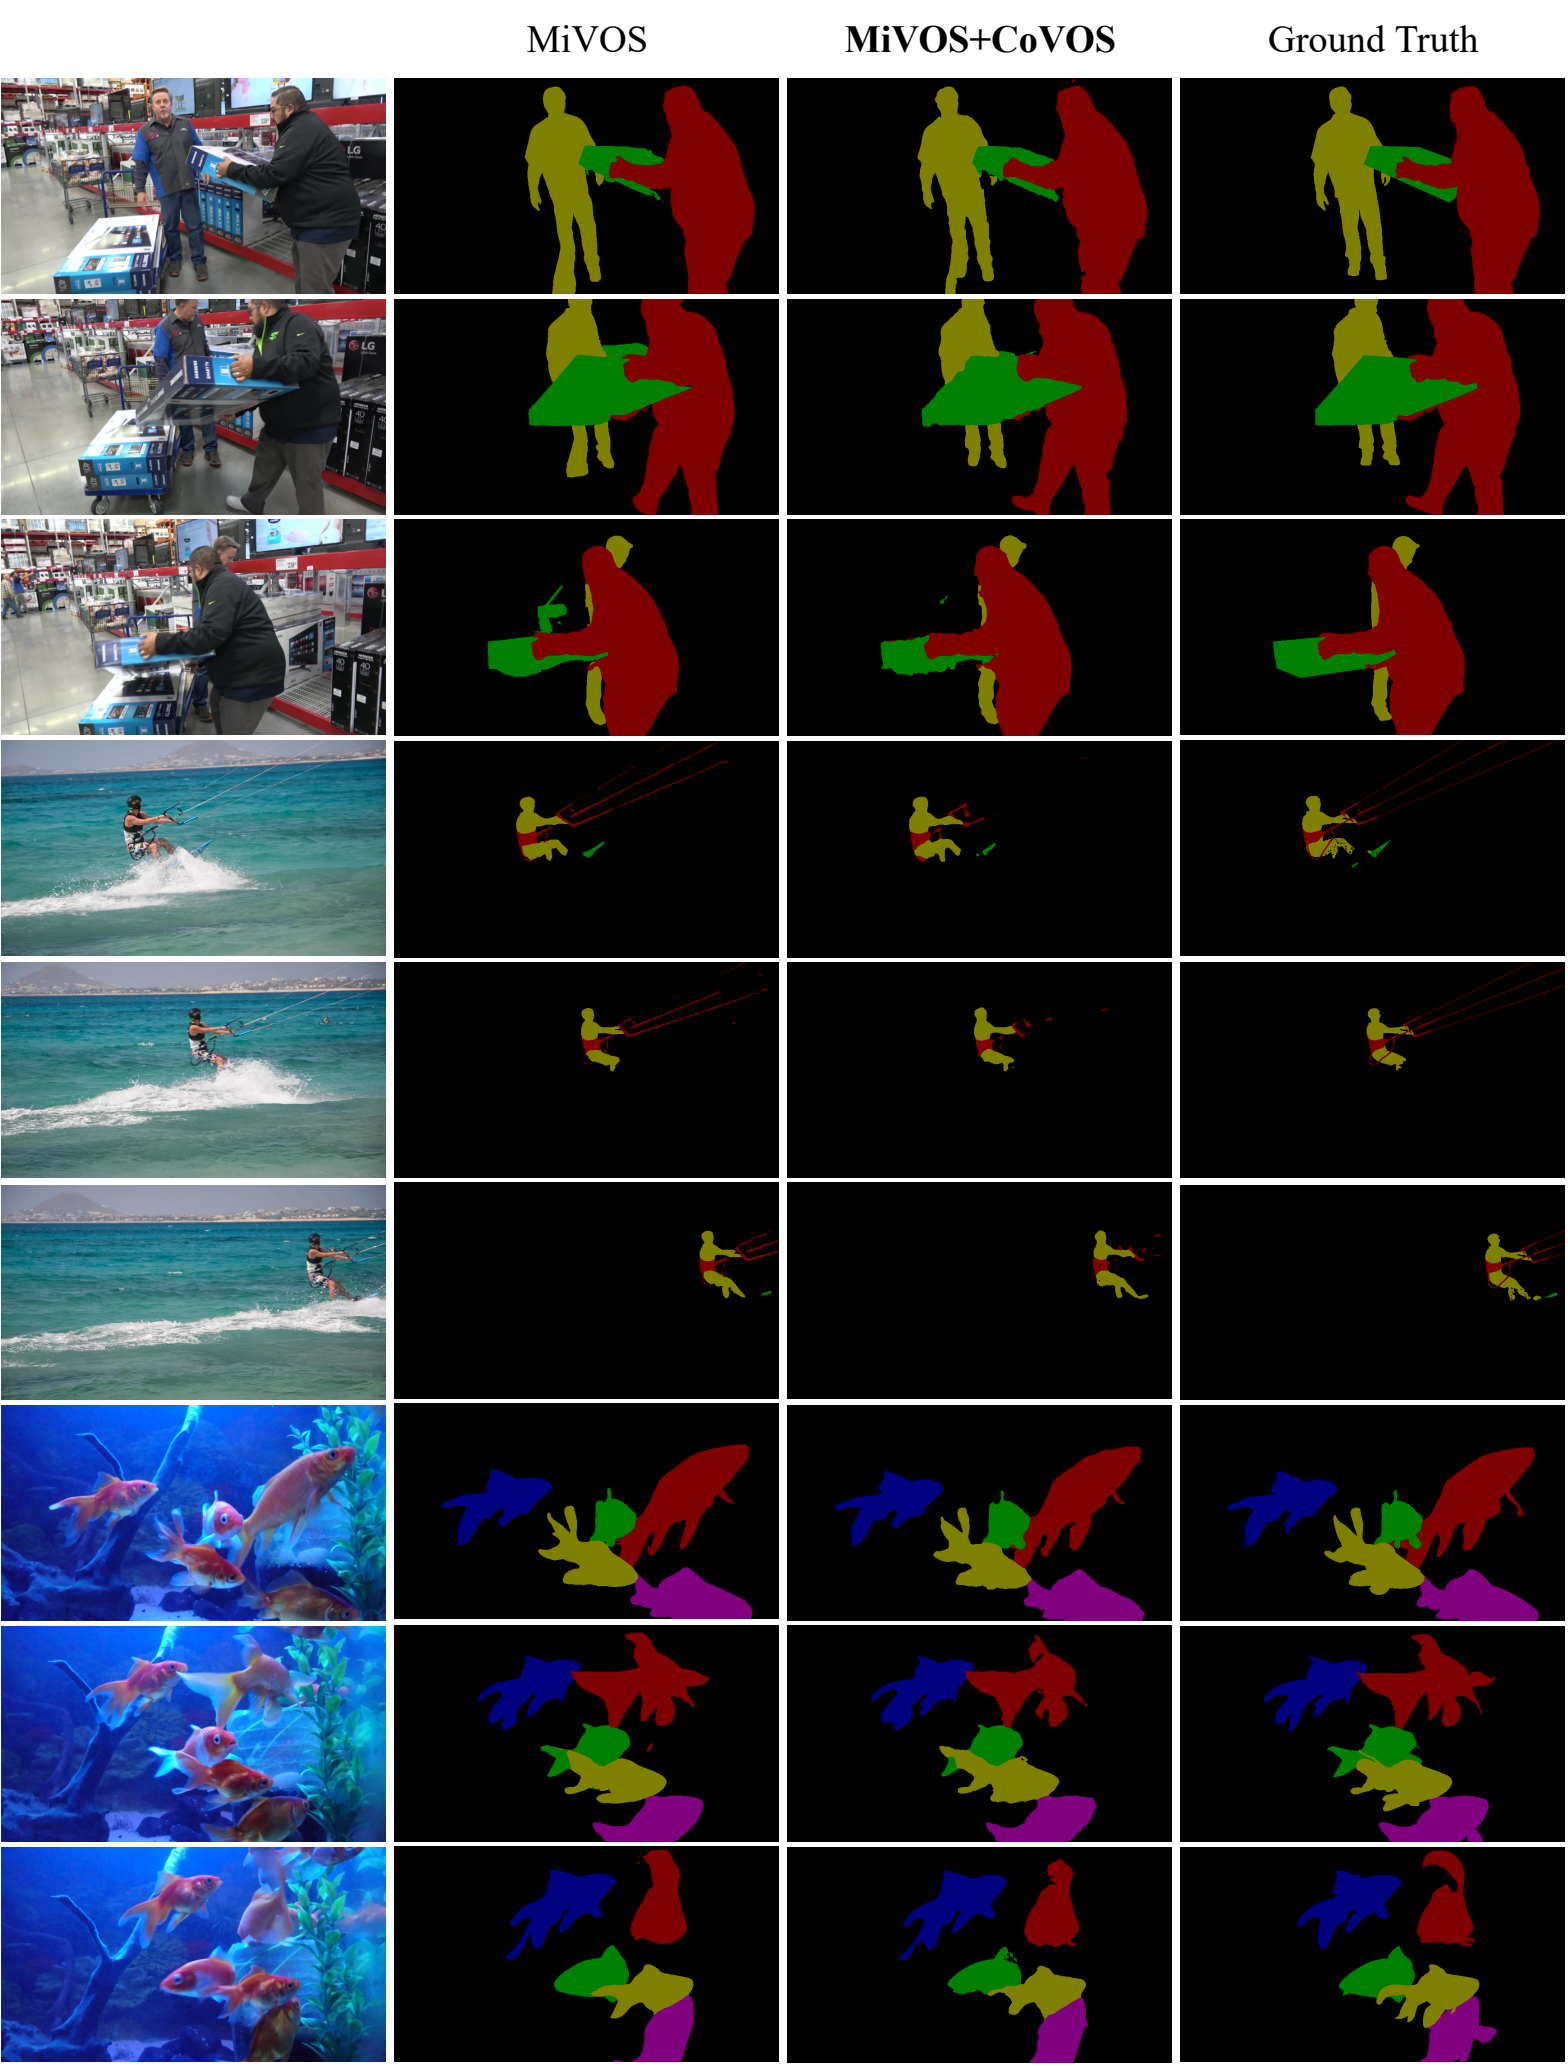 | 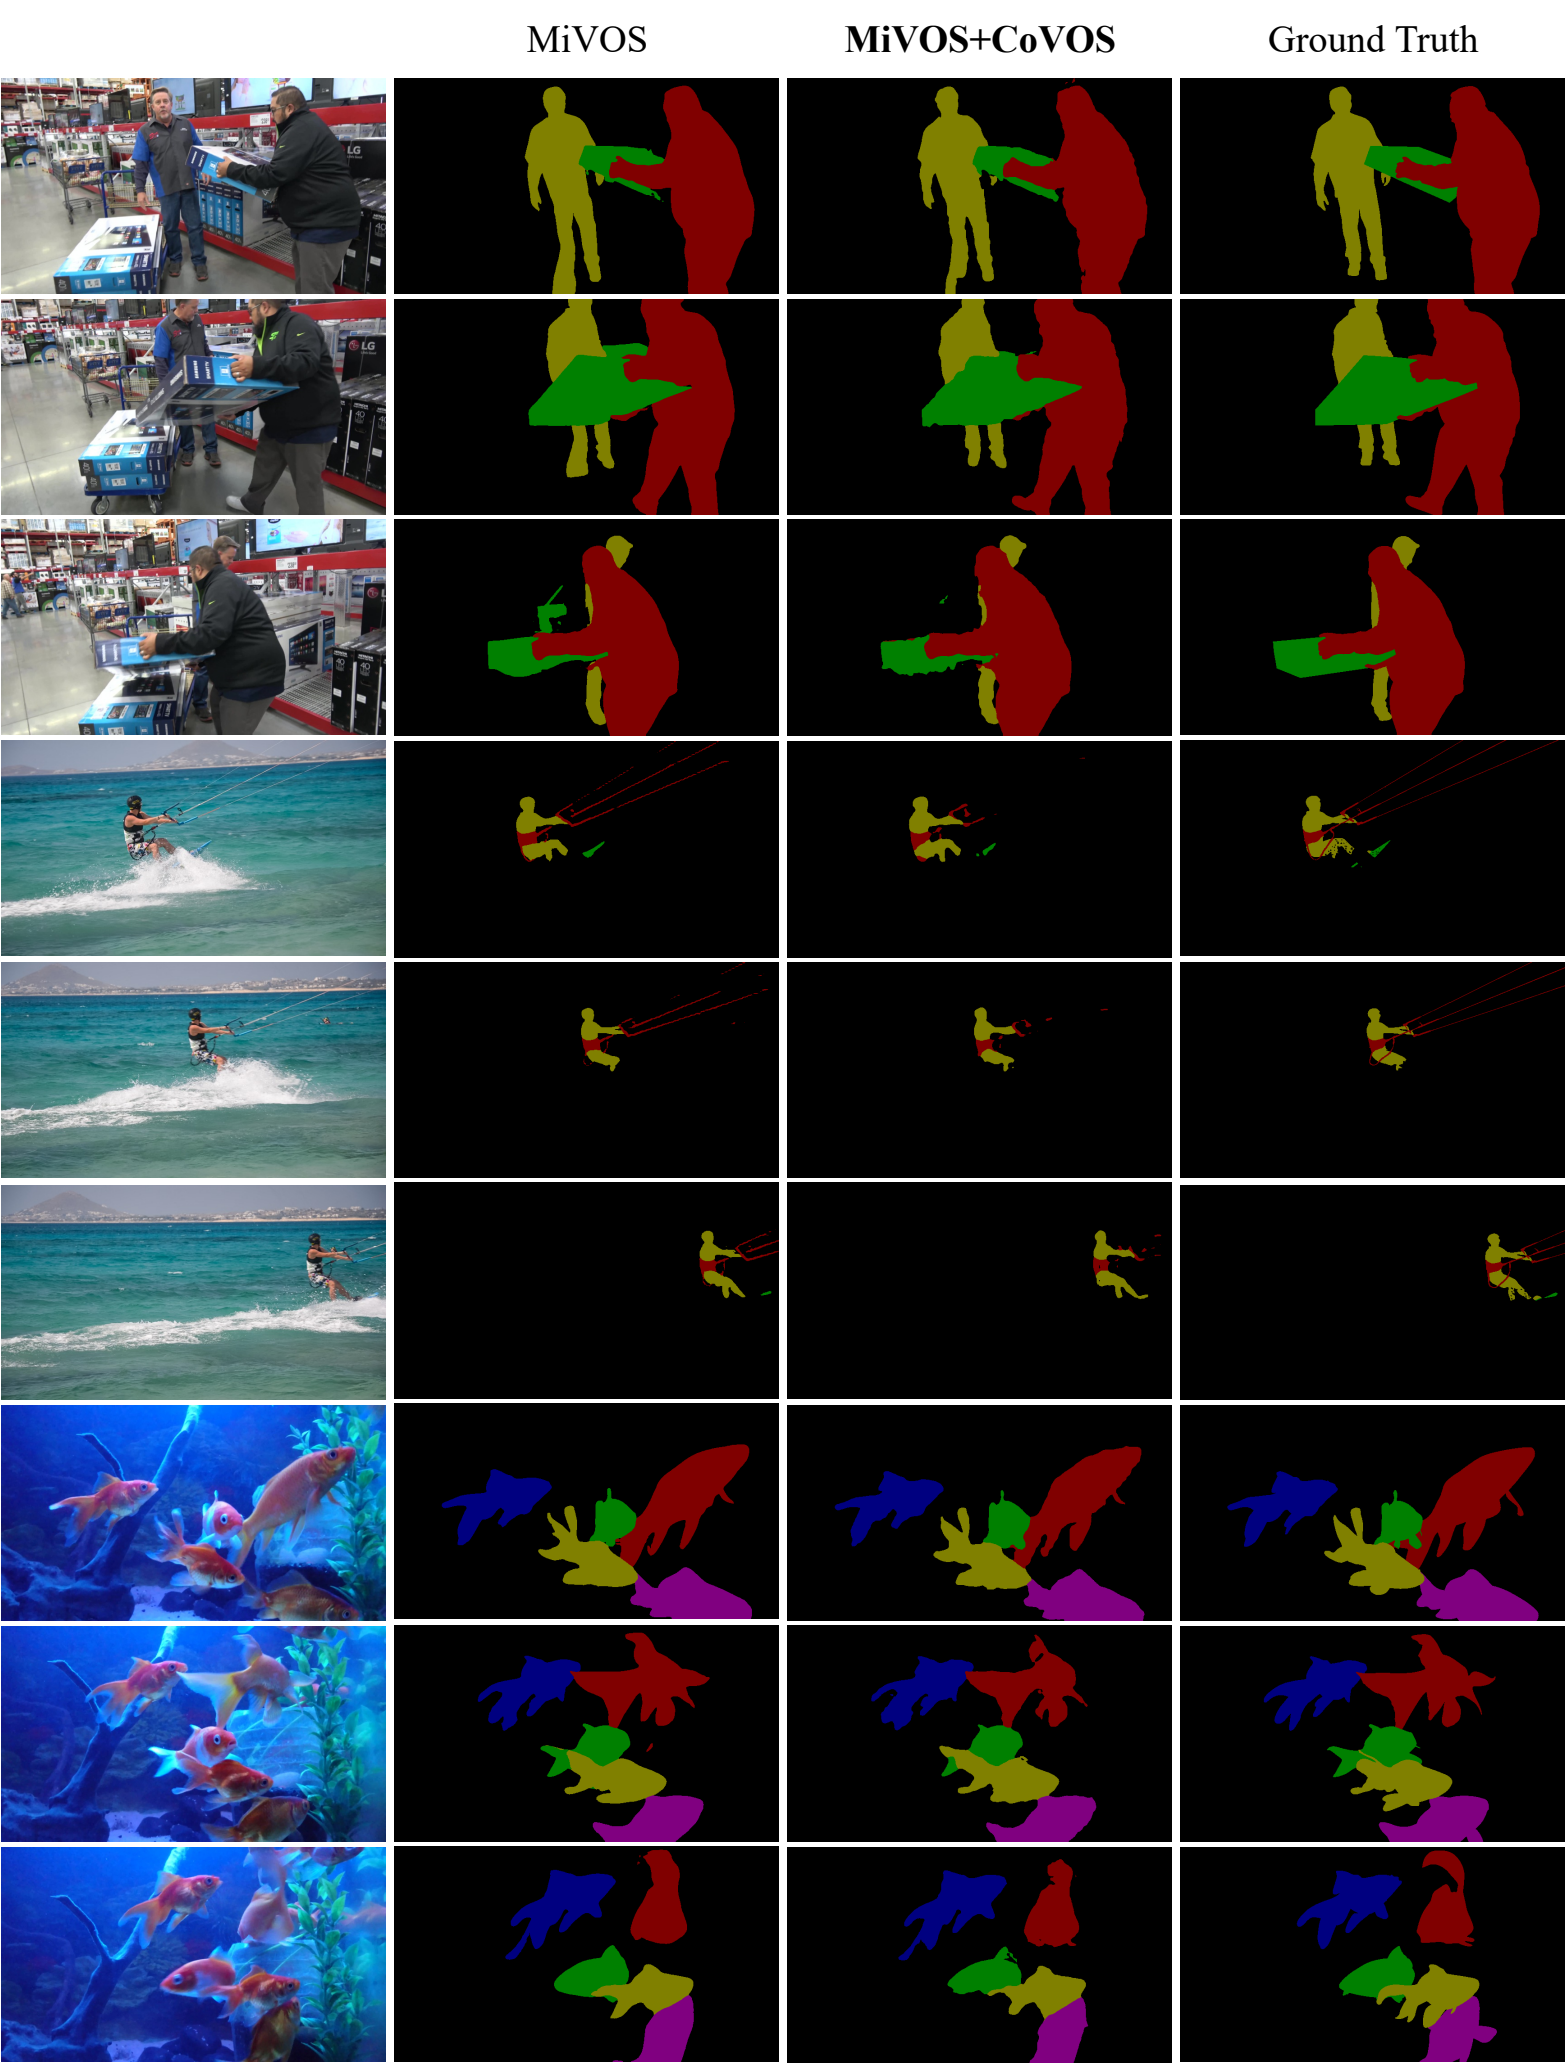 | 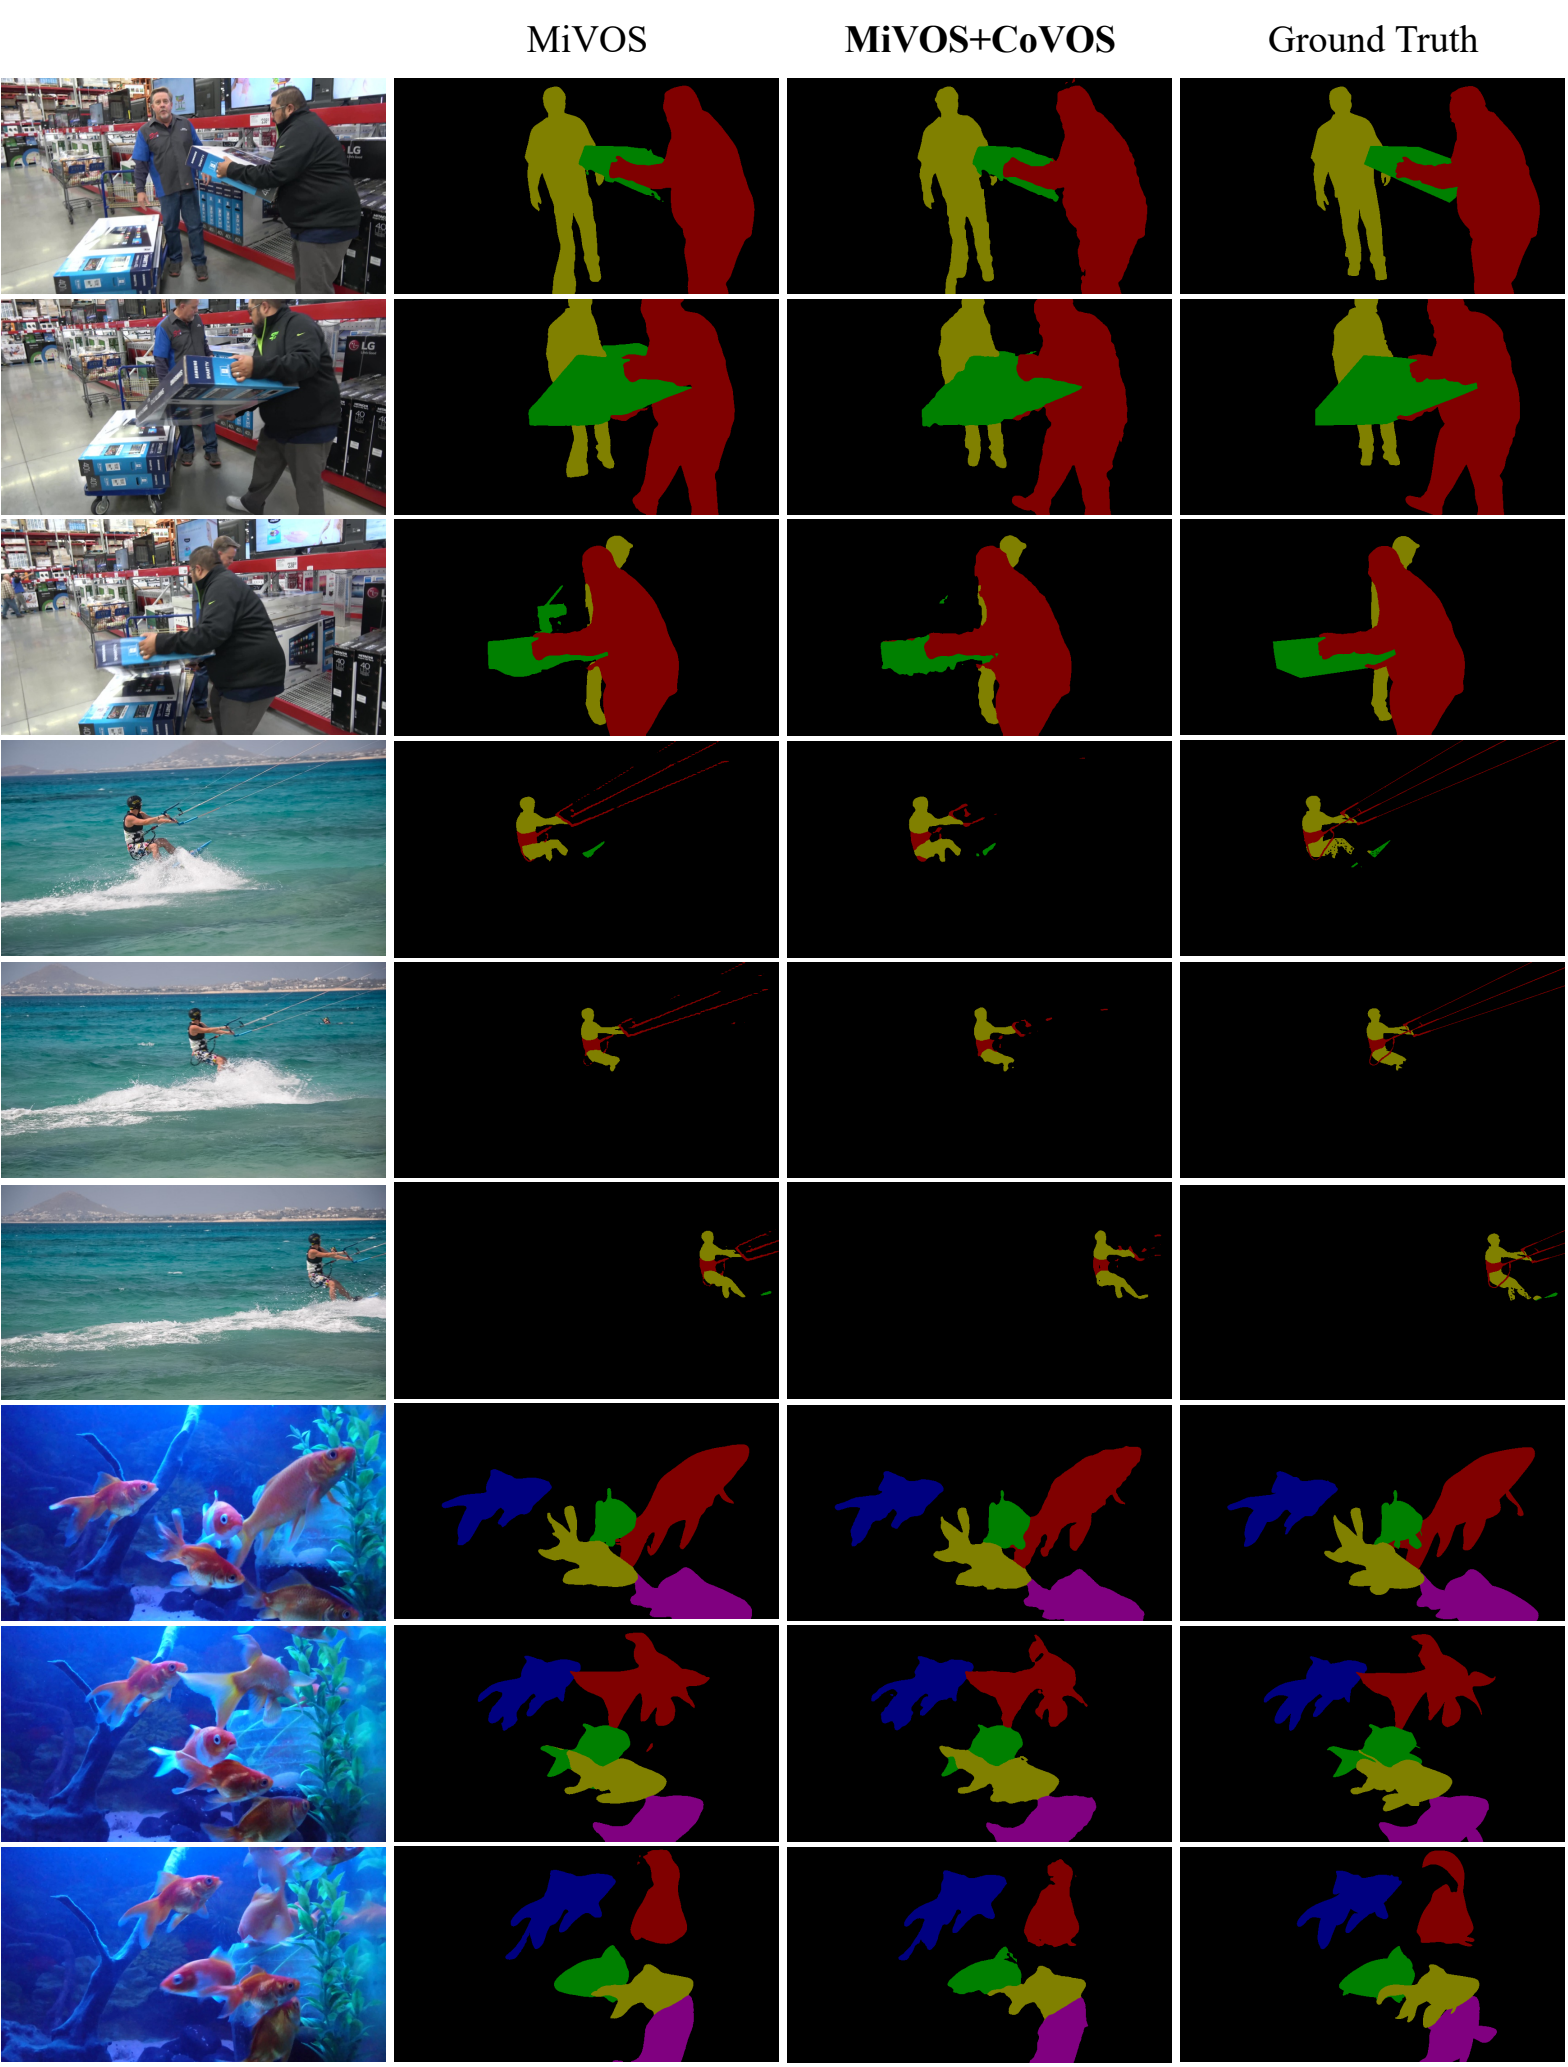 |
| 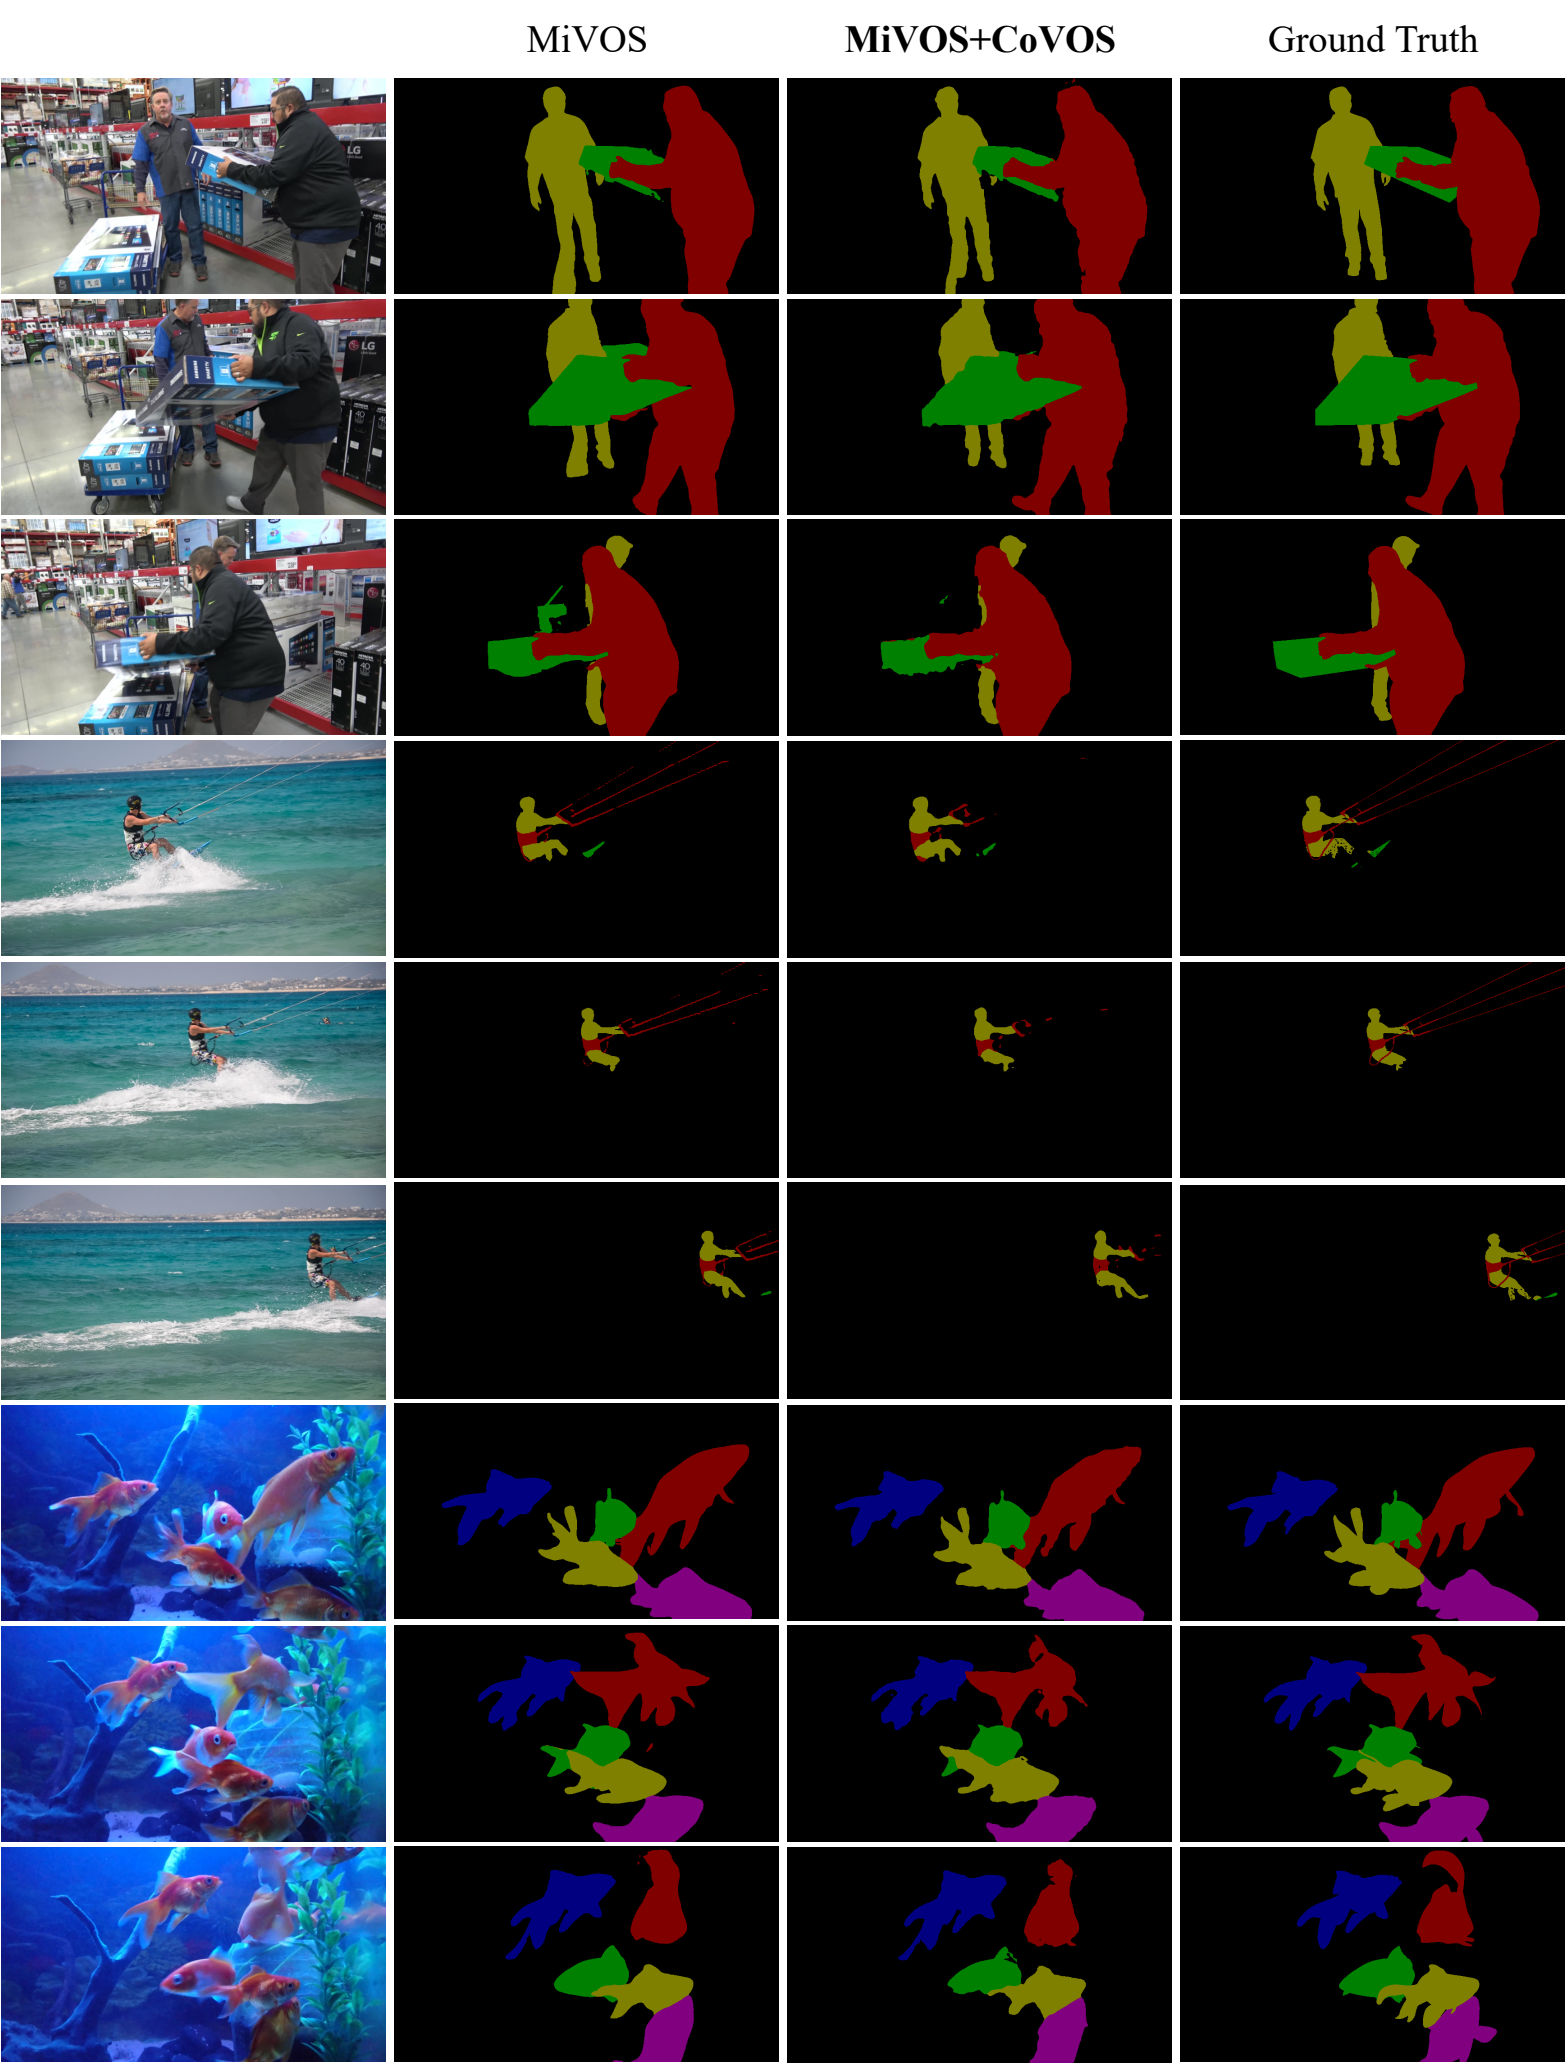 | 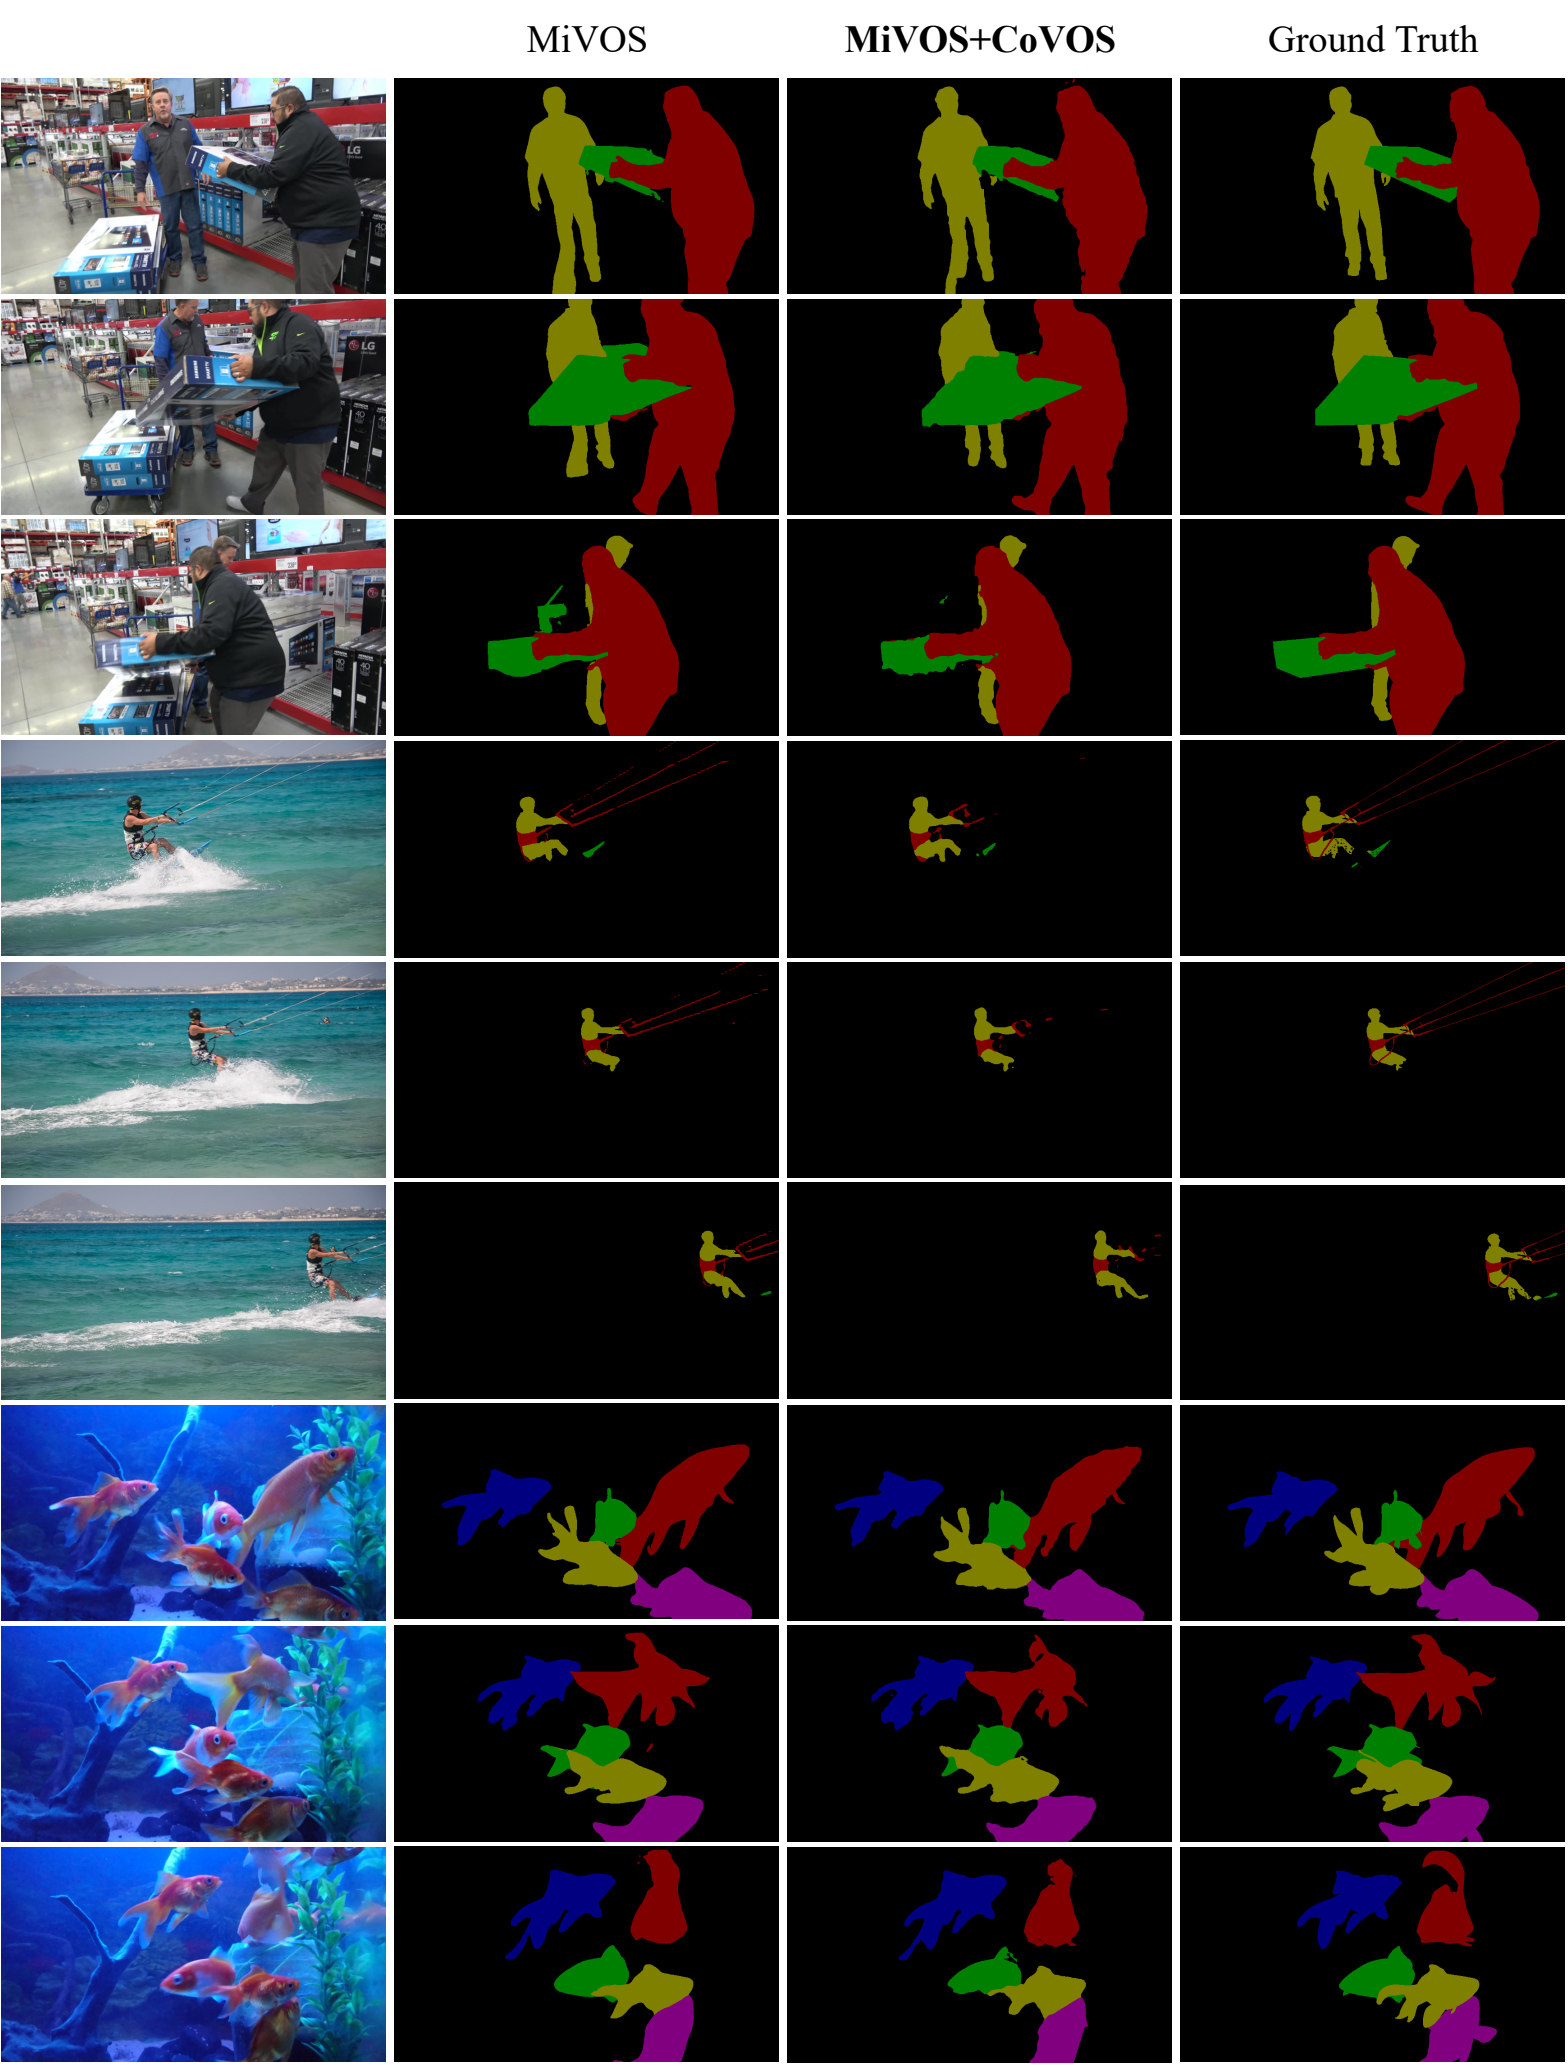 | 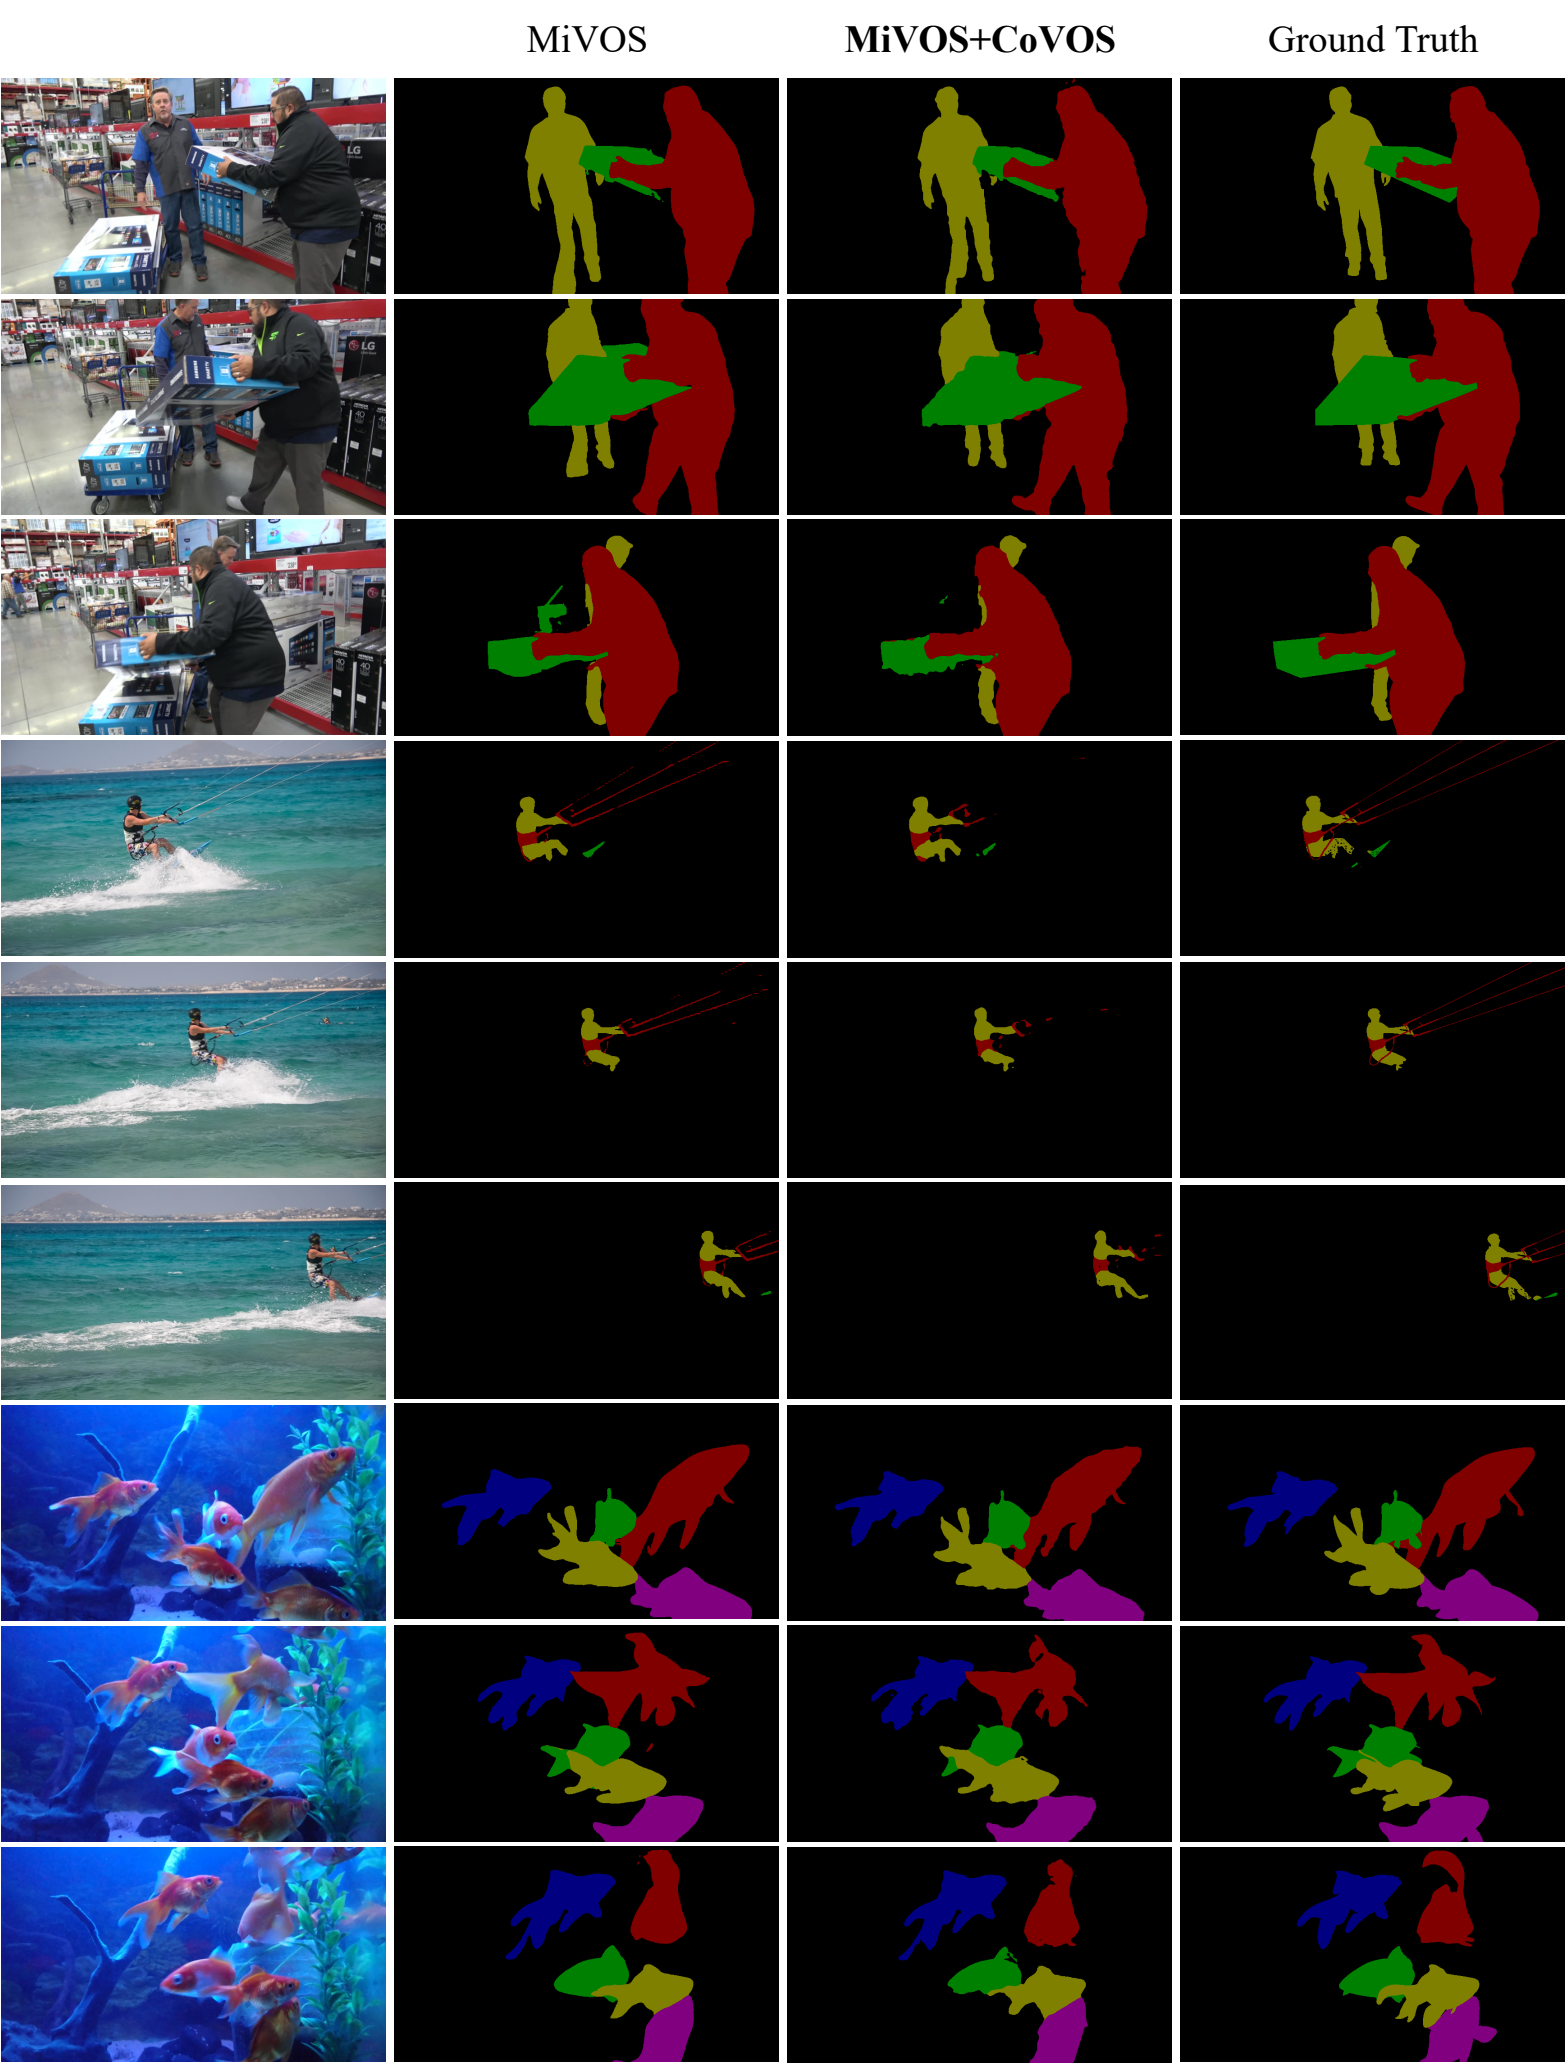 | 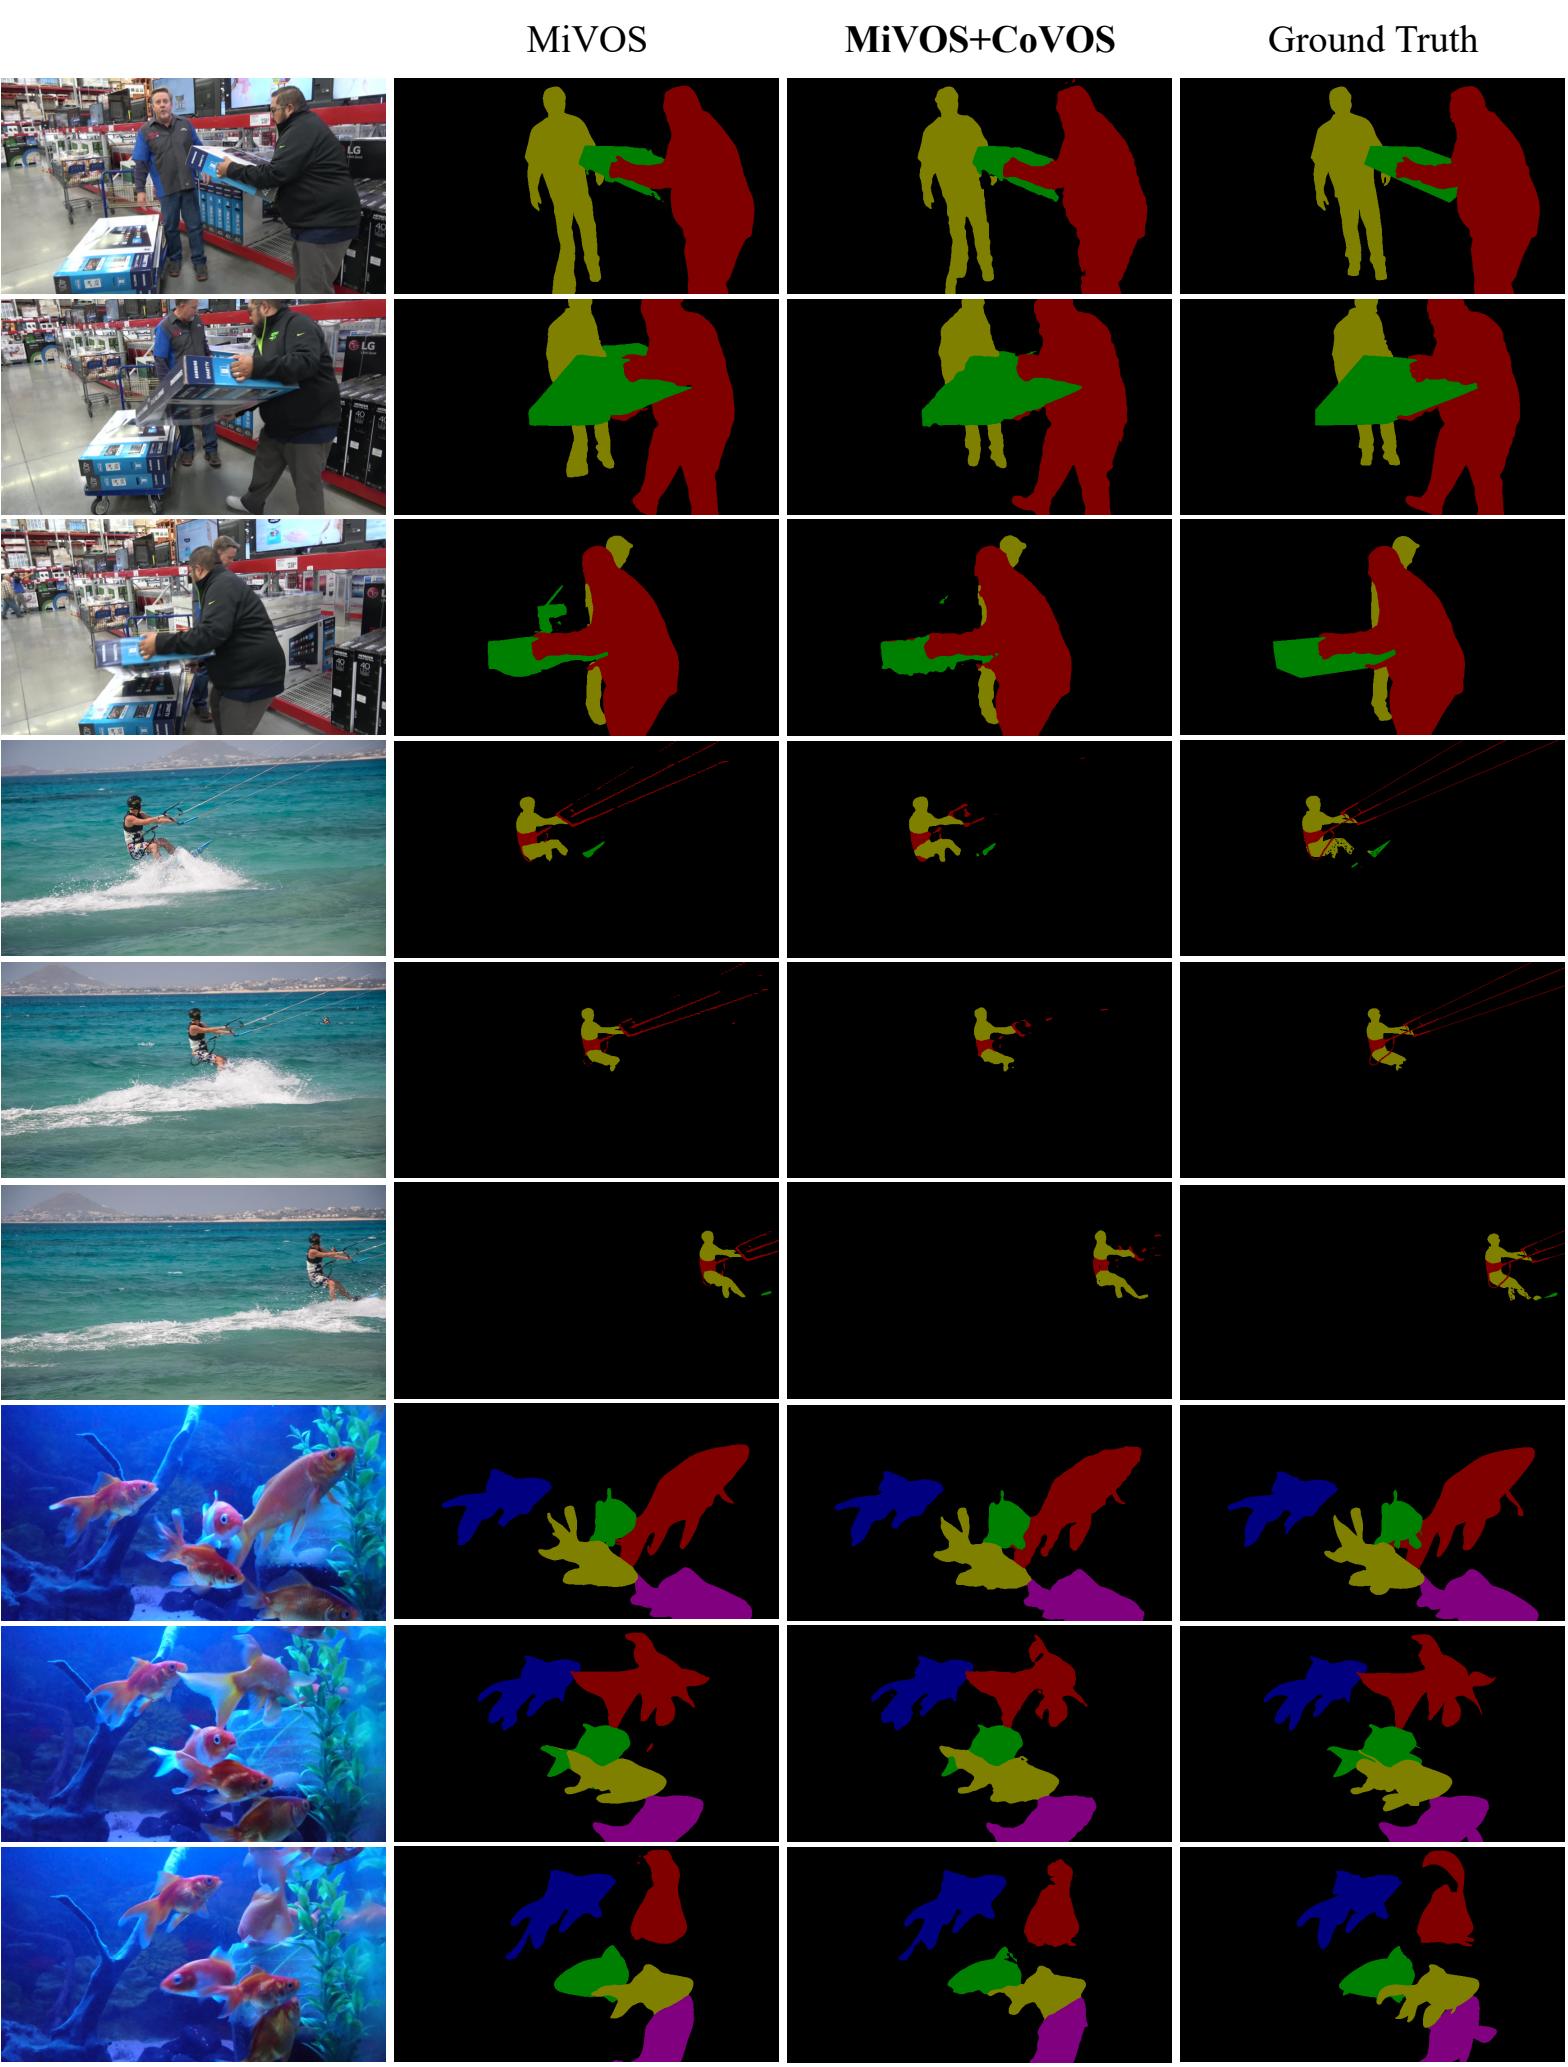 |

|                                                                                   | MiVOS                                                                               | MiVOS+CoVOS                                                                          | Ground Truth                                                                          |
|-----------------------------------------------------------------------------------|-------------------------------------------------------------------------------------|--------------------------------------------------------------------------------------|---------------------------------------------------------------------------------------|
| 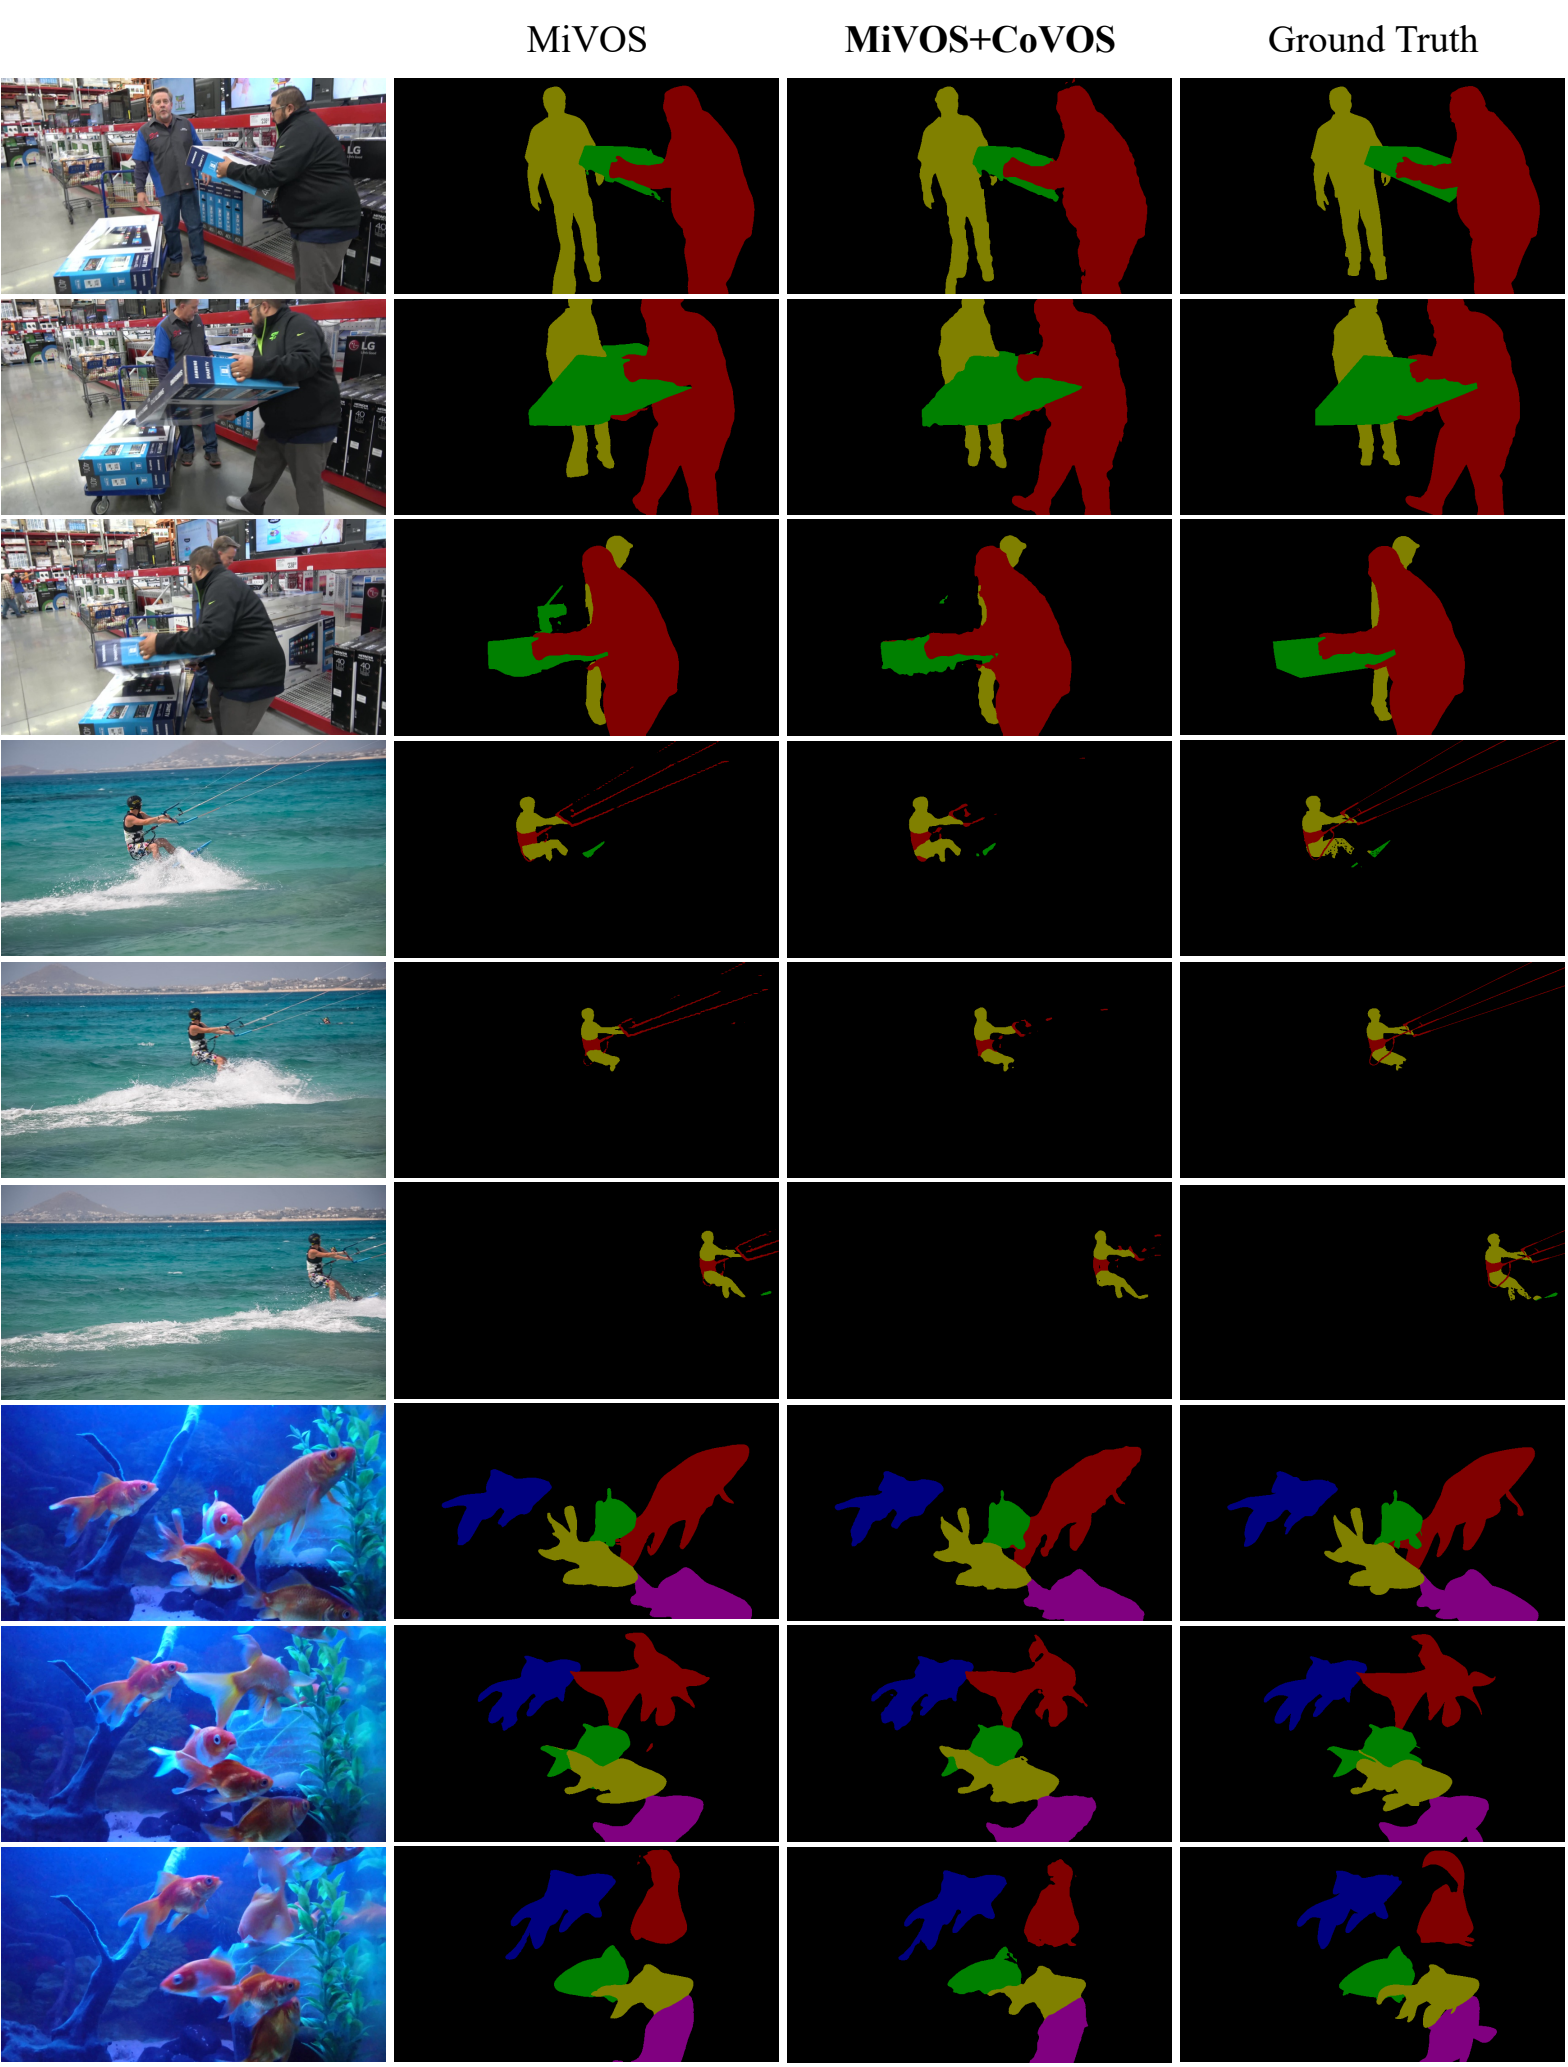    | 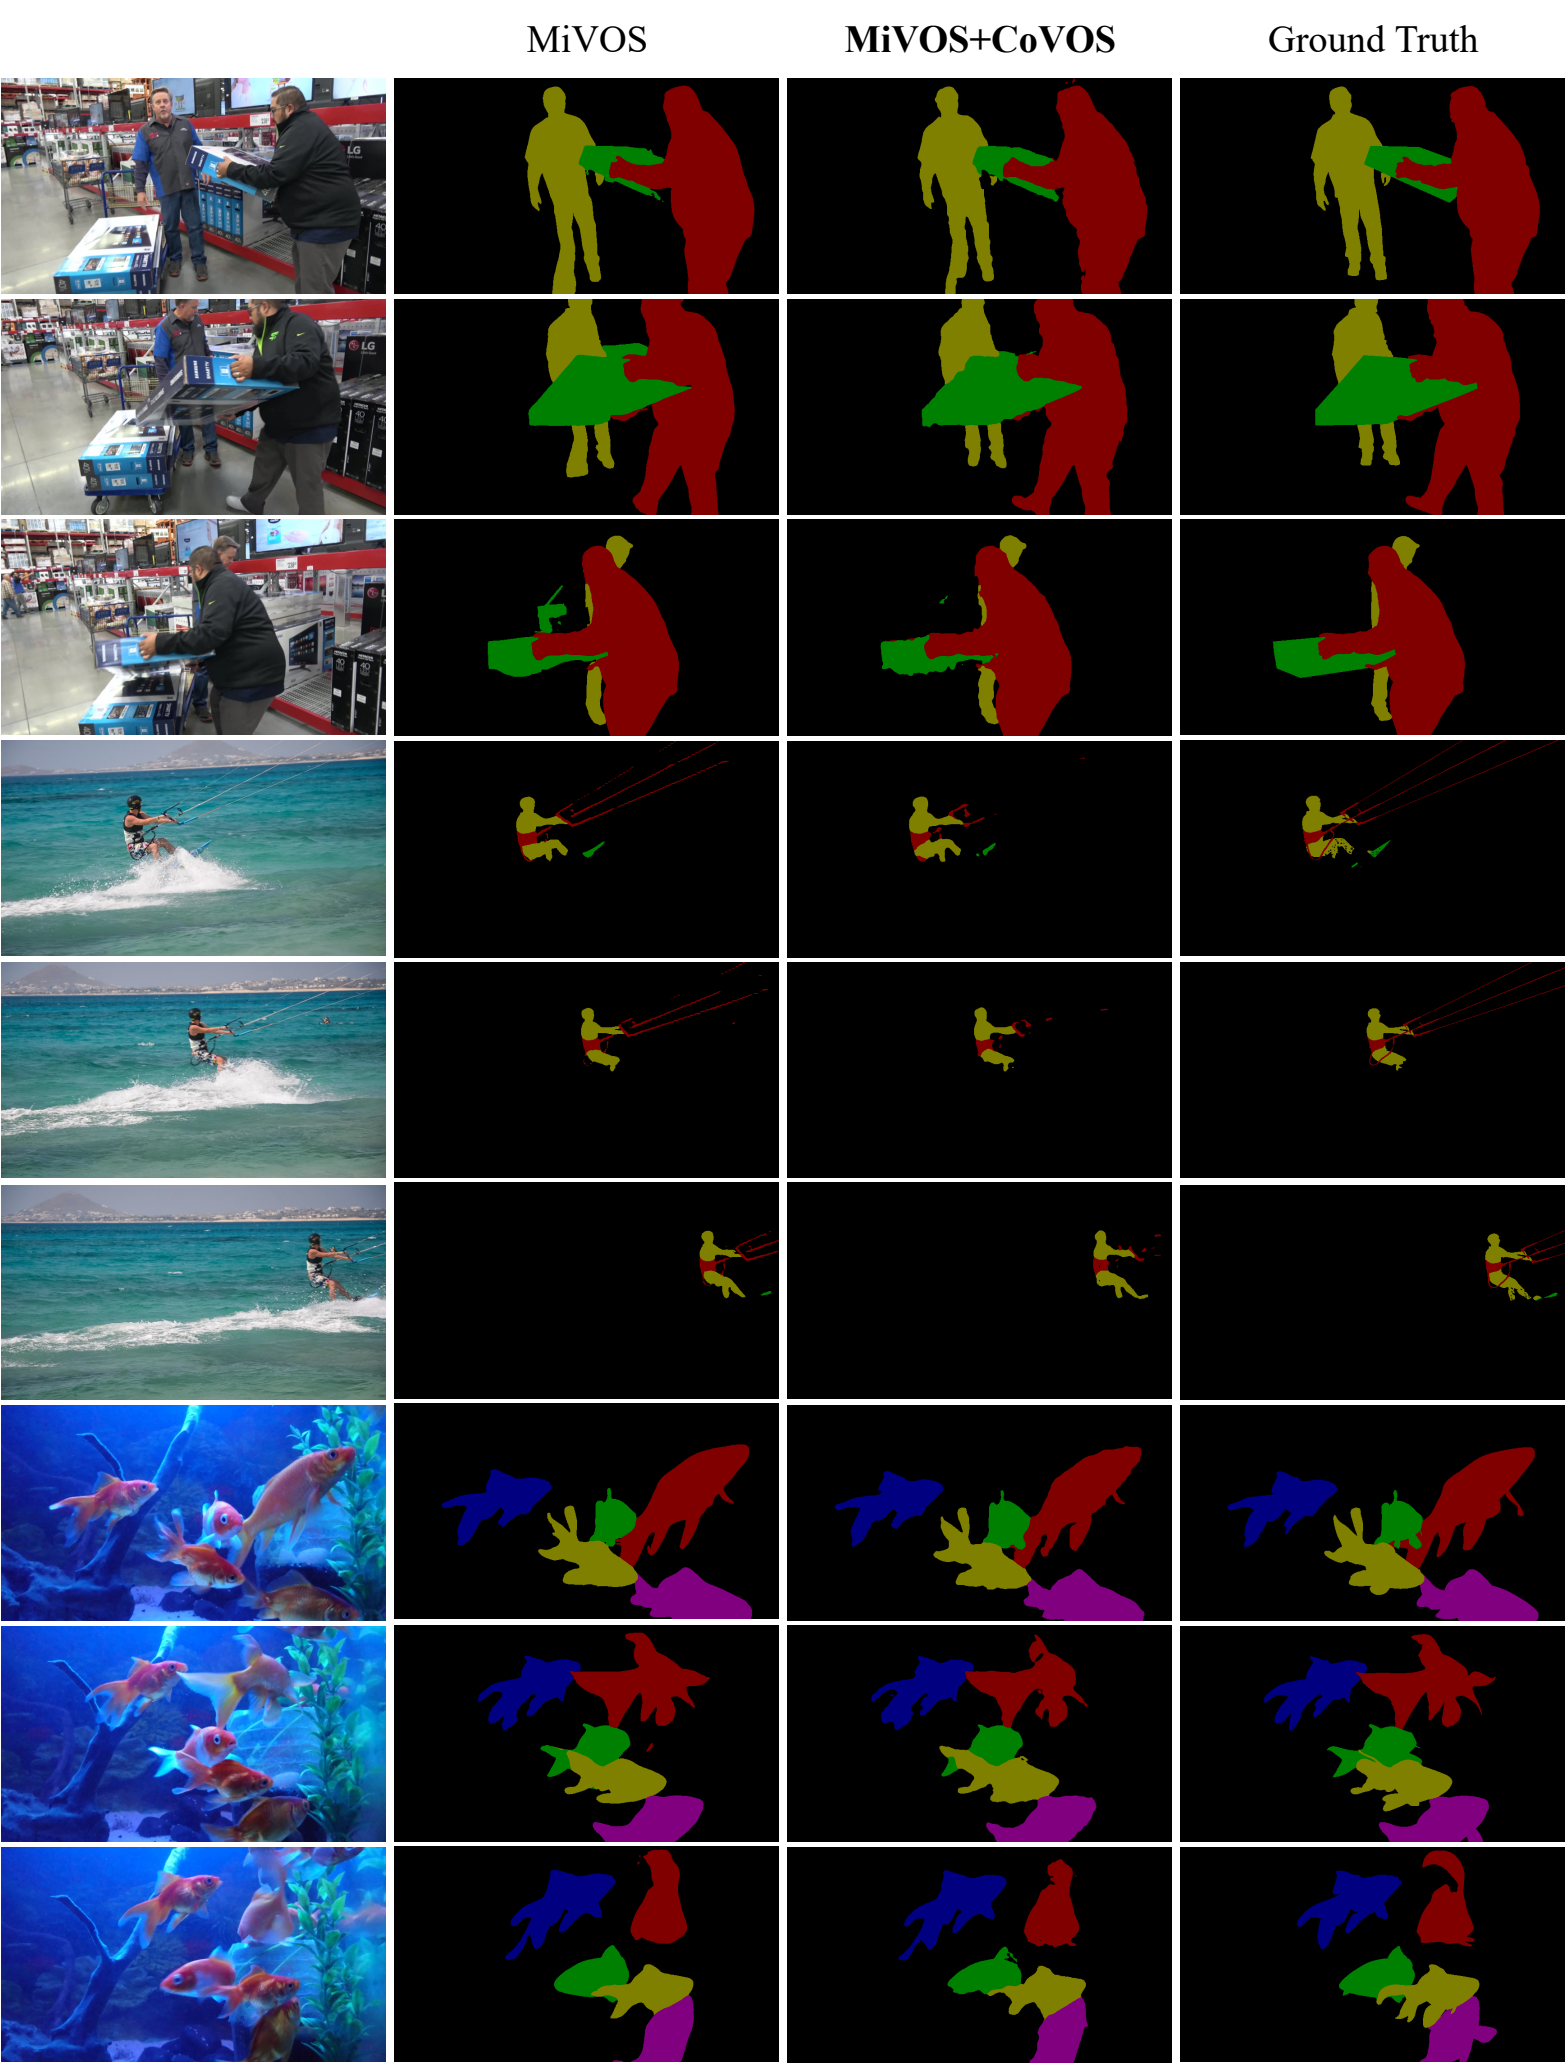    | 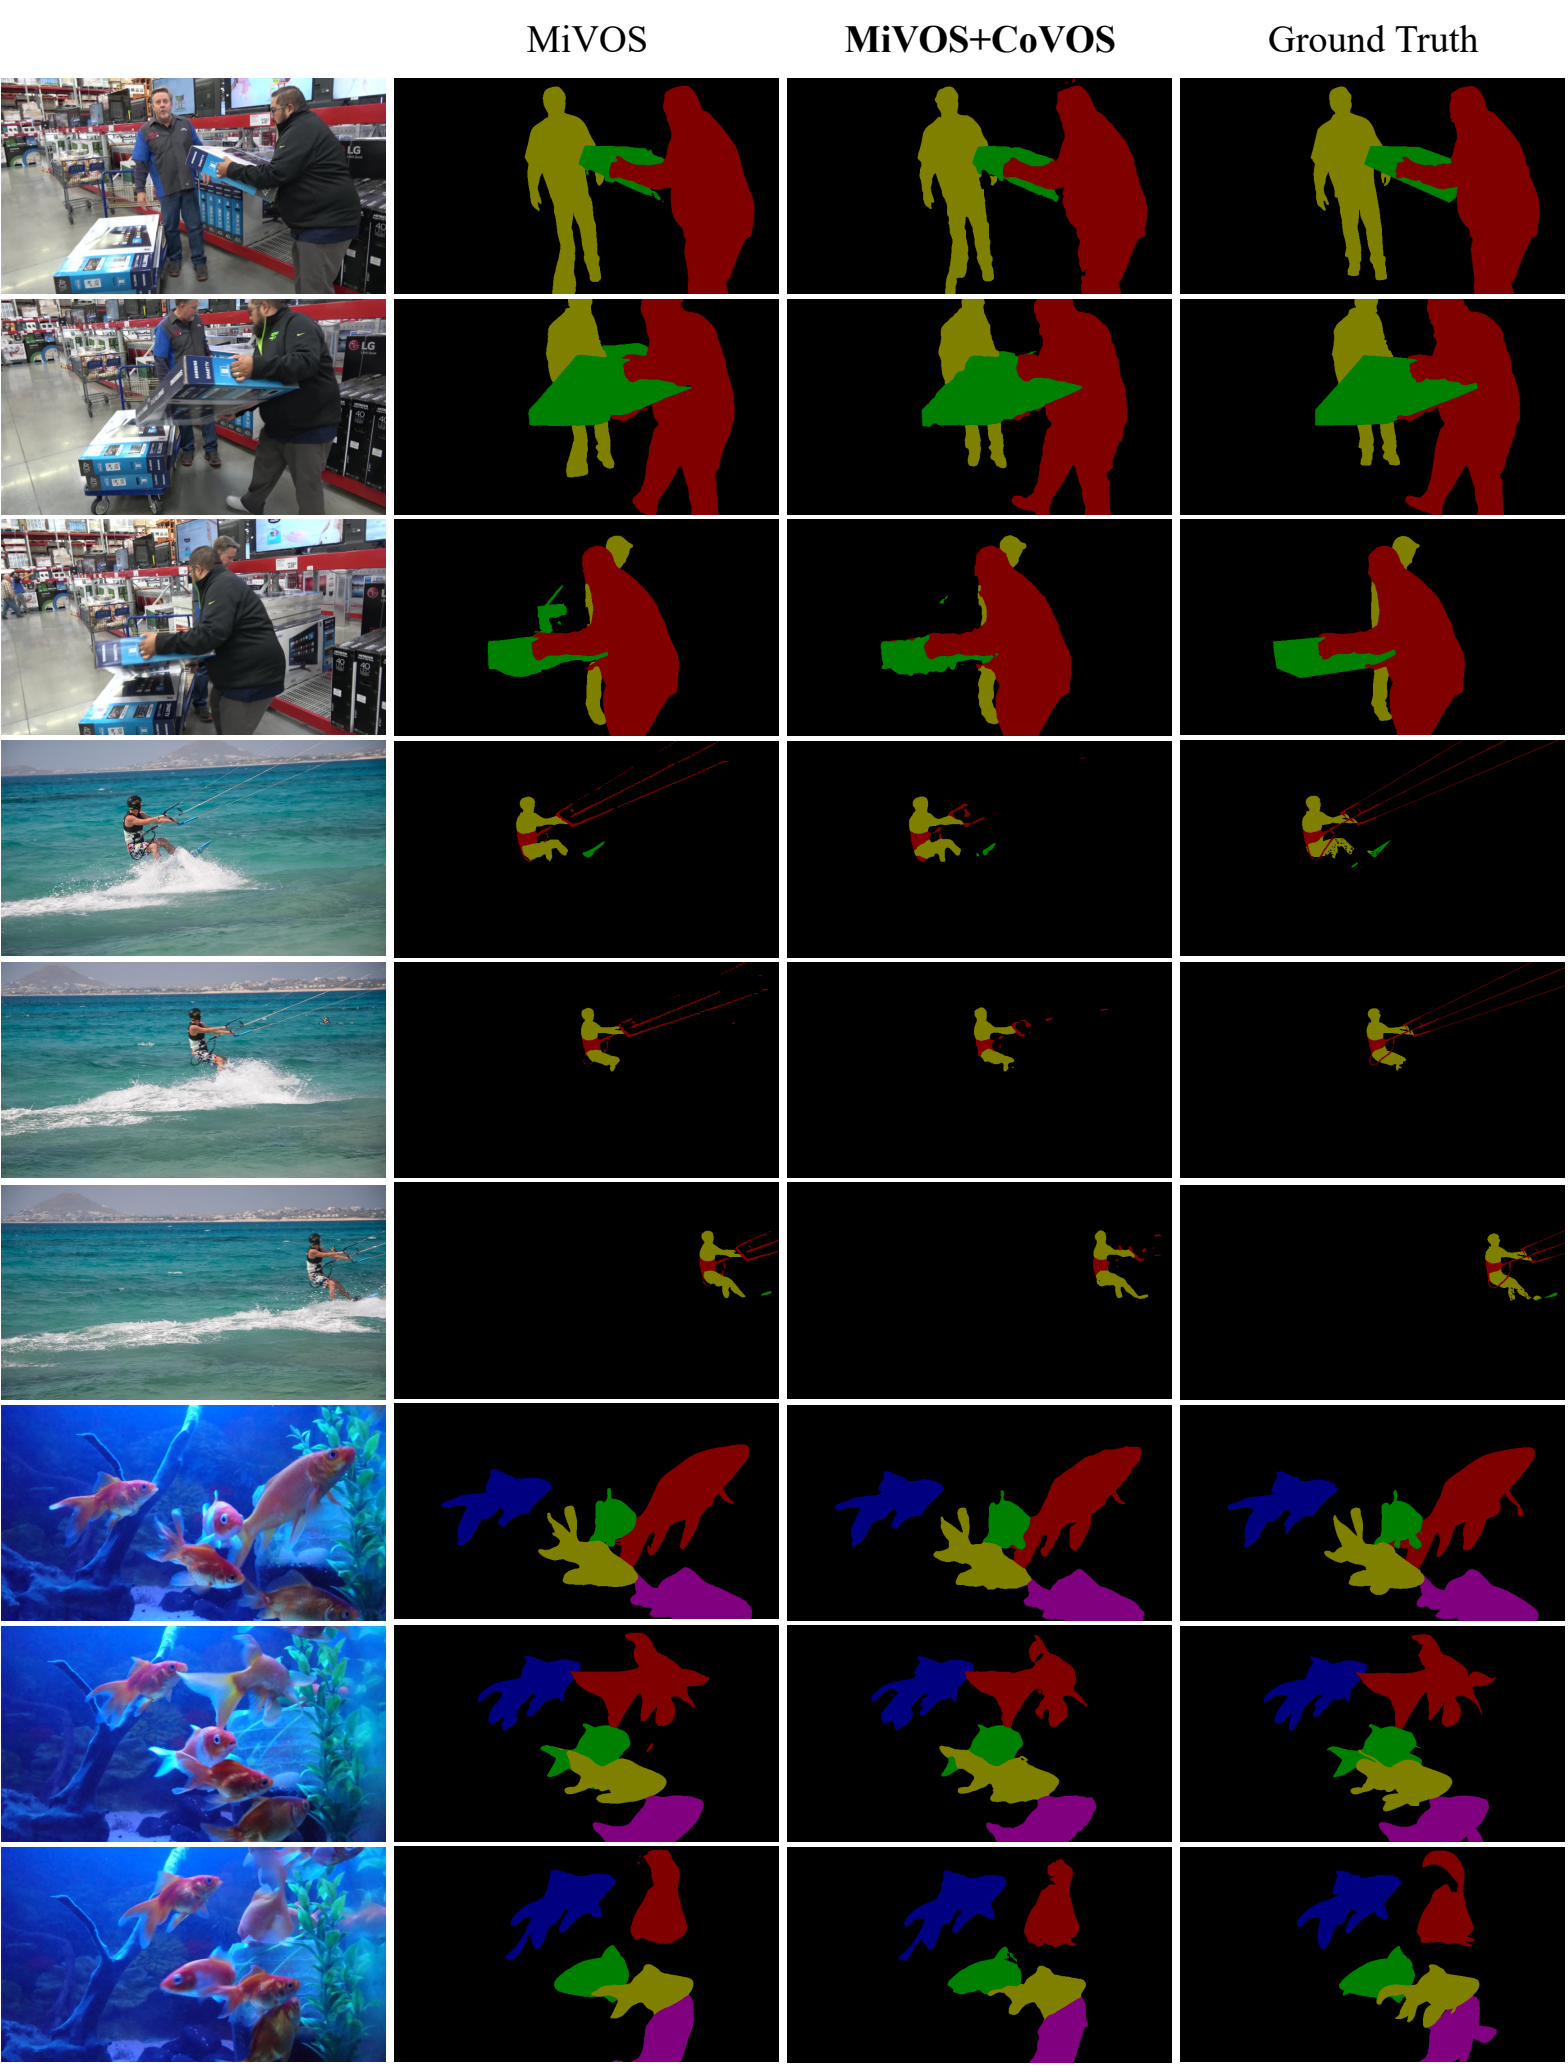    | 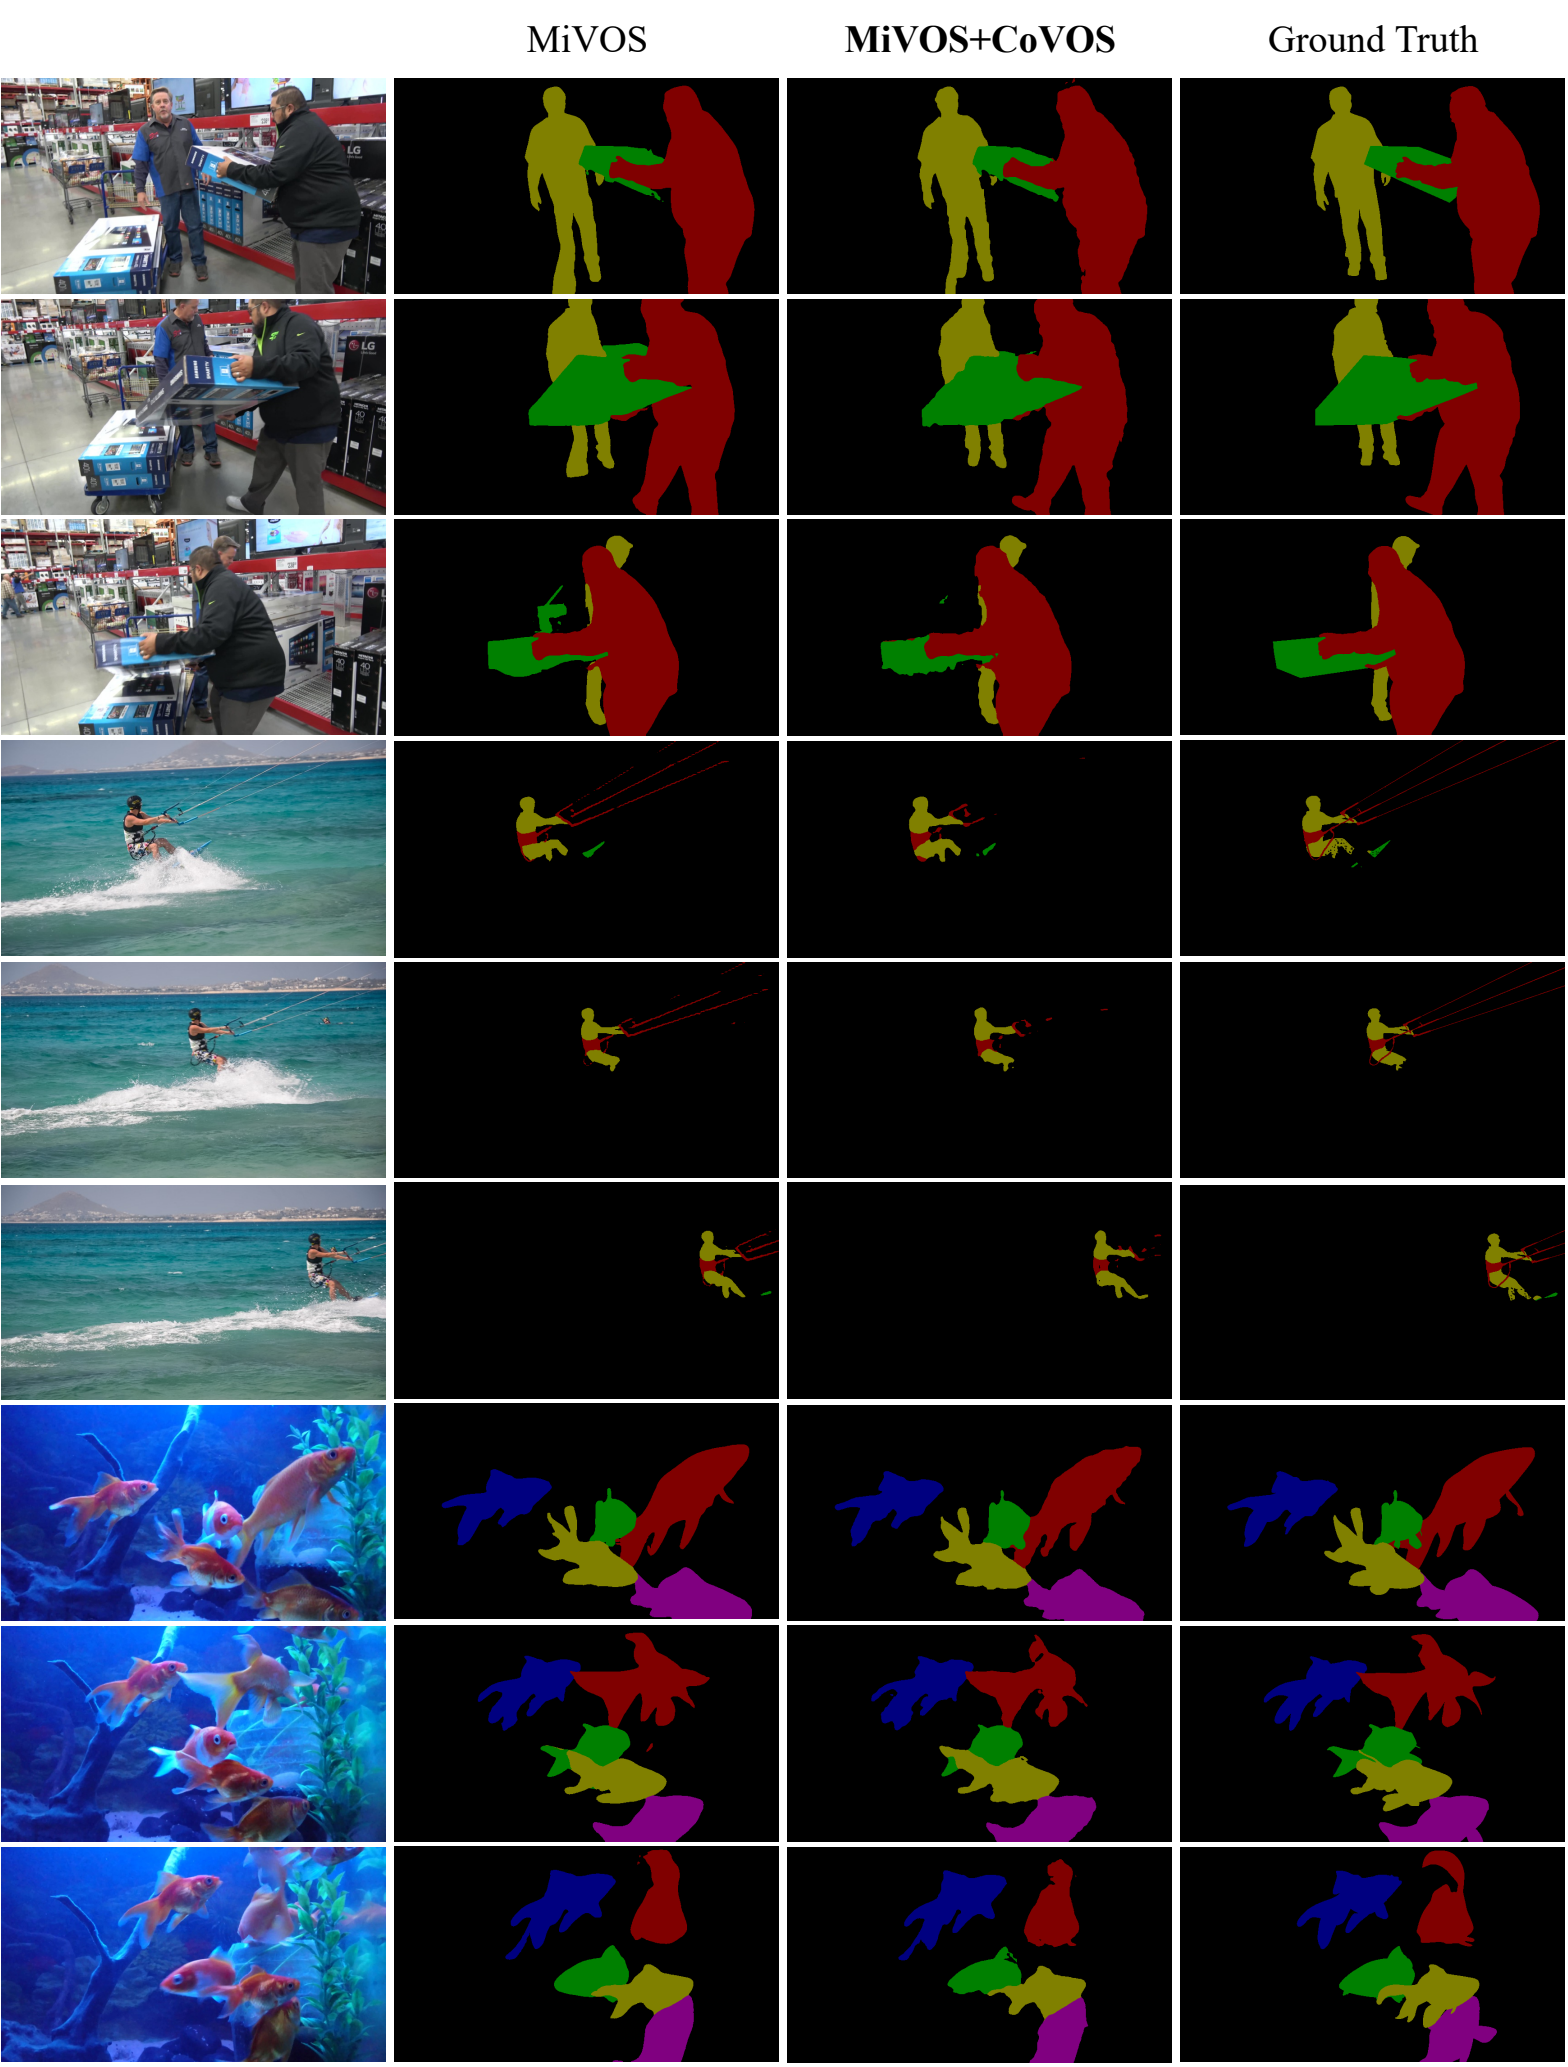    |
| 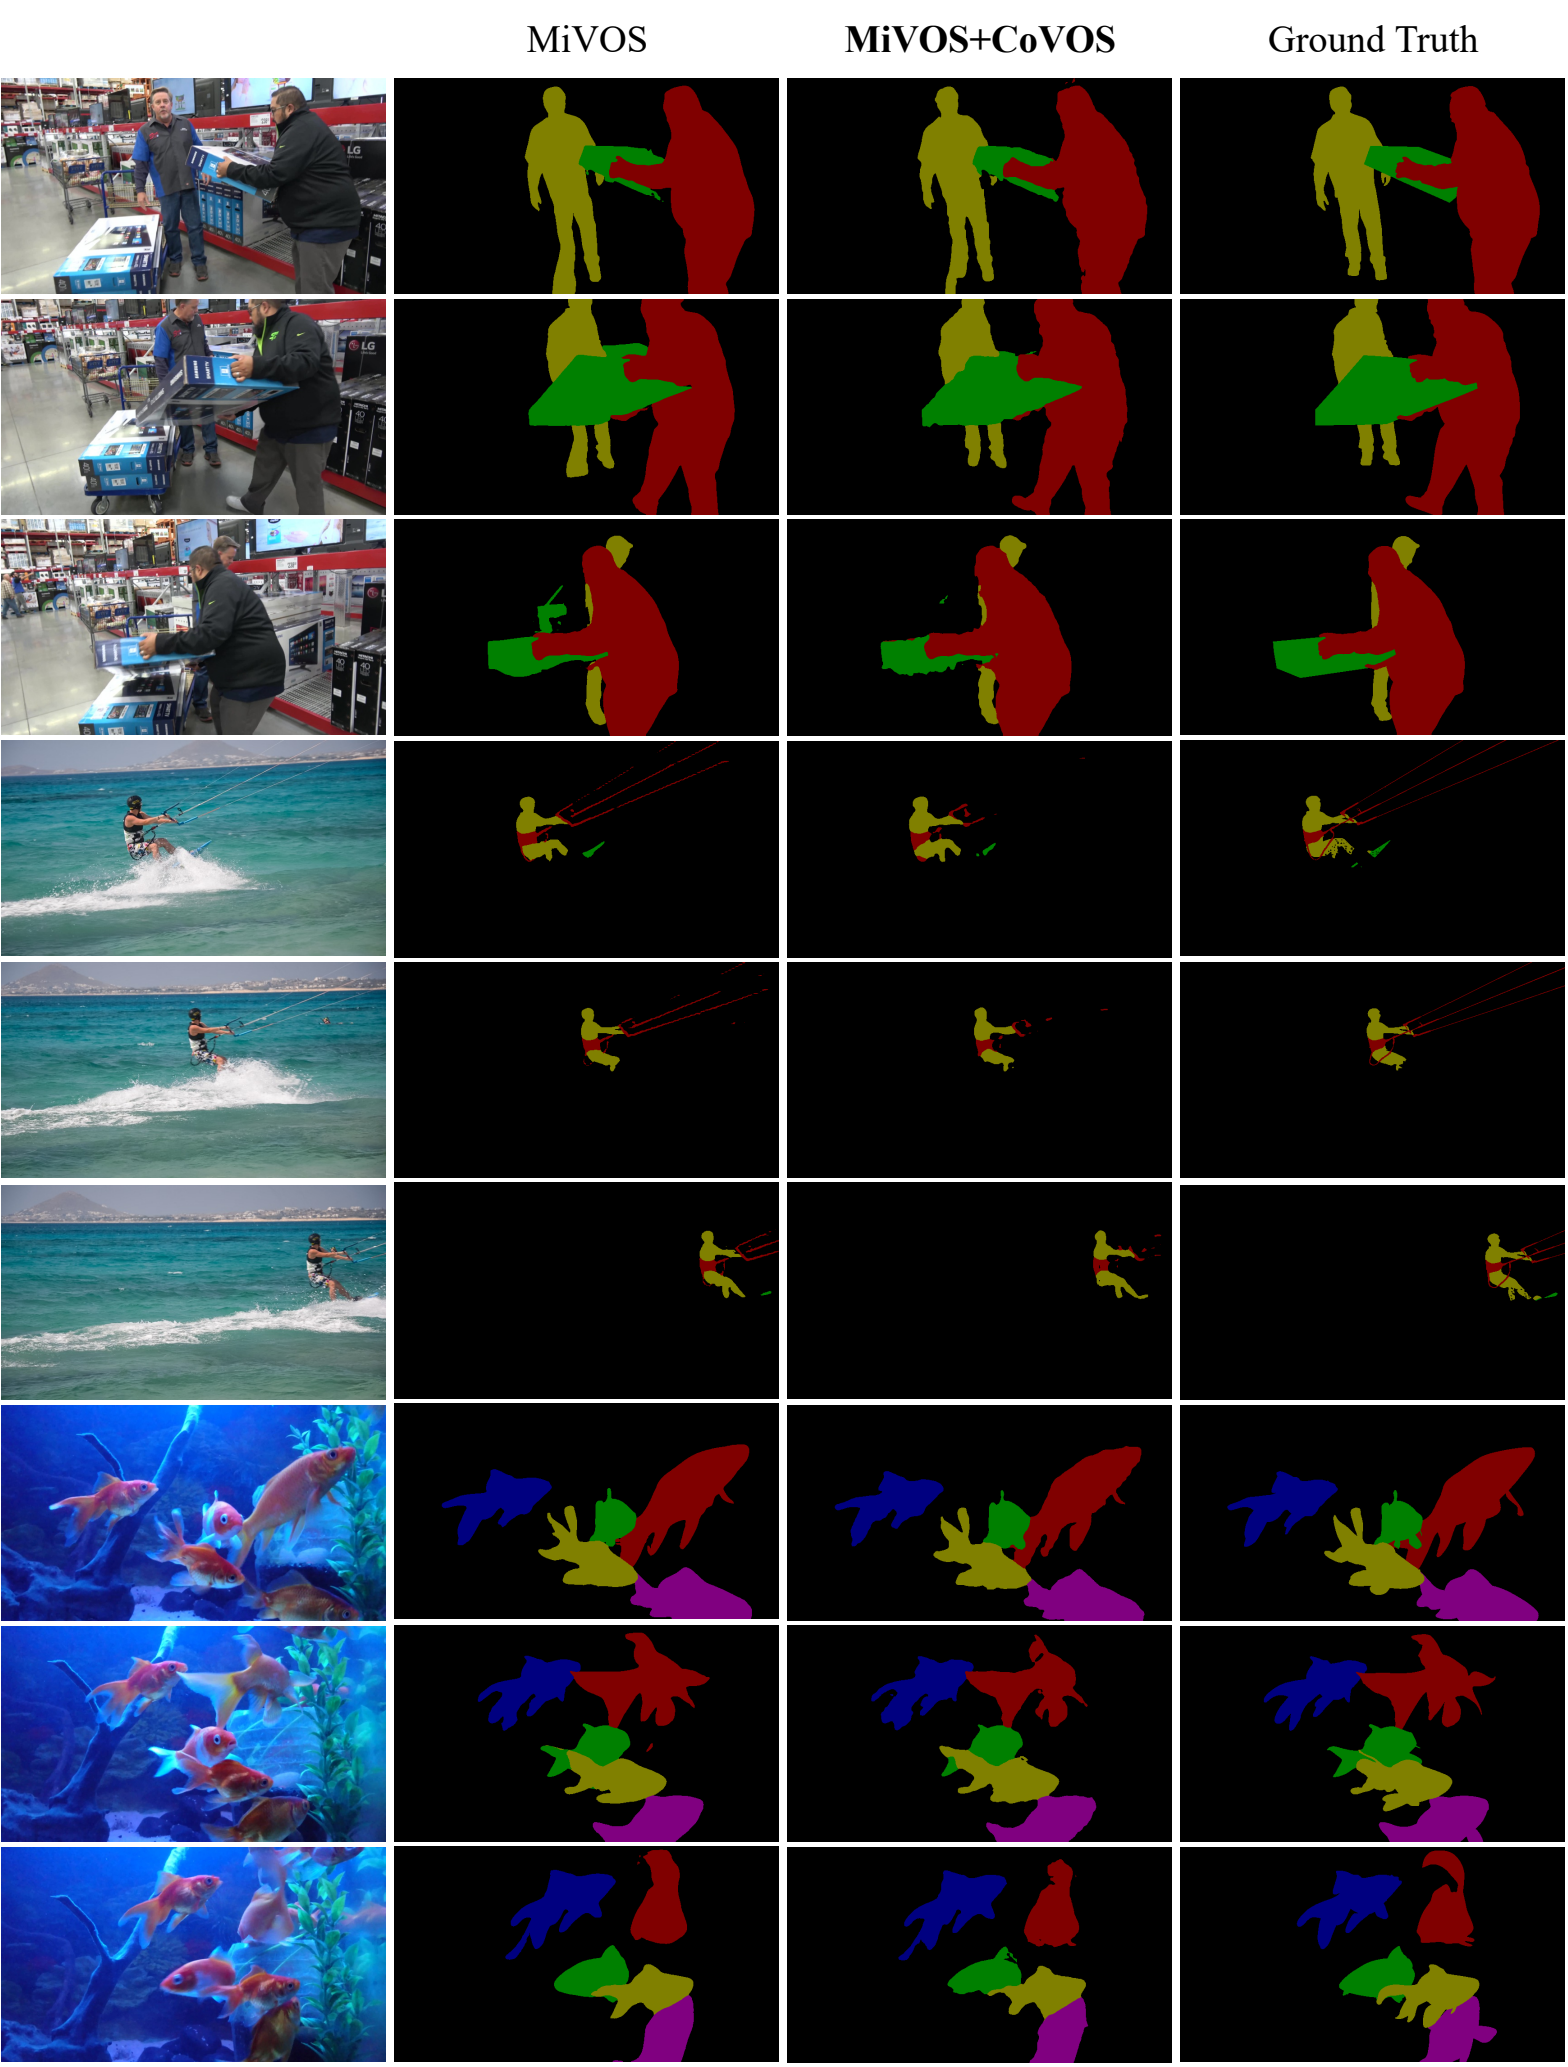   | 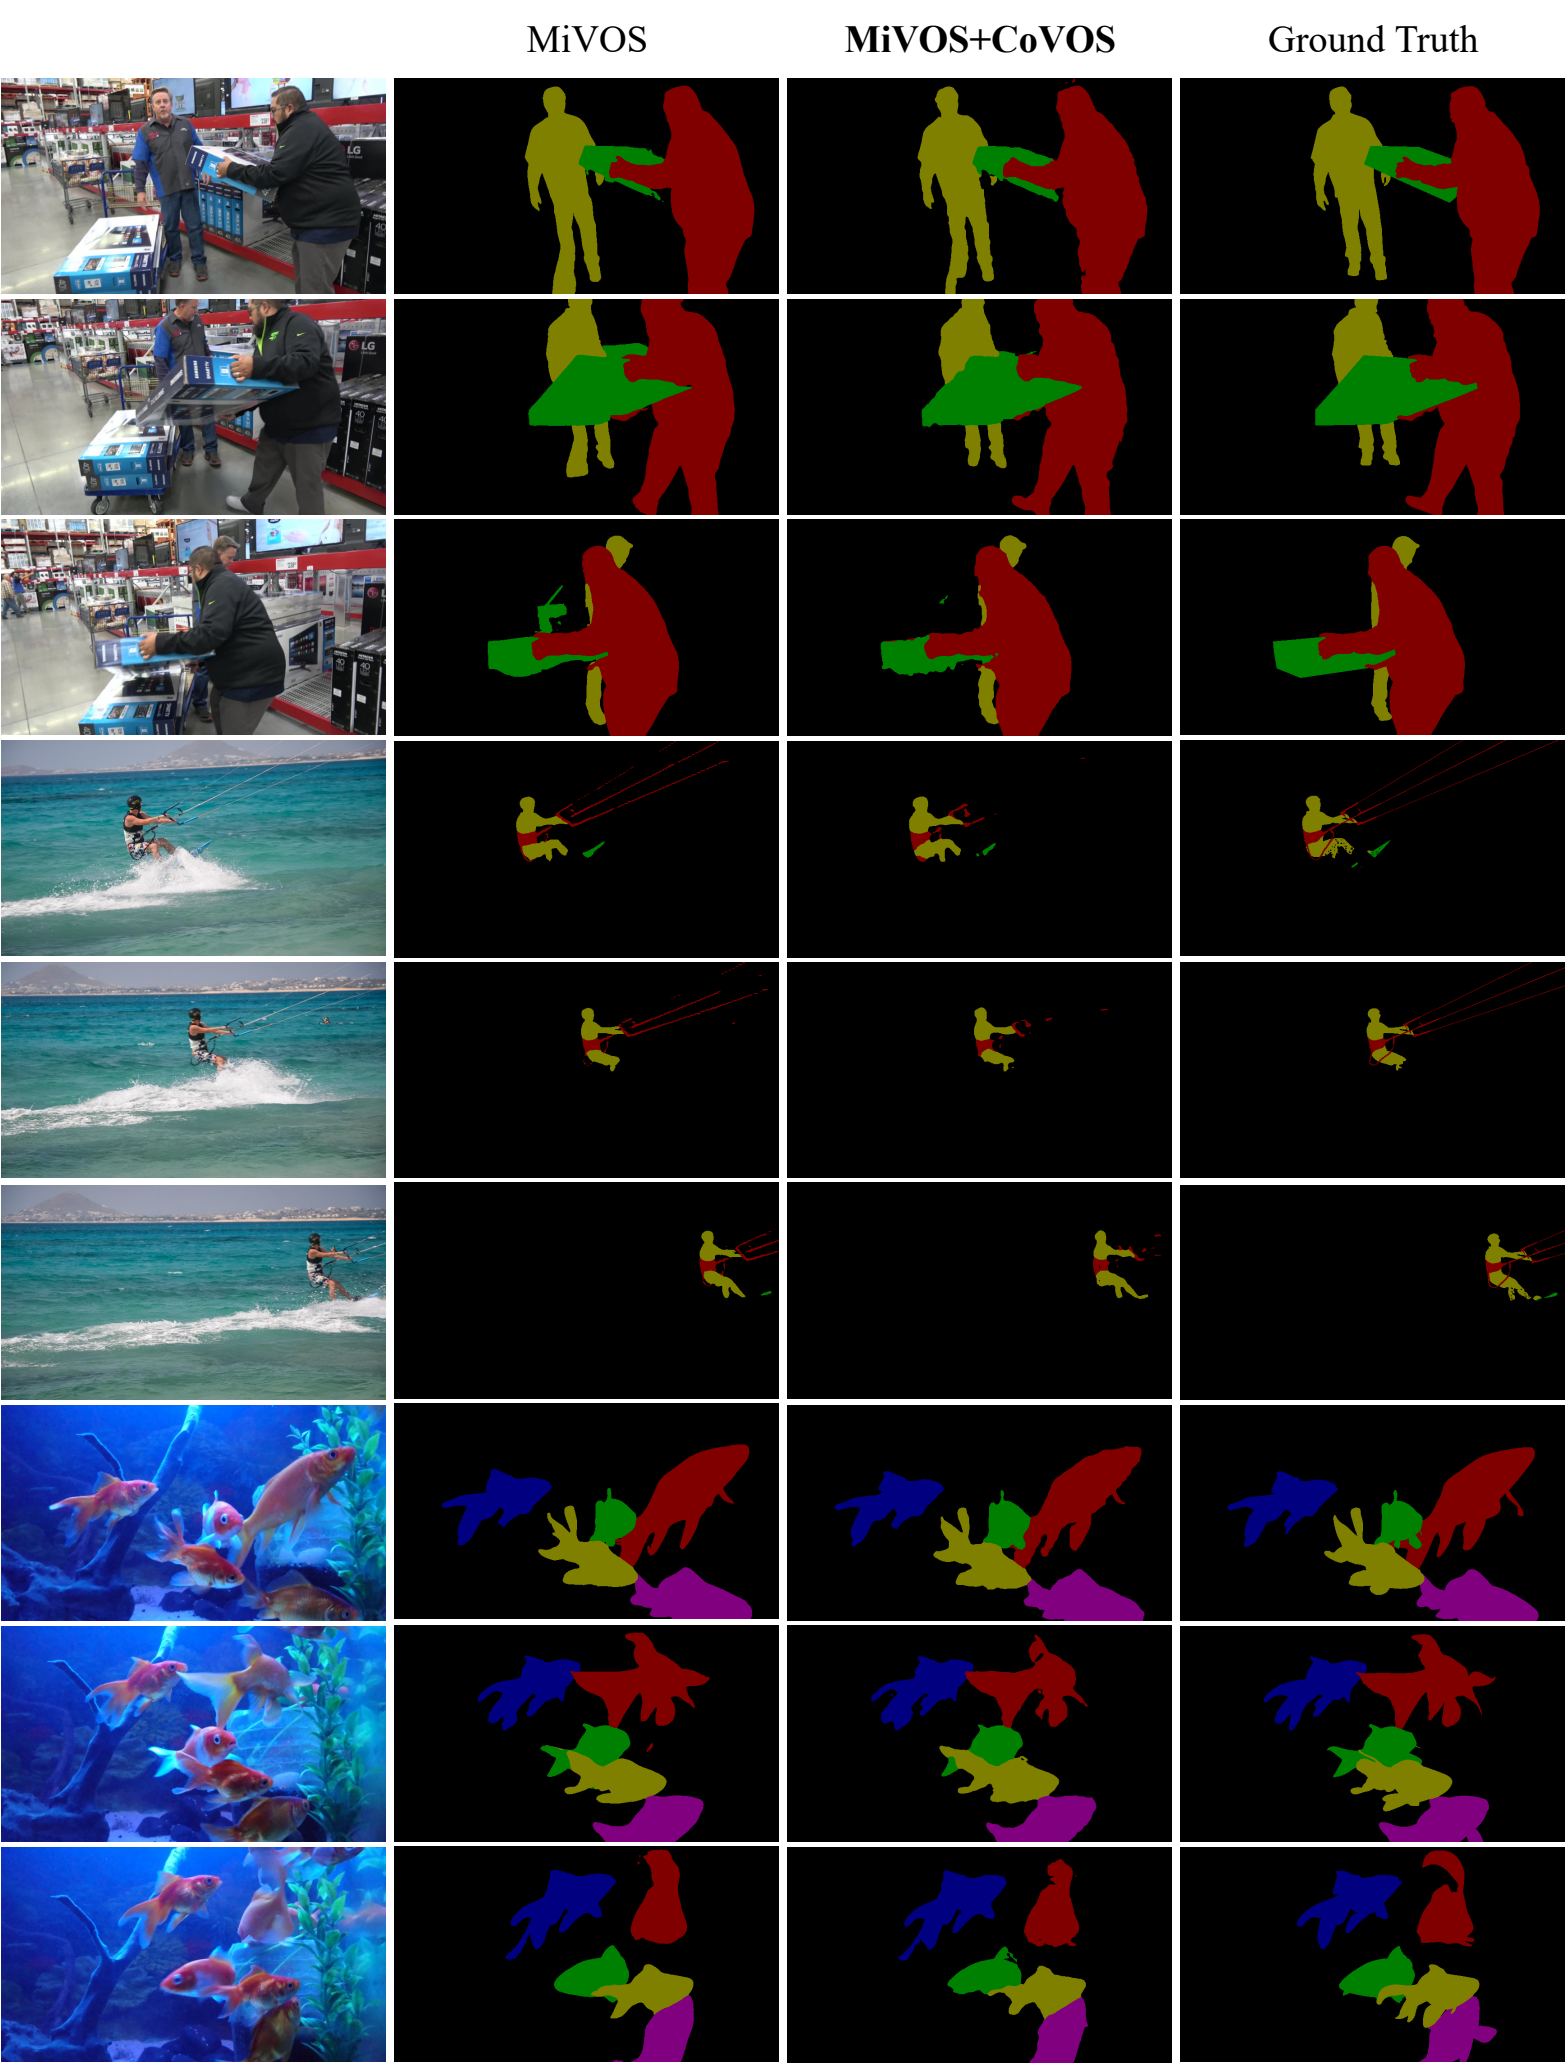   | 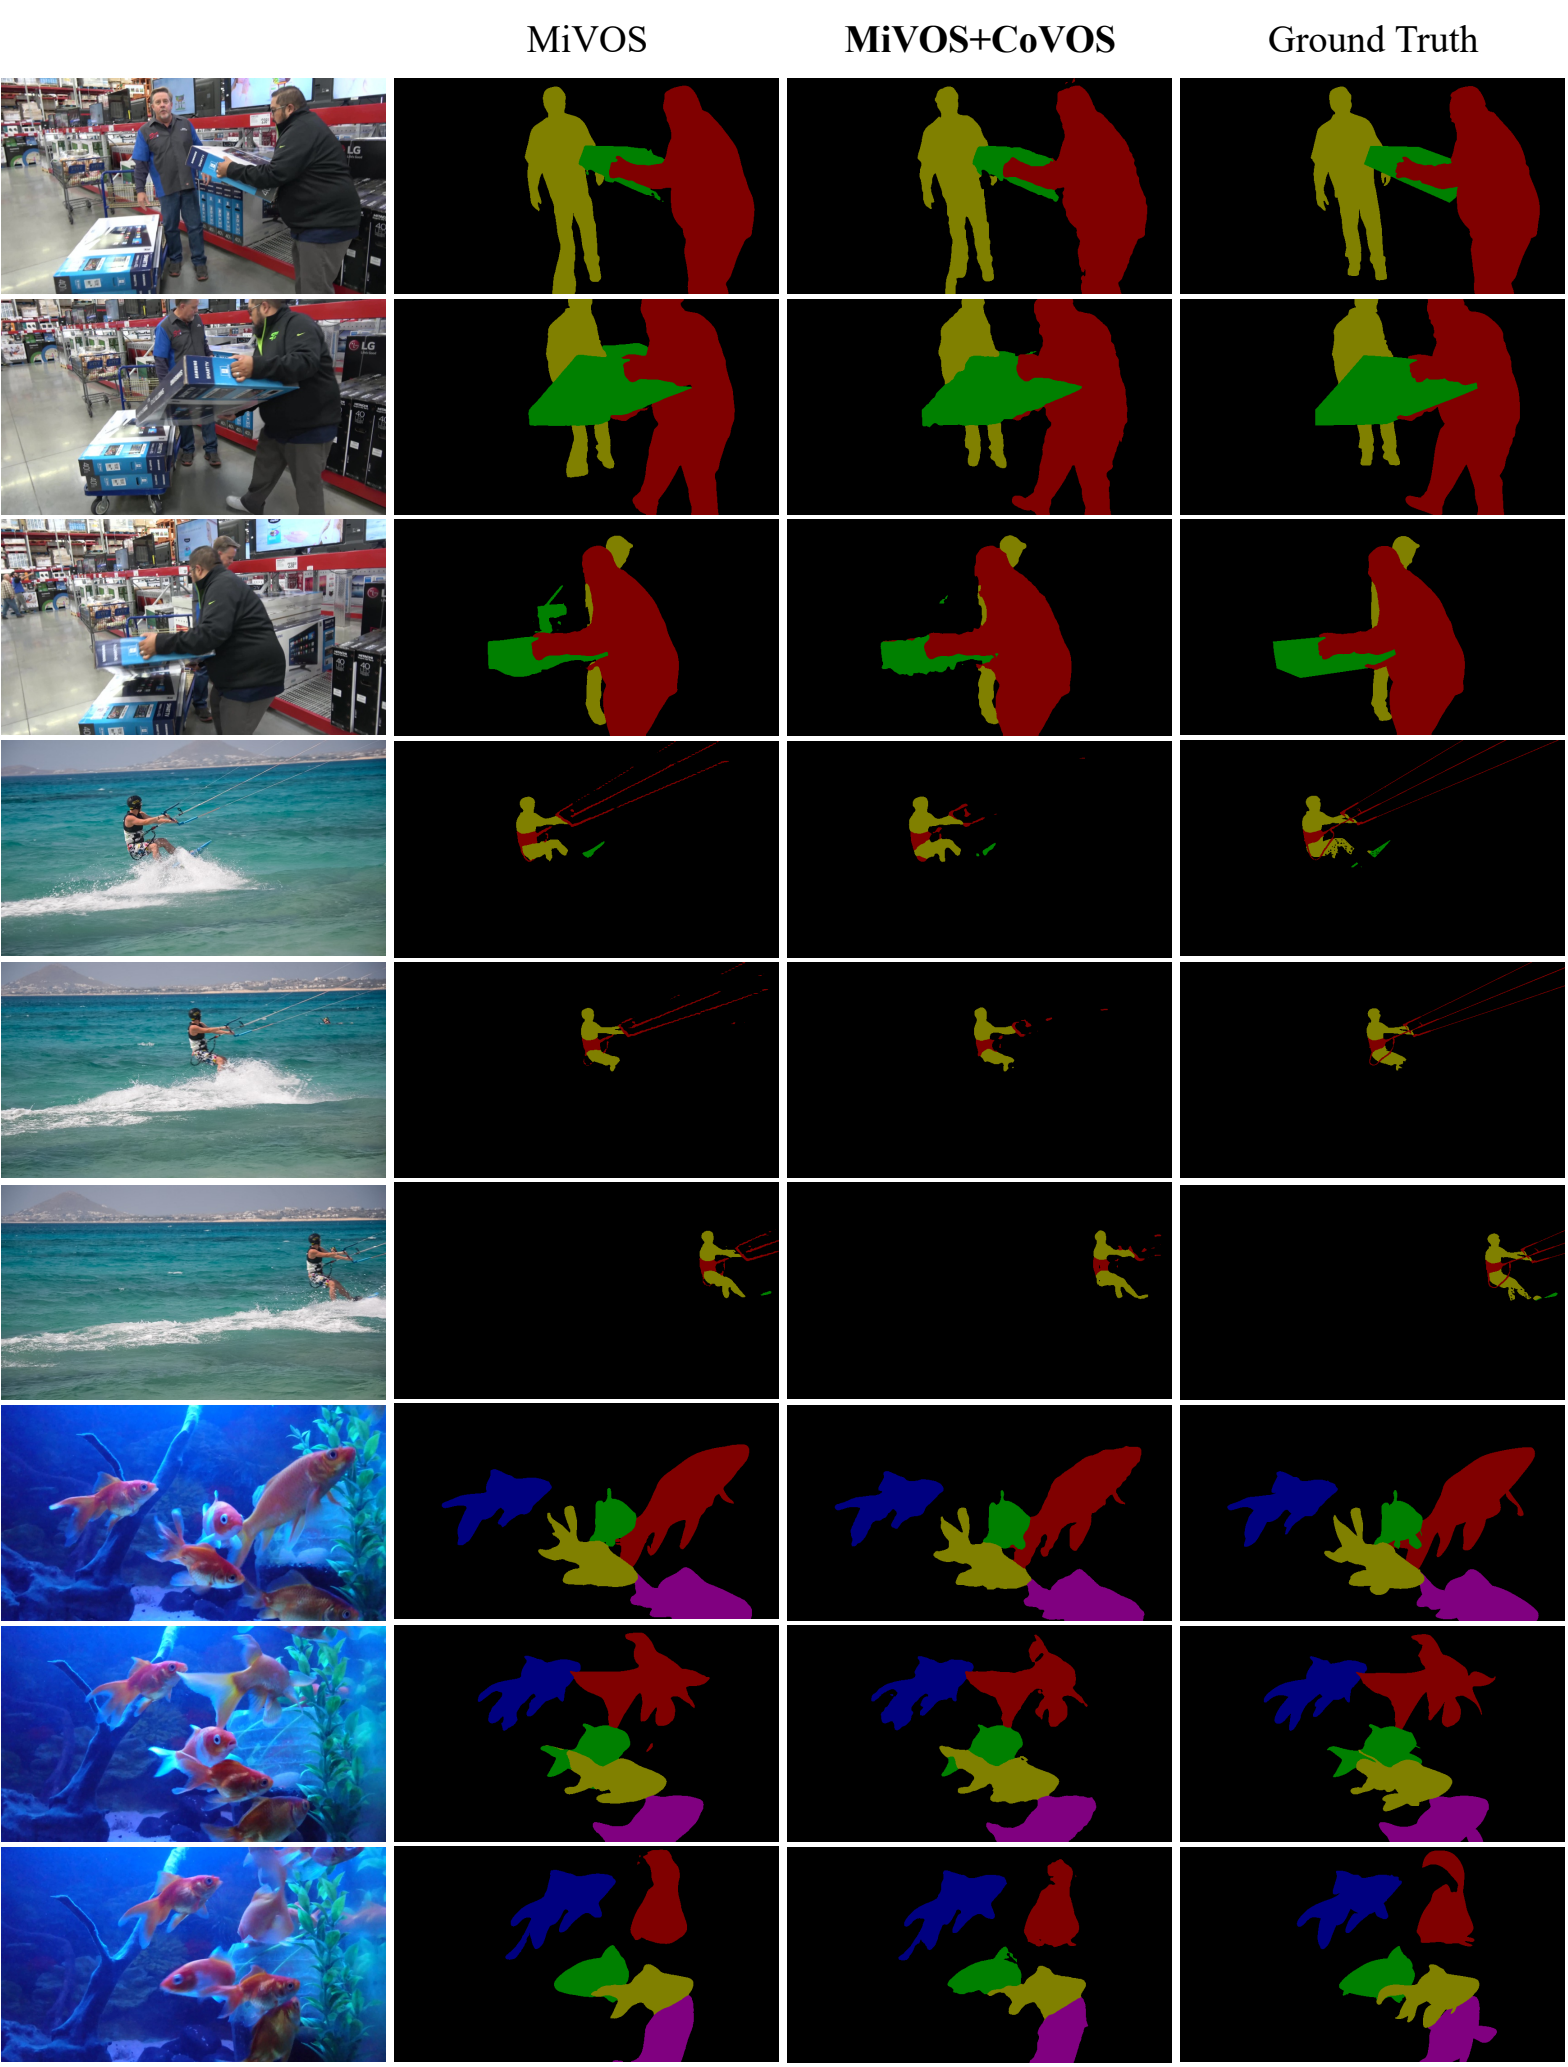   | 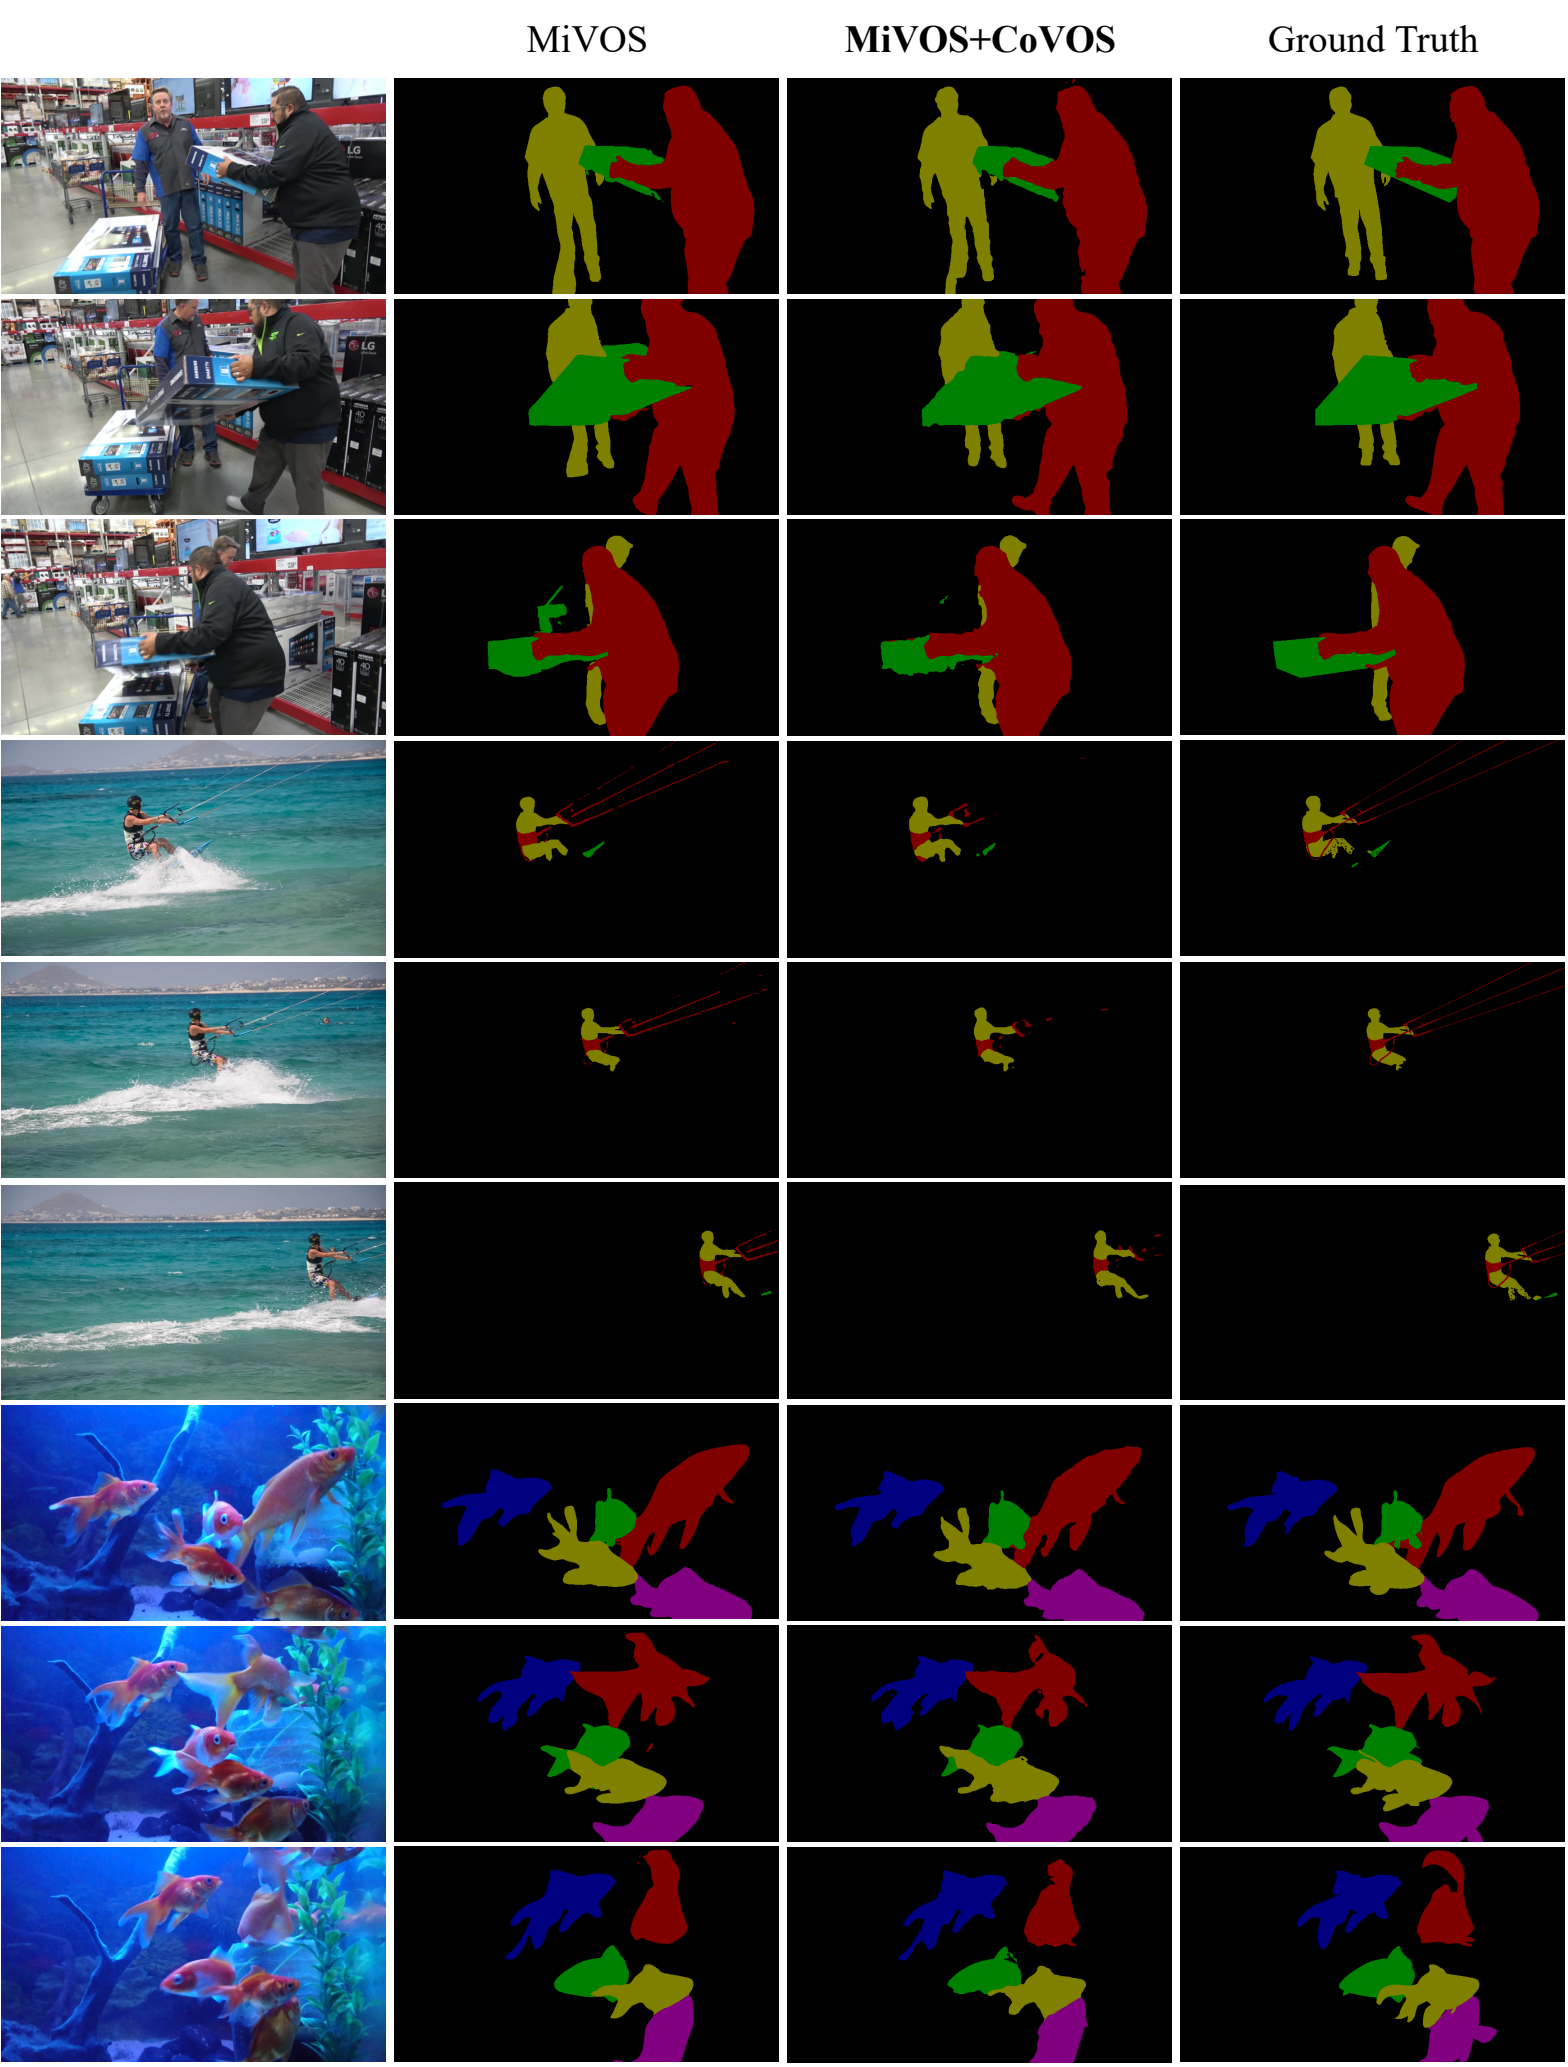   |
| 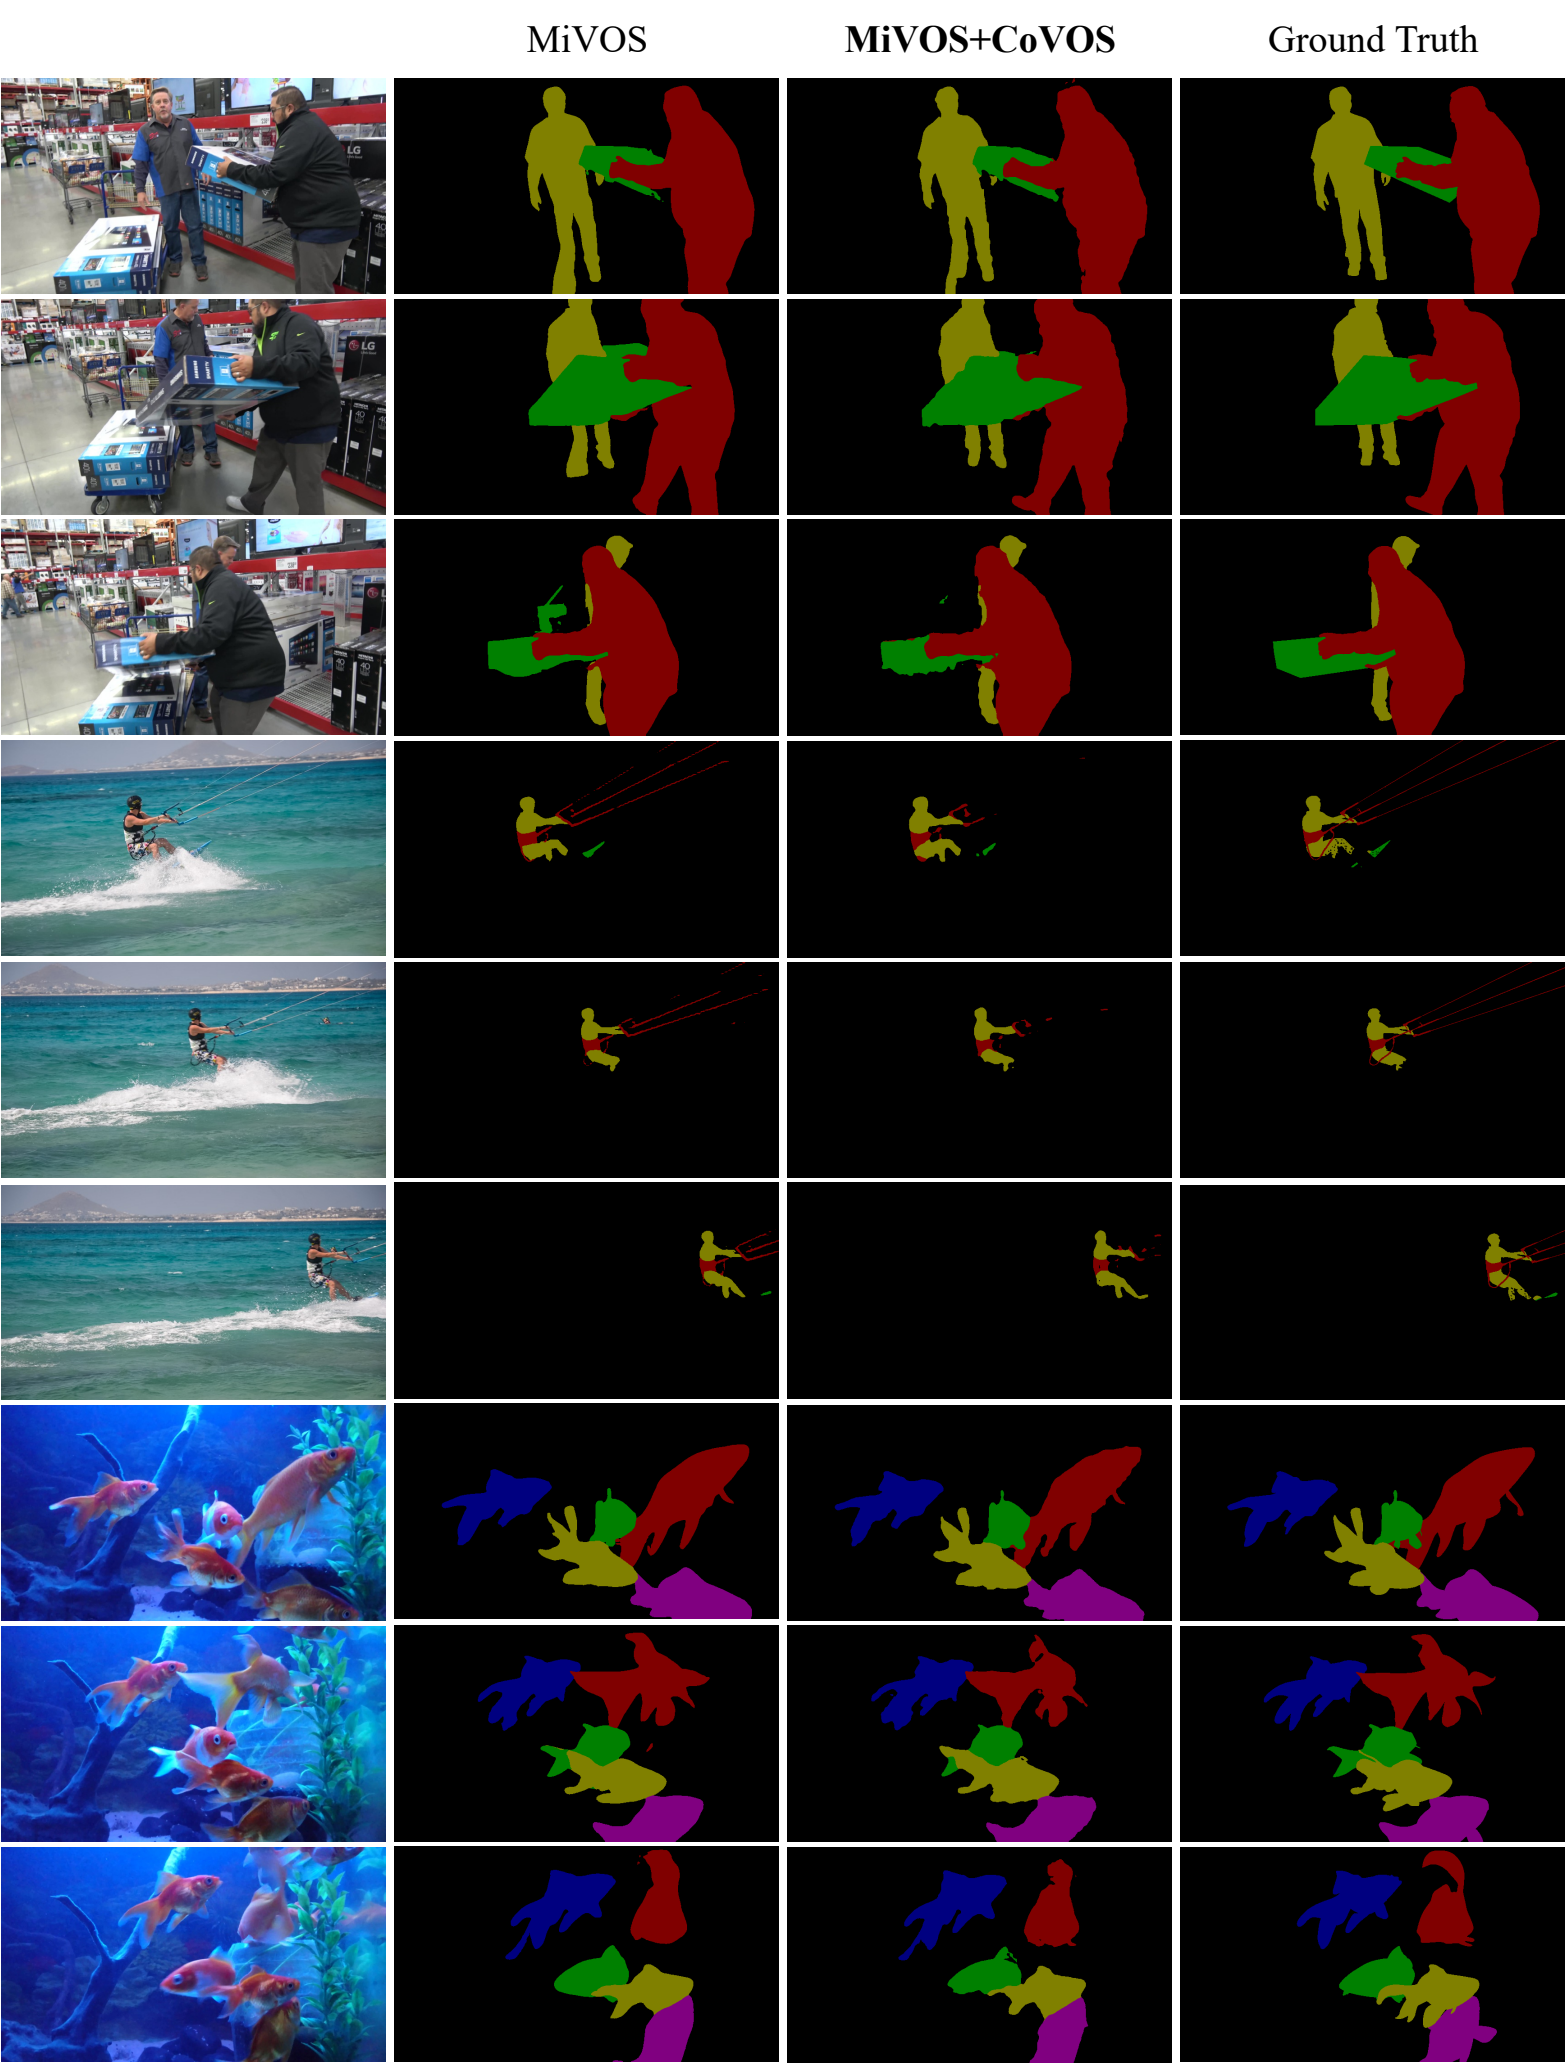   | 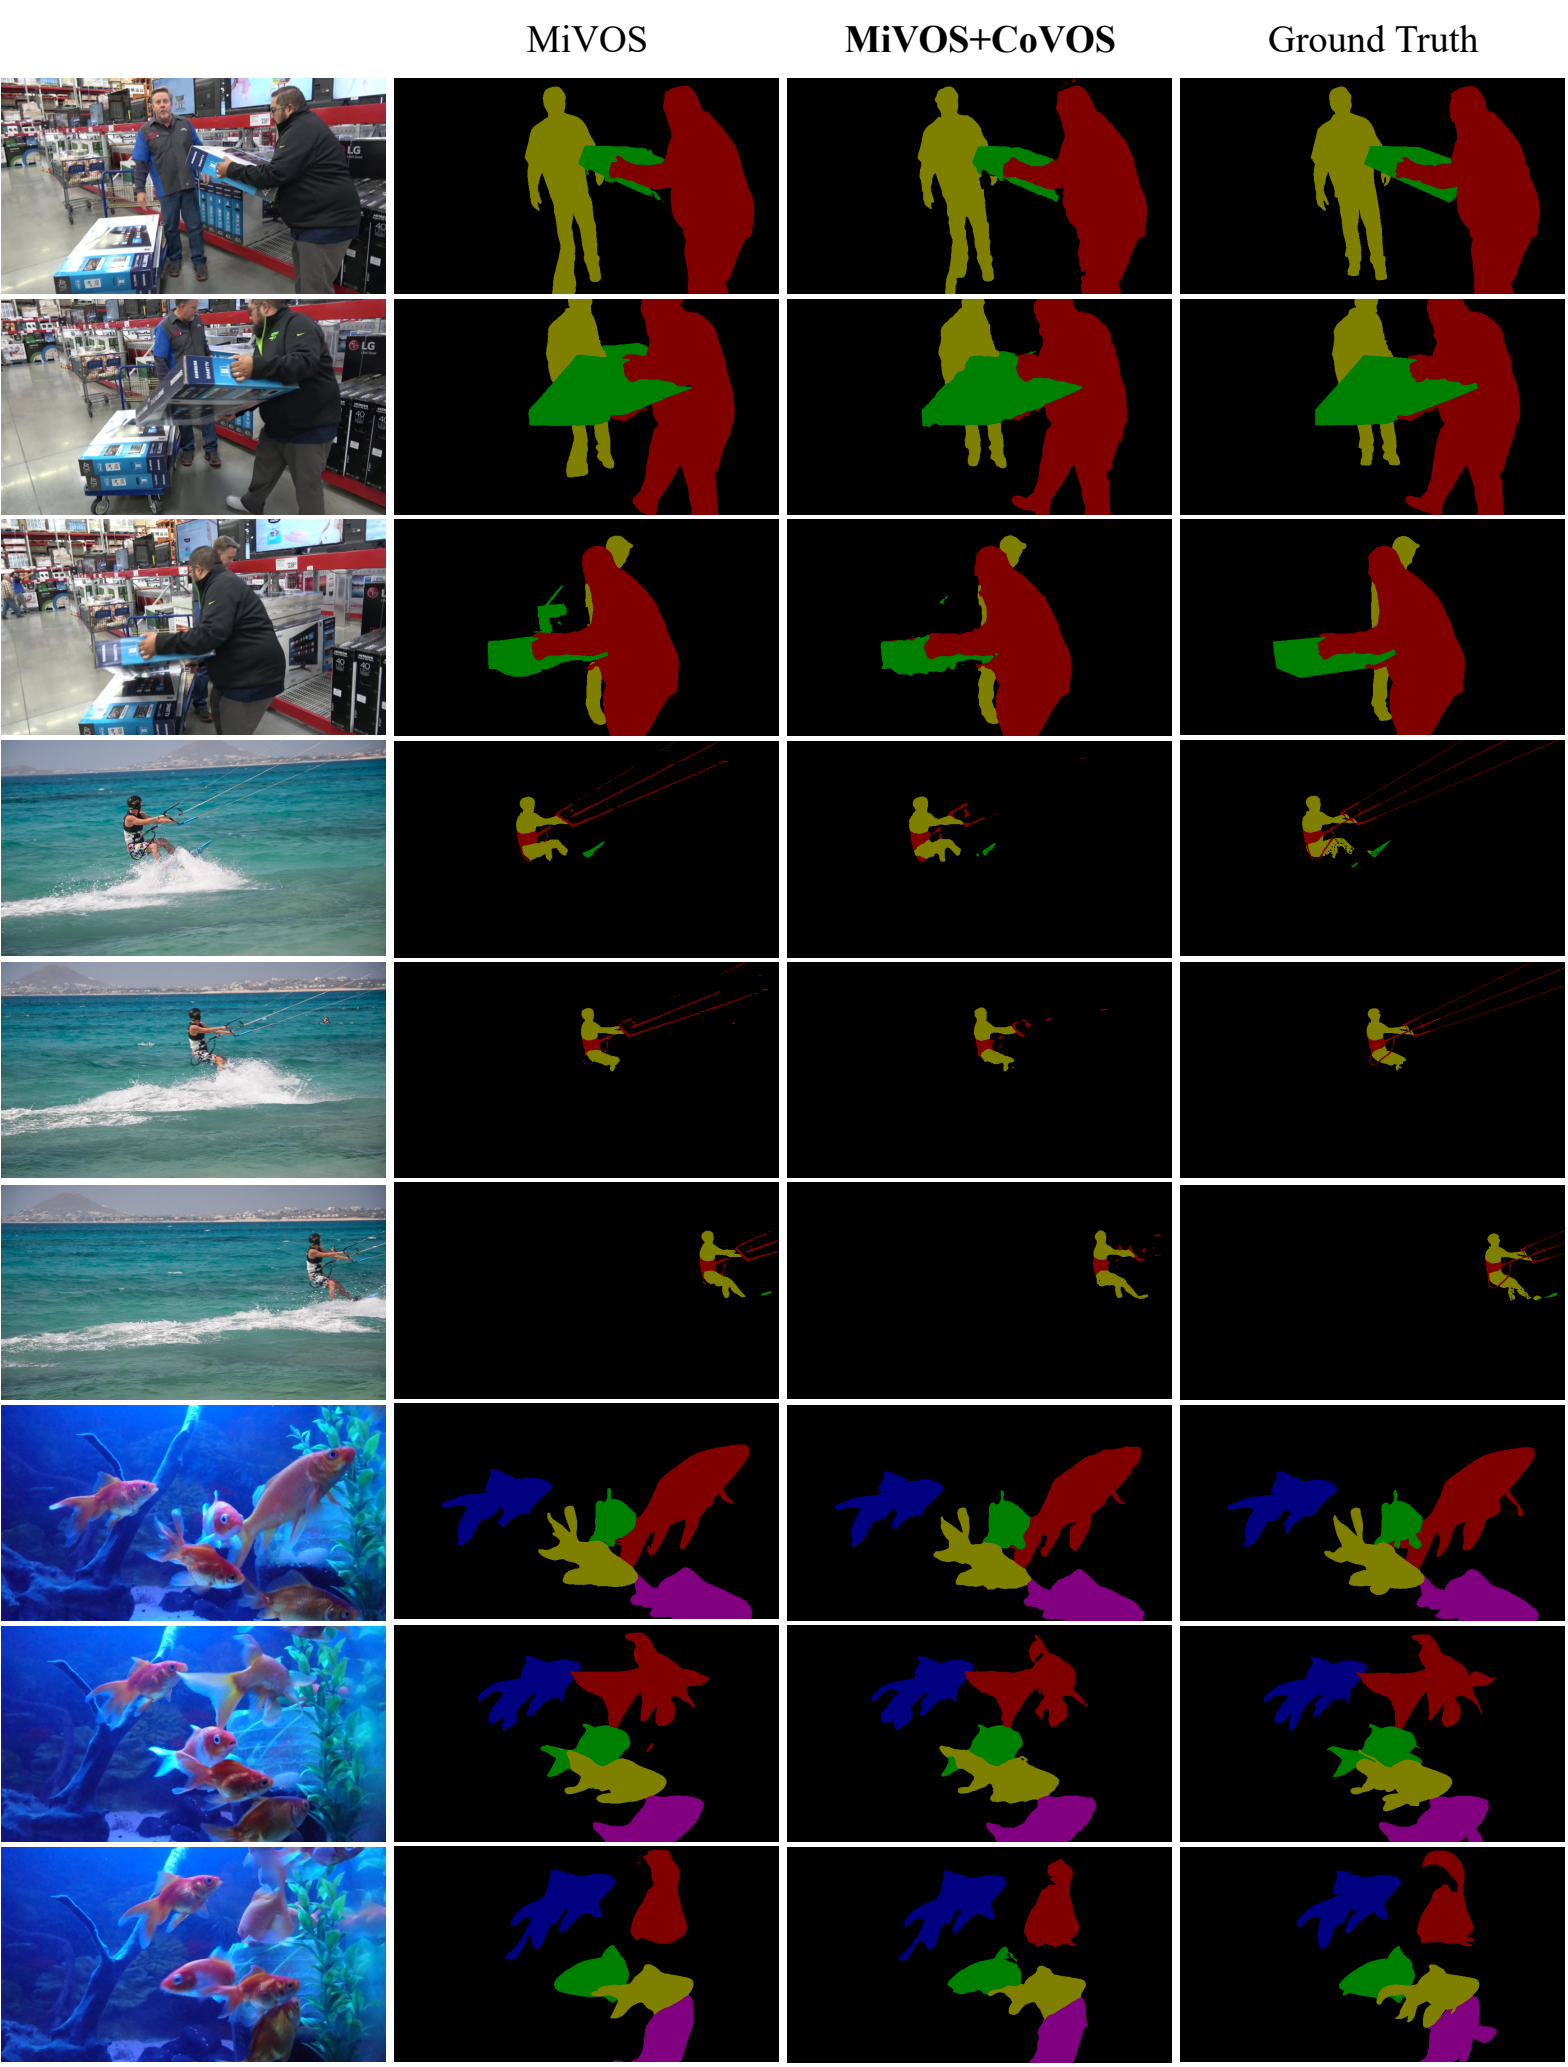   | 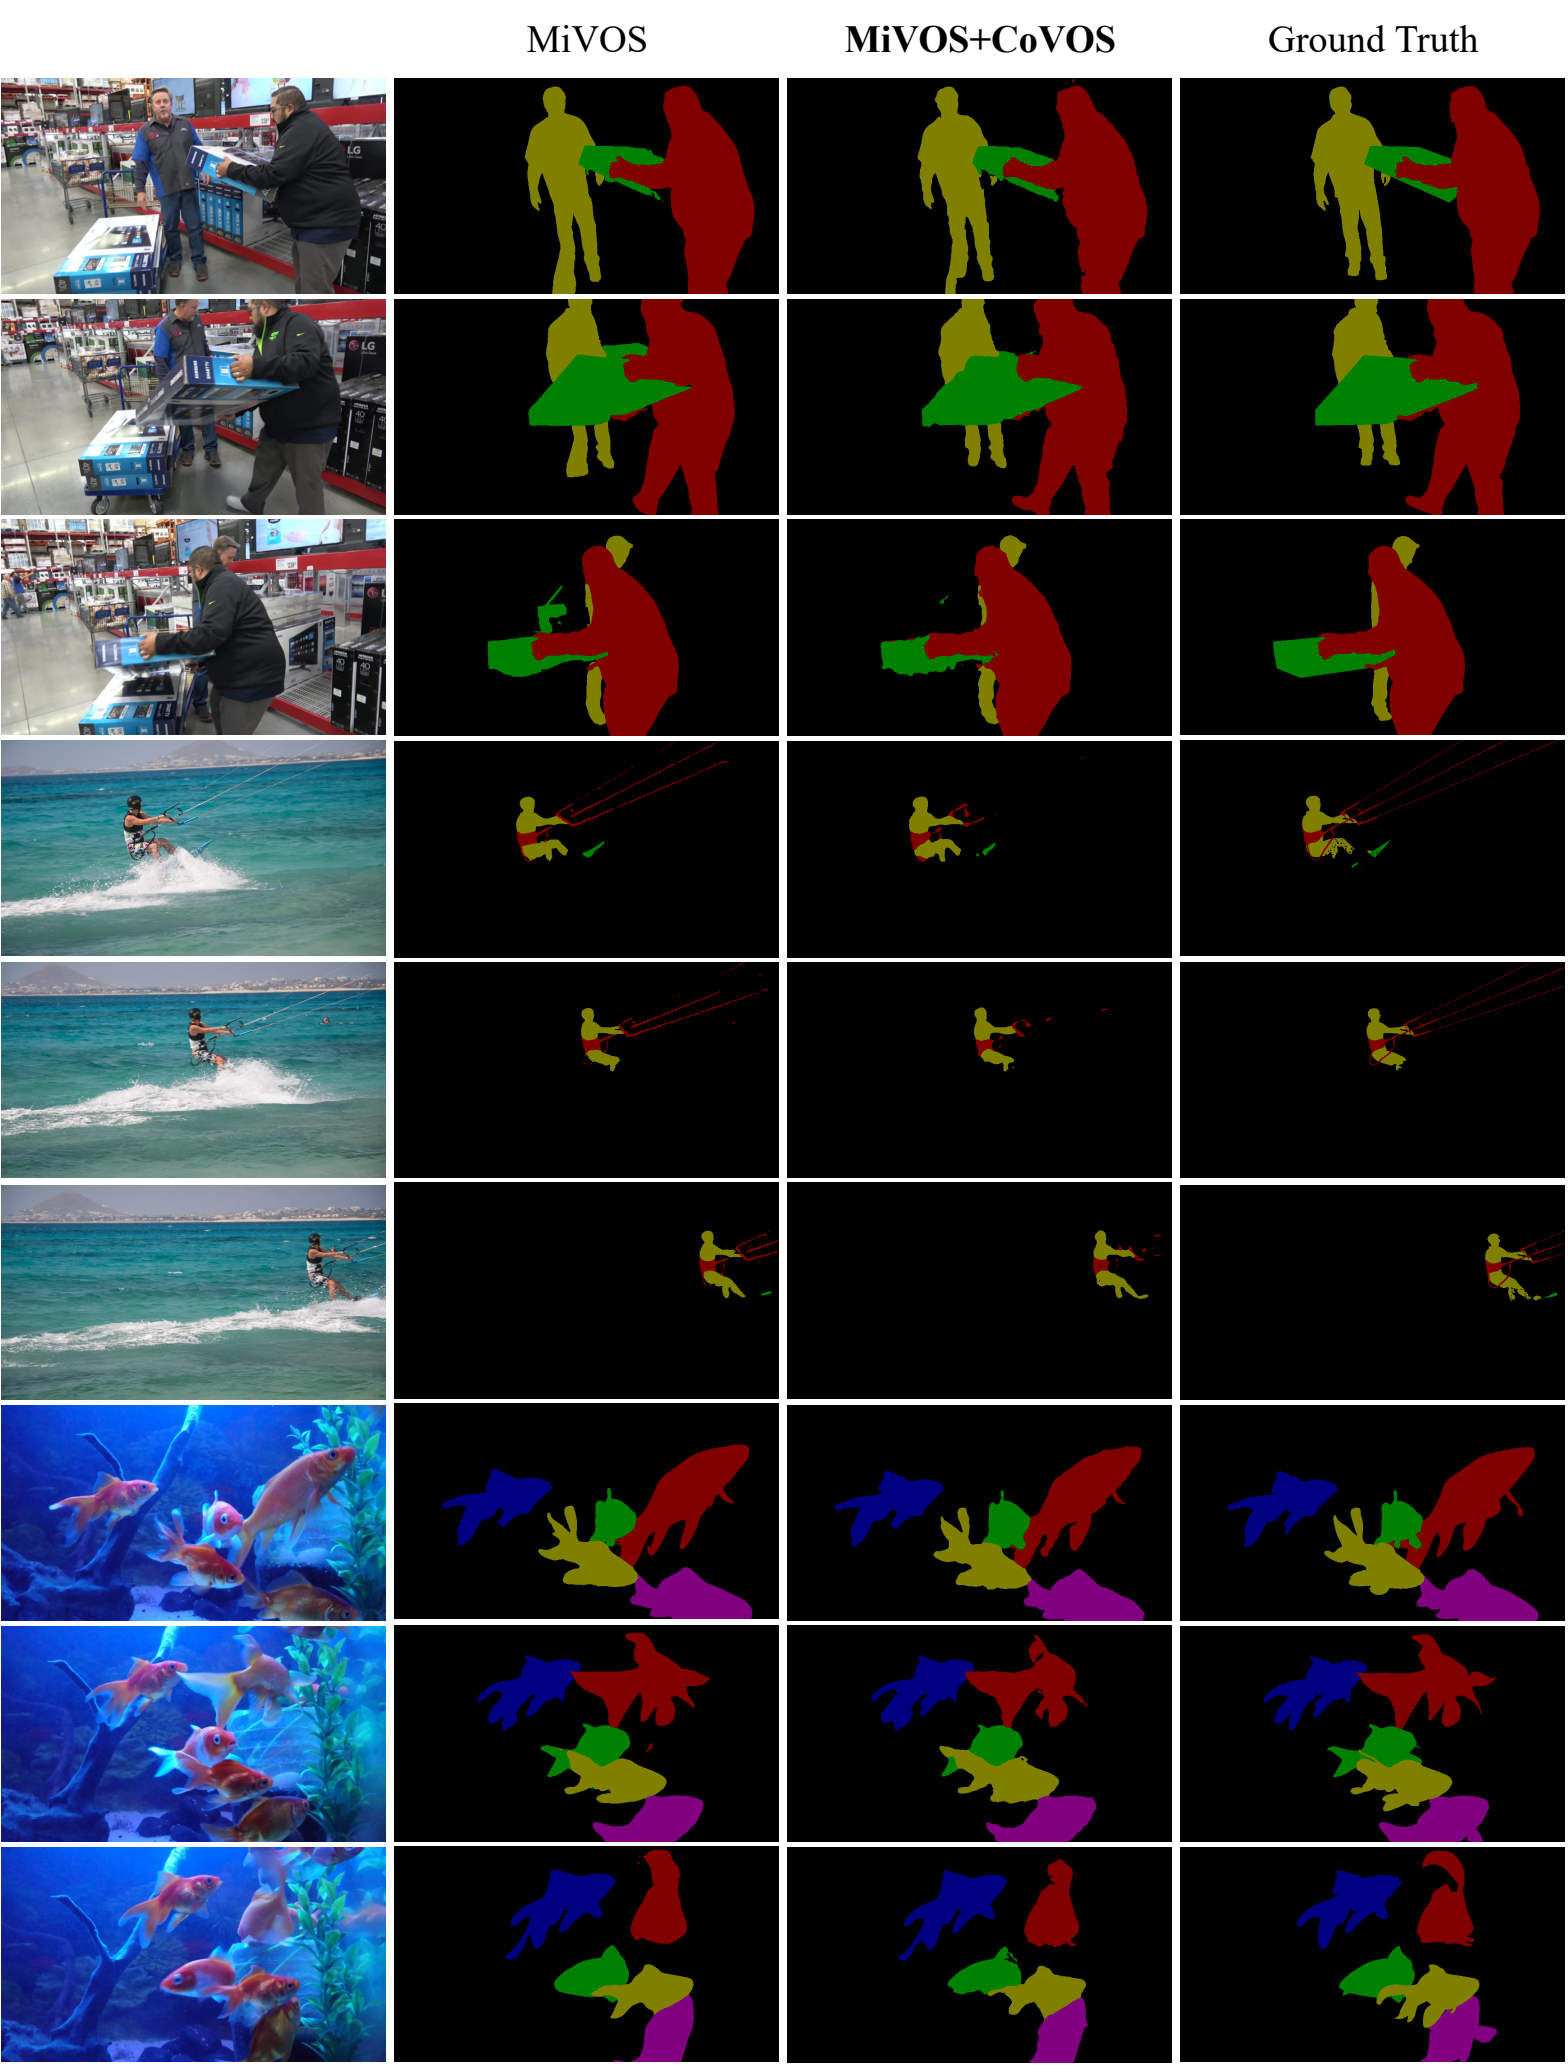   | 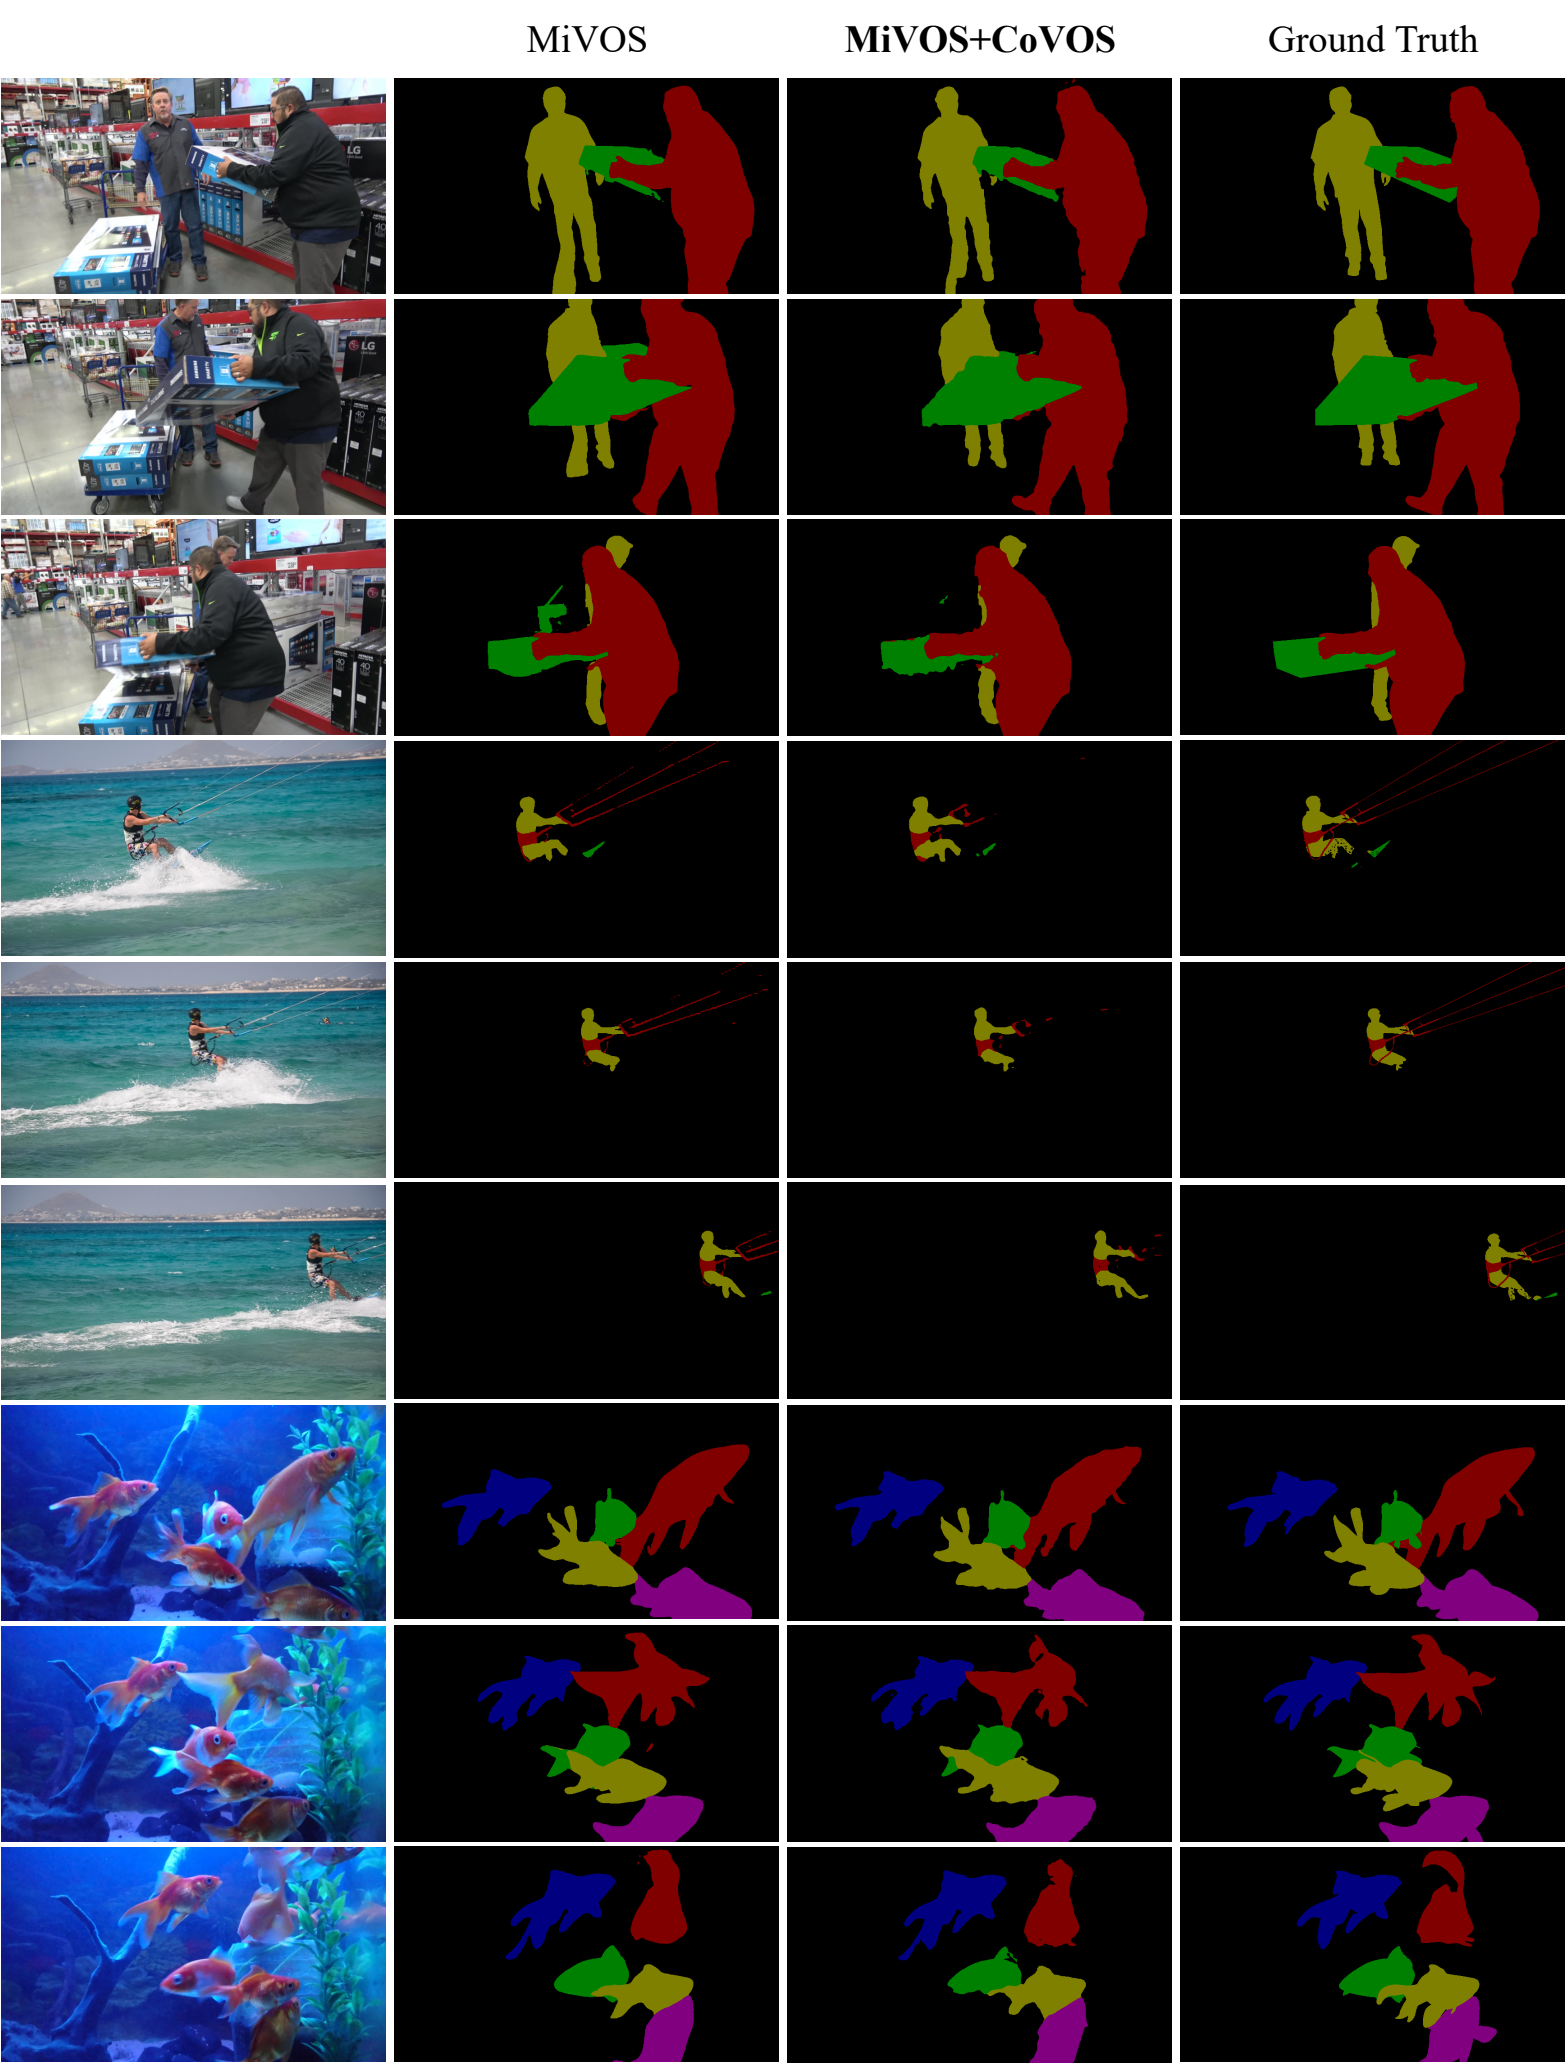   |
| 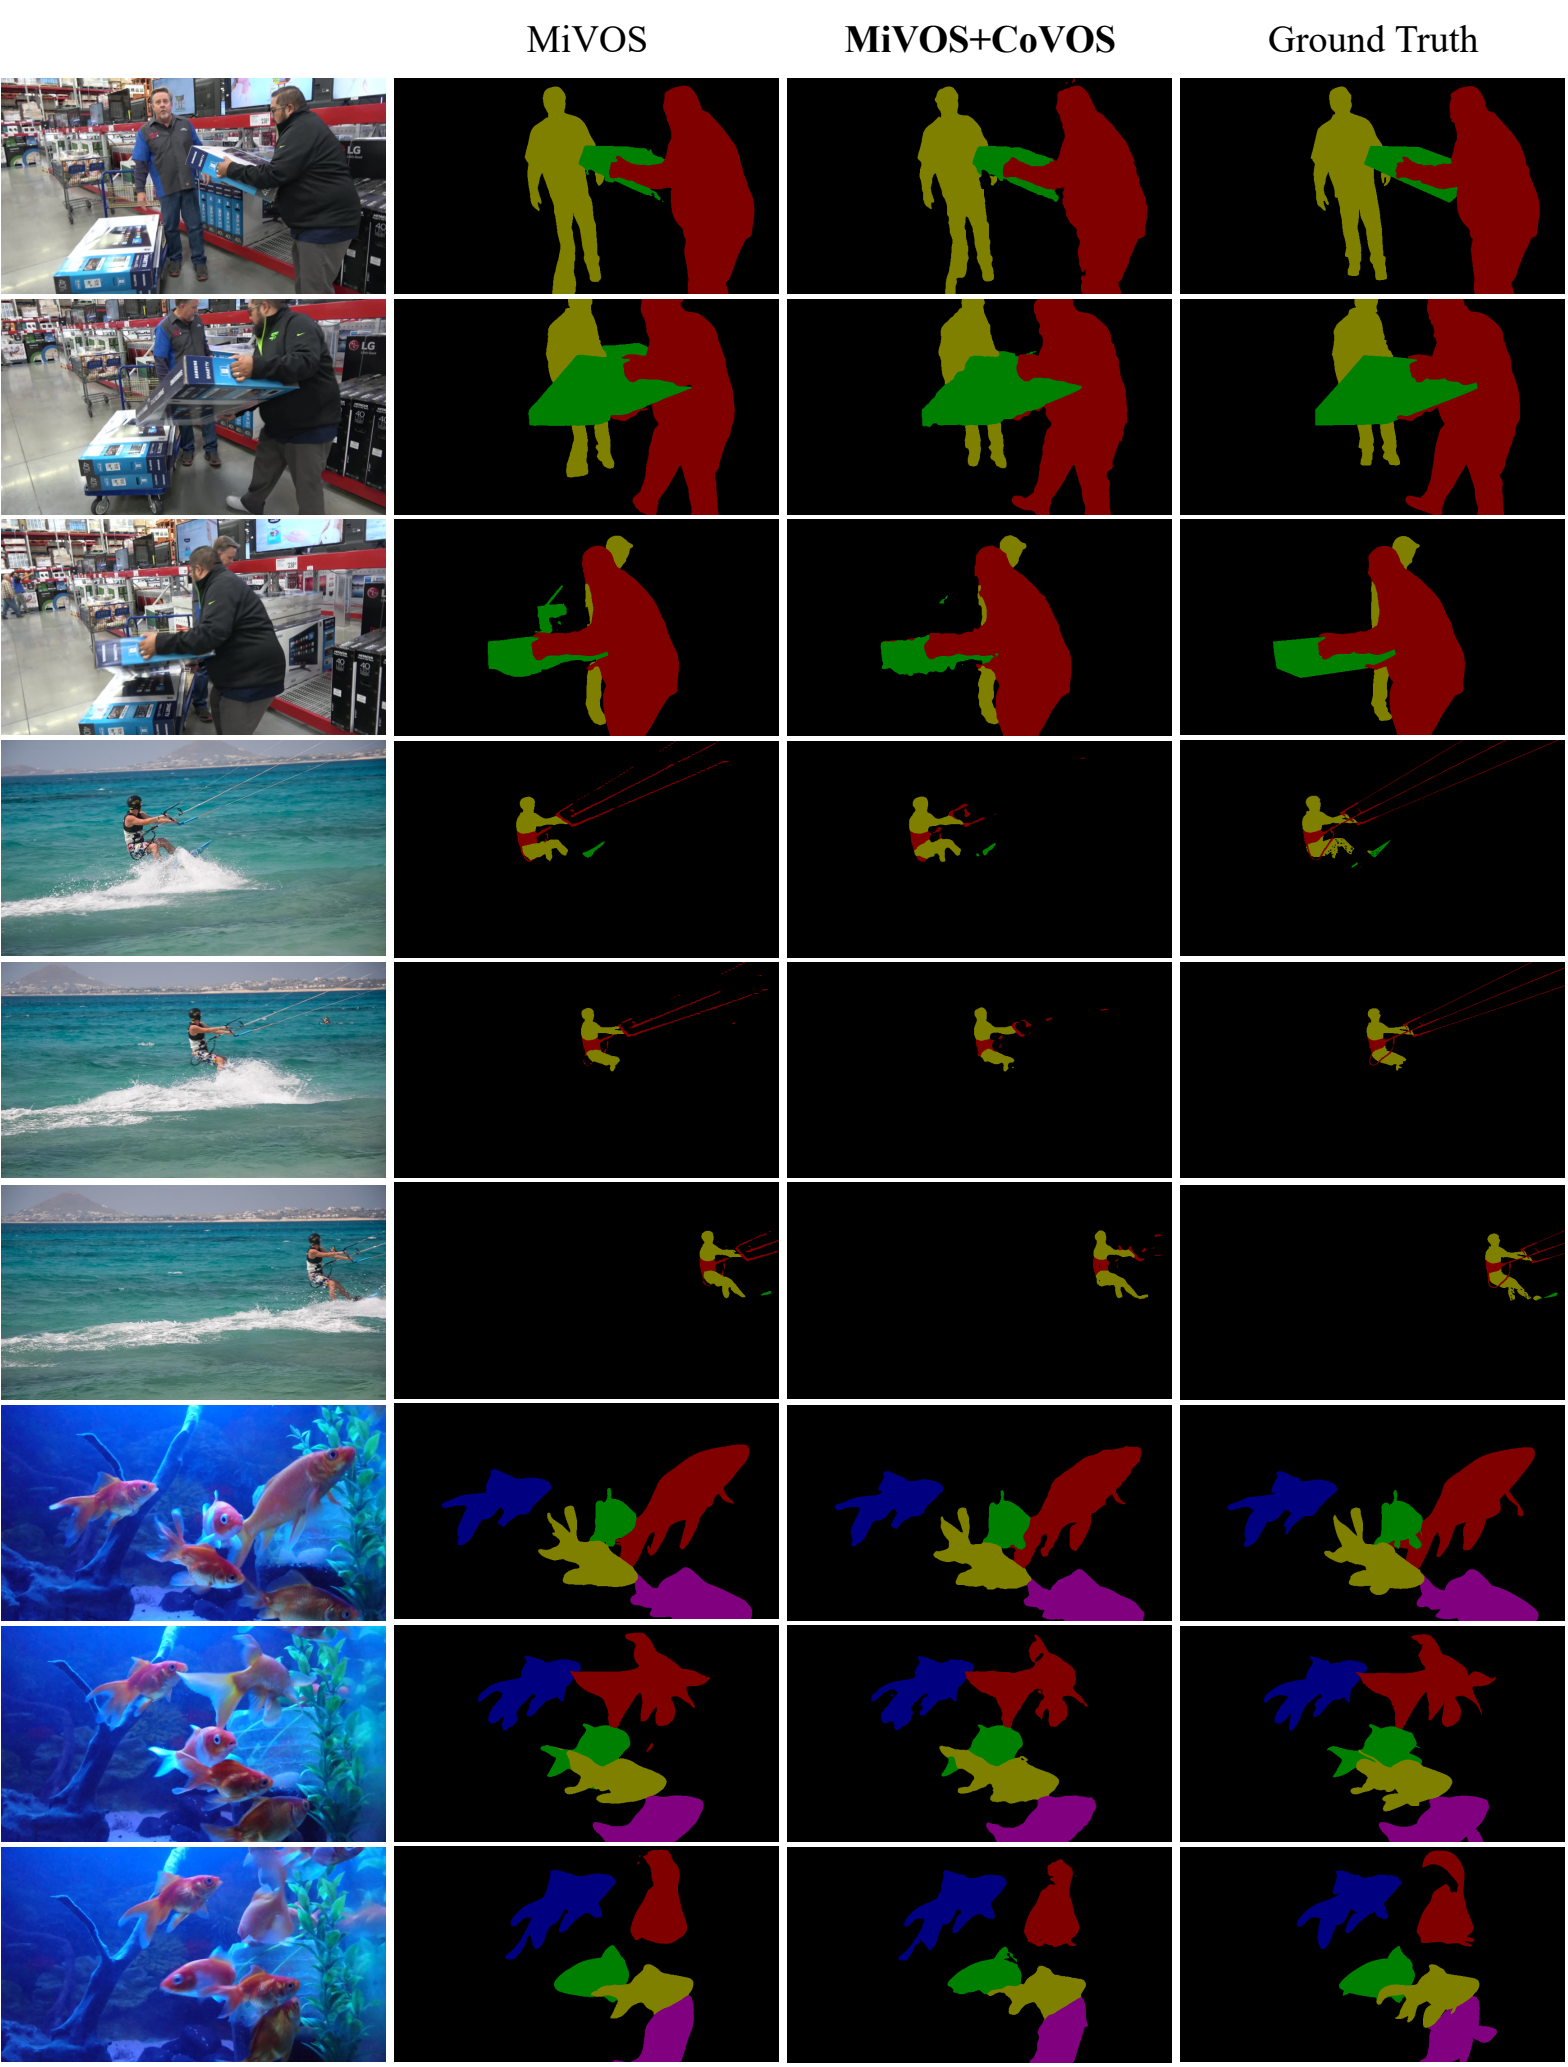   | 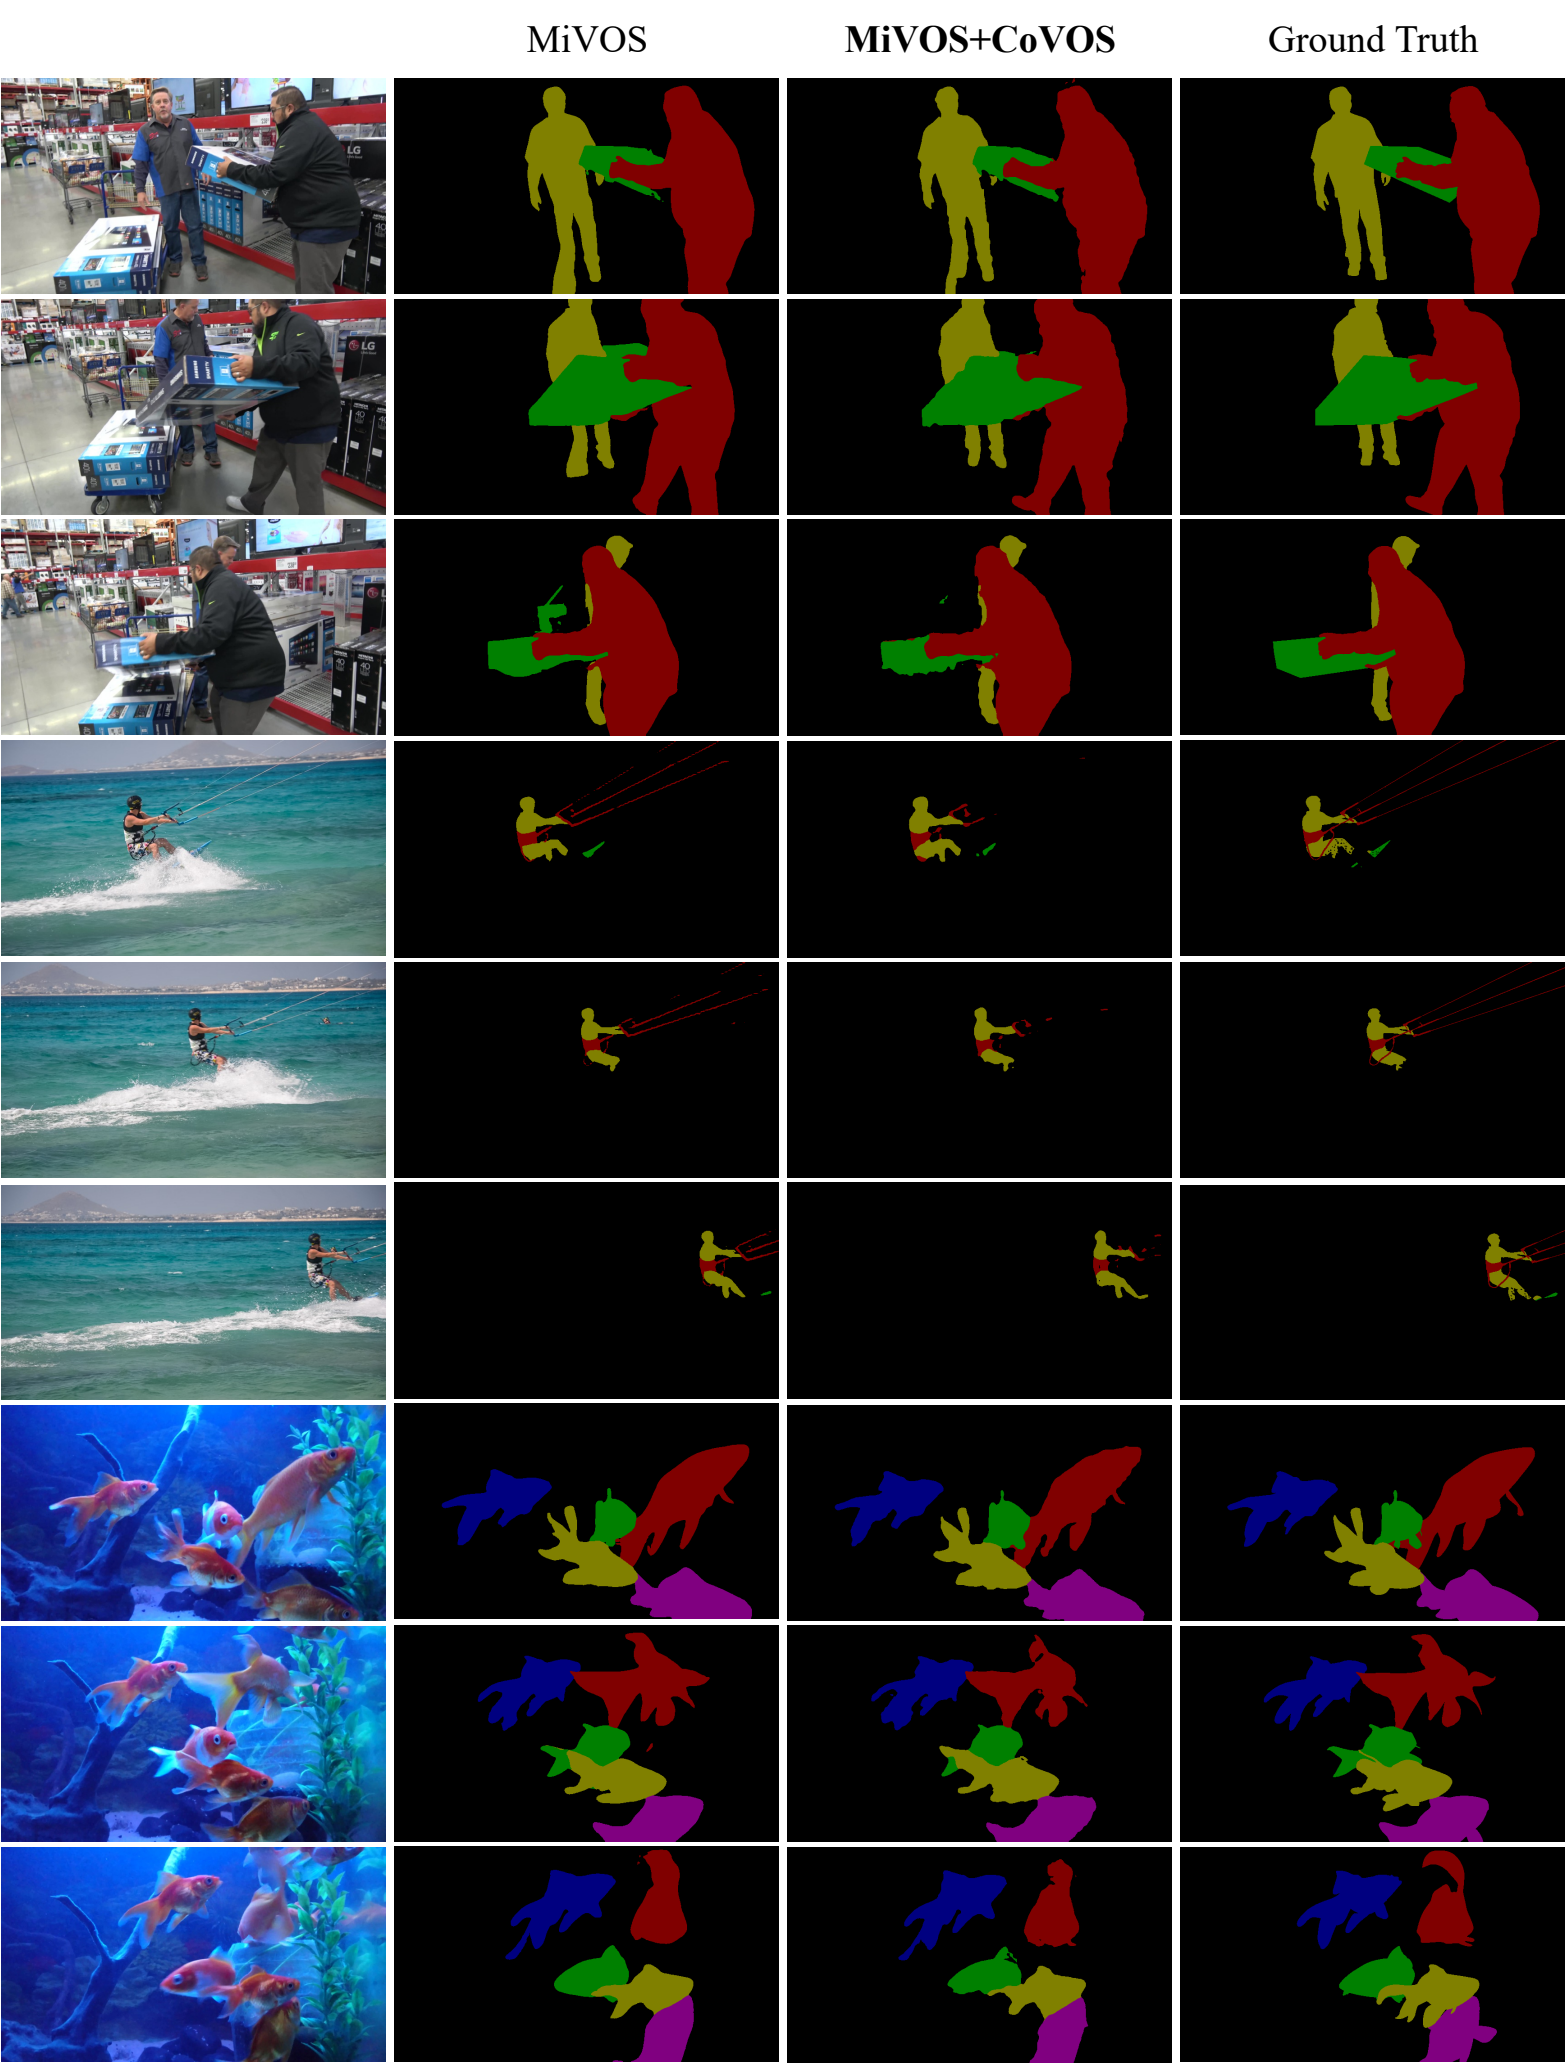   | 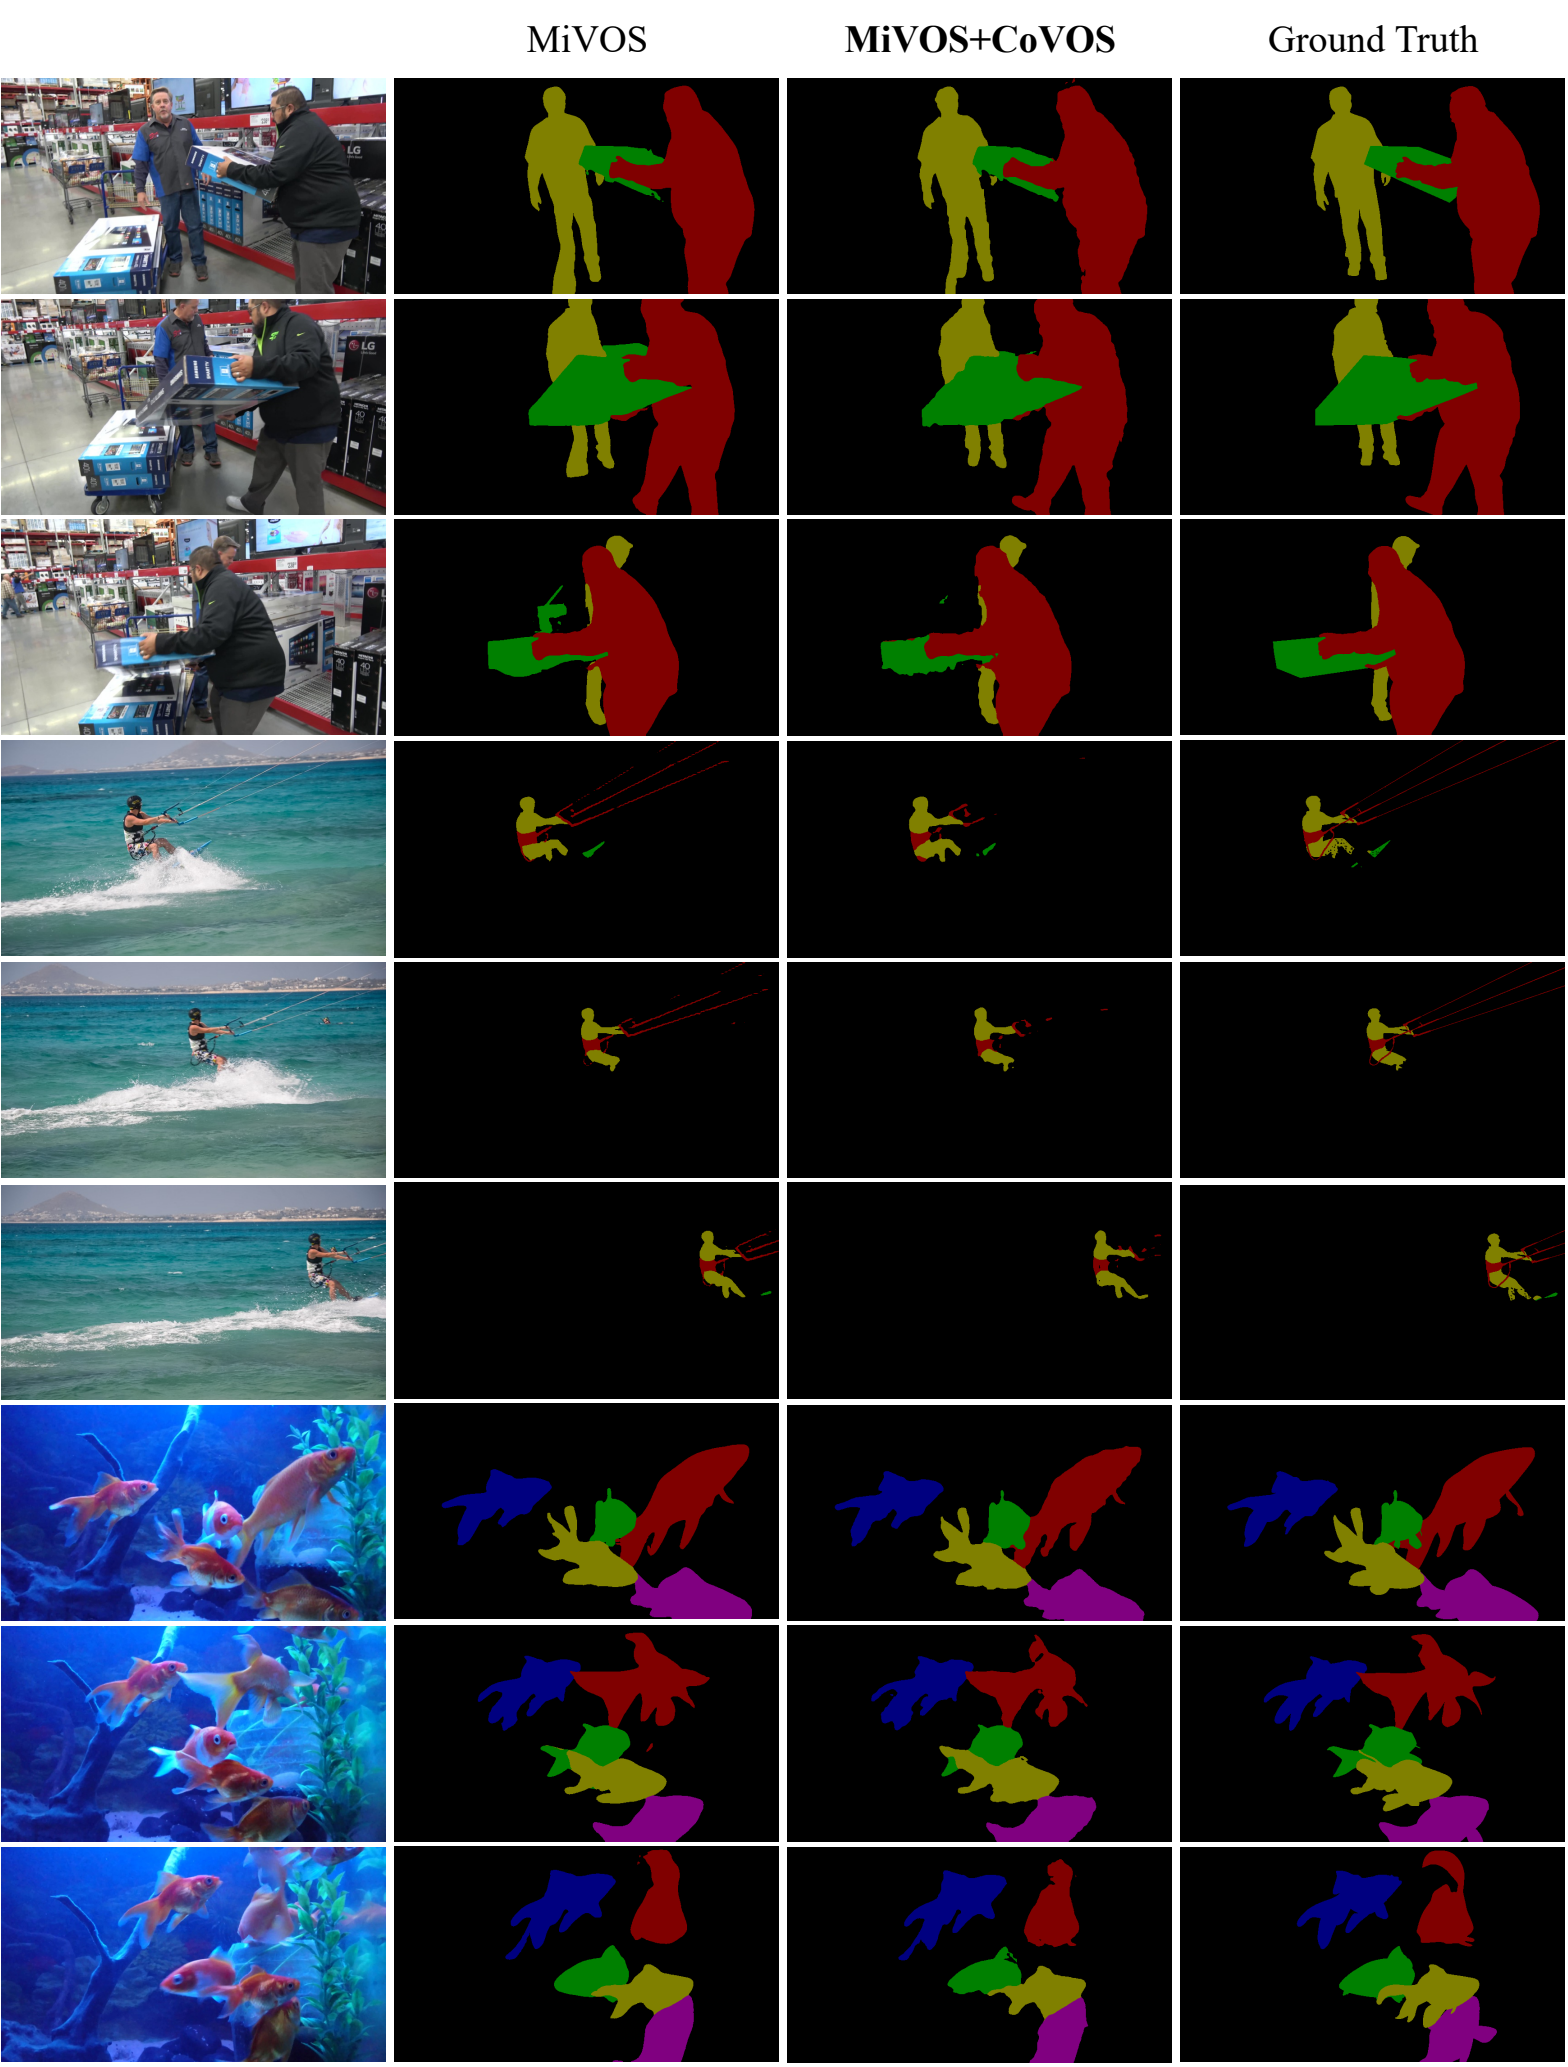   | 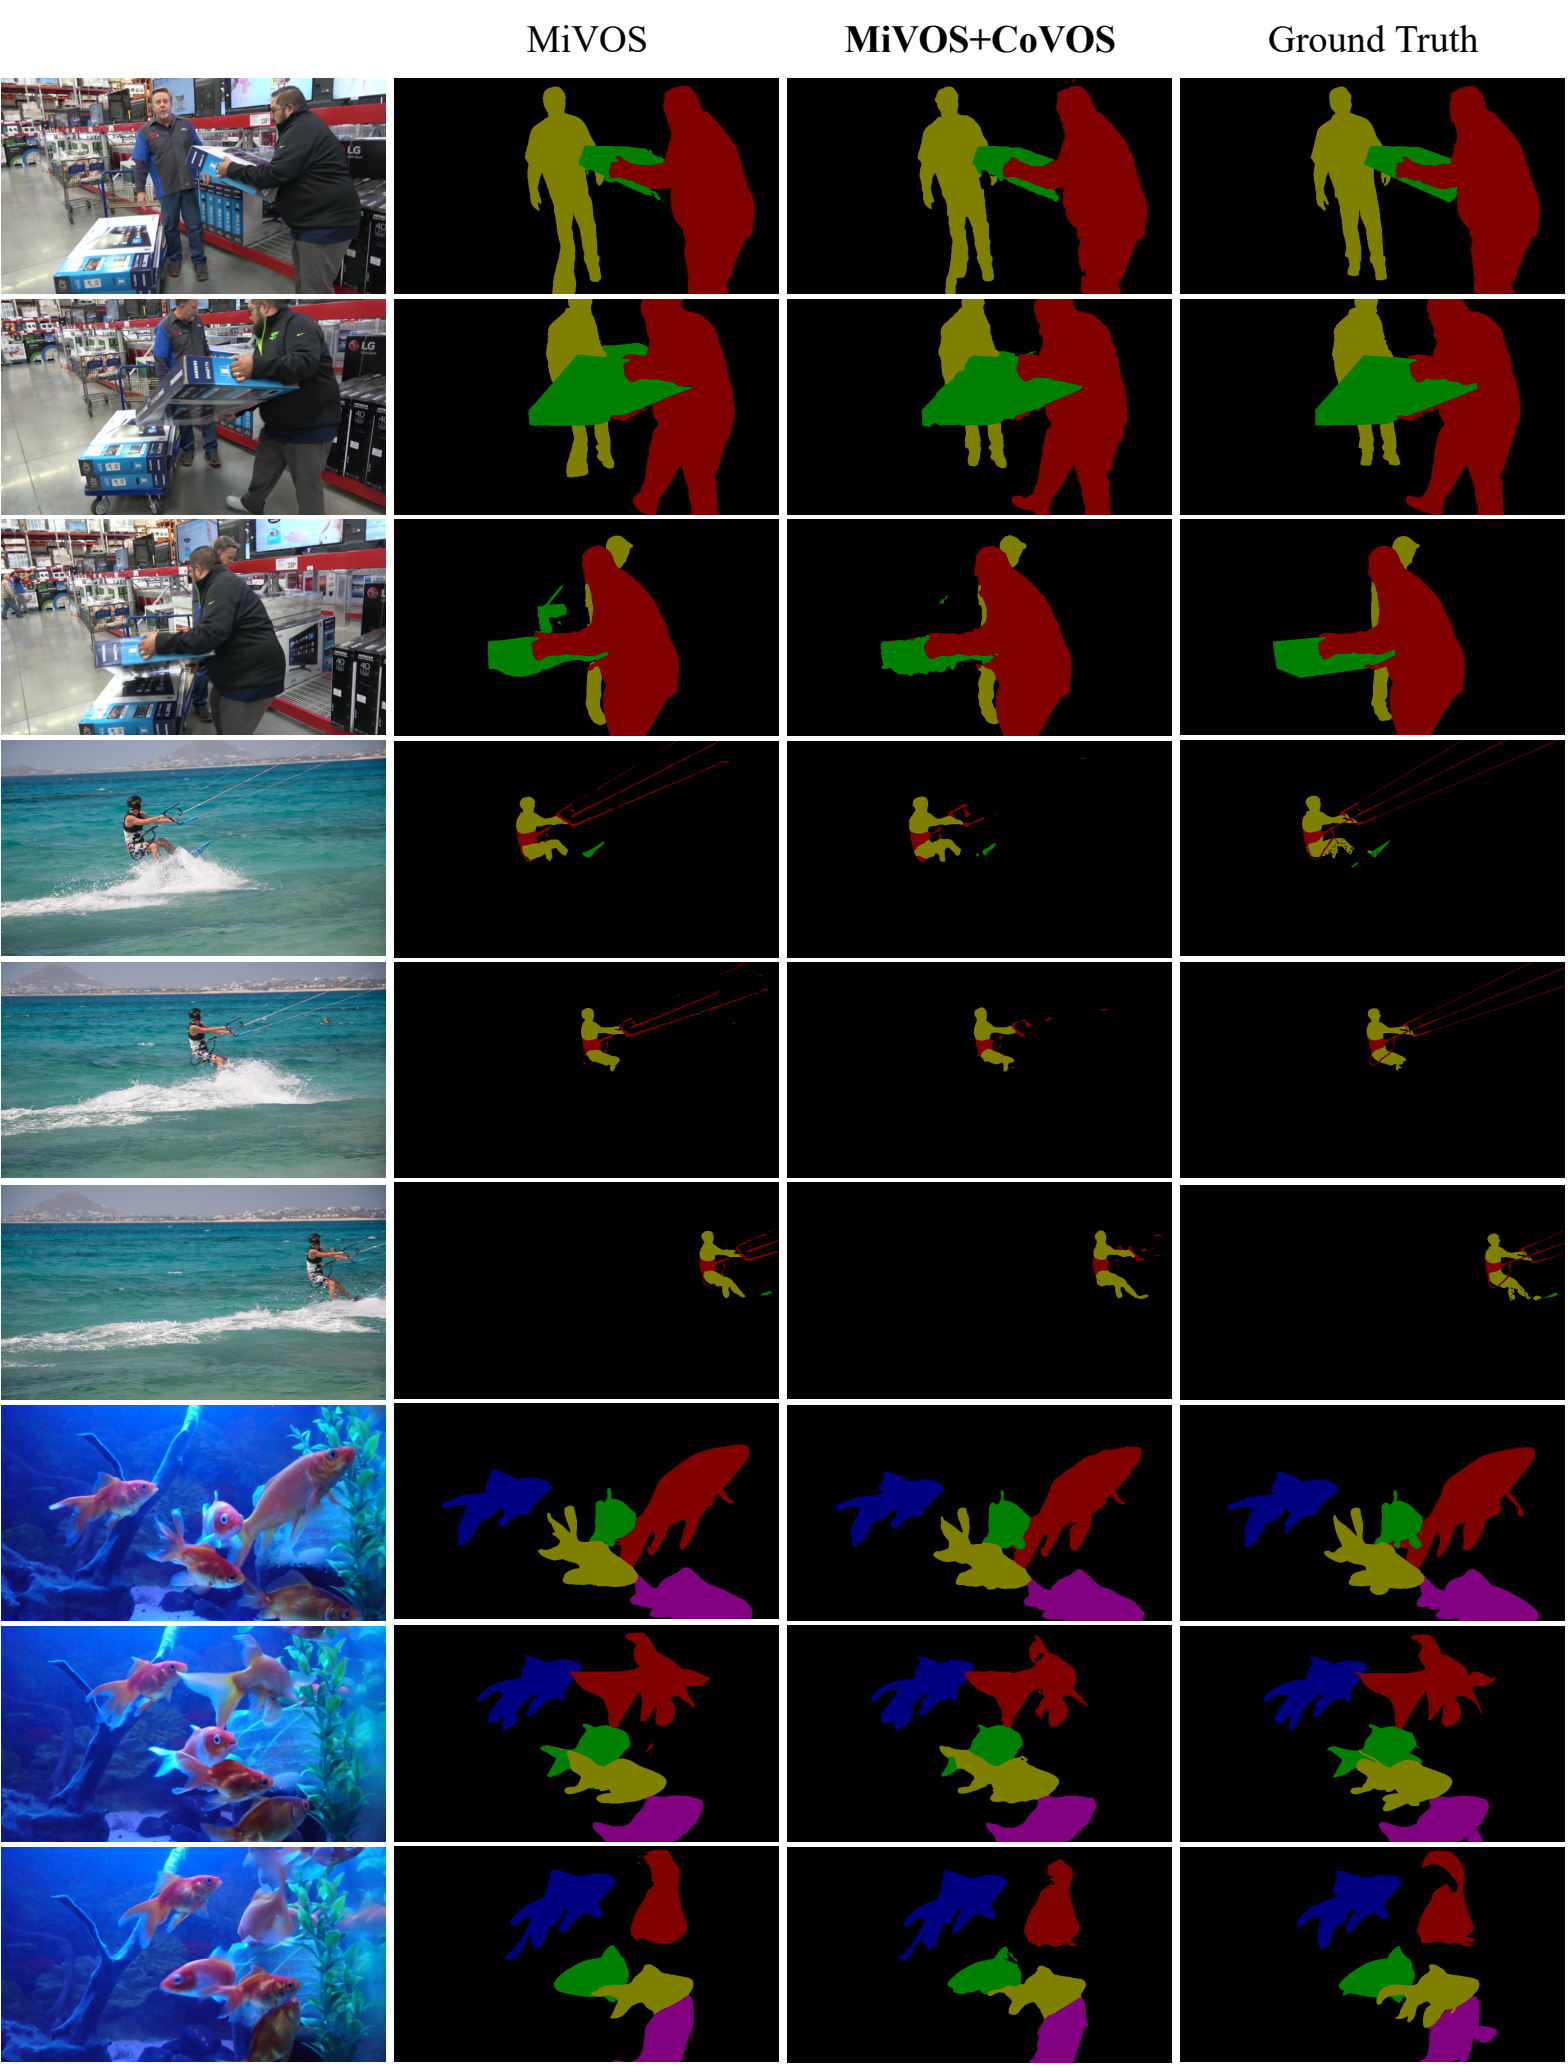   |
| 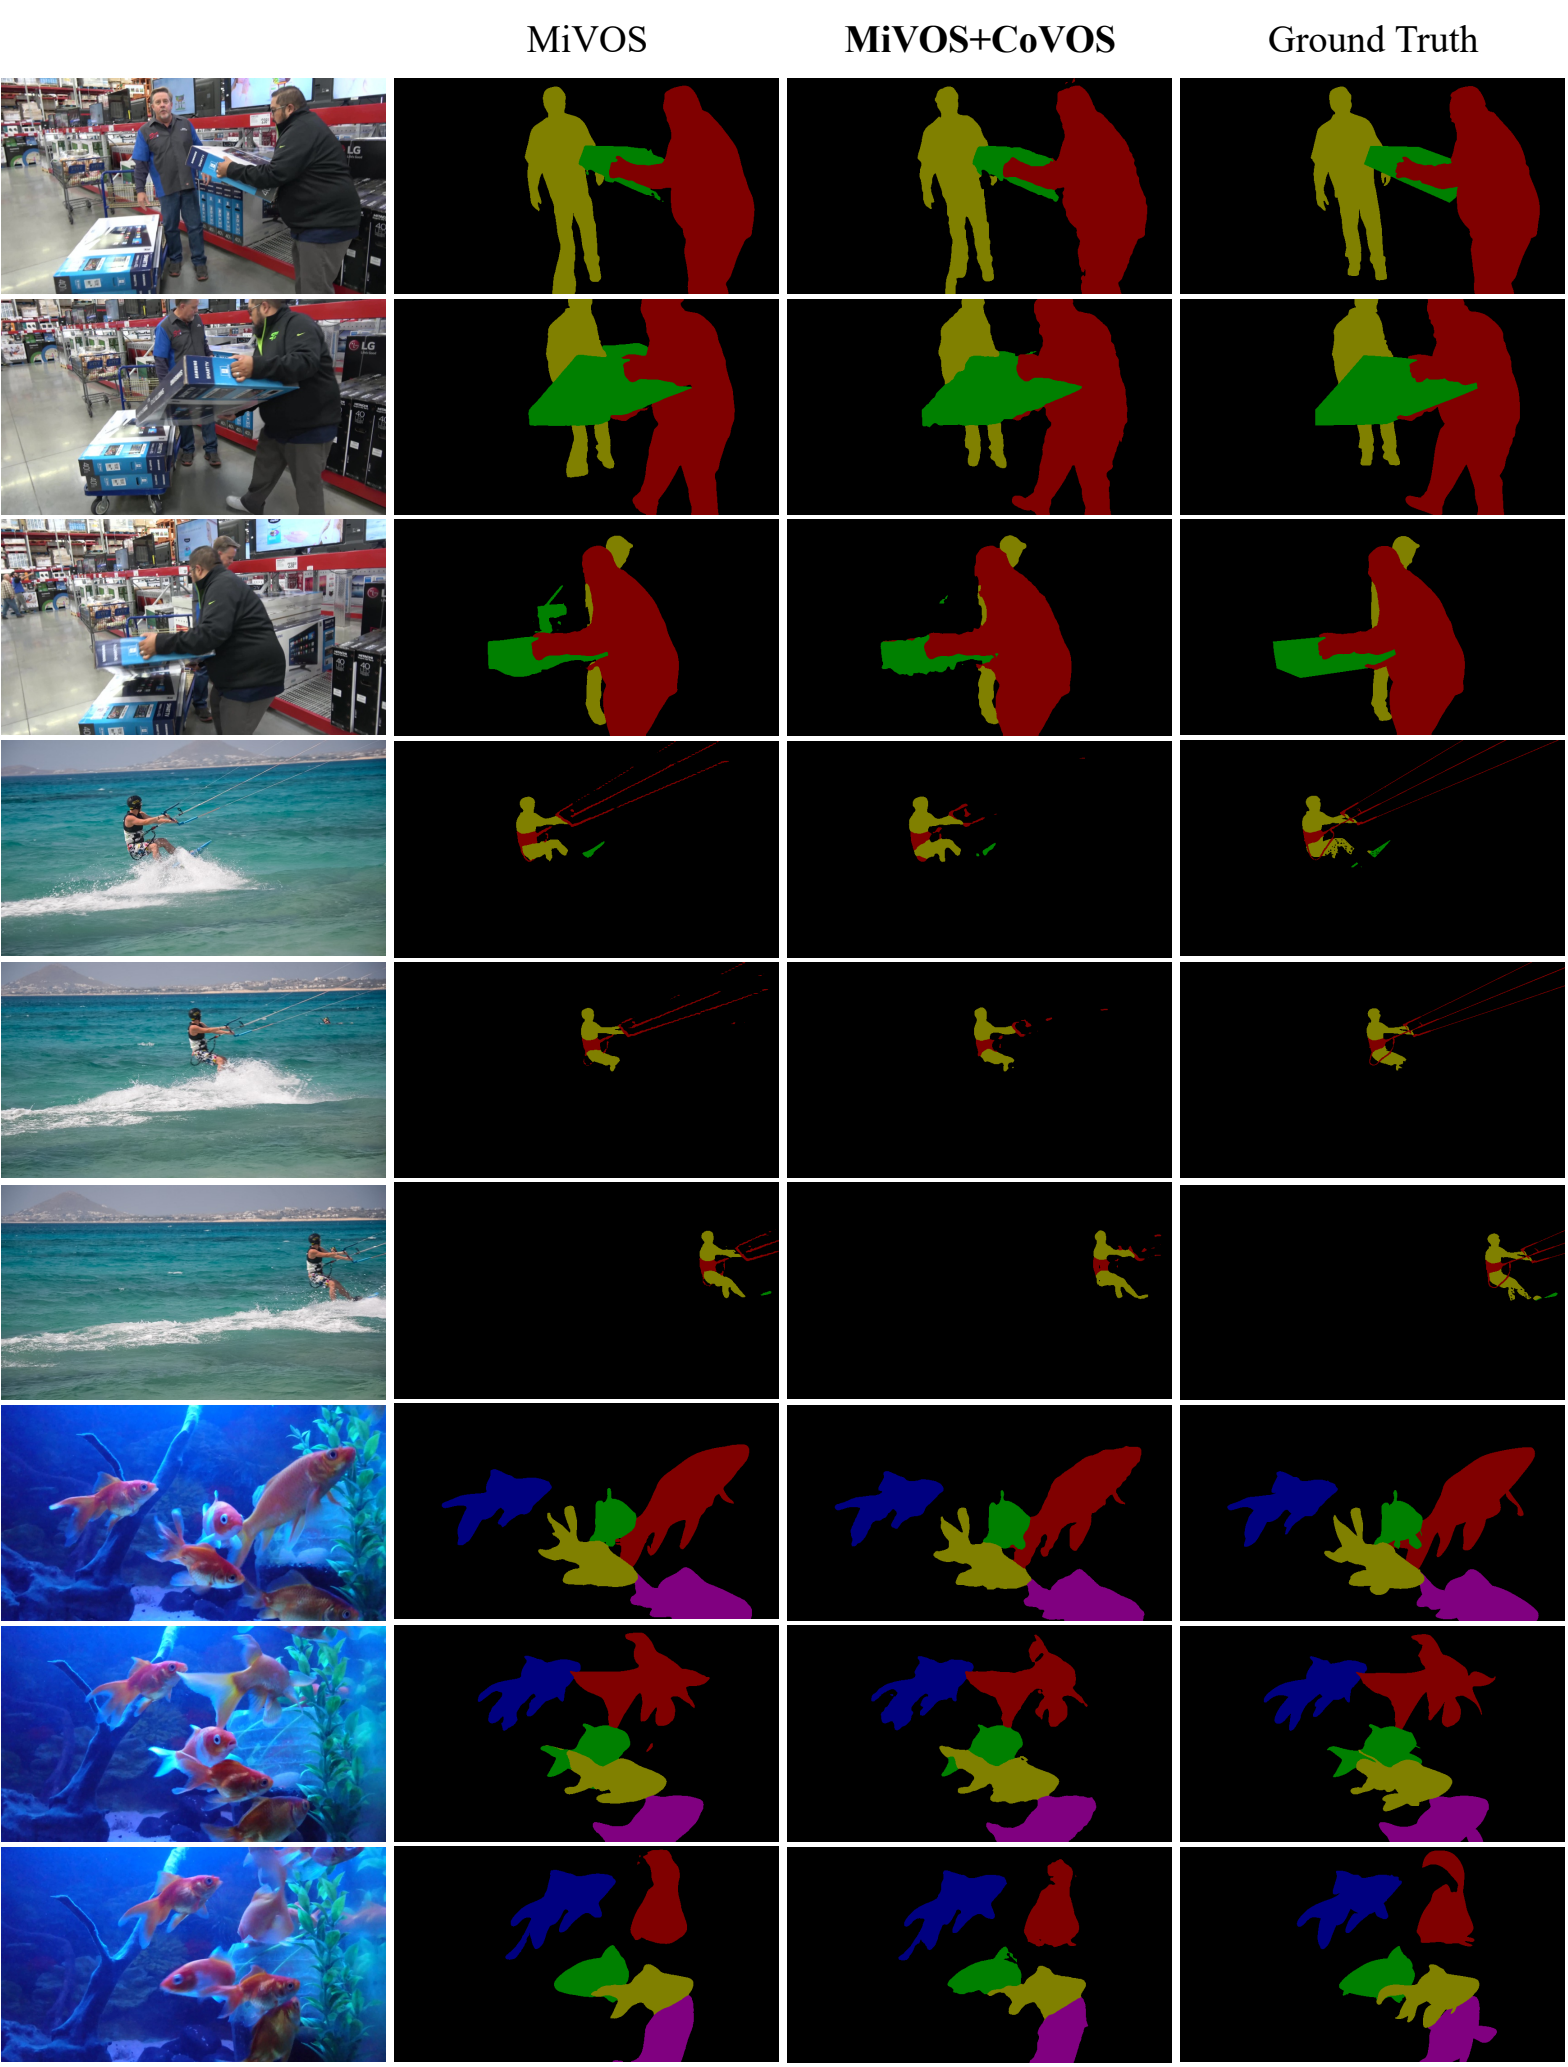  | 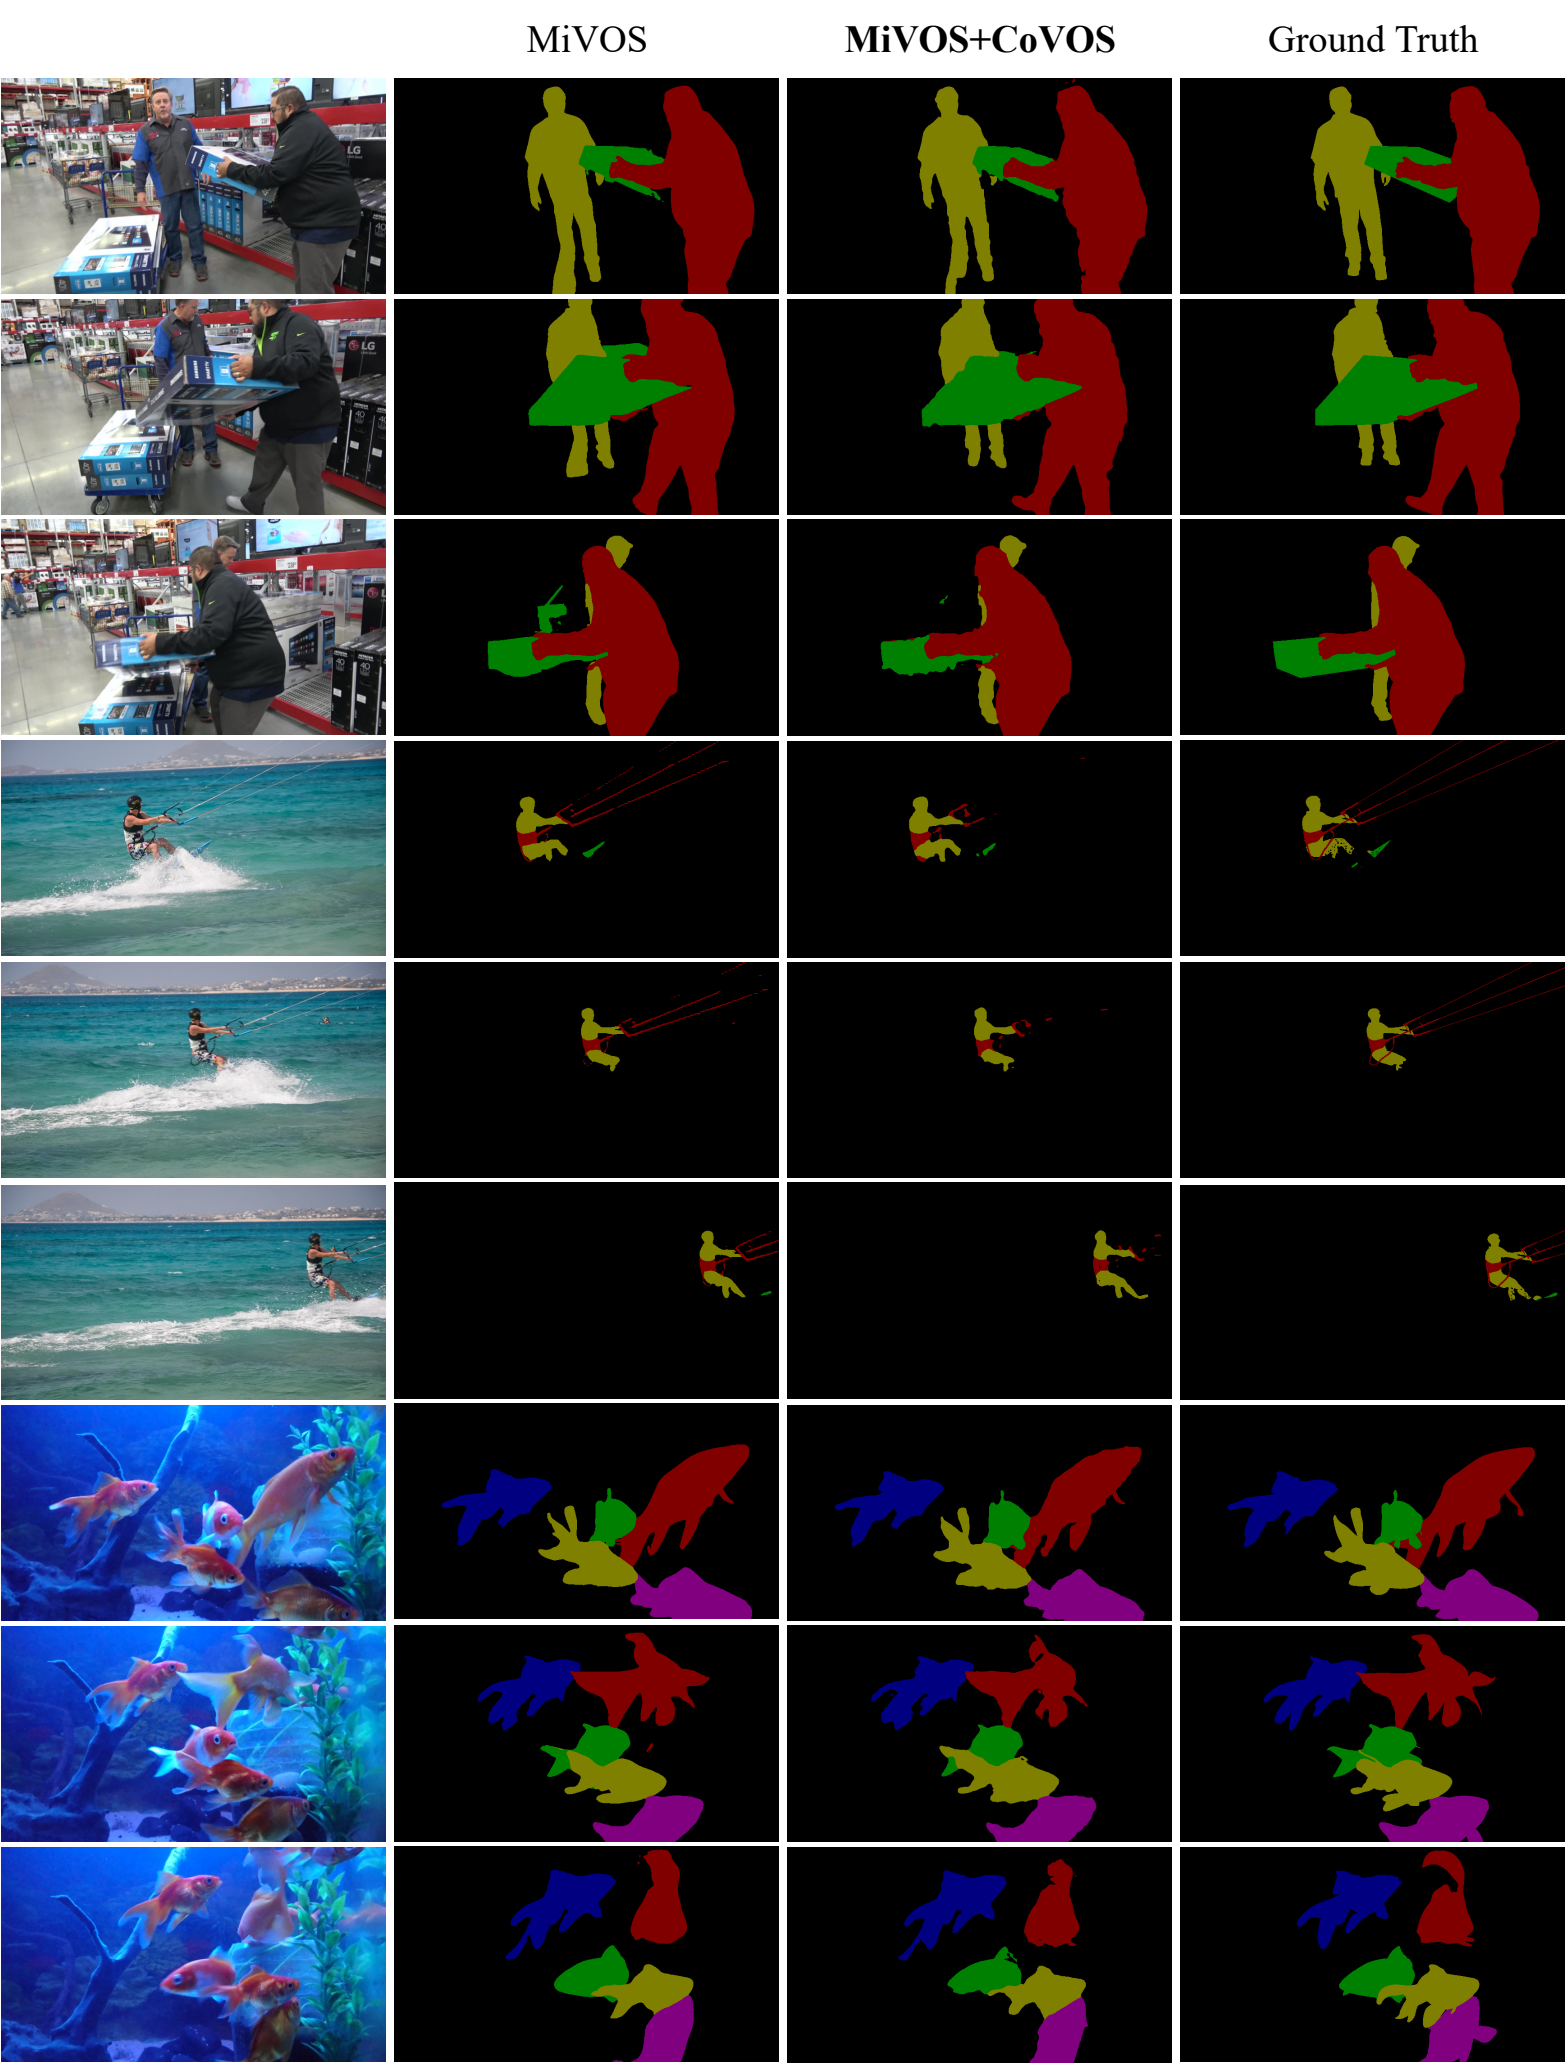  | 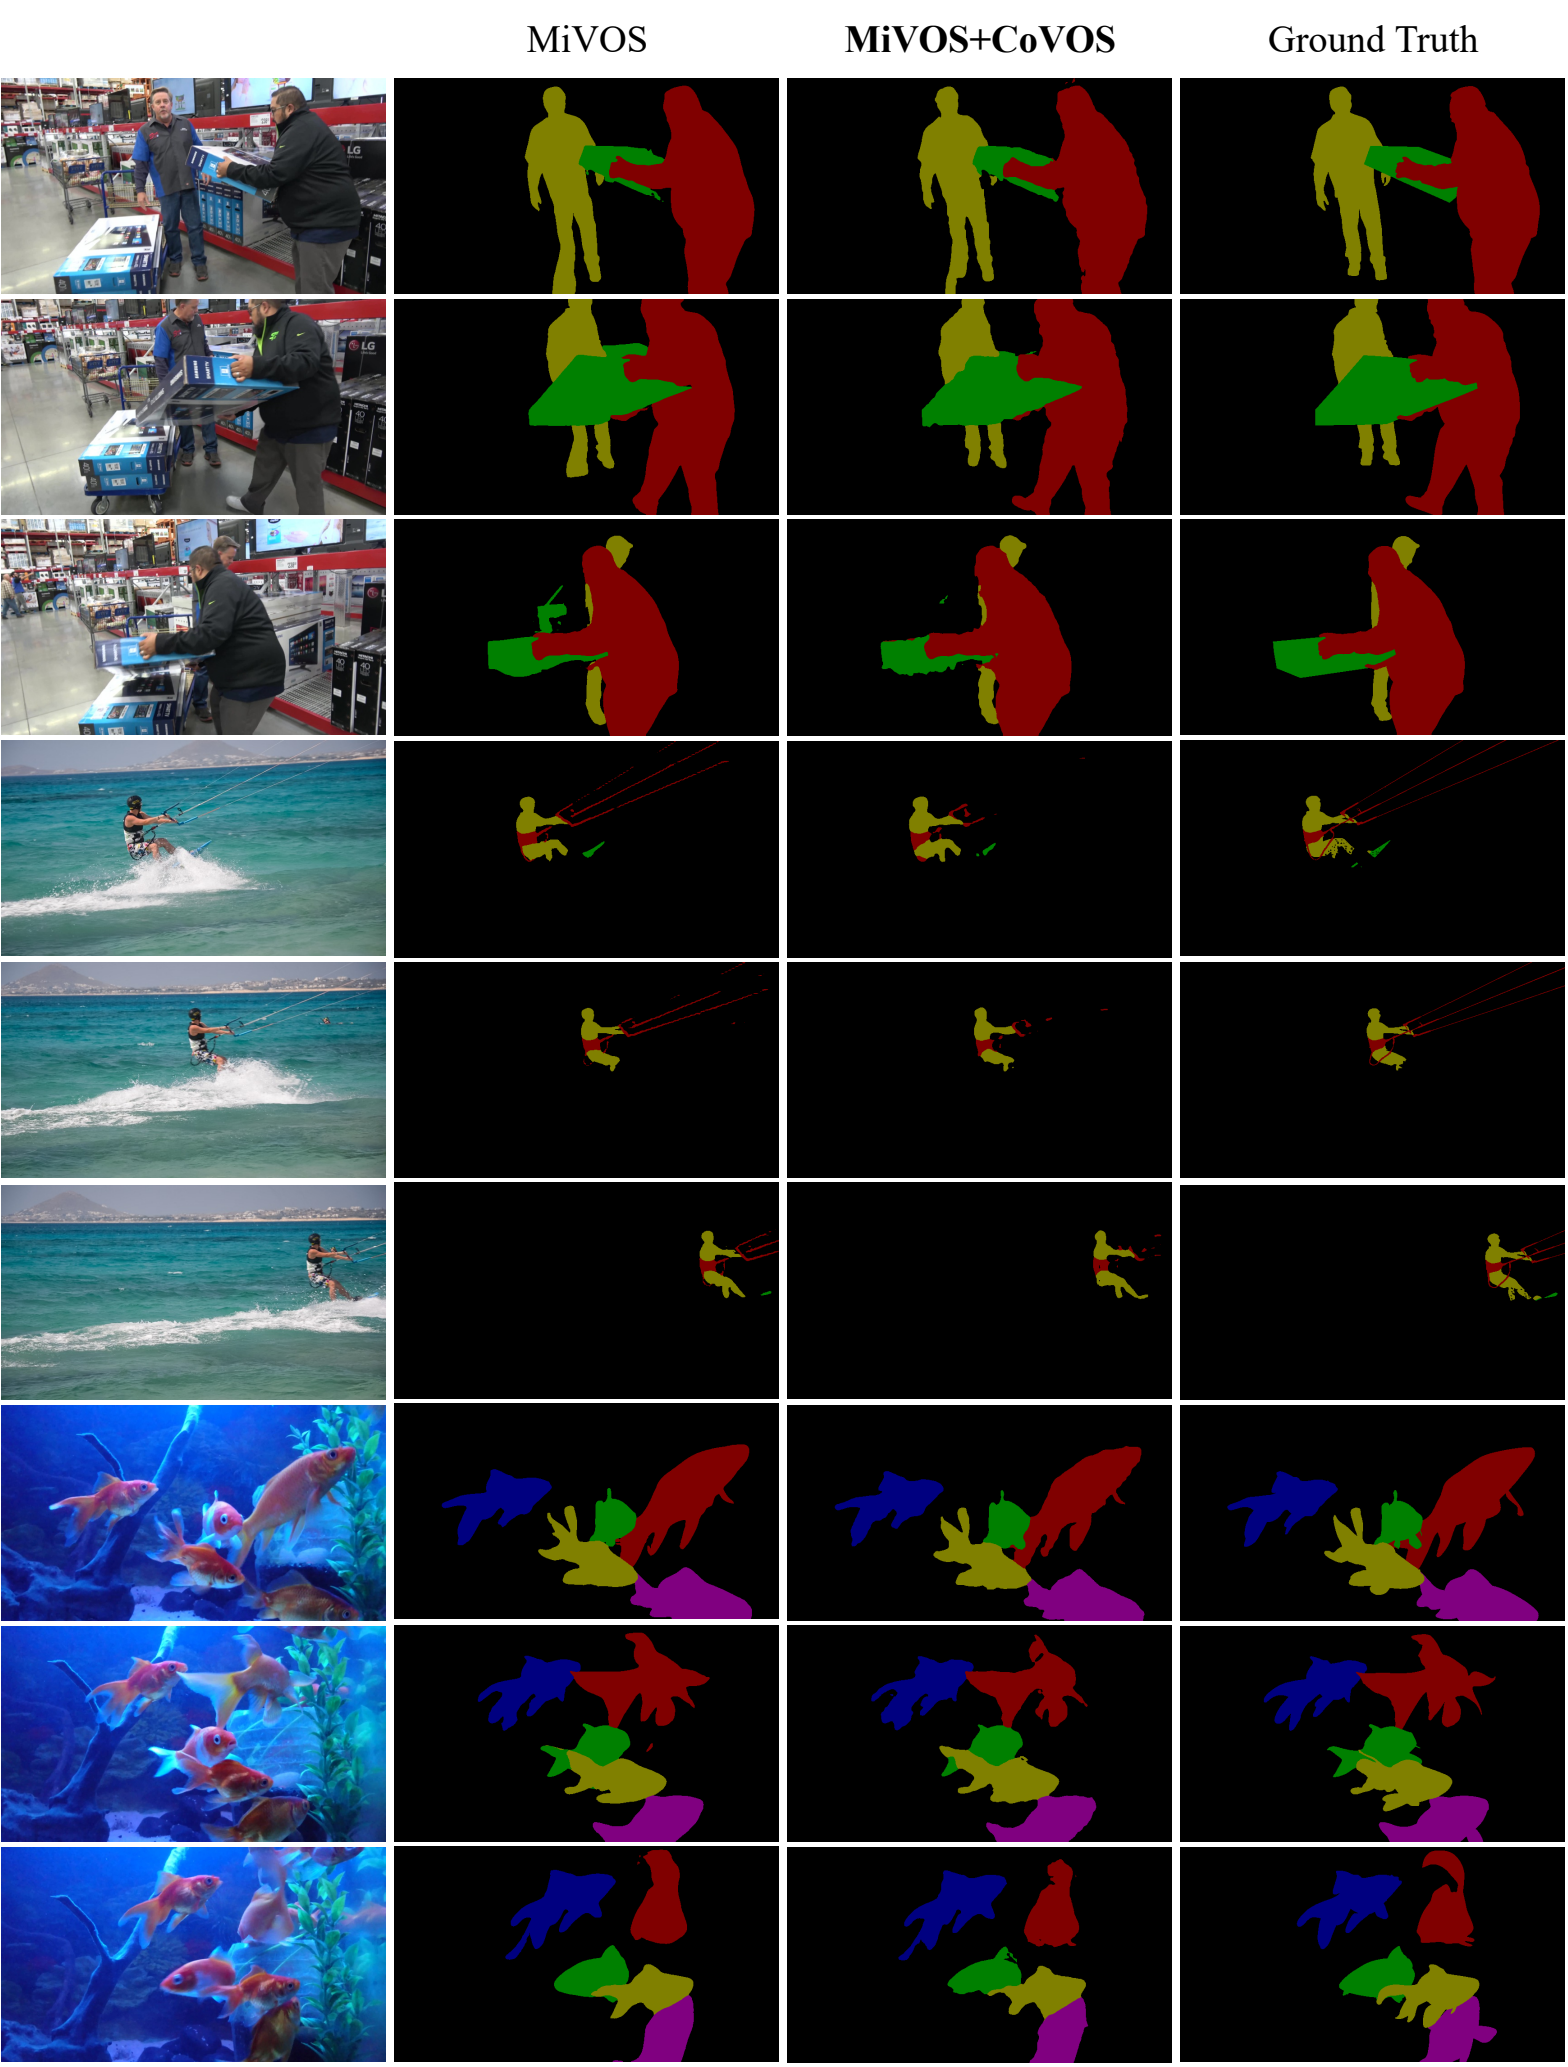  | 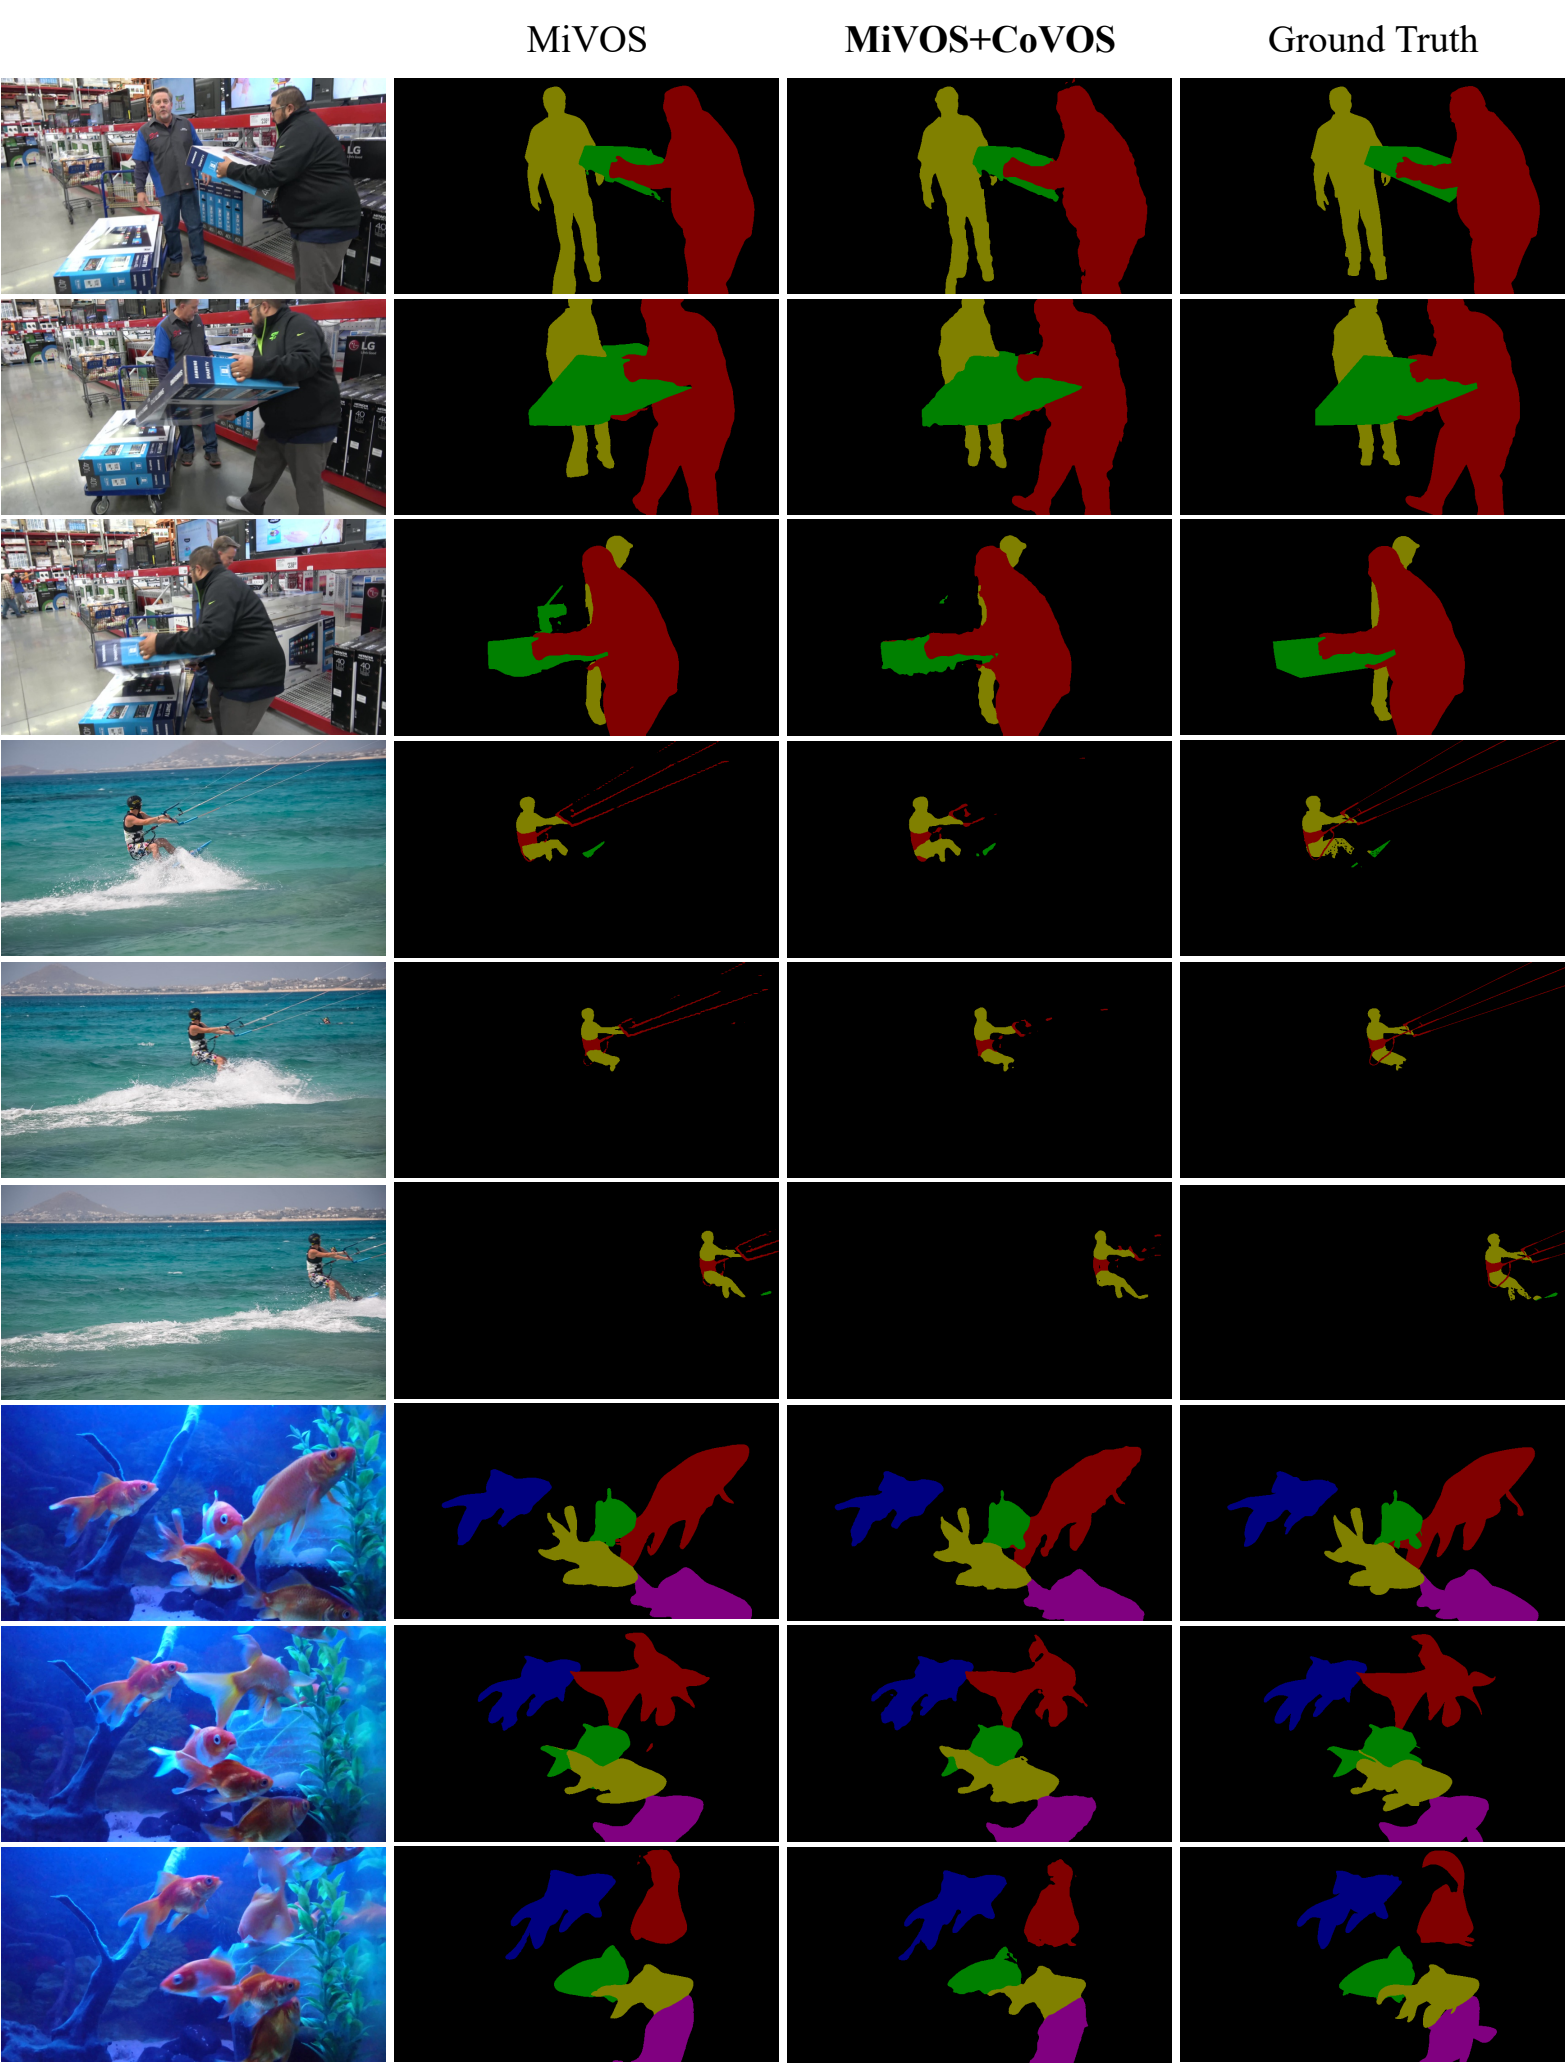  |
| 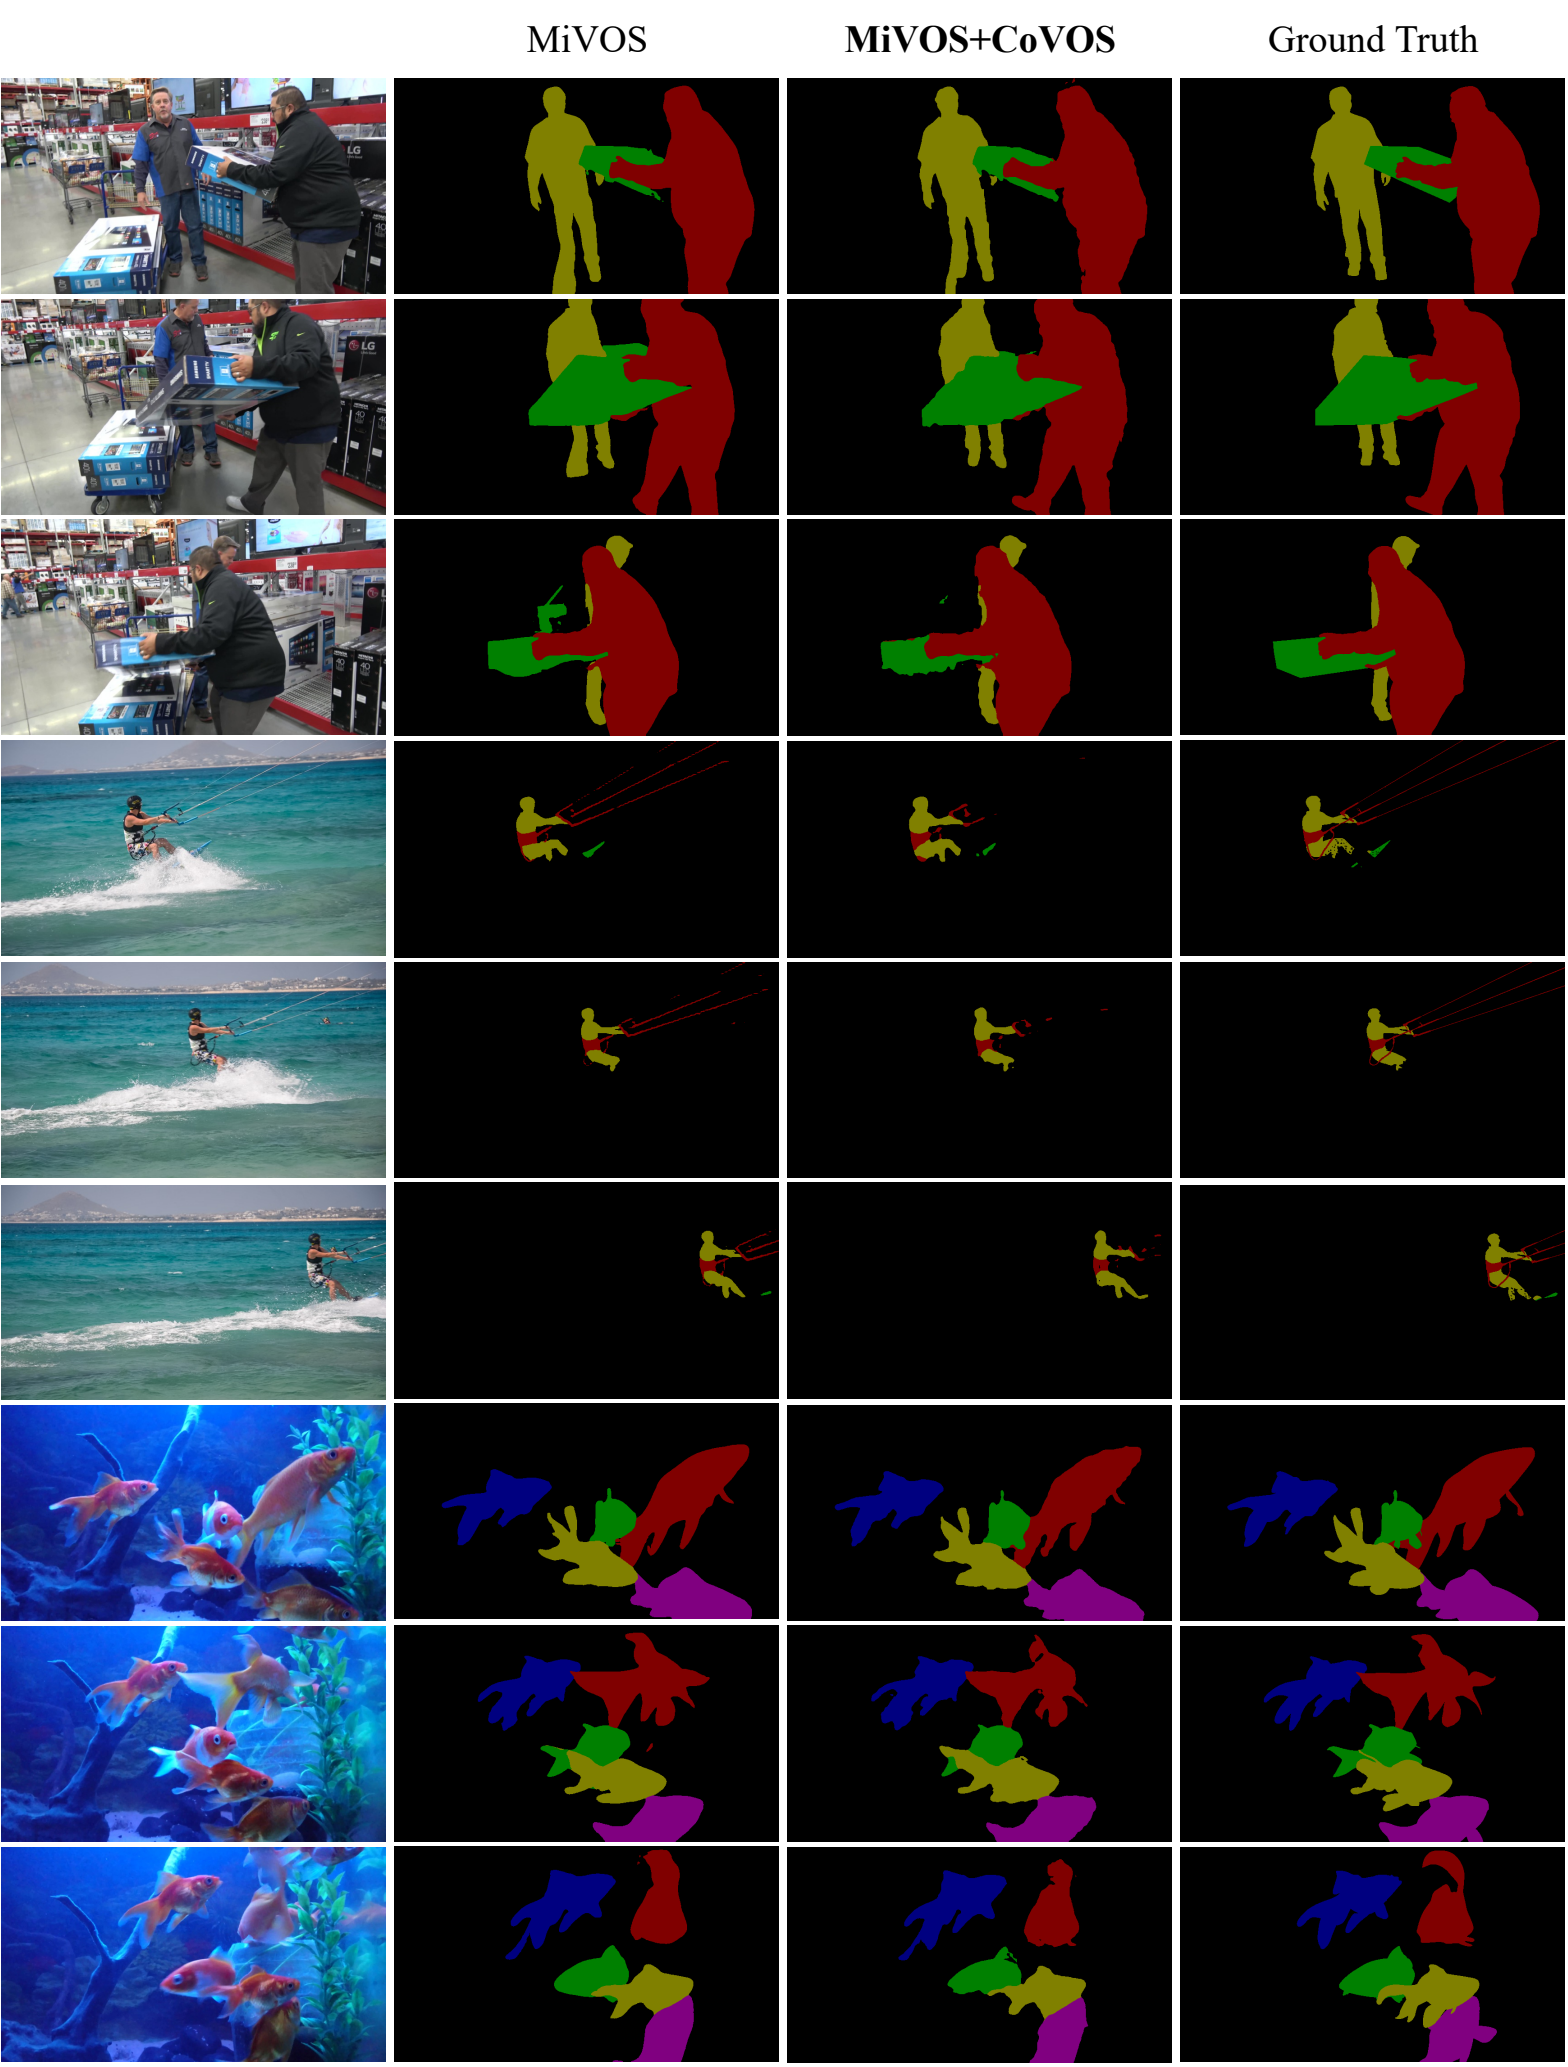 | 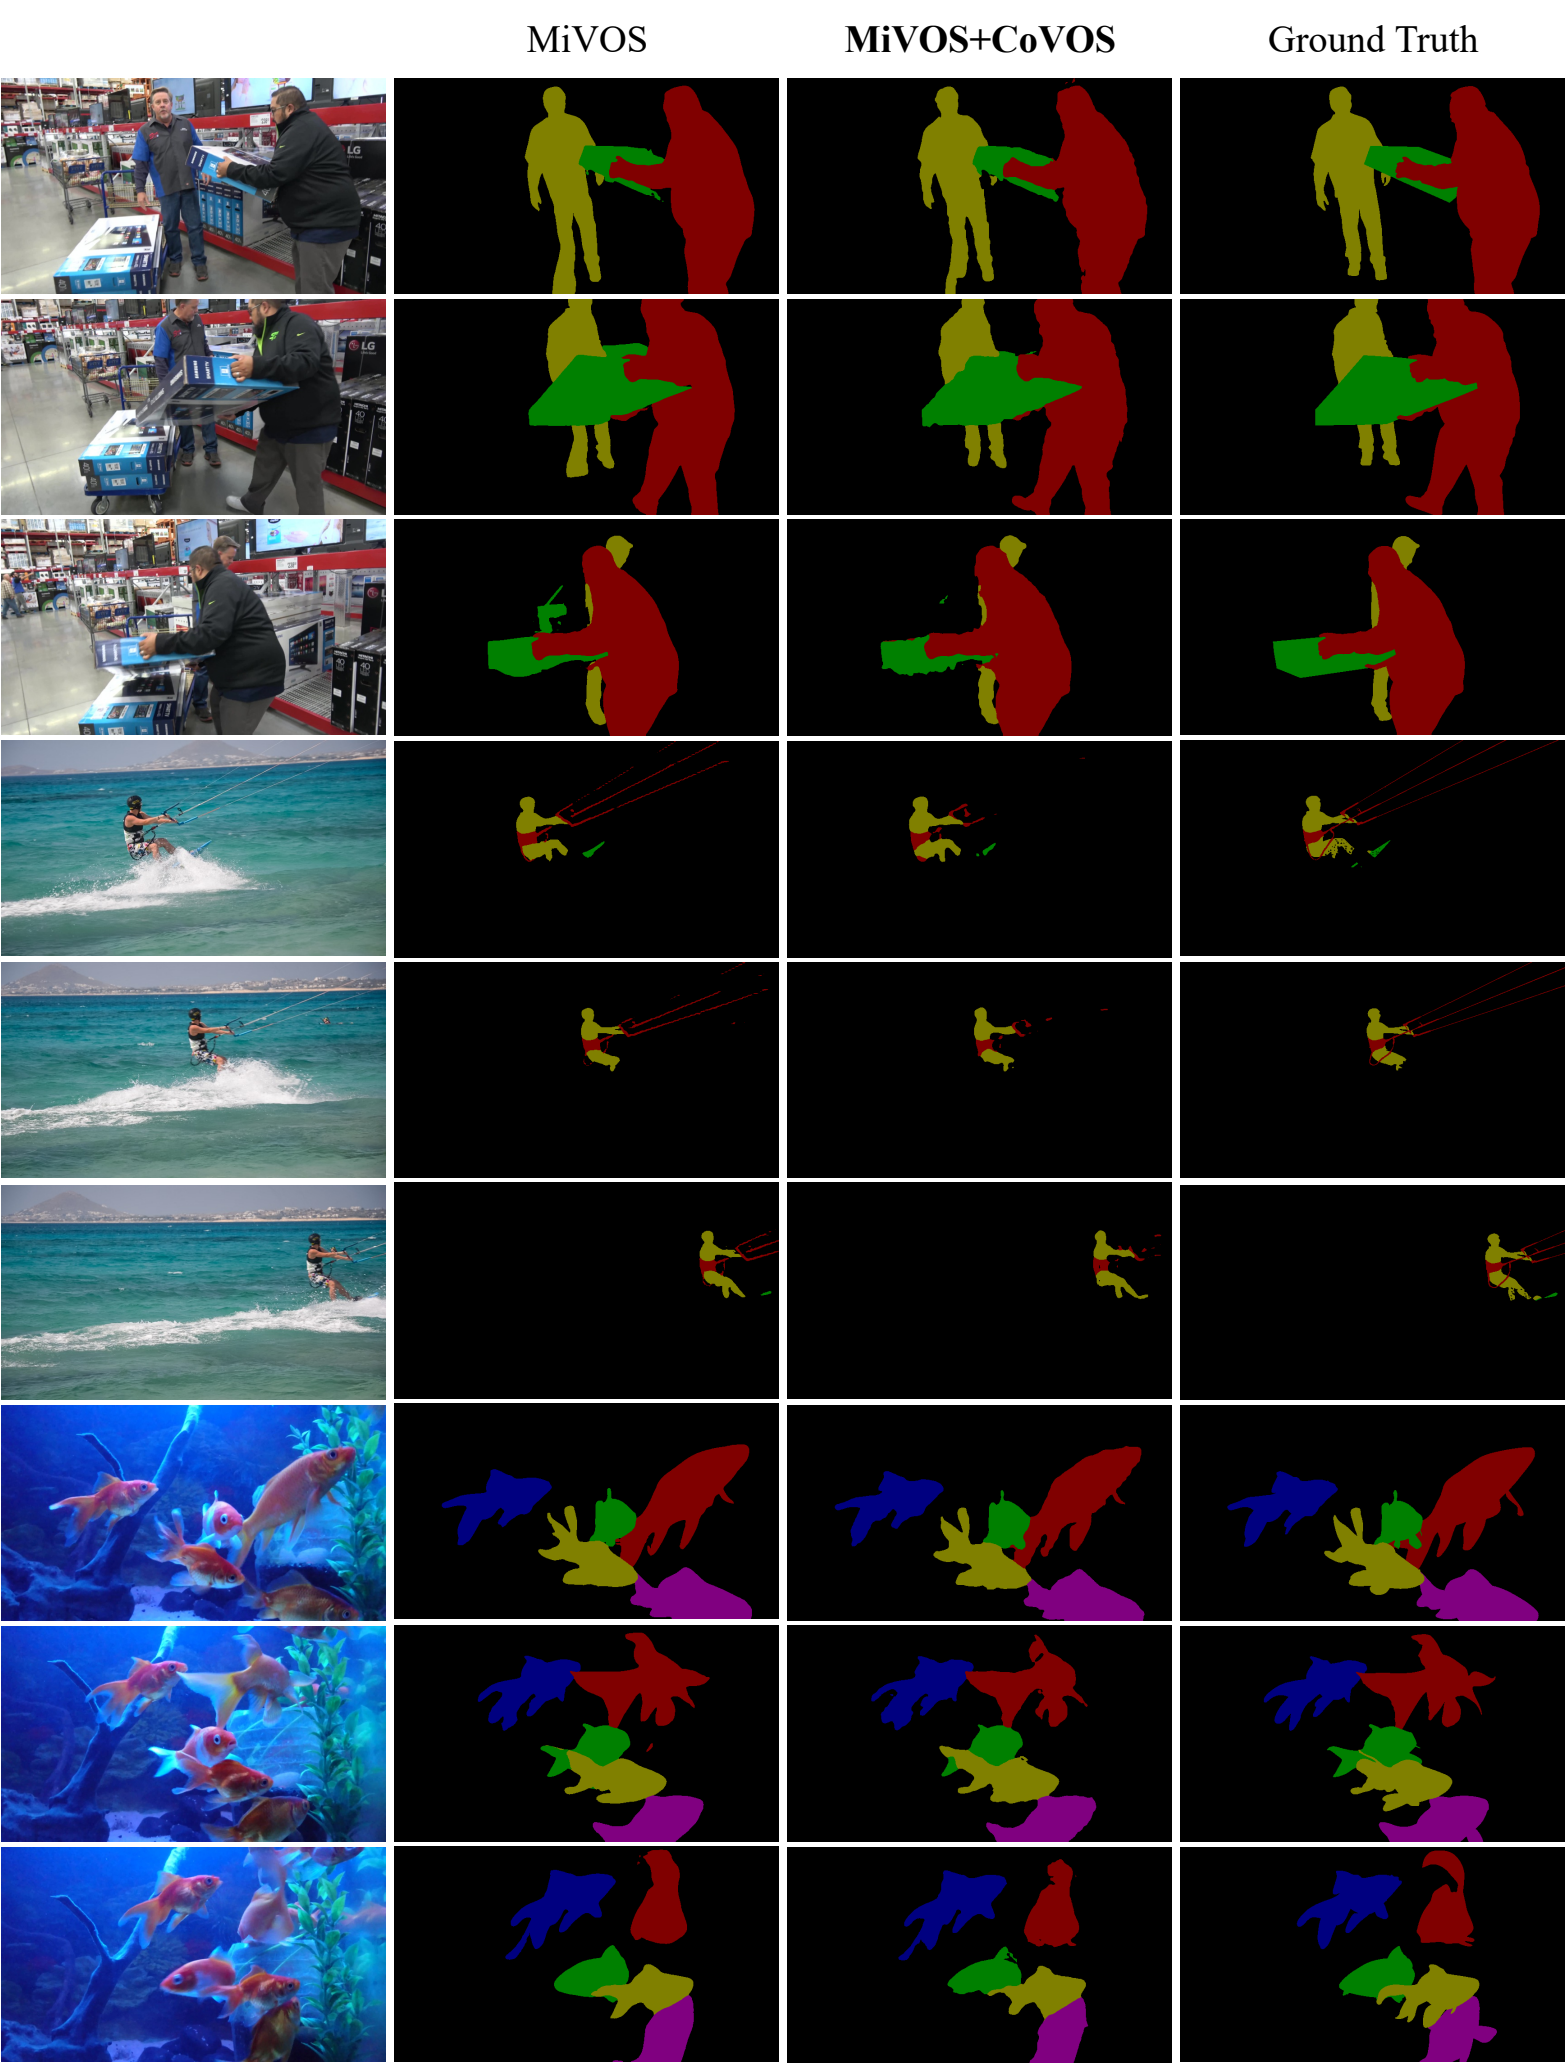 | 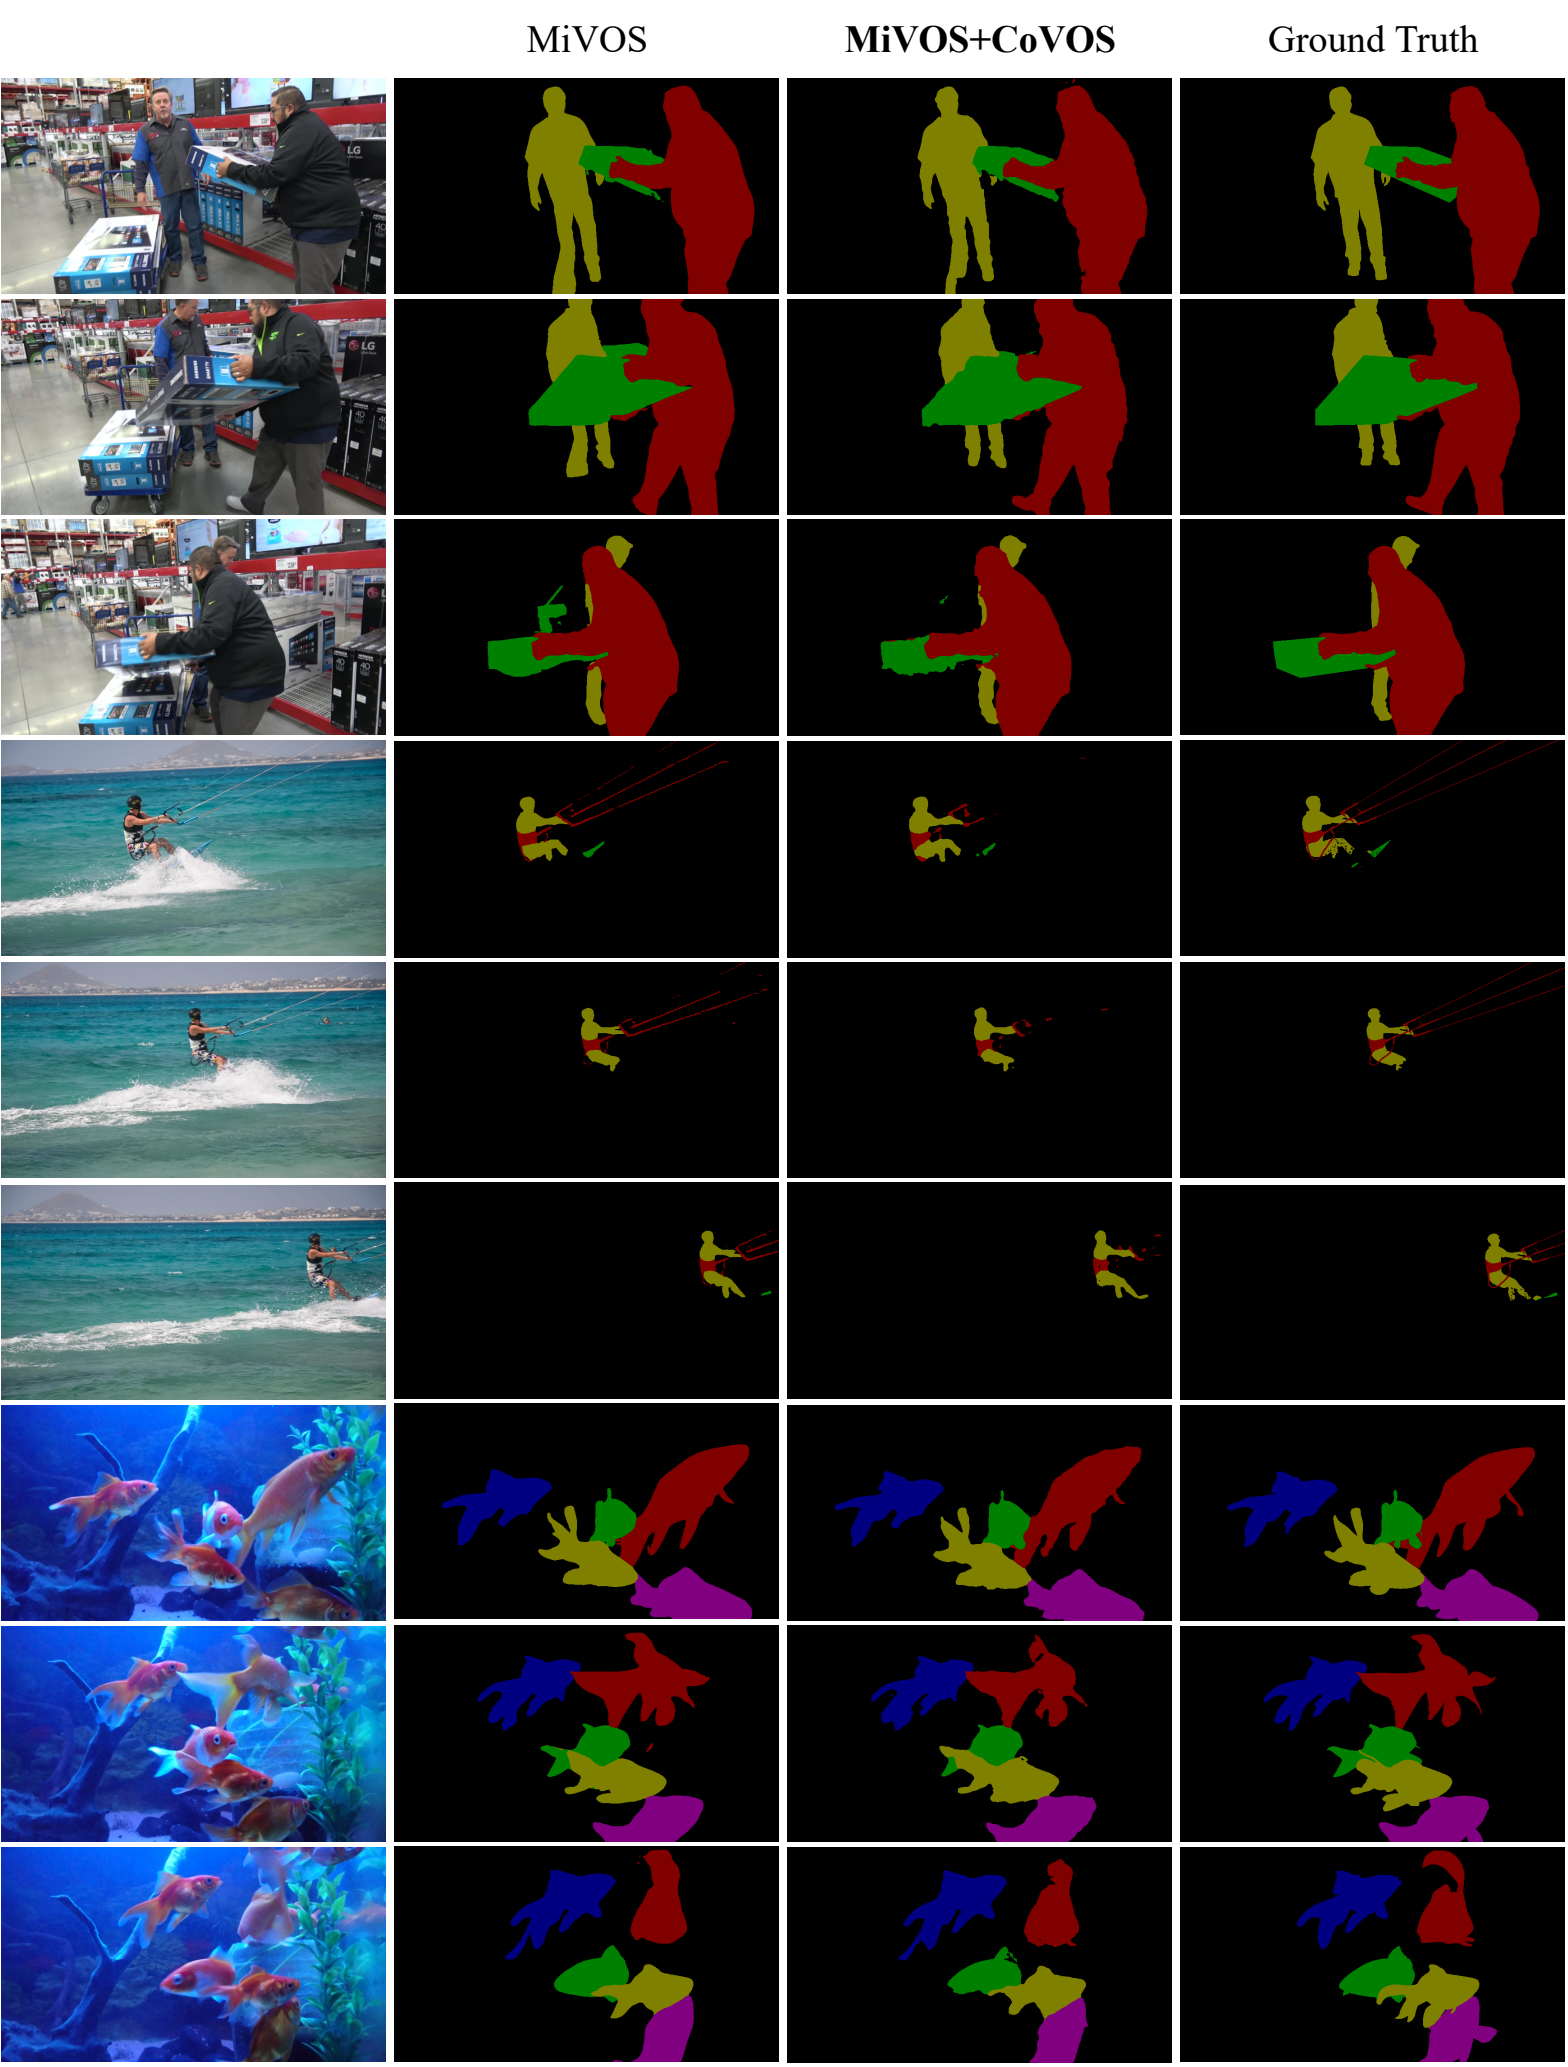 | 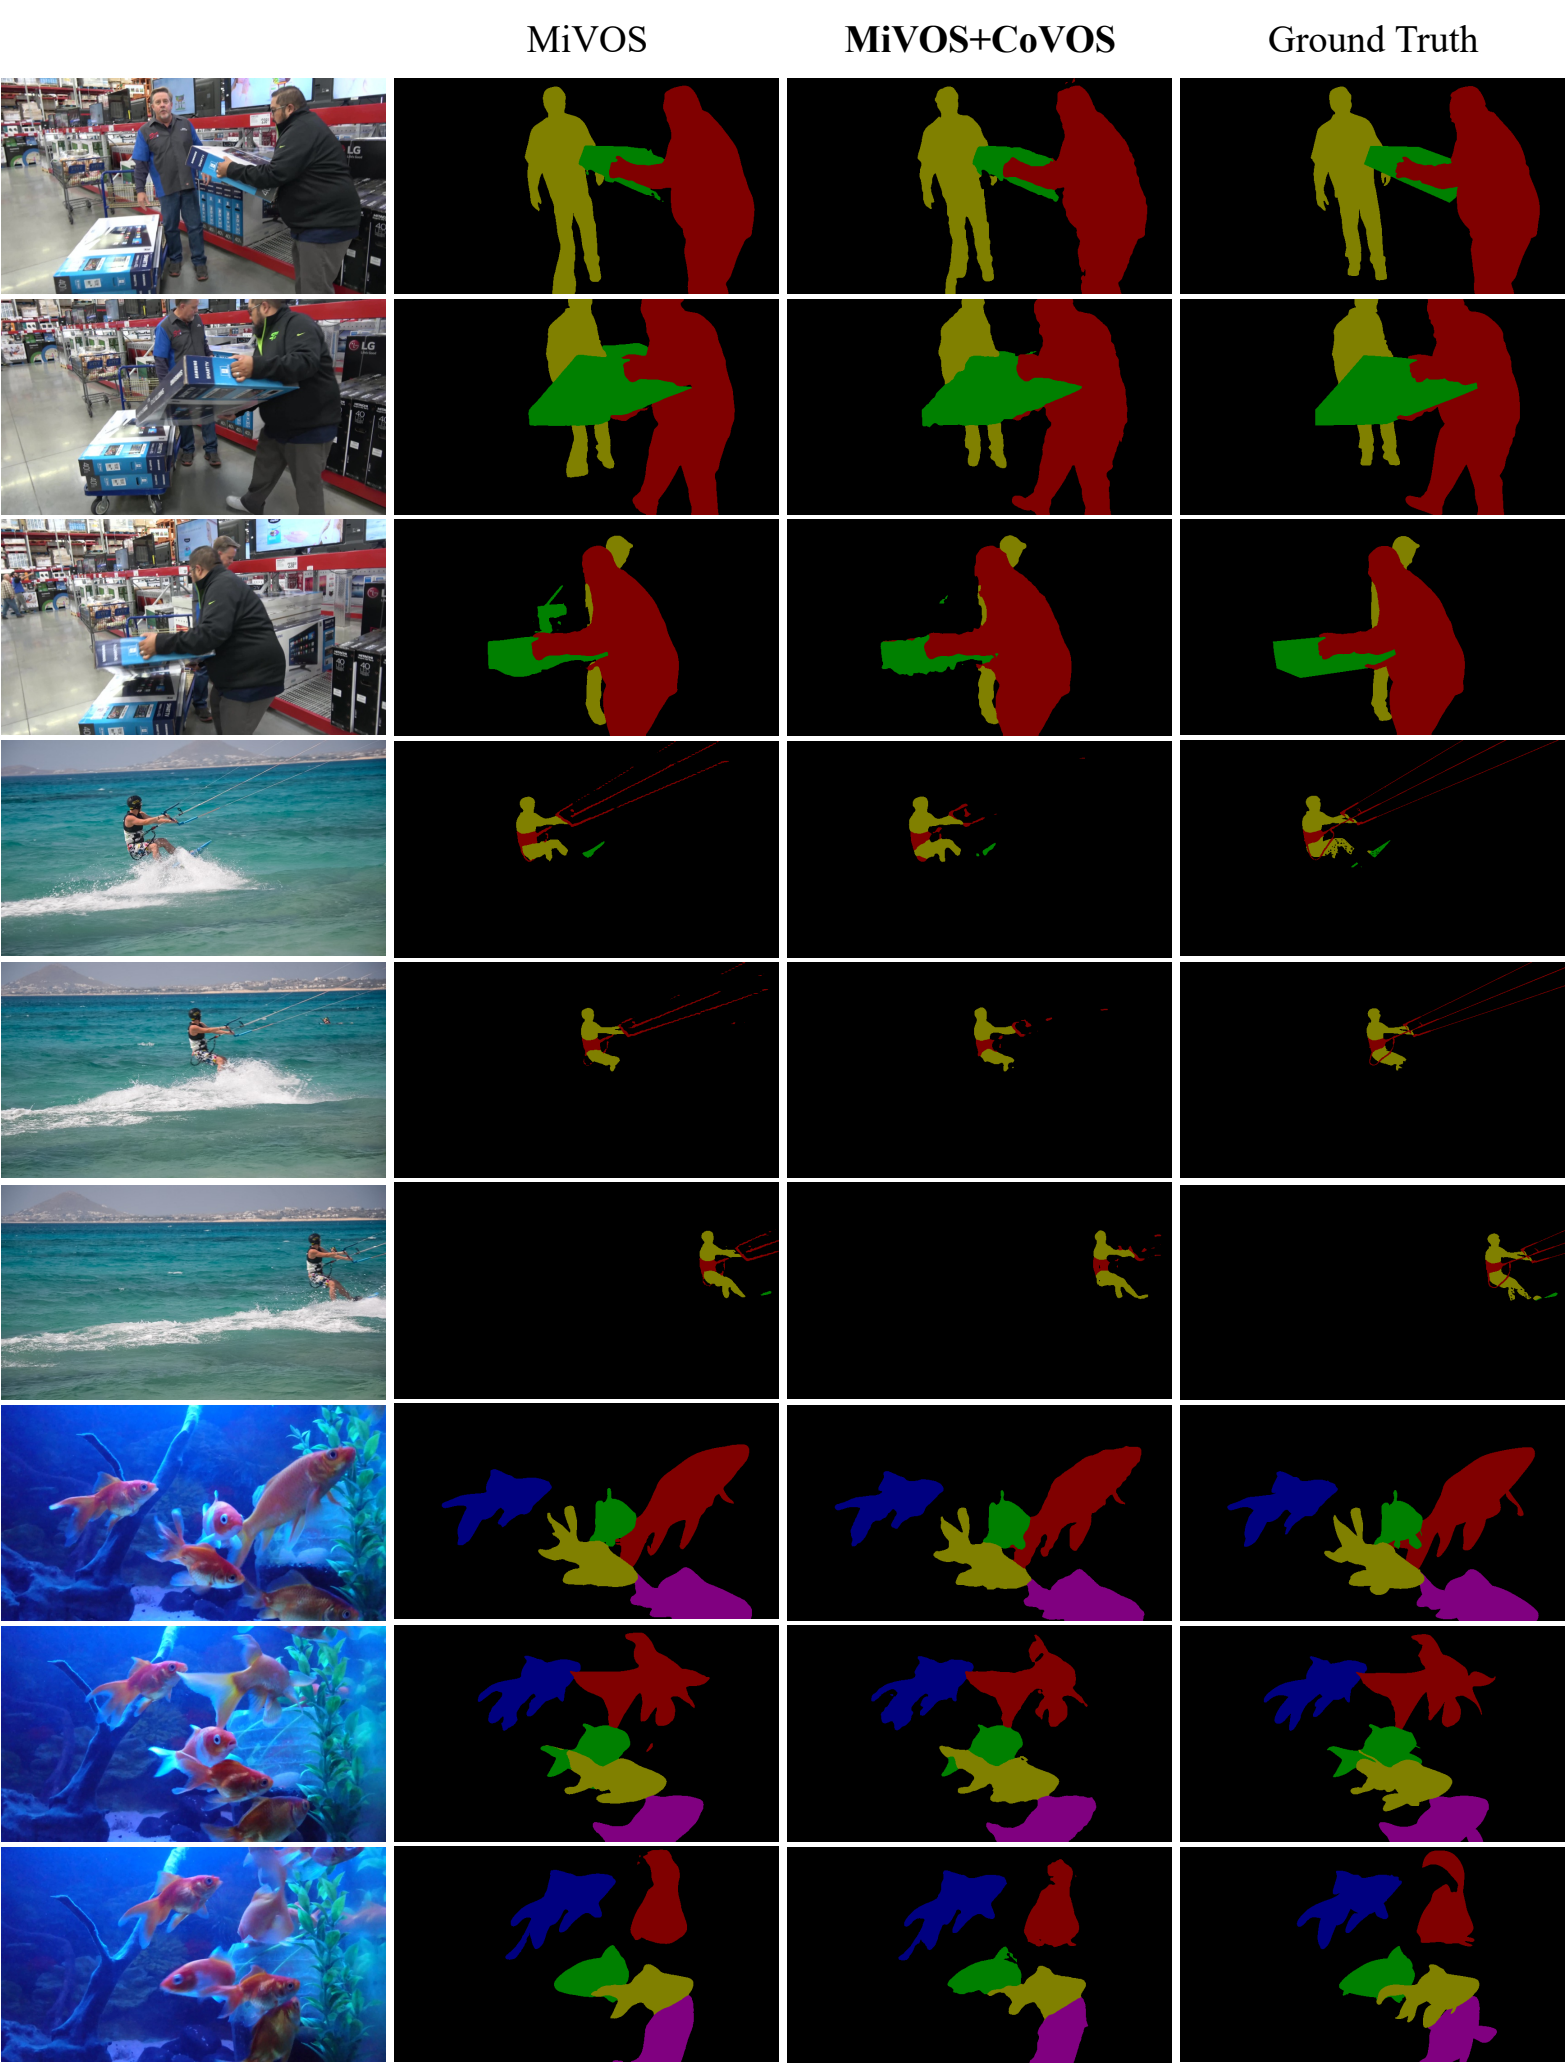 |
| 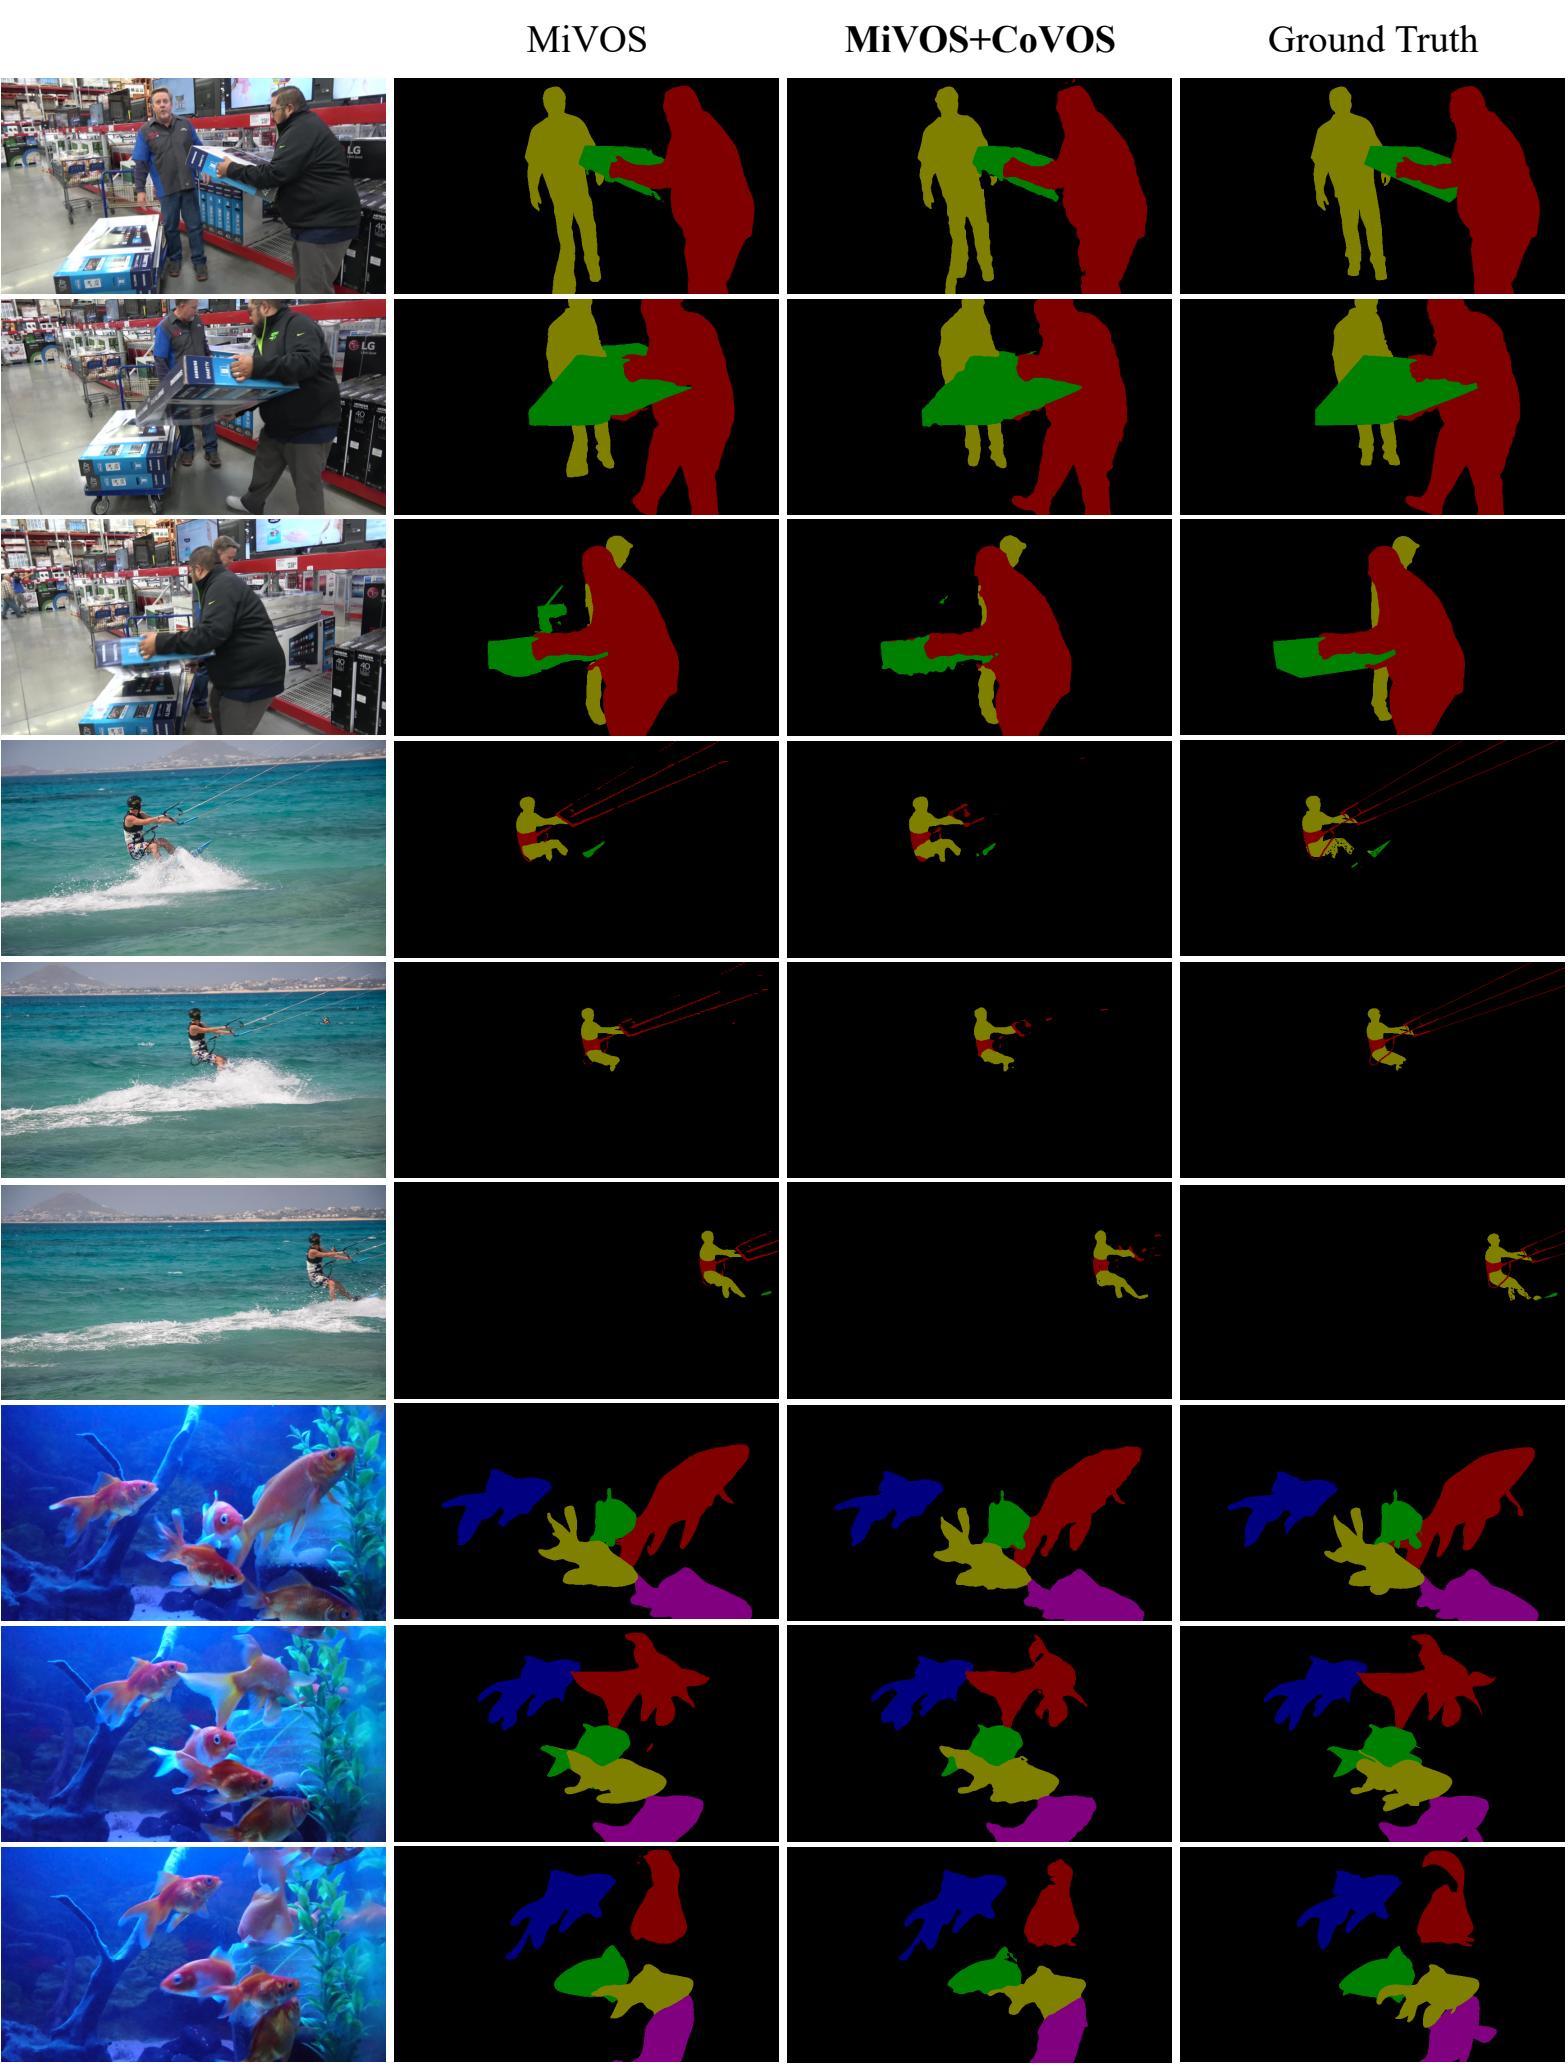 | 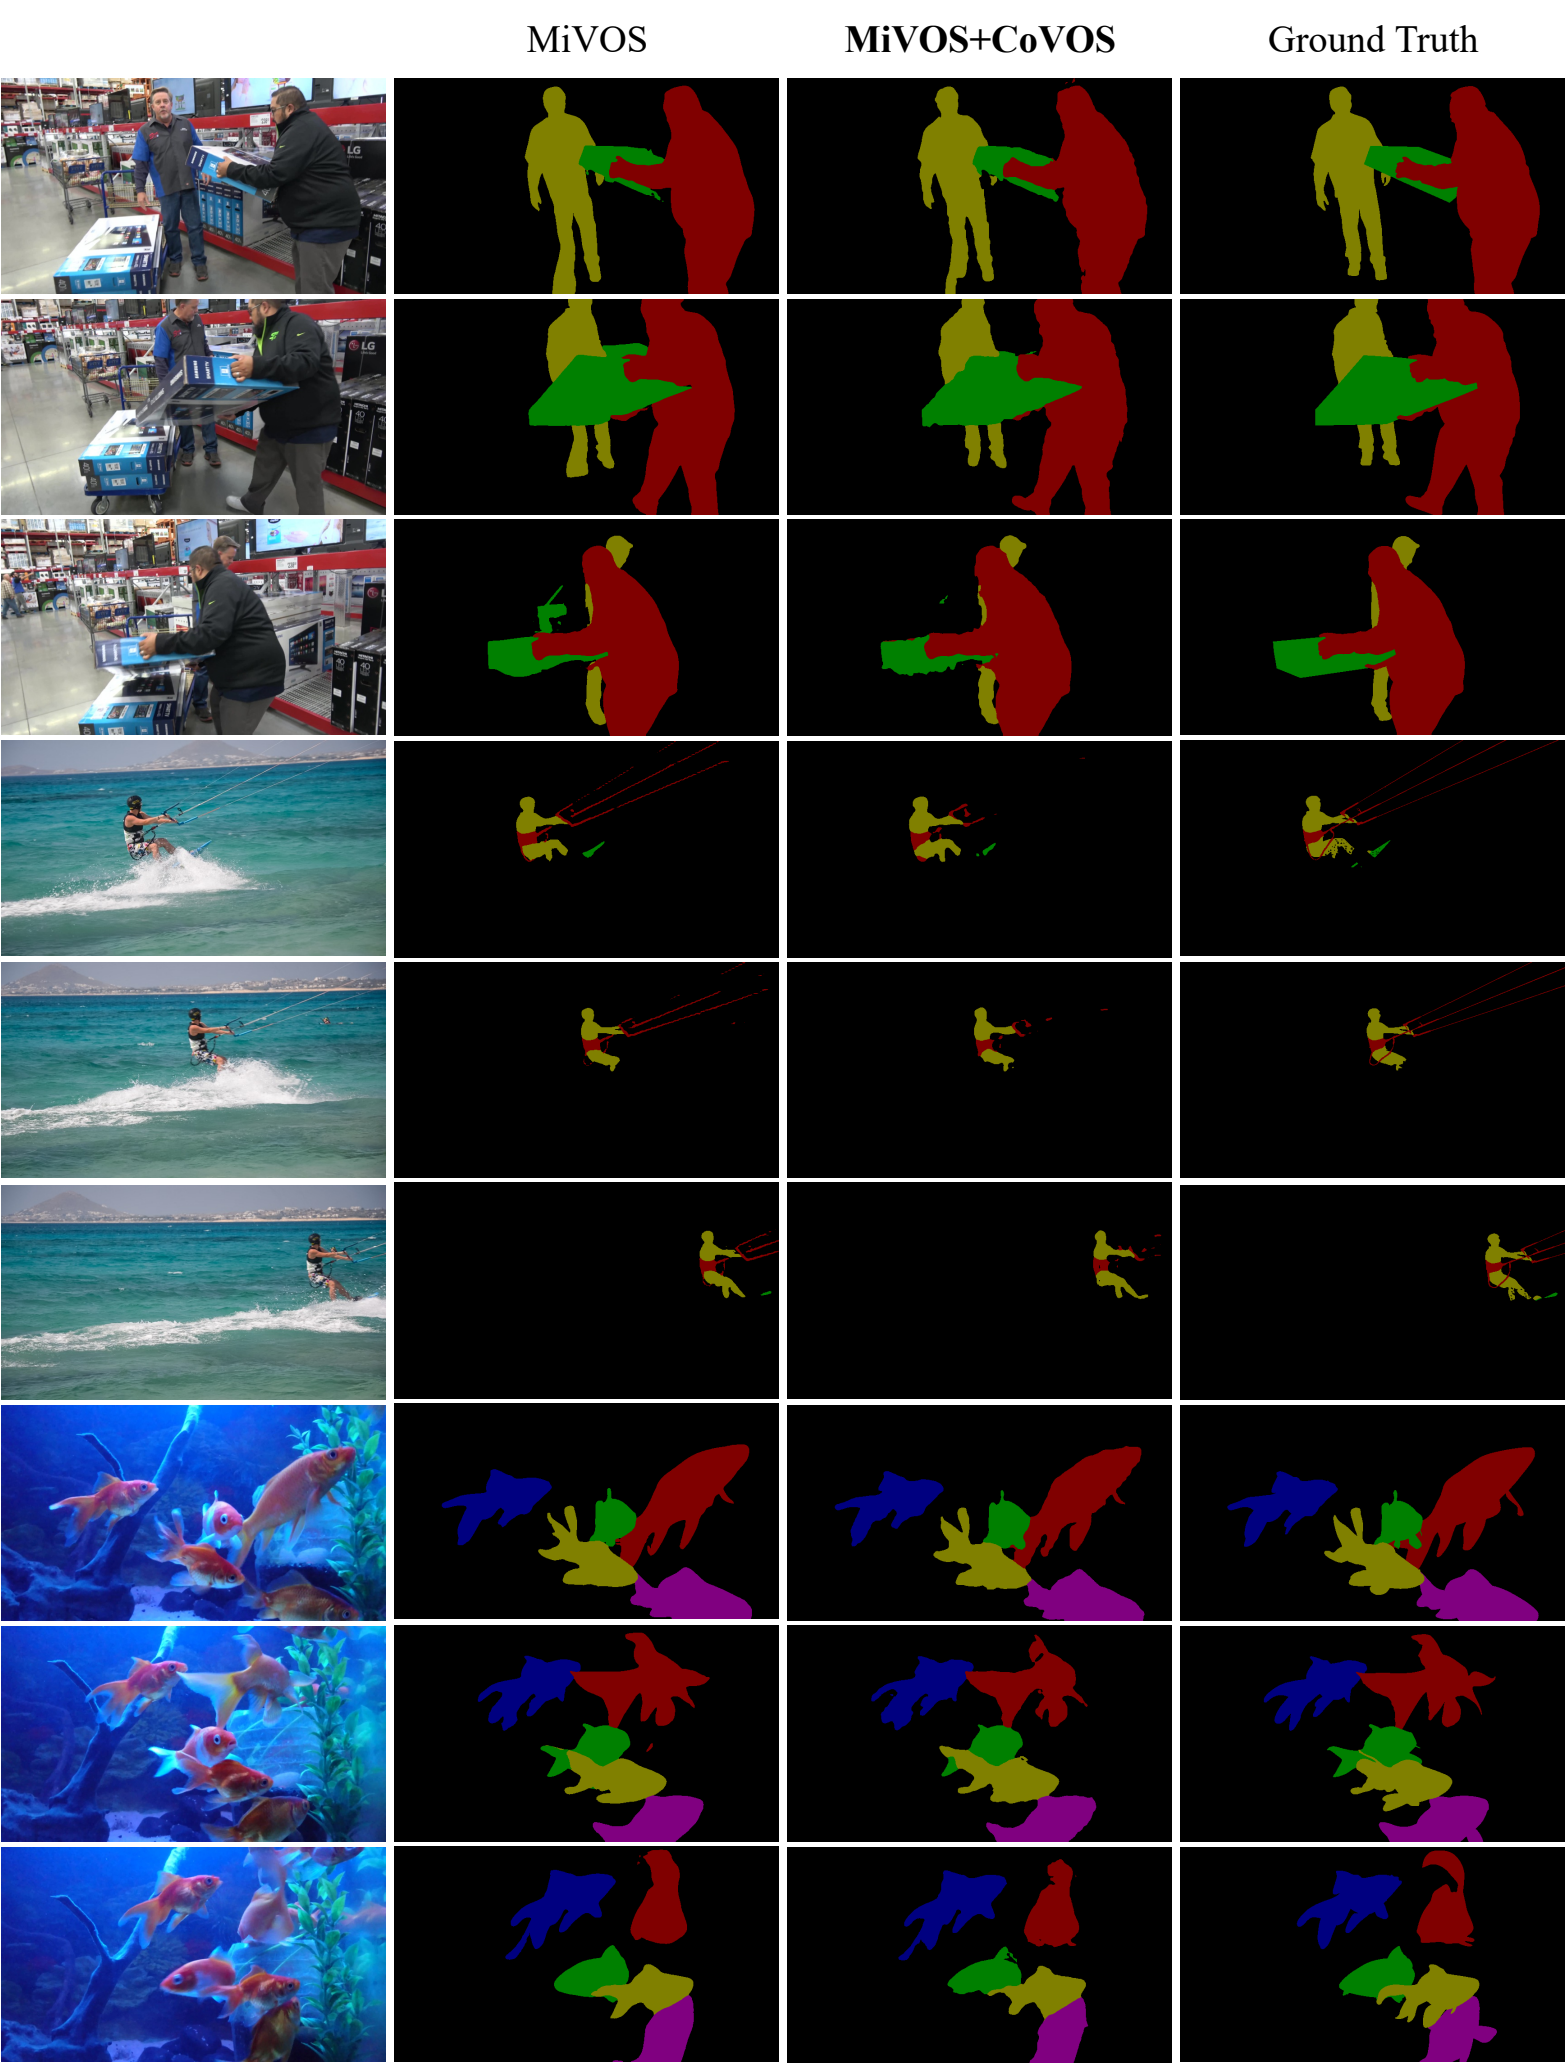 | 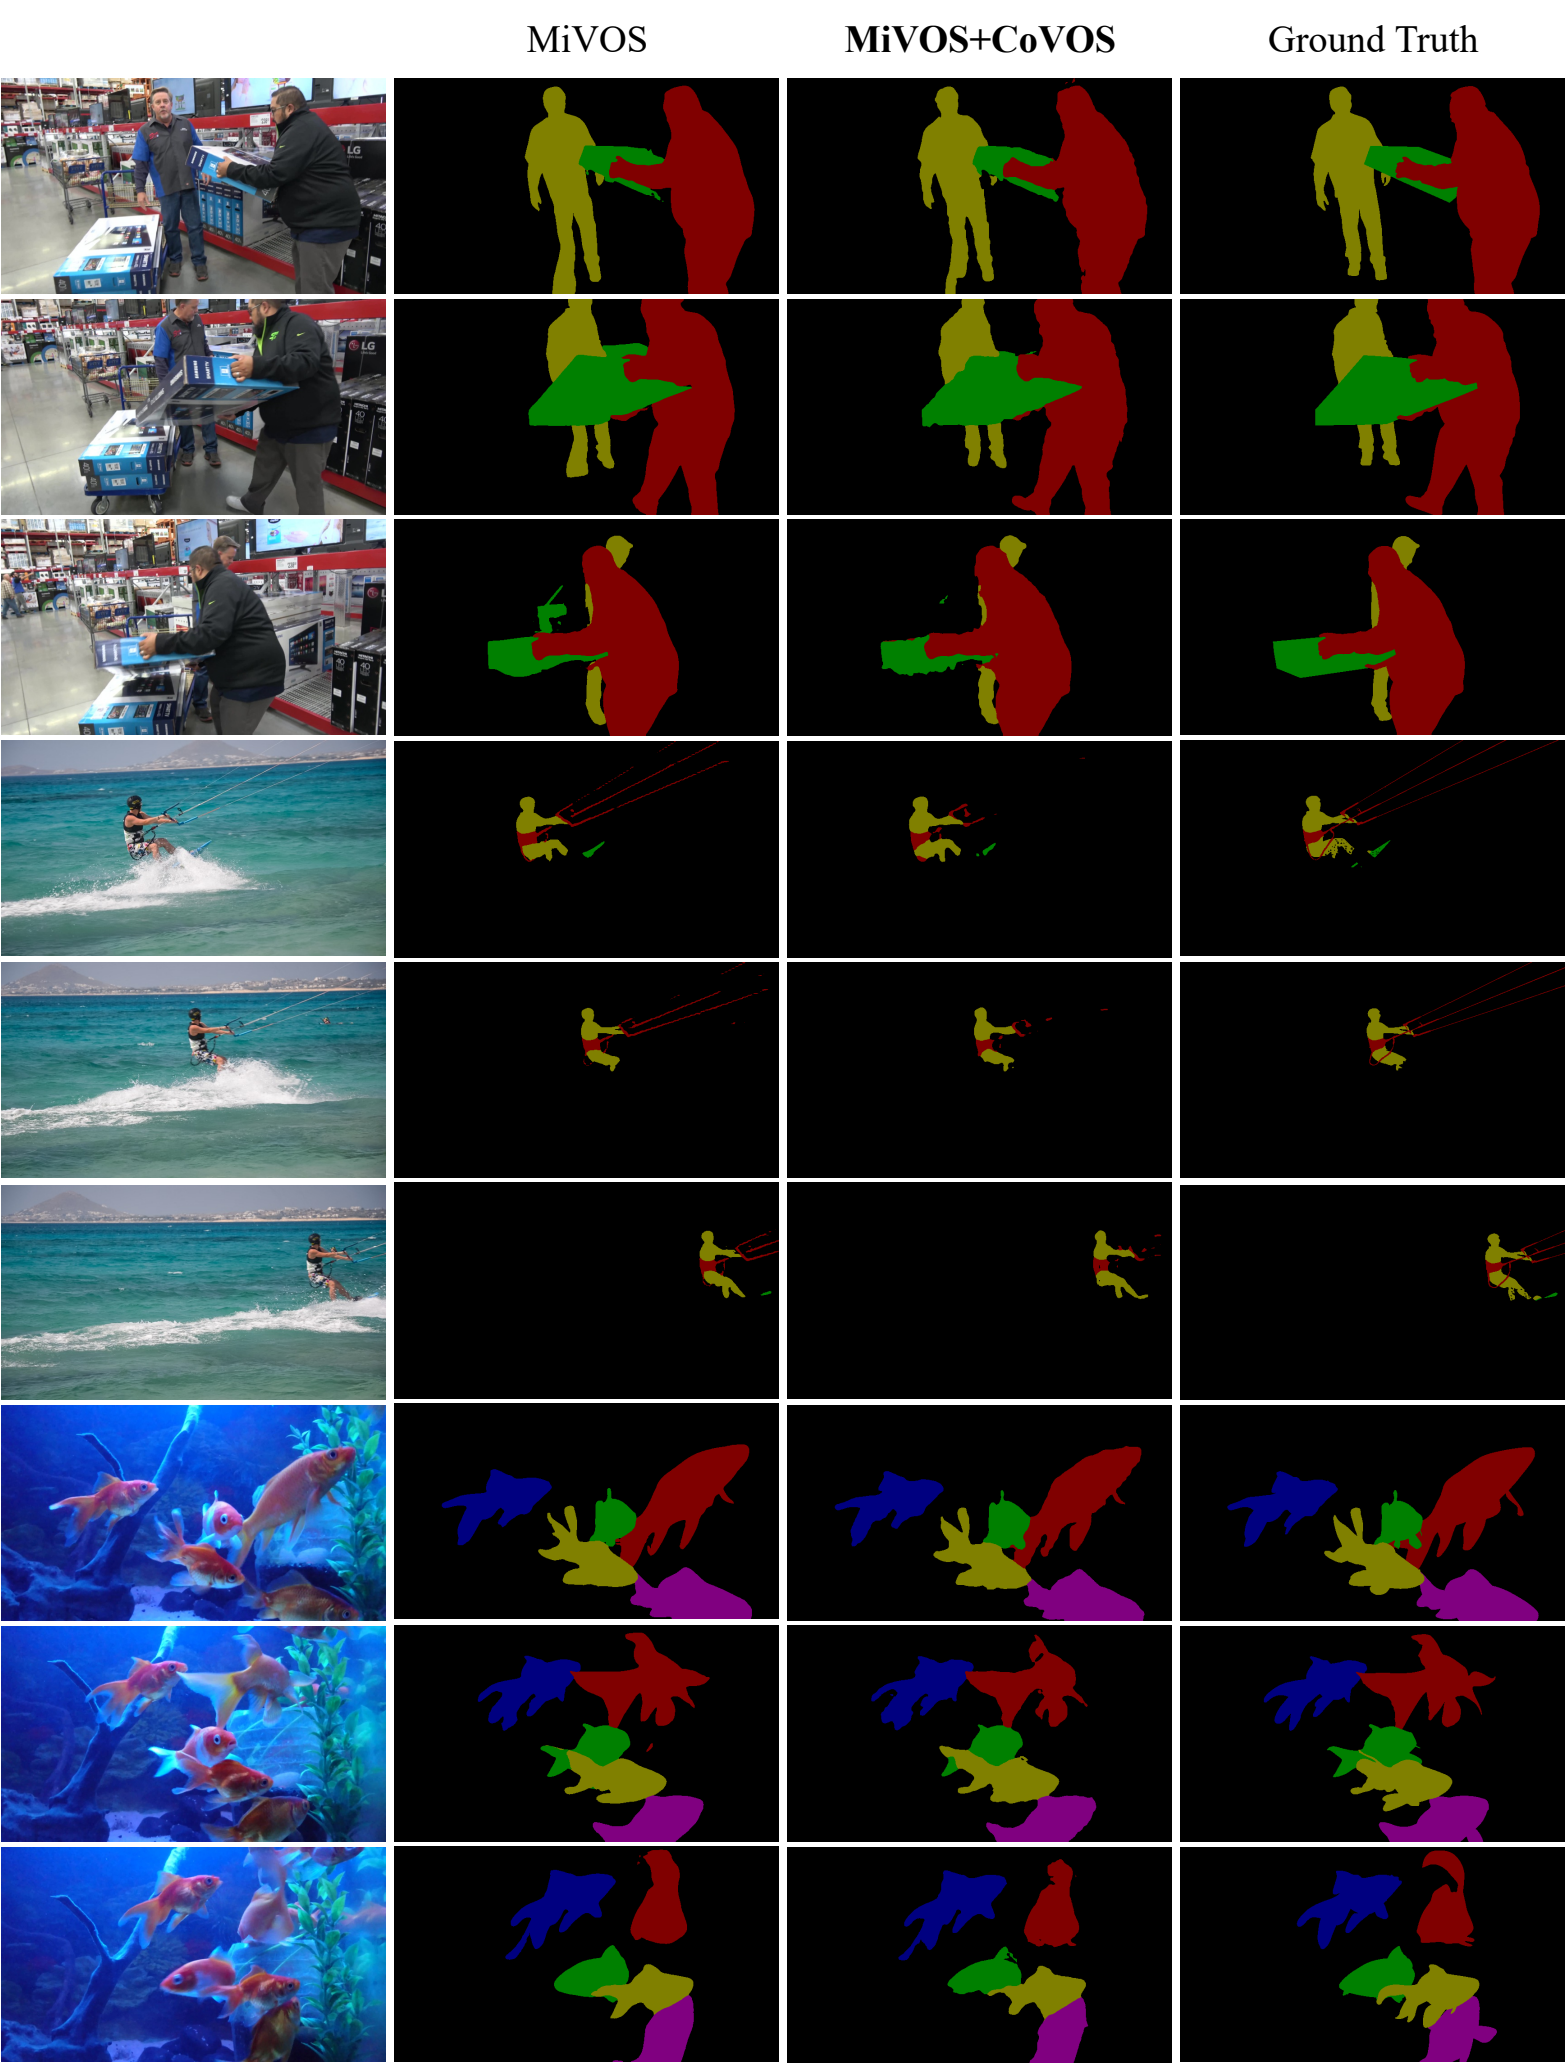 | 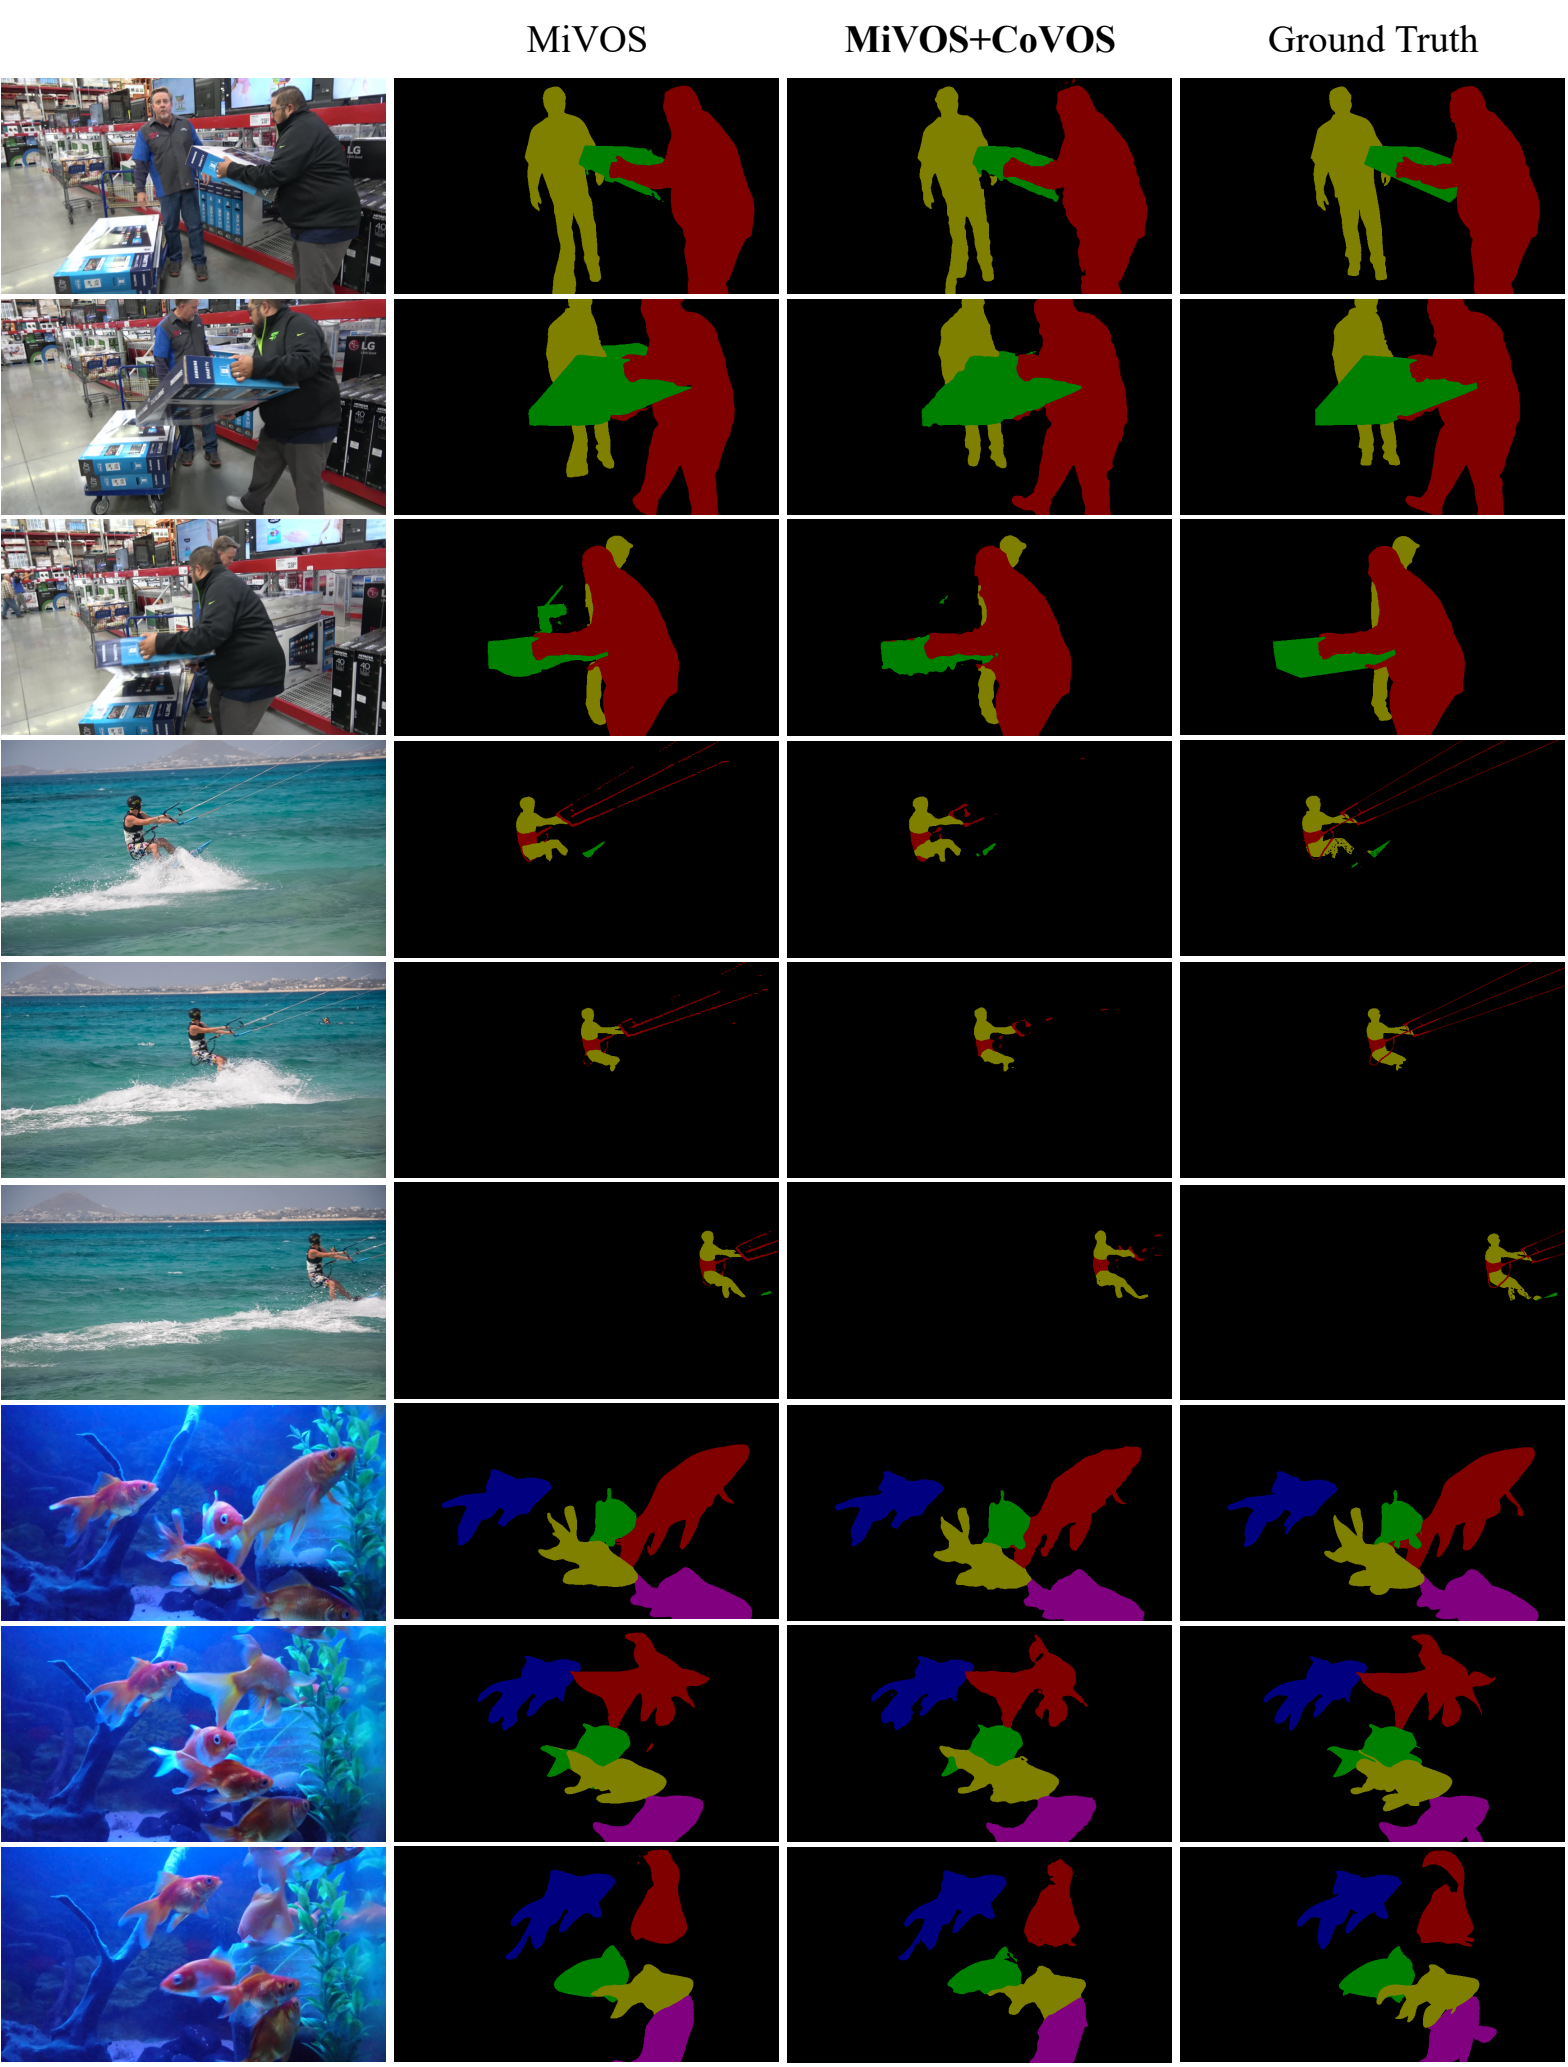 |
| 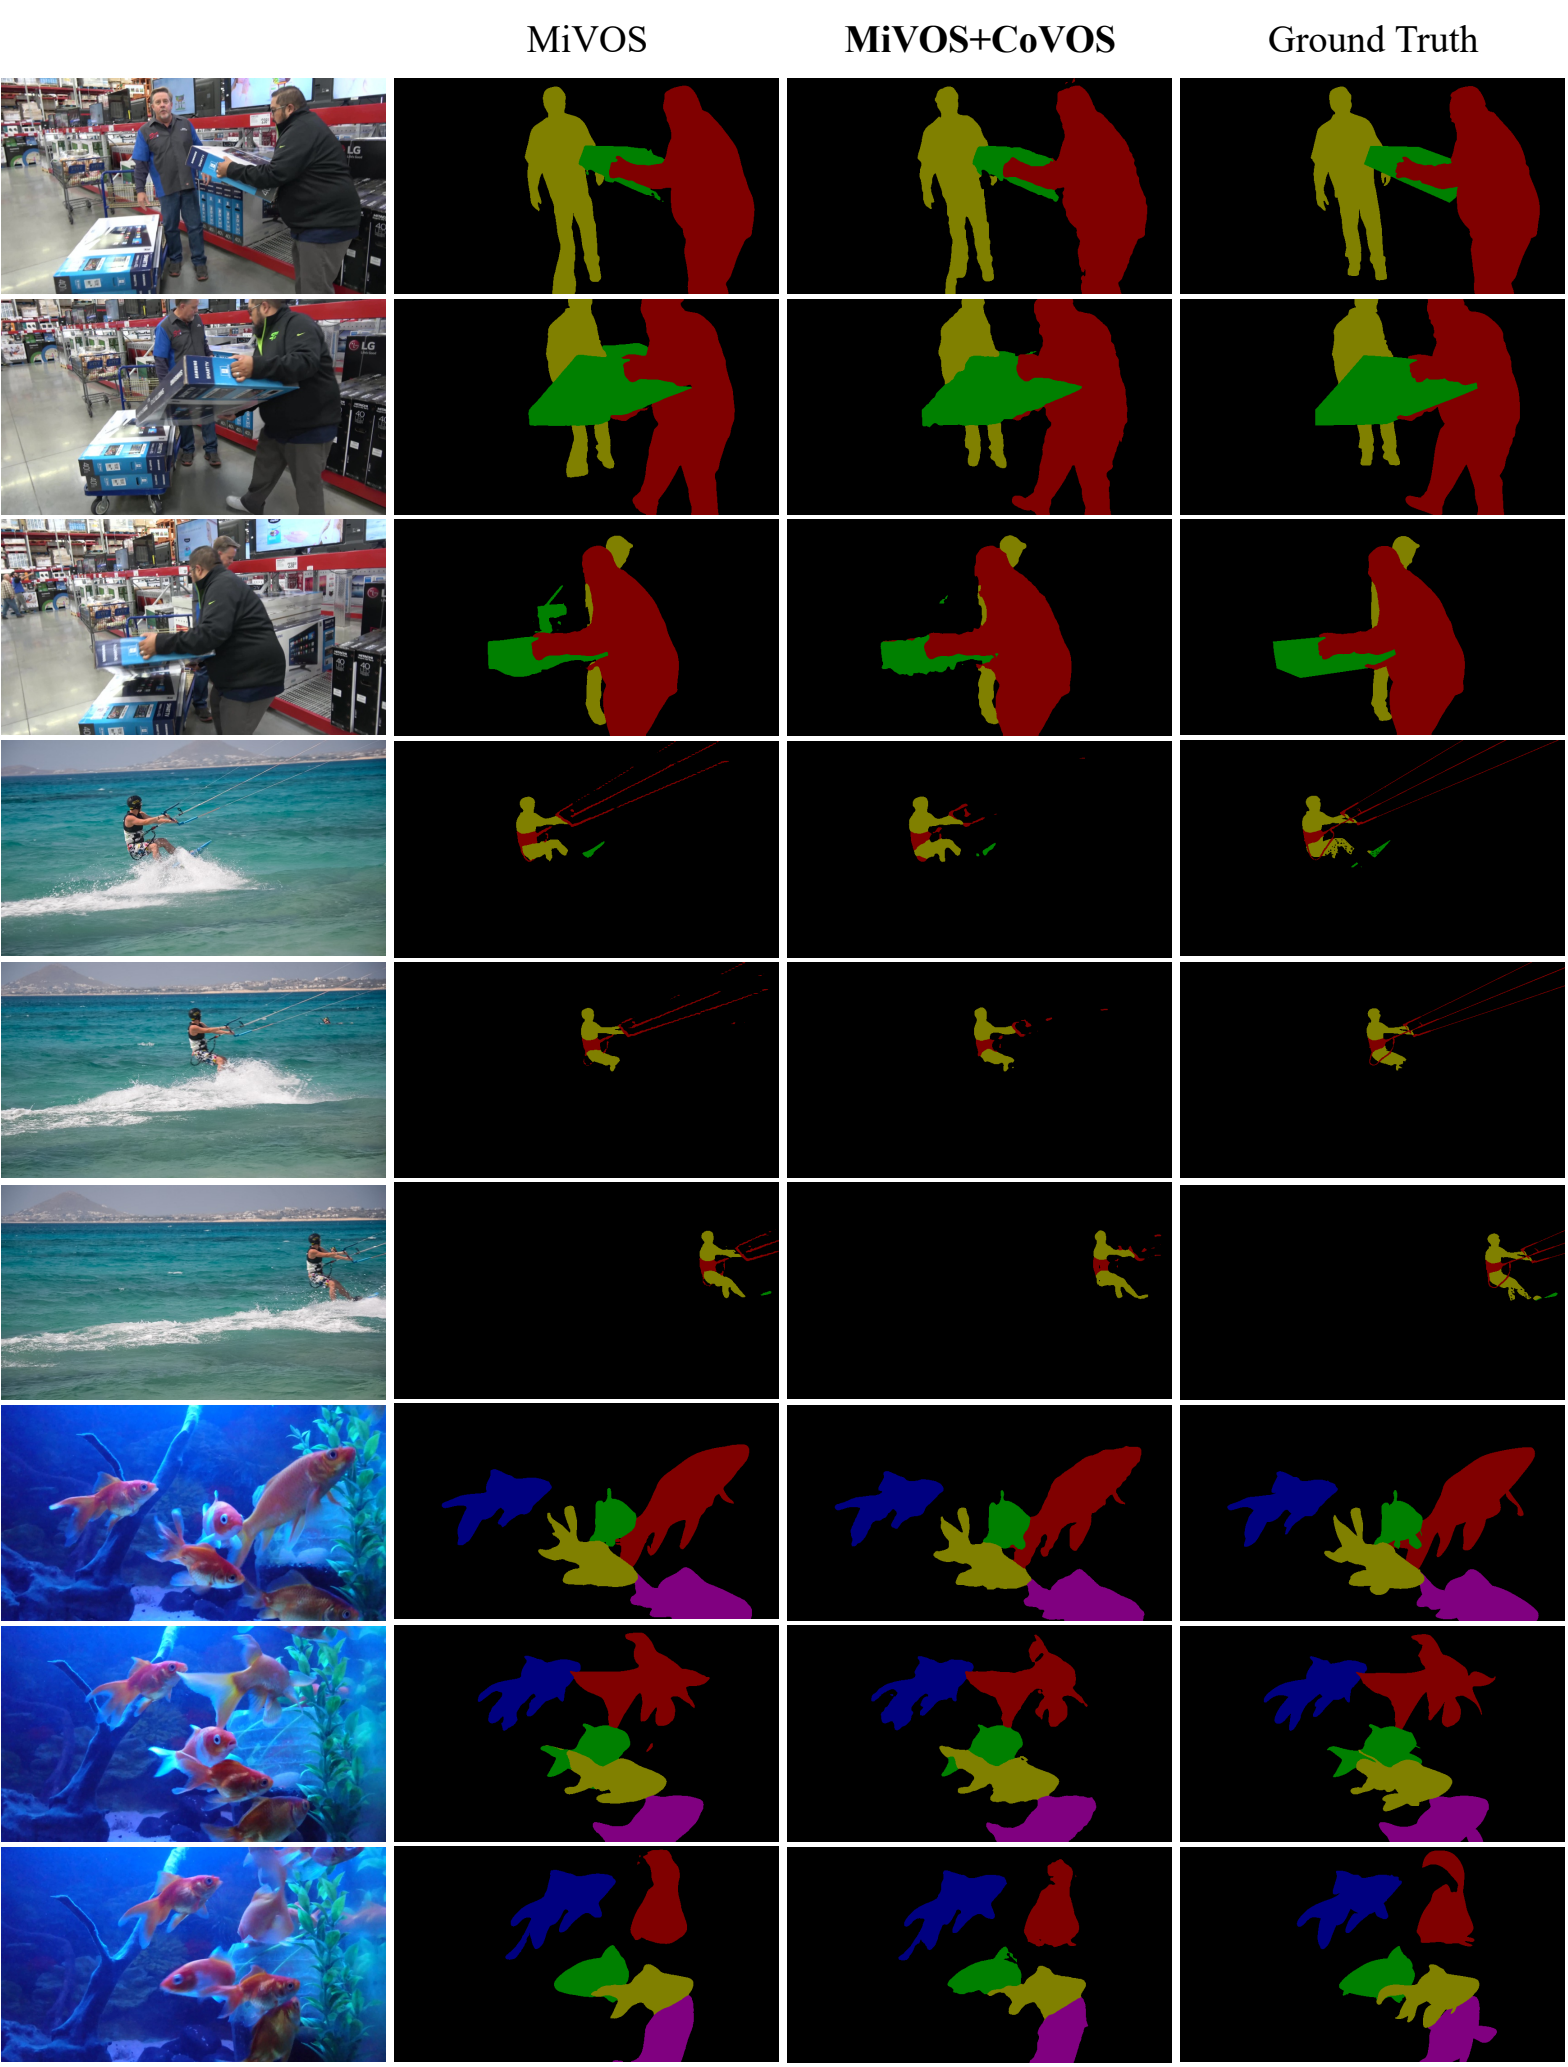 | 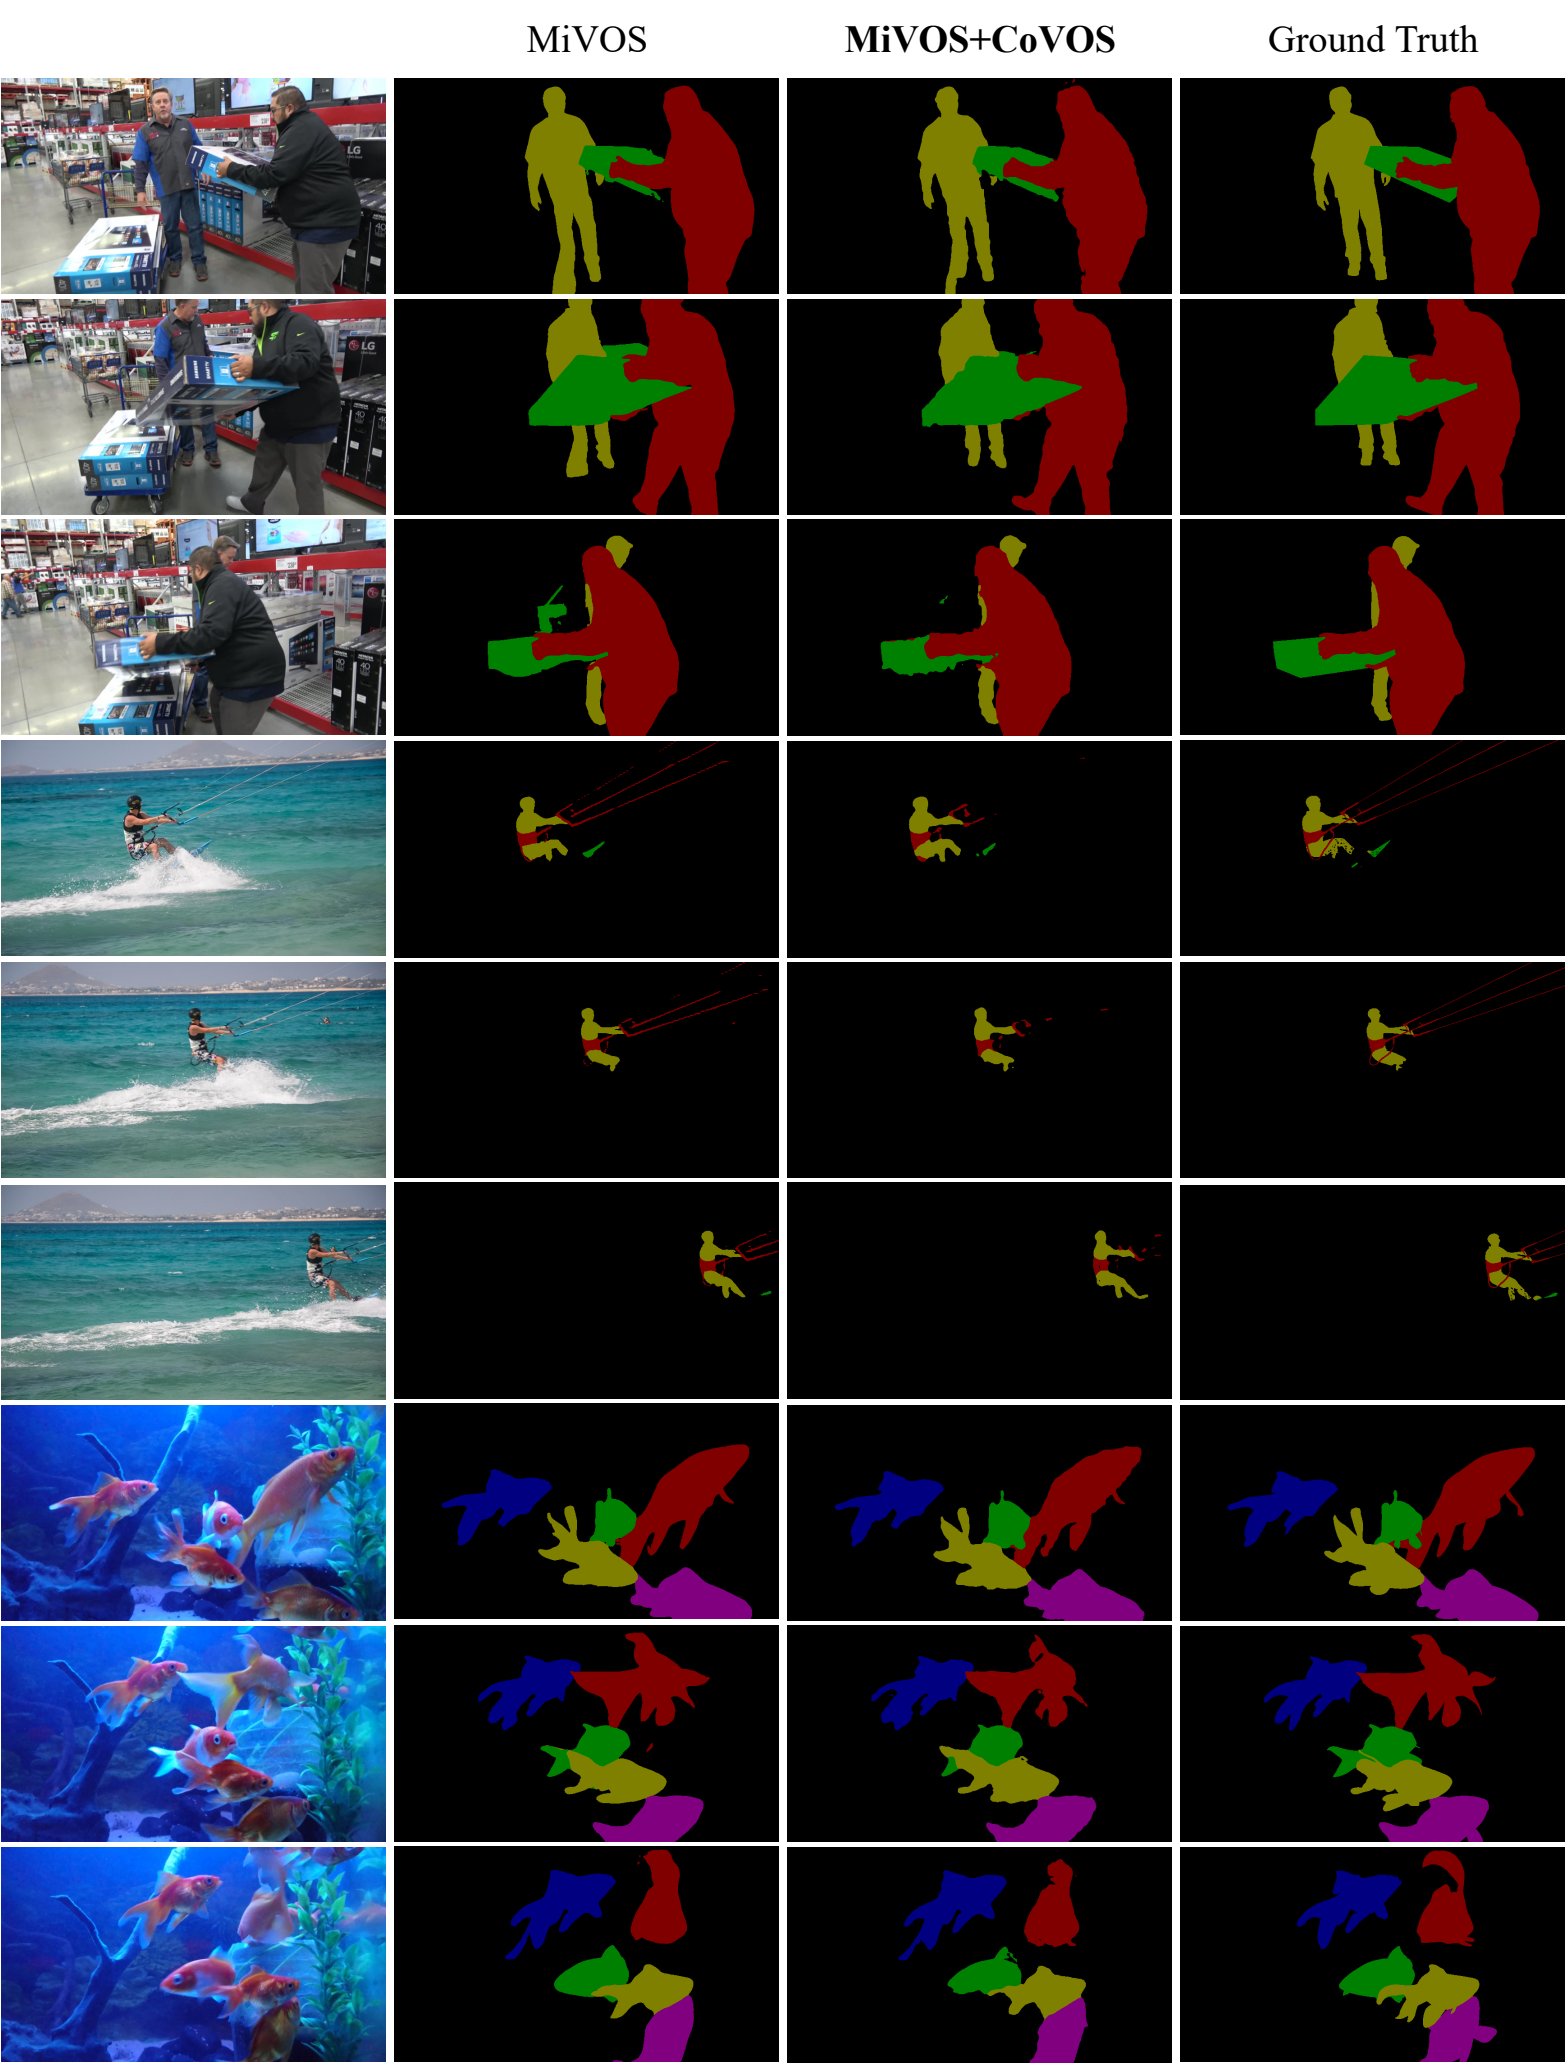 | 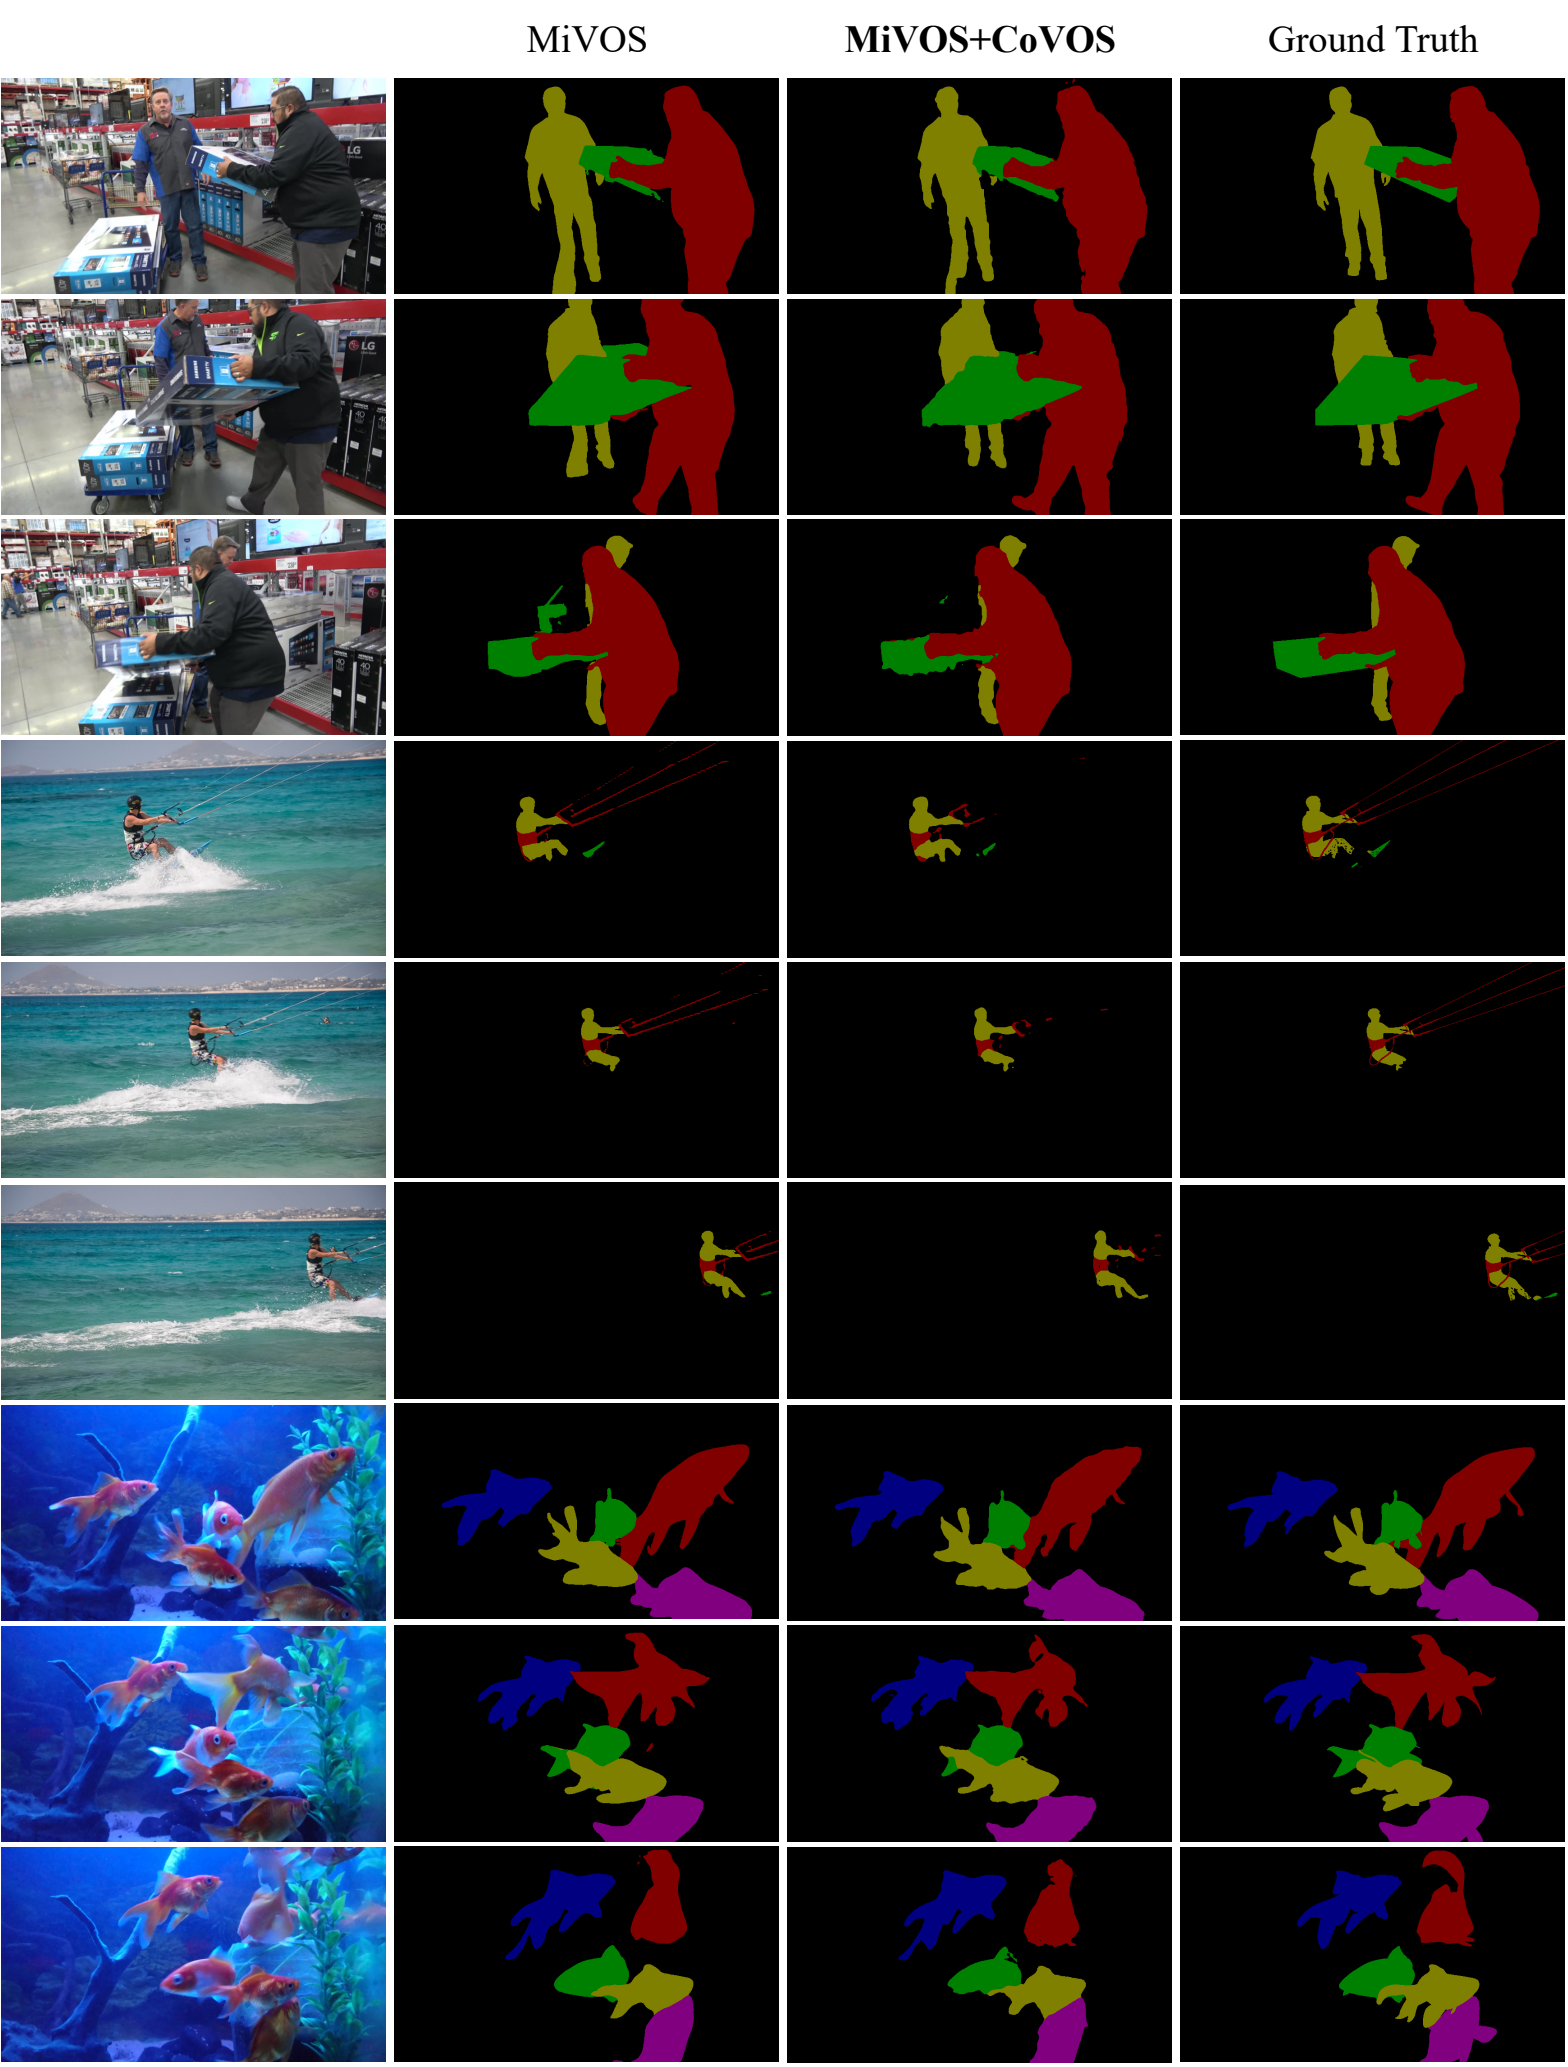 | 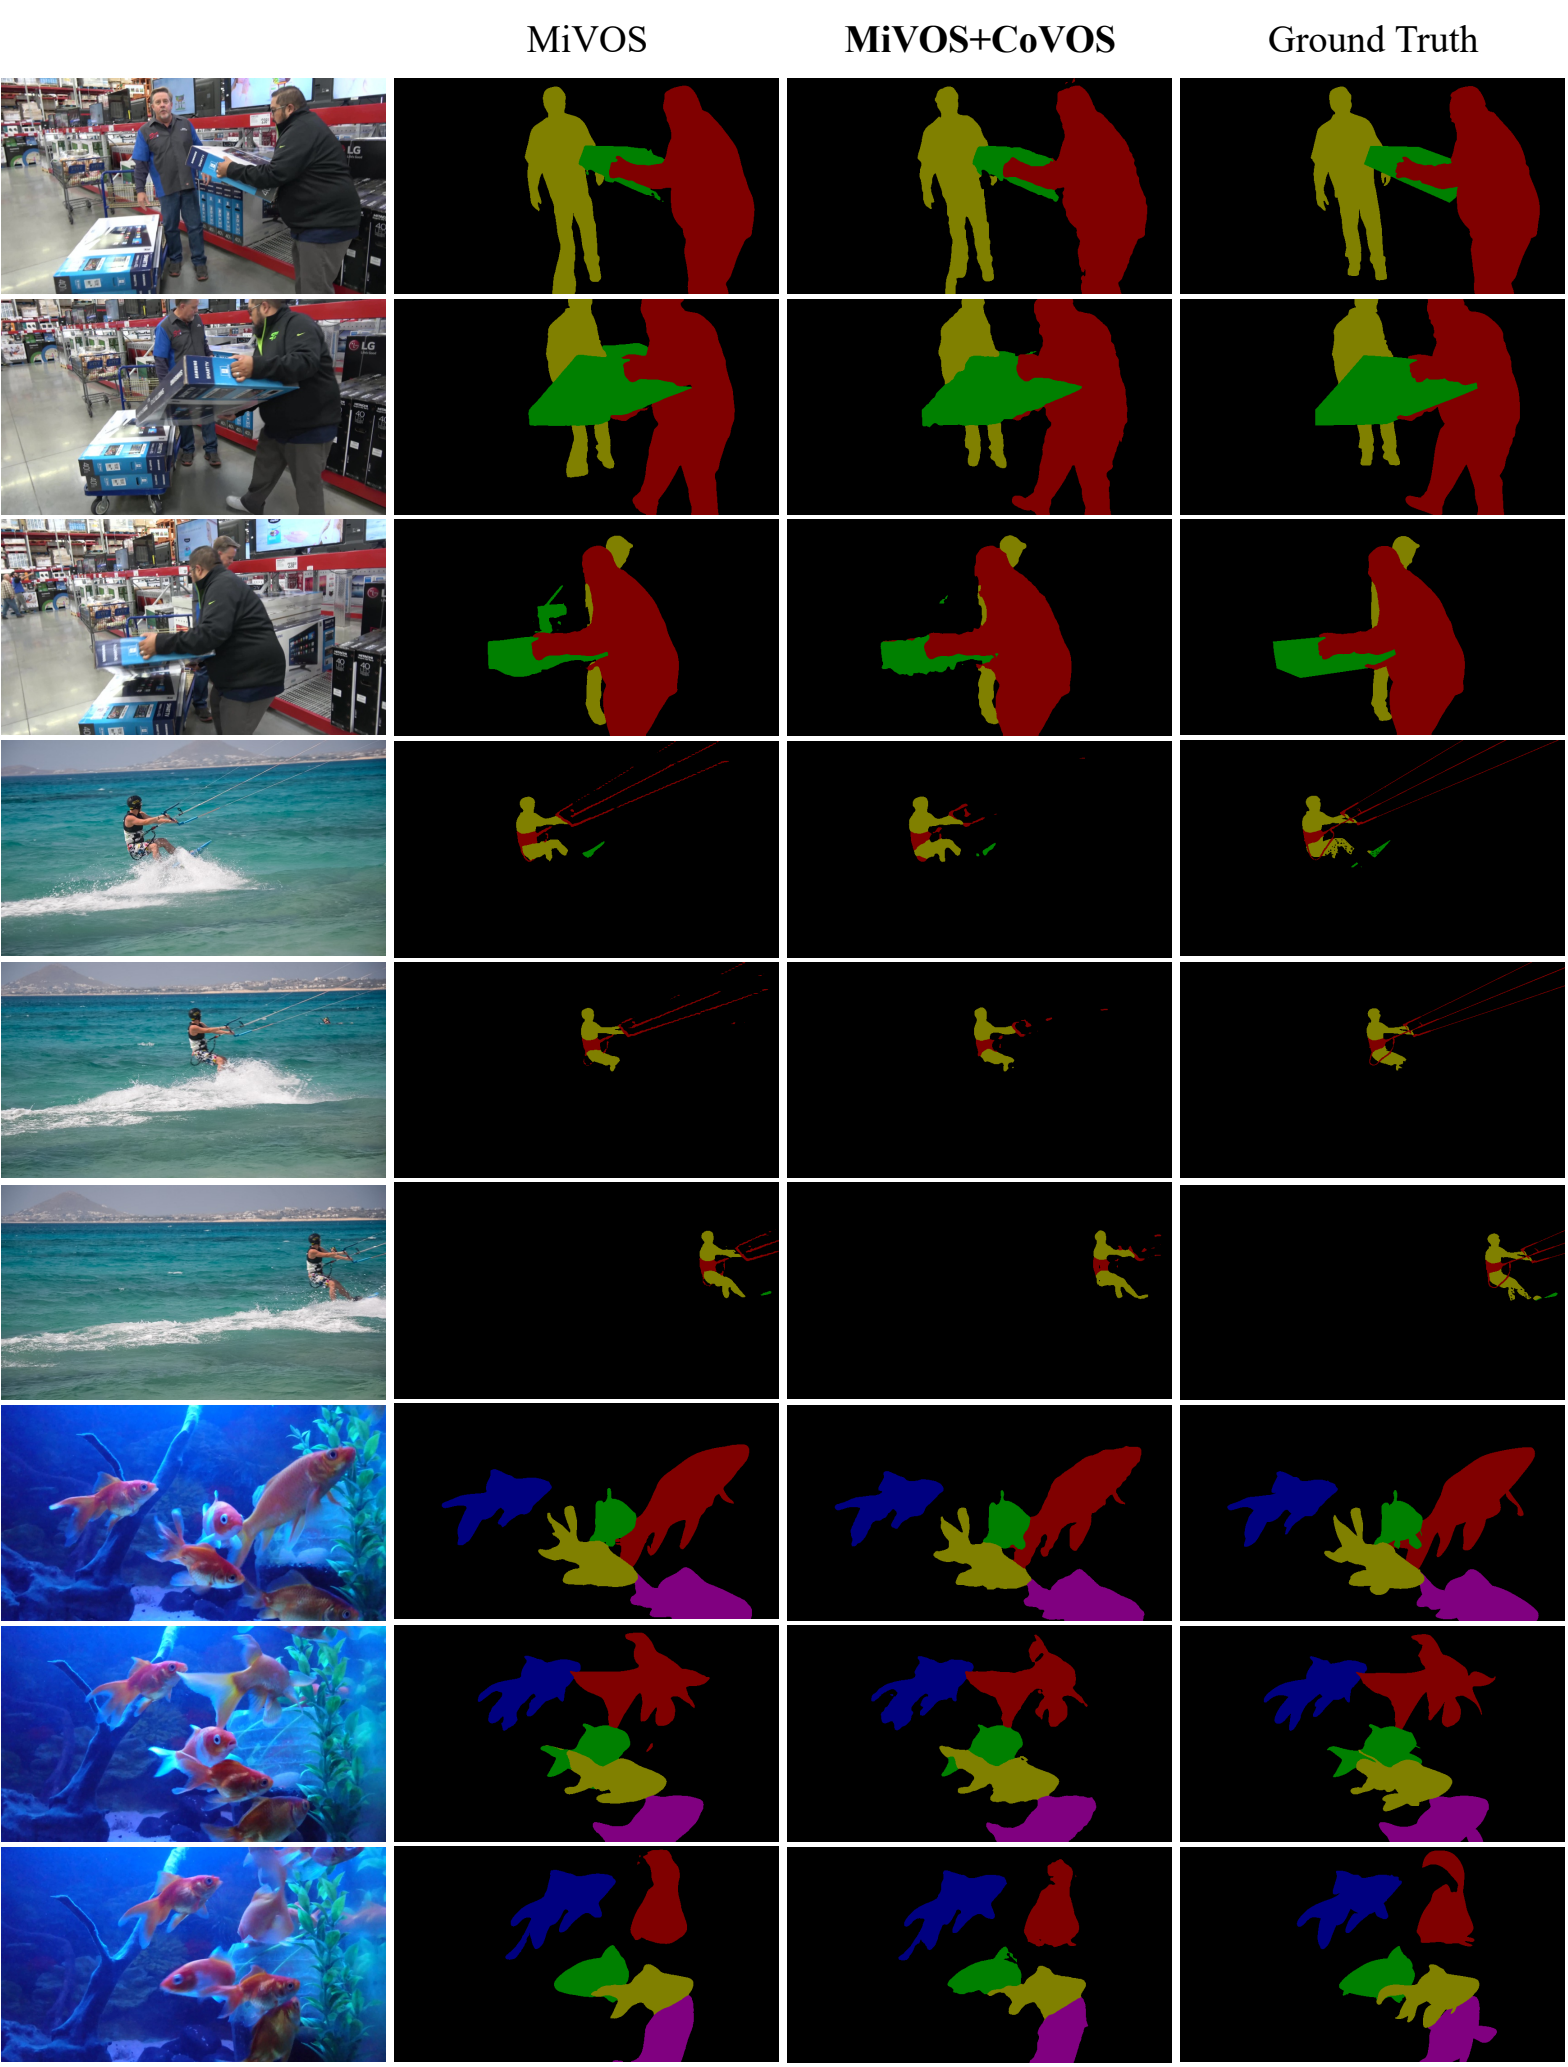 |
| 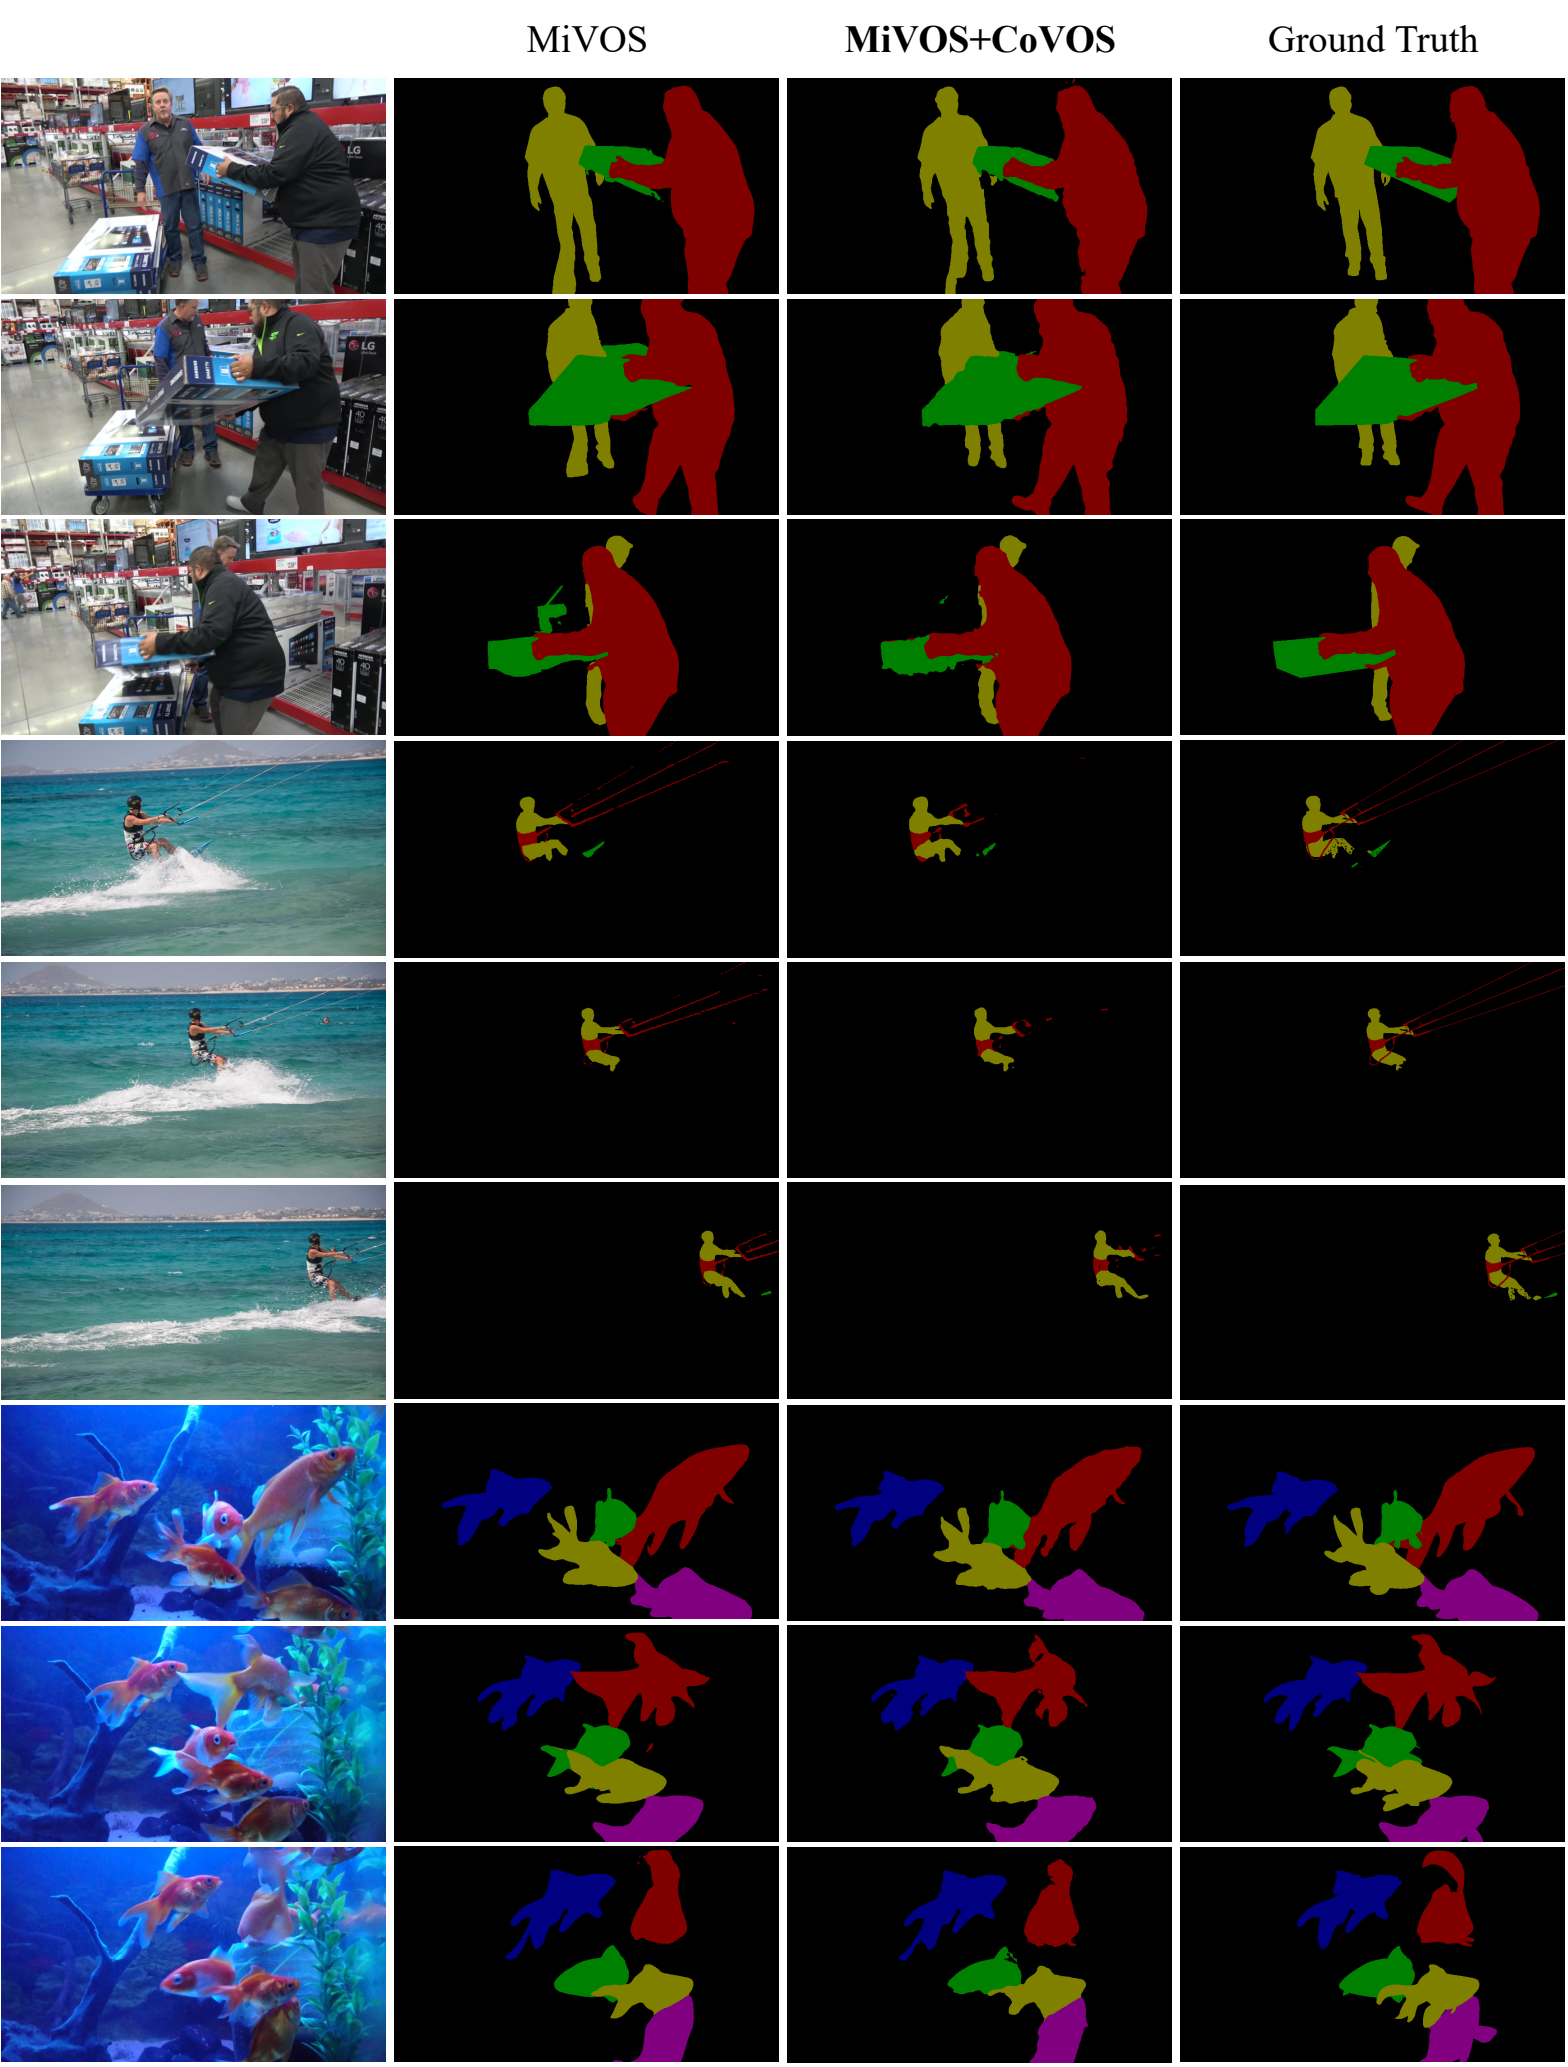 | 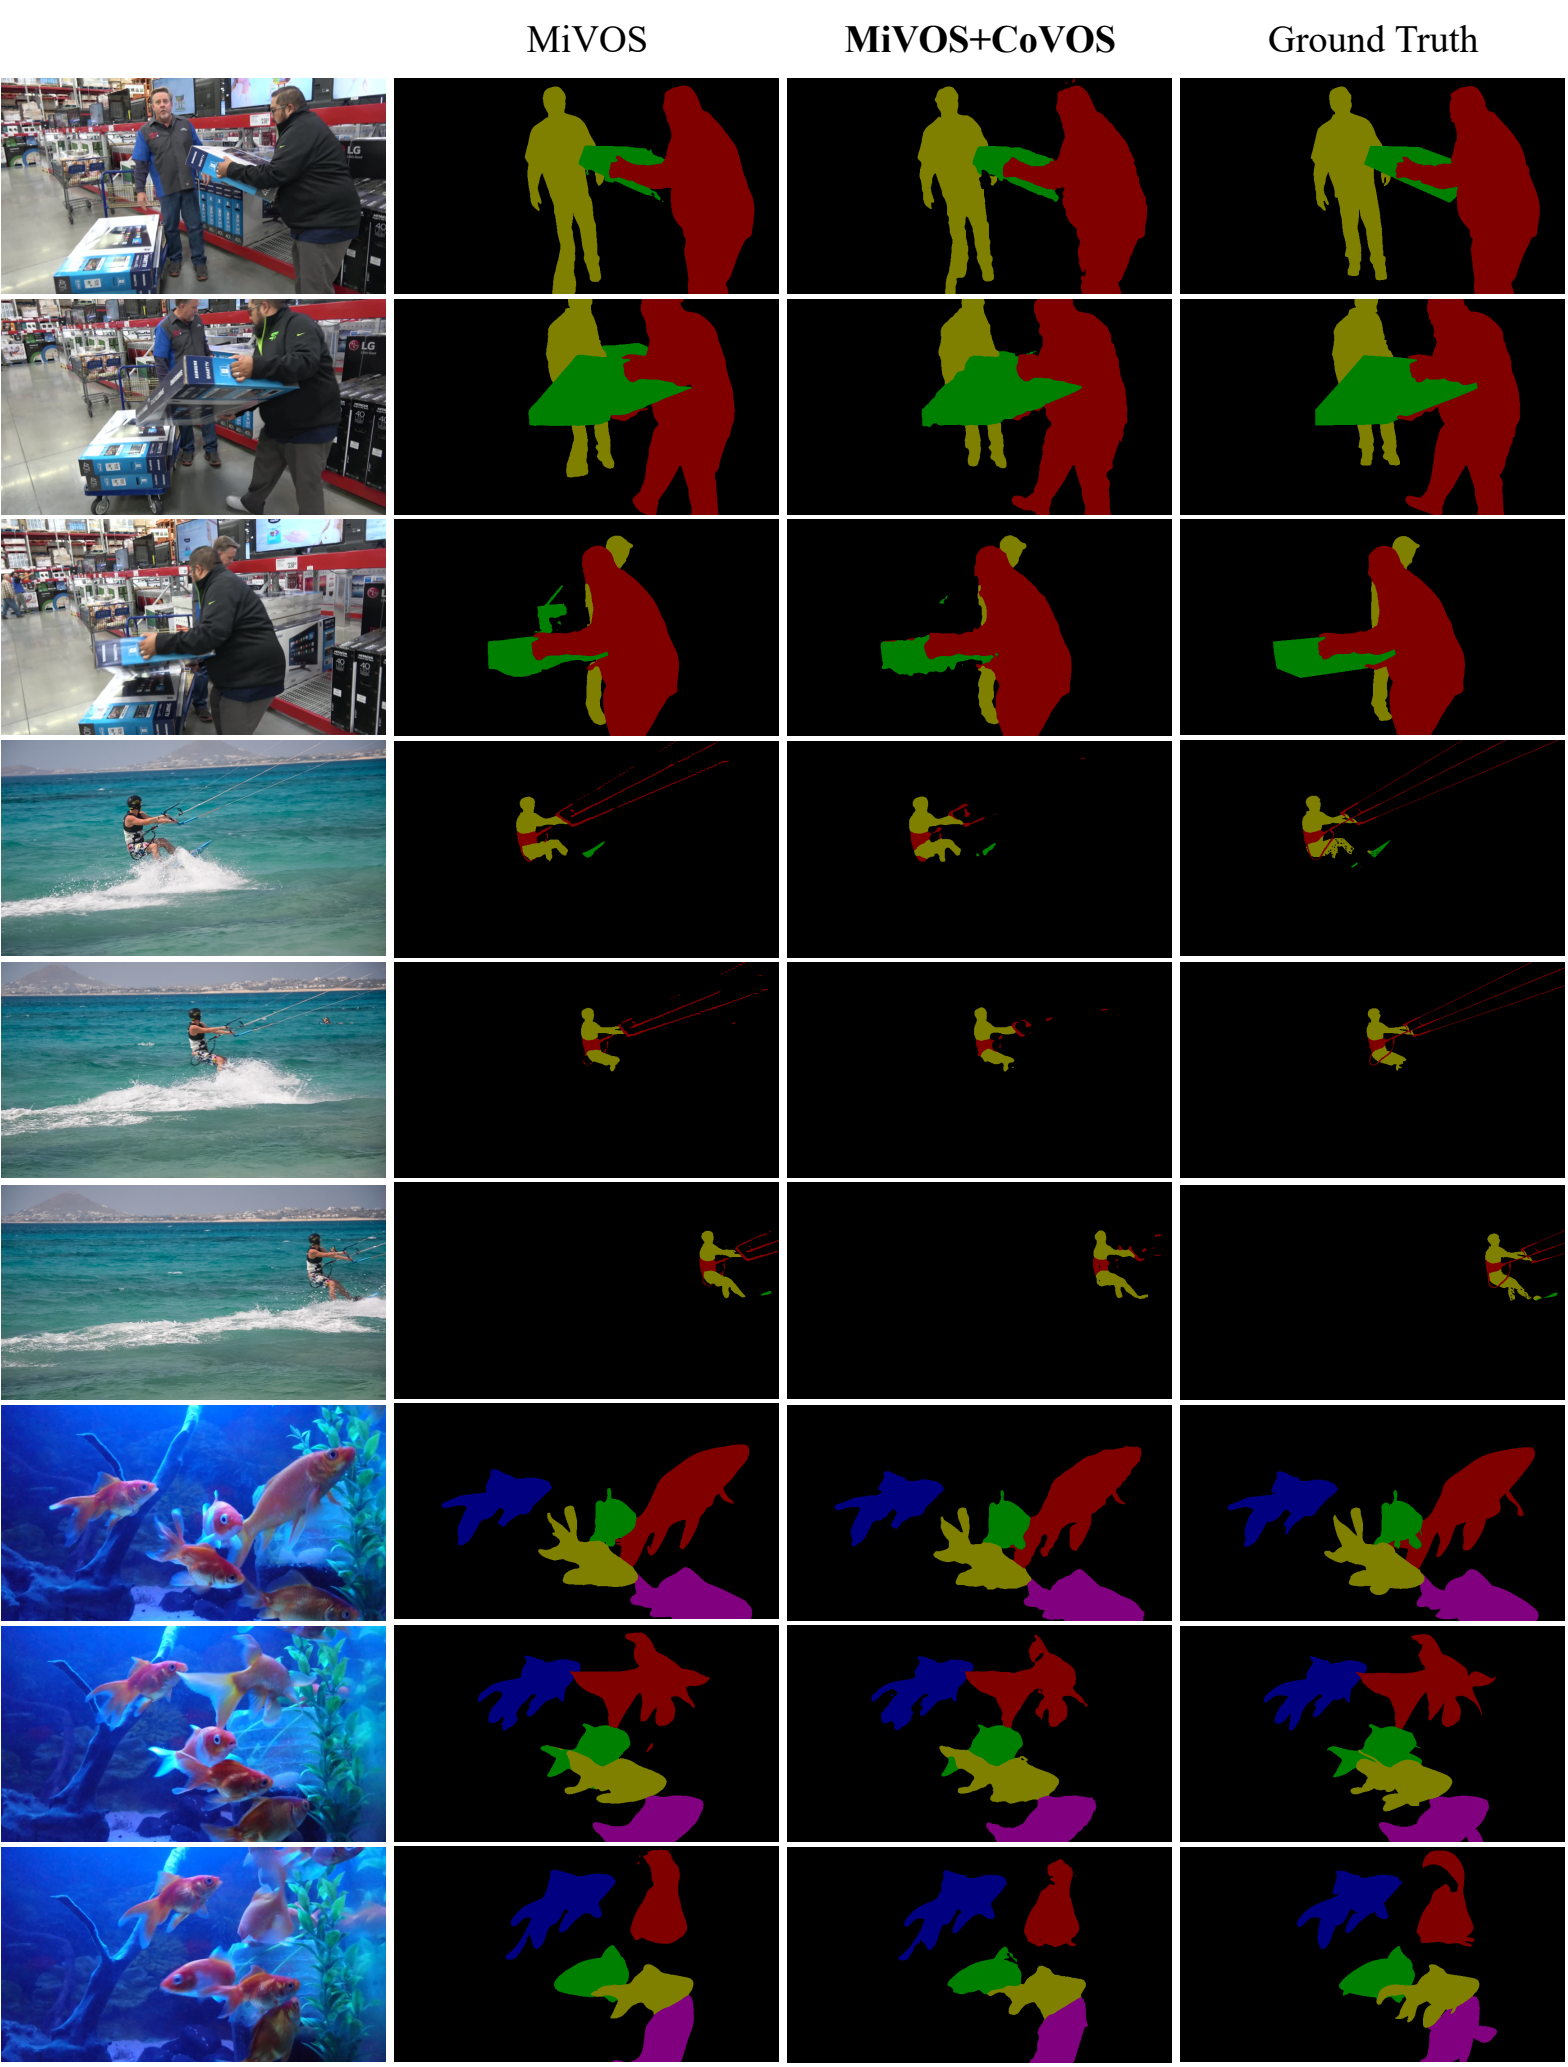 | 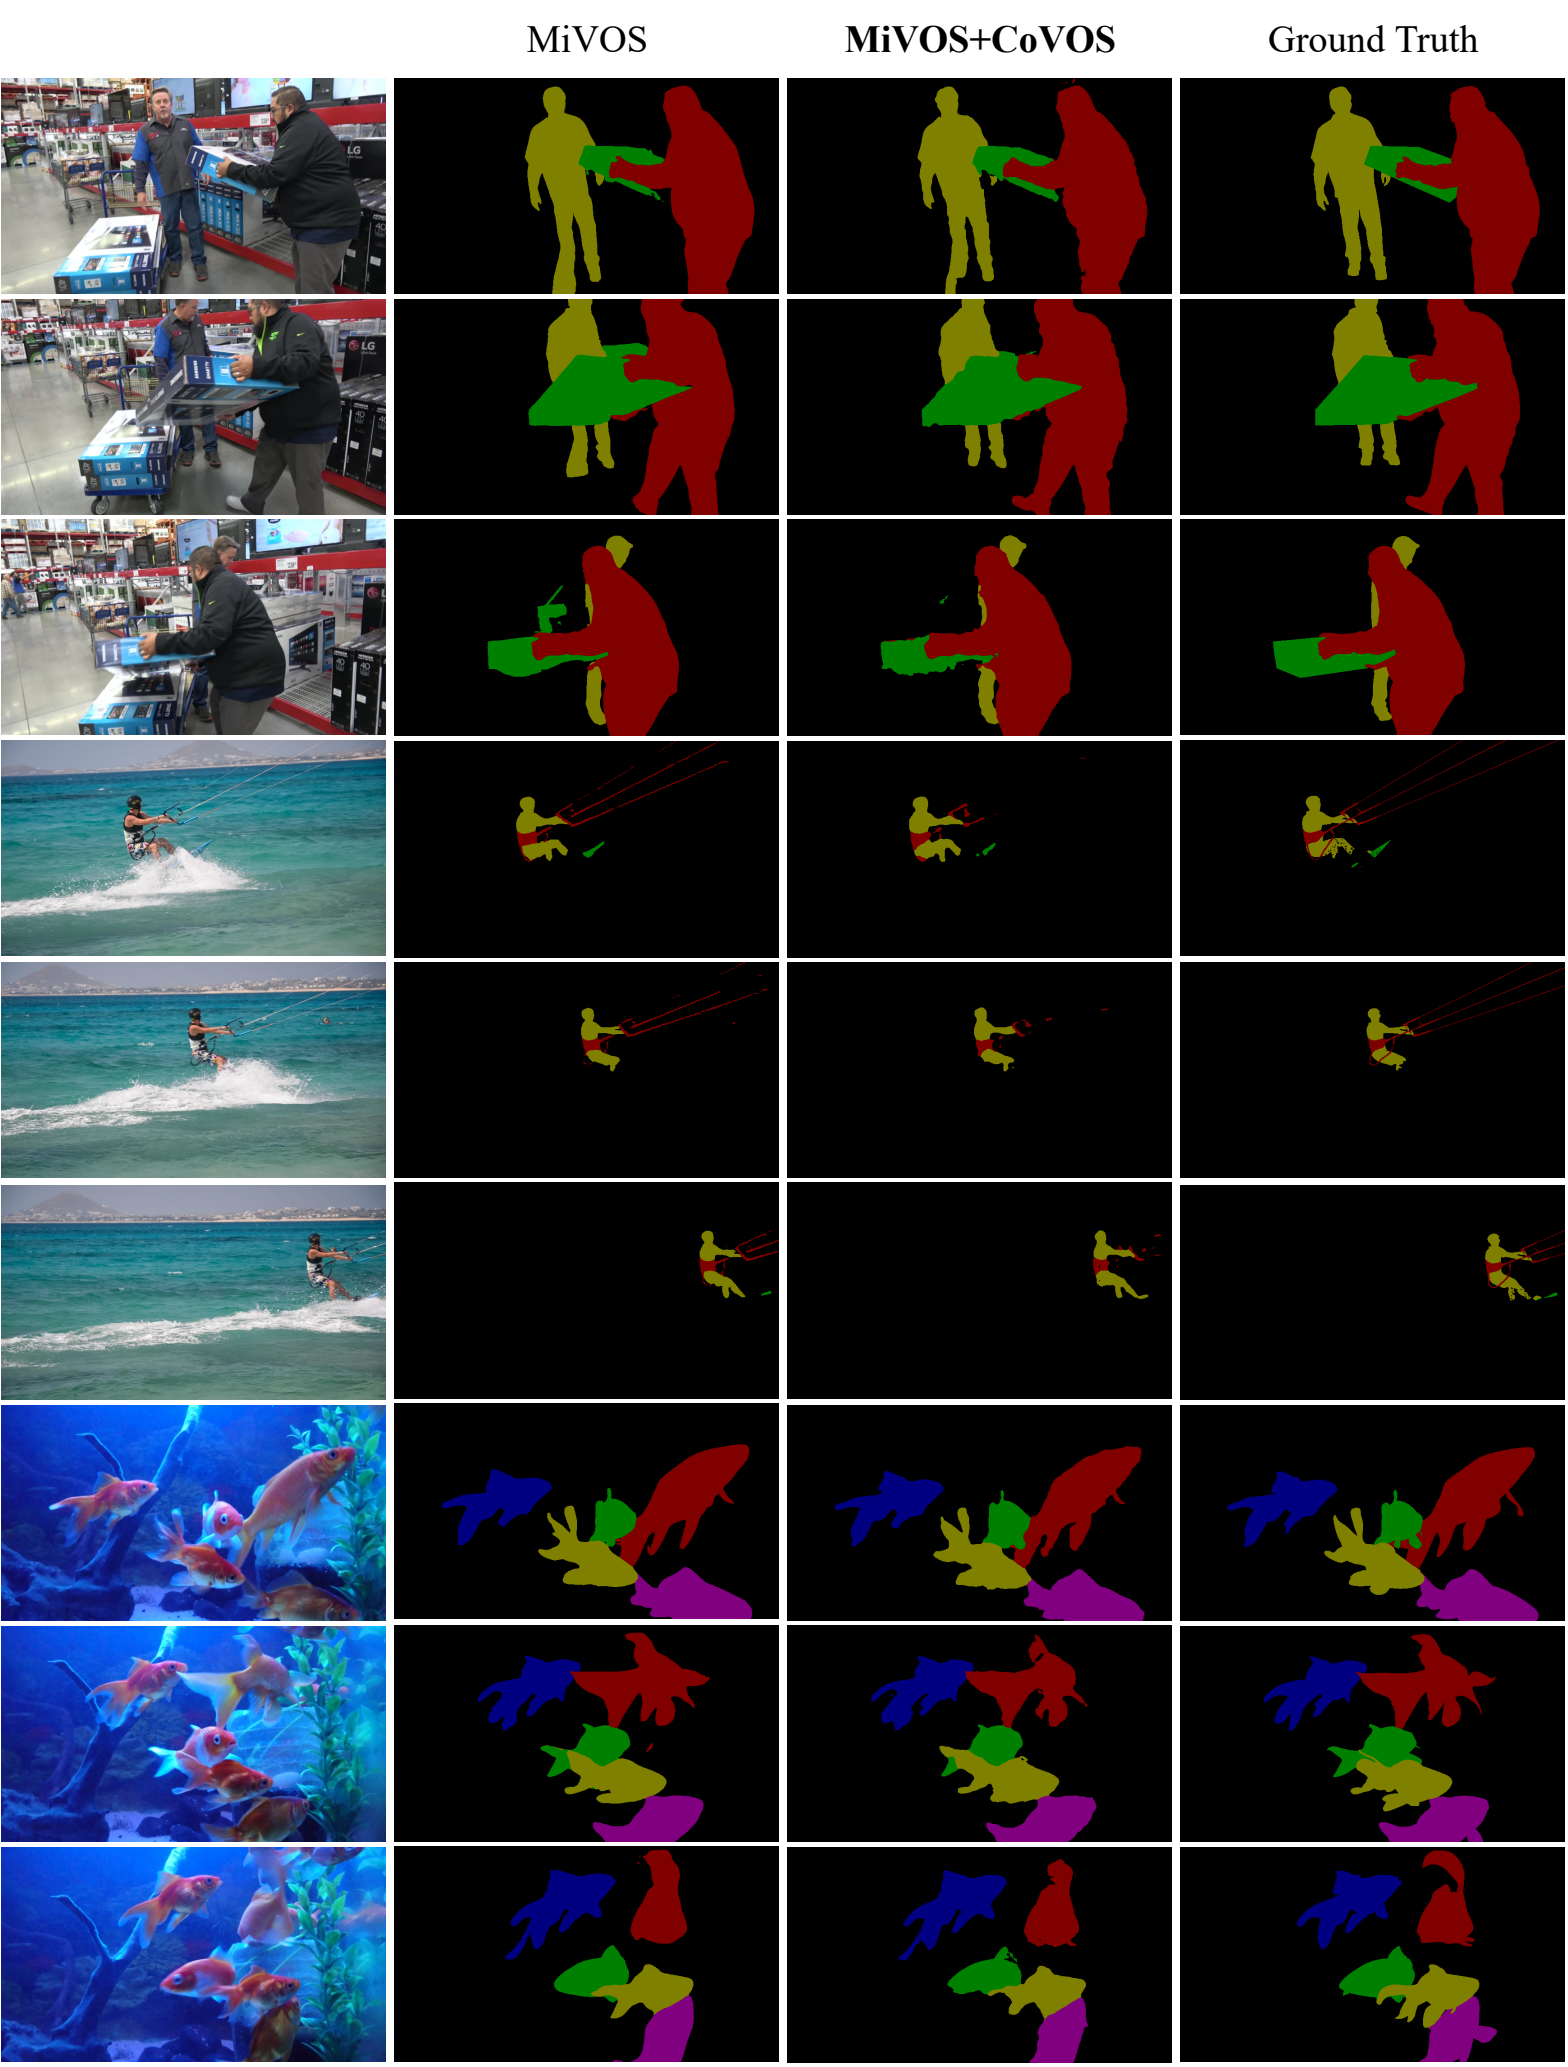 | 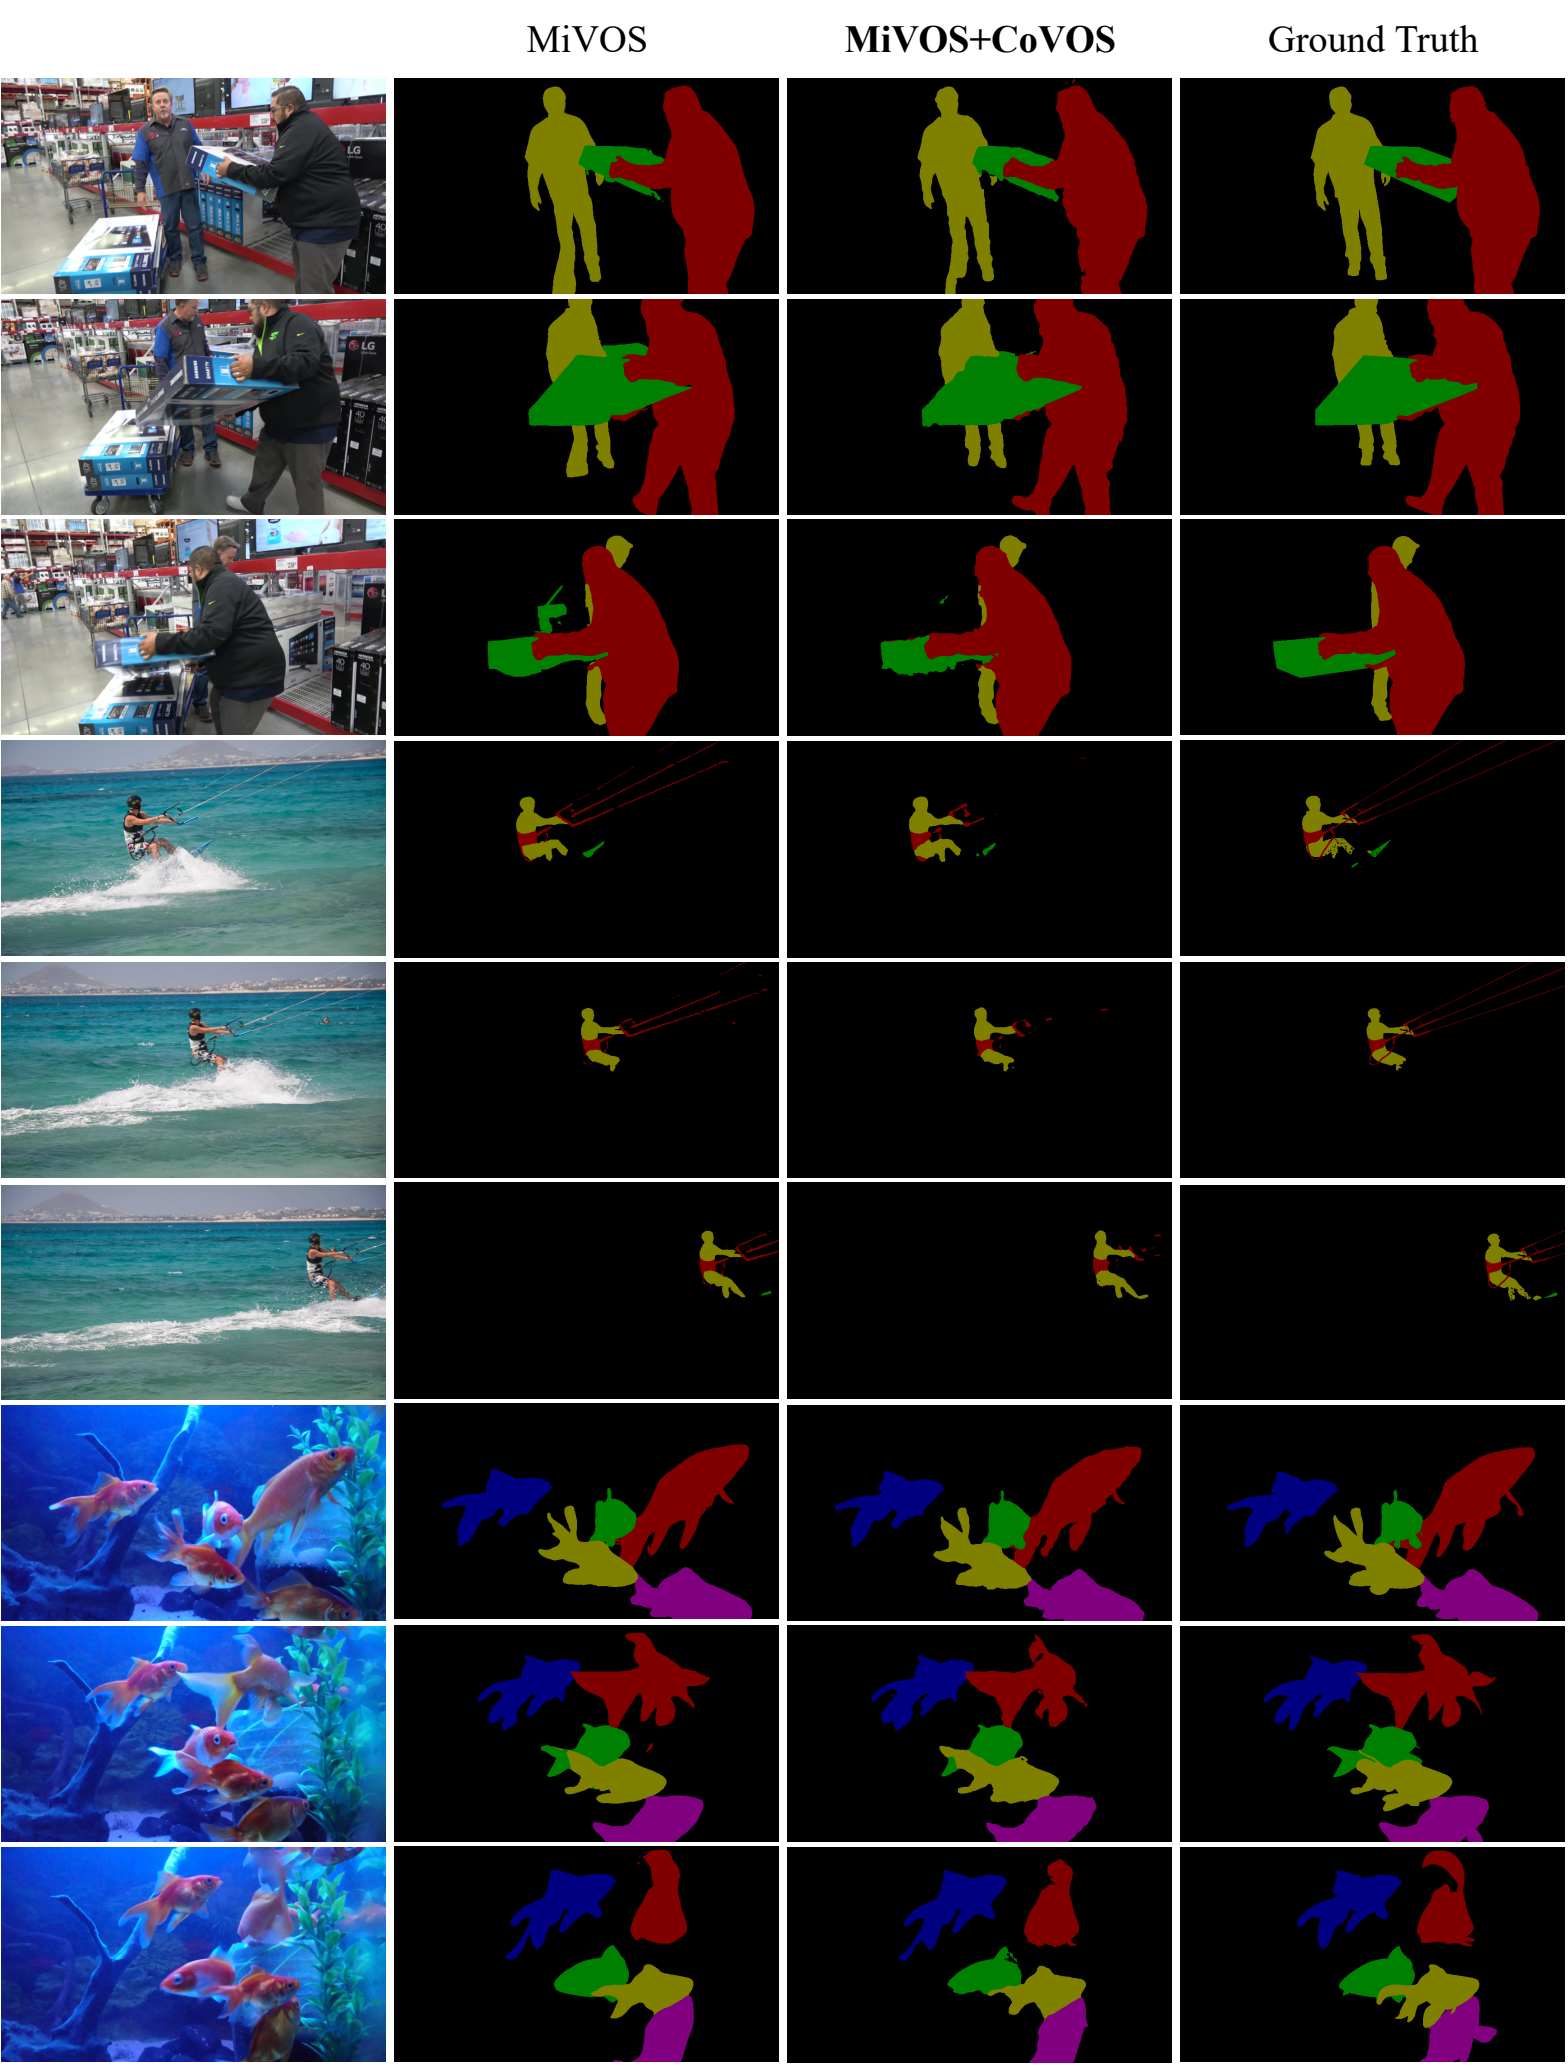 |
